# Supplementary material for: Exotic branes and mixed-symmetry potentials I: predictions from $E_{11}$ symmetry
Source: arXiv:1907.07177 ancillary file (2020-04-23)
Supplement: Supplementary file 1 [file appendixH.pdf]

# H SUSY potentials from $B$ to $Z$

| n | O(10, 10) rep. | $E_{11}$ roots $\alpha_i$ | type IIA | type IIB |
|---|---|---|---|---|
| 0 | [0,1,0,0,0,0,0,0,0,0,0] | [-1,-2,-2,-2,-2,-2,-2,-2,-1,0,-1] | $\beta^2$, $B_1^1$, $B_2$ | |
| 1 | [0,0,0,0,0,0,0,0,0,1,0] | [0,0,0,0,0,0,0,0,0,1,0] | $C_1$ [5] | $C_0$ [6] |
| 2 | [0,0,0,1,0,0,0,0,0,0,0] | [0,0,0,0,1,2,3,4,3,2,2] | $D_6$ [5] | |
| 3 | [0,1,0,0,0,0,0,0,0,1,0] | [0,0,1,2,3,4,5,6,4,3,3] | $E_{8,1}$ [13] | $E_8$ [14] |
| 4 | [1,0,0,0,0,0,1,0,0,0] | [0,1,2,3,4,5,6,8,6,4,4] | $F_{9,3}$ [14] | |
| | [0,1,0,1,0,0,0,0,0,0,0] | [0,0,1,2,4,6,8,10,7,4,5] | $F_{8,6}$ [9] | |
| | [0,0,0,0,0,0,0,0,0,2,0] | [1,2,3,4,5,6,7,8,5,4,4] | $F_{10,1,1}$ [5] | $F_{10}$ [6] |
| 5 | [0,0,0,0,0,1,0,0,1,0] | [1,2,3,4,5,6,8,10,7,5,5] | $G_{10,4,1}$ [17] | $G_{10,4}$ [18] |
| | [1,0,0,1,0,0,0,0,0,1] | [0,1,2,3,5,7,9,11,8,5,5] | $G_{9,6}$ [28] | $G_{9,6,1}$ [28] |
| | [0,2,0,0,0,0,0,0,0,1,0] | [0,0,2,4,6,8,10,12,8,5,6] | $G_{8,8,1}$ [13] | $G_{8,8}$ [14] |
| 6 | [0,0,0,1,0,0,0,1,0,0] | [1,2,3,4,6,8,10,12,9,6,6] | $H_{10,6,2}$ [25] | |
| | [1,1,0,0,0,0,0,0,0,1,1] | [0,1,3,5,7,9,11,13,9,6,6] | $H_{9,8,1}$ [32] | |
| | [1,0,1,0,0,1,0,0,0,0] | [0,1,2,4,6,8,11,14,10,6,7] | $H_{9,7,4}$ [24] | |
| | [0,2,0,1,0,0,0,0,0,0,0] | [0,0,2,4,7,10,13,16,11,6,8] | $H_{8,8,6}$ [9] | |
| 7 | [0,1,0,0,0,0,0,1,1,0] | [1,2,4,6,8,10,12,14,10,7,7] | $I_{10,8,2,1}$ [31] | $I_{10,8,2}$ [32] |
| | [0,0,1,0,0,1,0,0,0,1] | [1,2,3,5,7,9,12,15,11,7,7] | $I_{10,7,4}$ [40] | $I_{10,7,4,1}$ [40] |
| | [2,0,0,0,0,0,1,0,0,1] | [0,2,4,6,8,10,12,15,11,7,7] | $I_{9,9,3}$ [28] | $I_{9,9,3,1}$ [28] |
| | [0,0,0,2,0,0,0,0,1,0] | [1,2,3,4,7,10,13,16,11,7,8] | $I_{10,6,6,1}$ [17] | $I_{10,6,6}$ [18] |
| | [1,1,0,0,1,0,0,0,1,0] | [0,1,3,5,7,10,13,16,11,7,8] | $I_{9,8,5,1}$ [48] | $I_{9,8,5}$ [48] |
| | [1,0,2,0,0,0,0,0,0,1] | [0,1,2,5,8,11,14,17,12,7,8] | $I_{9,7,7}$ [24] | $I_{9,7,7,1}$ [24] |
| | [0,3,0,0,0,0,0,0,0,1,0] | [0,0,3,6,9,12,15,18,12,7,9] | $I_{8,8,8,1}$ [13] | $I_{8,8,8}$ [14] |
| 8 | [0,1,0,0,1,0,0,0,1,1] | [1,2,4,6,8,11,14,17,12,8,8] | $J_{10,8,5,1}$ [60] | |
| | [1,0,0,0,0,0,1,1,0,0] | [1,3,5,7,9,11,13,16,12,8,8] | $J_{10,9,3,2}$ [28] | |
| | [0,0,1,1,0,0,1,0,0,0] | [1,2,3,5,8,11,14,18,13,8,9] | $J_{10,7,6,3}$ [32] | |
| | [0,1,0,0,0,2,0,0,0,0] | [1,2,4,6,8,10,14,18,13,8,9] | $J_{10,8,4,4}$ [15] | |
| | [1,1,1,0,0,0,0,0,1,0,0] | [0,1,3,6,9,12,15,18,13,8,9] | $J_{9,8,7,2}$ [48] | |
| | [2,0,0,0,1,0,1,0,0,0] | [0,2,4,6,8,11,14,18,13,8,9] | $J_{9,9,5,3}$ [30] | |
| | [1,1,0,1,1,0,0,0,0,0] | [0,1,3,5,8,12,16,20,14,8,10] | $J_{9,8,6,5}$ [24] | |
| | [0,3,0,1,0,0,0,0,0,0,0] | [0,0,3,6,10,14,18,22,15,8,11] | $J_{8,8,8,6}$ [9] | |
| | [1,0,3,0,0,0,0,0,0,0,0] | [0,1,2,6,10,14,18,22,15,8,11] | $J_{9,7,7,7}$ [6] | |
| | [0,0,0,0,0,0,0,1,2,0] | [2,4,6,8,10,12,14,16,11,8,8] | $J_{10,10,2,1,1}$ [13] | $J_{10,10,2}$ [14] |
| | [0,0,2,0,0,0,0,0,0,2] | [1,2,3,6,9,12,15,18,13,8,8] | $J_{10,7,7}$ [16] | $J_{10,7,7,1,1}$ [16] |
| | [2,0,0,1,0,0,0,0,0,2] | [0,2,4,6,9,12,15,18,13,8,8] | $J_{9,9,6}$ [28] | $J_{9,9,6,1,1}$ [28] |
| | [2,0,0,1,0,0,0,0,2,0] | [0,2,4,6,9,12,15,18,12,8,9] | $J_{9,9,6,1,1}$ [28] | $J_{9,9,6}$ [28] |
| 9 | [0,0,0,0,0,1,0,1,1,0] | [2,4,6,8,10,12,15,18,13,9,9] | $K_{10,10,4,2,1}$ [31] | $K_{10,10,4,2}$ [32] |
| | [1,0,0,1,0,0,0,0,2,1] | [1,3,5,7,10,13,16,19,13,9,9] | $K_{10,9,6,1,1}$ [48] | $K_{10,9,6,1}$ [48] |
| | [0,1,1,0,0,0,0,1,0,1] | [1,2,4,7,10,13,16,19,14,9,9] | $K_{10,8,7,2}$ [54] | $K_{10,8,7,2,1}$ [54] |
| | [1,0,0,0,1,0,1,0,0,1] | [1,3,5,7,9,12,15,19,14,9,9] | $K_{10,9,5,3}$ [60] | $K_{10,9,5,3,1}$ [60] |
| | [2,1,0,0,0,0,0,0,0,1,2] | [0,2,5,8,11,14,17,20,14,9,9] | $K_{9,9,8,1}$ [32] | $K_{9,9,8,1,1}$ [32] |
| | [0,2,0,0,0,0,0,0,0,3,0] | [1,2,5,8,11,14,17,20,13,9,10] | $K_{10,8,8,1,1,1}$ [13] | $K_{10,8,8}$ [14] |
| | [0,1,0,1,0,1,0,0,1,0] | [1,2,4,6,9,12,16,20,14,9,10] | $K_{10,8,6,4,1}$ [67] | $K_{10,8,6,4}$ [68] |
| | [2,0,1,0,0,0,1,0,1,0] | [0,2,4,7,10,13,16,20,14,9,10] | $K_{9,9,7,3,1}$ [60] | $K_{9,9,7,3}$ [60] |
| | [0,0,2,0,1,0,0,0,0,1] | [1,2,3,6,9,13,17,21,15,9,10] | $K_{10,7,7,5}$ [36] | $K_{10,7,7,5,1}$ [36] |
| | [1,2,0,0,0,1,0,0,0,1] | [0,1,4,7,10,13,17,21,15,9,10] | $K_{9,8,8,4}$ [50] | $K_{9,8,8,4,1}$ [50] |
| | [2,0,0,1,1,0,0,0,0,1] | [0,2,4,6,9,13,17,21,15,9,10] | $K_{9,9,6,5}$ [48] | $K_{9,9,6,5,1}$ [48] |
| | [1,1,1,1,0,0,0,0,1,0] | [0,1,3,6,10,14,18,22,15,9,11] | $K_{9,8,7,6,1}$ [56] | $K_{9,8,7,6}$ [56] |
| | [0,4,0,0,0,0,0,0,0,1,0] | [0,0,4,8,12,16,20,24,16,9,12] | $K_{8,8,8,8,1}$ [13] | $K_{8,8,8,8}$ [14] |
| 10 | [0,0,0,0,1,1,0,0,1,1] | [2,4,6,8,10,13,17,21,15,10,10] | $L_{10,10,5,4,1}$ [48] | |
| | [0,0,0,1,0,0,0,2,0,0] | [2,4,6,8,11,14,17,20,15,10,10] | $L_{10,10,6,2,2}$ [25] | |
| | [1,0,1,0,0,0,1,0,1,1] | [1,3,5,8,11,14,17,21,15,10,10] | $L_{10,9,7,3,1}$ [90] | |
| | [0,1,1,0,1,0,0,1,0,0] | [1,2,4,7,10,14,18,22,16,10,11] | $L_{10,8,7,5,2}$ [72] | |
| | [1,0,0,1,0,1,1,0,0,0] | [1,3,5,7,10,13,17,22,16,10,11] | $L_{10,9,6,4,3}$ [48] | |
| | [2,0,1,1,0,0,0,0,1,1] | [0,2,4,7,11,15,19,23,16,10,11] | $L_{9,9,7,6,1}$ [72] | |
| | [2,1,0,0,0,1,0,1,0,0] | [0,2,5,8,11,14,18,22,16,10,11] | $L_{9,9,8,4,2}$ [60] | |
| | [0,0,3,0,0,0,1,0,0,0] | [1,2,3,7,11,15,19,24,17,10,12] | $L_{10,7,7,7,3}$ [20] | |
| | [0,1,0,2,0,1,0,0,0,0] | [1,2,4,6,10,14,19,24,17,10,12] | $L_{10,8,6,6,4}$ [27] | |
| | [1,2,0,1,0,0,1,0,0,0] | [0,1,4,7,11,15,19,24,17,10,12] | $L_{9,8,8,6,3}$ [48] | |
| | [2,0,1,0,1,1,0,0,0,0] | [0,2,4,7,10,14,19,24,17,10,12] | $L_{9,9,7,5,4}$ [36] | |
| | [1,1,2,0,1,0,0,0,0,0] | [0,1,3,7,11,16,21,26,18,10,13] | $L_{9,8,7,7,5}$ [24] | |
| | [2,0,0,3,0,0,0,0,0,0] | [0,2,4,6,11,16,21,26,18,10,13] | $L_{9,9,6,6,6}$ [8] | |
| | [0,4,0,1,0,0,0,0,0,0,0] | [0,0,4,8,13,18,23,28,19,10,14] | $L_{8,8,8,8,6}$ [9] | |
| | [0,0,1,0,0,0,0,0,3,1] | [2,4,6,9,12,15,18,21,14,10,10] | $L_{10,10,7,1,1,1}$ [28] | $L_{10,10,7,1}$ [28] |
| | [0,2,0,0,0,1,0,0,0,2] | [1,2,5,8,11,14,18,22,16,10,10] | $L_{10,8,8,4}$ [38] | $L_{10,8,8,4,1,1}$ [37] |
| | [1,0,0,1,1,0,0,0,0,2] | [1,3,5,7,10,14,18,22,16,10,10] | $L_{10,9,6,5}$ [48] | $L_{10,9,6,5,1,1}$ [48] |
| | [3,0,0,0,0,0,1,0,0,2] | [0,3,6,9,12,15,18,22,16,10,10] | $L_{9,9,9,3}$ [28] | $L_{9,9,9,3,1,1}$ [28] |
| | [0,2,0,0,0,1,0,0,2,0] | [1,2,5,8,11,14,18,22,15,10,11] | $L_{10,8,8,4,1,1}$ [37] | $L_{10,8,8,4}$ [38] |
| | [1,0,0,1,1,0,0,0,2,0] | [1,3,5,7,10,14,18,22,15,10,11] | $L_{10,9,6,5,1,1}$ [48] | $L_{10,9,6,5}$ [48] |

| | | | | |
|---|---|---|---|---|
| | [3,0,0,0,0,0,1,0,2,0] | [0,3,6,9,12,15,18,22,15,10,11] | $L_{9,9,9,3,1,1}$ [28] | $L_{9,9,9,3}$ [28] |
| | [1,2,1,0,0,0,0,0,0,2] | [0,1,4,8,12,16,20,24,17,10,11] | $L_{9,8,8,7}$ [32] | $L_{9,8,8,7,1,1}$ [32] |
| | [1,2,1,0,0,0,0,0,2,0] | [0,1,4,8,12,16,20,24,16,10,12] | $L_{9,8,8,7,1,1}$ [32] | $L_{9,8,8,7}$ [32] |
| 11 | [0,0,1,0,0,1,0,0,2,1] | [2,4,6,9,12,15,19,23,16,11,11] | $M_{10,10,7,4,1,1}$ [64] | $M_{10,10,7,4,1}$ [64] |
| | [0,1,0,0,0,0,0,2,1,0] | [2,4,7,10,13,16,19,22,16,11,11] | $M_{10,10,8,2,2,1}$ [31] | $M_{10,10,8,2,2}$ [32] |
| | [2,0,0,0,0,0,1,0,2,1] | [1,4,7,10,13,16,19,23,16,11,11] | $M_{10,9,9,3,1,1}$ [42] | $M_{10,9,9,3,1}$ [42] |
| | [0,0,0,1,1,0,0,1,0,1] | [2,4,6,8,11,15,19,23,17,11,11] | $M_{10,10,6,5,2}$ [60] | $M_{10,10,6,5,2,1}$ [60] |
| | [0,0,1,0,0,0,2,0,0,1] | [2,4,6,9,12,15,18,23,17,11,11] | $M_{10,10,7,3,3}$ [40] | $M_{10,10,7,3,3,1}$ [40] |
| | [1,0,1,1,0,0,0,0,1,2] | [1,3,5,8,12,16,20,24,17,11,11] | $M_{10,9,7,6,1}$ [72] | $M_{10,9,7,6,1,1}$ [72] |
| | [1,1,0,0,0,1,0,1,0,1] | [1,3,6,9,12,15,19,23,17,11,11] | $M_{10,9,8,4,2}$ [90] | $M_{10,9,8,4,2,1}$ [90] |
| | [0,2,1,0,0,0,0,0,0,3] | [1,2,5,9,13,17,21,25,18,11,11] | $M_{10,8,8,7}$ [24] | $M_{10,8,8,7,1,1,1}$ [24] |
| | [3,0,0,1,0,0,0,0,0,3] | [0,3,6,9,13,17,21,25,18,11,11] | $M_{9,9,9,6}$ [28] | $M_{9,9,9,6,1,1,1}$ [28] |
| | [0,0,0,0,0,0,0,0,5,0] | [3,6,9,12,15,18,21,24,15,11,12] | $M_{10,10,10,1,1,1,1,1}$ [5] | $M_{10,10,10}$ [6] |
| | [0,0,0,2,0,0,0,0,3,0] | [2,4,6,8,12,16,20,24,16,11,12] | $M_{10,10,6,6,1,1,1}$ [17] | $M_{10,10,6,6}$ [18] |
| | [1,1,0,0,1,0,0,0,3,0] | [1,3,6,9,12,16,20,24,16,11,12] | $M_{10,9,8,5,1,1,1}$ [48] | $M_{10,9,8,5}$ [48] |
| | [0,0,0,1,0,2,0,0,1,0] | [2,4,6,8,11,14,19,24,17,11,12] | $M_{10,10,6,4,4,1}$ [37] | $M_{10,10,6,4,4}$ [38] |
| | [0,2,0,1,0,0,0,1,1,0] | [1,2,5,8,12,16,20,24,17,11,12] | $M_{10,8,8,6,2,1}$ [67] | $M_{10,8,8,6,2}$ [68] |
| | [1,0,1,0,1,0,1,0,1,0] | [1,3,5,8,11,15,19,24,17,11,12] | $M_{10,9,7,5,3,1}$ [108] | $M_{10,9,7,5,3}$ [108] |
| | [2,1,1,0,0,0,0,0,2,1] | [0,2,5,9,13,17,21,25,17,11,12] | $M_{9,9,8,7,1,1}$ [56] | $M_{9,9,8,7,1}$ [56] |
| | [3,0,0,0,1,0,0,1,1,0] | [0,3,6,9,12,16,20,24,17,11,12] | $M_{9,9,9,5,2,1}$ [60] | $M_{9,9,9,5,2}$ [60] |
| | [0,1,2,0,0,0,1,0,0,1] | [1,2,4,8,12,16,20,25,18,11,12] | $M_{10,8,7,7,3}$ [60] | $M_{10,8,7,7,3,1}$ [60] |
| | [0,2,0,0,1,1,0,0,0,1] | [1,2,5,8,11,15,20,25,18,11,12] | $M_{10,8,8,5,4}$ [60] | $M_{10,8,8,5,4,1}$ [60] |
| | [1,0,0,2,0,1,0,0,0,1] | [1,3,5,7,11,15,20,25,18,11,12] | $M_{10,9,6,6,4}$ [60] | $M_{10,9,6,6,4,1}$ [60] |
| | [2,1,0,1,0,0,1,0,0,1] | [0,2,5,8,12,16,20,25,18,11,12] | $M_{9,9,8,6,3}$ [96] | $M_{9,9,8,6,3,1}$ [96] |
| | [3,0,0,0,0,2,0,0,0,1] | [0,3,6,9,12,15,20,25,18,11,12] | $M_{9,9,9,4,4}$ [30] | $M_{9,9,9,4,4,1}$ [30] |
| | [0,1,1,1,1,0,0,0,1,0] | [1,2,4,7,11,16,21,26,18,11,13] | $M_{10,8,7,6,5,1}$ [72] | $M_{10,8,7,6,5}$ [72] |
| | [1,3,0,0,0,0,1,0,1,0] | [0,1,5,9,13,17,21,26,18,11,13] | $M_{9,8,8,8,3,1}$ [48] | $M_{9,8,8,8,3}$ [48] |
| | [2,0,2,0,0,1,0,0,1,0] | [0,2,4,8,12,16,21,26,18,11,13] | $M_{9,9,7,7,4,1}$ [60] | $M_{9,9,7,7,4}$ [60] |
| | [2,1,0,0,2,0,0,0,1,0] | [0,2,5,8,11,16,21,26,18,11,13] | $M_{9,9,8,5,5,1}$ [48] | $M_{9,9,8,5,5}$ [48] |
| | [1,2,1,0,1,0,0,0,0,1] | [0,1,4,8,12,17,22,27,19,11,13] | $M_{9,8,8,7,5}$ [72] | $M_{9,8,8,7,5,1}$ [72] |
| | [2,0,1,2,0,0,0,0,0,1] | [0,2,4,7,12,17,22,27,19,11,13] | $M_{9,9,7,6,6}$ [42] | $M_{9,9,7,6,6,1}$ [42] |
| | [0,0,4,0,0,0,0,0,1,0] | [1,2,3,8,13,18,23,28,19,11,14] | $M_{10,7,7,7,7,1}$ [16] | $M_{10,7,7,7,7}$ [16] |
| | [0,5,0,0,0,0,0,0,1,0] | [0,0,5,10,15,20,25,30,20,11,15] | $M_{8,8,8,8,8,1}$ [13] | $M_{8,8,8,8,8}$ [14] |
| 12 | [0,0,1,1,0,0,0,1,1,1] | [2,4,6,9,13,17,21,25,18,12,12] | $N_{10,10,7,6,2,1}$ [80] | |
| | [0,1,0,0,0,1,1,0,1,1] | [2,4,7,10,13,16,20,25,18,12,12] | $N_{10,10,8,4,3,1}$ [90] | |
| | [1,0,0,0,0,0,1,2,0,0] | [2,5,8,11,14,17,20,24,18,12,12] | $N_{10,10,9,3,2,2}$ [28] | |
| | [1,1,1,0,0,0,0,0,2,2] | [1,3,6,10,14,18,22,26,18,12,12] | $N_{10,9,8,7,1,1}$ [56] | |
| | [2,0,0,0,1,0,0,1,1,1] | [1,4,7,10,13,17,21,25,18,12,12] | $N_{10,9,9,5,2,1}$ [80] | |
| | [0,0,0,2,0,1,0,1,0,0] | [2,4,6,8,12,16,21,26,19,12,13] | $N_{10,10,6,6,4,2}$ [45] | |
| | [0,0,1,0,1,0,2,0,0,0] | [2,4,6,9,12,16,20,26,19,12,13] | $N_{10,10,7,5,3,3}$ [36] | |
| | [0,2,1,0,0,1,0,0,1,1] | [1,2,5,9,13,17,22,27,19,12,13] | $N_{10,8,8,7,4,1}$ [96] | |
| | [0,3,0,0,0,0,0,2,0,0] | [1,2,6,10,14,18,22,26,19,12,13] | $N_{10,8,8,8,2,2}$ [21] | |
| | [1,0,1,1,1,0,0,0,1,1] | [1,3,5,8,12,17,22,27,19,12,13] | $N_{10,9,7,6,5,1}$ [120] | |
| | [1,0,2,0,0,0,1,1,0,0] | [1,3,5,9,13,17,21,26,19,12,13] | $N_{10,9,7,7,3,2}$ [60] | |
| | [1,1,0,0,1,1,0,1,0,0] | [1,3,6,9,12,16,21,26,19,12,13] | $N_{10,9,8,5,4,2}$ [96] | |
| | [2,0,0,0,0,1,2,0,0,0] | [1,4,7,10,13,16,20,26,19,12,13] | $N_{10,9,9,4,3,3}$ [24] | |
| | [2,2,0,0,0,0,1,0,1,1] | [0,2,6,10,14,18,22,27,19,12,13] | $N_{9,9,8,8,3,1}$ [72] | |
| | [3,0,0,1,0,1,0,0,1,1] | [0,3,6,9,13,17,22,27,19,12,13] | $N_{9,9,9,6,4,1}$ [96] | |
| | [3,0,1,0,0,0,0,2,0,0] | [0,3,6,10,14,18,22,26,19,12,13] | $N_{9,9,9,7,2,2}$ [36] | |
| | [0,1,2,1,0,0,0,1,0,0] | [1,2,4,8,13,18,23,28,20,12,14] | $N_{10,8,7,7,6,2}$ [60] | |
| | [0,2,0,1,1,0,1,0,0,0] | [1,2,5,8,12,17,22,28,20,12,14] | $N_{10,8,8,6,5,3}$ [54] | |
| | [1,0,1,1,0,2,0,0,0,0] | [1,3,5,8,12,16,22,28,20,12,14] | $N_{10,9,7,6,4,4}$ [36] | |
| | [1,3,0,1,0,0,0,0,1,1] | [0,1,5,9,14,19,24,29,20,12,14] | $N_{9,8,8,8,6,1}$ [72] | |
| | [2,0,3,0,0,0,0,0,1,1] | [0,2,4,9,14,19,24,29,20,12,14] | $N_{9,9,7,7,7,1}$ [42] | |
| | [2,1,0,2,0,0,0,1,0,0] | [0,2,5,8,13,18,23,28,20,12,14] | $N_{9,9,8,6,6,2}$ [60] | |
| | [2,1,1,0,0,1,1,0,0,0] | [0,2,5,9,13,17,22,28,20,12,14] | $N_{9,9,8,7,4,3}$ [64] | |
| | [3,0,0,0,2,0,1,0,0,0] | [0,3,6,9,12,17,22,28,20,12,14] | $N_{9,9,9,5,5,3}$ [30] | |
| | [0,1,2,0,2,0,0,0,0,0] | [1,2,4,8,12,18,24,30,21,12,15] | $N_{10,8,7,7,5,5}$ [18] | |
| | [1,0,0,3,1,0,0,0,0,0] | [1,3,5,7,12,18,24,30,21,12,15] | $N_{10,9,6,6,6,5}$ [16] | |
| | [1,2,2,0,0,0,1,0,0,0] | [0,1,4,9,14,19,24,30,21,12,15] | $N_{9,8,8,7,7,3}$ [40] | |
| | [1,3,0,0,1,1,0,0,0,0] | [0,1,5,9,13,18,24,30,21,12,15] | $N_{9,8,8,8,5,4}$ [32] | |
| | [2,0,2,1,0,1,0,0,0,0] | [0,2,4,8,13,18,24,30,21,12,15] | $N_{9,9,7,7,6,4}$ [36] | |
| | [2,1,0,1,2,0,0,0,0,0] | [0,2,5,8,12,18,24,30,21,12,15] | $N_{9,9,8,6,5,5}$ [24] | |
| | [1,2,1,2,0,0,0,0,0,0] | [0,1,4,8,14,20,26,32,22,12,16] | $N_{9,8,8,7,6,6}$ [16] | |
| | [0,5,0,1,0,0,0,0,0,0] | [0,0,5,10,16,22,28,34,23,12,17] | $N_{8,8,8,8,8,6}$ [9] | |
| | [0,0,0,0,0,0,0,2,2,0] | [3,6,9,12,15,18,21,24,17,12,12] | $N_{10,10,10,2,2,1,1}$ [13] | $N_{10,10,10,2,2}$ [14] |
| | [1,0,0,0,0,1,0,0,3,1] | [2,5,8,11,14,17,21,25,17,12,12] | $N_{10,10,9,4,1,1,1}$ [48] | $N_{10,10,9,4,1}$ [48] |
| | [0,0,1,0,1,1,0,0,0,2] | [2,4,6,9,12,16,21,26,19,12,12] | $N_{10,10,7,5,4}$ [60] | $N_{10,10,7,5,4,1,1}$ [60] |
| | [1,1,0,1,0,0,1,0,0,2] | [1,3,6,9,13,17,21,26,19,12,12] | $N_{10,9,8,6,3}$ [96] | $N_{10,9,8,6,3,1,1}$ [96] |
| | [2,0,0,0,0,2,0,0,0,2] | [1,4,7,10,13,16,21,26,19,12,12] | $N_{10,9,9,4,4}$ [30] | $N_{10,9,9,4,4,1,1}$ [30] |
| | [3,1,0,0,0,0,0,0,1,3] | [0,3,7,11,15,19,23,27,19,12,12] | $N_{9,9,9,8,1}$ [32] | $N_{9,9,9,8,1,1,1}$ [32] |

| | | | | |
|---|---|---|---|---|
| | [0,1,0,1,0,0,0,0,4,0] | [2,4,7,10,14,18,22,26,17,12,13] | $N_{10,10,8,6,1,1,1,1}$ [31] | $N_{10,10,8,6}$ [32] |
| | [0,0,1,0,1,1,0,0,2,0] | [2,4,6,9,12,16,21,26,18,12,13] | $N_{10,10,7,5,4,1,1}$ [60] | $N_{10,10,7,5,4}$ [60] |
| | [1,1,0,1,0,0,1,0,2,0] | [1,3,6,9,13,17,21,26,18,12,13] | $N_{10,9,8,6,3,1,1}$ [96] | $N_{10,9,8,6,3}$ [96] |
| | [3,1,0,0,0,0,0,0,3,1] | [0,3,7,11,15,19,23,27,18,12,13] | $N_{9,9,9,8,1,1,1}$ [32] | $N_{9,9,9,8,1}$ [32] |
| | [2,1,1,0,1,0,0,0,0,2] | [0,2,5,9,13,18,23,28,20,12,13] | $N_{9,9,8,7,5}$ [72] | $N_{9,9,8,7,5,1,1}$ [72] |
| | [0,2,0,2,0,0,0,0,2,0] | [1,2,5,8,13,18,23,28,19,12,14] | $N_{10,8,8,6,6,1,1}$ [31] | $N_{10,8,8,6,6}$ [32] |
| | [2,1,1,0,1,0,0,0,2,0] | [0,2,5,9,13,18,23,28,19,12,14] | $N_{9,9,8,7,5,1,1}$ [72] | $N_{9,9,8,7,5}$ [72] |
| 13 | [0,0,0,0,0,1,0,2,1,0] | [3,6,9,12,15,18,22,26,19,13,13] | $O_{10,10,10,4,2,2,1}$ [31] | $O_{10,10,10,4,2,2}$ [32] |
| | [0,1,1,0,0,0,0,1,2,1] | [2,4,7,11,15,19,23,27,19,13,13] | $O_{10,10,8,7,2,1,1}$ [72] | $O_{10,10,8,7,2,1}$ [72] |
| | [1,0,0,0,1,0,1,0,2,1] | [2,5,8,11,14,18,22,27,19,13,13] | $O_{10,10,9,5,3,1,1}$ [90] | $O_{10,10,9,5,3,1}$ [90] |
| | [2,1,0,0,0,0,0,0,3,2] | [1,4,8,12,16,20,24,28,19,13,13] | $O_{10,9,9,8,1,1,1}$ [32] | $O_{10,9,9,8,1,1}$ [32] |
| | [0,0,0,0,0,0,3,0,0,1] | [3,6,9,12,15,18,21,27,20,13,13] | $O_{10,10,10,3,3,3}$ [16] | $O_{10,10,10,3,3,3,1}$ [16] |
| | [0,0,2,0,0,1,0,0,1,2] | [2,4,6,10,14,18,23,28,20,13,13] | $O_{10,10,7,7,4,1}$ [64] | $O_{10,10,7,7,4,1,1}$ [64] |
| | [0,1,0,0,2,0,0,0,1,2] | [2,4,7,10,13,18,23,28,20,13,13] | $O_{10,10,8,5,5,1}$ [60] | $O_{10,10,8,5,5,1,1}$ [60] |
| | [0,1,0,1,0,0,1,1,0,1] | [2,4,7,10,14,18,22,27,20,13,13] | $O_{10,10,8,6,3,2}$ [108] | $O_{10,10,8,6,3,2,1}$ [108] |
| | [1,0,0,0,0,2,0,1,0,1] | [2,5,8,11,14,17,22,27,20,13,13] | $O_{10,10,9,4,4,2}$ [54] | $O_{10,10,9,4,4,2,1}$ [54] |
| | [1,2,0,0,0,0,1,0,1,2] | [1,3,7,11,15,19,23,28,20,13,13] | $O_{10,9,8,8,3,1}$ [72] | $O_{10,9,8,8,3,1,1}$ [72] |
| | [2,0,0,1,0,1,0,0,1,2] | [1,4,7,10,14,18,23,28,20,13,13] | $O_{10,9,9,6,4,1}$ [96] | $O_{10,9,9,6,4,1,1}$ [96] |
| | [2,0,1,0,0,0,0,2,0,1] | [1,4,7,11,15,19,23,27,20,13,13] | $O_{10,9,9,7,2,2}$ [54] | $O_{10,9,9,7,2,2,1}$ [54] |
| | [0,0,1,2,0,0,0,0,0,3] | [2,4,6,9,14,19,24,29,21,13,13] | $O_{10,10,7,6,6}$ [28] | $O_{10,10,7,6,6,1,1,1}$ [28] |
| | [1,1,1,0,1,0,0,0,0,3] | [1,3,6,10,14,19,24,29,21,13,13] | $O_{10,9,8,7,5}$ [72] | $O_{10,9,8,7,5,1,1,1}$ [72] |
| | [4,0,0,0,0,0,1,0,0,3] | [0,4,8,12,16,20,24,29,21,13,13] | $O_{9,9,9,9,3}$ [28] | $O_{9,9,9,9,3,1,1,1}$ [28] |
| | [0,0,0,1,0,0,0,0,5,0] | [3,6,9,12,16,20,24,28,18,13,14] | $O_{10,10,10,6,1,1,1,1,1}$ [17] | $O_{10,10,10,6}$ [18] |
| | [0,1,0,1,0,1,0,0,3,0] | [2,4,7,10,14,18,23,28,19,13,14] | $O_{10,10,8,6,4,1,1,1}$ [67] | $O_{10,10,8,6,4}$ [68] |
| | [2,0,1,0,0,0,1,0,3,0] | [1,4,7,11,15,19,23,28,19,13,14] | $O_{10,9,9,7,3,1,1,1}$ [60] | $O_{10,9,9,7,3}$ [60] |
| | [0,0,1,1,1,0,0,1,1,0] | [2,4,6,9,13,18,23,28,20,13,14] | $O_{10,10,7,6,5,2,1}$ [96] | $O_{10,10,7,6,5,2}$ [96] |
| | [0,0,2,0,0,0,2,0,1,0] | [2,4,6,10,14,18,22,28,20,13,14] | $O_{10,10,7,7,3,3,1}$ [40] | $O_{10,10,7,7,3,3}$ [40] |
| | [0,1,0,0,1,1,1,0,1,0] | [2,4,7,10,13,17,22,28,20,13,14] | $O_{10,10,8,5,4,3,1}$ [96] | $O_{10,10,8,5,4,3}$ [96] |
| | [1,1,0,2,0,0,0,0,2,1] | [1,3,6,9,14,19,24,29,20,13,14] | $O_{10,9,8,6,6,1,1}$ [72] | $O_{10,9,8,6,6,1}$ [72] |
| | [1,1,1,0,0,1,0,1,1,0] | [1,3,6,10,14,18,23,28,20,13,14] | $O_{10,9,8,7,4,2,1}$ [144] | $O_{10,9,8,7,4,2}$ [144] |
| | [2,0,0,0,2,0,0,1,1,0] | [1,4,7,10,13,18,23,28,20,13,14] | $O_{10,9,9,5,5,2,1}$ [60] | $O_{10,9,9,5,5,2}$ [60] |
| | [2,0,0,1,0,0,2,0,1,0] | [1,4,7,10,14,18,22,28,20,13,14] | $O_{10,9,9,6,3,3,1}$ [64] | $O_{10,9,9,6,3,3}$ [64] |
| | [3,1,0,0,0,1,0,0,2,1] | [0,3,7,11,15,19,24,29,20,13,14] | $O_{9,9,9,8,4,1,1}$ [80] | $O_{9,9,9,8,4,1}$ [80] |
| | [4,0,0,0,0,0,0,2,1,0] | [0,4,8,12,16,20,24,28,20,13,14] | $O_{9,9,9,9,2,2,1}$ [24] | $O_{9,9,9,9,2,2}$ [24] |
| | [0,0,1,1,0,2,0,0,0,1] | [2,4,6,9,13,17,23,29,21,13,14] | $O_{10,10,7,6,4,4}$ [60] | $O_{10,10,7,6,4,4,1}$ [60] |
| | [0,2,2,0,0,0,0,0,1,2] | [1,2,5,10,15,20,25,30,21,13,14] | $O_{10,8,8,7,7,1}$ [42] | $O_{10,8,8,7,7,1,1}$ [42] |
| | [0,3,0,0,1,0,0,1,0,1] | [1,2,6,10,14,19,24,29,21,13,14] | $O_{10,8,8,8,5,2}$ [72] | $O_{10,8,8,8,5,2,1}$ [72] |
| | [1,0,2,1,0,0,0,1,0,1] | [1,3,5,9,14,19,24,29,21,13,14] | $O_{10,9,7,7,6,2}$ [90] | $O_{10,9,7,7,6,2,1}$ [90] |
| | [1,1,0,1,1,0,1,0,0,1] | [1,3,6,9,13,18,23,29,21,13,14] | $O_{10,9,8,6,5,3}$ [144] | $O_{10,9,8,6,5,3,1}$ [144] |
| | [2,0,0,0,1,2,0,0,0,1] | [1,4,7,10,13,17,23,29,21,13,14] | $O_{10,9,9,5,4,4}$ [50] | $O_{10,9,9,5,4,4,1}$ [50] |
| | [2,2,0,1,0,0,0,0,1,2] | [0,2,6,10,15,20,25,30,21,13,14] | $O_{9,9,8,8,6,1}$ [72] | $O_{9,9,8,8,6,1,1}$ [72] |
| | [3,0,1,0,1,0,0,1,0,1] | [0,3,6,10,14,19,24,29,21,13,14] | $O_{9,9,9,7,5,2}$ [108] | $O_{9,9,9,7,5,2,1}$ [108] |
| | [3,1,0,0,0,0,2,0,0,1] | [0,3,7,11,15,19,23,29,21,13,14] | $O_{9,9,9,8,3,3}$ [48] | $O_{9,9,9,8,3,3,1}$ [48] |
| | [0,3,0,1,0,0,0,0,3,0] | [1,2,6,10,15,20,25,30,20,13,15] | $O_{10,8,8,8,6,1,1,1}$ [31] | $O_{10,8,8,8,6}$ [32] |
| | [3,0,1,1,0,0,0,0,3,0] | [0,3,6,10,15,20,25,30,20,13,15] | $O_{9,9,9,7,6,1,1,1}$ [42] | $O_{9,9,9,7,6}$ [42] |
| | [0,0,0,3,0,1,0,0,1,0] | [2,4,6,8,13,18,24,30,21,13,15] | $O_{10,10,6,6,6,4,1}$ [37] | $O_{10,10,6,6,6,4}$ [38] |
| | [0,2,1,1,0,0,1,0,1,0] | [1,2,5,9,14,19,24,30,21,13,15] | $O_{10,8,8,7,6,3,1}$ [96] | $O_{10,8,8,7,6,3}$ [96] |
| | [0,3,0,0,0,2,0,0,1,0] | [1,2,6,10,14,18,24,30,21,13,15] | $O_{10,8,8,8,4,4,1}$ [37] | $O_{10,8,8,8,4,4}$ [38] |
| | [1,0,2,0,1,1,0,0,1,0] | [1,3,5,9,13,18,24,30,21,13,15] | $O_{10,9,7,7,5,4,1}$ [90] | $O_{10,9,7,7,5,4}$ [90] |
| | [2,1,2,0,0,0,0,1,1,0] | [0,2,5,10,15,20,25,30,21,13,15] | $O_{9,9,8,7,7,2,1}$ [72] | $O_{9,9,8,7,7,2}$ [72] |
| | [2,2,0,0,1,0,1,0,1,0] | [0,2,6,10,14,19,24,30,21,13,15] | $O_{9,9,8,8,5,3,1}$ [96] | $O_{9,9,8,8,5,3}$ [96] |
| | [3,0,0,2,0,0,1,0,1,0] | [0,3,6,9,14,19,24,30,21,13,15] | $O_{9,9,9,6,6,3,1}$ [64] | $O_{9,9,9,6,6,3}$ [64] |
| | [3,0,1,0,0,2,0,0,1,0] | [0,3,6,10,14,18,24,30,21,13,15] | $O_{9,9,9,7,4,4,1}$ [60] | $O_{9,9,9,7,4,4}$ [60] |
| | [0,2,1,0,2,0,0,0,0,1] | [1,2,5,9,13,19,25,31,22,13,15] | $O_{10,8,8,7,5,5}$ [54] | $O_{10,8,8,7,5,5,1}$ [54] |
| | [1,0,1,2,1,0,0,0,0,1] | [1,3,5,8,13,19,25,31,22,13,15] | $O_{10,9,7,6,6,5}$ [72] | $O_{10,9,7,6,6,5,1}$ [72] |
| | [1,4,0,0,0,0,0,1,0,1] | [0,1,6,11,16,21,26,31,22,13,15] | $O_{9,8,8,8,8,2}$ [42] | $O_{9,8,8,8,8,2,1}$ [42] |
| | [2,1,1,1,0,1,0,0,0,1] | [0,2,5,9,14,19,25,31,22,13,15] | $O_{9,9,8,7,6,4}$ [120] | $O_{9,9,8,7,6,4,1}$ [120] |
| | [3,0,0,1,2,0,0,0,0,1] | [0,3,6,9,13,19,25,31,22,13,15] | $O_{9,9,9,6,5,5}$ [48] | $O_{9,9,9,6,5,5,1}$ [48] |
| | [0,1,3,0,1,0,0,0,1,0] | [1,2,4,9,14,20,26,32,22,13,16] | $O_{10,8,7,7,7,5,1}$ [54] | $O_{10,8,7,7,7,5}$ [54] |
| | [0,2,0,3,0,0,0,0,1,0] | [1,2,5,8,14,20,26,32,22,13,16] | $O_{10,8,8,6,6,6,1}$ [31] | $O_{10,8,8,6,6,6}$ [32] |
| | [1,3,1,0,0,1,0,0,1,0] | [0,1,5,10,15,20,26,32,22,13,16] | $O_{9,8,8,8,7,4,1}$ [80] | $O_{9,8,8,8,7,4}$ [80] |
| | [1,3,0,2,0,0,0,0,0,1] | [0,1,5,9,15,21,27,33,23,13,16] | $O_{9,8,8,8,6,6}$ [42] | $O_{9,8,8,8,6,6,1}$ [42] |
| | [2,0,3,1,0,0,0,0,0,1] | [0,2,4,9,15,21,27,33,23,13,16] | $O_{9,9,7,7,7,6}$ [42] | $O_{9,9,7,7,7,6,1}$ [42] |
| | [1,2,3,0,0,0,0,0,1,0] | [0,1,4,10,16,22,28,34,23,13,17] | $O_{9,8,8,7,7,7,1}$ [32] | $O_{9,8,8,7,7,7}$ [32] |
| | [0,6,0,0,0,0,0,0,1,0] | [0,0,6,12,18,24,30,36,24,13,18] | $O_{8,8,8,8,8,8,1}$ [13] | $O_{8,8,8,8,8,8}$ [14] |
| 14 | [0,0,0,0,1,0,2,0,1,1] | [3,6,9,12,15,19,23,29,21,14,14] | $P_{10,10,10,5,3,3,1}$ [54] | |
| | [0,0,0,1,0,0,0,3,0,0] | [3,6,9,12,16,20,24,28,21,14,14] | $P_{10,10,10,6,2,2,2}$ [25] | |
| | [0,1,1,0,1,0,0,0,2,2] | [2,4,7,11,15,20,25,30,21,14,14] | $P_{10,10,8,7,5,1,1}$ [90] | |
| | [0,2,0,0,0,0,1,1,1,1] | [2,4,8,12,16,20,24,29,21,14,14] | $P_{10,10,8,8,3,2,1}$ [72] | |
| | [1,0,0,1,0,1,0,1,1,1] | [2,5,8,11,15,19,24,29,21,14,14] | $P_{10,10,9,6,4,2,1}$ [144] | |
| | [2,1,0,0,0,1,0,0,2,2] | [1,4,8,12,16,20,25,30,21,14,14] | $P_{10,9,9,8,4,1,1}$ [80] | |

| | | | | |
|---|---|---|---|---|
| | [3,0,0,0,0,0,0,2,1,1] | [1,5,9,13,17,21,25,29,21,14,14] | $P_{10,9,9,9,2,2,1}$ [32] | |
| | [0,0,2,0,1,1,0,0,1,1] | [2,4,6,10,14,19,25,31,22,14,15] | $P_{10,10,7,7,5,4,1}$ [96] | |
| | [0,0,2,1,0,0,0,2,0,0] | [2,4,6,10,15,20,25,30,22,14,15] | $P_{10,10,7,7,6,2,2}$ [40] | |
| | [0,1,0,1,1,0,1,1,0,0] | [2,4,7,10,14,19,24,30,22,14,15] | $P_{10,10,8,6,5,3,2}$ [108] | |
| | [1,0,0,0,1,2,0,1,0,0] | [2,5,8,11,14,18,24,30,22,14,15] | $P_{10,10,9,5,4,4,2}$ [60] | |
| | [1,0,0,1,0,0,3,0,0,0] | [2,5,8,11,15,19,23,30,22,14,15] | $P_{10,10,9,6,3,3,3}$ [32] | |
| | [1,1,1,1,0,0,1,0,1,1] | [1,3,6,10,15,20,25,31,22,14,15] | $P_{10,9,8,7,6,3,1}$ [192] | |
| | [1,2,0,0,0,2,0,0,1,1] | [1,3,7,11,15,19,25,31,22,14,15] | $P_{10,9,8,8,4,4,1}$ [80] | |
| | [1,2,0,0,1,0,0,2,0,0] | [1,3,7,11,15,20,25,30,22,14,15] | $P_{10,9,8,8,5,2,2}$ [64] | |
| | [2,0,0,1,1,1,0,0,1,1] | [1,4,7,10,14,19,25,31,22,14,15] | $P_{10,9,9,6,5,4,1}$ [128] | |
| | [2,0,1,0,0,1,1,1,0,0] | [1,4,7,11,15,19,24,30,22,14,15] | $P_{10,9,9,7,4,3,2}$ [96] | |
| | [3,1,0,1,0,0,0,1,1,1] | [0,3,7,11,16,21,26,31,22,14,15] | $P_{9,9,9,8,6,2,1}$ [120] | |
| | [4,0,0,0,0,1,1,0,1,1] | [0,4,8,12,16,20,25,31,22,14,15] | $P_{9,9,9,9,4,3,1}$ [72] | |
| | [0,0,1,2,0,1,1,0,0,0] | [2,4,6,9,14,19,25,32,23,14,16] | $P_{10,10,7,6,6,4,3}$ [48] | |
| | [0,1,0,1,0,3,0,0,0,0] | [2,4,7,10,14,18,25,32,23,14,16] | $P_{10,10,8,6,4,4,4}$ [27] | |
| | [0,2,2,0,1,0,0,0,1,1] | [1,2,5,10,15,21,27,33,23,14,16] | $P_{10,8,8,7,7,5,1}$ [90] | |
| | [0,3,0,1,0,1,0,1,0,0] | [1,2,6,10,15,20,26,32,23,14,16] | $P_{10,8,8,8,6,4,2}$ [81] | |
| | [1,0,2,2,0,0,0,0,1,1] | [1,3,5,9,15,21,27,33,23,14,16] | $P_{10,9,7,7,6,6,1}$ [72] | |
| | [1,0,3,0,0,1,0,1,0,0] | [1,3,5,10,15,20,26,32,23,14,16] | $P_{10,9,7,7,7,4,2}$ [72] | |
| | [1,1,0,2,1,0,0,1,0,0] | [1,3,6,9,14,20,26,32,23,14,16] | $P_{10,9,8,6,6,5,2}$ [96] | |
| | [1,1,1,0,1,1,1,0,0,0] | [1,3,6,10,14,19,25,32,23,14,16] | $P_{10,9,8,7,5,4,3}$ [96] | |
| | [2,2,0,1,1,0,0,0,1,1] | [0,2,6,10,15,21,27,33,23,14,16] | $P_{9,9,8,8,6,5,1}$ [120] | |
| | [2,2,1,0,0,0,1,1,0,0] | [0,2,6,11,16,21,26,32,23,14,16] | $P_{9,9,8,8,7,3,2}$ [80] | |
| | [3,0,1,1,0,1,0,1,0,0] | [0,3,6,10,15,20,26,32,23,14,16] | $P_{9,9,9,7,6,4,2}$ [108] | |
| | [3,1,0,0,1,0,2,0,0,0] | [0,3,7,11,15,20,25,32,23,14,16] | $P_{9,9,9,8,5,3,3}$ [48] | |
| | [0,2,1,2,0,0,1,0,0,0] | [1,2,5,9,15,21,27,34,24,14,17] | $P_{10,8,8,7,6,6,3}$ [48] | |
| | [0,3,0,0,2,1,0,0,0,0] | [1,2,6,10,14,20,27,34,24,14,17] | $P_{10,8,8,8,5,5,4}$ [24] | |
| | [1,0,2,1,1,1,0,0,0,0] | [1,3,5,9,14,20,27,34,24,14,17] | $P_{10,9,7,7,6,5,4}$ [48] | |
| | [1,3,2,0,0,0,0,0,1,1] | [0,1,5,11,17,23,29,35,24,14,17] | $P_{9,8,8,8,7,7,1}$ [56] | |
| | [1,4,0,0,1,0,0,1,0,0] | [0,1,6,11,16,22,28,34,24,14,17] | $P_{9,8,8,8,8,5,2}$ [64] | |
| | [2,1,2,0,1,0,1,0,0,0] | [0,2,5,10,15,21,27,34,24,14,17] | $P_{9,9,8,7,7,5,3}$ [72] | |
| | [2,2,0,1,0,2,0,0,0,0] | [0,2,6,10,15,20,27,34,24,14,17] | $P_{9,9,8,8,6,4,4}$ [36] | |
| | [3,0,0,3,0,0,1,0,0,0] | [0,3,6,9,15,21,27,34,24,14,17] | $P_{9,9,9,6,6,6,3}$ [32] | |
| | [3,0,1,0,2,1,0,0,0,0] | [0,3,6,10,14,20,27,34,24,14,17] | $P_{9,9,9,7,5,5,4}$ [36] | |
| | [0,0,0,5,0,0,0,0,0,0] | [2,4,6,8,15,22,29,36,25,14,18] | $P_{10,10,6,6,6,6,6}$ [5] | |
| | [0,1,4,0,0,1,0,0,0,0] | [1,2,4,10,16,22,29,36,25,14,18] | $P_{10,8,7,7,7,7,4}$ [24] | |
| | [1,3,1,1,0,1,0,0,0,0] | [0,1,5,10,16,22,29,36,25,14,18] | $P_{9,8,8,8,7,6,4}$ [48] | |
| | [2,1,1,2,1,0,0,0,0,0] | [0,2,5,9,15,22,29,36,25,14,18] | $P_{9,9,8,7,6,6,5}$ [32] | |
| | [2,0,4,1,0,0,0,0,0,0] | [0,2,4,10,17,24,31,38,26,14,19] | $P_{9,9,7,7,7,7,6}$ [12] | |
| | [0,6,0,1,0,0,0,0,0,0] | [0,0,6,12,19,26,33,40,27,14,20] | $P_{8,8,8,8,8,8,6}$ [9] | |
| | [0,0,0,1,0,0,1,0,3,1] | [3,6,9,12,16,20,24,29,20,14,14] | $P_{10,10,10,6,3,1,1,1}$ [60] | $P_{10,10,10,6,3,1}$ [60] |
| | [1,1,0,0,0,0,0,1,3,1] | [2,5,9,13,17,21,25,29,20,14,14] | $P_{10,10,9,8,2,1,1,1}$ [56] | $P_{10,10,9,8,2,1}$ [56] |
| | [0,0,0,0,0,3,0,0,0,2] | [3,6,9,12,15,18,24,30,22,14,14] | $P_{10,10,10,4,4,4}$ [18] | $P_{10,10,10,4,4,4,1,1}$ [17] |
| | [0,0,3,0,0,0,0,0,1,3] | [2,4,6,11,16,21,26,31,22,14,14] | $P_{10,10,7,7,7,1}$ [28] | $P_{10,10,7,7,7,1,1,1}$ [28] |
| | [0,1,0,2,0,0,0,1,0,2] | [2,4,7,10,15,20,25,30,22,14,14] | $P_{10,10,8,6,6,2}$ [68] | $P_{10,10,8,6,6,2,1,1}$ [67] |
| | [0,1,1,0,0,1,1,0,0,2] | [2,4,7,11,15,19,24,30,22,14,14] | $P_{10,10,8,7,4,3}$ [96] | $P_{10,10,8,7,4,3,1,1}$ [96] |
| | [1,0,0,0,2,0,1,0,0,2] | [2,5,8,11,14,19,24,30,22,14,14] | $P_{10,10,9,5,5,3}$ [60] | $P_{10,10,9,5,5,3,1,1}$ [60] |
| | [1,2,0,1,0,0,0,0,1,3] | [1,3,7,11,16,21,26,31,22,14,14] | $P_{10,9,8,8,6,1}$ [72] | $P_{10,9,8,8,6,1,1,1}$ [72] |
| | [2,0,1,0,1,0,0,1,0,2] | [1,4,7,11,15,20,25,30,22,14,14] | $P_{10,9,9,7,5,2}$ [108] | $P_{10,9,9,7,5,2,1,1}$ [108] |
| | [2,1,0,0,0,0,2,0,0,2] | [1,4,8,12,16,20,24,30,22,14,14] | $P_{10,9,9,8,3,3}$ [48] | $P_{10,9,9,8,3,3,1,1}$ [48] |
| | [4,0,0,1,0,0,0,0,0,4] | [0,4,8,12,17,22,27,32,23,14,14] | $P_{9,9,9,9,6}$ [28] | $P_{9,9,9,9,6,1,1,1,1}$ [28] |
| | [1,0,1,0,0,1,0,0,4,0] | [2,5,8,12,16,20,25,30,20,14,15] | $P_{10,10,9,7,4,1,1,1,1}$ [60] | $P_{10,10,9,7,4}$ [60] |
| | [0,0,0,0,0,3,0,0,2,0] | [3,6,9,12,15,18,24,30,21,14,15] | $P_{10,10,10,4,4,4,1,1}$ [17] | $P_{10,10,10,4,4,4}$ [18] |
| | [0,1,0,2,0,0,0,1,2,0] | [2,4,7,10,15,20,25,30,21,14,15] | $P_{10,10,8,6,6,2,1,1}$ [67] | $P_{10,10,8,6,6,2}$ [68] |
| | [0,1,1,0,0,1,1,0,2,0] | [2,4,7,11,15,19,24,30,21,14,15] | $P_{10,10,8,7,4,3,1,1}$ [96] | $P_{10,10,8,7,4,3}$ [96] |
| | [1,0,0,0,2,0,1,0,2,0] | [2,5,8,11,14,19,24,30,21,14,15] | $P_{10,10,9,5,5,3,1,1}$ [60] | $P_{10,10,9,5,5,3}$ [60] |
| | [1,2,0,1,0,0,0,0,3,1] | [1,3,7,11,16,21,26,31,21,14,15] | $P_{10,9,8,8,6,1,1,1}$ [72] | $P_{10,9,8,8,6,1}$ [72] |
| | [2,0,1,0,1,0,0,1,2,0] | [1,4,7,11,15,20,25,30,21,14,15] | $P_{10,9,9,7,5,2,1,1}$ [108] | $P_{10,9,9,7,5,2}$ [108] |
| | [2,1,0,0,0,0,2,0,2,0] | [1,4,8,12,16,20,24,30,21,14,15] | $P_{10,9,9,8,3,3,1,1}$ [48] | $P_{10,9,9,8,3,3}$ [48] |
| | [0,0,1,2,1,0,0,0,0,2] | [2,4,6,9,14,20,26,32,23,14,15] | $P_{10,10,7,6,6,5}$ [48] | $P_{10,10,7,6,6,5,1,1}$ [48] |
| | [0,3,1,0,0,0,1,0,0,2] | [1,2,6,11,16,21,26,32,23,14,15] | $P_{10,8,8,8,7,3}$ [60] | $P_{10,8,8,8,7,3,1,1}$ [60] |
| | [1,1,1,0,2,0,0,0,0,2] | [1,3,6,10,14,20,26,32,23,14,15] | $P_{10,9,8,7,5,5}$ [72] | $P_{10,9,8,7,5,5,1,1}$ [72] |
| | [2,3,0,0,0,0,0,1,0,2] | [0,2,7,12,17,22,27,32,23,14,15] | $P_{9,9,8,8,8,2}$ [42] | $P_{9,9,8,8,8,2,1,1}$ [42] |
| | [3,0,2,0,0,0,1,0,0,2] | [0,3,6,11,16,21,26,32,23,14,15] | $P_{9,9,9,7,7,3}$ [60] | $P_{9,9,9,7,7,3,1,1}$ [60] |
| | [3,1,0,0,1,1,0,0,0,2] | [0,3,7,11,15,20,26,32,23,14,15] | $P_{9,9,9,8,5,4}$ [80] | $P_{9,9,9,8,5,4,1,1}$ [80] |
| | [4,0,0,1,0,0,0,0,4,0] | [0,4,8,12,17,22,27,32,21,14,16] | $P_{9,9,9,9,6,1,1,1,1}$ [28] | $P_{9,9,9,9,6}$ [28] |
| | [0,0,1,2,1,0,0,0,2,0] | [2,4,6,9,14,20,26,32,22,14,16] | $P_{10,10,7,6,6,5,1,1}$ [48] | $P_{10,10,7,6,6,5}$ [48] |
| | [0,3,1,0,0,0,1,0,2,0] | [1,2,6,11,16,21,26,32,22,14,16] | $P_{10,8,8,8,7,3,1,1}$ [60] | $P_{10,8,8,8,7,3}$ [60] |
| | [1,1,1,0,2,0,0,0,2,0] | [1,3,6,10,14,20,26,32,22,14,16] | $P_{10,9,8,7,5,5,1,1}$ [72] | $P_{10,9,8,7,5,5}$ [72] |
| | [2,3,0,0,0,0,0,1,2,0] | [0,2,7,12,17,22,27,32,22,14,16] | $P_{9,9,8,8,8,2,1,1}$ [42] | $P_{9,9,8,8,8,2}$ [42] |
| | [3,0,2,0,0,0,1,0,2,0] | [0,3,6,11,16,21,26,32,22,14,16] | $P_{9,9,9,7,7,3,1,1}$ [60] | $P_{9,9,9,7,7,3}$ [60] |

| | | | | |
|---|---|---|---|---|
| | [3,1,0,0,1,1,0,0,2,0] | [0,3,7,11,15,20,26,32,22,14,16] | $P_{9,9,9,8,5,4,1,1}$ [80] | $P_{9,9,9,8,5,4}$ [80] |
| | [2,1,2,1,0,0,0,0,0,2] | [0,2,5,10,16,22,28,34,24,14,16] | $P_{9,9,8,7,7,6}$ [56] | $P_{9,9,8,7,7,6,1,1}$ [56] |
| | [2,1,2,1,0,0,0,0,2,0] | [0,2,5,10,16,22,28,34,23,14,17] | $P_{9,9,8,7,7,6,1,1}$ [56] | $P_{9,9,8,7,7,6}$ [56] |
| 15 | [1,0,0,0,0,0,0,1,4,1] | [3,7,11,15,19,23,27,31,21,15,15] | $Q_{10,10,10,9,2,1,1,1,1}$ [32] | $Q_{10,10,10,9,2,1}$ [32] |
| | [0,0,0,1,1,0,0,1,2,1] | [3,6,9,12,16,21,26,31,22,15,15] | $Q_{10,10,10,6,5,2,1,1}$ [80] | $Q_{10,10,10,6,5,2,1}$ [80] |
| | [0,0,1,0,0,0,2,0,2,1] | [3,6,9,13,17,21,25,31,22,15,15] | $Q_{10,10,10,7,3,3,1,1}$ [60] | $Q_{10,10,10,7,3,3,1}$ [60] |
| | [0,1,0,0,0,0,0,3,1,0] | [3,6,10,14,18,22,26,30,22,15,15] | $Q_{10,10,10,8,2,2,2,1}$ [31] | $Q_{10,10,10,8,2,2,2}$ [32] |
| | [1,0,1,1,0,0,0,0,3,2] | [2,5,8,12,17,22,27,32,22,15,15] | $Q_{10,10,9,7,6,1,1,1}$ [72] | $Q_{10,10,9,7,6,1,1}$ [72] |
| | [1,1,0,0,0,1,0,1,2,1] | [2,5,9,13,17,21,26,31,22,15,15] | $Q_{10,10,9,8,4,2,1,1}$ [120] | $Q_{10,10,9,8,4,2,1}$ [120] |
| | [0,0,0,0,2,1,0,0,1,2] | [3,6,9,12,15,20,26,32,23,15,15] | $Q_{10,10,10,5,5,4,1}$ [48] | $Q_{10,10,10,5,5,4,1,1}$ [48] |
| | [0,0,0,1,0,1,1,1,0,1] | [3,6,9,12,16,20,25,31,23,15,15] | $Q_{10,10,10,6,4,3,2}$ [90] | $Q_{10,10,10,6,4,3,2,1}$ [90] |
| | [0,1,2,0,0,0,0,1,1,2] | [2,4,7,12,17,22,27,32,23,15,15] | $Q_{10,10,8,7,7,2,1}$ [72] | $Q_{10,10,8,7,7,2,1,1}$ [72] |
| | [0,2,0,0,1,0,1,0,1,2] | [2,4,8,12,16,21,26,32,23,15,15] | $Q_{10,10,8,8,5,3,1}$ [108] | $Q_{10,10,8,8,5,3,1,1}$ [108] |
| | [1,0,0,2,0,0,1,0,1,2] | [2,5,8,11,16,21,26,32,23,15,15] | $Q_{10,10,9,6,6,3,1}$ [96] | $Q_{10,10,9,6,6,3,1,1}$ [96] |
| | [1,0,1,0,0,2,0,0,1,2] | [2,5,8,12,16,20,26,32,23,15,15] | $Q_{10,10,9,7,4,4,1}$ [96] | $Q_{10,10,9,7,4,4,1,1}$ [96] |
| | [1,0,1,0,1,0,0,2,0,1] | [2,5,8,12,16,21,26,31,23,15,15] | $Q_{10,10,9,7,5,2,2}$ [108] | $Q_{10,10,9,7,5,2,2,1}$ [108] |
| | [1,1,0,0,0,0,2,1,0,1] | [2,5,9,13,17,21,25,31,23,15,15] | $Q_{10,10,9,8,3,3,2}$ [72] | $Q_{10,10,9,8,3,3,2,1}$ [72] |
| | [2,1,0,1,0,0,0,1,1,2] | [1,4,8,12,17,22,27,32,23,15,15] | $Q_{10,9,9,8,6,2,1}$ [120] | $Q_{10,9,9,8,6,2,1,1}$ [120] |
| | [3,0,0,0,0,1,1,0,1,2] | [1,5,9,13,17,21,26,32,23,15,15] | $Q_{10,9,9,9,4,3,1}$ [72] | $Q_{10,9,9,9,4,3,1,1}$ [72] |
| | [0,1,1,1,0,1,0,0,0,3] | [2,4,7,11,16,21,27,33,24,15,15] | $Q_{10,10,8,7,6,4}$ [90] | $Q_{10,10,8,7,6,4,1,1,1}$ [90] |
| | [1,0,0,1,2,0,0,0,0,3] | [2,5,8,11,15,21,27,33,24,15,15] | $Q_{10,10,9,6,5,5}$ [48] | $Q_{10,10,9,6,5,5,1,1,1}$ [48] |
| | [1,3,0,0,0,0,0,1,0,3] | [1,3,8,13,18,23,28,33,24,15,15] | $Q_{10,9,8,8,8,2}$ [42] | $Q_{10,9,8,8,8,2,1,1,1}$ [42] |
| | [2,0,2,0,0,0,1,0,0,3] | [1,4,7,12,17,22,27,33,24,15,15] | $Q_{10,9,9,7,7,3}$ [60] | $Q_{10,9,9,7,7,3,1,1,1}$ [60] |
| | [2,1,0,0,1,1,0,0,0,3] | [1,4,8,12,16,21,27,33,24,15,15] | $Q_{10,9,9,8,5,4}$ [80] | $Q_{10,9,9,8,5,4,1,1,1}$ [80] |
| | [4,1,0,0,0,0,0,0,1,4] | [0,4,9,14,19,24,29,34,24,15,15] | $Q_{9,9,9,9,8,1}$ [32] | $Q_{9,9,9,9,8,1,1,1,1}$ [32] |
| | [0,1,0,0,0,1,0,0,5,0] | [3,6,10,14,18,22,27,32,21,15,16] | $Q_{10,10,10,8,4,1,1,1,1,1}$ [37] | $Q_{10,10,10,8,4}$ [38] |
| | [0,0,0,1,0,2,0,0,3,0] | [3,6,9,12,16,20,26,32,22,15,16] | $Q_{10,10,10,6,4,4,1,1,1}$ [37] | $Q_{10,10,10,6,4,4}$ [38] |
| | [0,2,0,1,0,0,0,1,3,0] | [2,4,8,12,17,22,27,32,22,15,16] | $Q_{10,10,8,8,6,2,1,1,1}$ [67] | $Q_{10,10,8,8,6,2}$ [68] |
| | [1,0,1,0,1,0,1,0,3,0] | [2,5,8,12,16,21,26,32,22,15,16] | $Q_{10,10,9,7,5,3,1,1,1}$ [108] | $Q_{10,10,9,7,5,3}$ [108] |
| | [2,1,1,0,0,0,0,0,4,1] | [1,4,8,13,18,23,28,33,22,15,16] | $Q_{10,9,9,8,7,1,1,1,1}$ [56] | $Q_{10,9,9,8,7,1}$ [56] |
| | [3,0,0,0,1,0,0,1,3,0] | [1,5,9,13,17,22,27,32,22,15,16] | $Q_{10,9,9,9,5,2,1,1,1}$ [60] | $Q_{10,9,9,9,5,2}$ [60] |
| | [0,0,0,0,2,0,2,0,1,0] | [3,6,9,12,15,20,25,32,23,15,16] | $Q_{10,10,10,5,5,3,3,1}$ [36] | $Q_{10,10,10,5,5,3,3}$ [36] |
| | [0,1,1,0,2,0,0,0,2,1] | [2,4,7,11,15,21,27,33,23,15,16] | $Q_{10,10,8,7,5,5,1,1}$ [90] | $Q_{10,10,8,7,5,5,1}$ [90] |
| | [0,1,1,1,0,0,1,1,1,0] | [2,4,7,11,16,21,26,32,23,15,16] | $Q_{10,10,8,7,6,3,2,1}$ [144] | $Q_{10,10,8,7,6,3,2}$ [144] |
| | [0,2,0,0,0,2,0,1,1,0] | [2,4,8,12,16,20,26,32,23,15,16] | $Q_{10,10,8,8,4,4,2,1}$ [67] | $Q_{10,10,8,8,4,4,2}$ [68] |
| | [1,0,0,1,1,1,0,1,1,0] | [2,5,8,11,15,20,26,32,23,15,16] | $Q_{10,10,9,6,5,4,2,1}$ [144] | $Q_{10,10,9,6,5,4,2}$ [144] |
| | [1,0,1,0,0,1,2,0,1,0] | [2,5,8,12,16,20,25,32,23,15,16] | $Q_{10,10,9,7,4,3,3,1}$ [96] | $Q_{10,10,9,7,4,3,3}$ [96] |
| | [1,2,1,0,0,0,1,0,2,1] | [1,3,7,12,17,22,27,33,23,15,16] | $Q_{10,9,8,8,7,3,1,1}$ [120] | $Q_{10,9,8,8,7,3,1}$ [120] |
| | [2,0,1,1,0,1,0,0,2,1] | [1,4,7,11,16,21,27,33,23,15,16] | $Q_{10,9,9,7,6,4,1,1}$ [144] | $Q_{10,9,9,7,6,4,1}$ [144] |
| | [2,0,2,0,0,0,0,2,1,0] | [1,4,7,12,17,22,27,32,23,15,16] | $Q_{10,9,9,7,7,2,2,1}$ [54] | $Q_{10,9,9,7,7,2,2}$ [54] |
| | [2,1,0,0,1,0,1,1,1,0] | [1,4,8,12,16,21,26,32,23,15,16] | $Q_{10,9,9,8,5,3,2,1}$ [144] | $Q_{10,9,9,8,5,3,2}$ [144] |
| | [4,0,1,0,0,0,0,1,2,1] | [0,4,8,13,18,23,28,33,23,15,16] | $Q_{9,9,9,9,7,2,1,1}$ [72] | $Q_{9,9,9,9,7,2,1}$ [72] |
| | [0,0,0,0,1,3,0,0,0,1] | [3,6,9,12,15,19,26,33,24,15,16] | $Q_{10,10,10,5,4,4,4}$ [30] | $Q_{10,10,10,5,4,4,4,1}$ [30] |
| | [0,0,2,2,0,0,0,0,1,2] | [2,4,6,10,16,22,28,34,24,15,16] | $Q_{10,10,7,7,6,6,1}$ [48] | $Q_{10,10,7,7,6,6,1,1}$ [48] |
| | [0,0,3,0,0,1,0,1,0,1] | [2,4,6,11,16,21,27,33,24,15,16] | $Q_{10,10,7,7,7,4,2}$ [72] | $Q_{10,10,7,7,7,4,2,1}$ [72] |
| | [0,1,0,2,1,0,0,1,0,1] | [2,4,7,10,15,21,27,33,24,15,16] | $Q_{10,10,8,6,6,5,2}$ [108] | $Q_{10,10,8,6,6,5,2,1}$ [108] |
| | [0,1,1,0,1,1,1,0,0,1] | [2,4,7,11,15,20,26,33,24,15,16] | $Q_{10,10,8,7,5,4,3}$ [144] | $Q_{10,10,8,7,5,4,3,1}$ [144] |
| | [1,1,2,0,1,0,0,0,1,2] | [1,3,6,11,16,22,28,34,24,15,16] | $Q_{10,9,8,7,7,5,1}$ [120] | $Q_{10,9,8,7,7,5,1,1}$ [120] |
| | [1,2,0,1,0,1,0,1,0,1] | [1,3,7,11,16,21,27,33,24,15,16] | $Q_{10,9,8,8,6,4,2}$ [162] | $Q_{10,9,8,8,6,4,2,1}$ [162] |
| | [2,0,0,3,0,0,0,0,1,2] | [1,4,7,10,16,22,28,34,24,15,16] | $Q_{10,9,9,6,6,6,1}$ [48] | $Q_{10,9,9,6,6,6,1,1}$ [48] |
| | [2,0,1,0,2,0,0,1,0,1] | [1,4,7,11,15,21,27,33,24,15,16] | $Q_{10,9,9,7,5,5,2}$ [108] | $Q_{10,9,9,7,5,5,2,1}$ [108] |
| | [2,0,1,1,0,0,2,0,0,1] | [1,4,7,11,16,21,26,33,24,15,16] | $Q_{10,9,9,7,6,3,3}$ [96] | $Q_{10,9,9,7,6,3,3,1}$ [96] |
| | [2,1,0,0,0,2,1,0,0,1] | [1,4,8,12,16,20,26,33,24,15,16] | $Q_{10,9,9,8,4,4,3}$ [80] | $Q_{10,9,9,8,4,4,3,1}$ [80] |
| | [3,1,1,0,0,1,0,0,1,2] | [0,3,7,12,17,22,28,34,24,15,16] | $Q_{9,9,9,8,7,4,1}$ [128] | $Q_{9,9,9,8,7,4,1,1}$ [128] |
| | [3,2,0,0,0,0,0,2,0,1] | [0,3,8,13,18,23,28,33,24,15,16] | $Q_{9,9,9,8,8,2,2}$ [42] | $Q_{9,9,9,8,8,2,2,1}$ [42] |
| | [4,0,0,0,2,0,0,0,1,2] | [0,4,8,12,16,22,28,34,24,15,16] | $Q_{9,9,9,9,5,5,1}$ [50] | $Q_{9,9,9,9,5,5,1,1}$ [50] |
| | [4,0,0,1,0,0,1,1,0,1] | [0,4,8,12,17,22,27,33,24,15,16] | $Q_{9,9,9,9,6,3,2}$ [96] | $Q_{9,9,9,9,6,3,2,1}$ [96] |
| | [0,4,0,0,1,0,0,0,0,3] | [1,2,7,12,17,23,29,35,25,15,16] | $Q_{10,8,8,8,8,5}$ [36] | $Q_{10,8,8,8,8,5,1,1,1}$ [36] |
| | [3,1,0,2,0,0,0,0,0,3] | [0,3,7,11,17,23,29,35,25,15,16] | $Q_{9,9,9,8,6,6}$ [42] | $Q_{9,9,9,8,6,6,1,1,1}$ [42] |
| | [0,1,0,3,0,0,0,0,3,0] | [2,4,7,10,16,22,28,34,23,15,17] | $Q_{10,10,8,6,6,6,1,1,1}$ [31] | $Q_{10,10,8,6,6,6}$ [32] |
| | [1,2,0,1,1,0,0,0,3,0] | [1,3,7,11,16,22,28,34,23,15,17] | $Q_{10,9,8,8,6,5,1,1,1}$ [72] | $Q_{10,9,8,8,6,5}$ [72] |
| | [3,2,0,0,0,0,1,0,3,0] | [0,3,8,13,18,23,28,34,23,15,17] | $Q_{9,9,9,8,8,3,1,1,1}$ [48] | $Q_{9,9,9,8,8,3}$ [48] |
| | [4,0,0,1,0,1,0,0,3,0] | [0,4,8,12,17,22,28,34,23,15,17] | $Q_{9,9,9,9,6,4,1,1,1}$ [60] | $Q_{9,9,9,9,6,4}$ [60] |
| | [0,0,2,1,1,0,1,0,1,0] | [2,4,6,10,15,21,27,34,24,15,17] | $Q_{10,10,7,7,6,5,3,1}$ [96] | $Q_{10,10,7,7,6,5,3}$ [96] |
| | [0,1,0,2,0,2,0,0,1,0] | [2,4,7,10,15,20,27,34,24,15,17] | $Q_{10,10,8,6,6,4,4,1}$ [67] | $Q_{10,10,8,6,6,4,4}$ [68] |
| | [0,3,1,1,0,0,0,0,2,1] | [1,2,6,11,17,23,29,35,24,15,17] | $Q_{10,8,8,8,7,6,1,1}$ [72] | $Q_{10,8,8,8,7,6,1}$ [72] |
| | [0,4,0,0,0,1,0,1,1,0] | [1,2,7,12,17,22,28,34,24,15,17] | $Q_{10,8,8,8,8,4,2,1}$ [67] | $Q_{10,8,8,8,8,4,2}$ [68] |
| | [1,1,1,2,0,0,0,1,1,0] | [1,3,6,10,16,22,28,34,24,15,17] | $Q_{10,9,8,7,6,6,2,1}$ [120] | $Q_{10,9,8,7,6,6,2}$ [120] |
| | [1,1,2,0,0,1,1,0,1,0] | [1,3,6,11,16,21,27,34,24,15,17] | $Q_{10,9,8,7,7,4,3,1}$ [128] | $Q_{10,9,8,7,7,4,3}$ [128] |
| | [1,2,0,0,2,0,1,0,1,0] | [1,3,7,11,15,21,27,34,24,15,17] | $Q_{10,9,8,8,5,5,3,1}$ [96] | $Q_{10,9,8,8,5,5,3}$ [96] |
| | [2,0,0,2,1,0,1,0,1,0] | [1,4,7,10,15,21,27,34,24,15,17] | $Q_{10,9,9,6,6,5,3,1}$ [96] | $Q_{10,9,9,6,6,5,3}$ [96] |

| | | | | |
|---|---|---|---|---|
| | [2,0,1,0,1,2,0,0,1,0] | [1,4,7,11,15,20,27,34,24,15,17] | $Q_{10,9,9,7,5,4,4,1}$ [90] | $Q_{10,9,9,7,5,4,4}$ [90] |
| | [2,3,0,0,1,0,0,0,2,1] | [0,2,7,12,17,23,29,35,24,15,17] | $Q_{9,9,8,8,8,5,1,1}$ [80] | $Q_{9,9,8,8,8,5,1}$ [80] |
| | [3,0,2,1,0,0,0,0,2,1] | [0,3,6,11,17,23,29,35,24,15,17] | $Q_{9,9,9,7,7,6,1,1}$ [72] | $Q_{9,9,9,7,7,6,1}$ [72] |
| | [3,1,0,1,1,0,0,1,1,0] | [0,3,7,11,16,22,28,34,24,15,17] | $Q_{9,9,9,8,6,5,2,1}$ [144] | $Q_{9,9,9,8,6,5,2}$ [144] |
| | [3,1,1,0,0,0,2,0,1,0] | [0,3,7,12,17,22,27,34,24,15,17] | $Q_{9,9,9,8,7,3,3,1}$ [80] | $Q_{9,9,9,8,7,3,3}$ [80] |
| | [4,0,0,0,1,1,1,0,1,0] | [0,4,8,12,16,21,27,34,24,15,17] | $Q_{9,9,9,9,5,4,3,1}$ [80] | $Q_{9,9,9,9,5,4,3}$ [80] |
| | [0,3,1,0,1,0,1,0,0,1] | [1,2,6,11,16,22,28,35,25,15,17] | $Q_{10,8,8,8,7,5,3}$ [108] | $Q_{10,8,8,8,7,5,3,1}$ [108] |
| | [1,0,4,0,0,0,0,1,0,1] | [1,3,5,11,17,23,29,35,25,15,17] | $Q_{10,9,7,7,7,7,2}$ [54] | $Q_{10,9,7,7,7,7,2,1}$ [54] |
| | [1,1,1,1,1,1,0,0,0,1] | [1,3,6,10,15,21,28,35,25,15,17] | $Q_{10,9,8,7,6,5,4}$ [160] | $Q_{10,9,8,7,6,5,4,1}$ [160] |
| | [2,2,1,1,0,0,0,1,0,1] | [0,2,6,11,17,23,29,35,25,15,17] | $Q_{9,9,8,8,7,6,2}$ [120] | $Q_{9,9,8,8,7,6,2,1}$ [120] |
| | [2,3,0,0,0,1,1,0,0,1] | [0,2,7,12,17,22,28,35,25,15,17] | $Q_{9,9,8,8,8,4,3}$ [80] | $Q_{9,9,8,8,8,4,3,1}$ [80] |
| | [3,0,2,0,1,0,1,0,0,1] | [0,3,6,11,16,22,28,35,25,15,17] | $Q_{9,9,9,7,7,5,3}$ [108] | $Q_{9,9,9,7,7,5,3,1}$ [108] |
| | [3,1,0,1,0,2,0,0,0,1] | [0,3,7,11,16,21,28,35,25,15,17] | $Q_{9,9,9,8,6,4,4}$ [90] | $Q_{9,9,9,8,6,4,4,1}$ [90] |
| | [2,2,2,0,0,0,0,0,3,0] | [0,2,6,12,18,24,30,36,24,15,18] | $Q_{9,9,8,8,7,7,1,1,1}$ [32] | $Q_{9,9,8,8,7,7}$ [32] |
| | [0,0,1,3,1,0,0,0,1,0] | [2,4,6,9,15,22,29,36,25,15,18] | $Q_{10,10,7,6,6,6,5,1}$ [48] | $Q_{10,10,7,6,6,6,5}$ [48] |
| | [0,2,3,0,0,0,1,0,1,0] | [1,2,5,11,17,23,29,36,25,15,18] | $Q_{10,8,8,7,7,7,3,1}$ [60] | $Q_{10,8,8,7,7,7,3}$ [60] |
| | [0,3,0,2,0,1,0,0,1,0] | [1,2,6,10,16,22,29,36,25,15,18] | $Q_{10,8,8,8,6,6,4,1}$ [67] | $Q_{10,8,8,8,6,6,4}$ [68] |
| | [1,0,3,1,0,1,0,0,1,0] | [1,3,5,10,16,22,29,36,25,15,18] | $Q_{10,9,7,7,7,6,4,1}$ [90] | $Q_{10,9,7,7,7,6,4}$ [90] |
| | [1,5,0,0,0,0,0,0,2,1] | [0,1,7,13,19,25,31,37,25,15,18] | $Q_{9,8,8,8,8,8,1,1}$ [32] | $Q_{9,8,8,8,8,8,1}$ [32] |
| | [2,2,1,0,1,1,0,0,1,0] | [0,2,6,11,16,22,29,36,25,15,18] | $Q_{9,9,8,8,7,5,4,1}$ [120] | $Q_{9,9,8,8,7,5,4}$ [120] |
| | [3,0,1,2,0,1,0,0,1,0] | [0,3,6,10,16,22,29,36,25,15,18] | $Q_{9,9,9,7,6,6,4,1}$ [90] | $Q_{9,9,9,7,6,6,4}$ [90] |
| | [3,1,0,0,3,0,0,0,1,0] | [0,3,7,11,15,22,29,36,25,15,18] | $Q_{9,9,9,8,5,5,5,1}$ [48] | $Q_{9,9,9,8,5,5,5}$ [48] |
| | [0,2,2,1,1,0,0,0,0,1] | [1,2,5,10,16,23,30,37,26,15,18] | $Q_{10,8,8,7,7,6,5}$ [72] | $Q_{10,8,8,7,7,6,5,1}$ [72] |
| | [1,1,0,4,0,0,0,0,0,1] | [1,3,6,9,16,23,30,37,26,15,18] | $Q_{10,9,8,6,6,6,6}$ [42] | $Q_{10,9,8,6,6,6,6,1}$ [42] |
| | [1,4,1,0,0,0,1,0,0,1] | [0,1,6,12,18,24,30,37,26,15,18] | $Q_{9,8,8,8,8,7,3}$ [80] | $Q_{9,8,8,8,8,7,3,1}$ [80] |
| | [2,1,3,0,0,1,0,0,0,1] | [0,2,5,11,17,23,30,37,26,15,18] | $Q_{9,9,8,7,7,7,4}$ [80] | $Q_{9,9,8,7,7,7,4,1}$ [80] |
| | [2,2,0,2,1,0,0,0,0,1] | [0,2,6,10,16,23,30,37,26,15,18] | $Q_{9,9,8,8,6,6,5}$ [72] | $Q_{9,9,8,8,6,6,5,1}$ [72] |
| | [1,4,0,1,1,0,0,0,1,0] | [0,1,6,11,17,24,31,38,26,15,19] | $Q_{9,8,8,8,8,6,5,1}$ [72] | $Q_{9,8,8,8,8,6,5}$ [72] |
| | [2,1,2,2,0,0,0,0,1,0] | [0,2,5,10,17,24,31,38,26,15,19] | $Q_{9,9,8,7,7,6,6,1}$ [56] | $Q_{9,9,8,7,7,6,6}$ [56] |
| | [1,3,2,1,0,0,0,0,0,1] | [0,1,5,11,18,25,32,39,27,15,19] | $Q_{9,8,8,8,7,7,6}$ [56] | $Q_{9,8,8,8,7,7,6,1}$ [56] |
| | [0,7,0,0,0,0,0,0,1,0] | [0,0,7,14,21,28,35,42,28,15,21] | $Q_{8,8,8,8,8,8,8,1}$ [13] | $Q_{8,8,8,8,8,8,8}$ [14] |
| 16 | [0,0,0,2,0,1,0,0,2,2] | [3,6,9,12,17,22,28,34,24,16,16] | $R_{10,10,10,6,6,4,1,1}$ [60] | |
| | [0,0,1,0,1,0,1,1,1,1] | [3,6,9,13,17,22,27,33,24,16,16] | $R_{10,10,10,7,5,3,2,1}$ [144] | |
| | [0,3,0,0,0,0,0,1,2,2] | [2,4,9,14,19,24,29,34,24,16,16] | $R_{10,10,8,8,8,2,1,1}$ [42] | |
| | [1,0,0,0,0,0,1,3,0,0] | [3,7,11,15,19,23,27,32,24,16,16] | $R_{10,10,10,9,3,2,2,2}$ [28] | |
| | [1,0,2,0,0,0,1,0,2,2] | [2,5,8,13,18,23,28,34,24,16,16] | $R_{10,10,9,7,7,3,1,1}$ [90] | |
| | [1,1,0,0,1,1,0,0,2,2] | [2,5,9,13,17,22,28,34,24,16,16] | $R_{10,10,9,8,5,4,1,1}$ [128] | |
| | [1,1,0,1,0,0,0,2,1,1] | [2,5,9,13,18,23,28,33,24,16,16] | $R_{10,10,9,8,6,2,2,1}$ [120] | |
| | [2,0,0,0,0,1,1,1,1,1] | [2,6,10,14,18,22,27,33,24,16,16] | $R_{10,10,9,9,4,3,2,1}$ [96] | |
| | [3,0,1,0,0,0,0,1,2,2] | [1,5,9,14,19,24,29,34,24,16,16] | $R_{10,9,9,9,7,2,1,1}$ [72] | |
| | [0,0,0,1,1,1,1,1,0,0] | [3,6,9,12,16,21,27,34,25,16,17] | $R_{10,10,10,6,5,4,3,2}$ [80] | |
| | [0,1,0,0,0,0,4,0,0,0] | [3,6,10,14,18,22,26,34,25,16,17] | $R_{10,10,10,8,3,3,3,3}$ [18] | |
| | [0,1,1,2,0,0,0,1,1,1] | [2,4,7,11,17,23,29,35,25,16,17] | $R_{10,10,8,7,6,6,2,1}$ [120] | |
| | [0,1,2,0,0,1,1,0,1,1] | [2,4,7,12,17,22,28,35,25,16,17] | $R_{10,10,8,7,7,4,3,1}$ [144] | |
| | [0,2,0,0,2,0,1,0,1,1] | [2,4,8,12,16,22,28,35,25,16,17] | $R_{10,10,8,8,5,5,3,1}$ [108] | |
| | [0,2,0,1,0,1,0,2,0,0] | [2,4,8,12,17,22,28,34,25,16,17] | $R_{10,10,8,8,6,4,2,2}$ [81] | |
| | [1,0,0,2,1,0,1,0,1,1] | [2,5,8,11,16,22,28,35,25,16,17] | $R_{10,10,9,6,6,5,3,1}$ [144] | |
| | [1,0,1,0,1,2,0,0,1,1] | [2,5,8,12,16,21,28,35,25,16,17] | $R_{10,10,9,7,5,4,4,1}$ [144] | |
| | [1,0,1,0,2,0,0,2,0,0] | [2,5,8,12,16,22,28,34,25,16,17] | $R_{10,10,9,7,5,5,2,2}$ [72] | |
| | [1,0,1,1,0,0,2,1,0,0] | [2,5,8,12,17,22,27,34,25,16,17] | $R_{10,10,9,7,6,3,3,2}$ [96] | |
| | [1,1,0,0,0,2,1,1,0,0] | [2,5,9,13,17,21,27,34,25,16,17] | $R_{10,10,9,8,4,4,3,2}$ [80] | |
| | [1,2,1,1,0,0,0,0,2,2] | [1,3,7,12,18,24,30,36,25,16,17] | $R_{10,9,8,8,7,6,1,1}$ [96] | |
| | [1,3,0,0,0,1,0,1,1,1] | [1,3,8,13,18,23,29,35,25,16,17] | $R_{10,9,8,8,8,4,2,1}$ [120] | |
| | [2,0,2,0,1,0,0,1,1,1] | [1,4,7,12,17,23,29,35,25,16,17] | $R_{10,9,9,7,7,5,2,1}$ [144] | |
| | [2,1,0,1,0,1,1,0,1,1] | [1,4,8,12,17,22,28,35,25,16,17] | $R_{10,9,9,8,6,4,3,1}$ [216] | |
| | [2,1,1,0,0,0,1,2,0,0] | [1,4,8,13,18,23,28,34,25,16,17] | $R_{10,9,9,8,7,3,2,2}$ [80] | |
| | [3,0,0,0,1,1,0,2,0,0] | [1,5,9,13,17,22,28,34,25,16,17] | $R_{10,9,9,9,5,4,2,2}$ [60] | |
| | [4,0,1,0,1,0,0,0,2,2] | [0,4,8,13,18,24,30,36,25,16,17] | $R_{9,9,9,9,7,5,1,1}$ [90] | |
| | [4,1,0,0,0,0,1,1,1,1] | [0,4,9,14,19,24,29,35,25,16,17] | $R_{9,9,9,9,8,3,2,1}$ [96] | |
| | [0,0,3,0,2,0,0,0,1,1] | [2,4,6,11,16,23,30,37,26,16,18] | $R_{10,10,7,7,7,5,5,1}$ [60] | |
| | [0,0,3,1,0,0,1,1,0,0] | [2,4,6,11,17,23,29,36,26,16,18] | $R_{10,10,7,7,7,6,3,2}$ [64] | |
| | [0,1,0,3,1,0,0,0,1,1] | [2,4,7,10,16,23,30,37,26,16,18] | $R_{10,10,8,6,6,6,5,1}$ [90] | |
| | [0,1,1,1,1,0,2,0,0,0] | [2,4,7,11,16,22,28,36,26,16,18] | $R_{10,10,8,7,6,5,3,3}$ [72] | |
| | [0,2,0,0,1,2,1,0,0,0] | [2,4,8,12,16,21,28,36,26,16,18] | $R_{10,10,8,8,5,4,4,3}$ [48] | |
| | [0,4,0,1,0,0,1,0,1,1] | [1,2,7,12,18,24,30,37,26,16,18] | $R_{10,8,8,8,8,6,3,1}$ [108] | |
| | [1,0,0,2,0,2,1,0,0,0] | [2,5,8,11,16,21,28,36,26,16,18] | $R_{10,10,9,6,6,4,4,3}$ [48] | |
| | [1,1,2,1,0,1,0,0,1,1] | [1,3,6,11,17,23,30,37,26,16,18] | $R_{10,9,8,7,7,6,4,1}$ [192] | |
| | [1,1,3,0,0,0,0,2,0,0] | [1,3,6,12,18,24,30,36,26,16,18] | $R_{10,9,8,7,7,7,2,2}$ [48] | |
| | [1,2,0,1,2,0,0,0,1,1] | [1,3,7,11,16,23,30,37,26,16,18] | $R_{10,9,8,8,6,5,5,1}$ [120] | |
| | [1,2,0,2,0,0,1,1,0,0] | [1,3,7,11,17,23,29,36,26,16,18] | $R_{10,9,8,8,6,6,3,2}$ [96] | |
| | [1,2,1,0,0,2,0,1,0,0] | [1,3,7,12,17,22,29,36,26,16,18] | $R_{10,9,8,8,7,4,4,2}$ [96] | |

| | | | | |
|---|---|---|---|---|
| | [2,0,1,1,1,1,0,1,0,0] | [1,4,7,11,16,22,29,36,26,16,18] | $R_{10,9,9,7,6,5,4,2}$ [144] | |
| | [2,0,2,0,0,1,2,0,0,0] | [1,4,7,12,17,22,28,36,26,16,18] | $R_{10,9,9,7,7,4,3,3}$ [48] | |
| | [2,1,0,0,2,0,2,0,0,0] | [1,4,8,12,16,22,28,36,26,16,18] | $R_{10,9,9,8,5,5,3,3}$ [48] | |
| | [2,3,1,0,0,0,0,1,1,1] | [0,2,7,13,19,25,31,37,26,16,18] | $R_{9,9,8,8,8,7,2,1}$ [96] | |
| | [3,0,0,0,0,3,1,0,0,0] | [1,5,9,13,17,21,28,36,26,16,18] | $R_{10,9,9,9,4,4,4,3}$ [24] | |
| | [3,1,1,0,1,1,0,0,1,1] | [0,3,7,12,17,23,30,37,26,16,18] | $R_{9,9,9,8,7,5,4,1}$ [192] | |
| | [3,1,1,1,0,0,0,2,0,0] | [0,3,7,12,18,24,30,36,26,16,18] | $R_{9,9,9,8,7,6,2,2}$ [80] | |
| | [3,2,0,0,0,1,1,1,0,0] | [0,3,8,13,18,23,29,36,26,16,18] | $R_{9,9,9,8,8,4,3,2}$ [80] | |
| | [4,0,0,1,1,0,1,1,0,0] | [0,4,8,12,17,23,29,36,26,16,18] | $R_{9,9,9,9,6,5,3,2}$ [96] | |
| | [0,0,2,2,1,0,1,0,0,0] | [2,4,6,10,16,23,30,38,27,16,19] | $R_{10,10,7,7,6,6,5,3}$ [48] | |
| | [0,0,3,0,1,2,0,0,0,0] | [2,4,6,11,16,22,30,38,27,16,19] | $R_{10,10,7,7,7,5,4,4}$ [24] | |
| | [0,1,0,3,0,2,0,0,0,0] | [2,4,7,10,16,22,30,38,27,16,19] | $R_{10,10,8,6,6,6,4,4}$ [27] | |
| | [0,3,1,1,1,0,0,1,0,0] | [1,2,6,11,17,24,31,38,27,16,19] | $R_{10,8,8,8,7,6,5,2}$ [96] | |
| | [0,3,2,0,0,0,2,0,0,0] | [1,2,6,12,18,24,30,38,27,16,19] | $R_{10,8,8,8,7,7,3,3}$ [30] | |
| | [0,4,0,0,1,1,1,0,0,0] | [1,2,7,12,17,23,30,38,27,16,19] | $R_{10,8,8,8,8,5,4,3}$ [48] | |
| | [1,0,4,1,0,0,0,0,1,1] | [1,3,5,11,18,25,32,39,27,16,19] | $R_{10,9,7,7,7,7,6,1}$ [72] | |
| | [1,1,1,3,0,0,0,1,0,0] | [1,3,6,10,17,24,31,38,27,16,19] | $R_{10,9,8,7,6,6,6,2}$ [80] | |
| | [1,1,2,0,2,0,1,0,0,0] | [1,3,6,11,16,23,30,38,27,16,19] | $R_{10,9,8,7,7,5,5,3}$ [72] | |
| | [1,2,0,1,1,2,0,0,0,0] | [1,3,7,11,16,22,30,38,27,16,19] | $R_{10,9,8,8,6,5,4,4}$ [48] | |
| | [2,0,0,3,1,0,1,0,0,0] | [1,4,7,10,16,23,30,38,27,16,19] | $R_{10,9,9,6,6,6,5,3}$ [48] | |
| | [2,2,1,2,0,0,0,0,1,1] | [0,2,6,11,18,25,32,39,27,16,19] | $R_{9,9,8,8,7,6,6,1}$ [96] | |
| | [2,2,2,0,0,1,0,1,0,0] | [0,2,6,12,18,24,31,38,27,16,19] | $R_{9,9,8,8,7,7,4,2}$ [96] | |
| | [2,3,0,0,2,0,0,1,0,0] | [0,2,7,12,17,24,31,38,27,16,19] | $R_{9,9,8,8,8,5,5,2}$ [64] | |
| | [2,3,0,1,0,0,2,0,0,0] | [0,2,7,12,18,24,30,38,27,16,19] | $R_{9,9,8,8,8,6,3,3}$ [48] | |
| | [3,0,2,1,1,0,0,1,0,0] | [0,3,6,11,17,24,31,38,27,16,19] | $R_{9,9,9,7,7,6,5,2}$ [96] | |
| | [3,0,3,0,0,0,2,0,0,0] | [0,3,6,12,18,24,30,38,27,16,19] | $R_{9,9,9,7,7,7,3,3}$ [30] | |
| | [3,1,0,2,0,1,1,0,0,0] | [0,3,7,11,17,23,30,38,27,16,19] | $R_{9,9,9,8,6,6,4,3}$ [72] | |
| | [4,0,0,0,3,0,1,0,0,0] | [0,4,8,12,16,23,30,38,27,16,19] | $R_{9,9,9,9,5,5,5,3}$ [30] | |
| | [4,0,0,1,0,3,0,0,0,0] | [0,4,8,12,17,22,30,38,27,16,19] | $R_{9,9,9,9,6,4,4,4}$ [24] | |
| | [0,2,3,1,0,0,1,0,0,0] | [1,2,5,11,18,25,32,40,28,16,20] | $R_{10,8,8,7,7,7,6,3}$ [48] | |
| | [1,0,4,0,1,1,0,0,0,0] | [1,3,5,11,17,24,32,40,28,16,20] | $R_{10,9,7,7,7,7,5,4}$ [36] | |
| | [1,1,1,2,2,0,0,0,0,0] | [1,3,6,10,16,24,32,40,28,16,20] | $R_{10,9,8,7,6,6,5,5}$ [32] | |
| | [1,4,1,1,0,0,0,1,0,0] | [0,1,6,12,19,26,33,40,28,16,20] | $R_{9,8,8,8,8,7,6,2}$ [80] | |
| | [1,5,0,0,0,1,1,0,0,0] | [0,1,7,13,19,25,32,40,28,16,20] | $R_{9,8,8,8,8,8,4,3}$ [40] | |
| | [2,1,4,0,0,0,0,1,0,0] | [0,2,5,12,19,26,33,40,28,16,20] | $R_{9,9,8,7,7,7,7,2}$ [48] | |
| | [2,2,1,1,1,1,0,0,0,0] | [0,2,6,11,17,24,32,40,28,16,20] | $R_{9,9,8,8,7,6,5,4}$ [64] | |
| | [3,1,0,1,3,0,0,0,0,0] | [0,3,7,11,16,24,32,40,28,16,20] | $R_{9,9,9,8,6,5,5,5}$ [24] | |
| | [0,3,0,4,0,0,0,0,0,0] | [1,2,6,10,18,26,34,42,29,16,21] | $R_{10,8,8,8,6,6,6,6}$ [9] | |
| | [1,4,1,0,2,0,0,0,0,0] | [0,1,6,12,18,26,34,42,29,16,21] | $R_{9,8,8,8,8,7,5,5}$ [24] | |
| | [2,1,3,1,1,0,0,0,0,0] | [0,2,5,11,18,26,34,42,29,16,21] | $R_{9,9,8,7,7,7,6,5}$ [32] | |
| | [3,0,1,4,0,0,0,0,0,0] | [0,3,6,10,18,26,34,42,29,16,21] | $R_{9,9,9,7,6,6,6,6}$ [12] | |
| | [1,3,3,1,0,0,0,0,0,0] | [0,1,5,12,20,28,36,44,30,16,22] | $R_{9,8,8,8,7,7,7,6}$ [16] | |
| | [0,7,0,1,0,0,0,0,0,0] | [0,0,7,14,22,30,38,46,31,16,23] | $R_{8,8,8,8,8,8,8,6}$ [9] | |
| | [0,0,0,0,0,0,0,3,2,0] | [4,8,12,16,20,24,28,32,23,16,16] | $R_{10,10,10,10,2,2,2,1,1}$ [13] | $R_{10,10,10,10,2,2,2}$ [14] |
| | [0,0,2,0,0,0,0,0,4,2] | [3,6,9,14,19,24,29,34,23,16,16] | $R_{10,10,10,7,7,1,1,1,1}$ [28] | $R_{10,10,10,7,7,1,1}$ [28] |
| | [0,1,0,0,1,0,0,1,3,1] | [3,6,10,14,18,23,28,33,23,16,16] | $R_{10,10,10,8,5,2,1,1,1}$ [96] | $R_{10,10,10,8,5,2,1}$ [96] |
| | [1,0,0,0,0,0,2,0,3,1] | [3,7,11,15,19,23,27,33,23,16,16] | $R_{10,10,10,9,3,3,1,1,1}$ [42] | $R_{10,10,10,9,3,3,1}$ [42] |
| | [2,0,0,1,0,0,0,0,4,2] | [2,6,10,14,19,24,29,34,23,16,16] | $R_{10,10,9,9,6,1,1,1,1}$ [48] | $R_{10,10,9,9,6,1,1}$ [48] |
| | [0,0,0,1,2,0,0,1,0,2] | [3,6,9,12,16,22,28,34,25,16,16] | $R_{10,10,10,6,5,5,2}$ [60] | $R_{10,10,10,6,5,5,2,1,1}$ [60] |
| | [0,0,0,2,0,0,2,0,0,2] | [3,6,9,12,17,22,27,34,25,16,16] | $R_{10,10,10,6,6,3,3}$ [40] | $R_{10,10,10,6,6,3,3,1,1}$ [40] |
| | [0,0,1,0,0,2,1,0,0,2] | [3,6,9,13,17,21,27,34,25,16,16] | $R_{10,10,10,7,4,4,3}$ [64] | $R_{10,10,10,7,4,4,3,1,1}$ [64] |
| | [0,2,0,1,1,0,0,0,1,3] | [2,4,8,12,17,23,29,35,25,16,16] | $R_{10,10,8,8,6,5,1}$ [90] | $R_{10,10,8,8,6,5,1,1,1}$ [90] |
| | [0,2,1,0,0,0,1,1,0,2] | [2,4,8,13,18,23,28,34,25,16,16] | $R_{10,10,8,8,7,3,2}$ [90] | $R_{10,10,8,8,7,3,2,1,1}$ [90] |
| | [1,0,1,1,0,1,0,1,0,2] | [2,5,8,12,17,22,28,34,25,16,16] | $R_{10,10,9,7,6,4,2}$ [162] | $R_{10,10,9,7,6,4,2,1,1}$ [162] |
| | [1,1,0,0,1,0,2,0,0,2] | [2,5,9,13,17,22,27,34,25,16,16] | $R_{10,10,9,8,5,3,3}$ [96] | $R_{10,10,9,8,5,3,3,1,1}$ [96] |
| | [2,1,1,0,0,1,0,0,1,3] | [1,4,8,13,18,23,29,35,25,16,16] | $R_{10,9,9,8,7,4,1}$ [128] | $R_{10,9,9,8,7,4,1,1,1}$ [128] |
| | [2,2,0,0,0,0,0,2,0,2] | [1,4,9,14,19,24,29,34,25,16,16] | $R_{10,9,9,8,8,2,2}$ [42] | $R_{10,9,9,8,8,2,2,1,1}$ [42] |
| | [3,0,0,0,2,0,0,0,1,3] | [1,5,9,13,17,23,29,35,25,16,16] | $R_{10,9,9,9,5,5,1}$ [50] | $R_{10,9,9,9,5,5,1,1,1}$ [50] |
| | [3,0,0,1,0,0,1,1,0,2] | [1,5,9,13,18,23,28,34,25,16,16] | $R_{10,9,9,9,6,3,2}$ [96] | $R_{10,9,9,9,6,3,2,1,1}$ [96] |
| | [0,1,2,1,0,0,0,0,0,4] | [2,4,7,12,18,24,30,36,26,16,16] | $R_{10,10,8,7,7,6}$ [42] | $R_{10,10,8,7,7,6,1,1,1,1}$ [42] |
| | [2,1,0,2,0,0,0,0,0,4] | [1,4,8,12,18,24,30,36,26,16,16] | $R_{10,9,9,8,6,6}$ [42] | $R_{10,9,9,8,6,6,1,1,1,1}$ [42] |
| | [5,0,0,0,0,0,1,0,0,4] | [0,5,10,15,20,25,30,36,26,16,16] | $R_{9,9,9,9,9,3}$ [28] | $R_{9,9,9,9,9,3,1,1,1,1}$ [28] |
| | [0,0,1,1,0,0,1,0,4,0] | [3,6,9,13,18,23,28,34,23,16,17] | $R_{10,10,10,7,6,3,1,1,1,1}$ [64] | $R_{10,10,10,7,6,3}$ [64] |
| | [0,1,0,0,0,2,0,0,4,0] | [3,6,10,14,18,22,28,34,23,16,17] | $R_{10,10,10,8,4,4,1,1,1,1}$ [37] | $R_{10,10,10,8,4,4}$ [38] |
| | [1,1,1,0,0,0,0,1,4,0] | [2,5,9,14,19,24,29,34,23,16,17] | $R_{10,10,9,8,7,2,1,1,1,1}$ [72] | $R_{10,10,9,8,7,2}$ [72] |
| | [2,0,0,0,1,0,1,0,4,0] | [2,6,10,14,18,23,28,34,23,16,17] | $R_{10,10,9,9,5,3,1,1,1,1}$ [60] | $R_{10,10,9,9,5,3}$ [60] |
| | [0,0,0,1,2,0,0,1,2,0] | [3,6,9,12,16,22,28,34,24,16,17] | $R_{10,10,10,6,5,5,2,1,1}$ [60] | $R_{10,10,10,6,5,5,2}$ [60] |
| | [0,0,1,0,0,2,1,0,2,0] | [3,6,9,13,17,21,27,34,24,16,17] | $R_{10,10,10,7,4,4,3,1,1}$ [64] | $R_{10,10,10,7,4,4,3}$ [64] |
| | [0,2,0,1,1,0,0,0,3,1] | [2,4,8,12,17,23,29,35,24,16,17] | $R_{10,10,8,8,6,5,1,1,1}$ [90] | $R_{10,10,8,8,6,5,1}$ [90] |
| | [0,2,1,0,0,0,1,1,2,0] | [2,4,8,13,18,23,28,34,24,16,17] | $R_{10,10,8,8,7,3,2,1,1}$ [90] | $R_{10,10,8,8,7,3,2}$ [90] |
| | [1,0,1,1,0,1,0,1,2,0] | [2,5,8,12,17,22,28,34,24,16,17] | $R_{10,10,9,7,6,4,2,1,1}$ [162] | $R_{10,10,9,7,6,4,2}$ [162] |

| | | | | |
|---|---|---|---|---|
| | [1,1,0,0,1,0,2,0,2,0] | [2,5,9,13,17,22,27,34,24,16,17] | $R_{10,10,9,8,5,3,3,1,1}$ [96] | $R_{10,10,9,8,5,3,3}$ [96] |
| | [2,1,1,0,0,1,0,0,3,1] | [1,4,8,13,18,23,29,35,24,16,17] | $R_{10,9,9,8,7,4,1,1,1}$ [128] | $R_{10,9,9,8,7,4,1}$ [128] |
| | [3,0,0,0,2,0,0,0,3,1] | [1,5,9,13,17,23,29,35,24,16,17] | $R_{10,9,9,9,5,5,1,1,1}$ [50] | $R_{10,9,9,9,5,5,1}$ [50] |
| | [3,0,0,1,0,0,1,1,2,0] | [1,5,9,13,18,23,28,34,24,16,17] | $R_{10,9,9,9,6,3,2,1,1}$ [96] | $R_{10,9,9,9,6,3,2}$ [96] |
| | [0,0,4,0,0,0,0,1,0,2] | [2,4,6,12,18,24,30,36,26,16,17] | $R_{10,10,7,7,7,7,2}$ [36] | $R_{10,10,7,7,7,7,2,1,1}$ [36] |
| | [0,1,1,1,1,1,0,0,0,2] | [2,4,7,11,16,22,29,36,26,16,17] | $R_{10,10,8,7,6,5,4}$ [120] | $R_{10,10,8,7,6,5,4,1,1}$ [120] |
| | [1,2,1,0,1,0,1,0,0,2] | [1,3,7,12,17,23,29,36,26,16,17] | $R_{10,9,8,8,7,5,3}$ [144] | $R_{10,9,8,8,7,5,3,1,1}$ [144] |
| | [2,0,1,2,0,0,1,0,0,2] | [1,4,7,11,17,23,29,36,26,16,17] | $R_{10,9,9,7,6,6,3}$ [96] | $R_{10,9,9,7,6,6,3,1,1}$ [96] |
| | [2,1,0,0,2,1,0,0,0,2] | [1,4,8,12,16,22,29,36,26,16,17] | $R_{10,9,9,8,5,5,4}$ [80] | $R_{10,9,9,8,5,5,4,1,1}$ [80] |
| | [3,1,2,0,0,0,0,0,1,3] | [0,3,7,13,19,25,31,37,26,16,17] | $R_{9,9,9,8,7,7,1}$ [56] | $R_{9,9,9,8,7,7,1,1,1}$ [56] |
| | [3,2,0,0,1,0,0,1,0,2] | [0,3,8,13,18,24,30,36,26,16,17] | $R_{9,9,9,8,8,5,2}$ [96] | $R_{9,9,9,8,8,5,2,1,1}$ [96] |
| | [4,0,0,2,0,0,0,1,0,2] | [0,4,8,12,18,24,30,36,26,16,17] | $R_{9,9,9,9,6,6,2}$ [60] | $R_{9,9,9,9,6,6,2,1,1}$ [60] |
| | [4,0,1,0,0,1,1,0,0,2] | [0,4,8,13,18,23,29,36,26,16,17] | $R_{9,9,9,9,7,4,3}$ [96] | $R_{9,9,9,9,7,4,3,1,1}$ [96] |
| | [0,5,0,0,0,0,0,0,0,4] | [1,2,8,14,20,26,32,38,27,16,17] | $R_{10,8,8,8,8,8}$ [14] | $R_{10,8,8,8,8,8,1,1,1,1}$ [13] |
| | [2,1,0,2,0,0,0,0,4,0] | [1,4,8,12,18,24,30,36,24,16,18] | $R_{10,9,9,8,6,6,1,1,1,1}$ [42] | $R_{10,9,9,8,6,6}$ [42] |
| | [5,0,0,0,0,0,1,0,4,0] | [0,5,10,15,20,25,30,36,24,16,18] | $R_{9,9,9,9,9,3,1,1,1,1}$ [28] | $R_{9,9,9,9,9,3}$ [28] |
| | [0,1,1,1,1,1,0,0,2,0] | [2,4,7,11,16,22,29,36,25,16,18] | $R_{10,10,8,7,6,5,4,1,1}$ [120] | $R_{10,10,8,7,6,5,4}$ [120] |
| | [1,2,1,0,1,0,1,0,2,0] | [1,3,7,12,17,23,29,36,25,16,18] | $R_{10,9,8,8,7,5,3,1,1}$ [144] | $R_{10,9,8,8,7,5,3}$ [144] |
| | [2,0,1,2,0,0,1,0,2,0] | [1,4,7,11,17,23,29,36,25,16,18] | $R_{10,9,9,7,6,6,3,1,1}$ [96] | $R_{10,9,9,7,6,6,3}$ [96] |
| | [2,0,2,0,0,2,0,0,2,0] | [1,4,7,12,17,22,29,36,25,16,18] | $R_{10,9,9,7,7,4,4,1,1}$ [60] | $R_{10,9,9,7,7,4,4}$ [60] |
| | [2,1,0,0,2,1,0,0,2,0] | [1,4,8,12,16,22,29,36,25,16,18] | $R_{10,9,9,8,5,5,4,1,1}$ [80] | $R_{10,9,9,8,5,5,4}$ [80] |
| | [3,1,2,0,0,0,0,0,3,1] | [0,3,7,13,19,25,31,37,25,16,18] | $R_{9,9,9,8,7,7,1,1,1}$ [56] | $R_{9,9,9,8,7,7,1}$ [56] |
| | [3,2,0,0,1,0,0,1,2,0] | [0,3,8,13,18,24,30,36,25,16,18] | $R_{9,9,9,8,8,5,2,1,1}$ [96] | $R_{9,9,9,8,8,5,2}$ [96] |
| | [4,0,0,2,0,0,0,1,2,0] | [0,4,8,12,18,24,30,36,25,16,18] | $R_{9,9,9,9,6,6,2,1,1}$ [60] | $R_{9,9,9,9,6,6,2}$ [60] |
| | [4,0,1,0,0,1,1,0,2,0] | [0,4,8,13,18,23,29,36,25,16,18] | $R_{9,9,9,9,7,4,3,1,1}$ [96] | $R_{9,9,9,9,7,4,3}$ [96] |
| | [0,0,2,3,0,0,0,0,0,2] | [2,4,6,10,17,24,31,38,27,16,18] | $R_{10,10,7,7,6,6,6}$ [28] | $R_{10,10,7,7,6,6,6,1,1}$ [28] |
| | [0,3,2,0,0,1,0,0,0,2] | [1,2,6,12,18,24,31,38,27,16,18] | $R_{10,8,8,8,7,7,4}$ [60] | $R_{10,8,8,8,7,7,4,1,1}$ [60] |
| | [0,4,0,0,2,0,0,0,0,2] | [1,2,7,12,17,24,31,38,27,16,18] | $R_{10,8,8,8,8,5,5}$ [36] | $R_{10,8,8,8,8,5,5,1,1}$ [36] |
| | [2,0,0,4,0,0,0,0,0,2] | [1,4,7,10,17,24,31,38,27,16,18] | $R_{10,9,9,6,6,6,6}$ [28] | $R_{10,9,9,6,6,6,6,1,1}$ [28] |
| | [2,3,0,1,0,1,0,0,0,2] | [0,2,7,12,18,24,31,38,27,16,18] | $R_{9,9,8,8,8,6,4}$ [90] | $R_{9,9,8,8,8,6,4,1,1}$ [90] |
| | [3,0,3,0,0,1,0,0,0,2] | [0,3,6,12,18,24,31,38,27,16,18] | $R_{9,9,9,7,7,7,4}$ [60] | $R_{9,9,9,7,7,7,4,1,1}$ [60] |
| | [3,1,0,2,1,0,0,0,0,2] | [0,3,7,11,17,24,31,38,27,16,18] | $R_{9,9,9,8,6,6,5}$ [72] | $R_{9,9,9,8,6,6,5,1,1}$ [72] |
| | [0,5,0,0,0,0,0,0,4,0] | [1,2,8,14,20,26,32,38,25,16,19] | $R_{10,8,8,8,8,8,1,1,1,1}$ [13] | $R_{10,8,8,8,8,8}$ [14] |
| | [0,0,2,3,0,0,0,0,2,0] | [2,4,6,10,17,24,31,38,26,16,19] | $R_{10,10,7,7,6,6,6,1,1}$ [28] | $R_{10,10,7,7,6,6,6}$ [28] |
| | [0,3,2,0,0,1,0,0,2,0] | [1,2,6,12,18,24,31,38,26,16,19] | $R_{10,8,8,8,7,7,4,1,1}$ [60] | $R_{10,8,8,8,7,7,4}$ [60] |
| | [2,3,0,1,0,1,0,0,2,0] | [0,2,7,12,18,24,31,38,26,16,19] | $R_{9,9,8,8,8,6,4,1,1}$ [90] | $R_{9,9,8,8,8,6,4}$ [90] |
| | [3,0,3,0,0,1,0,0,2,0] | [0,3,6,12,18,24,31,38,26,16,19] | $R_{9,9,9,7,7,7,4,1,1}$ [60] | $R_{9,9,9,7,7,7,4}$ [60] |
| | [3,1,0,2,1,0,0,0,2,0] | [0,3,7,11,17,24,31,38,26,16,19] | $R_{9,9,9,8,6,6,5,1,1}$ [72] | $R_{9,9,9,8,6,6,5}$ [72] |
| | [1,5,0,0,1,0,0,0,0,2] | [0,1,7,13,19,26,33,40,28,16,19] | $R_{9,8,8,8,8,8,5}$ [48] | $R_{9,8,8,8,8,8,5,1,1}$ [48] |
| | [0,2,4,0,0,0,0,0,2,0] | [1,2,5,12,19,26,33,40,27,16,20] | $R_{10,8,8,7,7,7,7,1,1}$ [24] | $R_{10,8,8,7,7,7,7}$ [24] |
| | [1,5,0,0,1,0,0,0,2,0] | [0,1,7,13,19,26,33,40,27,16,20] | $R_{9,8,8,8,8,8,5,1,1}$ [48] | $R_{9,8,8,8,8,8,5}$ [48] |
| 17 | [0,0,0,0,1,0,0,1,4,1] | [4,8,12,16,20,25,30,35,24,17,17] | $S_{10,10,10,10,5,2,1,1,1,1}$ [48] | $S_{10,10,10,10,5,2,1}$ [48] |
| | [1,0,1,0,0,0,0,0,5,2] | [3,7,11,16,21,26,31,36,24,17,17] | $S_{10,10,10,9,7,1,1,1,1,1}$ [42] | $S_{10,10,10,9,7,1,1}$ [42] |
| | [0,0,0,0,0,0,3,0,2,1] | [4,8,12,16,20,24,28,35,25,17,17] | $S_{10,10,10,10,3,3,3,1,1}$ [24] | $S_{10,10,10,10,3,3,3,1}$ [24] |
| | [0,0,0,0,0,1,0,3,1,0] | [4,8,12,16,20,24,29,34,25,17,17] | $S_{10,10,10,10,4,2,2,2,1}$ [31] | $S_{10,10,10,10,4,2,2,2}$ [32] |
| | [0,0,2,0,0,1,0,0,3,2] | [3,6,9,14,19,24,30,36,25,17,17] | $S_{10,10,10,7,7,4,1,1,1}$ [64] | $S_{10,10,10,7,7,4,1,1}$ [64] |
| | [0,1,0,0,2,0,0,0,3,2] | [3,6,10,14,18,24,30,36,25,17,17] | $S_{10,10,10,8,5,5,1,1,1}$ [60] | $S_{10,10,10,8,5,5,1,1}$ [60] |
| | [0,1,0,1,0,0,1,1,2,1] | [3,6,10,14,19,24,29,35,25,17,17] | $S_{10,10,10,8,6,3,2,1,1}$ [144] | $S_{10,10,10,8,6,3,2,1}$ [144] |
| | [1,0,0,0,0,2,0,1,2,1] | [3,7,11,15,19,23,29,35,25,17,17] | $S_{10,10,10,9,4,4,2,1,1}$ [72] | $S_{10,10,10,9,4,4,2,1}$ [72] |
| | [1,2,0,0,0,0,1,0,3,2] | [2,5,10,15,20,25,30,36,25,17,17] | $S_{10,10,9,8,8,3,1,1,1}$ [72] | $S_{10,10,9,8,8,3,1,1}$ [72] |
| | [2,0,0,1,0,1,0,0,3,2] | [2,6,10,14,19,24,30,36,25,17,17] | $S_{10,10,9,9,6,4,1,1,1}$ [96] | $S_{10,10,9,9,6,4,1,1}$ [96] |
| | [2,0,1,0,0,0,0,2,2,1] | [2,6,10,15,20,25,30,35,25,17,17] | $S_{10,10,9,9,7,2,2,1,1}$ [72] | $S_{10,10,9,9,7,2,2,1}$ [72] |
| | [0,0,1,1,0,1,1,0,1,2] | [3,6,9,13,18,23,29,36,26,17,17] | $S_{10,10,10,7,6,4,3,1}$ [144] | $S_{10,10,10,7,6,4,3,1,1}$ [144] |
| | [0,0,2,0,0,0,1,2,0,1] | [3,6,9,14,19,24,29,35,26,17,17] | $S_{10,10,10,7,7,3,2,2}$ [60] | $S_{10,10,10,7,7,3,2,2,1}$ [60] |
| | [0,1,0,0,1,1,0,2,0,1] | [3,6,10,14,18,23,29,35,26,17,17] | $S_{10,10,10,8,5,4,2,2}$ [108] | $S_{10,10,10,8,5,4,2,2,1}$ [108] |
| | [0,3,0,0,1,0,0,0,2,3] | [2,4,9,14,19,25,31,37,26,17,17] | $S_{10,10,8,8,8,5,1,1}$ [60] | $S_{10,10,8,8,8,5,1,1,1}$ [60] |
| | [1,0,0,0,0,1,2,1,0,1] | [3,7,11,15,19,23,28,35,26,17,17] | $S_{10,10,10,9,4,3,3,2}$ [72] | $S_{10,10,10,9,4,3,3,2,1}$ [72] |
| | [1,0,2,1,0,0,0,0,2,3] | [2,5,8,13,19,25,31,37,26,17,17] | $S_{10,10,9,7,7,6,1,1}$ [72] | $S_{10,10,9,7,7,6,1,1,1}$ [72] |
| | [1,1,0,1,1,0,0,1,1,2] | [2,5,9,13,18,24,30,36,26,17,17] | $S_{10,10,9,8,6,5,2,1}$ [192] | $S_{10,10,9,8,6,5,2,1,1}$ [192] |
| | [1,1,1,0,0,0,2,0,1,2] | [2,5,9,14,19,24,29,36,26,17,17] | $S_{10,10,9,8,7,3,3,1}$ [120] | $S_{10,10,9,8,7,3,3,1,1}$ [120] |
| | [1,2,0,0,0,0,0,3,0,1] | [2,5,10,15,20,25,30,35,26,17,17] | $S_{10,10,9,8,8,2,2,2}$ [42] | $S_{10,10,9,8,8,2,2,2,1}$ [42] |
| | [2,0,0,0,1,1,1,0,1,2] | [2,6,10,14,18,23,29,36,26,17,17] | $S_{10,10,9,9,5,4,3,1}$ [120] | $S_{10,10,9,9,5,4,3,1,1}$ [120] |
| | [2,0,0,1,0,0,1,2,0,1] | [2,6,10,14,19,24,29,35,26,17,17] | $S_{10,10,9,9,6,3,2,2}$ [96] | $S_{10,10,9,9,6,3,2,2,1}$ [96] |
| | [3,0,1,0,1,0,0,0,2,3] | [1,5,9,14,19,25,31,37,26,17,17] | $S_{10,9,9,9,7,5,1,1}$ [90] | $S_{10,9,9,9,7,5,1,1,1}$ [90] |
| | [3,1,0,0,0,0,1,1,1,2] | [1,5,10,15,20,25,30,36,26,17,17] | $S_{10,9,9,9,8,3,2,1}$ [96] | $S_{10,9,9,9,8,3,2,1,1}$ [96] |
| | [0,0,0,3,0,0,1,0,0,3] | [3,6,9,12,18,24,30,37,27,17,17] | $S_{10,10,10,6,6,6,3}$ [40] | $S_{10,10,10,6,6,6,3,1,1,1}$ [40] |
| | [0,0,1,0,2,1,0,0,0,3] | [3,6,9,13,17,23,30,37,27,17,17] | $S_{10,10,10,7,5,5,4}$ [60] | $S_{10,10,10,7,5,5,4,1,1,1}$ [60] |
| | [0,2,1,1,0,0,0,1,0,3] | [2,4,8,13,19,25,31,37,27,17,17] | $S_{10,10,8,8,7,6,2}$ [90] | $S_{10,10,8,8,7,6,2,1,1,1}$ [90] |
| | [0,3,0,0,0,1,1,0,0,3] | [2,4,9,14,19,24,30,37,27,17,17] | $S_{10,10,8,8,8,4,3}$ [60] | $S_{10,10,8,8,8,4,3,1,1,1}$ [60] |
| | [1,0,2,0,1,0,1,0,0,3] | [2,5,8,13,18,24,30,37,27,17,17] | $S_{10,10,9,7,7,5,3}$ [108] | $S_{10,10,9,7,7,5,3,1,1,1}$ [108] |
| | [1,1,0,1,0,2,0,0,0,3] | [2,5,9,13,18,23,30,37,27,17,17] | $S_{10,10,9,8,6,4,4}$ [90] | $S_{10,10,9,8,6,4,4,1,1,1}$ [90] |

| | | | | |
|---|---|---|---|---|
| | [2,1,2,0,0,0,0,0,1,4] | [1,4,8,14,20,26,32,38,27,17,17] | $S_{10,9,9,8,7,7,1}$ [56] | $S_{10,9,9,8,7,7,1,1,1,1}$ [56] |
| | [2,2,0,0,1,0,0,1,0,3] | [1,4,9,14,19,25,31,37,27,17,17] | $S_{10,9,9,8,8,5,2}$ [96] | $S_{10,9,9,8,8,5,2,1,1,1}$ [96] |
| | [3,0,0,2,0,0,0,1,0,3] | [1,5,9,13,19,25,31,37,27,17,17] | $S_{10,9,9,9,6,6,2}$ [60] | $S_{10,9,9,9,6,6,2,1,1,1}$ [60] |
| | [3,0,1,0,0,1,1,0,0,3] | [1,5,9,14,19,24,30,37,27,17,17] | $S_{10,9,9,9,7,4,3}$ [96] | $S_{10,9,9,9,7,4,3,1,1,1}$ [96] |
| | [5,0,0,1,0,0,0,0,0,5] | [0,5,10,15,21,27,33,39,28,17,17] | $S_{9,9,9,9,9,6}$ [28] | $S_{9,9,9,9,9,6,1,1,1,1,1}$ [28] |
| | [0,0,0,0,0,2,0,0,5,0] | [4,8,12,16,20,24,30,36,24,17,18] | $S_{10,10,10,10,4,4,1,1,1,1,1,1}$ [17] | $S_{10,10,10,10,4,4}$ [18] |
| | [0,2,0,0,0,0,0,1,5,0] | [3,6,11,16,21,26,31,36,24,17,18] | $S_{10,10,10,8,8,2,1,1,1,1,1}$ [31] | $S_{10,10,10,8,8,2}$ [32] |
| | [1,0,0,1,0,0,1,0,5,0] | [3,7,11,15,20,25,30,36,24,17,18] | $S_{10,10,10,9,6,3,1,1,1,1,1}$ [64] | $S_{10,10,10,9,6,3}$ [64] |
| | [0,0,1,1,1,0,0,1,3,0] | [3,6,9,13,18,24,30,36,25,17,18] | $S_{10,10,10,7,6,5,2,1,1,1}$ [96] | $S_{10,10,10,7,6,5,2}$ [96] |
| | [0,0,2,0,0,0,2,0,3,0] | [3,6,9,14,19,24,29,36,25,17,18] | $S_{10,10,10,7,7,3,3,1,1,1}$ [40] | $S_{10,10,10,7,7,3,3}$ [40] |
| | [0,1,0,0,1,1,1,0,3,0] | [3,6,10,14,18,23,29,36,25,17,18] | $S_{10,10,10,8,5,4,3,1,1,1}$ [96] | $S_{10,10,10,8,5,4,3}$ [96] |
| | [1,1,0,2,0,0,0,0,4,1] | [2,5,9,13,19,25,31,37,25,17,18] | $S_{10,10,9,8,6,6,1,1,1,1}$ [72] | $S_{10,10,9,8,6,6,1}$ [72] |
| | [1,1,1,0,0,1,0,1,3,0] | [2,5,9,14,19,24,30,36,25,17,18] | $S_{10,10,9,8,7,4,2,1,1,1}$ [144] | $S_{10,10,9,8,7,4,2}$ [144] |
| | [2,0,0,0,2,0,0,1,3,0] | [2,6,10,14,18,24,30,36,25,17,18] | $S_{10,10,9,9,5,5,2,1,1,1}$ [60] | $S_{10,10,9,9,5,5,2}$ [60] |
| | [2,0,0,1,0,0,2,0,3,0] | [2,6,10,14,19,24,29,36,25,17,18] | $S_{10,10,9,9,6,3,3,1,1,1}$ [64] | $S_{10,10,9,9,6,3,3}$ [64] |
| | [3,1,0,0,0,1,0,0,4,1] | [1,5,10,15,20,25,31,37,25,17,18] | $S_{10,9,9,9,8,4,1,1,1,1}$ [80] | $S_{10,9,9,9,8,4,1}$ [80] |
| | [4,0,0,0,0,0,0,2,3,0] | [1,6,11,16,21,26,31,36,25,17,18] | $S_{10,9,9,9,9,2,2,1,1,1}$ [24] | $S_{10,9,9,9,9,2,2}$ [24] |
| | [0,0,0,2,1,1,0,0,2,1] | [3,6,9,12,17,23,30,37,26,17,18] | $S_{10,10,10,6,6,5,4,1,1}$ [80] | $S_{10,10,10,6,6,5,4,1}$ [80] |
| | [0,0,0,3,0,0,0,2,1,0] | [3,6,9,12,18,24,30,36,26,17,18] | $S_{10,10,10,6,6,6,2,2,1}$ [37] | $S_{10,10,10,6,6,6,2,2}$ [38] |
| | [0,0,1,0,2,0,1,1,1,0] | [3,6,9,13,17,23,29,36,26,17,18] | $S_{10,10,10,7,5,5,3,2,1}$ [108] | $S_{10,10,10,7,5,5,3,2}$ [108] |
| | [0,1,0,0,0,3,0,1,1,0] | [3,6,10,14,18,22,29,36,26,17,18] | $S_{10,10,10,8,4,4,4,2,1}$ [67] | $S_{10,10,10,8,4,4,4,2}$ [68] |
| | [0,1,0,0,1,0,3,0,1,0] | [3,6,10,14,18,23,28,36,26,17,18] | $S_{10,10,10,8,5,3,3,3,1}$ [72] | $S_{10,10,10,8,5,3,3,3}$ [72] |
| | [0,2,1,0,1,0,1,0,2,1] | [2,4,8,13,18,24,30,37,26,17,18] | $S_{10,10,8,8,7,5,3,1,1}$ [162] | $S_{10,10,8,8,7,5,3,1}$ [162] |
| | [0,3,0,0,0,1,0,2,1,0] | [2,4,9,14,19,24,30,36,26,17,18] | $S_{10,10,8,8,8,4,2,2,1}$ [67] | $S_{10,10,8,8,8,4,2,2}$ [68] |
| | [1,0,1,2,0,0,1,0,2,1] | [2,5,8,12,18,24,30,37,26,17,18] | $S_{10,10,9,7,6,6,3,1,1}$ [144] | $S_{10,10,9,7,6,6,3,1}$ [144] |
| | [1,0,2,0,0,2,0,0,2,1] | [2,5,8,13,18,23,30,37,26,17,18] | $S_{10,10,9,7,7,4,4,1,1}$ [96] | $S_{10,10,9,7,7,4,4,1}$ [96] |
| | [1,0,2,0,1,0,0,2,1,0] | [2,5,8,13,18,24,30,36,26,17,18] | $S_{10,10,9,7,7,5,2,2,1}$ [108] | $S_{10,10,9,7,7,5,2,2}$ [108] |
| | [1,1,0,0,2,1,0,0,2,1] | [2,5,9,13,17,23,30,37,26,17,18] | $S_{10,10,9,8,5,5,4,1,1}$ [128] | $S_{10,10,9,8,5,5,4,1}$ [128] |
| | [1,1,0,1,0,1,1,1,1,0] | [2,5,9,13,18,23,29,36,26,17,18] | $S_{10,10,9,8,6,4,3,2,1}$ [216] | $S_{10,10,9,8,6,4,3,2}$ [216] |
| | [2,1,1,1,0,0,0,1,2,1] | [1,4,8,13,19,25,31,37,26,17,18] | $S_{10,9,9,8,7,6,2,1,1}$ [160] | $S_{10,9,9,8,7,6,2,1}$ [160] |
| | [2,2,0,0,0,1,1,0,2,1] | [1,4,9,14,19,24,30,37,26,17,18] | $S_{10,9,9,8,8,4,3,1,1}$ [120] | $S_{10,9,9,8,8,4,3,1}$ [120] |
| | [3,0,0,1,1,0,1,0,2,1] | [1,5,9,13,18,24,30,37,26,17,18] | $S_{10,9,9,9,6,5,3,1,1}$ [144] | $S_{10,9,9,9,6,5,3,1}$ [144] |
| | [3,0,1,0,0,1,0,2,1,0] | [1,5,9,14,19,24,30,36,26,17,18] | $S_{10,9,9,9,7,4,2,2,1}$ [108] | $S_{10,9,9,9,7,4,2,2}$ [108] |
| | [5,0,0,0,1,0,0,0,3,2] | [0,5,10,15,20,26,32,38,26,17,18] | $S_{9,9,9,9,9,5,1,1,1}$ [50] | $S_{9,9,9,9,9,5,1,1}$ [50] |
| | [0,0,0,2,1,0,2,0,0,1] | [3,6,9,12,17,23,29,37,27,17,18] | $S_{10,10,10,6,6,5,3,3}$ [60] | $S_{10,10,10,6,6,5,3,3,1}$ [60] |
| | [0,0,1,0,1,2,1,0,0,1] | [3,6,9,13,17,22,29,37,27,17,18] | $S_{10,10,10,7,5,4,4,3}$ [96] | $S_{10,10,10,7,5,4,4,3,1}$ [96] |
| | [0,1,2,1,0,1,0,0,1,2] | [2,4,7,12,18,24,31,38,27,17,18] | $S_{10,10,8,7,7,6,4,1}$ [144] | $S_{10,10,8,7,7,6,4,1,1}$ [144] |
| | [0,1,3,0,0,0,0,2,0,1] | [2,4,7,13,19,25,31,37,27,17,18] | $S_{10,10,8,7,7,7,2,2}$ [54] | $S_{10,10,8,7,7,7,2,2,1}$ [54] |
| | [0,2,0,1,2,0,0,0,1,2] | [2,4,8,12,17,24,31,38,27,17,18] | $S_{10,10,8,8,6,5,5,1}$ [90] | $S_{10,10,8,8,6,5,5,1,1}$ [90] |
| | [0,2,0,2,0,0,1,1,0,1] | [2,4,8,12,18,24,30,37,27,17,18] | $S_{10,10,8,8,6,6,3,2}$ [108] | $S_{10,10,8,8,6,6,3,2,1}$ [108] |
| | [0,2,1,0,0,2,0,1,0,1] | [2,4,8,13,18,23,30,37,27,17,18] | $S_{10,10,8,8,7,4,4,2}$ [108] | $S_{10,10,8,8,7,4,4,2,1}$ [108] |
| | [1,0,1,1,1,1,0,1,0,1] | [2,5,8,12,17,23,30,37,27,17,18] | $S_{10,10,9,7,6,5,4,2}$ [216] | $S_{10,10,9,7,6,5,4,2,1}$ [216] |
| | [1,0,2,0,0,1,2,0,0,1] | [2,5,8,13,18,23,29,37,27,17,18] | $S_{10,10,9,7,7,4,3,3}$ [96] | $S_{10,10,9,7,7,4,3,3,1}$ [96] |
| | [1,1,0,0,2,0,2,0,0,1] | [2,5,9,13,17,23,29,37,27,17,18] | $S_{10,10,9,8,5,5,3,3}$ [96] | $S_{10,10,9,8,5,5,3,3,1}$ [96] |
| | [1,3,0,1,0,0,1,0,1,2] | [1,3,8,13,19,25,31,38,27,17,18] | $S_{10,9,8,8,8,6,3,1}$ [144] | $S_{10,9,8,8,8,6,3,1,1}$ [144] |
| | [2,0,0,0,0,3,1,0,0,1] | [2,6,10,14,18,22,29,37,27,17,18] | $S_{10,10,9,9,4,4,4,3}$ [48] | $S_{10,10,9,9,4,4,4,3,1}$ [48] |
| | [2,0,3,0,0,0,1,0,1,2] | [1,4,7,13,19,25,31,38,27,17,18] | $S_{10,9,9,7,7,7,3,1}$ [90] | $S_{10,9,9,7,7,7,3,1,1}$ [90] |
| | [2,1,0,2,0,1,0,0,1,2] | [1,4,8,12,18,24,31,38,27,17,18] | $S_{10,9,9,8,6,6,4,1}$ [144] | $S_{10,9,9,8,6,6,4,1,1}$ [144] |
| | [2,1,1,0,1,0,1,1,0,1] | [1,4,8,13,18,24,30,37,27,17,18] | $S_{10,9,9,8,7,5,3,2}$ [216] | $S_{10,9,9,8,7,5,3,2,1}$ [216] |
| | [3,0,0,0,3,0,0,0,1,2] | [1,5,9,13,17,24,31,38,27,17,18] | $S_{10,9,9,9,5,5,5,1}$ [50] | $S_{10,9,9,9,5,5,5,1,1}$ [50] |
| | [3,0,0,1,0,2,0,1,0,1] | [1,5,9,13,18,23,30,37,27,17,18] | $S_{10,9,9,9,6,4,4,2}$ [108] | $S_{10,9,9,9,6,4,4,2,1}$ [108] |
| | [3,0,1,0,0,0,3,0,0,1] | [1,5,9,14,19,24,29,37,27,17,18] | $S_{10,9,9,9,7,3,3,3}$ [60] | $S_{10,9,9,9,7,3,3,3,1}$ [60] |
| | [3,3,0,0,0,0,0,0,2,3] | [0,3,9,15,21,27,33,39,27,17,18] | $S_{9,9,9,8,8,8,1,1}$ [32] | $S_{9,9,9,8,8,8,1,1,1}$ [32] |
| | [4,0,2,0,0,0,0,1,1,2] | [0,4,8,14,20,26,32,38,27,17,18] | $S_{9,9,9,9,7,7,2,1}$ [72] | $S_{9,9,9,9,7,7,2,1,1}$ [72] |
| | [4,1,0,0,1,0,1,0,1,2] | [0,4,9,14,19,25,31,38,27,17,18] | $S_{9,9,9,9,8,5,3,1}$ [144] | $S_{9,9,9,9,8,5,3,1,1}$ [144] |
| | [5,0,0,0,0,1,0,2,0,1] | [0,5,10,15,20,25,31,37,27,17,18] | $S_{9,9,9,9,9,4,2,2}$ [54] | $S_{9,9,9,9,9,4,2,2,1}$ [54] |
| | [1,0,0,4,0,0,0,0,0,3] | [2,5,8,11,18,25,32,39,28,17,18] | $S_{10,10,9,6,6,6,6}$ [28] | $S_{10,10,9,6,6,6,6,1,1,1}$ [28] |
| | [1,2,2,0,0,1,0,0,0,3] | [1,3,7,13,19,25,32,39,28,17,18] | $S_{10,9,8,8,7,7,4}$ [80] | $S_{10,9,8,8,7,7,4,1,1,1}$ [80] |
| | [1,3,0,0,2,0,0,0,0,3] | [1,3,8,13,18,25,32,39,28,17,18] | $S_{10,9,8,8,8,5,5}$ [48] | $S_{10,9,8,8,8,5,5,1,1,1}$ [48] |
| | [2,0,2,1,1,0,0,0,0,3] | [1,4,7,12,18,25,32,39,28,17,18] | $S_{10,9,9,7,7,6,5}$ [72] | $S_{10,9,9,7,7,6,5,1,1,1}$ [72] |
| | [3,2,1,0,0,0,1,0,0,3] | [0,3,8,14,20,26,32,39,28,17,18] | $S_{9,9,9,8,8,7,3}$ [80] | $S_{9,9,9,8,8,7,3,1,1,1}$ [80] |
| | [4,0,1,1,0,1,0,0,0,3] | [0,4,8,13,19,25,32,39,28,17,18] | $S_{9,9,9,9,7,6,4}$ [90] | $S_{9,9,9,9,7,6,4,1,1,1}$ [90] |
| | [0,3,0,1,0,0,0,0,5,0] | [2,4,9,14,20,26,32,38,25,17,19] | $S_{10,10,8,8,8,6,1,1,1,1,1}$ [31] | $S_{10,10,8,8,8,6}$ [32] |
| | [3,0,1,1,0,0,0,0,5,0] | [1,5,9,14,20,26,32,38,25,17,19] | $S_{10,9,9,9,7,6,1,1,1,1,1}$ [42] | $S_{10,9,9,9,7,6}$ [42] |
| | [0,2,0,2,0,1,0,0,3,0] | [2,4,8,12,18,24,31,38,26,17,19] | $S_{10,10,8,8,6,6,4,1,1,1}$ [67] | $S_{10,10,8,8,6,6,4}$ [68] |
| | [1,0,1,1,2,0,0,0,3,0] | [2,5,8,12,17,24,31,38,26,17,19] | $S_{10,10,9,7,6,5,5,1,1,1}$ [72] | $S_{10,10,9,7,6,5,5}$ [72] |
| | [1,3,1,0,0,0,0,1,3,0] | [1,3,8,14,20,26,32,38,26,17,19] | $S_{10,9,8,8,8,7,2,1,1,1}$ [72] | $S_{10,9,8,8,8,7,2}$ [72] |
| | [2,1,1,0,1,1,0,0,3,0] | [1,4,8,13,18,24,31,38,26,17,19] | $S_{10,9,9,8,7,5,4,1,1,1}$ [120] | $S_{10,9,9,8,7,5,4}$ [120] |
| | [4,1,0,1,0,0,0,1,3,0] | [0,4,9,14,20,26,32,38,26,17,19] | $S_{9,9,9,9,8,6,2,1,1,1}$ [90] | $S_{9,9,9,9,8,6,2}$ [90] |
| | [5,0,0,0,0,1,1,0,3,0] | [0,5,10,15,20,25,31,38,26,17,19] | $S_{9,9,9,9,9,4,3,1,1,1}$ [48] | $S_{9,9,9,9,9,4,3}$ [48] |
| | [0,0,0,2,0,3,0,0,1,0] | [3,6,9,12,17,22,30,38,27,17,19] | $S_{10,10,10,6,6,4,4,4,1}$ [37] | $S_{10,10,10,6,6,4,4,4}$ [38] |

| | | | | |
|---|---|---|---|---|
| | [0,1,1,3,0,0,0,0,2,1] | [2,4,7,11,18,25,32,39,27,17,19] | $S_{10,10,8,7,6,6,6,1,1}$ [72] | $S_{10,10,8,7,6,6,6,1}$ [72] |
| | [0,1,2,0,2,0,0,1,1,0] | [2,4,7,12,17,24,31,38,27,17,19] | $S_{10,10,8,7,7,5,5,2,1}$ [108] | $S_{10,10,8,7,7,5,5,2}$ [108] |
| | [0,1,2,1,0,0,2,0,1,0] | [2,4,7,12,18,24,30,38,27,17,19] | $S_{10,10,8,7,7,6,3,3,1}$ [96] | $S_{10,10,8,7,7,6,3,3}$ [96] |
| | [0,2,0,1,1,1,1,0,1,0] | [2,4,8,12,17,23,30,38,27,17,19] | $S_{10,10,8,8,6,5,4,3,1}$ [144] | $S_{10,10,8,8,6,5,4,3}$ [144] |
| | [1,0,0,3,1,0,0,1,1,0] | [2,5,8,11,17,24,31,38,27,17,19] | $S_{10,10,9,6,6,6,5,2,1}$ [96] | $S_{10,10,9,6,6,6,5,2}$ [96] |
| | [1,1,0,0,1,3,0,0,1,0] | [2,5,9,13,17,22,30,38,27,17,19] | $S_{10,10,9,8,5,4,4,4,1}$ [80] | $S_{10,10,9,8,5,4,4,4}$ [80] |
| | [1,2,1,1,1,0,0,0,2,1] | [1,3,7,12,18,25,32,39,27,17,19] | $S_{10,9,8,8,7,6,5,1,1}$ [160] | $S_{10,9,8,8,7,6,5,1}$ [160] |
| | [1,2,2,0,0,0,1,1,1,0] | [1,3,7,13,19,25,31,38,27,17,19] | $S_{10,9,8,8,7,7,3,2,1}$ [120] | $S_{10,9,8,8,7,7,3,2}$ [120] |
| | [1,3,0,0,1,1,0,1,1,0] | [1,3,8,13,18,24,31,38,27,17,19] | $S_{10,9,8,8,8,5,4,2,1}$ [144] | $S_{10,9,8,8,8,5,4,2}$ [144] |
| | [2,0,2,1,0,1,0,1,1,0] | [1,4,7,12,18,24,31,38,27,17,19] | $S_{10,9,9,7,7,6,4,2,1}$ [162] | $S_{10,9,9,7,7,6,4,2}$ [162] |
| | [2,1,0,1,2,0,0,1,1,0] | [1,4,8,12,17,24,31,38,27,17,19] | $S_{10,9,9,8,6,5,5,2,1}$ [144] | $S_{10,9,9,8,6,5,5,2}$ [144] |
| | [2,1,0,2,0,0,2,0,1,0] | [1,4,8,12,18,24,30,38,27,17,19] | $S_{10,9,9,8,6,6,3,3,1}$ [96] | $S_{10,9,9,8,6,6,3,3}$ [96] |
| | [2,1,1,0,0,2,1,0,1,0] | [1,4,8,13,18,23,30,38,27,17,19] | $S_{10,9,9,8,7,4,4,3,1}$ [128] | $S_{10,9,9,8,7,4,4,3}$ [128] |
| | [3,0,0,0,2,1,1,0,1,0] | [1,5,9,13,17,23,30,38,27,17,19] | $S_{10,9,9,9,5,5,4,3,1}$ [80] | $S_{10,9,9,9,5,5,4,3}$ [80] |
| | [3,2,0,1,0,1,0,0,2,1] | [0,3,8,13,19,25,32,39,27,17,19] | $S_{9,9,9,8,8,6,4,1,1}$ [144] | $S_{9,9,9,8,8,6,4,1}$ [144] |
| | [3,2,1,0,0,0,0,2,1,0] | [0,3,8,14,20,26,32,38,27,17,19] | $S_{9,9,9,8,8,7,2,2,1}$ [72] | $S_{9,9,9,8,8,7,2,2}$ [72] |
| | [4,0,1,0,2,0,0,0,2,1] | [0,4,8,13,18,25,32,39,27,17,19] | $S_{9,9,9,9,7,5,5,1,1}$ [90] | $S_{9,9,9,9,7,5,5,1}$ [90] |
| | [4,0,1,1,0,0,1,1,1,0] | [0,4,8,13,19,25,31,38,27,17,19] | $S_{9,9,9,9,7,6,3,2,1}$ [144] | $S_{9,9,9,9,7,6,3,2}$ [144] |
| | [4,1,0,0,0,2,0,1,1,0] | [0,4,9,14,19,24,31,38,27,17,19] | $S_{9,9,9,9,8,4,4,2,1}$ [90] | $S_{9,9,9,9,8,4,4,2}$ [90] |
| | [5,0,0,0,0,0,3,0,1,0] | [0,5,10,15,20,25,30,38,27,17,19] | $S_{9,9,9,9,9,3,3,3,1}$ [28] | $S_{9,9,9,9,9,3,3,3}$ [28] |
| | [0,0,4,0,1,0,0,1,0,1] | [2,4,6,12,18,25,32,39,28,17,19] | $S_{10,10,7,7,7,7,5,2}$ [72] | $S_{10,10,7,7,7,7,5,2,1}$ [72] |
| | [0,1,1,2,1,0,1,0,0,1] | [2,4,7,11,17,24,31,39,28,17,19] | $S_{10,10,8,7,6,6,5,3}$ [144] | $S_{10,10,8,7,6,6,5,3,1}$ [144] |
| | [0,1,2,0,1,2,0,0,0,1] | [2,4,7,12,17,23,31,39,28,17,19] | $S_{10,10,8,7,7,5,4,4}$ [90] | $S_{10,10,8,7,7,5,4,4,1}$ [90] |
| | [0,4,1,0,1,0,0,0,1,2] | [1,2,7,13,19,26,33,40,28,17,19] | $S_{10,8,8,8,8,7,5,1}$ [90] | $S_{10,8,8,8,8,7,5,1,1}$ [90] |
| | [0,5,0,0,0,0,1,1,0,1] | [1,2,8,14,20,26,32,39,28,17,19] | $S_{10,8,8,8,8,8,3,2}$ [54] | $S_{10,8,8,8,8,8,3,2,1}$ [54] |
| | [1,0,0,3,0,2,0,0,0,1] | [2,5,8,11,17,23,31,39,28,17,19] | $S_{10,10,9,6,6,6,4,4}$ [60] | $S_{10,10,9,6,6,6,4,4,1}$ [60] |
| | [1,1,3,1,0,0,0,0,1,2] | [1,3,6,12,19,26,33,40,28,17,19] | $S_{10,9,8,7,7,7,6,1}$ [96] | $S_{10,9,8,7,7,7,6,1,1}$ [96] |
| | [1,2,1,1,0,1,1,0,0,1] | [1,3,7,12,18,24,31,39,28,17,19] | $S_{10,9,8,8,7,6,4,3}$ [192] | $S_{10,9,8,8,7,6,4,3,1}$ [192] |
| | [2,0,1,3,0,0,0,1,0,1] | [1,4,7,11,18,25,32,39,28,17,19] | $S_{10,9,9,7,6,6,6,2}$ [90] | $S_{10,9,9,7,6,6,6,2,1}$ [90] |
| | [2,0,2,0,2,0,1,0,0,1] | [1,4,7,12,17,24,31,39,28,17,19] | $S_{10,9,9,7,7,5,5,3}$ [108] | $S_{10,9,9,7,7,5,5,3,1}$ [108] |
| | [2,1,0,1,1,2,0,0,0,1] | [1,4,8,12,17,23,31,39,28,17,19] | $S_{10,9,9,8,6,5,4,4}$ [120] | $S_{10,9,9,8,6,5,4,4,1}$ [120] |
| | [2,4,0,0,0,1,0,0,1,2] | [0,2,8,14,20,26,33,40,28,17,19] | $S_{9,9,8,8,8,8,4,1}$ [80] | $S_{9,9,8,8,8,8,4,1,1}$ [80] |
| | [3,1,1,2,0,0,0,0,1,2] | [0,3,7,12,19,26,33,40,28,17,19] | $S_{9,9,9,8,7,6,6,1}$ [96] | $S_{9,9,9,8,7,6,6,1,1}$ [96] |
| | [3,1,2,0,0,1,0,1,0,1] | [0,3,7,13,19,25,32,39,28,17,19] | $S_{9,9,9,8,7,7,4,2}$ [144] | $S_{9,9,9,8,7,7,4,2,1}$ [144] |
| | [3,2,0,0,2,0,0,1,0,1] | [0,3,8,13,18,25,32,39,28,17,19] | $S_{9,9,9,8,8,5,5,2}$ [96] | $S_{9,9,9,8,8,5,5,2,1}$ [96] |
| | [3,2,0,1,0,0,2,0,0,1] | [0,3,8,13,19,25,31,39,28,17,19] | $S_{9,9,9,8,8,6,3,3}$ [96] | $S_{9,9,9,8,8,6,3,3,1}$ [96] |
| | [4,0,0,2,1,0,0,1,0,1] | [0,4,8,12,18,25,32,39,28,17,19] | $S_{9,9,9,9,6,6,5,2}$ [96] | $S_{9,9,9,9,6,6,5,2,1}$ [96] |
| | [4,0,1,0,1,1,1,0,0,1] | [0,4,8,13,18,24,31,39,28,17,19] | $S_{9,9,9,9,7,5,4,3}$ [144] | $S_{9,9,9,9,7,5,4,3,1}$ [144] |
| | [2,3,1,1,0,0,0,0,0,3] | [0,2,7,13,20,27,34,41,29,17,19] | $S_{9,9,8,8,8,7,6}$ [56] | $S_{9,9,8,8,8,7,6,1,1,1}$ [56] |
| | [0,5,0,0,0,1,0,0,3,0] | [1,2,8,14,20,26,33,40,27,17,20] | $S_{10,8,8,8,8,8,4,1,1,1}$ [37] | $S_{10,8,8,8,8,8,4}$ [38] |
| | [3,1,2,0,1,0,0,0,3,0] | [0,3,7,13,19,26,33,40,27,17,20] | $S_{9,9,9,8,7,7,5,1,1,1}$ [72] | $S_{9,9,9,8,7,7,5}$ [72] |
| | [4,0,0,3,0,0,0,0,3,0] | [0,4,8,12,19,26,33,40,27,17,20] | $S_{9,9,9,9,6,6,6,1,1,1}$ [28] | $S_{9,9,9,9,6,6,6}$ [28] |
| | [0,0,3,2,0,0,1,0,1,0] | [2,4,6,11,18,25,32,40,28,17,20] | $S_{10,10,7,7,7,6,6,3,1}$ [64] | $S_{10,10,7,7,7,6,6,3}$ [64] |
| | [0,0,4,0,0,2,0,0,1,0] | [2,4,6,12,18,24,32,40,28,17,20] | $S_{10,10,7,7,7,7,4,4,1}$ [40] | $S_{10,10,7,7,7,7,4,4}$ [40] |
| | [0,3,3,0,0,0,0,0,2,1] | [1,2,6,13,20,27,34,41,28,17,20] | $S_{10,8,8,8,7,7,7,1,1}$ [42] | $S_{10,8,8,8,7,7,7,1}$ [42] |
| | [0,4,0,2,0,0,0,1,1,0] | [1,2,7,12,19,26,33,40,28,17,20] | $S_{10,8,8,8,8,6,6,2,1}$ [67] | $S_{10,8,8,8,8,6,6,2}$ [68] |
| | [0,4,1,0,0,1,1,0,1,0] | [1,2,7,13,19,25,32,40,28,17,20] | $S_{10,8,8,8,8,7,4,3,1}$ [96] | $S_{10,8,8,8,8,7,4,3}$ [96] |
| | [1,1,3,0,1,0,1,0,1,0] | [1,3,6,12,18,25,32,40,28,17,20] | $S_{10,9,8,7,7,7,5,3,1}$ [144] | $S_{10,9,8,7,7,7,5,3}$ [144] |
| | [1,2,0,3,0,0,1,0,1,0] | [1,3,7,11,18,25,32,40,28,17,20] | $S_{10,9,8,8,6,6,6,3,1}$ [96] | $S_{10,9,8,8,6,6,6,3}$ [96] |
| | [1,2,1,0,2,1,0,0,1,0] | [1,3,7,12,17,24,32,40,28,17,20] | $S_{10,9,8,8,7,5,5,4,1}$ [120] | $S_{10,9,8,8,7,5,5,4}$ [120] |
| | [2,0,1,2,1,1,0,0,1,0] | [1,4,7,11,17,24,32,40,28,17,20] | $S_{10,9,9,7,6,6,5,4,1}$ [120] | $S_{10,9,9,7,6,6,5,4}$ [120] |
| | [2,3,1,0,1,0,0,1,1,0] | [0,2,7,13,19,26,33,40,28,17,20] | $S_{9,9,8,8,8,7,5,2,1}$ [144] | $S_{9,9,8,8,8,7,5,2}$ [144] |
| | [2,4,0,0,0,0,2,0,1,0] | [0,2,8,14,20,26,32,40,28,17,20] | $S_{9,9,8,8,8,8,3,3,1}$ [48] | $S_{9,9,8,8,8,8,3,3}$ [48] |
| | [3,0,4,0,0,0,0,0,2,1] | [0,3,6,13,20,27,34,41,28,17,20] | $S_{9,9,9,7,7,7,7,1,1}$ [42] | $S_{9,9,9,7,7,7,7,1}$ [42] |
| | [3,1,1,1,1,0,1,0,1,0] | [0,3,7,12,18,25,32,40,28,17,20] | $S_{9,9,9,8,7,6,5,3,1}$ [192] | $S_{9,9,9,8,7,6,5,3}$ [192] |
| | [3,2,0,0,1,2,0,0,1,0] | [0,3,8,13,18,24,32,40,28,17,20] | $S_{9,9,9,8,8,5,4,4,1}$ [80] | $S_{9,9,9,8,8,5,4,4}$ [80] |
| | [4,0,0,2,0,2,0,0,1,0] | [0,4,8,12,18,24,32,40,28,17,20] | $S_{9,9,9,9,6,6,4,4,1}$ [60] | $S_{9,9,9,9,6,6,4,4}$ [60] |
| | [0,0,3,1,2,0,0,0,0,1] | [2,4,6,11,17,25,33,41,29,17,20] | $S_{10,10,7,7,7,6,5,5}$ [48] | $S_{10,10,7,7,7,6,5,5,1}$ [48] |
| | [0,3,2,1,0,0,1,0,0,1] | [1,2,6,12,19,26,33,41,29,17,20] | $S_{10,8,8,8,7,7,6,3}$ [96] | $S_{10,8,8,8,7,7,6,3,1}$ [96] |
| | [0,4,0,1,1,1,0,0,0,1] | [1,2,7,12,18,25,33,41,29,17,20] | $S_{10,8,8,8,8,6,5,4}$ [90] | $S_{10,8,8,8,8,6,5,4,1}$ [90] |
| | [1,1,2,2,0,1,0,0,0,1] | [1,3,6,11,18,25,33,41,29,17,20] | $S_{10,9,8,7,7,6,6,4}$ [120] | $S_{10,9,8,7,7,6,6,4,1}$ [120] |
| | [1,2,0,2,2,0,0,0,0,1] | [1,3,7,11,17,25,33,41,29,17,20] | $S_{10,9,8,8,6,6,5,5}$ [72] | $S_{10,9,8,8,6,6,5,5,1}$ [72] |
| | [2,2,3,0,0,0,0,1,0,1] | [0,2,6,13,20,27,34,41,29,17,20] | $S_{9,9,8,8,7,7,7,2}$ [72] | $S_{9,9,8,8,7,7,7,2,1}$ [72] |
| | [2,3,0,2,0,0,1,0,0,1] | [0,2,7,12,19,26,33,41,29,17,20] | $S_{9,9,8,8,8,6,6,3}$ [96] | $S_{9,9,8,8,8,6,6,3,1}$ [96] |
| | [2,3,1,0,0,2,0,0,0,1] | [0,2,7,13,19,25,33,41,29,17,20] | $S_{9,9,8,8,8,7,4,4}$ [80] | $S_{9,9,8,8,8,7,4,4,1}$ [80] |
| | [3,0,3,1,0,0,1,0,0,1] | [0,3,6,12,19,26,33,41,29,17,20] | $S_{9,9,9,7,7,7,6,3}$ [96] | $S_{9,9,9,7,7,7,6,3,1}$ [96] |
| | [4,0,0,1,3,0,0,0,0,1] | [0,4,8,12,17,25,33,41,29,17,20] | $S_{9,9,9,9,6,5,5,5}$ [48] | $S_{9,9,9,9,6,5,5,5,1}$ [48] |
| | [1,6,0,0,0,0,0,0,0,3] | [0,1,8,15,22,29,36,43,30,17,20] | $S_{9,8,8,8,8,8,8}$ [18] | $S_{9,8,8,8,8,8,8,1,1,1}$ [18] |
| | [0,1,0,5,0,0,0,0,1,0] | [2,4,7,10,18,26,34,42,29,17,21] | $S_{10,10,8,6,6,6,6,6,1}$ [31] | $S_{10,10,8,6,6,6,6,6}$ [32] |
| | [0,3,2,0,2,0,0,0,1,0] | [1,2,6,12,18,26,34,42,29,17,21] | $S_{10,8,8,8,7,7,5,5,1}$ [54] | $S_{10,8,8,8,7,7,5,5}$ [54] |
| | [1,5,1,0,0,0,0,1,1,0] | [0,1,7,14,21,28,35,42,29,17,21] | $S_{9,8,8,8,8,8,7,2,1}$ [72] | $S_{9,8,8,8,8,8,7,2}$ [72] |

| | | | | |
|---|---|---|---|---|
| | [2,2,2,1,0,1,0,0,1,0] | [0,2,6,12,19,26,34,42,29,17,21] | $S_{9,9,8,8,7,7,6,4,1}$ [120] | $S_{9,9,8,8,7,7,6,4}$ [120] |
| | [2,3,0,1,2,0,0,0,1,0] | [0,2,7,12,18,26,34,42,29,17,21] | $S_{9,9,8,8,8,6,5,5,1}$ [72] | $S_{9,9,8,8,8,6,5,5}$ [72] |
| | [3,0,3,0,2,0,0,0,1,0] | [0,3,6,12,18,26,34,42,29,17,21] | $S_{9,9,9,7,7,7,5,5,1}$ [54] | $S_{9,9,9,7,7,7,5,5}$ [54] |
| | [3,1,0,3,1,0,0,0,1,0] | [0,3,7,11,18,26,34,42,29,17,21] | $S_{9,9,9,8,6,6,6,5,1}$ [72] | $S_{9,9,9,8,6,6,6,5}$ [72] |
| | [0,3,1,3,0,0,0,0,0,1] | [1,2,6,11,19,27,35,43,30,17,21] | $S_{10,8,8,8,7,6,6,6}$ [42] | $S_{10,8,8,8,7,6,6,6,1}$ [42] |
| | [1,0,5,0,1,0,0,0,0,1] | [1,3,5,12,19,27,35,43,30,17,21] | $S_{10,9,7,7,7,7,7,5}$ [54] | $S_{10,9,7,7,7,7,7,5,1}$ [54] |
| | [1,5,0,1,0,1,0,0,0,1] | [0,1,7,13,20,27,35,43,30,17,21] | $S_{9,8,8,8,8,8,6,4}$ [90] | $S_{9,8,8,8,8,8,6,4,1}$ [90] |
| | [3,0,2,3,0,0,0,0,0,1] | [0,3,6,11,19,27,35,43,30,17,21] | $S_{9,9,9,7,7,6,6,6}$ [42] | $S_{9,9,9,7,7,6,6,6,1}$ [42] |
| | [0,2,4,1,0,0,0,0,1,0] | [1,2,5,12,20,28,36,44,30,17,22] | $S_{10,8,8,7,7,7,7,6,1}$ [42] | $S_{10,8,8,7,7,7,7,6}$ [42] |
| | [1,4,2,0,1,0,0,0,1,0] | [0,1,6,13,20,28,36,44,30,17,22] | $S_{9,8,8,8,8,7,7,5,1}$ [72] | $S_{9,8,8,8,8,7,7,5}$ [72] |
| | [2,1,5,0,0,0,0,0,0,1] | [0,2,5,13,21,29,37,45,31,17,22] | $S_{9,9,8,7,7,7,7,7}$ [32] | $S_{9,9,8,7,7,7,7,7,1}$ [32] |
| | [0,8,0,0,0,0,0,0,1,0] | [0,0,8,16,24,32,40,48,32,17,24] | $S_{8,8,8,8,8,8,8,8,1}$ [13] | $S_{8,8,8,8,8,8,8,8}$ [14] |
| 18 | [0,0,0,0,0,2,1,1,1,1] | [4,8,12,16,20,24,30,37,27,18,18] | $T_{10,10,10,10,4,4,3,2,1}$ [56] | |
| | [0,0,0,1,0,0,0,4,0,0] | [4,8,12,16,21,26,31,36,27,18,18] | $T_{10,10,10,10,6,2,2,2,2}$ [25] | |
| | [0,0,2,1,0,0,0,1,2,2] | [3,6,9,14,20,26,32,38,27,18,18] | $T_{10,10,10,7,7,6,2,1,1}$ [80] | |
| | [0,1,0,1,1,0,1,0,2,2] | [3,6,10,14,19,25,31,38,27,18,18] | $T_{10,10,10,8,6,5,3,1,1}$ [162] | |
| | [0,1,1,0,0,1,0,2,1,1] | [3,6,10,15,20,25,31,37,27,18,18] | $T_{10,10,10,8,7,4,2,2,1}$ [144] | |
| | [1,0,0,0,1,2,0,0,2,2] | [3,7,11,15,19,24,31,38,27,18,18] | $T_{10,10,10,9,5,4,4,1,1}$ [80] | |
| | [1,0,0,0,2,0,0,2,1,1] | [3,7,11,15,19,25,31,37,27,18,18] | $T_{10,10,10,9,5,5,2,2,1}$ [80] | |
| | [1,0,0,1,0,0,2,1,1,1] | [3,7,11,15,20,25,30,37,27,18,18] | $T_{10,10,10,9,6,3,3,2,1}$ [128] | |
| | [1,1,2,0,0,0,0,0,3,3] | [2,5,9,15,21,27,33,39,27,18,18] | $T_{10,10,9,8,7,7,1,1,1}$ [56] | |
| | [1,2,0,0,1,0,0,1,2,2] | [2,5,10,15,20,26,32,38,27,18,18] | $T_{10,10,9,8,8,5,2,1,1}$ [128] | |
| | [2,0,0,2,0,0,0,1,2,2] | [2,6,10,14,20,26,32,38,27,18,18] | $T_{10,10,9,9,6,6,2,1,1}$ [80] | |
| | [2,0,1,0,0,1,1,0,2,2] | [2,6,10,15,20,25,31,38,27,18,18] | $T_{10,10,9,9,7,4,3,1,1}$ [144] | |
| | [2,1,0,0,0,0,1,2,1,1] | [2,6,11,16,21,26,31,37,27,18,18] | $T_{10,10,9,9,8,3,2,2,1}$ [96] | |
| | [4,0,0,0,1,0,0,0,3,3] | [1,6,11,16,21,27,33,39,27,18,18] | $T_{10,9,9,9,9,5,1,1,1}$ [50] | |
| | [0,0,1,1,1,1,1,0,1,1] | [3,6,9,13,18,24,31,39,28,18,19] | $T_{10,10,10,7,6,5,4,3,1}$ [192] | |
| | [0,0,1,2,0,0,1,2,0,0] | [3,6,9,13,19,25,31,38,28,18,19] | $T_{10,10,10,7,6,6,3,2,2}$ [64] | |
| | [0,1,0,0,2,1,0,2,0,0] | [3,6,10,14,18,24,31,38,28,18,19] | $T_{10,10,10,8,5,5,4,2,2}$ [72] | |
| | [0,1,0,1,0,1,2,1,0,0] | [3,6,10,14,19,24,30,38,28,18,19] | $T_{10,10,10,8,6,4,3,3,2}$ [108] | |
| | [0,2,1,1,1,0,0,0,2,2] | [2,4,8,13,19,26,33,40,28,18,19] | $T_{10,10,8,8,7,6,5,1,1}$ [120] | |
| | [0,2,2,0,0,0,1,1,1,1] | [2,4,8,14,20,26,32,39,28,18,19] | $T_{10,10,8,8,7,7,3,2,1}$ [120] | |
| | [0,3,0,0,1,1,0,1,1,1] | [2,4,9,14,19,25,32,39,28,18,19] | $T_{10,10,8,8,8,5,4,2,1}$ [144] | |
| | [1,0,0,0,0,4,0,0,1,1] | [3,7,11,15,19,23,31,39,28,18,19] | $T_{10,10,10,9,4,4,4,4,1}$ [48] | |
| | [1,0,2,1,0,1,0,1,1,1] | [2,5,8,13,19,25,32,39,28,18,19] | $T_{10,10,9,7,7,6,4,2,1}$ [216] | |
| | [1,1,0,1,2,0,0,1,1,1] | [2,5,9,13,18,25,32,39,28,18,19] | $T_{10,10,9,8,6,5,5,2,1}$ [192] | |
| | [1,1,0,2,0,0,2,0,1,1] | [2,5,9,13,19,25,31,39,28,18,19] | $T_{10,10,9,8,6,6,3,3,1}$ [144] | |
| | [1,1,1,0,0,2,1,0,1,1] | [2,5,9,14,19,24,31,39,28,18,19] | $T_{10,10,9,8,7,4,4,3,1}$ [192] | |
| | [1,1,1,0,1,0,1,2,0,0] | [2,5,9,14,19,25,31,38,28,18,19] | $T_{10,10,9,8,7,5,3,2,2}$ [144] | |
| | [2,0,0,0,2,1,1,0,1,1] | [2,6,10,14,18,24,31,39,28,18,19] | $T_{10,10,9,9,5,5,4,3,1}$ [120] | |
| | [2,0,0,1,0,2,0,2,0,0] | [2,6,10,14,19,24,31,38,28,18,19] | $T_{10,10,9,9,6,4,4,2,2}$ [72] | |
| | [2,0,1,0,0,0,3,1,0,0] | [2,6,10,15,20,25,30,38,28,18,19] | $T_{10,10,9,9,7,3,3,3,2}$ [60] | |
| | [2,1,2,0,0,1,0,0,2,2] | [1,4,8,14,20,26,33,40,28,18,19] | $T_{10,9,9,8,7,7,4,1,1}$ [128] | |
| | [2,2,0,1,0,0,1,1,1,1] | [1,4,9,14,20,26,32,39,28,18,19] | $T_{10,9,9,8,8,6,3,2,1}$ [192] | |
| | [3,0,0,2,1,0,0,0,2,2] | [1,5,9,13,19,26,33,40,28,18,19] | $T_{10,9,9,9,6,6,5,1,1}$ [80] | |
| | [3,0,1,0,1,1,0,1,1,1] | [1,5,9,14,19,25,32,39,28,18,19] | $T_{10,9,9,9,7,5,4,2,1}$ [216] | |
| | [3,1,0,0,0,1,2,0,1,1] | [1,5,10,15,20,25,31,39,28,18,19] | $T_{10,9,9,9,8,4,3,3,1}$ [120] | |
| | [3,1,0,0,1,0,0,3,0,0] | [1,5,10,15,20,26,32,38,28,18,19] | $T_{10,9,9,9,8,5,2,2,2}$ [64] | |
| | [4,2,0,0,0,0,0,1,2,2] | [0,4,10,16,22,28,34,40,28,18,19] | $T_{9,9,9,9,8,8,2,1,1}$ [56] | |
| | [5,0,0,1,0,0,1,0,2,2] | [0,5,10,15,21,27,33,40,28,18,19] | $T_{9,9,9,9,9,6,3,1,1}$ [96] | |
| | [0,0,0,3,0,2,0,1,0,0] | [3,6,9,12,18,24,32,40,29,18,20] | $T_{10,10,10,6,6,6,4,4,2}$ [45] | |
| | [0,1,0,0,1,3,1,0,0,0] | [3,6,10,14,18,23,31,40,29,18,20] | $T_{10,10,10,8,5,4,4,4,3}$ [48] | |
| | [0,1,2,2,0,0,1,0,1,1] | [2,4,7,12,19,26,33,41,29,18,20] | $T_{10,10,8,7,7,6,6,3,1}$ [144] | |
| | [0,1,3,0,0,2,0,0,1,1] | [2,4,7,13,19,25,33,41,29,18,20] | $T_{10,10,8,7,7,7,4,4,1}$ [96] | |
| | [0,1,3,0,1,0,0,2,0,0] | [2,4,7,13,19,26,33,40,29,18,20] | $T_{10,10,8,7,7,7,5,2,2}$ [72] | |
| | [0,2,0,2,1,1,0,0,1,1] | [2,4,8,12,18,25,33,41,29,18,20] | $T_{10,10,8,8,6,6,5,4,1}$ [144] | |
| | [0,2,0,3,0,0,0,2,0,0] | [2,4,8,12,19,26,33,40,29,18,20] | $T_{10,10,8,8,6,6,6,2,2}$ [45] | |
| | [0,2,1,0,2,0,1,1,0,0] | [2,4,8,13,18,25,32,40,29,18,20] | $T_{10,10,8,8,7,5,5,3,2}$ [108] | |
| | [0,3,0,0,0,3,0,1,0,0] | [2,4,9,14,19,24,32,40,29,18,20] | $T_{10,10,8,8,8,4,4,4,2}$ [45] | |
| | [1,0,1,2,1,0,1,1,0,0] | [2,5,8,12,18,25,32,40,29,18,20] | $T_{10,10,9,7,6,6,5,3,2}$ [144] | |
| | [1,0,2,0,1,2,0,1,0,0] | [2,5,8,13,18,24,32,40,29,18,20] | $T_{10,10,9,7,7,5,4,4,2}$ [108] | |
| | [1,0,2,1,0,0,3,0,0,0] | [2,5,8,13,19,25,31,40,29,18,20] | $T_{10,10,9,7,7,6,3,3,3}$ [48] | |
| | [1,1,0,1,1,1,2,0,0,0] | [2,5,9,13,18,24,31,40,29,18,20] | $T_{10,10,9,8,6,5,4,3,3}$ [96] | |
| | [1,2,2,1,0,0,0,1,1,1] | [1,3,7,13,20,27,34,41,29,18,20] | $T_{10,9,8,8,7,7,6,2,1}$ [160] | |
| | [1,3,0,1,1,0,1,0,1,1] | [1,3,8,13,19,26,33,41,29,18,20] | $T_{10,9,8,8,8,6,5,3,1}$ [216] | |
| | [1,3,1,0,0,1,0,2,0,0] | [1,3,8,14,20,26,33,40,29,18,20] | $T_{10,9,8,8,8,7,4,2,2}$ [96] | |
| | [2,0,3,0,1,0,1,0,1,1] | [1,4,7,13,19,26,33,41,29,18,20] | $T_{10,9,9,7,7,7,5,3,1}$ [162] | |
| | [2,1,0,3,0,0,1,0,1,1] | [1,4,8,12,19,26,33,41,29,18,20] | $T_{10,9,9,8,6,6,6,3,1}$ [144] | |
| | [2,1,1,0,2,1,0,0,1,1] | [1,4,8,13,18,25,33,41,29,18,20] | $T_{10,9,9,8,7,5,5,4,1}$ [192] | |
| | [2,1,1,1,0,1,1,1,0,0] | [1,4,8,13,19,25,32,40,29,18,20] | $T_{10,9,9,8,7,6,4,3,2}$ [192] | |
| | [3,0,0,1,2,0,1,1,0,0] | [1,5,9,13,18,25,32,40,29,18,20] | $T_{10,9,9,9,6,5,5,3,2}$ [96] | |

| | | | | |
|---|---|---|---|---|
| | [3,0,1,0,0,3,0,1,0,0] | [1,5,9,14,19,24,32,40,29,18,20] | $T_{10,9,9,9,7,4,4,4,2}$ [72] | |
| | [3,0,1,0,1,0,3,0,0,0] | [1,5,9,14,19,25,31,40,29,18,20] | $T_{10,9,9,9,7,5,3,3,3}$ [54] | |
| | [3,2,1,0,1,0,0,1,1,1] | [0,3,8,14,20,27,34,41,29,18,20] | $T_{9,9,9,8,8,7,5,2,1}$ [192] | |
| | [3,3,0,0,0,0,2,0,1,1] | [0,3,9,15,21,27,33,41,29,18,20] | $T_{9,9,9,8,8,8,3,3,1}$ [72] | |
| | [4,0,1,2,0,0,0,1,1,1] | [0,4,8,13,20,27,34,41,29,18,20] | $T_{9,9,9,9,7,6,6,2,1}$ [120] | |
| | [4,0,2,0,0,1,1,0,1,1] | [0,4,8,14,20,26,33,41,29,18,20] | $T_{9,9,9,9,7,7,4,3,1}$ [144] | |
| | [4,1,0,0,2,0,1,0,1,1] | [0,4,9,14,19,26,33,41,29,18,20] | $T_{9,9,9,9,8,5,5,3,1}$ [144] | |
| | [4,1,0,1,0,1,0,2,0,0] | [0,4,9,14,20,26,33,40,29,18,20] | $T_{9,9,9,9,8,6,4,2,2}$ [108] | |
| | [5,0,0,0,0,3,0,0,1,1] | [0,5,10,15,20,25,33,41,29,18,20] | $T_{9,9,9,9,9,4,4,4,1}$ [48] | |
| | [5,0,0,0,1,0,2,1,0,0] | [0,5,10,15,20,26,32,40,29,18,20] | $T_{9,9,9,9,9,5,3,3,2}$ [60] | |
| | [0,0,4,1,1,0,0,0,1,1] | [2,4,6,12,19,27,35,43,30,18,21] | $T_{10,10,7,7,7,7,6,5,1}$ [80] | |
| | [0,0,5,0,0,0,1,1,0,0] | [2,4,6,13,20,27,34,42,30,18,21] | $T_{10,10,7,7,7,7,7,3,2}$ [40] | |
| | [0,1,1,4,0,0,0,0,1,1] | [2,4,7,11,19,27,35,43,30,18,21] | $T_{10,10,8,7,6,6,6,6,1}$ [72] | |
| | [0,1,2,1,1,1,1,0,0,0] | [2,4,7,12,18,25,33,42,30,18,21] | $T_{10,10,8,7,7,6,5,4,3}$ [96] | |
| | [0,2,1,0,1,3,0,0,0,0] | [2,4,8,13,18,24,33,42,30,18,21] | $T_{10,10,8,8,7,5,4,4,4}$ [36] | |
| | [0,4,1,1,0,1,0,0,1,1] | [1,2,7,13,20,27,35,43,30,18,21] | $T_{10,8,8,8,8,7,6,4,1}$ [144] | |
| | [0,5,0,0,1,0,1,1,0,0] | [1,2,8,14,20,27,34,42,30,18,21] | $T_{10,8,8,8,8,8,5,3,2}$ [72] | |
| | [1,0,0,4,1,0,0,1,0,0] | [2,5,8,11,18,26,34,42,30,18,21] | $T_{10,10,9,6,6,6,6,5,2}$ [64] | |
| | [1,0,1,2,0,3,0,0,0,0] | [2,5,8,12,18,24,33,42,30,18,21] | $T_{10,10,9,7,6,6,4,4,4}$ [36] | |
| | [1,1,4,0,0,1,0,0,1,1] | [1,3,6,13,20,27,35,43,30,18,21] | $T_{10,9,8,7,7,7,7,4,1}$ [128] | |
| | [1,2,1,2,0,1,0,1,0,0] | [1,3,7,12,19,26,34,42,30,18,21] | $T_{10,9,8,8,7,6,6,4,2}$ [144] | |
| | [1,2,2,0,1,0,2,0,0,0] | [1,3,7,13,19,26,33,42,30,18,21] | $T_{10,9,8,8,7,7,5,3,3}$ [72] | |
| | [1,3,0,0,3,0,0,1,0,0] | [1,3,8,13,18,26,34,42,30,18,21] | $T_{10,9,8,8,8,5,5,5,2}$ [64] | |
| | [1,3,0,1,0,2,1,0,0,0] | [1,3,8,13,19,25,33,42,30,18,21] | $T_{10,9,8,8,8,6,4,4,3}$ [72] | |
| | [2,0,2,1,2,0,0,1,0,0] | [1,4,7,12,18,26,34,42,30,18,21] | $T_{10,9,9,7,7,6,5,5,2}$ [96] | |
| | [2,0,3,0,0,2,1,0,0,0] | [1,4,7,13,19,25,33,42,30,18,21] | $T_{10,9,9,7,7,7,4,4,3}$ [48] | |
| | [2,1,0,2,1,1,1,0,0,0] | [1,4,8,12,18,25,33,42,30,18,21] | $T_{10,9,9,8,6,6,5,4,3}$ [96] | |
| | [2,3,2,0,0,0,1,0,1,1] | [0,2,7,14,21,28,35,43,30,18,21] | $T_{9,9,8,8,8,7,7,3,1}$ [120] | |
| | [2,4,0,0,1,1,0,0,1,1] | [0,2,8,14,20,27,35,43,30,18,21] | $T_{9,9,8,8,8,8,5,4,1}$ [128] | |
| | [2,4,0,1,0,0,0,2,0,0] | [0,2,8,14,21,28,35,42,30,18,21] | $T_{9,9,8,8,8,8,6,2,2}$ [60] | |
| | [3,0,0,1,1,3,0,0,0,0] | [1,5,9,13,18,24,33,42,30,18,21] | $T_{10,9,9,9,6,5,4,4,4}$ [32] | |
| | [3,1,2,0,2,0,0,0,1,1] | [0,3,7,13,19,27,35,43,30,18,21] | $T_{9,9,9,8,7,7,5,5,1}$ [120] | |
| | [3,1,2,1,0,0,1,1,0,0] | [0,3,7,13,20,27,34,42,30,18,21] | $T_{9,9,9,8,7,7,6,3,2}$ [128] | |
| | [3,2,0,1,1,1,0,1,0,0] | [0,3,8,13,19,26,34,42,30,18,21] | $T_{9,9,9,8,8,6,5,4,2}$ [144] | |
| | [3,2,1,0,0,1,2,0,0,0] | [0,3,8,14,20,26,33,42,30,18,21] | $T_{9,9,9,8,8,7,4,3,3}$ [64] | |
| | [4,0,0,3,1,0,0,0,1,1] | [0,4,8,12,19,27,35,43,30,18,21] | $T_{9,9,9,9,6,6,6,5,1}$ [80] | |
| | [4,0,1,1,1,0,2,0,0,0] | [0,4,8,13,19,26,33,42,30,18,21] | $T_{9,9,9,9,7,6,5,3,3}$ [72] | |
| | [4,1,0,0,1,2,1,0,0,0] | [0,4,9,14,19,25,33,42,30,18,21] | $T_{9,9,9,9,8,5,4,4,3}$ [64] | |
| | [0,0,4,1,0,2,0,0,0,0] | [2,4,6,12,19,26,35,44,31,18,22] | $T_{10,10,7,7,7,7,6,4,4}$ [24] | |
| | [0,1,1,3,1,1,0,0,0,0] | [2,4,7,11,18,26,35,44,31,18,22] | $T_{10,10,8,7,6,6,6,5,4}$ [48] | |
| | [0,3,3,0,1,0,0,1,0,0] | [1,2,6,13,20,28,36,44,31,18,22] | $T_{10,8,8,8,7,7,7,5,2}$ [72] | |
| | [0,4,0,3,0,0,0,1,0,0] | [1,2,7,12,20,28,36,44,31,18,22] | $T_{10,8,8,8,8,6,6,6,2}$ [45] | |
| | [0,4,1,0,2,0,1,0,0,0] | [1,2,7,13,19,27,35,44,31,18,22] | $T_{10,8,8,8,8,7,5,5,3}$ [54] | |
| | [0,5,0,0,0,3,0,0,0,0] | [1,2,8,14,20,26,35,44,31,18,22] | $T_{10,8,8,8,8,8,4,4,4}$ [15] | |
| | [1,1,3,1,1,0,1,0,0,0] | [1,3,6,12,19,27,35,44,31,18,22] | $T_{10,9,8,7,7,7,6,5,3}$ [96] | |
| | [1,2,1,1,2,1,0,0,0,0] | [1,3,7,12,18,26,35,44,31,18,22] | $T_{10,9,8,8,7,6,5,5,4}$ [64] | |
| | [1,6,0,0,0,1,0,0,1,1] | [0,1,8,15,22,29,37,45,31,18,22] | $T_{9,8,8,8,8,8,8,4,1}$ [80] | |
| | [2,0,1,4,0,0,1,0,0,0] | [1,4,7,11,19,27,35,44,31,18,22] | $T_{10,9,9,7,6,6,6,6,3}$ [48] | |
| | [2,2,3,1,0,0,0,0,1,1] | [0,2,6,13,21,29,37,45,31,18,22] | $T_{9,9,8,8,7,7,7,6,1}$ [96] | |
| | [2,3,1,1,0,1,1,0,0,0] | [0,2,7,13,20,27,35,44,31,18,22] | $T_{9,9,8,8,8,7,6,4,3}$ [96] | |
| | [3,0,4,0,1,0,0,1,0,0] | [0,3,6,13,20,28,36,44,31,18,22] | $T_{9,9,9,7,7,7,7,5,2}$ [72] | |
| | [3,1,1,2,1,0,1,0,0,0] | [0,3,7,12,19,27,35,44,31,18,22] | $T_{9,9,9,8,7,6,6,5,3}$ [96] | |
| | [3,1,2,0,1,2,0,0,0,0] | [0,3,7,13,19,26,35,44,31,18,22] | $T_{9,9,9,8,7,7,5,4,4}$ [48] | |
| | [4,0,0,3,0,2,0,0,0,0] | [0,4,8,12,19,26,35,44,31,18,22] | $T_{9,9,9,9,6,6,6,4,4}$ [24] | |
| | [4,0,1,0,3,1,0,0,0,0] | [0,4,8,13,18,26,35,44,31,18,22] | $T_{9,9,9,9,7,5,5,5,4}$ [36] | |
| | [0,3,2,2,0,1,0,0,0,0] | [1,2,6,12,20,28,37,46,32,18,23] | $T_{10,8,8,8,7,7,6,6,4}$ [36] | |
| | [1,2,0,4,1,0,0,0,0,0] | [1,3,7,11,19,28,37,46,32,18,23] | $T_{10,9,8,8,6,6,6,6,5}$ [24] | |
| | [1,5,1,0,1,0,1,0,0,0] | [0,1,7,14,21,29,37,46,32,18,23] | $T_{9,8,8,8,8,8,7,5,3}$ [72] | |
| | [2,2,3,0,1,1,0,0,0,0] | [0,2,6,13,20,28,37,46,32,18,23] | $T_{9,9,8,8,7,7,7,5,4}$ [48] | |
| | [2,3,0,3,0,1,0,0,0,0] | [0,2,7,12,20,28,37,46,32,18,23] | $T_{9,9,8,8,8,6,6,6,4}$ [36] | |
| | [2,3,1,0,3,0,0,0,0,0] | [0,2,7,13,19,28,37,46,32,18,23] | $T_{9,9,8,8,8,7,5,5,5}$ [24] | |
| | [3,0,3,2,0,1,0,0,0,0] | [0,3,6,12,20,28,37,46,32,18,23] | $T_{9,9,9,7,7,7,6,6,4}$ [36] | |
| | [1,0,6,0,1,0,0,0,0,0] | [1,3,5,13,21,30,39,48,33,18,24] | $T_{10,9,7,7,7,7,7,7,5}$ [18] | |
| | [1,4,3,0,0,1,0,0,0,0] | [0,1,6,14,22,30,39,48,33,18,24] | $T_{9,8,8,8,8,7,7,7,4}$ [32] | |
| | [1,5,0,2,1,0,0,0,0,0] | [0,1,7,13,21,30,39,48,33,18,24] | $T_{9,8,8,8,8,8,6,6,5}$ [24] | |
| | [2,2,2,3,0,0,0,0,0,0] | [0,2,6,12,21,30,39,48,33,18,24] | $T_{9,9,8,8,7,7,6,6,6}$ [16] | |
| | [0,8,0,1,0,0,0,0,0,0] | [0,0,8,16,25,34,43,52,35,18,26] | $T_{8,8,8,8,8,8,8,8,6}$ [9] | |
| | [0,0,0,0,1,1,0,1,3,1] | [4,8,12,16,20,25,31,37,26,18,18] | $T_{10,10,10,10,5,4,2,1,1,1}$ [72] | $T_{10,10,10,10,5,4,2,1}$ [72] |
| | [0,2,0,0,0,1,0,0,4,2] | [3,6,11,16,21,26,32,38,26,18,18] | $T_{10,10,10,8,8,4,1,1,1,1}$ [60] | $T_{10,10,10,8,8,4,1,1}$ [60] |
| | [1,0,0,1,1,0,0,0,4,2] | [3,7,11,15,20,26,32,38,26,18,18] | $T_{10,10,10,9,6,5,1,1,1,1}$ [80] | $T_{10,10,10,9,6,5,1,1}$ [80] |
| | [1,0,1,0,0,0,1,1,3,1] | [3,7,11,16,21,26,31,37,26,18,18] | $T_{10,10,10,9,7,3,2,1,1,1}$ [120] | $T_{10,10,10,9,7,3,2,1}$ [120] |

| | | | | |
|---|---|---|---|---|
| | [3,0,0,0,0,0,1,0,4,2] | [2,7,12,17,22,27,32,38,26,18,18] | $T_{10,10,9,9,9,3,1,1,1,1}$ [42] | $T_{10,10,9,9,9,3,1,1}$ [42] |
| | [0,0,1,2,0,1,0,0,1,3] | [3,6,9,13,19,25,32,39,28,18,18] | $T_{10,10,10,7,6,6,4,1}$ [96] | $T_{10,10,10,7,6,6,4,1,1,1}$ [96] |
| | [0,0,2,0,1,0,1,1,0,2] | [3,6,9,14,19,25,31,38,28,18,18] | $T_{10,10,10,7,7,5,3,2}$ [108] | $T_{10,10,10,7,7,5,3,2,1,1}$ [108] |
| | [0,1,0,0,3,0,0,0,1,3] | [3,6,10,14,18,25,32,39,28,18,18] | $T_{10,10,10,8,5,5,5,1}$ [60] | $T_{10,10,10,8,5,5,5,1,1,1}$ [60] |
| | [0,1,0,1,0,2,0,1,0,2] | [3,6,10,14,19,24,31,38,28,18,18] | $T_{10,10,10,8,6,4,4,2}$ [122] | $T_{10,10,10,8,6,4,4,2,1,1}$ [121] |
| | [0,1,1,0,0,0,3,0,0,2] | [3,6,10,15,20,25,30,38,28,18,18] | $T_{10,10,10,8,7,3,3,3}$ [60] | $T_{10,10,10,8,7,3,3,3,1,1}$ [60] |
| | [0,3,1,0,0,0,0,1,1,3] | [2,4,9,15,21,27,33,39,28,18,18] | $T_{10,10,8,8,8,7,2,1}$ [72] | $T_{10,10,8,8,8,7,2,1,1,1}$ [72] |
| | [1,0,0,0,1,1,2,0,0,2] | [3,7,11,15,19,24,30,38,28,18,18] | $T_{10,10,10,9,5,4,3,3}$ [80] | $T_{10,10,10,9,5,4,3,3,1,1}$ [80] |
| | [1,1,1,0,1,1,0,0,1,3] | [2,5,9,14,19,25,32,39,28,18,18] | $T_{10,10,9,8,7,5,4,1}$ [192] | $T_{10,10,9,8,7,5,4,1,1,1}$ [192] |
| | [1,1,1,1,0,0,0,2,0,2] | [2,5,9,14,20,26,32,38,28,18,18] | $T_{10,10,9,8,7,6,2,2}$ [120] | $T_{10,10,9,8,7,6,2,2,1,1}$ [120] |
| | [1,2,0,0,0,1,1,1,0,2] | [2,5,10,15,20,25,31,38,28,18,18] | $T_{10,10,9,8,8,4,3,2}$ [120] | $T_{10,10,9,8,8,4,3,2,1,1}$ [120] |
| | [2,0,0,1,1,0,1,1,0,2] | [2,6,10,14,19,25,31,38,28,18,18] | $T_{10,10,9,9,6,5,3,2}$ [144] | $T_{10,10,9,9,6,5,3,2,1,1}$ [144] |
| | [2,3,0,0,0,0,0,0,2,4] | [1,4,10,16,22,28,34,40,28,18,18] | $T_{10,9,9,8,8,8,1,1}$ [32] | $T_{10,9,9,8,8,8,1,1,1,1}$ [32] |
| | [3,0,2,0,0,0,0,1,1,3] | [1,5,9,15,21,27,33,39,28,18,18] | $T_{10,9,9,9,7,7,2,1}$ [72] | $T_{10,9,9,9,7,7,2,1,1,1}$ [72] |
| | [3,1,0,0,1,0,1,0,1,3] | [1,5,10,15,20,26,32,39,28,18,18] | $T_{10,9,9,9,8,5,3,1}$ [144] | $T_{10,9,9,9,8,5,3,1,1,1}$ [144] |
| | [4,0,0,0,0,1,0,2,0,2] | [1,6,11,16,21,26,32,38,28,18,18] | $T_{10,9,9,9,9,4,2,2}$ [54] | $T_{10,9,9,9,9,4,2,2,1,1}$ [54] |
| | [0,3,0,1,0,1,0,0,0,4] | [2,4,9,14,20,26,33,40,29,18,18] | $T_{10,10,8,8,8,6,4}$ [68] | $T_{10,10,8,8,8,6,4,1,1,1,1}$ [67] |
| | [1,0,3,0,0,1,0,0,0,4] | [2,5,8,14,20,26,33,40,29,18,18] | $T_{10,10,9,7,7,7,4}$ [60] | $T_{10,10,9,7,7,7,4,1,1,1,1}$ [60] |
| | [1,1,0,2,1,0,0,0,0,4] | [2,5,9,13,19,26,33,40,29,18,18] | $T_{10,10,9,8,6,6,5}$ [72] | $T_{10,10,9,8,6,6,5,1,1,1,1}$ [72] |
| | [2,2,1,0,0,0,1,0,0,4] | [1,4,9,15,21,27,33,40,29,18,18] | $T_{10,9,9,8,8,7,3}$ [80] | $T_{10,9,9,8,8,7,3,1,1,1,1}$ [80] |
| | [3,0,1,1,0,1,0,0,0,4] | [1,5,9,14,20,26,33,40,29,18,18] | $T_{10,9,9,9,7,6,4}$ [90] | $T_{10,9,9,9,7,6,4,1,1,1,1}$ [90] |
| | [5,1,0,0,0,0,0,0,1,5] | [0,5,11,17,23,29,35,41,29,18,18] | $T_{9,9,9,9,9,8,1}$ [32] | $T_{9,9,9,9,9,8,1,1,1,1,1}$ [32] |
| | [0,1,0,0,0,0,0,1,6,0] | [4,8,13,18,23,28,33,38,25,18,19] | $T_{10,10,10,10,8,2,1,1,1,1,1,1}$ [31] | $T_{10,10,10,10,8,2}$ [32] |
| | [0,1,1,0,1,0,0,1,4,0] | [3,6,10,15,20,26,32,38,26,18,19] | $T_{10,10,10,8,7,5,2,1,1,1,1}$ [108] | $T_{10,10,10,8,7,5,2}$ [108] |
| | [1,0,0,1,0,1,1,0,4,0] | [3,7,11,15,20,25,31,38,26,18,19] | $T_{10,10,10,9,6,4,3,1,1,1,1}$ [96] | $T_{10,10,10,9,6,4,3}$ [96] |
| | [2,0,1,1,0,0,0,0,5,1] | [2,6,10,15,21,27,33,39,26,18,19] | $T_{10,10,9,9,7,6,1,1,1,1,1}$ [72] | $T_{10,10,9,9,7,6,1}$ [72] |
| | [2,1,0,0,0,1,0,1,4,0] | [2,6,11,16,21,26,32,38,26,18,19] | $T_{10,10,9,9,8,4,2,1,1,1,1}$ [90] | $T_{10,10,9,9,8,4,2}$ [90] |
| | [0,0,1,2,0,1,0,0,3,1] | [3,6,9,13,19,25,32,39,27,18,19] | $T_{10,10,10,7,6,6,4,1,1,1}$ [96] | $T_{10,10,10,7,6,6,4,1}$ [96] |
| | [0,0,2,0,1,0,1,1,2,0] | [3,6,9,14,19,25,31,38,27,18,19] | $T_{10,10,10,7,7,5,3,2,1,1}$ [108] | $T_{10,10,10,7,7,5,3,2}$ [108] |
| | [0,1,0,0,3,0,0,0,3,1] | [3,6,10,14,18,25,32,39,27,18,19] | $T_{10,10,10,8,5,5,5,1,1,1}$ [60] | $T_{10,10,10,8,5,5,5,1}$ [60] |
| | [0,1,0,1,0,2,0,1,2,0] | [3,6,10,14,19,24,31,38,27,18,19] | $T_{10,10,10,8,6,4,4,2,1,1}$ [121] | $T_{10,10,10,8,6,4,4,2}$ [122] |
| | [0,1,1,0,0,0,3,0,2,0] | [3,6,10,15,20,25,30,38,27,18,19] | $T_{10,10,10,8,7,3,3,3,1,1}$ [60] | $T_{10,10,10,8,7,3,3,3}$ [60] |
| | [0,3,1,0,0,0,0,1,3,1] | [2,4,9,15,21,27,33,39,27,18,19] | $T_{10,10,8,8,8,7,2,1,1,1}$ [72] | $T_{10,10,8,8,8,7,2,1}$ [72] |
| | [1,0,0,0,1,1,2,0,2,0] | [3,7,11,15,19,24,30,38,27,18,19] | $T_{10,10,10,9,5,4,3,3,1,1}$ [80] | $T_{10,10,10,9,5,4,3,3}$ [80] |
| | [1,1,1,0,1,1,0,0,3,1] | [2,5,9,14,19,25,32,39,27,18,19] | $T_{10,10,9,8,7,5,4,1,1,1}$ [192] | $T_{10,10,9,8,7,5,4,1}$ [192] |
| | [1,1,1,1,0,0,0,2,2,0] | [2,5,9,14,20,26,32,38,27,18,19] | $T_{10,10,9,8,7,6,2,2,1,1}$ [120] | $T_{10,10,9,8,7,6,2,2}$ [120] |
| | [1,2,0,0,0,1,1,1,2,0] | [2,5,10,15,20,25,31,38,27,18,19] | $T_{10,10,9,8,8,4,3,2,1,1}$ [120] | $T_{10,10,9,8,8,4,3,2}$ [120] |
| | [2,0,0,1,1,0,1,1,2,0] | [2,6,10,14,19,25,31,38,27,18,19] | $T_{10,10,9,9,6,5,3,2,1,1}$ [144] | $T_{10,10,9,9,6,5,3,2}$ [144] |
| | [2,3,0,0,0,0,0,0,4,2] | [1,4,10,16,22,28,34,40,27,18,19] | $T_{10,9,9,8,8,8,1,1,1,1}$ [32] | $T_{10,9,9,8,8,8,1,1}$ [32] |
| | [3,0,2,0,0,0,0,1,3,1] | [1,5,9,15,21,27,33,39,27,18,19] | $T_{10,9,9,9,7,7,2,1,1,1}$ [72] | $T_{10,9,9,9,7,7,2,1}$ [72] |
| | [3,1,0,0,1,0,1,0,3,1] | [1,5,10,15,20,26,32,39,27,18,19] | $T_{10,9,9,9,8,5,3,1,1,1}$ [144] | $T_{10,9,9,9,8,5,3,1}$ [144] |
| | [4,0,0,0,0,1,0,2,2,0] | [1,6,11,16,21,26,32,38,27,18,19] | $T_{10,9,9,9,9,4,2,2,1,1}$ [54] | $T_{10,9,9,9,9,4,2,2}$ [54] |
| | [0,0,0,3,1,0,1,0,0,2] | [3,6,9,12,18,25,32,40,29,18,19] | $T_{10,10,10,6,6,6,5,3}$ [60] | $T_{10,10,10,6,6,6,5,3,1,1}$ [60] |
| | [0,1,3,1,0,0,0,0,1,3] | [2,4,7,13,20,27,34,41,29,18,19] | $T_{10,10,8,7,7,7,6,1}$ [72] | $T_{10,10,8,7,7,7,6,1,1,1}$ [72] |
| | [0,2,1,1,0,1,1,0,0,2] | [2,4,8,13,19,25,32,40,29,18,19] | $T_{10,10,8,8,7,6,4,3}$ [144] | $T_{10,10,8,8,7,6,4,3,1,1}$ [144] |
| | [1,0,1,3,0,0,0,1,0,2] | [2,5,8,12,19,26,33,40,29,18,19] | $T_{10,10,9,7,6,6,6,2}$ [90] | $T_{10,10,9,7,6,6,6,2,1,1}$ [90] |
| | [1,0,2,0,2,0,1,0,0,2] | [2,5,8,13,18,25,32,40,29,18,19] | $T_{10,10,9,7,7,5,5,3}$ [108] | $T_{10,10,9,7,7,5,5,3,1,1}$ [108] |
| | [1,1,0,1,1,2,0,0,0,2] | [2,5,9,13,18,24,32,40,29,18,19] | $T_{10,10,9,8,6,5,4,4}$ [120] | $T_{10,10,9,8,6,5,4,4,1,1}$ [120] |
| | [1,3,1,0,1,0,0,0,1,3] | [1,3,8,14,20,27,34,41,29,18,19] | $T_{10,9,8,8,8,7,5,1}$ [120] | $T_{10,9,8,8,8,7,5,1,1,1}$ [120] |
| | [1,4,0,0,0,0,1,1,0,2] | [1,3,9,15,21,27,33,40,29,18,19] | $T_{10,9,8,8,8,8,3,2}$ [72] | $T_{10,9,8,8,8,8,3,2,1,1}$ [72] |
| | [2,1,1,1,1,0,0,1,0,2] | [1,4,8,13,19,26,33,40,29,18,19] | $T_{10,9,9,8,7,6,5,2}$ [192] | $T_{10,9,9,8,7,6,5,2,1,1}$ [192] |
| | [2,1,2,0,0,0,2,0,0,2] | [1,4,8,14,20,26,32,40,29,18,19] | $T_{10,9,9,8,7,7,3,3}$ [80] | $T_{10,9,9,8,7,7,3,3,1,1}$ [80] |
| | [2,2,0,0,1,1,1,0,0,2] | [1,4,9,14,19,25,32,40,29,18,19] | $T_{10,9,9,8,8,5,4,3}$ [128] | $T_{10,9,9,8,8,5,4,3,1,1}$ [128] |
| | [3,0,0,2,0,1,1,0,0,2] | [1,5,9,13,19,25,32,40,29,18,19] | $T_{10,9,9,9,6,6,4,3}$ [96] | $T_{10,9,9,9,6,6,4,3,1,1}$ [96] |
| | [4,1,0,1,1,0,0,0,1,3] | [0,4,9,14,20,27,34,41,29,18,19] | $T_{9,9,9,9,8,6,5,1}$ [120] | $T_{9,9,9,9,8,6,5,1,1,1}$ [120] |
| | [4,1,1,0,0,0,1,1,0,2] | [0,4,9,15,21,27,33,40,29,18,19] | $T_{9,9,9,9,8,7,3,2}$ [120] | $T_{9,9,9,9,8,7,3,2,1,1}$ [120] |
| | [5,0,0,0,1,1,0,1,0,2] | [0,5,10,15,20,26,33,40,29,18,19] | $T_{9,9,9,9,9,5,4,2}$ [90] | $T_{9,9,9,9,9,5,4,2,1,1}$ [90] |
| | [3,3,0,0,1,0,0,0,0,4] | [0,3,9,15,21,28,35,42,30,18,19] | $T_{9,9,9,8,8,8,5}$ [48] | $T_{9,9,9,8,8,8,5,1,1,1,1}$ [48] |
| | [4,0,2,1,0,0,0,0,0,4] | [0,4,8,14,21,28,35,42,30,18,19] | $T_{9,9,9,9,7,7,6}$ [42] | $T_{9,9,9,9,7,7,6,1,1,1,1}$ [42] |
| | [1,2,1,0,0,0,0,0,6,0] | [2,5,10,16,22,28,34,40,26,18,20] | $T_{10,10,9,8,8,7,1,1,1,1,1,1}$ [32] | $T_{10,10,9,8,8,7}$ [32] |
| | [0,3,0,1,0,1,0,0,4,0] | [2,4,9,14,20,26,33,40,27,18,20] | $T_{10,10,8,8,8,6,4,1,1,1,1}$ [67] | $T_{10,10,8,8,8,6,4}$ [68] |
| | [1,1,0,2,1,0,0,0,4,0] | [2,5,9,13,19,26,33,40,27,18,20] | $T_{10,10,9,8,6,6,5,1,1,1,1}$ [72] | $T_{10,10,9,8,6,6,5}$ [72] |
| | [2,2,1,0,0,0,1,0,4,0] | [1,4,9,15,21,27,33,40,27,18,20] | $T_{10,9,9,8,8,7,3,1,1,1,1}$ [80] | $T_{10,9,9,8,8,7,3}$ [80] |
| | [3,0,1,1,0,1,0,0,4,0] | [1,5,9,14,20,26,33,40,27,18,20] | $T_{10,9,9,9,7,6,4,1,1,1,1}$ [90] | $T_{10,9,9,9,7,6,4}$ [90] |
| | [5,1,0,0,0,0,0,0,5,1] | [0,5,11,17,23,29,35,41,27,18,20] | $T_{9,9,9,9,9,8,1,1,1,1,1}$ [32] | $T_{9,9,9,9,9,8,1}$ [32] |
| | [0,0,0,3,1,0,1,0,2,0] | [3,6,9,12,18,25,32,40,28,18,20] | $T_{10,10,10,6,6,6,5,3,1,1}$ [60] | $T_{10,10,10,6,6,6,5,3}$ [60] |
| | [0,2,1,1,0,1,1,0,2,0] | [2,4,8,13,19,25,32,40,28,18,20] | $T_{10,10,8,8,7,6,4,3,1,1}$ [144] | $T_{10,10,8,8,7,6,4,3}$ [144] |
| | [1,0,1,3,0,0,0,1,2,0] | [2,5,8,12,19,26,33,40,28,18,20] | $T_{10,10,9,7,6,6,6,2,1,1}$ [90] | $T_{10,10,9,7,6,6,6,2}$ [90] |
| | [1,0,2,0,2,0,1,0,2,0] | [2,5,8,13,18,25,32,40,28,18,20] | $T_{10,10,9,7,7,5,5,3,1,1}$ [108] | $T_{10,10,9,7,7,5,5,3}$ [108] |
| | [1,1,0,1,1,2,0,0,2,0] | [2,5,9,13,18,24,32,40,28,18,20] | $T_{10,10,9,8,6,5,4,4,1,1}$ [120] | $T_{10,10,9,8,6,5,4,4}$ [120] |
| | [1,3,1,0,1,0,0,0,3,1] | [1,3,8,14,20,27,34,41,28,18,20] | $T_{10,9,8,8,8,7,5,1,1,1}$ [120] | $T_{10,9,8,8,8,7,5,1}$ [120] |

| | | | | |
|---|---|---|---|---|
| | [1,4,0,0,0,0,1,1,2,0] | [1,3,9,15,21,27,33,40,28,18,20] | $T_{10,9,8,8,8,8,3,2,1,1}$ [72] | $T_{10,9,8,8,8,8,3,2}$ [72] |
| | [2,1,1,1,1,0,0,1,2,0] | [1,4,8,13,19,26,33,40,28,18,20] | $T_{10,9,9,8,7,6,5,2,1,1}$ [192] | $T_{10,9,9,8,7,6,5,2}$ [192] |
| | [2,1,2,0,0,0,2,0,2,0] | [1,4,8,14,20,26,32,40,28,18,20] | $T_{10,9,9,8,7,7,3,3,1,1}$ [80] | $T_{10,9,9,8,7,7,3,3}$ [80] |
| | [2,2,0,0,1,1,1,0,2,0] | [1,4,9,14,19,25,32,40,28,18,20] | $T_{10,9,9,8,8,5,4,3,1,1}$ [128] | $T_{10,9,9,8,8,5,4,3}$ [128] |
| | [3,0,0,2,0,1,1,0,2,0] | [1,5,9,13,19,25,32,40,28,18,20] | $T_{10,9,9,9,6,6,4,3,1,1}$ [96] | $T_{10,9,9,9,6,6,4,3}$ [96] |
| | [4,1,0,1,1,0,0,0,3,1] | [0,4,9,14,20,27,34,41,28,18,20] | $T_{9,9,9,9,8,6,5,1,1,1}$ [120] | $T_{9,9,9,9,8,6,5,1}$ [120] |
| | [4,1,1,0,0,0,1,1,2,0] | [0,4,9,15,21,27,33,40,28,18,20] | $T_{9,9,9,9,8,7,3,2,1,1}$ [120] | $T_{9,9,9,9,8,7,3,2}$ [120] |
| | [5,0,0,0,1,1,0,1,2,0] | [0,5,10,15,20,26,33,40,28,18,20] | $T_{9,9,9,9,9,5,4,2,1,1}$ [90] | $T_{9,9,9,9,9,5,4,2}$ [90] |
| | [0,1,2,1,2,0,0,0,0,2] | [2,4,7,12,18,26,34,42,30,18,20] | $T_{10,10,8,7,7,6,5,5}$ [72] | $T_{10,10,8,7,7,6,5,5,1,1}$ [72] |
| | [0,5,0,1,0,0,0,1,0,2] | [1,2,8,14,21,28,35,42,30,18,20] | $T_{10,8,8,8,8,8,6,2}$ [68] | $T_{10,8,8,8,8,8,6,2,1,1}$ [67] |
| | [1,2,2,0,1,1,0,0,0,2] | [1,3,7,13,19,26,34,42,30,18,20] | $T_{10,9,8,8,7,7,5,4}$ [120] | $T_{10,9,8,8,7,7,5,4,1,1}$ [120] |
| | [2,0,2,2,0,1,0,0,0,2] | [1,4,7,12,19,26,34,42,30,18,20] | $T_{10,9,9,7,7,6,6,4}$ [90] | $T_{10,9,9,7,7,6,6,4,1,1}$ [90] |
| | [2,1,0,2,2,0,0,0,0,2] | [1,4,8,12,18,26,34,42,30,18,20] | $T_{10,9,9,8,6,6,5,5}$ [72] | $T_{10,9,9,8,6,6,5,5,1,1}$ [72] |
| | [2,4,1,0,0,0,0,0,1,3] | [0,2,8,15,22,29,36,43,30,18,20] | $T_{9,9,8,8,8,8,7,1}$ [56] | $T_{9,9,8,8,8,8,7,1,1,1}$ [56] |
| | [3,1,3,0,0,0,0,1,0,2] | [0,3,7,14,21,28,35,42,30,18,20] | $T_{9,9,9,8,7,7,7,2}$ [72] | $T_{9,9,9,8,7,7,7,2,1,1}$ [72] |
| | [3,2,0,2,0,0,1,0,0,2] | [0,3,8,13,20,27,34,42,30,18,20] | $T_{9,9,9,8,8,6,6,3}$ [96] | $T_{9,9,9,8,8,6,6,3,1,1}$ [96] |
| | [3,2,1,0,0,2,0,0,0,2] | [0,3,8,14,20,26,34,42,30,18,20] | $T_{9,9,9,8,8,7,4,4}$ [80] | $T_{9,9,9,8,8,7,4,4,1,1}$ [80] |
| | [4,0,1,1,1,1,0,0,0,2] | [0,4,8,13,19,26,34,42,30,18,20] | $T_{9,9,9,9,7,6,5,4}$ [120] | $T_{9,9,9,9,7,6,5,4,1,1}$ [120] |
| | [3,3,0,0,1,0,0,0,4,0] | [0,3,9,15,21,28,35,42,28,18,21] | $T_{9,9,9,8,8,8,5,1,1,1,1}$ [48] | $T_{9,9,9,8,8,8,5}$ [48] |
| | [4,0,2,1,0,0,0,0,4,0] | [0,4,8,14,21,28,35,42,28,18,21] | $T_{9,9,9,9,7,7,6,1,1,1,1}$ [42] | $T_{9,9,9,9,7,7,6}$ [42] |
| | [0,1,2,1,2,0,0,0,2,0] | [2,4,7,12,18,26,34,42,29,18,21] | $T_{10,10,8,7,7,6,5,5,1,1}$ [72] | $T_{10,10,8,7,7,6,5,5}$ [72] |
| | [0,5,0,1,0,0,0,1,2,0] | [1,2,8,14,21,28,35,42,29,18,21] | $T_{10,8,8,8,8,8,6,2,1,1}$ [67] | $T_{10,8,8,8,8,8,6,2}$ [68] |
| | [1,2,2,0,1,1,0,0,2,0] | [1,3,7,13,19,26,34,42,29,18,21] | $T_{10,9,8,8,7,7,5,4,1,1}$ [120] | $T_{10,9,8,8,7,7,5,4}$ [120] |
| | [2,0,2,2,0,1,0,0,2,0] | [1,4,7,12,19,26,34,42,29,18,21] | $T_{10,9,9,7,7,6,6,4,1,1}$ [90] | $T_{10,9,9,7,7,6,6,4}$ [90] |
| | [2,1,0,2,2,0,0,0,2,0] | [1,4,8,12,18,26,34,42,29,18,21] | $T_{10,9,9,8,6,6,5,5,1,1}$ [72] | $T_{10,9,9,8,6,6,5,5}$ [72] |
| | [2,4,1,0,0,0,0,0,3,1] | [0,2,8,15,22,29,36,43,29,18,21] | $T_{9,9,8,8,8,8,7,1,1,1}$ [56] | $T_{9,9,8,8,8,8,7,1}$ [56] |
| | [3,1,3,0,0,0,0,1,2,0] | [0,3,7,14,21,28,35,42,29,18,21] | $T_{9,9,9,8,7,7,7,2,1,1}$ [72] | $T_{9,9,9,8,7,7,7,2}$ [72] |
| | [3,2,0,2,0,0,1,0,2,0] | [0,3,8,13,20,27,34,42,29,18,21] | $T_{9,9,9,8,8,6,6,3,1,1}$ [96] | $T_{9,9,9,8,8,6,6,3}$ [96] |
| | [3,2,1,0,0,2,0,0,2,0] | [0,3,8,14,20,26,34,42,29,18,21] | $T_{9,9,9,8,8,7,4,4,1,1}$ [80] | $T_{9,9,9,8,8,7,4,4}$ [80] |
| | [4,0,1,1,1,1,0,0,2,0] | [0,4,8,13,19,26,34,42,29,18,21] | $T_{9,9,9,9,7,6,5,4,1,1}$ [120] | $T_{9,9,9,9,7,6,5,4}$ [120] |
| | [1,1,3,2,0,0,0,0,0,2] | [1,3,6,12,20,28,36,44,31,18,21] | $T_{10,9,8,7,7,7,6,6}$ [56] | $T_{10,9,8,7,7,7,6,6,1,1}$ [56] |
| | [2,3,1,1,1,0,0,0,0,2] | [0,2,7,13,20,28,36,44,31,18,21] | $T_{9,9,8,8,8,7,6,5}$ [96] | $T_{9,9,8,8,8,7,6,5,1,1}$ [96] |
| | [3,1,1,3,0,0,0,0,0,2] | [0,3,7,12,20,28,36,44,31,18,21] | $T_{9,9,9,8,7,6,6,6}$ [56] | $T_{9,9,9,8,7,6,6,6,1,1}$ [56] |
| | [1,1,3,2,0,0,0,0,2,0] | [1,3,6,12,20,28,36,44,30,18,22] | $T_{10,9,8,7,7,7,6,6,1,1}$ [56] | $T_{10,9,8,7,7,7,6,6}$ [56] |
| | [2,3,1,1,1,0,0,0,2,0] | [0,2,7,13,20,28,36,44,30,18,22] | $T_{9,9,8,8,8,7,6,5,1,1}$ [96] | $T_{9,9,8,8,8,7,6,5}$ [96] |
| | [3,1,1,3,0,0,0,0,2,0] | [0,3,7,12,20,28,36,44,30,18,22] | $T_{9,9,9,8,7,6,6,6,1,1}$ [56] | $T_{9,9,9,8,7,6,6,6}$ [56] |
| | [1,5,1,1,0,0,0,0,0,2] | [0,1,7,14,22,30,38,46,32,18,22] | $T_{9,8,8,8,8,8,7,6}$ [56] | $T_{9,8,8,8,8,8,7,6,1,1}$ [56] |
| | [1,5,1,1,0,0,0,0,2,0] | [0,1,7,14,22,30,38,46,31,18,23] | $T_{9,8,8,8,8,8,7,6,1,1}$ [56] | $T_{9,8,8,8,8,8,7,6}$ [56] |
| 19 | [0,0,1,0,1,0,0,0,5,2] | [4,8,12,17,22,28,34,40,27,19,19] | $U_{10,10,10,10,7,5,1,1,1,1,1}$ [60] | $U_{10,10,10,10,7,5,1,1}$ [60] |
| | [0,1,0,0,0,0,1,1,4,1] | [4,8,13,18,23,28,33,39,27,19,19] | $U_{10,10,10,10,8,3,2,1,1,1,1}$ [72] | $U_{10,10,10,10,8,3,2,1}$ [72] |
| | [2,0,0,0,0,1,0,0,5,2] | [3,8,13,18,23,28,34,40,27,19,19] | $U_{10,10,10,9,9,4,1,1,1,1,1}$ [48] | $U_{10,10,10,9,9,4,1,1}$ [48] |
| | [0,0,0,0,2,1,0,0,3,2] | [4,8,12,16,20,26,33,40,28,19,19] | $U_{10,10,10,10,5,5,4,1,1,1}$ [48] | $U_{10,10,10,10,5,5,4,1,1}$ [48] |
| | [0,0,0,1,0,1,1,1,2,1] | [4,8,12,16,21,26,32,39,28,19,19] | $U_{10,10,10,10,6,4,3,2,1,1}$ [120] | $U_{10,10,10,10,6,4,3,2,1}$ [120] |
| | [0,1,0,0,0,0,0,4,1,0] | [4,8,13,18,23,28,33,38,28,19,19] | $U_{10,10,10,10,8,2,2,2,2,1}$ [31] | $U_{10,10,10,10,8,2,2,2,2}$ [32] |
| | [0,1,2,0,0,0,0,1,3,2] | [3,6,10,16,22,28,34,40,28,19,19] | $U_{10,10,10,8,7,7,2,1,1,1}$ [72] | $U_{10,10,10,8,7,7,2,1,1}$ [72] |
| | [0,2,0,0,1,0,1,0,3,2] | [3,6,11,16,21,27,33,40,28,19,19] | $U_{10,10,10,8,8,5,3,1,1,1}$ [108] | $U_{10,10,10,8,8,5,3,1,1}$ [108] |
| | [1,0,0,2,0,0,1,0,3,2] | [3,7,11,15,21,27,33,40,28,19,19] | $U_{10,10,10,9,6,6,3,1,1,1}$ [96] | $U_{10,10,10,9,6,6,3,1,1}$ [96] |
| | [1,0,1,0,0,2,0,0,3,2] | [3,7,11,16,21,26,33,40,28,19,19] | $U_{10,10,10,9,7,4,4,1,1,1}$ [96] | $U_{10,10,10,9,7,4,4,1,1}$ [96] |
| | [1,0,1,0,1,0,0,2,2,1] | [3,7,11,16,21,27,33,39,28,19,19] | $U_{10,10,10,9,7,5,2,2,1,1}$ [144] | $U_{10,10,10,9,7,5,2,2,1}$ [144] |
| | [1,1,0,0,0,0,2,1,2,1] | [3,7,12,17,22,27,32,39,28,19,19] | $U_{10,10,10,9,8,3,3,2,1,1}$ [96] | $U_{10,10,10,9,8,3,3,2,1}$ [96] |
| | [2,1,0,1,0,0,0,1,3,2] | [2,6,11,16,22,28,34,40,28,19,19] | $U_{10,10,9,9,8,6,2,1,1,1}$ [120] | $U_{10,10,9,9,8,6,2,1,1}$ [120] |
| | [3,0,0,0,0,1,1,0,3,2] | [2,7,12,17,22,27,33,40,28,19,19] | $U_{10,10,9,9,9,4,3,1,1,1}$ [72] | $U_{10,10,9,9,9,4,3,1,1}$ [72] |
| | [0,0,0,0,1,2,1,0,1,2] | [4,8,12,16,20,25,32,40,29,19,19] | $U_{10,10,10,10,5,4,4,3,1}$ [72] | $U_{10,10,10,10,5,4,4,3,1,1}$ [72] |
| | [0,0,0,0,2,0,1,2,0,1] | [4,8,12,16,20,26,32,39,29,19,19] | $U_{10,10,10,10,5,5,3,2,2}$ [54] | $U_{10,10,10,10,5,5,3,2,2,1}$ [54] |
| | [0,0,3,0,0,1,0,0,2,3] | [3,6,9,15,21,27,34,41,29,19,19] | $U_{10,10,10,7,7,7,4,1,1}$ [64] | $U_{10,10,10,7,7,7,4,1,1,1}$ [64] |
| | [0,1,0,2,1,0,0,0,2,3] | [3,6,10,14,20,27,34,41,29,19,19] | $U_{10,10,10,8,6,6,5,1,1}$ [90] | $U_{10,10,10,8,6,6,5,1,1,1}$ [90] |
| | [0,1,1,0,1,1,0,1,1,2] | [3,6,10,15,20,26,33,40,29,19,19] | $U_{10,10,10,8,7,5,4,2,1}$ [216] | $U_{10,10,10,8,7,5,4,2,1,1}$ [216] |
| | [0,2,0,0,0,1,2,0,1,2] | [3,6,11,16,21,26,32,40,29,19,19] | $U_{10,10,10,8,8,4,3,3,1}$ [90] | $U_{10,10,10,8,8,4,3,3,1,1}$ [90] |
| | [0,2,0,0,1,0,0,3,0,1] | [3,6,11,16,21,27,33,39,29,19,19] | $U_{10,10,10,8,8,5,2,2,2}$ [72] | $U_{10,10,10,8,8,5,2,2,2,1}$ [72] |
| | [1,0,0,1,1,0,2,0,1,2] | [3,7,11,15,20,26,32,40,29,19,19] | $U_{10,10,10,9,6,5,3,3,1}$ [144] | $U_{10,10,10,9,6,5,3,3,1,1}$ [144] |
| | [1,0,0,2,0,0,0,3,0,1] | [3,7,11,15,21,27,33,39,29,19,19] | $U_{10,10,10,9,6,6,2,2,2}$ [60] | $U_{10,10,10,9,6,6,2,2,2,1}$ [60] |
| | [1,0,1,0,0,1,1,2,0,1] | [3,7,11,16,21,26,32,39,29,19,19] | $U_{10,10,10,9,7,4,3,2,2}$ [144] | $U_{10,10,10,9,7,4,3,2,2,1}$ [144] |
| | [1,2,0,1,0,1,0,0,2,3] | [2,5,10,15,21,27,34,41,29,19,19] | $U_{10,10,9,8,8,6,4,1,1}$ [144] | $U_{10,10,9,8,8,6,4,1,1,1}$ [144] |
| | [1,2,1,0,0,0,0,2,1,2] | [2,5,10,16,22,28,34,40,29,19,19] | $U_{10,10,9,8,8,7,2,2,1}$ [96] | $U_{10,10,9,8,8,7,2,2,1,1}$ [96] |
| | [2,0,1,0,2,0,0,0,2,3] | [2,6,10,15,20,27,34,41,29,19,19] | $U_{10,10,9,9,7,5,5,1,1}$ [90] | $U_{10,10,9,9,7,5,5,1,1,1}$ [90] |
| | [2,0,1,1,0,0,1,1,1,2] | [2,6,10,15,21,27,33,40,29,19,19] | $U_{10,10,9,9,7,6,3,2,1}$ [192] | $U_{10,10,9,9,7,6,3,2,1,1}$ [192] |
| | [2,1,0,0,0,2,0,1,1,2] | [2,6,11,16,21,26,33,40,29,19,19] | $U_{10,10,9,9,8,4,4,2,1}$ [120] | $U_{10,10,9,9,8,4,4,2,1,1}$ [120] |
| | [3,0,0,0,0,0,3,0,1,2] | [2,7,12,17,22,27,32,40,29,19,19] | $U_{10,10,9,9,9,3,3,3,1}$ [42] | $U_{10,10,9,9,9,3,3,3,1,1}$ [42] |
| | [3,0,0,0,0,1,0,3,0,1] | [2,7,12,17,22,27,33,39,29,19,19] | $U_{10,10,9,9,9,4,2,2,2}$ [54] | $U_{10,10,9,9,9,4,2,2,2,1}$ [54] |
| | [3,2,0,0,0,0,0,1,2,3] | [1,5,11,17,23,29,35,41,29,19,19] | $U_{10,9,9,9,8,8,2,1,1}$ [56] | $U_{10,9,9,9,8,8,2,1,1,1}$ [56] |
| | [4,0,0,1,0,0,1,0,2,3] | [1,6,11,16,22,28,34,41,29,19,19] | $U_{10,9,9,9,9,6,3,1,1}$ [96] | $U_{10,9,9,9,9,6,3,1,1,1}$ [96] |

| | | | | |
|---|---|---|---|---|
| | [0,0,2,1,1,0,0,1,0,3] | [3,6,9,14,20,27,34,41,30,19,19] | $U_{10,10,10,7,7,6,5,2}$ [96] | $U_{10,10,10,7,7,6,5,2,1,1,1}$ [96] |
| | [0,0,3,0,0,0,2,0,0,3] | [3,6,9,15,21,27,33,41,30,19,19] | $U_{10,10,10,7,7,7,3,3}$ [40] | $U_{10,10,10,7,7,7,3,3,1,1,1}$ [40] |
| | [0,1,0,2,0,1,1,0,0,3] | [3,6,10,14,20,26,33,41,30,19,19] | $U_{10,10,10,8,6,6,4,3}$ [108] | $U_{10,10,10,8,6,6,4,3,1,1,1}$ [108] |
| | [0,4,0,0,0,1,0,0,1,4] | [2,4,10,16,22,28,35,42,30,19,19] | $U_{10,10,8,8,8,8,4,1}$ [60] | $U_{10,10,8,8,8,8,4,1,1,1,1}$ [60] |
| | [1,0,0,0,3,0,1,0,0,3] | [3,7,11,15,19,26,33,41,30,19,19] | $U_{10,10,10,9,5,5,5,3}$ [60] | $U_{10,10,10,9,5,5,5,3,1,1,1}$ [60] |
| | [1,0,0,1,0,3,0,0,0,3] | [3,7,11,15,20,25,33,41,30,19,19] | $U_{10,10,10,9,6,4,4,4}$ [60] | $U_{10,10,10,9,6,4,4,4,1,1,1}$ [60] |
| | [1,1,1,2,0,0,0,0,1,4] | [2,5,9,14,21,28,35,42,30,19,19] | $U_{10,10,9,8,7,6,6,1}$ [96] | $U_{10,10,9,8,7,6,6,1,1,1,1}$ [96] |
| | [1,1,2,0,0,1,0,1,0,3] | [2,5,9,15,21,27,34,41,30,19,19] | $U_{10,10,9,8,7,7,4,2}$ [144] | $U_{10,10,9,8,7,7,4,2,1,1,1}$ [144] |
| | [1,2,0,0,2,0,0,1,0,3] | [2,5,10,15,20,27,34,41,30,19,19] | $U_{10,10,9,8,8,5,5,2}$ [96] | $U_{10,10,9,8,8,5,5,2,1,1,1}$ [96] |
| | [1,2,0,1,0,0,2,0,0,3] | [2,5,10,15,21,27,33,41,30,19,19] | $U_{10,10,9,8,8,6,3,3}$ [96] | $U_{10,10,9,8,8,6,3,3,1,1,1}$ [96] |
| | [2,0,0,2,1,0,0,1,0,3] | [2,6,10,14,20,27,34,41,30,19,19] | $U_{10,10,9,9,6,6,5,2}$ [96] | $U_{10,10,9,9,6,6,5,2,1,1,1}$ [96] |
| | [2,0,1,0,1,1,1,0,0,3] | [2,6,10,15,20,26,33,41,30,19,19] | $U_{10,10,9,9,7,5,4,3}$ [144] | $U_{10,10,9,9,7,5,4,3,1,1,1}$ [144] |
| | [3,1,0,1,1,0,0,0,1,4] | [1,5,10,15,21,28,35,42,30,19,19] | $U_{10,9,9,9,8,6,5,1}$ [120] | $U_{10,9,9,9,8,6,5,1,1,1,1}$ [120] |
| | [3,1,1,0,0,0,1,1,0,3] | [1,5,10,16,22,28,34,41,30,19,19] | $U_{10,9,9,9,8,7,3,2}$ [120] | $U_{10,9,9,9,8,7,3,2,1,1,1}$ [120] |
| | [4,0,0,0,1,1,0,1,0,3] | [1,6,11,16,21,27,34,41,30,19,19] | $U_{10,9,9,9,9,5,4,2}$ [90] | $U_{10,9,9,9,9,5,4,2,1,1,1}$ [90] |
| | [0,3,1,1,0,0,0,0,0,5] | [2,4,9,15,22,29,36,43,31,19,19] | $U_{10,10,8,8,8,7,6}$ [42] | $U_{10,10,8,8,8,7,6,1,1,1,1,1}$ [42] |
| | [2,3,0,0,1,0,0,0,0,5] | [1,4,10,16,22,29,36,43,31,19,19] | $U_{10,9,9,8,8,8,5}$ [48] | $U_{10,9,9,8,8,8,5,1,1,1,1,1}$ [48] |
| | [3,0,2,1,0,0,0,0,0,5] | [1,5,9,15,22,29,36,43,31,19,19] | $U_{10,9,9,9,7,7,6}$ [42] | $U_{10,9,9,9,7,7,6,1,1,1,1,1}$ [42] |
| | [6,0,0,0,0,0,1,0,0,5] | [0,6,12,18,24,30,36,43,31,19,19] | $U_{9,9,9,9,9,9,3}$ [28] | $U_{9,9,9,9,9,9,3,1,1,1,1,1}$ [28] |
| | [0,0,0,2,0,0,0,1,5,0] | [4,8,12,16,22,28,34,40,27,19,20] | $U_{10,10,10,10,6,6,2,1,1,1,1,1}$ [37] | $U_{10,10,10,10,6,6,2}$ [38] |
| | [0,0,1,0,0,1,1,0,5,0] | [4,8,12,17,22,27,33,40,27,19,20] | $U_{10,10,10,10,7,4,3,1,1,1,1,1}$ [64] | $U_{10,10,10,10,7,4,3}$ [64] |
| | [1,0,2,0,0,0,0,0,6,1] | [3,7,11,17,23,29,35,41,27,19,20] | $U_{10,10,10,9,7,7,1,1,1,1,1,1}$ [42] | $U_{10,10,10,9,7,7,1}$ [42] |
| | [1,1,0,0,1,0,0,1,5,0] | [3,7,12,17,22,28,34,40,27,19,20] | $U_{10,10,10,9,8,5,2,1,1,1,1,1}$ [96] | $U_{10,10,10,9,8,5,2}$ [96] |
| | [2,0,0,0,0,0,2,0,5,0] | [3,8,13,18,23,28,33,40,27,19,20] | $U_{10,10,10,9,9,3,3,1,1,1,1,1}$ [28] | $U_{10,10,10,9,9,3,3}$ [28] |
| | [0,0,0,0,2,0,2,0,3,0] | [4,8,12,16,20,26,32,40,28,19,20] | $U_{10,10,10,10,5,5,3,3,1,1,1}$ [36] | $U_{10,10,10,10,5,5,3,3}$ [36] |
| | [0,1,1,0,2,0,0,0,4,1] | [3,6,10,15,20,27,34,41,28,19,20] | $U_{10,10,10,8,7,5,5,1,1,1,1}$ [90] | $U_{10,10,10,8,7,5,5,1}$ [90] |
| | [0,1,1,1,0,0,1,1,3,0] | [3,6,10,15,21,27,33,40,28,19,20] | $U_{10,10,10,8,7,6,3,2,1,1,1}$ [144] | $U_{10,10,10,8,7,6,3,2}$ [144] |
| | [0,2,0,0,0,2,0,1,3,0] | [3,6,11,16,21,26,33,40,28,19,20] | $U_{10,10,10,8,8,4,4,2,1,1,1}$ [67] | $U_{10,10,10,8,8,4,4,2}$ [68] |
| | [1,0,0,1,1,1,0,1,3,0] | [3,7,11,15,20,26,33,40,28,19,20] | $U_{10,10,10,9,6,5,4,2,1,1,1}$ [144] | $U_{10,10,10,9,6,5,4,2}$ [144] |
| | [1,0,1,0,0,1,2,0,3,0] | [3,7,11,16,21,26,32,40,28,19,20] | $U_{10,10,10,9,7,4,3,3,1,1,1}$ [96] | $U_{10,10,10,9,7,4,3,3}$ [96] |
| | [1,2,1,0,0,0,1,0,4,1] | [2,5,10,16,22,28,34,41,28,19,20] | $U_{10,10,9,8,8,7,3,1,1,1,1}$ [120] | $U_{10,10,9,8,8,7,3,1}$ [120] |
| | [2,0,1,1,0,1,0,0,4,1] | [2,6,10,15,21,27,34,41,28,19,20] | $U_{10,10,9,9,7,6,4,1,1,1,1}$ [144] | $U_{10,10,9,9,7,6,4,1}$ [144] |
| | [2,0,2,0,0,0,0,2,3,0] | [2,6,10,16,22,28,34,40,28,19,20] | $U_{10,10,9,9,7,7,2,2,1,1,1}$ [54] | $U_{10,10,9,9,7,7,2,2}$ [54] |
| | [2,1,0,0,1,0,1,1,3,0] | [2,6,11,16,21,27,33,40,28,19,20] | $U_{10,10,9,9,8,5,3,2,1,1,1}$ [144] | $U_{10,10,9,9,8,5,3,2}$ [144] |
| | [4,0,1,0,0,0,0,1,4,1] | [1,6,11,17,23,29,35,41,28,19,20] | $U_{10,9,9,9,9,7,2,1,1,1,1}$ [72] | $U_{10,9,9,9,9,7,2,1}$ [72] |
| | [0,0,0,1,0,0,4,0,1,0] | [4,8,12,16,21,26,31,40,29,19,20] | $U_{10,10,10,10,6,3,3,3,3,1}$ [40] | $U_{10,10,10,10,6,3,3,3,3}$ [40] |
| | [0,0,2,1,0,1,1,0,2,1] | [3,6,9,14,20,26,33,41,29,19,20] | $U_{10,10,10,7,7,6,4,3,1,1}$ [144] | $U_{10,10,10,7,7,6,4,3,1}$ [144] |
| | [0,0,3,0,0,0,1,2,1,0] | [3,6,9,15,21,27,33,40,29,19,20] | $U_{10,10,10,7,7,7,3,2,2,1}$ [60] | $U_{10,10,10,7,7,7,3,2,2}$ [60] |
| | [0,1,0,1,2,0,1,0,2,1] | [3,6,10,14,19,26,33,41,29,19,20] | $U_{10,10,10,8,6,5,5,3,1,1}$ [162] | $U_{10,10,10,8,6,5,5,3,1}$ [162] |
| | [0,1,0,2,0,1,0,2,1,0] | [3,6,10,14,20,26,33,40,29,19,20] | $U_{10,10,10,8,6,6,4,2,2,1}$ [121] | $U_{10,10,10,8,6,6,4,2,2}$ [122] |
| | [0,1,1,0,0,3,0,0,2,1] | [3,6,10,15,20,25,33,41,29,19,20] | $U_{10,10,10,8,7,4,4,4,1,1}$ [96] | $U_{10,10,10,8,7,4,4,4,1}$ [96] |
| | [0,1,1,0,1,0,2,1,1,0] | [3,6,10,15,20,26,32,40,29,19,20] | $U_{10,10,10,8,7,5,3,3,2,1}$ [162] | $U_{10,10,10,8,7,5,3,3,2}$ [162] |
| | [0,3,1,0,1,0,0,0,3,2] | [2,4,9,15,21,28,35,42,29,19,20] | $U_{10,10,8,8,8,7,5,1,1,1}$ [90] | $U_{10,10,8,8,8,7,5,1,1}$ [90] |
| | [0,4,0,0,0,0,1,1,2,1] | [2,4,10,16,22,28,34,41,29,19,20] | $U_{10,10,8,8,8,8,3,2,1,1}$ [72] | $U_{10,10,8,8,8,8,3,2,1}$ [72] |
| | [1,0,0,0,2,2,0,0,2,1] | [3,7,11,15,19,25,33,41,29,19,20] | $U_{10,10,10,9,5,5,4,4,1,1}$ [80] | $U_{10,10,10,9,5,5,4,4,1}$ [80] |
| | [1,0,0,0,3,0,0,2,1,0] | [3,7,11,15,19,26,33,40,29,19,20] | $U_{10,10,10,9,5,5,5,2,2,1}$ [60] | $U_{10,10,10,9,5,5,5,2,2}$ [60] |
| | [1,0,0,1,0,2,1,1,1,0] | [3,7,11,15,20,25,32,40,29,19,20] | $U_{10,10,10,9,6,4,4,3,2,1}$ [144] | $U_{10,10,10,9,6,4,4,3,2}$ [144] |
| | [1,1,1,1,1,0,0,1,2,1] | [2,5,9,14,20,27,34,41,29,19,20] | $U_{10,10,9,8,7,6,5,2,1,1}$ [256] | $U_{10,10,9,8,7,6,5,2,1}$ [256] |
| | [1,1,2,0,0,0,2,0,2,1] | [2,5,9,15,21,27,33,41,29,19,20] | $U_{10,10,9,8,7,7,3,3,1,1}$ [120] | $U_{10,10,9,8,7,7,3,3,1}$ [120] |
| | [1,2,0,0,1,1,1,0,2,1] | [2,5,10,15,20,26,33,41,29,19,20] | $U_{10,10,9,8,8,5,4,3,1,1}$ [192] | $U_{10,10,9,8,8,5,4,3,1}$ [192] |
| | [1,2,0,1,0,0,1,2,1,0] | [2,5,10,15,21,27,33,40,29,19,20] | $U_{10,10,9,8,8,6,3,2,2,1}$ [144] | $U_{10,10,9,8,8,6,3,2,2}$ [144] |
| | [2,0,0,2,0,1,1,0,2,1] | [2,6,10,14,20,26,33,41,29,19,20] | $U_{10,10,9,9,6,6,4,3,1,1}$ [144] | $U_{10,10,9,9,6,6,4,3,1}$ [144] |
| | [2,0,1,0,1,1,0,2,1,0] | [2,6,10,15,20,26,33,40,29,19,20] | $U_{10,10,9,9,7,5,4,2,2,1}$ [162] | $U_{10,10,9,9,7,5,4,2,2}$ [162] |
| | [2,1,0,0,0,1,2,1,1,0] | [2,6,11,16,21,26,32,40,29,19,20] | $U_{10,10,9,9,8,4,3,3,2,1}$ [120] | $U_{10,10,9,9,8,4,3,3,2}$ [120] |
| | [2,3,0,0,0,1,0,0,3,2] | [1,4,10,16,22,28,35,42,29,19,20] | $U_{10,9,9,8,8,8,4,1,1,1}$ [80] | $U_{10,9,9,8,8,8,4,1,1}$ [80] |
| | [3,0,2,0,1,0,0,0,3,2] | [1,5,9,15,21,28,35,42,29,19,20] | $U_{10,9,9,9,7,7,5,1,1,1}$ [90] | $U_{10,9,9,9,7,7,5,1,1}$ [90] |
| | [3,1,0,1,0,1,0,1,2,1] | [1,5,10,15,21,27,34,41,29,19,20] | $U_{10,9,9,9,8,6,4,2,1,1}$ [216] | $U_{10,9,9,9,8,6,4,2,1}$ [216] |
| | [4,0,0,0,1,0,2,0,2,1] | [1,6,11,16,21,27,33,41,29,19,20] | $U_{10,9,9,9,9,5,3,3,1,1}$ [90] | $U_{10,9,9,9,9,5,3,3,1}$ [90] |
| | [4,0,0,1,0,0,0,3,1,0] | [1,6,11,16,22,28,34,40,29,19,20] | $U_{10,9,9,9,9,6,2,2,2,1}$ [60] | $U_{10,9,9,9,9,6,2,2,2}$ [60] |
| | [6,0,0,0,0,0,0,1,3,2] | [0,6,12,18,24,30,36,42,29,19,20] | $U_{9,9,9,9,9,9,2,1,1,1}$ [32] | $U_{9,9,9,9,9,9,2,1,1}$ [32] |
| | [0,0,1,2,1,1,0,0,1,2] | [3,6,9,13,19,26,34,42,30,19,20] | $U_{10,10,10,7,6,6,5,4,1}$ [128] | $U_{10,10,10,7,6,6,5,4,1,1}$ [128] |
| | [0,0,1,3,0,0,0,2,0,1] | [3,6,9,13,20,27,34,41,30,19,20] | $U_{10,10,10,7,6,6,6,2,2}$ [60] | $U_{10,10,10,7,6,6,6,2,2,1}$ [60] |
| | [0,0,2,0,2,0,1,1,0,1] | [3,6,9,14,19,26,33,41,30,19,20] | $U_{10,10,10,7,7,5,5,3,2}$ [108] | $U_{10,10,10,7,7,5,5,3,2,1}$ [108] |
| | [0,1,0,1,1,2,0,1,0,1] | [3,6,10,14,19,25,33,41,30,19,20] | $U_{10,10,10,8,6,5,4,4,2}$ [162] | $U_{10,10,10,8,6,5,4,4,2,1}$ [162] |
| | [0,1,0,2,0,0,3,0,0,1] | [3,6,10,14,20,26,32,41,30,19,20] | $U_{10,10,10,8,6,6,3,3,3}$ [72] | $U_{10,10,10,8,6,6,3,3,3,1}$ [72] |
| | [0,1,1,0,0,2,2,0,0,1] | [3,6,10,15,20,25,32,41,30,19,20] | $U_{10,10,10,8,7,4,4,3,3}$ [96] | $U_{10,10,10,8,7,4,4,3,3,1}$ [96] |
| | [0,2,2,1,0,0,0,1,1,2] | [2,4,8,14,21,28,35,42,30,19,20] | $U_{10,10,8,8,7,7,6,2,1}$ [120] | $U_{10,10,8,8,7,7,6,2,1,1}$ [120] |
| | [0,3,0,1,1,0,1,0,1,2] | [2,4,9,14,20,27,34,42,30,19,20] | $U_{10,10,8,8,8,6,5,3,1}$ [162] | $U_{10,10,8,8,8,6,5,3,1,1}$ [162] |
| | [0,3,1,0,0,1,0,2,0,1] | [2,4,9,15,21,27,34,41,30,19,20] | $U_{10,10,8,8,8,7,4,2,2}$ [108] | $U_{10,10,8,8,8,7,4,2,2,1}$ [108] |
| | [1,0,0,0,2,1,2,0,0,1] | [3,7,11,15,19,25,32,41,30,19,20] | $U_{10,10,10,9,5,5,4,3,3}$ [80] | $U_{10,10,10,9,5,5,4,3,3,1}$ [80] |
| | [1,0,3,0,1,0,1,0,1,2] | [2,5,8,14,20,27,34,42,30,19,20] | $U_{10,10,9,7,7,7,5,3,1}$ [162] | $U_{10,10,9,7,7,7,5,3,1,1}$ [162] |

| | | | | |
|---|---|---|---|---|
| | [1,1,0,3,0,0,1,0,1,2] | [2,5,9,13,20,27,34,42,30,19,20] | $U_{10,10,9,8,6,6,6,3,1}$ [144] | $U_{10,10,9,8,6,6,6,3,1,1}$ [144] |
| | [1,1,1,0,2,1,0,0,1,2] | [2,5,9,14,19,26,34,42,30,19,20] | $U_{10,10,9,8,7,5,5,4,1}$ [192] | $U_{10,10,9,8,7,5,5,4,1,1}$ [192] |
| | [1,1,1,1,0,1,1,1,0,1] | [2,5,9,14,20,26,33,41,30,19,20] | $U_{10,10,9,8,7,6,4,3,2}$ [288] | $U_{10,10,9,8,7,6,4,3,2,1}$ [288] |
| | [2,0,0,1,2,0,1,1,0,1] | [2,6,10,14,19,26,33,41,30,19,20] | $U_{10,10,9,9,6,5,5,3,2}$ [144] | $U_{10,10,9,9,6,5,5,3,2,1}$ [144] |
| | [2,0,1,0,0,3,0,1,0,1] | [2,6,10,15,20,25,33,41,30,19,20] | $U_{10,10,9,9,7,4,4,4,2}$ [108] | $U_{10,10,9,9,7,4,4,4,2,1}$ [108] |
| | [2,0,1,0,1,0,3,0,0,1] | [2,6,10,15,20,26,32,41,30,19,20] | $U_{10,10,9,9,7,5,3,3,3}$ [108] | $U_{10,10,9,9,7,5,3,3,3,1}$ [108] |
| | [2,1,3,0,0,0,0,0,2,3] | [1,4,8,15,22,29,36,43,30,19,20] | $U_{10,9,9,8,7,7,7,1,1}$ [56] | $U_{10,9,9,8,7,7,7,1,1,1}$ [56] |
| | [2,2,0,2,0,0,0,1,1,2] | [1,4,9,14,21,28,35,42,30,19,20] | $U_{10,9,9,8,8,6,6,2,1}$ [120] | $U_{10,9,9,8,8,6,6,2,1,1}$ [120] |
| | [2,2,1,0,0,1,1,0,1,2] | [1,4,9,15,21,27,34,42,30,19,20] | $U_{10,9,9,8,8,7,4,3,1}$ [192] | $U_{10,9,9,8,8,7,4,3,1,1}$ [192] |
| | [2,3,0,0,0,0,1,2,0,1] | [1,4,10,16,22,28,34,41,30,19,20] | $U_{10,9,9,8,8,8,3,2,2}$ [72] | $U_{10,9,9,8,8,8,3,2,2,1}$ [72] |
| | [3,0,1,1,1,0,1,0,1,2] | [1,5,9,14,20,27,34,42,30,19,20] | $U_{10,9,9,9,7,6,5,3,1}$ [216] | $U_{10,9,9,9,7,6,5,3,1,1}$ [216] |
| | [3,0,2,0,0,1,0,2,0,1] | [1,5,9,15,21,27,34,41,30,19,20] | $U_{10,9,9,9,7,7,4,2,2}$ [108] | $U_{10,9,9,9,7,7,4,2,2,1}$ [108] |
| | [3,1,0,0,1,2,0,0,1,2] | [1,5,10,15,20,26,34,42,30,19,20] | $U_{10,9,9,9,8,5,4,4,1}$ [128] | $U_{10,9,9,9,8,5,4,4,1,1}$ [128] |
| | [3,1,0,0,2,0,0,2,0,1] | [1,5,10,15,20,27,34,41,30,19,20] | $U_{10,9,9,9,8,5,5,2,2}$ [96] | $U_{10,9,9,9,8,5,5,2,2,1}$ [96] |
| | [3,1,0,1,0,0,2,1,0,1] | [1,5,10,15,21,27,33,41,30,19,20] | $U_{10,9,9,9,8,6,3,3,2}$ [144] | $U_{10,9,9,9,8,6,3,3,2,1}$ [144] |
| | [4,0,0,0,0,2,1,1,0,1] | [1,6,11,16,21,26,33,41,30,19,20] | $U_{10,9,9,9,9,4,4,3,2}$ [72] | $U_{10,9,9,9,9,4,4,3,2,1}$ [72] |
| | [4,2,0,0,1,0,0,0,2,3] | [0,4,10,16,22,29,36,43,30,19,20] | $U_{9,9,9,9,8,8,5,1,1}$ [80] | $U_{9,9,9,9,8,8,5,1,1,1}$ [80] |
| | [5,0,0,2,0,0,0,0,2,3] | [0,5,10,15,22,29,36,43,30,19,20] | $U_{9,9,9,9,9,6,6,1,1}$ [48] | $U_{9,9,9,9,9,6,6,1,1,1}$ [48] |
| | [5,0,1,0,0,1,0,1,1,2] | [0,5,10,16,22,28,35,42,30,19,20] | $U_{9,9,9,9,9,7,4,2,1}$ [144] | $U_{9,9,9,9,9,7,4,2,1,1}$ [144] |
| | [0,2,2,0,1,1,0,0,0,3] | [2,4,8,14,20,27,35,43,31,19,20] | $U_{10,10,8,8,7,7,5,4}$ [90] | $U_{10,10,8,8,7,7,5,4,1,1,1}$ [90] |
| | [1,0,2,2,0,1,0,0,0,3] | [2,5,8,13,20,27,35,43,31,19,20] | $U_{10,10,9,7,7,6,6,4}$ [90] | $U_{10,10,9,7,7,6,6,4,1,1,1}$ [90] |
| | [1,1,0,2,2,0,0,0,0,3] | [2,5,9,13,19,27,35,43,31,19,20] | $U_{10,10,9,8,6,6,5,5}$ [72] | $U_{10,10,9,8,6,6,5,5,1,1,1}$ [72] |
| | [1,4,0,1,0,0,0,1,0,3] | [1,3,9,15,22,29,36,43,31,19,20] | $U_{10,9,8,8,8,8,6,2}$ [90] | $U_{10,9,8,8,8,8,6,2,1,1,1}$ [90] |
| | [2,1,2,1,0,0,1,0,0,3] | [1,4,8,14,21,28,35,43,31,19,20] | $U_{10,9,9,8,7,7,6,3}$ [128] | $U_{10,9,9,8,7,7,6,3,1,1,1}$ [128] |
| | [2,2,0,1,1,1,0,0,0,3] | [1,4,9,14,20,27,35,43,31,19,20] | $U_{10,9,9,8,8,6,5,4}$ [120] | $U_{10,9,9,8,8,6,5,4,1,1,1}$ [120] |
| | [4,1,1,1,0,0,0,1,0,3] | [0,4,9,15,22,29,36,43,31,19,20] | $U_{9,9,9,9,8,7,6,2}$ [120] | $U_{9,9,9,9,8,7,6,2,1,1,1}$ [120] |
| | [4,2,0,0,0,1,1,0,0,3] | [0,4,10,16,22,28,35,43,31,19,20] | $U_{9,9,9,9,8,8,4,3}$ [80] | $U_{9,9,9,9,8,8,4,3,1,1,1}$ [80] |
| | [5,0,0,1,1,0,1,0,0,3] | [0,5,10,15,21,28,35,43,31,19,20] | $U_{9,9,9,9,9,6,5,3}$ [96] | $U_{9,9,9,9,9,6,5,3,1,1,1}$ [96] |
| | [3,4,0,0,0,0,0,0,0,5] | [0,3,10,17,24,31,38,45,32,19,20] | $U_{9,9,9,8,8,8,8}$ [18] | $U_{9,9,9,8,8,8,8,1,1,1,1,1}$ [18] |
| | [0,3,0,0,0,0,0,0,7,0] | [3,6,12,18,24,30,36,42,27,19,21] | $U_{10,10,10,8,8,8,1,1,1,1,1,1,1}$ [13] | $U_{10,10,10,8,8,8}$ [14] |
| | [0,1,0,3,0,0,0,0,5,0] | [3,6,10,14,21,28,35,42,28,19,21] | $U_{10,10,10,8,6,6,6,1,1,1,1,1}$ [31] | $U_{10,10,10,8,6,6,6}$ [32] |
| | [1,2,0,1,1,0,0,0,5,0] | [2,5,10,15,21,28,35,42,28,19,21] | $U_{10,10,9,8,8,6,5,1,1,1,1,1}$ [72] | $U_{10,10,9,8,8,6,5}$ [72] |
| | [3,2,0,0,0,0,1,0,5,0] | [1,5,11,17,23,29,35,42,28,19,21] | $U_{10,9,9,9,8,8,3,1,1,1,1,1}$ [48] | $U_{10,9,9,9,8,8,3}$ [48] |
| | [4,0,0,1,0,1,0,0,5,0] | [1,6,11,16,22,28,35,42,28,19,21] | $U_{10,9,9,9,9,6,4,1,1,1,1,1}$ [60] | $U_{10,9,9,9,9,6,4}$ [60] |
| | [0,0,1,3,0,0,1,0,3,0] | [3,6,9,13,20,27,34,42,29,19,21] | $U_{10,10,10,7,6,6,6,3,1,1,1}$ [64] | $U_{10,10,10,7,6,6,6,3}$ [64] |
| | [0,0,2,0,2,1,0,0,3,0] | [3,6,9,14,19,26,34,42,29,19,21] | $U_{10,10,10,7,7,5,5,4,1,1,1}$ [60] | $U_{10,10,10,7,7,5,5,4}$ [60] |
| | [0,3,0,2,0,0,0,1,3,0] | [2,4,9,14,21,28,35,42,29,19,21] | $U_{10,10,8,8,8,6,6,2,1,1,1}$ [67] | $U_{10,10,8,8,8,6,6,2}$ [68] |
| | [0,3,1,0,0,1,1,0,3,0] | [2,4,9,15,21,27,34,42,29,19,21] | $U_{10,10,8,8,8,7,4,3,1,1,1}$ [96] | $U_{10,10,8,8,8,7,4,3}$ [96] |
| | [1,1,1,1,0,2,0,0,3,0] | [2,5,9,14,20,26,34,42,29,19,21] | $U_{10,10,9,8,7,6,4,4,1,1,1}$ [120] | $U_{10,10,9,8,7,6,4,4}$ [120] |
| | [2,0,0,1,2,1,0,0,3,0] | [2,6,10,14,19,26,34,42,29,19,21] | $U_{10,10,9,9,6,5,5,4,1,1,1}$ [80] | $U_{10,10,9,9,6,5,5,4}$ [80] |
| | [2,2,1,0,1,0,0,1,3,0] | [1,4,9,15,21,28,35,42,29,19,21] | $U_{10,9,9,8,8,7,5,2,1,1,1}$ [144] | $U_{10,9,9,8,8,7,5,2}$ [144] |
| | [2,3,0,0,0,0,2,0,3,0] | [1,4,10,16,22,28,34,42,29,19,21] | $U_{10,9,9,8,8,8,3,3,1,1,1}$ [48] | $U_{10,9,9,8,8,8,3,3}$ [48] |
| | [3,0,1,2,0,0,0,1,3,0] | [1,5,9,14,21,28,35,42,29,19,21] | $U_{10,9,9,9,7,6,6,2,1,1,1}$ [90] | $U_{10,9,9,9,7,6,6,2}$ [90] |
| | [3,0,2,0,0,1,1,0,3,0] | [1,5,9,15,21,27,34,42,29,19,21] | $U_{10,9,9,9,7,7,4,3,1,1,1}$ [96] | $U_{10,9,9,9,7,7,4,3}$ [96] |
| | [3,1,0,0,2,0,1,0,3,0] | [1,5,10,15,20,27,34,42,29,19,21] | $U_{10,9,9,9,8,5,5,3,1,1,1}$ [96] | $U_{10,9,9,9,8,5,5,3}$ [96] |
| | [5,0,1,0,1,0,0,0,4,1] | [0,5,10,16,22,29,36,43,29,19,21] | $U_{9,9,9,9,9,7,5,1,1,1,1}$ [90] | $U_{9,9,9,9,9,7,5,1}$ [90] |
| | [5,1,0,0,0,0,1,1,3,0] | [0,5,11,17,23,29,35,42,29,19,21] | $U_{9,9,9,9,9,8,3,2,1,1,1}$ [72] | $U_{9,9,9,9,9,8,3,2}$ [72] |
| | [0,0,0,0,0,5,0,0,1,0] | [4,8,12,16,20,24,33,42,30,19,21] | $U_{10,10,10,10,4,4,4,4,4,1}$ [17] | $U_{10,10,10,10,4,4,4,4,4}$ [18] |
| | [0,0,1,2,1,0,2,0,1,0] | [3,6,9,13,19,26,33,42,30,19,21] | $U_{10,10,10,7,6,6,5,3,3,1}$ [96] | $U_{10,10,10,7,6,6,5,3,3}$ [96] |
| | [0,0,2,0,1,2,1,0,1,0] | [3,6,9,14,19,25,33,42,30,19,21] | $U_{10,10,10,7,7,5,4,4,3,1}$ [96] | $U_{10,10,10,7,7,5,4,4,3}$ [96] |
| | [0,2,1,2,0,1,0,0,2,1] | [2,4,8,13,20,27,35,43,30,19,21] | $U_{10,10,8,8,7,6,6,4,1,1}$ [144] | $U_{10,10,8,8,7,6,6,4,1}$ [144] |
| | [0,2,2,0,1,0,1,1,1,0] | [2,4,8,14,20,27,34,42,30,19,21] | $U_{10,10,8,8,7,7,5,3,2,1}$ [162] | $U_{10,10,8,8,7,7,5,3,2}$ [162] |
| | [0,3,0,0,3,0,0,0,2,1] | [2,4,9,14,19,27,35,43,30,19,21] | $U_{10,10,8,8,8,5,5,5,1,1}$ [60] | $U_{10,10,8,8,8,5,5,5,1}$ [60] |
| | [0,3,0,1,0,2,0,1,1,0] | [2,4,9,14,20,26,34,42,30,19,21] | $U_{10,10,8,8,8,6,4,4,2,1}$ [121] | $U_{10,10,8,8,8,6,4,4,2}$ [122] |
| | [1,0,2,1,2,0,0,0,2,1] | [2,5,8,13,19,27,35,43,30,19,21] | $U_{10,10,9,7,7,6,5,5,1,1}$ [120] | $U_{10,10,9,7,7,6,5,5,1}$ [120] |
| | [1,0,2,2,0,0,1,1,1,0] | [2,5,8,13,20,27,34,42,30,19,21] | $U_{10,10,9,7,7,6,6,3,2,1}$ [144] | $U_{10,10,9,7,7,6,6,3,2}$ [144] |
| | [1,0,3,0,0,2,0,1,1,0] | [2,5,8,14,20,26,34,42,30,19,21] | $U_{10,10,9,7,7,7,4,4,2,1}$ [108] | $U_{10,10,9,7,7,7,4,4,2}$ [108] |
| | [1,1,0,2,1,1,0,1,1,0] | [2,5,9,13,19,26,34,42,30,19,21] | $U_{10,10,9,8,6,6,5,4,2,1}$ [216] | $U_{10,10,9,8,6,6,5,4,2}$ [216] |
| | [1,1,1,0,2,0,2,0,1,0] | [2,5,9,14,19,26,33,42,30,19,21] | $U_{10,10,9,8,7,5,5,3,3,1}$ [144] | $U_{10,10,9,8,7,5,5,3,3}$ [144] |
| | [1,2,0,0,0,3,1,0,1,0] | [2,5,10,15,20,25,33,42,30,19,21] | $U_{10,10,9,8,8,4,4,4,3,1}$ [80] | $U_{10,10,9,8,8,4,4,4,3}$ [80] |
| | [1,3,2,0,0,0,0,1,2,1] | [1,3,8,15,22,29,36,43,30,19,21] | $U_{10,9,8,8,8,7,7,2,1,1}$ [96] | $U_{10,9,8,8,8,7,7,2,1}$ [96] |
| | [1,4,0,0,1,0,1,0,2,1] | [1,3,9,15,21,28,35,43,30,19,21] | $U_{10,9,8,8,8,8,5,3,1,1}$ [144] | $U_{10,9,8,8,8,8,5,3,1}$ [144] |
| | [2,0,0,1,1,2,1,0,1,0] | [2,6,10,14,19,25,33,42,30,19,21] | $U_{10,10,9,9,6,5,4,4,3,1}$ [128] | $U_{10,10,9,9,6,5,4,4,3}$ [128] |
| | [2,1,2,0,1,1,0,0,2,1] | [1,4,8,14,20,27,35,43,30,19,21] | $U_{10,9,9,8,7,7,5,4,1,1}$ [192] | $U_{10,9,9,8,7,7,5,4,1}$ [192] |
| | [2,1,2,1,0,0,0,2,1,0] | [1,4,8,14,21,28,35,42,30,19,21] | $U_{10,9,9,8,7,7,6,2,2,1}$ [120] | $U_{10,9,9,8,7,7,6,2,2}$ [120] |
| | [2,2,0,1,1,0,1,1,1,0] | [1,4,9,14,20,27,34,42,30,19,21] | $U_{10,9,9,8,8,6,5,3,2,1}$ [216] | $U_{10,9,9,8,8,6,5,3,2}$ [216] |
| | [3,0,0,3,0,1,0,0,2,1] | [1,5,9,13,20,27,35,43,30,19,21] | $U_{10,9,9,9,6,6,6,4,1,1}$ [96] | $U_{10,9,9,9,6,6,6,4,1}$ [96] |
| | [3,0,1,0,3,0,0,0,2,1] | [1,5,9,14,19,27,35,43,30,19,21] | $U_{10,9,9,9,7,5,5,5,1,1}$ [90] | $U_{10,9,9,9,7,5,5,5,1}$ [90] |
| | [3,0,1,1,0,2,0,1,1,0] | [1,5,9,14,20,26,34,42,30,19,21] | $U_{10,9,9,9,7,6,4,4,2,1}$ [162] | $U_{10,9,9,9,7,6,4,4,2}$ [162] |
| | [3,0,2,0,0,0,3,0,1,0] | [1,5,9,15,21,27,33,42,30,19,21] | $U_{10,9,9,9,7,7,3,3,3,1}$ [60] | $U_{10,9,9,9,7,7,3,3,3}$ [60] |
| | [3,1,0,0,1,1,2,0,1,0] | [1,5,10,15,20,26,33,42,30,19,21] | $U_{10,9,9,9,8,5,4,3,3,1}$ [128] | $U_{10,9,9,9,8,5,4,3,3}$ [128] |

| | | | | |
|---|---|---|---|---|
| | [3,3,1,0,0,0,0,0,3,2] | [0,3,9,16,23,30,37,44,30,19,21] | $U_{9,9,9,8,8,8,7,1,1,1}$ [56] | $U_{9,9,9,8,8,8,7,1,1}$ [56] |
| | [4,1,1,0,1,0,1,0,2,1] | [0,4,9,15,21,28,35,43,30,19,21] | $U_{9,9,9,9,8,7,5,3,1,1}$ [216] | $U_{9,9,9,9,8,7,5,3,1}$ [216] |
| | [4,2,0,0,0,1,0,2,1,0] | [0,4,10,16,22,28,35,42,30,19,21] | $U_{9,9,9,9,8,8,4,2,2,1}$ [90] | $U_{9,9,9,9,8,8,4,2,2}$ [90] |
| | [5,0,0,1,0,2,0,0,2,1] | [0,5,10,15,21,27,35,43,30,19,21] | $U_{9,9,9,9,9,6,4,4,1,1}$ [96] | $U_{9,9,9,9,9,6,4,4,1}$ [96] |
| | [5,0,0,1,1,0,0,2,1,0] | [0,5,10,15,21,28,35,42,30,19,21] | $U_{9,9,9,9,9,6,5,2,2,1}$ [96] | $U_{9,9,9,9,9,6,5,2,2}$ [96] |
| | [5,0,1,0,0,0,2,1,1,0] | [0,5,10,16,22,28,34,42,30,19,21] | $U_{9,9,9,9,9,7,3,3,2,1}$ [90] | $U_{9,9,9,9,9,7,3,3,2}$ [90] |
| | [0,0,0,4,1,0,0,1,0,1] | [3,6,9,12,19,27,35,43,31,19,21] | $U_{10,10,10,6,6,6,6,5,2}$ [60] | $U_{10,10,10,6,6,6,6,5,2,1}$ [60] |
| | [0,0,1,2,0,3,0,0,0,1] | [3,6,9,13,19,25,34,43,31,19,21] | $U_{10,10,10,7,6,6,4,4,4}$ [60] | $U_{10,10,10,7,6,6,4,4,4,1}$ [60] |
| | [0,1,3,1,1,0,0,0,1,2] | [2,4,7,13,20,28,36,44,31,19,21] | $U_{10,10,8,7,7,7,6,5,1}$ [120] | $U_{10,10,8,7,7,7,6,5,1,1}$ [120] |
| | [0,1,4,0,0,0,1,1,0,1] | [2,4,7,14,21,28,35,43,31,19,21] | $U_{10,10,8,7,7,7,7,3,2}$ [90] | $U_{10,10,8,7,7,7,7,3,2,1}$ [90] |
| | [0,2,1,1,2,0,0,1,0,1] | [2,4,8,13,19,27,35,43,31,19,21] | $U_{10,10,8,8,7,6,5,5,2}$ [144] | $U_{10,10,8,8,7,6,5,5,2,1}$ [144] |
| | [0,2,1,2,0,0,2,0,0,1] | [2,4,8,13,20,27,34,43,31,19,21] | $U_{10,10,8,8,7,6,6,3,3}$ [96] | $U_{10,10,8,8,7,6,6,3,3,1}$ [96] |
| | [0,2,2,0,0,2,1,0,0,1] | [2,4,8,14,20,26,34,43,31,19,21] | $U_{10,10,8,8,7,7,4,4,3}$ [96] | $U_{10,10,8,8,7,7,4,4,3,1}$ [96] |
| | [0,3,0,0,2,1,1,0,0,1] | [2,4,9,14,19,26,34,43,31,19,21] | $U_{10,10,8,8,8,5,5,4,3}$ [96] | $U_{10,10,8,8,8,5,5,4,3,1}$ [96] |
| | [1,0,1,4,0,0,0,0,1,2] | [2,5,8,12,20,28,36,44,31,19,21] | $U_{10,10,9,7,6,6,6,6,1}$ [72] | $U_{10,10,9,7,6,6,6,6,1,1}$ [72] |
| | [1,0,2,1,1,1,1,0,0,1] | [2,5,8,13,19,26,34,43,31,19,21] | $U_{10,10,9,7,7,6,5,4,3}$ [192] | $U_{10,10,9,7,7,6,5,4,3,1}$ [192] |
| | [1,1,1,0,1,3,0,0,0,1] | [2,5,9,14,19,25,34,43,31,19,21] | $U_{10,10,9,8,7,5,4,4,4}$ [120] | $U_{10,10,9,8,7,5,4,4,4,1}$ [120] |
| | [1,3,1,0,2,0,0,0,1,2] | [1,3,8,14,20,28,36,44,31,19,21] | $U_{10,9,8,8,8,7,5,5,1}$ [120] | $U_{10,9,8,8,8,7,5,5,1,1}$ [120] |
| | [1,3,1,1,0,0,1,1,0,1] | [1,3,8,14,21,28,35,43,31,19,21] | $U_{10,9,8,8,8,7,6,3,2}$ [192] | $U_{10,9,8,8,8,7,6,3,2,1}$ [192] |
| | [1,4,0,0,0,2,0,1,0,1] | [1,3,9,15,21,27,35,43,31,19,21] | $U_{10,9,8,8,8,8,4,4,2}$ [90] | $U_{10,9,8,8,8,8,4,4,2,1}$ [90] |
| | [2,0,4,0,0,1,0,0,1,2] | [1,4,7,14,21,28,36,44,31,19,21] | $U_{10,9,9,7,7,7,7,4,1}$ [96] | $U_{10,9,9,7,7,7,7,4,1,1}$ [96] |
| | [2,1,1,2,0,1,0,1,0,1] | [1,4,8,13,20,27,35,43,31,19,21] | $U_{10,9,9,8,7,6,6,4,2}$ [216] | $U_{10,9,9,8,7,6,6,4,2,1}$ [216] |
| | [2,1,2,0,1,0,2,0,0,1] | [1,4,8,14,20,27,34,43,31,19,21] | $U_{10,9,9,8,7,7,5,3,3}$ [144] | $U_{10,9,9,8,7,7,5,3,3,1}$ [144] |
| | [2,2,0,0,3,0,0,1,0,1] | [1,4,9,14,19,27,35,43,31,19,21] | $U_{10,9,9,8,8,5,5,5,2}$ [96] | $U_{10,9,9,8,8,5,5,5,2,1}$ [96] |
| | [2,2,0,1,0,2,1,0,0,1] | [1,4,9,14,20,26,34,43,31,19,21] | $U_{10,9,9,8,8,6,4,4,3}$ [144] | $U_{10,9,9,8,8,6,4,4,3,1}$ [144] |
| | [3,0,0,2,2,0,0,1,0,1] | [1,5,9,13,19,27,35,43,31,19,21] | $U_{10,9,9,9,6,6,5,5,2}$ [96] | $U_{10,9,9,9,6,6,5,5,2,1}$ [96] |
| | [3,0,0,3,0,0,2,0,0,1] | [1,5,9,13,20,27,34,43,31,19,21] | $U_{10,9,9,9,6,6,6,3,3}$ [64] | $U_{10,9,9,9,6,6,6,3,3,1}$ [64] |
| | [3,0,1,0,2,1,1,0,0,1] | [1,5,9,14,19,26,34,43,31,19,21] | $U_{10,9,9,9,7,5,5,4,3}$ [144] | $U_{10,9,9,9,7,5,5,4,3,1}$ [144] |
| | [3,2,2,0,0,0,1,0,1,2] | [0,3,8,15,22,29,36,44,31,19,21] | $U_{9,9,9,8,8,7,7,3,1}$ [120] | $U_{9,9,9,8,8,7,7,3,1,1}$ [120] |
| | [3,3,0,0,1,1,0,0,1,2] | [0,3,9,15,21,28,36,44,31,19,21] | $U_{9,9,9,8,8,8,5,4,1}$ [128] | $U_{9,9,9,8,8,8,5,4,1,1}$ [128] |
| | [3,3,0,1,0,0,0,2,0,1] | [0,3,9,15,22,29,36,43,31,19,21] | $U_{9,9,9,8,8,8,6,2,2}$ [90] | $U_{9,9,9,8,8,8,6,2,2,1}$ [90] |
| | [4,0,2,1,0,1,0,0,1,2] | [0,4,8,14,21,28,36,44,31,19,21] | $U_{9,9,9,9,7,7,6,4,1}$ [144] | $U_{9,9,9,9,7,7,6,4,1,1}$ [144] |
| | [4,0,3,0,0,0,0,2,0,1] | [0,4,8,15,22,29,36,43,31,19,21] | $U_{9,9,9,9,7,7,7,2,2}$ [54] | $U_{9,9,9,9,7,7,7,2,2,1}$ [54] |
| | [4,1,0,1,2,0,0,0,1,2] | [0,4,9,14,20,28,36,44,31,19,21] | $U_{9,9,9,9,8,6,5,5,1}$ [120] | $U_{9,9,9,9,8,6,5,5,1,1}$ [120] |
| | [4,1,0,2,0,0,1,1,0,1] | [0,4,9,14,21,28,35,43,31,19,21] | $U_{9,9,9,9,8,6,6,3,2}$ [144] | $U_{9,9,9,9,8,6,6,3,2,1}$ [144] |
| | [4,1,1,0,0,2,0,1,0,1] | [0,4,9,15,21,27,35,43,31,19,21] | $U_{9,9,9,9,8,7,4,4,2}$ [144] | $U_{9,9,9,9,8,7,4,4,2,1}$ [144] |
| | [4,2,0,0,0,0,3,0,0,1] | [0,4,10,16,22,28,34,43,31,19,21] | $U_{9,9,9,9,8,8,3,3,3}$ [48] | $U_{9,9,9,9,8,8,3,3,3,1}$ [48] |
| | [5,0,0,0,2,1,0,1,0,1] | [0,5,10,15,20,27,35,43,31,19,21] | $U_{9,9,9,9,9,5,5,4,2}$ [90] | $U_{9,9,9,9,9,5,5,4,2,1}$ [90] |
| | [5,0,0,1,0,1,2,0,0,1] | [0,5,10,15,21,27,34,43,31,19,21] | $U_{9,9,9,9,9,6,4,3,3}$ [96] | $U_{9,9,9,9,9,6,4,3,3,1}$ [96] |
| | [0,6,0,0,0,0,1,0,0,3] | [1,2,9,16,23,30,37,45,32,19,21] | $U_{10,8,8,8,8,8,8,3}$ [36] | $U_{10,8,8,8,8,8,8,3,1,1,1}$ [36] |
| | [1,2,3,0,1,0,0,0,0,3] | [1,3,7,14,21,29,37,45,32,19,21] | $U_{10,9,8,8,7,7,7,5}$ [72] | $U_{10,9,8,8,7,7,7,5,1,1,1}$ [72] |
| | [2,0,3,2,0,0,0,0,0,3] | [1,4,7,13,21,29,37,45,32,19,21] | $U_{10,9,9,7,7,7,6,6}$ [42] | $U_{10,9,9,7,7,7,6,6,1,1,1}$ [42] |
| | [3,2,1,1,1,0,0,0,0,3] | [0,3,8,14,21,29,37,45,32,19,21] | $U_{9,9,9,8,8,7,6,5}$ [96] | $U_{9,9,9,8,8,7,6,5,1,1,1}$ [96] |
| | [4,2,0,1,0,0,0,0,5,0] | [0,4,10,16,23,30,37,44,29,19,22] | $U_{9,9,9,9,8,8,6,1,1,1,1,1}$ [42] | $U_{9,9,9,9,8,8,6}$ [42] |
| | [0,0,0,5,0,0,0,0,3,0] | [3,6,9,12,20,28,36,44,30,19,22] | $U_{10,10,10,6,6,6,6,6,1,1,1}$ [17] | $U_{10,10,10,6,6,6,6,6}$ [18] |
| | [1,3,1,1,0,1,0,0,3,0] | [1,3,8,14,21,28,36,44,30,19,22] | $U_{10,9,8,8,8,7,6,4,1,1,1}$ [120] | $U_{10,9,8,8,8,7,6,4}$ [120] |
| | [2,1,1,2,1,0,0,0,3,0] | [1,4,8,13,20,28,36,44,30,19,22] | $U_{10,9,9,8,7,6,6,5,1,1,1}$ [96] | $U_{10,9,9,8,7,6,6,5}$ [96] |
| | [3,3,0,1,0,0,1,0,3,0] | [0,3,9,15,22,29,36,44,30,19,22] | $U_{9,9,9,8,8,8,6,3,1,1,1}$ [96] | $U_{9,9,9,8,8,8,6,3}$ [96] |
| | [4,0,3,0,0,0,1,0,3,0] | [0,4,8,15,22,29,36,44,30,19,22] | $U_{9,9,9,9,7,7,7,3,1,1,1}$ [60] | $U_{9,9,9,9,7,7,7,3}$ [60] |
| | [4,1,0,2,0,1,0,0,3,0] | [0,4,9,14,21,28,36,44,30,19,22] | $U_{9,9,9,9,8,6,6,4,1,1,1}$ [90] | $U_{9,9,9,9,8,6,6,4}$ [90] |
| | [5,0,0,0,3,0,0,0,3,0] | [0,5,10,15,20,28,36,44,30,19,22] | $U_{9,9,9,9,9,5,5,5,1,1,1}$ [30] | $U_{9,9,9,9,9,5,5,5}$ [30] |
| | [0,0,0,4,0,2,0,0,1,0] | [3,6,9,12,19,26,35,44,31,19,22] | $U_{10,10,10,6,6,6,6,4,4,1}$ [37] | $U_{10,10,10,6,6,6,6,4,4}$ [38] |
| | [0,1,3,1,0,1,1,0,1,0] | [2,4,7,13,20,27,35,44,31,19,22] | $U_{10,10,8,7,7,7,6,4,3,1}$ [144] | $U_{10,10,8,7,7,7,6,4,3}$ [144] |
| | [0,2,0,4,0,0,0,1,1,0] | [2,4,8,12,20,28,36,44,31,19,22] | $U_{10,10,8,8,6,6,6,6,2,1}$ [67] | $U_{10,10,8,8,6,6,6,6,2}$ [68] |
| | [0,2,1,1,1,2,0,0,1,0] | [2,4,8,13,19,26,35,44,31,19,22] | $U_{10,10,8,8,7,6,5,4,4,1}$ [120] | $U_{10,10,8,8,7,6,5,4,4}$ [120] |
| | [0,5,1,0,0,1,0,0,2,1] | [1,2,8,15,22,29,37,45,31,19,22] | $U_{10,8,8,8,8,8,7,4,1,1}$ [96] | $U_{10,8,8,8,8,8,7,4,1}$ [96] |
| | [0,6,0,0,0,0,0,2,1,0] | [1,2,9,16,23,30,37,44,31,19,22] | $U_{10,8,8,8,8,8,8,2,2,1}$ [31] | $U_{10,8,8,8,8,8,8,2,2}$ [32] |
| | [1,0,1,3,1,0,1,0,1,0] | [2,5,8,12,19,27,35,44,31,19,22] | $U_{10,10,9,7,6,6,6,5,3,1}$ [144] | $U_{10,10,9,7,6,6,6,5,3}$ [144] |
| | [1,2,2,2,0,0,0,0,2,1] | [1,3,7,13,21,29,37,45,31,19,22] | $U_{10,9,8,8,7,7,6,6,1,1}$ [96] | $U_{10,9,8,8,7,7,6,6,1}$ [96] |
| | [1,2,3,0,0,1,0,1,1,0] | [1,3,7,14,21,28,36,44,31,19,22] | $U_{10,9,8,8,7,7,7,4,2,1}$ [144] | $U_{10,9,8,8,7,7,7,4,2}$ [144] |
| | [1,3,0,2,1,0,0,1,1,0] | [1,3,8,13,20,28,36,44,31,19,22] | $U_{10,9,8,8,8,6,6,5,2,1}$ [144] | $U_{10,9,8,8,8,6,6,5,2}$ [144] |
| | [1,3,1,0,1,1,1,0,1,0] | [1,3,8,14,20,27,35,44,31,19,22] | $U_{10,9,8,8,8,7,5,4,3,1}$ [192] | $U_{10,9,8,8,8,7,5,4,3}$ [192] |
| | [2,0,3,1,1,0,0,1,1,0] | [1,4,7,13,20,28,36,44,31,19,22] | $U_{10,9,9,7,7,7,6,5,2,1}$ [144] | $U_{10,9,9,7,7,7,6,5,2}$ [144] |
| | [2,0,4,0,0,0,2,0,1,0] | [1,4,7,14,21,28,35,44,31,19,22] | $U_{10,9,9,7,7,7,7,3,3,1}$ [60] | $U_{10,9,9,7,7,7,7,3,3}$ [60] |
| | [2,1,1,1,2,0,1,0,1,0] | [1,4,8,13,19,27,35,44,31,19,22] | $U_{10,9,9,8,7,6,5,5,3,1}$ [192] | $U_{10,9,9,8,7,6,5,5,3}$ [192] |
| | [2,1,2,0,0,3,0,0,1,0] | [1,4,8,14,20,26,35,44,31,19,22] | $U_{10,9,9,8,7,7,4,4,4,1}$ [80] | $U_{10,9,9,8,7,7,4,4,4}$ [80] |
| | [2,2,0,0,2,2,0,0,1,0] | [1,4,9,14,19,26,35,44,31,19,22] | $U_{10,9,9,8,8,5,5,4,4,1}$ [80] | $U_{10,9,9,8,8,5,5,4,4}$ [80] |
| | [2,5,0,0,0,0,1,0,2,1] | [0,2,9,16,23,30,37,45,31,19,22] | $U_{9,9,8,8,8,8,8,3,1,1}$ [72] | $U_{9,9,8,8,8,8,8,3,1}$ [72] |
| | [3,0,0,2,1,2,0,0,1,0] | [1,5,9,13,19,26,35,44,31,19,22] | $U_{10,9,9,9,6,6,5,4,4,1}$ [80] | $U_{10,9,9,9,6,6,5,4,4}$ [80] |
| | [3,2,1,1,0,1,0,1,1,0] | [0,3,8,14,21,28,36,44,31,19,22] | $U_{9,9,9,8,8,7,6,4,2,1}$ [216] | $U_{9,9,9,8,8,7,6,4,2}$ [216] |
| | [3,3,0,0,1,0,2,0,1,0] | [0,3,9,15,21,28,35,44,31,19,22] | $U_{9,9,9,8,8,8,5,3,3,1}$ [96] | $U_{9,9,9,8,8,8,5,3,3}$ [96] |

| | | | | |
|---|---|---|---|---|
| | [4,0,1,3,0,0,0,0,2,1] | [0,4,8,13,21,29,37,45,31,19,22] | $U_{9,9,9,9,7,6,6,6,1,1}$ [72] | $U_{9,9,9,9,7,6,6,6,1}$ [72] |
| | [4,0,2,0,2,0,0,1,1,0] | [0,4,8,14,20,28,36,44,31,19,22] | $U_{9,9,9,9,7,7,5,5,2,1}$ [108] | $U_{9,9,9,9,7,7,5,5,2}$ [108] |
| | [4,0,2,1,0,0,2,0,1,0] | [0,4,8,14,21,28,35,44,31,19,22] | $U_{9,9,9,9,7,7,6,3,3,1}$ [96] | $U_{9,9,9,9,7,7,6,3,3}$ [96] |
| | [4,1,0,1,1,1,1,0,1,0] | [0,4,9,14,20,27,35,44,31,19,22] | $U_{9,9,9,9,8,6,5,4,3,1}$ [192] | $U_{9,9,9,9,8,6,5,4,3}$ [192] |
| | [0,0,6,0,0,0,0,0,1,2] | [2,4,6,14,22,30,38,46,32,19,22] | $U_{10,10,7,7,7,7,7,7,1}$ [28] | $U_{10,10,7,7,7,7,7,7,1,1}$ [28] |
| | [0,1,2,3,0,0,1,0,0,1] | [2,4,7,12,20,28,36,45,32,19,22] | $U_{10,10,8,7,7,6,6,6,3}$ [96] | $U_{10,10,8,7,7,6,6,6,3,1}$ [96] |
| | [0,1,3,0,2,1,0,0,0,1] | [2,4,7,13,19,27,36,45,32,19,22] | $U_{10,10,8,7,7,7,5,5,4}$ [90] | $U_{10,10,8,7,7,7,5,5,4,1}$ [90] |
| | [0,2,0,3,1,1,0,0,0,1] | [2,4,8,12,19,27,36,45,32,19,22] | $U_{10,10,8,8,6,6,6,5,4}$ [90] | $U_{10,10,8,8,6,6,6,5,4,1}$ [90] |
| | [0,4,2,1,0,0,0,0,1,2] | [1,2,7,14,22,30,38,46,32,19,22] | $U_{10,8,8,8,8,7,7,6,1}$ [72] | $U_{10,8,8,8,8,7,7,6,1,1}$ [72] |
| | [0,5,0,1,1,0,0,1,0,1] | [1,2,8,14,21,29,37,45,32,19,22] | $U_{10,8,8,8,8,8,6,5,2}$ [108] | $U_{10,8,8,8,8,8,6,5,2,1}$ [108] |
| | [0,5,1,0,0,0,2,0,0,1] | [1,2,8,15,22,29,36,45,32,19,22] | $U_{10,8,8,8,8,8,7,3,3}$ [60] | $U_{10,8,8,8,8,8,7,3,3,1}$ [60] |
| | [1,2,2,1,1,0,1,0,0,1] | [1,3,7,13,20,28,36,45,32,19,22] | $U_{10,9,8,8,7,7,6,5,3}$ [192] | $U_{10,9,8,8,7,7,6,5,3,1}$ [192] |
| | [1,3,0,2,0,2,0,0,0,1] | [1,3,8,13,20,27,36,45,32,19,22] | $U_{10,9,8,8,8,6,6,4,4}$ [90] | $U_{10,9,8,8,8,6,6,4,4,1}$ [90] |
| | [2,0,3,1,0,2,0,0,0,1] | [1,4,7,13,20,27,36,45,32,19,22] | $U_{10,9,9,7,7,7,6,4,4}$ [90] | $U_{10,9,9,7,7,7,6,4,4,1}$ [90] |
| | [2,1,0,4,0,0,1,0,0,1] | [1,4,8,12,20,28,36,45,32,19,22] | $U_{10,9,9,8,6,6,6,6,3}$ [96] | $U_{10,9,9,8,6,6,6,6,3,1}$ [96] |
| | [2,4,0,2,0,0,0,0,1,2] | [0,2,8,14,22,30,38,46,32,19,22] | $U_{9,9,8,8,8,8,6,6,1}$ [72] | $U_{9,9,8,8,8,8,6,6,1,1}$ [72] |
| | [2,4,1,0,0,1,0,1,0,1] | [0,2,8,15,22,29,37,45,32,19,22] | $U_{9,9,8,8,8,8,7,4,2}$ [144] | $U_{9,9,8,8,8,8,7,4,2,1}$ [144] |
| | [3,1,3,0,1,0,0,1,0,1] | [0,3,7,14,21,29,37,45,32,19,22] | $U_{9,9,9,8,7,7,7,5,2}$ [144] | $U_{9,9,9,8,7,7,7,5,2,1}$ [144] |
| | [3,2,0,3,0,0,0,1,0,1] | [0,3,8,13,21,29,37,45,32,19,22] | $U_{9,9,9,8,8,6,6,6,2}$ [90] | $U_{9,9,9,8,8,6,6,6,2,1}$ [90] |
| | [3,2,1,0,2,0,1,0,0,1] | [0,3,8,14,20,28,36,45,32,19,22] | $U_{9,9,9,8,8,7,5,5,3}$ [144] | $U_{9,9,9,8,8,7,5,5,3,1}$ [144] |
| | [3,3,0,0,0,3,0,0,0,1] | [0,3,9,15,21,27,36,45,32,19,22] | $U_{9,9,9,8,8,8,4,4,4}$ [50] | $U_{9,9,9,8,8,8,4,4,4,1}$ [50] |
| | [4,0,1,2,1,0,1,0,0,1] | [0,4,8,13,20,28,36,45,32,19,22] | $U_{9,9,9,9,7,6,6,5,3}$ [144] | $U_{9,9,9,9,7,6,6,5,3,1}$ [144] |
| | [4,0,2,0,1,2,0,0,0,1] | [0,4,8,14,20,27,36,45,32,19,22] | $U_{9,9,9,9,7,7,5,4,4}$ [90] | $U_{9,9,9,9,7,7,5,4,4,1}$ [90] |
| | [2,3,3,0,0,0,0,0,0,3] | [0,2,7,15,23,31,39,47,33,19,22] | $U_{9,9,8,8,8,7,7,7}$ [32] | $U_{9,9,8,8,8,7,7,7,1,1,1}$ [32] |
| | [0,5,0,2,0,0,0,0,3,0] | [1,2,8,14,22,30,38,46,31,19,23] | $U_{10,8,8,8,8,8,6,6,1,1,1}$ [31] | $U_{10,8,8,8,8,8,6,6}$ [32] |
| | [2,4,1,0,1,0,0,0,3,0] | [0,2,8,15,22,30,38,46,31,19,23] | $U_{9,9,8,8,8,8,7,5,1,1,1}$ [72] | $U_{9,9,8,8,8,8,7,5}$ [72] |
| | [3,1,3,1,0,0,0,0,3,0] | [0,3,7,14,22,30,38,46,31,19,23] | $U_{9,9,9,8,7,7,7,6,1,1,1}$ [56] | $U_{9,9,9,8,7,7,7,6}$ [56] |
| | [0,0,5,1,0,0,1,0,1,0] | [2,4,6,13,21,29,37,46,32,19,23] | $U_{10,10,7,7,7,7,7,6,3,1}$ [64] | $U_{10,10,7,7,7,7,7,6,3}$ [64] |
| | [0,1,2,2,2,0,0,0,1,0] | [2,4,7,12,19,28,37,46,32,19,23] | $U_{10,10,8,7,7,6,6,5,5,1}$ [72] | $U_{10,10,8,7,7,6,6,5,5}$ [72] |
| | [0,4,2,0,1,0,1,0,1,0] | [1,2,7,14,21,29,37,46,32,19,23] | $U_{10,8,8,8,8,7,7,5,3,1}$ [108] | $U_{10,8,8,8,8,7,7,5,3}$ [108] |
| | [0,5,0,1,0,2,0,0,1,0] | [1,2,8,14,21,28,37,46,32,19,23] | $U_{10,8,8,8,8,8,6,4,4,1}$ [67] | $U_{10,8,8,8,8,8,6,4,4}$ [68] |
| | [1,1,5,0,0,0,0,1,1,0] | [1,3,6,14,22,30,38,46,32,19,23] | $U_{10,9,8,7,7,7,7,7,2,1}$ [72] | $U_{10,9,8,7,7,7,7,7,2}$ [72] |
| | [1,3,0,1,3,0,0,0,1,0] | [1,3,8,13,19,28,37,46,32,19,23] | $U_{10,9,8,8,8,6,5,5,5,1}$ [72] | $U_{10,9,8,8,8,6,5,5,5}$ [72] |
| | [2,0,2,3,0,1,0,0,1,0] | [1,4,7,12,20,28,37,46,32,19,23] | $U_{10,9,9,7,7,6,6,6,4,1}$ [90] | $U_{10,9,9,7,7,6,6,6,4}$ [90] |
| | [2,0,3,0,3,0,0,0,1,0] | [1,4,7,13,19,28,37,46,32,19,23] | $U_{10,9,9,7,7,7,5,5,5,1}$ [54] | $U_{10,9,9,7,7,7,5,5,5}$ [54] |
| | [2,1,0,3,2,0,0,0,1,0] | [1,4,8,12,19,28,37,46,32,19,23] | $U_{10,9,9,8,6,6,6,5,5,1}$ [72] | $U_{10,9,9,8,6,6,6,5,5}$ [72] |
| | [2,3,2,1,0,0,0,1,1,0] | [0,2,7,14,22,30,38,46,32,19,23] | $U_{9,9,8,8,8,7,7,6,2,1}$ [120] | $U_{9,9,8,8,8,7,7,6,2}$ [120] |
| | [2,4,0,1,1,0,1,0,1,0] | [0,2,8,14,21,29,37,46,32,19,23] | $U_{9,9,8,8,8,8,6,5,3,1}$ [144] | $U_{9,9,8,8,8,8,6,5,3}$ [144] |
| | [3,1,2,2,0,0,1,0,1,0] | [0,3,7,13,21,29,37,46,32,19,23] | $U_{9,9,9,8,7,7,6,6,3,1}$ [128] | $U_{9,9,9,8,7,7,6,6,3}$ [128] |
| | [3,1,3,0,0,2,0,0,1,0] | [0,3,7,14,21,28,37,46,32,19,23] | $U_{9,9,9,8,7,7,7,4,4,1}$ [80] | $U_{9,9,9,8,7,7,7,4,4}$ [80] |
| | [3,2,0,2,1,1,0,0,1,0] | [0,3,8,13,20,28,37,46,32,19,23] | $U_{9,9,9,8,8,6,6,5,4,1}$ [120] | $U_{9,9,9,8,8,6,6,5,4}$ [120] |
| | [4,1,0,0,4,0,0,0,1,0] | [0,4,9,14,19,28,37,46,32,19,23] | $U_{9,9,9,9,8,5,5,5,5,1}$ [48] | $U_{9,9,9,9,8,5,5,5,5}$ [48] |
| | [0,0,5,0,2,0,0,0,0,1] | [2,4,6,13,20,29,38,47,33,19,23] | $U_{10,10,7,7,7,7,7,7,5,5}$ [36] | $U_{10,10,7,7,7,7,7,7,5,5,1}$ [36] |
| | [0,4,1,2,0,1,0,0,0,1] | [1,2,7,13,21,29,38,47,33,19,23] | $U_{10,8,8,8,8,7,6,6,4}$ [90] | $U_{10,8,8,8,8,7,6,6,4,1}$ [90] |
| | [0,5,0,0,3,0,0,0,0,1] | [1,2,8,14,20,29,38,47,33,19,23] | $U_{10,8,8,8,8,8,5,5,5}$ [36] | $U_{10,8,8,8,8,8,5,5,5,1}$ [36] |
| | [1,1,4,1,0,1,0,0,0,1] | [1,3,6,13,21,29,38,47,33,19,23] | $U_{10,9,8,7,7,7,7,6,4}$ [120] | $U_{10,9,8,7,7,7,7,6,4,1}$ [120] |
| | [1,2,1,3,1,0,0,0,0,1] | [1,3,7,12,20,29,38,47,33,19,23] | $U_{10,9,8,8,7,6,6,6,5}$ [96] | $U_{10,9,8,8,7,6,6,6,5,1}$ [96] |
| | [1,6,1,0,0,0,0,0,1,2] | [0,1,8,16,24,32,40,48,33,19,23] | $U_{9,8,8,8,8,8,8,7,1}$ [56] | $U_{9,8,8,8,8,8,8,7,1,1}$ [56] |
| | [2,3,2,0,1,1,0,0,0,1] | [0,2,7,14,21,29,38,47,33,19,23] | $U_{9,9,8,8,8,7,7,5,4}$ [120] | $U_{9,9,8,8,8,7,7,5,4,1}$ [120] |
| | [3,1,2,1,2,0,0,0,0,1] | [0,3,7,13,20,29,38,47,33,19,23] | $U_{9,9,9,8,7,7,6,5,5}$ [96] | $U_{9,9,9,8,7,7,6,5,5,1}$ [96] |
| | [0,3,4,0,0,1,0,0,1,0] | [1,2,6,14,22,30,39,48,33,19,24] | $U_{10,8,8,8,7,7,7,7,4,1}$ [60] | $U_{10,8,8,8,7,7,7,7,4}$ [60] |
| | [1,6,0,1,0,0,1,0,1,0] | [0,1,8,15,23,31,39,48,33,19,24] | $U_{9,8,8,8,8,8,8,6,3,1}$ [96] | $U_{9,8,8,8,8,8,8,6,3}$ [96] |
| | [2,3,1,2,1,0,0,0,1,0] | [0,2,7,13,21,30,39,48,33,19,24] | $U_{9,9,8,8,8,7,6,6,5,1}$ [96] | $U_{9,9,8,8,8,7,6,6,5}$ [96] |
| | [3,0,5,0,0,1,0,0,1,0] | [0,3,6,14,22,30,39,48,33,19,24] | $U_{9,9,9,7,7,7,7,7,4,1}$ [60] | $U_{9,9,9,7,7,7,7,7,4}$ [60] |
| | [4,0,0,5,0,0,0,0,1,0] | [0,4,8,12,21,30,39,48,33,19,24] | $U_{9,9,9,9,6,6,6,6,6,1}$ [28] | $U_{9,9,9,9,6,6,6,6,6}$ [28] |
| | [0,3,3,2,0,0,0,0,0,1] | [1,2,6,13,22,31,40,49,34,19,24] | $U_{10,8,8,8,7,7,7,6,6}$ [42] | $U_{10,8,8,8,7,7,7,6,6,1}$ [42] |
| | [1,5,2,0,0,1,0,0,0,1] | [0,1,7,15,23,31,40,49,34,19,24] | $U_{9,8,8,8,8,8,7,7,4}$ [80] | $U_{9,8,8,8,8,8,7,7,4,1}$ [80] |
| | [1,6,0,0,2,0,0,0,0,1] | [0,1,8,15,22,31,40,49,34,19,24] | $U_{9,8,8,8,8,8,8,5,5}$ [48] | $U_{9,8,8,8,8,8,8,5,5,1}$ [48] |
| | [2,2,4,0,1,0,0,0,0,1] | [0,2,6,14,22,31,40,49,34,19,24] | $U_{9,9,8,8,7,7,7,7,5}$ [72] | $U_{9,9,8,8,7,7,7,7,5,1}$ [72] |
| | [3,0,4,2,0,0,0,0,0,1] | [0,3,6,13,22,31,40,49,34,19,24] | $U_{9,9,9,7,7,7,7,6,6}$ [42] | $U_{9,9,9,7,7,7,7,6,6,1}$ [42] |
| | [1,5,1,2,0,0,0,0,1,0] | [0,1,7,14,23,32,41,50,34,19,25] | $U_{9,8,8,8,8,8,7,6,6,1}$ [56] | $U_{9,8,8,8,8,8,7,6,6}$ [56] |
| | [0,9,0,0,0,0,0,0,1,0] | [0,0,9,18,27,36,45,54,36,19,27] | $U_{8,8,8,8,8,8,8,8,8,1}$ [13] | $U_{8,8,8,8,8,8,8,8,8}$ [14] |
| 20 | [0,0,0,1,1,1,1,0,2,2] | [4,8,12,16,21,27,34,42,30,20,20] | $V_{10,10,10,10,6,5,4,3,1,1}$ [120] | |
| | [0,0,0,2,0,0,1,2,1,1] | [4,8,12,16,22,28,34,41,30,20,20] | $V_{10,10,10,10,6,6,3,2,2,1}$ [80] | |
| | [0,0,1,0,0,2,0,2,1,1] | [4,8,12,17,22,27,34,41,30,20,20] | $V_{10,10,10,10,7,4,4,2,2,1}$ [96] | |
| | [0,1,0,0,0,0,3,1,1,1] | [4,8,13,18,23,28,33,41,30,20,20] | $V_{10,10,10,10,8,3,3,3,2,1}$ [72] | |
| | [0,1,2,0,1,0,0,0,3,3] | [3,6,10,16,22,29,36,43,30,20,20] | $V_{10,10,10,8,7,7,5,1,1,1}$ [90] | |
| | [0,2,0,1,0,1,0,1,2,2] | [3,6,11,16,22,28,35,42,30,20,20] | $V_{10,10,10,8,8,6,4,2,1,1}$ [162] | |
| | [1,0,0,0,0,0,1,4,0,0] | [4,9,14,19,24,29,34,40,30,20,20] | $V_{10,10,10,10,9,3,2,2,2,2}$ [28] | |
| | [1,0,0,3,0,0,0,0,3,3] | [3,7,11,15,22,29,36,43,30,20,20] | $V_{10,10,10,9,6,6,6,1,1,1}$ [48] | |
| | [1,0,1,0,2,0,0,1,2,2] | [3,7,11,16,21,28,35,42,30,20,20] | $V_{10,10,10,9,7,5,5,2,1,1}$ [144] | |

| | | | |
|---|---|---|---|
| | [1,0,1,1,0,0,2,0,2,2] | [3,7,11,16,22,28,34,42,30,20,20] | $V_{10,10,10,9,7,6,3,3,1,1}$ [144] |
| | [1,0,2,0,0,0,0,3,1,1] | [3,7,11,17,23,29,35,41,30,20,20] | $V_{10,10,10,9,7,7,2,2,2,1}$ [72] |
| | [1,1,0,0,0,2,1,0,2,2] | [3,7,12,17,22,27,34,42,30,20,20] | $V_{10,10,10,9,8,4,4,3,1,1}$ [120] |
| | [1,1,0,0,1,0,1,2,1,1] | [3,7,12,17,22,28,34,41,30,20,20] | $V_{10,10,10,9,8,5,3,2,2,1}$ [192] |
| | [2,1,0,1,1,0,0,0,3,3] | [2,6,11,16,22,29,36,43,30,20,20] | $V_{10,10,9,9,8,6,5,1,1,1}$ [120] |
| | [2,1,1,0,0,0,1,1,2,2] | [2,6,11,17,23,29,35,42,30,20,20] | $V_{10,10,9,9,8,7,3,2,1,1}$ [160] |
| | [3,0,0,0,1,1,0,1,2,2] | [2,7,12,17,22,28,35,42,30,20,20] | $V_{10,10,9,9,9,5,4,2,1,1}$ [120] |
| | [5,0,0,0,0,0,0,1,3,3] | [1,7,13,19,25,31,37,43,30,20,20] | $V_{10,9,9,9,9,9,2,1,1,1}$ [32] |
| | [0,0,0,0,2,2,1,0,1,1] | [4,8,12,16,20,26,34,43,31,20,21] | $V_{10,10,10,10,5,5,4,4,3,1}$ [72] |
| | [0,0,0,0,3,0,1,2,0,0] | [4,8,12,16,20,27,34,42,31,20,21] | $V_{10,10,10,10,5,5,5,3,2,2}$ [36] |
| | [0,0,0,1,0,3,0,2,0,0] | [4,8,12,16,21,26,34,42,31,20,21] | $V_{10,10,10,10,6,4,4,4,2,2}$ [45] |
| | [0,0,0,1,1,0,3,1,0,0] | [4,8,12,16,21,27,33,42,31,20,21] | $V_{10,10,10,10,6,5,3,3,3,2}$ [60] |
| | [0,0,2,2,0,1,0,0,2,2] | [3,6,9,14,21,28,36,44,31,20,21] | $V_{10,10,10,7,7,6,6,4,1,1}$ [96] |
| | [0,0,3,0,1,0,1,1,1,1] | [3,6,9,15,21,28,35,43,31,20,21] | $V_{10,10,10,7,7,7,5,3,2,1}$ [144] |
| | [0,1,0,2,2,0,0,0,2,2] | [3,6,10,14,20,28,36,44,31,20,21] | $V_{10,10,10,8,6,6,5,5,1,1}$ [90] |
| | [0,1,0,3,0,0,1,1,1,1] | [3,6,10,14,21,28,35,43,31,20,21] | $V_{10,10,10,8,6,6,6,3,2,1}$ [144] |
| | [0,1,1,0,2,1,0,1,1,1] | [3,6,10,15,20,27,35,43,31,20,21] | $V_{10,10,10,8,7,5,5,4,2,1}$ [216] |
| | [0,1,1,1,0,1,2,0,1,1] | [3,6,10,15,21,27,34,43,31,20,21] | $V_{10,10,10,8,7,6,4,3,3,1}$ [216] |
| | [0,1,1,1,1,0,0,3,0,0] | [3,6,10,15,21,28,35,42,31,20,21] | $V_{10,10,10,8,7,6,5,2,2,2}$ [96] |
| | [0,1,2,0,0,0,2,2,0,0] | [3,6,10,16,22,28,34,42,31,20,21] | $V_{10,10,10,8,7,7,3,3,2,2}$ [60] |
| | [0,2,0,0,1,1,1,2,0,0] | [3,6,11,16,21,27,34,42,31,20,21] | $V_{10,10,10,8,8,5,4,3,2,2}$ [96] |
| | [0,3,2,0,0,0,0,1,2,2] | [2,4,9,16,23,30,37,44,31,20,21] | $V_{10,10,8,8,8,7,7,2,1,1}$ [72] |
| | [0,4,0,0,1,0,1,0,2,2] | [2,4,10,16,22,29,36,44,31,20,21] | $V_{10,10,8,8,8,8,5,3,1,1}$ [108] |
| | [1,0,0,1,2,0,2,0,1,1] | [3,7,11,15,20,27,34,43,31,20,21] | $V_{10,10,10,9,6,5,5,3,3,1}$ [144] |
| | [1,0,0,2,0,1,1,2,0,0] | [3,7,11,15,21,27,34,42,31,20,21] | $V_{10,10,10,9,6,6,4,3,2,2}$ [96] |
| | [1,0,1,0,0,3,1,0,1,1] | [3,7,11,16,21,26,34,43,31,20,21] | $V_{10,10,10,9,7,4,4,4,3,1}$ [144] |
| | [1,1,0,0,0,1,3,1,0,0] | [3,7,12,17,22,27,33,42,31,20,21] | $V_{10,10,10,9,8,4,3,3,3,2}$ [80] |
| | [1,1,2,0,1,1,0,0,2,2] | [2,5,9,15,21,28,36,44,31,20,21] | $V_{10,10,9,8,7,7,5,4,1,1}$ [192] |
| | [1,1,2,1,0,0,0,2,1,1] | [2,5,9,15,22,29,36,43,31,20,21] | $V_{10,10,9,8,7,7,6,2,2,1}$ [160] |
| | [1,2,0,1,1,0,1,1,1,1] | [2,5,10,15,21,28,35,43,31,20,21] | $V_{10,10,9,8,8,6,5,3,2,1}$ [288] |
| | [1,3,0,0,0,0,1,3,0,0] | [2,5,11,17,23,29,35,42,31,20,21] | $V_{10,10,9,8,8,8,3,2,2,2}$ [48] |
| | [2,0,0,3,0,1,0,0,2,2] | [2,6,10,14,21,28,36,44,31,20,21] | $V_{10,10,9,9,6,6,6,4,1,1}$ [96] |
| | [2,0,1,0,3,0,0,0,2,2] | [2,6,10,15,20,28,36,44,31,20,21] | $V_{10,10,9,9,7,5,5,5,1,1}$ [90] |
| | [2,0,1,1,0,2,0,1,1,1] | [2,6,10,15,21,27,35,43,31,20,21] | $V_{10,10,9,9,7,6,4,4,2,1}$ [216] |
| | [2,0,2,0,0,0,3,0,1,1] | [2,6,10,16,22,28,34,43,31,20,21] | $V_{10,10,9,9,7,7,3,3,3,1}$ [90] |
| | [2,0,2,0,0,1,0,3,0,0] | [2,6,10,16,22,28,35,42,31,20,21] | $V_{10,10,9,9,7,7,4,2,2,2}$ [72] |
| | [2,1,0,0,1,1,2,0,1,1] | [2,6,11,16,21,27,34,43,31,20,21] | $V_{10,10,9,9,8,5,4,3,3,1}$ [192] |
| | [2,1,0,0,2,0,0,3,0,0] | [2,6,11,16,21,28,35,42,31,20,21] | $V_{10,10,9,9,8,5,5,2,2,2}$ [64] |
| | [2,1,0,1,0,0,2,2,0,0] | [2,6,11,16,22,28,34,42,31,20,21] | $V_{10,10,9,9,8,6,3,3,2,2}$ [96] |
| | [2,3,0,1,0,0,0,1,2,2] | [1,4,10,16,23,30,37,44,31,20,21] | $V_{10,9,9,8,8,8,6,2,1,1}$ [120] |
| | [3,0,0,0,0,2,1,2,0,0] | [2,7,12,17,22,27,34,42,31,20,21] | $V_{10,10,9,9,9,4,4,3,2,2}$ [48] |
| | [3,0,3,0,0,0,0,1,2,2] | [1,5,9,16,23,30,37,44,31,20,21] | $V_{10,9,9,9,7,7,7,2,1,1}$ [72] |
| | [3,1,0,2,0,0,1,0,2,2] | [1,5,10,15,22,29,36,44,31,20,21] | $V_{10,9,9,9,8,6,6,3,1,1}$ [144] |
| | [3,1,1,0,0,2,0,0,2,2] | [1,5,10,16,22,28,36,44,31,20,21] | $V_{10,9,9,9,8,7,4,4,1,1}$ [128] |
| | [3,1,1,0,1,0,0,2,1,1] | [1,5,10,16,22,29,36,43,31,20,21] | $V_{10,9,9,9,8,7,5,2,2,1}$ [192] |
| | [3,2,0,0,0,0,2,1,1,1] | [1,5,11,17,23,29,35,43,31,20,21] | $V_{10,9,9,9,8,8,3,3,2,1}$ [96] |
| | [4,0,0,0,2,1,0,0,2,2] | [1,6,11,16,21,28,36,44,31,20,21] | $V_{10,9,9,9,9,5,5,4,1,1}$ [80] |
| | [4,0,0,1,0,1,1,1,1,1] | [1,6,11,16,22,28,35,43,31,20,21] | $V_{10,9,9,9,9,6,4,3,2,1}$ [192] |
| | [4,1,0,0,0,0,0,4,0,0] | [1,6,12,18,24,30,36,42,31,20,21] | $V_{10,9,9,9,9,8,2,2,2,2}$ [28] |
| | [5,1,0,1,0,0,0,0,3,3] | [0,5,11,17,24,31,38,45,31,20,21] | $V_{9,9,9,9,9,8,6,1,1,1}$ [72] |
| | [6,0,0,0,0,1,0,1,2,2] | [0,6,12,18,24,30,37,44,31,20,21] | $V_{9,9,9,9,9,9,4,2,1,1}$ [72] |
| | [0,0,1,3,1,0,1,0,1,1] | [3,6,9,13,20,28,36,45,32,20,22] | $V_{10,10,10,7,6,6,6,5,3,1}$ [144] |
| | [0,0,2,1,1,1,1,1,0,0] | [3,6,9,14,20,27,35,44,32,20,22] | $V_{10,10,10,7,7,6,5,4,3,2}$ [128] |
| | [0,1,1,0,1,3,0,1,0,0] | [3,6,10,15,20,26,35,44,32,20,22] | $V_{10,10,10,8,7,5,4,4,4,2}$ [108] |
| | [0,1,1,0,2,0,3,0,0,0] | [3,6,10,15,20,27,34,44,32,20,22] | $V_{10,10,10,8,7,5,5,3,3,3}$ [54] |
| | [0,2,0,0,0,3,2,0,0,0] | [3,6,11,16,21,26,34,44,32,20,22] | $V_{10,10,10,8,8,4,4,4,3,3}$ [30] |
| | [0,2,2,1,1,0,0,1,1,1] | [2,4,8,14,21,29,37,45,32,20,22] | $V_{10,10,8,8,7,7,6,5,2,1}$ [192] |
| | [0,2,3,0,0,0,2,0,1,1] | [2,4,8,15,22,29,36,45,32,20,22] | $V_{10,10,8,8,7,7,7,3,3,1}$ [90] |
| | [0,3,0,2,0,1,1,0,1,1] | [2,4,9,14,21,28,36,45,32,20,22] | $V_{10,10,8,8,8,6,6,4,3,1}$ [162] |
| | [0,3,1,0,1,1,0,2,0,0] | [2,4,9,15,21,28,36,44,32,20,22] | $V_{10,10,8,8,8,7,5,4,2,2}$ [108] |
| | [1,0,0,1,1,2,2,0,0,0] | [3,7,11,15,20,26,34,44,32,20,22] | $V_{10,10,10,9,6,5,4,4,3,3}$ [64] |
| | [1,0,3,1,0,1,1,0,1,1] | [2,5,8,14,21,28,36,45,32,20,22] | $V_{10,10,9,7,7,7,6,4,3,1}$ [216] |
| | [1,0,4,0,0,0,1,2,0,0] | [2,5,8,15,22,29,36,44,32,20,22] | $V_{10,10,9,7,7,7,7,3,2,2}$ [60] |
| | [1,1,0,4,0,0,0,1,1,1] | [2,5,9,13,21,29,37,45,32,20,22] | $V_{10,10,9,8,6,6,6,6,2,1}$ [120] |
| | [1,1,1,1,1,2,0,0,1,1] | [2,5,9,14,20,27,36,45,32,20,22] | $V_{10,10,9,8,7,6,5,4,4,1}$ [256] |
| | [1,1,1,1,2,0,0,2,0,0] | [2,5,9,14,20,28,36,44,32,20,22] | $V_{10,10,9,8,7,6,5,5,2,2}$ [128] |
| | [1,1,1,2,0,0,2,1,0,0] | [2,5,9,14,21,28,35,44,32,20,22] | $V_{10,10,9,8,7,6,6,3,3,2}$ [128] |
| | [1,1,2,0,0,2,1,1,0,0] | [2,5,9,15,21,27,35,44,32,20,22] | $V_{10,10,9,8,7,7,4,4,3,2}$ [128] |
| | [1,2,0,0,2,1,1,1,0,0] | [2,5,10,15,20,27,35,44,32,20,22] | $V_{10,10,9,8,8,5,5,4,3,2}$ [128] |
| | [1,4,0,1,1,0,0,0,2,2] | [1,3,9,15,22,30,38,46,32,20,22] | $V_{10,9,8,8,8,8,6,5,1,1}$ [120] |
| | [1,4,1,0,0,0,1,1,1,1] | [1,3,9,16,23,30,37,45,32,20,22] | $V_{10,9,8,8,8,8,7,3,2,1}$ [160] |

| | | | |
|---|---|---|---|
| | [2,0,0,2,1,1,1,1,0,0] | [2,6,10,14,20,27,35,44,32,20,22] | $V_{10,10,9,9,6,6,5,4,3,2}$ [128] |
| | [2,0,1,1,0,1,3,0,0,0] | [2,6,10,15,21,27,34,44,32,20,22] | $V_{10,10,9,9,7,6,4,3,3,3}$ [72] |
| | [2,1,0,0,0,4,0,1,0,0] | [2,6,11,16,21,26,35,44,32,20,22] | $V_{10,10,9,9,8,4,4,4,4,2}$ [60] |
| | [2,1,2,2,0,0,0,0,2,2] | [1,4,8,14,22,30,38,46,32,20,22] | $V_{10,9,9,8,7,7,6,6,1,1}$ [96] |
| | [2,1,3,0,0,1,0,1,1,1] | [1,4,8,15,22,29,37,45,32,20,22] | $V_{10,9,9,8,7,7,7,4,2,1}$ [192] |
| | [2,2,0,2,1,0,0,1,1,1] | [1,4,9,14,21,29,37,45,32,20,22] | $V_{10,9,9,8,8,6,6,5,2,1}$ [192] |
| | [2,2,1,0,1,1,1,0,1,1] | [1,4,9,15,21,28,36,45,32,20,22] | $V_{10,9,9,8,8,7,5,4,3,1}$ [288] |
| | [2,2,1,1,0,0,1,2,0,0] | [1,4,9,15,22,29,36,44,32,20,22] | $V_{10,9,9,8,8,7,6,3,2,2}$ [128] |
| | [2,3,0,0,0,2,0,2,0,0] | [1,4,10,16,22,28,36,44,32,20,22] | $V_{10,9,9,8,8,8,4,4,2,2}$ [60] |
| | [3,0,1,2,0,1,1,0,1,1] | [1,5,9,14,21,28,36,45,32,20,22] | $V_{10,9,9,9,7,6,6,4,3,1}$ [216] |
| | [3,0,2,0,1,1,0,2,0,0] | [1,5,9,15,21,28,36,44,32,20,22] | $V_{10,9,9,9,7,7,5,4,2,2}$ [108] |
| | [3,1,0,0,3,0,1,0,1,1] | [1,5,10,15,20,28,36,45,32,20,22] | $V_{10,9,9,9,8,5,5,5,3,1}$ [144] |
| | [3,1,0,1,0,3,0,0,1,1] | [1,5,10,15,21,27,36,45,32,20,22] | $V_{10,9,9,9,8,6,4,4,4,1}$ [144] |
| | [3,1,0,1,1,0,2,1,0,0] | [1,5,10,15,21,28,35,44,32,20,22] | $V_{10,9,9,9,8,6,5,3,3,2}$ [144] |
| | [3,4,0,0,0,0,1,0,2,2] | [0,3,10,17,24,31,38,46,32,20,22] | $V_{9,9,9,8,8,8,8,3,1,1}$ [72] |
| | [4,0,0,0,1,2,1,1,0,0] | [1,6,11,16,21,27,35,44,32,20,22] | $V_{10,9,9,9,9,5,4,4,3,2}$ [80] |
| | [4,1,1,1,1,0,0,0,2,2] | [0,4,9,15,22,30,38,46,32,20,22] | $V_{9,9,9,9,8,7,6,5,1,1}$ [160] |
| | [4,1,2,0,0,0,1,1,1,1] | [0,4,9,16,23,30,37,45,32,20,22] | $V_{9,9,9,9,8,7,7,3,2,1}$ [160] |
| | [4,2,0,0,1,1,0,1,1,1] | [0,4,10,16,22,29,37,45,32,20,22] | $V_{9,9,9,9,8,8,5,4,2,1}$ [192] |
| | [5,0,0,2,0,1,0,1,1,1] | [0,5,10,15,22,29,37,45,32,20,22] | $V_{9,9,9,9,9,6,6,4,2,1}$ [144] |
| | [5,0,1,0,1,0,2,0,1,1] | [0,5,10,16,22,29,36,45,32,20,22] | $V_{9,9,9,9,9,7,5,3,3,1}$ [162] |
| | [5,0,1,1,0,0,0,3,0,0] | [0,5,10,16,23,30,37,44,32,20,22] | $V_{9,9,9,9,9,7,6,2,2,2}$ [60] |
| | [5,1,0,0,0,1,1,2,0,0] | [0,5,11,17,23,29,36,44,32,20,22] | $V_{9,9,9,9,9,8,4,3,2,2}$ [80] |
| | [0,0,1,3,0,2,1,0,0,0] | [3,6,9,13,20,27,36,46,33,20,23] | $V_{10,10,10,7,6,6,6,4,4,3}$ [48] |
| | [0,1,0,2,0,4,0,0,0,0] | [3,6,10,14,20,26,36,46,33,20,23] | $V_{10,10,10,8,6,6,4,4,4,4}$ [27] |
| | [0,1,4,0,1,1,0,0,1,1] | [2,4,7,14,21,29,38,47,33,20,23] | $V_{10,10,8,7,7,7,7,5,4,1}$ [144] |
| | [0,1,4,1,0,0,0,2,0,0] | [2,4,7,14,22,30,38,46,33,20,23] | $V_{10,10,8,7,7,7,7,6,2,2}$ [60] |
| | [0,2,1,2,2,0,0,0,1,1] | [2,4,8,13,20,29,38,47,33,20,23] | $V_{10,10,8,8,7,6,6,5,5,1}$ [120] |
| | [0,2,1,3,0,0,1,1,0,0] | [2,4,8,13,21,29,37,46,33,20,23] | $V_{10,10,8,8,7,6,6,6,3,2}$ [96] |
| | [0,2,2,0,2,1,0,1,0,0] | [2,4,8,14,20,28,37,46,33,20,23] | $V_{10,10,8,8,7,7,5,5,4,2}$ [108] |
| | [0,2,2,1,0,1,2,0,0,0] | [2,4,8,14,21,28,36,46,33,20,23] | $V_{10,10,8,8,7,7,6,4,3,3}$ [72] |
| | [0,3,0,1,2,0,2,0,0,0] | [2,4,9,14,20,28,36,46,33,20,23] | $V_{10,10,8,8,8,6,5,5,3,3}$ [54] |
| | [0,3,1,0,0,3,1,0,0,0] | [2,4,9,15,21,27,36,46,33,20,23] | $V_{10,10,8,8,8,7,4,4,4,3}$ [48] |
| | [0,5,2,0,0,0,0,0,2,2] | [1,2,8,16,24,32,40,48,33,20,23] | $V_{10,8,8,8,8,8,7,7,1,1}$ [42] |
| | [0,6,0,0,1,0,0,1,1,1] | [1,2,9,16,23,31,39,47,33,20,23] | $V_{10,8,8,8,8,8,8,5,2,1}$ [96] |
| | [1,0,2,2,1,1,0,1,0,0] | [2,5,8,13,20,28,37,46,33,20,23] | $V_{10,10,9,7,7,6,6,5,4,2}$ [144] |
| | [1,0,3,0,2,0,2,0,0,0] | [2,5,8,14,20,28,36,46,33,20,23] | $V_{10,10,9,7,7,7,5,5,3,3}$ [54] |
| | [1,1,0,3,1,0,2,0,0,0] | [2,5,9,13,20,28,36,46,33,20,23] | $V_{10,10,9,8,6,6,6,5,3,3}$ [72] |
| | [1,2,4,0,0,0,0,1,1,1] | [1,3,7,15,23,31,39,47,33,20,23] | $V_{10,9,8,8,7,7,7,7,2,1}$ [96] |
| | [1,3,1,1,1,1,0,0,1,1] | [1,3,8,14,21,29,38,47,33,20,23] | $V_{10,9,8,8,8,7,6,5,4,1}$ [256] |
| | [1,3,1,2,0,0,0,2,0,0] | [1,3,8,14,22,30,38,46,33,20,23] | $V_{10,9,8,8,8,7,6,6,2,2}$ [80] |
| | [1,3,2,0,0,1,1,1,0,0] | [1,3,8,15,22,29,37,46,33,20,23] | $V_{10,9,8,8,8,7,7,4,3,2}$ [128] |
| | [1,4,0,0,2,0,1,1,0,0] | [1,3,9,15,21,29,37,46,33,20,23] | $V_{10,9,8,8,8,8,5,5,3,2}$ [96] |
| | [2,0,1,0,1,4,0,0,0,0] | [2,6,10,15,20,26,36,46,33,20,23] | $V_{10,10,9,9,7,5,4,4,4,4}$ [36] |
| | [2,0,4,1,0,0,1,0,1,1] | [1,4,7,14,22,30,38,47,33,20,23] | $V_{10,9,9,7,7,7,7,6,3,1}$ [144] |
| | [2,1,1,3,0,1,0,0,1,1] | [1,4,8,13,21,29,38,47,33,20,23] | $V_{10,9,9,8,7,6,6,6,4,1}$ [192] |
| | [2,1,2,0,3,0,0,0,1,1] | [1,4,8,14,20,29,38,47,33,20,23] | $V_{10,9,9,8,7,7,5,5,5,1}$ [120] |
| | [2,1,2,1,0,2,0,1,0,0] | [1,4,8,14,21,28,37,46,33,20,23] | $V_{10,9,9,8,7,7,6,4,4,2}$ [144] |
| | [2,1,3,0,0,0,3,0,0,0] | [1,4,8,15,22,29,36,46,33,20,23] | $V_{10,9,9,8,7,7,7,3,3,3}$ [40] |
| | [2,2,0,1,2,1,0,1,0,0] | [1,4,9,14,20,28,37,46,33,20,23] | $V_{10,9,9,8,8,6,5,5,4,2}$ [144] |
| | [2,2,0,2,0,1,2,0,0,0] | [1,4,9,14,21,28,36,46,33,20,23] | $V_{10,9,9,8,8,6,6,4,3,3}$ [72] |
| | [2,5,0,1,0,0,0,0,2,2] | [0,2,9,16,24,32,40,48,33,20,23] | $V_{9,9,8,8,8,8,8,6,1,1}$ [72] |
| | [3,0,0,3,2,0,0,0,1,1] | [1,5,9,13,20,29,38,47,33,20,23] | $V_{10,9,9,9,6,6,6,5,5,1}$ [80] |
| | [3,0,0,4,0,0,1,1,0,0] | [1,5,9,13,21,29,37,46,33,20,23] | $V_{10,9,9,9,6,6,6,6,3,2}$ [64] |
| | [3,0,1,1,2,0,2,0,0,0] | [1,5,9,14,20,28,36,46,33,20,23] | $V_{10,9,9,9,7,6,5,5,3,3}$ [72] |
| | [3,0,2,0,0,3,1,0,0,0] | [1,5,9,15,21,27,36,46,33,20,23] | $V_{10,9,9,9,7,7,4,4,4,3}$ [48] |
| | [3,1,0,0,2,2,1,0,0,0] | [1,5,10,15,20,27,36,46,33,20,23] | $V_{10,9,9,9,8,5,5,4,4,3}$ [64] |
| | [3,2,2,0,1,0,1,0,1,1] | [0,3,8,15,22,30,38,47,33,20,23] | $V_{9,9,9,8,8,7,7,5,3,1}$ [216] |
| | [3,3,0,1,0,2,0,0,1,1] | [0,3,9,15,22,29,38,47,33,20,23] | $V_{9,9,9,8,8,8,6,4,4,1}$ [144] |
| | [3,3,0,1,1,0,0,2,0,0] | [0,3,9,15,22,30,38,46,33,20,23] | $V_{9,9,9,8,8,8,6,5,2,2}$ [96] |
| | [3,3,1,0,0,0,2,1,0,0] | [0,3,9,16,23,30,37,46,33,20,23] | $V_{9,9,9,8,8,8,7,3,3,2}$ [80] |
| | [4,0,2,2,0,0,1,0,1,1] | [0,4,8,14,22,30,38,47,33,20,23] | $V_{9,9,9,9,7,7,6,6,3,1}$ [144] |
| | [4,0,3,0,0,2,0,0,1,1] | [0,4,8,15,22,29,38,47,33,20,23] | $V_{9,9,9,9,7,7,7,4,4,1}$ [96] |
| | [4,0,3,0,1,0,0,2,0,0] | [0,4,8,15,22,30,38,46,33,20,23] | $V_{9,9,9,9,7,7,7,5,2,2}$ [72] |
| | [4,1,0,2,1,1,0,0,1,1] | [0,4,9,14,21,29,38,47,33,20,23] | $V_{9,9,9,9,8,6,6,5,4,1}$ [192] |
| | [4,1,0,3,0,0,0,2,0,0] | [0,4,9,14,22,30,38,46,33,20,23] | $V_{9,9,9,9,8,6,6,6,2,2}$ [60] |
| | [4,1,1,0,2,0,1,1,0,0] | [0,4,9,15,21,29,37,46,33,20,23] | $V_{9,9,9,9,8,7,5,5,3,2}$ [144] |
| | [4,2,0,0,0,3,0,1,0,0] | [0,4,10,16,22,28,37,46,33,20,23] | $V_{9,9,9,9,8,8,4,4,4,2}$ [60] |
| | [4,2,0,0,1,0,3,0,0,0] | [0,4,10,16,22,29,36,46,33,20,23] | $V_{9,9,9,9,8,8,5,3,3,3}$ [48] |
| | [5,0,0,1,1,2,0,1,0,0] | [0,5,10,15,21,28,37,46,33,20,23] | $V_{9,9,9,9,9,6,5,4,4,2}$ [96] |
| | [5,0,0,2,0,0,3,0,0,0] | [0,5,10,15,22,29,36,46,33,20,23] | $V_{9,9,9,9,9,6,6,3,3,3}$ [32] |

| | | | | |
|---|---|---|---|---|
| | [5,0,1,0,0,2,2,0,0,0] | [0,5,10,16,22,28,36,46,33,20,23] | $V_{9,9,9,9,9,7,4,4,3,3}$ [48] | |
| | [0,0,0,5,1,0,1,0,0,0] | [3,6,9,12,20,29,38,48,34,20,24] | $V_{10,10,10,6,6,6,6,6,5,3}$ [30] | |
| | [0,1,3,2,0,1,1,0,0,0] | [2,4,7,13,21,29,38,48,34,20,24] | $V_{10,10,8,7,7,7,6,6,4,3}$ [72] | |
| | [0,2,1,2,1,2,0,0,0,0] | [2,4,8,13,20,28,38,48,34,20,24] | $V_{10,10,8,8,7,6,6,5,4,4}$ [48] | |
| | [0,4,3,0,0,1,0,0,1,1] | [1,2,7,15,23,31,40,49,34,20,24] | $V_{10,8,8,8,8,7,7,7,4,1}$ [96] | |
| | [0,5,0,2,1,0,0,0,1,1] | [1,2,8,14,22,31,40,49,34,20,24] | $V_{10,8,8,8,8,8,6,6,5,1}$ [90] | |
| | [0,5,1,0,1,1,0,1,0,0] | [1,2,8,15,22,30,39,48,34,20,24] | $V_{10,8,8,8,8,8,7,5,4,2}$ [108] | |
| | [0,6,0,0,0,1,2,0,0,0] | [1,2,9,16,23,30,38,48,34,20,24] | $V_{10,8,8,8,8,8,8,4,3,3}$ [30] | |
| | [1,0,1,5,0,0,0,1,0,0] | [2,5,8,12,21,30,39,48,34,20,24] | $V_{10,10,9,7,6,6,6,6,6,2}$ [60] | |
| | [1,2,2,3,0,0,0,0,1,1] | [1,3,7,13,22,31,40,49,34,20,24] | $V_{10,9,8,8,7,7,6,6,6,1}$ [96] | |
| | [1,2,3,0,2,0,0,1,0,0] | [1,3,7,14,21,30,39,48,34,20,24] | $V_{10,9,8,8,7,7,7,5,5,2}$ [96] | |
| | [1,2,3,1,0,0,2,0,0,0] | [1,3,7,14,22,30,38,48,34,20,24] | $V_{10,9,8,8,7,7,7,6,3,3}$ [64] | |
| | [1,3,0,3,1,0,0,1,0,0] | [1,3,8,13,21,30,39,48,34,20,24] | $V_{10,9,8,8,8,6,6,6,5,2}$ [96] | |
| | [1,4,0,0,1,3,0,0,0,0] | [1,3,9,15,21,28,38,48,34,20,24] | $V_{10,9,8,8,8,8,5,4,4,4}$ [32] | |
| | [2,0,3,2,1,0,0,1,0,0] | [1,4,7,13,21,30,39,48,34,20,24] | $V_{10,9,9,7,7,7,6,6,5,2}$ [96] | |
| | [2,0,4,0,1,1,1,0,0,0] | [1,4,7,14,21,29,38,48,34,20,24] | $V_{10,9,9,7,7,7,7,5,4,3}$ [72] | |
| | [2,1,1,2,2,0,1,0,0,0] | [1,4,8,13,20,29,38,48,34,20,24] | $V_{10,9,9,8,7,6,6,5,5,3}$ [96] | |
| | [2,1,2,0,2,2,0,0,0,0] | [1,4,8,14,20,28,38,48,34,20,24] | $V_{10,9,9,8,7,7,5,5,4,4}$ [48] | |
| | [2,4,1,0,2,0,0,0,1,1] | [0,2,8,15,22,31,40,49,34,20,24] | $V_{9,9,8,8,8,8,7,5,5,1}$ [120] | |
| | [2,4,1,1,0,0,1,1,0,0] | [0,2,8,15,23,31,39,48,34,20,24] | $V_{9,9,8,8,8,8,7,6,3,2}$ [128] | |
| | [2,5,0,0,0,2,0,1,0,0] | [0,2,9,16,23,30,39,48,34,20,24] | $V_{9,9,8,8,8,8,8,4,4,2}$ [60] | |
| | [3,0,0,3,1,2,0,0,0,0] | [1,5,9,13,20,28,38,48,34,20,24] | $V_{10,9,9,9,6,6,6,5,4,4}$ [32] | |
| | [3,1,3,1,1,0,0,0,1,1] | [0,3,7,14,22,31,40,49,34,20,24] | $V_{9,9,9,8,7,7,7,6,5,1}$ [160] | |
| | [3,1,4,0,0,0,1,1,0,0] | [0,3,7,15,23,31,39,48,34,20,24] | $V_{9,9,9,8,7,7,7,7,3,2}$ [80] | |
| | [3,2,1,1,2,0,0,1,0,0] | [0,3,8,14,21,30,39,48,34,20,24] | $V_{9,9,9,8,8,7,6,5,5,2}$ [128] | |
| | [3,2,1,2,0,0,2,0,0,0] | [0,3,8,14,22,30,38,48,34,20,24] | $V_{9,9,9,8,8,7,6,6,3,3}$ [64] | |
| | [3,2,2,0,0,2,1,0,0,0] | [0,3,8,15,22,29,38,48,34,20,24] | $V_{9,9,9,8,8,7,7,4,4,3}$ [64] | |
| | [3,3,0,0,2,1,1,0,0,0] | [0,3,9,15,21,29,38,48,34,20,24] | $V_{9,9,9,8,8,8,5,5,4,3}$ [64] | |
| | [4,0,1,4,0,0,0,0,1,1] | [0,4,8,13,22,31,40,49,34,20,24] | $V_{9,9,9,9,7,6,6,6,6,1}$ [72] | |
| | [4,0,2,1,1,1,1,0,0,0] | [0,4,8,14,21,29,38,48,34,20,24] | $V_{9,9,9,9,7,7,6,5,4,3}$ [96] | |
| | [4,1,1,0,1,3,0,0,0,0] | [0,4,9,15,21,28,38,48,34,20,24] | $V_{9,9,9,9,8,7,5,4,4,4}$ [48] | |
| | [5,0,0,0,4,0,1,0,0,0] | [0,5,10,15,20,29,38,48,34,20,24] | $V_{9,9,9,9,9,5,5,5,5,3}$ [30] | |
| | [0,0,6,0,1,0,1,0,0,0] | [2,4,6,14,22,31,40,50,35,20,25] | $V_{10,10,7,7,7,7,7,7,5,3}$ [36] | |
| | [0,1,3,1,3,0,0,0,0,0] | [2,4,7,13,20,30,40,50,35,20,25] | $V_{10,10,8,7,7,7,6,5,5,5}$ [24] | |
| | [0,2,0,5,0,1,0,0,0,0] | [2,4,8,12,21,30,40,50,35,20,25] | $V_{10,10,8,8,6,6,6,6,6,4}$ [27] | |
| | [0,4,2,1,1,0,1,0,0,0] | [1,2,7,14,22,31,40,50,35,20,25] | $V_{10,8,8,8,8,7,7,6,5,3}$ [72] | |
| | [0,5,0,2,0,2,0,0,0,0] | [1,2,8,14,22,30,40,50,35,20,25] | $V_{10,8,8,8,8,8,6,6,4,4}$ [27] | |
| | [1,0,1,4,2,0,0,0,0,0] | [2,5,8,12,20,30,40,50,35,20,25] | $V_{10,10,9,7,6,6,6,6,5,5}$ [24] | |
| | [1,1,5,1,0,0,0,1,0,0] | [1,3,6,14,23,32,41,50,35,20,25] | $V_{10,9,8,7,7,7,7,7,6,2}$ [80] | |
| | [1,2,2,2,1,1,0,0,0,0] | [1,3,7,13,21,30,40,50,35,20,25] | $V_{10,9,8,8,7,7,6,6,5,4}$ [64] | |
| | [1,3,1,0,4,0,0,0,0,0] | [1,3,8,14,20,30,40,50,35,20,25] | $V_{10,9,8,8,8,7,5,5,5,5}$ [24] | |
| | [1,6,1,0,1,0,0,0,1,1] | [0,1,8,16,24,33,42,51,35,20,25] | $V_{9,8,8,8,8,8,8,7,5,1}$ [120] | |
| | [1,7,0,0,0,0,1,1,0,0] | [0,1,9,17,25,33,41,50,35,20,25] | $V_{9,8,8,8,8,8,8,8,3,2}$ [48] | |
| | [2,3,2,2,0,0,0,1,0,0] | [0,2,7,14,23,32,41,50,35,20,25] | $V_{9,9,8,8,8,7,7,6,6,2}$ [80] | |
| | [2,3,3,0,0,1,1,0,0,0] | [0,2,7,15,23,31,40,50,35,20,25] | $V_{9,9,8,8,8,7,7,7,4,3}$ [64] | |
| | [2,4,0,2,1,0,1,0,0,0] | [0,2,8,14,22,31,40,50,35,20,25] | $V_{9,9,8,8,8,8,6,6,5,3}$ [72] | |
| | [2,4,1,0,1,2,0,0,0,0] | [0,2,8,15,22,30,40,50,35,20,25] | $V_{9,9,8,8,8,8,7,5,4,4}$ [48] | |
| | [3,1,3,1,0,2,0,0,0,0] | [0,3,7,14,22,30,40,50,35,20,25] | $V_{9,9,9,8,7,7,7,6,4,4}$ [48] | |
| | [3,2,0,4,0,0,1,0,0,0] | [0,3,8,13,22,31,40,50,35,20,25] | $V_{9,9,9,8,8,6,6,6,6,3}$ [48] | |
| | [4,0,1,3,1,1,0,0,0,0] | [0,4,8,13,21,30,40,50,35,20,25] | $V_{9,9,9,9,7,6,6,6,5,4}$ [48] | |
| | [4,1,0,1,4,0,0,0,0,0] | [0,4,9,14,20,30,40,50,35,20,25] | $V_{9,9,9,9,8,6,5,5,5,5}$ [24] | |
| | [0,3,5,0,0,0,1,0,0,0] | [1,2,6,15,24,33,42,52,36,20,26] | $V_{10,8,8,8,7,7,7,7,7,3}$ [30] | |
| | [1,1,5,0,2,0,0,0,0,0] | [1,3,6,14,22,32,42,52,36,20,26] | $V_{10,9,8,7,7,7,7,7,5,5}$ [24] | |
| | [1,5,3,0,0,0,0,1,0,0] | [0,1,7,16,25,34,43,52,36,20,26] | $V_{9,8,8,8,8,8,7,7,7,2}$ [48] | |
| | [1,6,0,2,0,0,1,0,0,0] | [0,1,8,15,24,33,42,52,36,20,26] | $V_{9,8,8,8,8,8,8,6,6,3}$ [48] | |
| | [1,6,1,0,0,2,0,0,0,0] | [0,1,8,16,24,32,42,52,36,20,26] | $V_{9,8,8,8,8,8,8,7,4,4}$ [32] | |
| | [2,1,0,6,0,0,0,0,0,0] | [1,4,8,12,22,32,42,52,36,20,26] | $V_{10,9,9,8,6,6,6,6,6,6}$ [12] | |
| | [2,3,2,1,2,0,0,0,0,0] | [0,2,7,14,22,32,42,52,36,20,26] | $V_{9,9,8,8,8,7,7,6,5,5}$ [32] | |
| | [3,0,6,0,0,0,1,0,0,0] | [0,3,6,15,24,33,42,52,36,20,26] | $V_{9,9,9,7,7,7,7,7,7,3}$ [30] | |
| | [3,1,2,3,1,0,0,0,0,0] | [0,3,7,13,22,32,42,52,36,20,26] | $V_{9,9,9,8,7,7,6,6,6,5}$ [32] | |
| | [0,3,4,2,0,0,0,0,0,0] | [1,2,6,14,24,34,44,54,37,20,27] | $V_{10,8,8,8,7,7,7,7,6,6}$ [12] | |
| | [1,5,2,1,1,0,0,0,0,0] | [0,1,7,15,24,34,44,54,37,20,27] | $V_{9,8,8,8,8,8,7,7,6,5}$ [32] | |
| | [2,2,5,0,1,0,0,0,0,0] | [0,2,6,15,24,34,44,54,37,20,27] | $V_{9,9,8,8,7,7,7,7,7,5}$ [24] | |
| | [3,0,5,2,0,0,0,0,0,0] | [0,3,6,14,24,34,44,54,37,20,27] | $V_{9,9,9,7,7,7,7,7,6,6}$ [12] | |
| | [0,9,0,1,0,0,0,0,0,0] | [0,0,9,18,28,38,48,58,39,20,29] | $V_{8,8,8,8,8,8,8,8,8,6}$ [9] | |
| | [0,0,0,0,0,1,0,0,6,2] | [5,10,15,20,25,30,36,42,28,20,20] | $V_{10,10,10,10,10,4,1,1,1,1,1,1}$ [28] | $V_{10,10,10,10,10,4,1,1}$ [28] |
| | [0,0,0,0,0,0,0,4,2,0] | [5,10,15,20,25,30,35,40,29,20,20] | $V_{10,10,10,10,10,2,2,2,2,1,1}$ [13] | $V_{10,10,10,10,10,2,2,2,2}$ [14] |
| | [0,0,1,0,1,1,0,0,4,2] | [4,8,12,17,22,28,35,42,29,20,20] | $V_{10,10,10,10,7,5,4,1,1,1,1}$ [96] | $V_{10,10,10,10,7,5,4,1,1}$ [96] |
| | [0,0,1,1,0,0,0,2,3,1] | [4,8,12,17,23,29,35,41,29,20,20] | $V_{10,10,10,10,7,6,2,2,1,1,1}$ [80] | $V_{10,10,10,10,7,6,2,2,1}$ [80] |
| | [0,1,0,0,0,1,1,1,3,1] | [4,8,13,18,23,28,34,41,29,20,20] | $V_{10,10,10,10,8,4,3,2,1,1,1}$ [120] | $V_{10,10,10,10,8,4,3,2,1}$ [120] |
| | [1,1,0,1,0,0,1,0,4,2] | [3,7,12,17,23,29,35,42,29,20,20] | $V_{10,10,10,9,8,6,3,1,1,1,1}$ [144] | $V_{10,10,10,9,8,6,3,1,1}$ [144] |

| | | | | |
|---|---|---|---|---|
| | [2,0,0,0,0,2,0,0,4,2] | [3,8,13,18,23,28,35,42,29,20,20] | $V_{10,10,10,9,9,4,4,1,1,1,1}$ [48] | $V_{10,10,10,9,9,4,4,1,1}$ [48] |
| | [2,0,0,0,1,0,0,2,3,1] | [3,8,13,18,23,29,35,41,29,20,20] | $V_{10,10,10,9,9,5,2,2,1,1,1}$ [80] | $V_{10,10,10,9,9,5,2,2,1}$ [80] |
| | [3,1,0,0,0,0,0,0,5,3] | [2,7,13,19,25,31,37,43,29,20,20] | $V_{10,10,9,9,9,8,1,1,1,1,1}$ [32] | $V_{10,10,9,9,9,8,1,1,1}$ [32] |
| | [0,0,0,0,3,1,0,0,1,3] | [4,8,12,16,20,27,35,43,31,20,20] | $V_{10,10,10,10,5,5,5,4,1}$ [48] | $V_{10,10,10,10,5,5,5,4,1,1,1}$ [48] |
| | [0,0,1,0,0,1,3,0,0,2] | [4,8,12,17,22,27,33,42,31,20,20] | $V_{10,10,10,10,7,4,3,3,3}$ [64] | $V_{10,10,10,10,7,4,3,3,3,1,1}$ [64] |
| | [0,0,4,0,0,0,0,0,2,4] | [3,6,9,16,23,30,37,44,31,20,20] | $V_{10,10,10,7,7,7,7,1,1}$ [28] | $V_{10,10,10,7,7,7,7,1,1,1,1}$ [28] |
| | [0,1,1,1,1,0,1,0,1,3] | [3,6,10,15,21,28,35,43,31,20,20] | $V_{10,10,10,8,7,6,5,3,1}$ [216] | $V_{10,10,10,8,7,6,5,3,1,1,1}$ [216] |
| | [0,1,2,0,0,1,0,2,0,2] | [3,6,10,16,22,28,35,42,31,20,20] | $V_{10,10,10,8,7,7,4,2,2}$ [108] | $V_{10,10,10,8,7,7,4,2,2,1,1}$ [108] |
| | [0,2,0,0,1,2,0,0,1,3] | [3,6,11,16,21,27,35,43,31,20,20] | $V_{10,10,10,8,8,5,4,4,1}$ [96] | $V_{10,10,10,8,8,5,4,4,1,1,1}$ [96] |
| | [0,2,0,0,2,0,0,2,0,2] | [3,6,11,16,21,28,35,42,31,20,20] | $V_{10,10,10,8,8,5,5,2,2}$ [72] | $V_{10,10,10,8,8,5,5,2,2,1,1}$ [72] |
| | [0,2,0,1,0,0,2,1,0,2] | [3,6,11,16,22,28,34,42,31,20,20] | $V_{10,10,10,8,8,6,3,3,2}$ [108] | $V_{10,10,10,8,8,6,3,3,2,1,1}$ [108] |
| | [1,0,0,2,0,2,0,0,1,3] | [3,7,11,15,21,27,35,43,31,20,20] | $V_{10,10,10,9,6,6,4,4,1}$ [96] | $V_{10,10,10,9,6,6,4,4,1,1,1}$ [96] |
| | [1,0,0,2,1,0,0,2,0,2] | [3,7,11,15,21,28,35,42,31,20,20] | $V_{10,10,10,9,6,6,5,2,2}$ [96] | $V_{10,10,10,9,6,6,5,2,2,1,1}$ [96] |
| | [1,0,1,0,1,1,1,1,0,2] | [3,7,11,16,21,27,34,42,31,20,20] | $V_{10,10,10,9,7,5,4,3,2}$ [216] | $V_{10,10,10,9,7,5,4,3,2,1,1}$ [216] |
| | [1,2,1,0,1,0,0,1,1,3] | [2,5,10,16,22,29,36,43,31,20,20] | $V_{10,10,9,8,8,7,5,2,1}$ [192] | $V_{10,10,9,8,8,7,5,2,1,1,1}$ [192] |
| | [1,3,0,0,0,0,2,0,1,3] | [2,5,11,17,23,29,35,43,31,20,20] | $V_{10,10,9,8,8,8,3,3,1}$ [72] | $V_{10,10,9,8,8,8,3,3,1,1,1}$ [72] |
| | [2,0,0,0,0,0,4,0,0,2] | [3,8,13,18,23,28,33,42,31,20,20] | $V_{10,10,10,9,9,3,3,3,3}$ [28] | $V_{10,10,10,9,9,3,3,3,3,1,1}$ [28] |
| | [2,0,1,2,0,0,0,1,1,3] | [2,6,10,15,22,29,36,43,31,20,20] | $V_{10,10,9,9,7,6,6,2,1}$ [120] | $V_{10,10,9,9,7,6,6,2,1,1,1}$ [120] |
| | [2,0,2,0,0,1,1,0,1,3] | [2,6,10,16,22,28,35,43,31,20,20] | $V_{10,10,9,9,7,7,4,3,1}$ [144] | $V_{10,10,9,9,7,7,4,3,1,1,1}$ [144] |
| | [2,1,0,0,2,0,1,0,1,3] | [2,6,11,16,21,28,35,43,31,20,20] | $V_{10,10,9,9,8,5,5,3,1}$ [144] | $V_{10,10,9,9,8,5,5,3,1,1,1}$ [144] |
| | [2,1,0,1,0,1,0,2,0,2] | [2,6,11,16,22,28,35,42,31,20,20] | $V_{10,10,9,9,8,6,4,2,2}$ [162] | $V_{10,10,9,9,8,6,4,2,2,1,1}$ [162] |
| | [3,0,0,0,0,3,0,0,1,3] | [2,7,12,17,22,27,35,43,31,20,20] | $V_{10,10,9,9,9,4,4,4,1}$ [48] | $V_{10,10,9,9,9,4,4,4,1,1,1}$ [48] |
| | [3,0,0,0,1,0,2,1,0,2] | [2,7,12,17,22,28,34,42,31,20,20] | $V_{10,10,9,9,9,5,3,3,2}$ [90] | $V_{10,10,9,9,9,5,3,3,2,1,1}$ [90] |
| | [3,2,0,0,1,0,0,0,2,4] | [1,5,11,17,23,30,37,44,31,20,20] | $V_{10,9,9,9,8,8,5,1,1}$ [80] | $V_{10,9,9,9,8,8,5,1,1,1,1}$ [80] |
| | [4,0,0,2,0,0,0,0,2,4] | [1,6,11,16,23,30,37,44,31,20,20] | $V_{10,9,9,9,9,6,6,1,1}$ [48] | $V_{10,9,9,9,9,6,6,1,1,1,1}$ [48] |
| | [4,0,1,0,0,1,0,1,1,3] | [1,6,11,17,23,29,36,43,31,20,20] | $V_{10,9,9,9,9,7,4,2,1}$ [144] | $V_{10,9,9,9,9,7,4,2,1,1,1}$ [144] |
| | [0,0,3,1,0,0,1,0,0,4] | [3,6,9,15,22,29,36,44,32,20,20] | $V_{10,10,10,7,7,7,6,3}$ [64] | $V_{10,10,10,7,7,7,6,3,1,1,1,1}$ [64] |
| | [0,4,1,0,0,0,0,0,1,5] | [2,4,10,17,24,31,38,45,32,20,20] | $V_{10,10,8,8,8,8,7,1}$ [42] | $V_{10,10,8,8,8,8,7,1,1,1,1,1}$ [42] |
| | [1,0,0,1,3,0,0,0,0,4] | [3,7,11,15,20,28,36,44,32,20,20] | $V_{10,10,10,9,6,5,5,5}$ [48] | $V_{10,10,10,9,6,5,5,5,1,1,1,1}$ [48] |
| | [1,1,3,0,0,0,0,1,0,4] | [2,5,9,16,23,30,37,44,32,20,20] | $V_{10,10,9,8,7,7,7,2}$ [72] | $V_{10,10,9,8,7,7,7,2,1,1,1,1}$ [72] |
| | [1,2,0,2,0,0,1,0,0,4] | [2,5,10,15,22,29,36,44,32,20,20] | $V_{10,10,9,8,8,6,6,3}$ [96] | $V_{10,10,9,8,8,6,6,3,1,1,1,1}$ [96] |
| | [1,2,1,0,0,2,0,0,0,4] | [2,5,10,16,22,28,36,44,32,20,20] | $V_{10,10,9,8,8,7,4,4}$ [80] | $V_{10,10,9,8,8,7,4,4,1,1,1,1}$ [80] |
| | [2,0,1,1,1,1,0,0,0,4] | [2,6,10,15,21,28,36,44,32,20,20] | $V_{10,10,9,9,7,6,5,4}$ [120] | $V_{10,10,9,9,7,6,5,4,1,1,1,1}$ [120] |
| | [3,1,1,1,0,0,0,1,0,4] | [1,5,10,16,23,30,37,44,32,20,20] | $V_{10,9,9,9,8,7,6,2}$ [120] | $V_{10,9,9,9,8,7,6,2,1,1,1,1}$ [120] |
| | [3,2,0,0,0,1,1,0,0,4] | [1,5,11,17,23,29,36,44,32,20,20] | $V_{10,9,9,9,8,8,4,3}$ [80] | $V_{10,9,9,9,8,8,4,3,1,1,1,1}$ [80] |
| | [4,0,0,1,1,0,1,0,0,4] | [1,6,11,16,22,29,36,44,32,20,20] | $V_{10,9,9,9,9,6,5,3}$ [96] | $V_{10,9,9,9,9,6,5,3,1,1,1,1}$ [96] |
| | [2,4,0,0,0,0,0,0,0,6] | [1,4,11,18,25,32,39,46,33,20,20] | $V_{10,9,9,8,8,8,8}$ [18] | $V_{10,9,9,8,8,8,8,1,1,1,1,1,1}$ [18] |
| | [6,0,0,1,0,0,0,0,0,6] | [0,6,12,18,25,32,39,46,33,20,20] | $V_{9,9,9,9,9,9,6}$ [28] | $V_{9,9,9,9,9,9,6,1,1,1,1,1,1}$ [28] |
| | [0,1,1,0,0,0,0,0,7,1] | [4,8,13,19,25,31,37,43,28,20,21] | $V_{10,10,10,10,8,7,1,1,1,1,1,1,1}$ [42] | $V_{10,10,10,10,8,7,1}$ [42] |
| | [1,0,0,0,1,0,0,1,6,0] | [4,9,14,19,24,30,36,42,28,20,21] | $V_{10,10,10,10,9,5,2,1,1,1,1,1,1}$ [60] | $V_{10,10,10,10,9,5,2}$ [60] |
| | [0,0,0,2,0,1,0,1,4,0] | [4,8,12,16,22,28,35,42,29,20,21] | $V_{10,10,10,10,6,6,4,2,1,1,1,1}$ [67] | $V_{10,10,10,10,6,6,4,2}$ [68] |
| | [0,0,1,0,1,0,2,0,4,0] | [4,8,12,17,22,28,34,42,29,20,21] | $V_{10,10,10,10,7,5,3,3,1,1,1,1}$ [72] | $V_{10,10,10,10,7,5,3,3}$ [72] |
| | [0,2,1,0,0,1,0,0,5,1] | [3,6,11,17,23,29,36,43,29,20,21] | $V_{10,10,10,8,8,7,4,1,1,1,1,1}$ [96] | $V_{10,10,10,8,8,7,4,1}$ [96] |
| | [0,3,0,0,0,0,0,2,4,0] | [3,6,12,18,24,30,36,42,29,20,21] | $V_{10,10,10,8,8,8,2,2,1,1,1,1}$ [31] | $V_{10,10,10,8,8,8,2,2}$ [32] |
| | [1,0,1,1,1,0,0,0,5,1] | [3,7,11,16,22,29,36,43,29,20,21] | $V_{10,10,10,9,7,6,5,1,1,1,1,1}$ [120] | $V_{10,10,10,9,7,6,5,1}$ [120] |
| | [1,0,2,0,0,0,1,1,4,0] | [3,7,11,17,23,29,35,42,29,20,21] | $V_{10,10,10,9,7,7,3,2,1,1,1,1}$ [90] | $V_{10,10,10,9,7,7,3,2}$ [90] |
| | [1,1,0,0,1,1,0,1,4,0] | [3,7,12,17,22,28,35,42,29,20,21] | $V_{10,10,10,9,8,5,4,2,1,1,1,1}$ [144] | $V_{10,10,10,9,8,5,4,2}$ [144] |
| | [2,0,0,0,0,1,2,0,4,0] | [3,8,13,18,23,28,34,42,29,20,21] | $V_{10,10,10,9,9,4,3,3,1,1,1,1}$ [48] | $V_{10,10,10,9,9,4,3,3}$ [48] |
| | [2,2,0,0,0,0,1,0,5,1] | [2,6,12,18,24,30,36,43,29,20,21] | $V_{10,10,9,9,8,8,3,1,1,1,1,1}$ [72] | $V_{10,10,9,9,8,8,3,1}$ [72] |
| | [3,0,0,1,0,1,0,0,5,1] | [2,7,12,17,23,29,36,43,29,20,21] | $V_{10,10,9,9,9,6,4,1,1,1,1,1}$ [96] | $V_{10,10,9,9,9,6,4,1}$ [96] |
| | [3,0,1,0,0,0,0,2,4,0] | [2,7,12,18,24,30,36,42,29,20,21] | $V_{10,10,9,9,9,7,2,2,1,1,1,1}$ [54] | $V_{10,10,9,9,9,7,2,2}$ [54] |
| | [0,0,0,0,3,1,0,0,3,1] | [4,8,12,16,20,27,35,43,30,20,21] | $V_{10,10,10,10,5,5,5,4,1,1,1}$ [48] | $V_{10,10,10,10,5,5,5,4,1}$ [48] |
| | [0,0,1,0,0,1,3,0,2,0] | [4,8,12,17,22,27,33,42,30,20,21] | $V_{10,10,10,10,7,4,3,3,3,1,1}$ [64] | $V_{10,10,10,10,7,4,3,3,3}$ [64] |
| | [0,1,1,1,1,0,1,0,3,1] | [3,6,10,15,21,28,35,43,30,20,21] | $V_{10,10,10,8,7,6,5,3,1,1,1}$ [216] | $V_{10,10,10,8,7,6,5,3,1}$ [216] |
| | [0,1,2,0,0,1,0,2,2,0] | [3,6,10,16,22,28,35,42,30,20,21] | $V_{10,10,10,8,7,7,4,2,2,1,1}$ [108] | $V_{10,10,10,8,7,7,4,2,2}$ [108] |
| | [0,2,0,0,1,2,0,0,3,1] | [3,6,11,16,21,27,35,43,30,20,21] | $V_{10,10,10,8,8,5,4,4,1,1,1}$ [96] | $V_{10,10,10,8,8,5,4,4,1}$ [96] |
| | [0,2,0,1,0,0,2,1,2,0] | [3,6,11,16,22,28,34,42,30,20,21] | $V_{10,10,10,8,8,6,3,3,2,1,1}$ [108] | $V_{10,10,10,8,8,6,3,3,2}$ [108] |
| | [1,0,0,2,0,2,0,0,3,1] | [3,7,11,15,21,27,35,43,30,20,21] | $V_{10,10,10,9,6,6,4,4,1,1,1}$ [96] | $V_{10,10,10,9,6,6,4,4,1}$ [96] |
| | [1,0,0,2,1,0,0,2,2,0] | [3,7,11,15,21,28,35,42,30,20,21] | $V_{10,10,10,9,6,6,5,2,2,1,1}$ [96] | $V_{10,10,10,9,6,6,5,2,2}$ [96] |
| | [1,0,1,0,1,1,1,1,2,0] | [3,7,11,16,21,27,34,42,30,20,21] | $V_{10,10,10,9,7,5,4,3,2,1,1}$ [216] | $V_{10,10,10,9,7,5,4,3,2}$ [216] |
| | [1,2,1,0,1,0,0,1,3,1] | [2,5,10,16,22,29,36,43,30,20,21] | $V_{10,10,9,8,8,7,5,2,1,1,1}$ [192] | $V_{10,10,9,8,8,7,5,2,1}$ [192] |
| | [1,3,0,0,0,0,2,0,3,1] | [2,5,11,17,23,29,35,43,30,20,21] | $V_{10,10,9,8,8,8,3,3,1,1,1}$ [72] | $V_{10,10,9,8,8,8,3,3,1}$ [72] |
| | [2,0,1,2,0,0,0,1,3,1] | [2,6,10,15,22,29,36,43,30,20,21] | $V_{10,10,9,9,7,6,6,2,1,1,1}$ [120] | $V_{10,10,9,9,7,6,6,2,1}$ [120] |
| | [2,0,2,0,0,1,1,0,3,1] | [2,6,10,16,22,28,35,43,30,20,21] | $V_{10,10,9,9,7,7,4,3,1,1,1}$ [144] | $V_{10,10,9,9,7,7,4,3,1}$ [144] |
| | [2,1,0,0,2,0,1,0,3,1] | [2,6,11,16,21,28,35,43,30,20,21] | $V_{10,10,9,9,8,5,5,3,1,1,1}$ [144] | $V_{10,10,9,9,8,5,5,3,1}$ [144] |
| | [2,1,0,1,0,1,0,2,2,0] | [2,6,11,16,22,28,35,42,30,20,21] | $V_{10,10,9,9,8,6,4,2,2,1,1}$ [162] | $V_{10,10,9,9,8,6,4,2,2}$ [162] |
| | [3,0,0,0,1,0,2,1,2,0] | [2,7,12,17,22,28,34,42,30,20,21] | $V_{10,10,9,9,9,5,3,3,2,1,1}$ [90] | $V_{10,10,9,9,9,5,3,3,2}$ [90] |
| | [3,2,0,0,1,0,0,0,4,2] | [1,5,11,17,23,30,37,44,30,20,21] | $V_{10,9,9,9,8,8,5,1,1,1,1}$ [80] | $V_{10,9,9,9,8,8,5,1,1}$ [80] |
| | [4,0,1,0,0,1,0,1,3,1] | [1,6,11,17,23,29,36,43,30,20,21] | $V_{10,9,9,9,9,7,4,2,1,1,1}$ [144] | $V_{10,9,9,9,9,7,4,2,1}$ [144] |
| | [0,0,2,1,2,0,0,1,0,2] | [3,6,9,14,20,28,36,44,32,20,21] | $V_{10,10,10,7,7,6,5,5,2}$ [96] | $V_{10,10,10,7,7,6,5,5,2,1,1}$ [96] |
| | [0,0,3,0,0,2,1,0,0,2] | [3,6,9,15,21,27,35,44,32,20,21] | $V_{10,10,10,7,7,7,4,4,3}$ [64] | $V_{10,10,10,7,7,7,4,4,3,1,1}$ [64] |

| | | | | |
|---|---|---|---|---|
| | [0,1,0,2,1,1,1,0,0,2] | [3,6,10,14,20,27,35,44,32,20,21] | $V_{10,10,10,8,6,6,5,4,3}$ [144] | $V_{10,10,10,8,6,6,5,4,3,1,1}$ [144] |
| | [0,3,1,0,2,0,0,0,1,3] | [2,4,9,15,21,29,37,45,32,20,21] | $V_{10,10,8,8,8,7,5,5,1}$ [90] | $V_{10,10,8,8,8,7,5,5,1,1,1}$ [90] |
| | [0,3,1,1,0,0,1,1,0,2] | [2,4,9,15,22,29,36,44,32,20,21] | $V_{10,10,8,8,8,7,6,3,2}$ [144] | $V_{10,10,8,8,8,7,6,3,2,1,1}$ [144] |
| | [0,4,0,0,0,2,0,1,0,2] | [2,4,10,16,22,28,36,44,32,20,21] | $V_{10,10,8,8,8,8,4,4,2}$ [68] | $V_{10,10,8,8,8,8,4,4,2,1,1}$ [67] |
| | [1,0,0,1,1,3,0,0,0,2] | [3,7,11,15,20,26,35,44,32,20,21] | $V_{10,10,10,9,6,5,4,4,4}$ [80] | $V_{10,10,10,9,6,5,4,4,4,1,1}$ [80] |
| | [1,0,4,0,0,1,0,0,1,3] | [2,5,8,15,22,29,37,45,32,20,21] | $V_{10,10,9,7,7,7,7,4,1}$ [96] | $V_{10,10,9,7,7,7,7,4,1,1,1}$ [96] |
| | [1,1,1,2,0,1,0,1,0,2] | [2,5,9,14,21,28,36,44,32,20,21] | $V_{10,10,9,8,7,6,6,4,2}$ [216] | $V_{10,10,9,8,7,6,6,4,2,1,1}$ [216] |
| | [1,1,2,0,1,0,2,0,0,2] | [2,5,9,15,21,28,35,44,32,20,21] | $V_{10,10,9,8,7,7,5,3,3}$ [144] | $V_{10,10,9,8,7,7,5,3,3,1,1}$ [144] |
| | [1,2,0,0,3,0,0,1,0,2] | [2,5,10,15,20,28,36,44,32,20,21] | $V_{10,10,9,8,8,5,5,5,2}$ [96] | $V_{10,10,9,8,8,5,5,5,2,1,1}$ [96] |
| | [1,2,0,1,0,2,1,0,0,2] | [2,5,10,15,21,27,35,44,32,20,21] | $V_{10,10,9,8,8,6,4,4,3}$ [144] | $V_{10,10,9,8,8,6,4,4,3,1,1}$ [144] |
| | [2,0,0,2,2,0,0,1,0,2] | [2,6,10,14,20,28,36,44,32,20,21] | $V_{10,10,9,9,6,6,5,5,2}$ [96] | $V_{10,10,9,9,6,6,5,5,2,1,1}$ [96] |
| | [2,0,0,3,0,0,2,0,0,2] | [2,6,10,14,21,28,35,44,32,20,21] | $V_{10,10,9,9,6,6,6,3,3}$ [64] | $V_{10,10,9,9,6,6,6,3,3,1,1}$ [64] |
| | [2,0,1,0,2,1,1,0,0,2] | [2,6,10,15,20,27,35,44,32,20,21] | $V_{10,10,9,9,7,5,5,4,3}$ [144] | $V_{10,10,9,9,7,5,5,4,3,1,1}$ [144] |
| | [2,2,1,1,0,1,0,0,1,3] | [1,4,9,15,22,29,37,45,32,20,21] | $V_{10,9,9,8,8,7,6,4,1}$ [192] | $V_{10,9,9,8,8,7,6,4,1,1,1}$ [192] |
| | [2,3,0,0,1,0,1,1,0,2] | [1,4,10,16,22,29,36,44,32,20,21] | $V_{10,9,9,8,8,8,5,3,2}$ [144] | $V_{10,9,9,8,8,8,5,3,2,1,1}$ [144] |
| | [3,0,2,0,2,0,0,0,1,3] | [1,5,9,15,21,29,37,45,32,20,21] | $V_{10,9,9,9,7,7,5,5,1}$ [90] | $V_{10,9,9,9,7,7,5,5,1,1,1}$ [90] |
| | [3,0,2,1,0,0,1,1,0,2] | [1,5,9,15,22,29,36,44,32,20,21] | $V_{10,9,9,9,7,7,6,3,2}$ [144] | $V_{10,9,9,9,7,7,6,3,2,1,1}$ [144] |
| | [3,1,0,1,1,1,0,1,0,2] | [1,5,10,15,21,28,36,44,32,20,21] | $V_{10,9,9,9,8,6,5,4,2}$ [216] | $V_{10,9,9,9,8,6,5,4,2,1,1}$ [216] |
| | [3,1,1,0,0,1,2,0,0,2] | [1,5,10,16,22,28,35,44,32,20,21] | $V_{10,9,9,9,8,7,4,3,3}$ [128] | $V_{10,9,9,9,8,7,4,3,3,1,1}$ [128] |
| | [4,2,1,0,0,0,0,1,1,3] | [0,4,10,17,24,31,38,45,32,20,21] | $V_{9,9,9,9,8,8,7,2,1}$ [96] | $V_{9,9,9,9,8,8,7,2,1,1,1}$ [96] |
| | [5,0,1,1,0,0,1,0,1,3] | [0,5,10,16,23,30,37,45,32,20,21] | $V_{9,9,9,9,9,7,6,3,1}$ [144] | $V_{9,9,9,9,9,7,6,3,1,1,1}$ [144] |
| | [5,1,0,0,0,2,0,0,1,3] | [0,5,11,17,23,29,37,45,32,20,21] | $V_{9,9,9,9,9,8,4,4,1}$ [80] | $V_{9,9,9,9,9,8,4,4,1,1,1}$ [80] |
| | [5,1,0,0,1,0,0,2,0,2] | [0,5,11,17,23,30,37,44,32,20,21] | $V_{9,9,9,9,9,8,5,2,2}$ [96] | $V_{9,9,9,9,9,8,5,2,2,1,1}$ [96] |
| | [6,0,0,0,0,0,2,1,0,2] | [0,6,12,18,24,30,36,44,32,20,21] | $V_{9,9,9,9,9,9,3,3,2}$ [42] | $V_{9,9,9,9,9,9,3,3,2,1,1}$ [42] |
| | [0,2,3,0,1,0,0,0,0,4] | [2,4,8,15,22,30,38,46,33,20,21] | $V_{10,10,8,8,7,7,7,5}$ [54] | $V_{10,10,8,8,7,7,7,5,1,1,1,1}$ [54] |
| | [1,0,3,2,0,0,0,0,0,4] | [2,5,8,14,22,30,38,46,33,20,21] | $V_{10,10,9,7,7,7,6,6}$ [42] | $V_{10,10,9,7,7,7,6,6,1,1,1,1}$ [42] |
| | [1,5,0,0,0,0,1,0,0,4] | [1,3,10,17,24,31,38,46,33,20,21] | $V_{10,9,8,8,8,8,8,3}$ [48] | $V_{10,9,8,8,8,8,8,3,1,1,1,1}$ [48] |
| | [3,0,1,3,0,0,0,0,0,4] | [1,5,9,14,22,30,38,46,33,20,21] | $V_{10,9,9,9,7,6,6,6}$ [42] | $V_{10,9,9,9,7,6,6,6,1,1,1,1}$ [42] |
| | [4,2,0,1,0,1,0,0,0,4] | [0,4,10,16,23,30,38,46,33,20,21] | $V_{9,9,9,9,8,8,6,4}$ [90] | $V_{9,9,9,9,8,8,6,4,1,1,1,1}$ [90] |
| | [5,0,1,0,2,0,0,0,0,4] | [0,5,10,16,22,30,38,46,33,20,21] | $V_{9,9,9,9,9,7,5,5}$ [54] | $V_{9,9,9,9,9,7,5,5,1,1,1,1}$ [54] |
| | [0,2,0,2,0,0,0,0,6,0] | [3,6,11,16,23,30,37,44,29,20,22] | $V_{10,10,10,8,8,6,6,1,1,1,1,1,1}$ [31] | $V_{10,10,10,8,8,6,6}$ [32] |
| | [2,1,1,0,1,0,0,0,6,0] | [2,6,11,17,23,30,37,44,29,20,22] | $V_{10,10,9,9,8,7,5,1,1,1,1,1,1}$ [72] | $V_{10,10,9,9,8,7,5}$ [72] |
| | [0,4,1,0,0,0,0,0,5,1] | [2,4,10,17,24,31,38,45,30,20,22] | $V_{10,10,8,8,8,8,7,1,1,1,1,1}$ [42] | $V_{10,10,8,8,8,8,7,1}$ [42] |
| | [1,0,0,1,3,0,0,0,4,0] | [3,7,11,15,20,28,36,44,30,20,22] | $V_{10,10,10,9,6,5,5,5,1,1,1,1}$ [48] | $V_{10,10,10,9,6,5,5,5}$ [48] |
| | [1,2,0,2,0,0,1,0,4,0] | [2,5,10,15,22,29,36,44,30,20,22] | $V_{10,10,9,8,8,6,6,3,1,1,1,1}$ [96] | $V_{10,10,9,8,8,6,6,3}$ [96] |
| | [1,2,1,0,0,2,0,0,4,0] | [2,5,10,16,22,28,36,44,30,20,22] | $V_{10,10,9,8,8,7,4,4,1,1,1,1}$ [80] | $V_{10,10,9,8,8,7,4,4}$ [80] |
| | [2,0,1,1,1,1,0,0,4,0] | [2,6,10,15,21,28,36,44,30,20,22] | $V_{10,10,9,9,7,6,5,4,1,1,1,1}$ [120] | $V_{10,10,9,9,7,6,5,4}$ [120] |
| | [3,1,1,1,0,0,0,1,4,0] | [1,5,10,16,23,30,37,44,30,20,22] | $V_{10,9,9,9,8,7,6,2,1,1,1,1}$ [120] | $V_{10,9,9,9,8,7,6,2}$ [120] |
| | [3,2,0,0,0,1,1,0,4,0] | [1,5,11,17,23,29,36,44,30,20,22] | $V_{10,9,9,9,8,8,4,3,1,1,1,1}$ [80] | $V_{10,9,9,9,8,8,4,3}$ [80] |
| | [4,0,0,1,1,0,1,0,4,0] | [1,6,11,16,22,29,36,44,30,20,22] | $V_{10,9,9,9,9,6,5,3,1,1,1,1}$ [96] | $V_{10,9,9,9,9,6,5,3}$ [96] |
| | [0,0,2,1,2,0,0,1,2,0] | [3,6,9,14,20,28,36,44,31,20,22] | $V_{10,10,10,7,7,6,5,5,2,1,1}$ [96] | $V_{10,10,10,7,7,6,5,5,2}$ [96] |
| | [0,0,2,2,0,0,2,0,2,0] | [3,6,9,14,21,28,35,44,31,20,22] | $V_{10,10,10,7,7,6,6,3,3,1,1}$ [64] | $V_{10,10,10,7,7,6,6,3,3}$ [64] |
| | [0,0,3,0,0,2,1,0,2,0] | [3,6,9,15,21,27,35,44,31,20,22] | $V_{10,10,10,7,7,7,4,4,3,1,1}$ [64] | $V_{10,10,10,7,7,7,4,4,3}$ [64] |
| | [0,1,0,2,1,1,1,0,2,0] | [3,6,10,14,20,27,35,44,31,20,22] | $V_{10,10,10,8,6,6,5,4,3,1,1}$ [144] | $V_{10,10,10,8,6,6,5,4,3}$ [144] |
| | [0,2,0,0,0,4,0,0,2,0] | [3,6,11,16,21,26,35,44,31,20,22] | $V_{10,10,10,8,8,4,4,4,4,1,1}$ [37] | $V_{10,10,10,8,8,4,4,4,4}$ [38] |
| | [0,3,1,0,2,0,0,0,3,1] | [2,4,9,15,21,29,37,45,31,20,22] | $V_{10,10,8,8,8,7,5,5,1,1,1}$ [90] | $V_{10,10,8,8,8,7,5,5,1}$ [90] |
| | [0,3,1,1,0,0,1,1,2,0] | [2,4,9,15,22,29,36,44,31,20,22] | $V_{10,10,8,8,8,7,6,3,2,1,1}$ [144] | $V_{10,10,8,8,8,7,6,3,2}$ [144] |
| | [0,4,0,0,0,2,0,1,2,0] | [2,4,10,16,22,28,36,44,31,20,22] | $V_{10,10,8,8,8,8,4,4,2,1,1}$ [67] | $V_{10,10,8,8,8,8,4,4,2}$ [68] |
| | [1,0,0,1,1,3,0,0,2,0] | [3,7,11,15,20,26,35,44,31,20,22] | $V_{10,10,10,9,6,5,4,4,4,1,1}$ [80] | $V_{10,10,10,9,6,5,4,4,4}$ [80] |
| | [1,1,1,2,0,1,0,1,2,0] | [2,5,9,14,21,28,36,44,31,20,22] | $V_{10,10,9,8,7,6,6,4,2,1,1}$ [216] | $V_{10,10,9,8,7,6,6,4,2}$ [216] |
| | [1,1,2,0,1,0,2,0,2,0] | [2,5,9,15,21,28,35,44,31,20,22] | $V_{10,10,9,8,7,7,5,3,3,1,1}$ [144] | $V_{10,10,9,8,7,7,5,3,3}$ [144] |
| | [1,2,0,0,3,0,0,1,2,0] | [2,5,10,15,20,28,36,44,31,20,22] | $V_{10,10,9,8,8,5,5,5,2,1,1}$ [96] | $V_{10,10,9,8,8,5,5,5,2}$ [96] |
| | [1,2,0,1,0,2,1,0,2,0] | [2,5,10,15,21,27,35,44,31,20,22] | $V_{10,10,9,8,8,6,4,4,3,1,1}$ [144] | $V_{10,10,9,8,8,6,4,4,3}$ [144] |
| | [2,0,0,2,2,0,0,1,2,0] | [2,6,10,14,20,28,36,44,31,20,22] | $V_{10,10,9,9,6,6,5,5,2,1,1}$ [96] | $V_{10,10,9,9,6,6,5,5,2}$ [96] |
| | [2,0,0,3,0,0,2,0,2,0] | [2,6,10,14,21,28,35,44,31,20,22] | $V_{10,10,9,9,6,6,6,3,3,1,1}$ [64] | $V_{10,10,9,9,6,6,6,3,3}$ [64] |
| | [2,0,1,0,2,1,1,0,2,0] | [2,6,10,15,20,27,35,44,31,20,22] | $V_{10,10,9,9,7,5,5,4,3,1,1}$ [144] | $V_{10,10,9,9,7,5,5,4,3}$ [144] |
| | [2,2,1,1,0,1,0,0,3,1] | [1,4,9,15,22,29,37,45,31,20,22] | $V_{10,9,9,8,8,7,6,4,1,1,1}$ [192] | $V_{10,9,9,8,8,7,6,4,1}$ [192] |
| | [2,2,2,0,0,0,0,2,2,0] | [1,4,9,16,23,30,37,44,31,20,22] | $V_{10,9,9,8,8,7,7,2,2,1,1}$ [72] | $V_{10,9,9,8,8,7,7,2,2}$ [72] |
| | [2,3,0,0,1,0,1,1,2,0] | [1,4,10,16,22,29,36,44,31,20,22] | $V_{10,9,9,8,8,8,5,3,2,1,1}$ [144] | $V_{10,9,9,8,8,8,5,3,2}$ [144] |
| | [3,0,2,0,2,0,0,0,3,1] | [1,5,9,15,21,29,37,45,31,20,22] | $V_{10,9,9,9,7,7,5,5,1,1,1}$ [90] | $V_{10,9,9,9,7,7,5,5,1}$ [90] |
| | [3,0,2,1,0,0,1,1,2,0] | [1,5,9,15,22,29,36,44,31,20,22] | $V_{10,9,9,9,7,7,6,3,2,1,1}$ [144] | $V_{10,9,9,9,7,7,6,3,2}$ [144] |
| | [3,1,0,1,1,1,0,1,2,0] | [1,5,10,15,21,28,36,44,31,20,22] | $V_{10,9,9,9,8,6,5,4,2,1,1}$ [216] | $V_{10,9,9,9,8,6,5,4,2}$ [216] |
| | [3,1,1,0,0,1,2,0,2,0] | [1,5,10,16,22,28,35,44,31,20,22] | $V_{10,9,9,9,8,7,4,3,3,1,1}$ [128] | $V_{10,9,9,9,8,7,4,3,3}$ [128] |
| | [4,0,0,0,2,0,2,0,2,0] | [1,6,11,16,21,28,35,44,31,20,22] | $V_{10,9,9,9,9,5,5,3,3,1,1}$ [60] | $V_{10,9,9,9,9,5,5,3,3}$ [60] |
| | [4,2,1,0,0,0,0,1,3,1] | [0,4,10,17,24,31,38,45,31,20,22] | $V_{9,9,9,9,8,8,7,2,1,1,1}$ [96] | $V_{9,9,9,9,8,8,7,2,1}$ [96] |
| | [5,0,1,1,0,0,1,0,3,1] | [0,5,10,16,23,30,37,45,31,20,22] | $V_{9,9,9,9,9,7,6,3,1,1,1}$ [144] | $V_{9,9,9,9,9,7,6,3,1}$ [144] |
| | [5,1,0,0,0,2,0,0,3,1] | [0,5,11,17,23,29,37,45,31,20,22] | $V_{9,9,9,9,9,8,4,4,1,1,1}$ [80] | $V_{9,9,9,9,9,8,4,4,1}$ [80] |
| | [5,1,0,0,1,0,0,2,2,0] | [0,5,11,17,23,30,37,44,31,20,22] | $V_{9,9,9,9,9,8,5,2,2,1,1}$ [96] | $V_{9,9,9,9,9,8,5,2,2}$ [96] |
| | [6,0,0,0,0,0,2,1,2,0] | [0,6,12,18,24,30,36,44,31,20,22] | $V_{9,9,9,9,9,9,3,3,2,1,1}$ [42] | $V_{9,9,9,9,9,9,3,3,2}$ [42] |
| | [0,1,5,0,0,0,0,0,1,3] | [2,4,7,15,23,31,39,47,33,20,22] | $V_{10,10,8,7,7,7,7,7,1}$ [42] | $V_{10,10,8,7,7,7,7,7,1,1,1}$ [42] |
| | [0,2,2,1,0,2,0,0,0,2] | [2,4,8,14,21,28,37,46,33,20,22] | $V_{10,10,8,8,7,7,6,4,4}$ [90] | $V_{10,10,8,8,7,7,6,4,4,1,1}$ [90] |

| | | | | |
|---|---|---|---|---|
| | [0,3,0,1,2,1,0,0,0,2] | [2,4,9,14,20,28,37,46,33,20,22] | $V_{10,10,8,8,8,6,5,5,4}$ [90] | $V_{10,10,8,8,8,6,5,5,4,1,1}$ [90] |
| | [1,0,2,3,0,0,1,0,0,2] | [2,5,8,13,21,29,37,46,33,20,22] | $V_{10,10,9,7,7,6,6,6,3}$ [96] | $V_{10,10,9,7,7,6,6,6,3,1,1}$ [96] |
| | [1,0,3,0,2,1,0,0,0,2] | [2,5,8,14,20,28,37,46,33,20,22] | $V_{10,10,9,7,7,7,5,5,4}$ [90] | $V_{10,10,9,7,7,7,5,5,4,1,1}$ [90] |
| | [1,1,0,3,1,1,0,0,0,2] | [2,5,9,13,20,28,37,46,33,20,22] | $V_{10,10,9,8,6,6,6,5,4}$ [120] | $V_{10,10,9,8,6,6,6,5,4,1,1}$ [120] |
| | [1,3,2,0,1,0,0,1,0,2] | [1,3,8,15,22,30,38,46,33,20,22] | $V_{10,9,8,8,8,7,7,5,2}$ [144] | $V_{10,9,8,8,8,7,7,5,2,1,1}$ [144] |
| | [1,4,0,1,0,1,1,0,0,2] | [1,3,9,15,22,29,37,46,33,20,22] | $V_{10,9,8,8,8,8,6,4,3}$ [144] | $V_{10,9,8,8,8,8,6,4,3,1,1}$ [144] |
| | [2,1,2,1,1,0,1,0,0,2] | [1,4,8,14,21,29,37,46,33,20,22] | $V_{10,9,9,8,7,7,6,5,3}$ [192] | $V_{10,9,9,8,7,7,6,5,3,1,1}$ [192] |
| | [2,2,0,2,0,2,0,0,0,2] | [1,4,9,14,21,28,37,46,33,20,22] | $V_{10,9,9,8,8,6,6,4,4}$ [90] | $V_{10,9,9,8,8,6,6,4,4,1,1}$ [90] |
| | [3,0,1,1,2,1,0,0,0,2] | [1,5,9,14,20,28,37,46,33,20,22] | $V_{10,9,9,9,7,6,5,5,4}$ [120] | $V_{10,9,9,9,7,6,5,5,4,1,1}$ [120] |
| | [3,3,0,2,0,0,0,0,1,3] | [0,3,9,15,23,31,39,47,33,20,22] | $V_{9,9,9,8,8,8,6,6,1}$ [72] | $V_{9,9,9,8,8,8,6,6,1,1,1}$ [72] |
| | [3,3,1,0,0,1,0,1,0,2] | [0,3,9,16,23,30,38,46,33,20,22] | $V_{9,9,9,8,8,8,7,4,2}$ [144] | $V_{9,9,9,8,8,8,7,4,2,1,1}$ [144] |
| | [4,0,3,1,0,0,0,0,1,3] | [0,4,8,15,23,31,39,47,33,20,22] | $V_{9,9,9,9,7,7,7,6,1}$ [72] | $V_{9,9,9,9,7,7,7,6,1,1,1}$ [72] |
| | [4,1,1,1,0,1,1,0,0,2] | [0,4,9,15,22,29,37,46,33,20,22] | $V_{9,9,9,9,8,7,6,4,3}$ [192] | $V_{9,9,9,9,8,7,6,4,3,1,1}$ [192] |
| | [5,0,0,1,2,0,1,0,0,2] | [0,5,10,15,21,29,37,46,33,20,22] | $V_{9,9,9,9,9,6,5,5,3}$ [96] | $V_{9,9,9,9,9,6,5,5,3,1,1}$ [96] |
| | [5,0,1,0,0,3,0,0,0,2] | [0,5,10,16,22,28,37,46,33,20,22] | $V_{9,9,9,9,9,7,4,4,4}$ [60] | $V_{9,9,9,9,9,7,4,4,4,1,1}$ [60] |
| | [3,2,3,0,0,0,0,0,0,4] | [0,3,8,16,24,32,40,48,34,20,22] | $V_{9,9,9,8,8,7,7,7}$ [32] | $V_{9,9,9,8,8,7,7,7,1,1,1,1}$ [32] |
| | [6,0,0,1,0,0,0,0,6,0] | [0,6,12,18,25,32,39,46,30,20,23] | $V_{9,9,9,9,9,9,6,1,1,1,1,1,1}$ [28] | $V_{9,9,9,9,9,9,6}$ [28] |
| | [0,3,0,3,0,0,0,0,4,0] | [2,4,9,14,22,30,38,46,31,20,23] | $V_{10,10,8,8,8,6,6,6,1,1,1,1}$ [31] | $V_{10,10,8,8,8,6,6,6}$ [32] |
| | [1,5,0,0,0,0,1,0,4,0] | [1,3,10,17,24,31,38,46,31,20,23] | $V_{10,9,8,8,8,8,8,3,1,1,1,1}$ [48] | $V_{10,9,8,8,8,8,8,3}$ [48] |
| | [3,0,1,3,0,0,0,0,4,0] | [1,5,9,14,22,30,38,46,31,20,23] | $V_{10,9,9,9,7,6,6,6,1,1,1,1}$ [42] | $V_{10,9,9,9,7,6,6,6}$ [42] |
| | [4,2,0,1,0,1,0,0,4,0] | [0,4,10,16,23,30,38,46,31,20,23] | $V_{9,9,9,9,8,8,6,4,1,1,1,1}$ [90] | $V_{9,9,9,9,8,8,6,4}$ [90] |
| | [5,0,1,0,2,0,0,0,4,0] | [0,5,10,16,22,30,38,46,31,20,23] | $V_{9,9,9,9,9,7,5,5,1,1,1,1}$ [54] | $V_{9,9,9,9,9,7,5,5}$ [54] |
| | [0,2,2,1,0,2,0,0,2,0] | [2,4,8,14,21,28,37,46,32,20,23] | $V_{10,10,8,8,7,7,6,4,4,1,1}$ [90] | $V_{10,10,8,8,7,7,6,4,4}$ [90] |
| | [0,3,0,1,2,1,0,0,2,0] | [2,4,9,14,20,28,37,46,32,20,23] | $V_{10,10,8,8,8,6,5,5,4,1,1}$ [90] | $V_{10,10,8,8,8,6,5,5,4}$ [90] |
| | [1,0,2,3,0,0,1,0,2,0] | [2,5,8,13,21,29,37,46,32,20,23] | $V_{10,10,9,7,7,6,6,6,3,1,1}$ [96] | $V_{10,10,9,7,7,6,6,6,3}$ [96] |
| | [1,0,3,0,2,1,0,0,2,0] | [2,5,8,14,20,28,37,46,32,20,23] | $V_{10,10,9,7,7,7,5,5,4,1,1}$ [90] | $V_{10,10,9,7,7,7,5,5,4}$ [90] |
| | [1,1,0,3,1,1,0,0,2,0] | [2,5,9,13,20,28,37,46,32,20,23] | $V_{10,10,9,8,6,6,6,5,4,1,1}$ [120] | $V_{10,10,9,8,6,6,6,5,4}$ [120] |
| | [1,3,2,0,1,0,0,1,2,0] | [1,3,8,15,22,30,38,46,32,20,23] | $V_{10,9,8,8,8,7,7,5,2,1,1}$ [144] | $V_{10,9,8,8,8,7,7,5,2}$ [144] |
| | [1,4,0,1,0,1,1,0,2,0] | [1,3,9,15,22,29,37,46,32,20,23] | $V_{10,9,8,8,8,8,6,4,3,1,1}$ [144] | $V_{10,9,8,8,8,8,6,4,3}$ [144] |
| | [2,1,2,1,1,0,1,0,2,0] | [1,4,8,14,21,29,37,46,32,20,23] | $V_{10,9,9,8,7,7,6,5,3,1,1}$ [192] | $V_{10,9,9,8,7,7,6,5,3}$ [192] |
| | [3,0,1,1,2,1,0,0,2,0] | [1,5,9,14,20,28,37,46,32,20,23] | $V_{10,9,9,9,7,6,5,5,4,1,1}$ [120] | $V_{10,9,9,9,7,6,5,5,4}$ [120] |
| | [3,3,0,2,0,0,0,0,3,1] | [0,3,9,15,23,31,39,47,32,20,23] | $V_{9,9,9,8,8,8,6,6,1,1,1}$ [72] | $V_{9,9,9,8,8,8,6,6,1}$ [72] |
| | [3,3,1,0,0,1,0,1,2,0] | [0,3,9,16,23,30,38,46,32,20,23] | $V_{9,9,9,8,8,8,7,4,2,1,1}$ [144] | $V_{9,9,9,8,8,8,7,4,2}$ [144] |
| | [4,0,3,1,0,0,0,0,3,1] | [0,4,8,15,23,31,39,47,32,20,23] | $V_{9,9,9,9,7,7,7,6,1,1,1}$ [72] | $V_{9,9,9,9,7,7,7,6,1}$ [72] |
| | [4,1,1,1,0,1,1,0,2,0] | [0,4,9,15,22,29,37,46,32,20,23] | $V_{9,9,9,9,8,7,6,4,3,1,1}$ [192] | $V_{9,9,9,9,8,7,6,4,3}$ [192] |
| | [5,0,0,1,2,0,1,0,2,0] | [0,5,10,15,21,29,37,46,32,20,23] | $V_{9,9,9,9,9,6,5,5,3,1,1}$ [96] | $V_{9,9,9,9,9,6,5,5,3}$ [96] |
| | [5,0,1,0,0,3,0,0,2,0] | [0,5,10,16,22,28,37,46,32,20,23] | $V_{9,9,9,9,9,7,4,4,4,1,1}$ [60] | $V_{9,9,9,9,9,7,4,4,4}$ [60] |
| | [0,1,3,2,1,0,0,0,0,2] | [2,4,7,13,21,30,39,48,34,20,23] | $V_{10,10,8,7,7,7,6,6,5}$ [72] | $V_{10,10,8,7,7,7,6,6,5,1,1}$ [72] |
| | [0,5,1,1,0,0,1,0,0,2] | [1,2,8,15,23,31,39,48,34,20,23] | $V_{10,8,8,8,8,8,7,6,3}$ [96] | $V_{10,8,8,8,8,8,7,6,3,1,1}$ [96] |
| | [1,2,3,1,0,1,0,0,0,2] | [1,3,7,14,22,30,39,48,34,20,23] | $V_{10,9,8,8,7,7,7,6,4}$ [120] | $V_{10,9,8,8,7,7,7,6,4,1,1}$ [120] |
| | [2,4,2,0,0,0,0,1,0,2] | [0,2,8,16,24,32,40,48,34,20,23] | $V_{9,9,8,8,8,8,7,7,2}$ [72] | $V_{9,9,8,8,8,8,7,7,2,1,1}$ [72] |
| | [2,5,0,0,1,0,1,0,0,2] | [0,2,9,16,23,31,39,48,34,20,23] | $V_{9,9,8,8,8,8,8,5,3}$ [96] | $V_{9,9,8,8,8,8,8,5,3,1,1}$ [96] |
| | [3,2,1,2,0,1,0,0,0,2] | [0,3,8,14,22,30,39,48,34,20,23] | $V_{9,9,9,8,8,7,6,6,4}$ [120] | $V_{9,9,9,8,8,7,6,6,4,1,1}$ [120] |
| | [3,3,0,0,3,0,0,0,0,2] | [0,3,9,15,21,30,39,48,34,20,23] | $V_{9,9,9,8,8,8,5,5,5}$ [48] | $V_{9,9,9,8,8,8,5,5,5,1,1}$ [48] |
| | [4,0,2,1,2,0,0,0,0,2] | [0,4,8,14,21,30,39,48,34,20,23] | $V_{9,9,9,9,7,7,6,5,5}$ [72] | $V_{9,9,9,9,7,7,6,5,5,1,1}$ [72] |
| | [3,2,3,0,0,0,0,0,4,0] | [0,3,8,16,24,32,40,48,32,20,24] | $V_{9,9,9,8,8,7,7,7,1,1,1,1}$ [32] | $V_{9,9,9,8,8,7,7,7}$ [32] |
| | [0,0,0,6,0,0,0,0,2,0] | [3,6,9,12,21,30,39,48,33,20,24] | $V_{10,10,10,6,6,6,6,6,6,1,1}$ [17] | $V_{10,10,10,6,6,6,6,6,6}$ [18] |
| | [0,1,3,2,1,0,0,0,2,0] | [2,4,7,13,21,30,39,48,33,20,24] | $V_{10,10,8,7,7,7,6,6,5,1,1}$ [72] | $V_{10,10,8,7,7,7,6,6,5}$ [72] |
| | [0,5,1,1,0,0,1,0,2,0] | [1,2,8,15,23,31,39,48,33,20,24] | $V_{10,8,8,8,8,8,7,6,3,1,1}$ [96] | $V_{10,8,8,8,8,8,7,6,3}$ [96] |
| | [0,6,0,0,0,2,0,0,2,0] | [1,2,9,16,23,30,39,48,33,20,24] | $V_{10,8,8,8,8,8,8,4,4,1,1}$ [37] | $V_{10,8,8,8,8,8,8,4,4}$ [38] |
| | [1,2,3,1,0,1,0,0,2,0] | [1,3,7,14,22,30,39,48,33,20,24] | $V_{10,9,8,8,7,7,7,6,4,1,1}$ [120] | $V_{10,9,8,8,7,7,7,6,4}$ [120] |
| | [2,0,4,0,2,0,0,0,2,0] | [1,4,7,14,21,30,39,48,33,20,24] | $V_{10,9,9,7,7,7,7,5,5,1,1}$ [54] | $V_{10,9,9,7,7,7,7,5,5}$ [54] |
| | [2,4,2,0,0,0,0,1,2,0] | [0,2,8,16,24,32,40,48,33,20,24] | $V_{9,9,8,8,8,8,7,7,2,1,1}$ [72] | $V_{9,9,8,8,8,8,7,7,2}$ [72] |
| | [2,5,0,0,1,0,1,0,2,0] | [0,2,9,16,23,31,39,48,33,20,24] | $V_{9,9,8,8,8,8,8,5,3,1,1}$ [96] | $V_{9,9,8,8,8,8,8,5,3}$ [96] |
| | [3,2,1,2,0,1,0,0,2,0] | [0,3,8,14,22,30,39,48,33,20,24] | $V_{9,9,9,8,8,7,6,6,4,1,1}$ [120] | $V_{9,9,9,8,8,7,6,6,4}$ [120] |
| | [3,3,0,0,3,0,0,0,2,0] | [0,3,9,15,21,30,39,48,33,20,24] | $V_{9,9,9,8,8,8,5,5,5,1,1}$ [48] | $V_{9,9,9,8,8,8,5,5,5}$ [48] |
| | [4,0,2,1,2,0,0,0,2,0] | [0,4,8,14,21,30,39,48,33,20,24] | $V_{9,9,9,9,7,7,6,5,5,1,1}$ [72] | $V_{9,9,9,9,7,7,6,5,5}$ [72] |
| | [0,0,6,1,0,0,0,0,0,2] | [2,4,6,14,23,32,41,50,35,20,24] | $V_{10,10,7,7,7,7,7,7,6}$ [28] | $V_{10,10,7,7,7,7,7,7,6,1,1}$ [28] |
| | [0,4,2,2,0,0,0,0,0,2] | [1,2,7,14,23,32,41,50,35,20,24] | $V_{10,8,8,8,8,7,7,6,6}$ [42] | $V_{10,8,8,8,8,7,7,6,6,1,1}$ [42] |
| | [2,3,3,0,1,0,0,0,0,2] | [0,2,7,15,23,32,41,50,35,20,24] | $V_{9,9,8,8,8,7,7,7,5}$ [72] | $V_{9,9,8,8,8,7,7,7,5,1,1}$ [72] |
| | [2,4,0,3,0,0,0,0,0,2] | [0,2,8,14,23,32,41,50,35,20,24] | $V_{9,9,8,8,8,8,6,6,6}$ [42] | $V_{9,9,8,8,8,8,6,6,6,1,1}$ [42] |
| | [0,0,6,1,0,0,0,0,2,0] | [2,4,6,14,23,32,41,50,34,20,25] | $V_{10,10,7,7,7,7,7,7,6,1,1}$ [28] | $V_{10,10,7,7,7,7,7,7,6}$ [28] |
| | [2,3,3,0,1,0,0,0,2,0] | [0,2,7,15,23,32,41,50,34,20,25] | $V_{9,9,8,8,8,7,7,7,5,1,1}$ [72] | $V_{9,9,8,8,8,7,7,7,5}$ [72] |
| | [2,4,0,3,0,0,0,0,2,0] | [0,2,8,14,23,32,41,50,34,20,25] | $V_{9,9,8,8,8,8,6,6,6,1,1}$ [42] | $V_{9,9,8,8,8,8,6,6,6}$ [42] |
| 21 | [0,0,0,0,0,1,1,1,4,1] | [5,10,15,20,25,30,36,43,30,21,21] | $W_{10,10,10,10,10,4,3,2,1,1,1,1}$ [56] | $W_{10,10,10,10,10,4,3,2,1}$ [56] |
| | [0,1,1,0,0,0,1,0,5,2] | [4,8,13,19,25,31,37,44,30,21,21] | $W_{10,10,10,10,8,7,3,1,1,1,1,1}$ [90] | $W_{10,10,10,10,8,7,3,1,1}$ [90] |
| | [1,0,0,0,1,1,0,0,5,2] | [4,9,14,19,24,30,37,44,30,21,21] | $W_{10,10,10,10,9,5,4,1,1,1,1,1}$ [80] | $W_{10,10,10,10,9,5,4,1,1}$ [80] |
| | [1,0,0,1,0,0,0,2,4,1] | [4,9,14,19,25,31,37,43,30,21,21] | $W_{10,10,10,10,9,6,2,2,1,1,1,1}$ [80] | $W_{10,10,10,10,9,6,2,2,1}$ [80] |
| | [2,1,0,0,0,0,0,1,5,2] | [3,8,14,20,26,32,38,44,30,21,21] | $W_{10,10,10,9,9,8,2,1,1,1,1,1}$ [56] | $W_{10,10,10,9,9,8,2,1,1}$ [56] |
| | [0,0,0,0,0,1,0,4,1,0] | [5,10,15,20,25,30,36,42,31,21,21] | $W_{10,10,10,10,10,4,2,2,2,2,1}$ [31] | $W_{10,10,10,10,10,4,2,2,2,2}$ [32] |
| | [0,0,1,1,0,1,1,0,3,2] | [4,8,12,17,23,29,36,44,31,21,21] | $W_{10,10,10,10,7,6,4,3,1,1,1}$ [144] | $W_{10,10,10,10,7,6,4,3,1,1}$ [144] |

| | | | | |
|---|---|---|---|---|
| | [0,0,2,0,0,0,1,2,2,1] | [4,8,12,18,24,30,36,43,31,21,21] | $W_{10,10,10,10,7,7,3,2,2,1,1}$ [80] | $W_{10,10,10,10,7,7,3,2,2,1}$ [80] |
| | [0,1,0,0,1,1,0,2,2,1] | [4,8,13,18,23,29,36,43,31,21,21] | $W_{10,10,10,10,8,5,4,2,2,1,1}$ [144] | $W_{10,10,10,10,8,5,4,2,2,1}$ [144] |
| | [0,3,0,0,1,0,0,0,4,3] | [3,6,12,18,24,31,38,45,31,21,21] | $W_{10,10,10,8,8,8,5,1,1,1,1}$ [60] | $W_{10,10,10,8,8,8,5,1,1,1}$ [60] |
| | [1,0,0,0,0,1,2,1,2,1] | [4,9,14,19,24,29,35,43,31,21,21] | $W_{10,10,10,10,9,4,3,3,2,1,1}$ [96] | $W_{10,10,10,10,9,4,3,3,2,1}$ [96] |
| | [1,0,2,1,0,0,0,0,4,3] | [3,7,11,17,24,31,38,45,31,21,21] | $W_{10,10,10,9,7,7,6,1,1,1,1}$ [72] | $W_{10,10,10,9,7,7,6,1,1,1}$ [72] |
| | [1,1,0,1,1,0,0,1,3,2] | [3,7,12,17,23,30,37,44,31,21,21] | $W_{10,10,10,9,8,6,5,2,1,1,1}$ [192] | $W_{10,10,10,9,8,6,5,2,1,1}$ [192] |
| | [1,1,1,0,0,0,2,0,3,2] | [3,7,12,18,24,30,36,44,31,21,21] | $W_{10,10,10,9,8,7,3,3,1,1,1}$ [120] | $W_{10,10,10,9,8,7,3,3,1,1}$ [120] |
| | [1,2,0,0,0,0,0,3,2,1] | [3,7,13,19,25,31,37,43,31,21,21] | $W_{10,10,10,9,8,8,2,2,2,1,1}$ [56] | $W_{10,10,10,9,8,8,2,2,2,1}$ [56] |
| | [2,0,0,0,1,1,1,0,3,2] | [3,8,13,18,23,29,36,44,31,21,21] | $W_{10,10,10,9,9,5,4,3,1,1,1}$ [120] | $W_{10,10,10,9,9,5,4,3,1,1}$ [120] |
| | [2,0,0,1,0,0,1,2,2,1] | [3,8,13,18,24,30,36,43,31,21,21] | $W_{10,10,10,9,9,6,3,2,2,1,1}$ [128] | $W_{10,10,10,9,9,6,3,2,2,1}$ [128] |
| | [3,0,1,0,1,0,0,0,4,3] | [2,7,12,18,24,31,38,45,31,21,21] | $W_{10,10,9,9,9,7,5,1,1,1,1}$ [90] | $W_{10,10,9,9,9,7,5,1,1,1}$ [90] |
| | [3,1,0,0,0,0,1,1,3,2] | [2,7,13,19,25,31,37,44,31,21,21] | $W_{10,10,9,9,9,8,3,2,1,1,1}$ [96] | $W_{10,10,9,9,9,8,3,2,1,1}$ [96] |
| | [0,0,0,2,1,0,1,1,1,2] | [4,8,12,16,22,29,36,44,32,21,21] | $W_{10,10,10,10,6,6,5,3,2,1}$ [120] | $W_{10,10,10,10,6,6,5,3,2,1,1}$ [120] |
| | [0,0,1,0,1,2,0,1,1,2] | [4,8,12,17,22,28,36,44,32,21,21] | $W_{10,10,10,10,7,5,4,4,2,1}$ [144] | $W_{10,10,10,10,7,5,4,4,2,1,1}$ [144] |
| | [0,0,1,1,0,0,3,0,1,2] | [4,8,12,17,23,29,35,44,32,21,21] | $W_{10,10,10,10,7,6,3,3,3,1}$ [96] | $W_{10,10,10,10,7,6,3,3,3,1,1}$ [96] |
| | [0,0,1,1,0,1,0,3,0,1] | [4,8,12,17,23,29,36,43,32,21,21] | $W_{10,10,10,10,7,6,4,2,2,2}$ [108] | $W_{10,10,10,10,7,6,4,2,2,2,1}$ [108] |
| | [0,1,0,0,0,2,2,0,1,2] | [4,8,13,18,23,28,35,44,32,21,21] | $W_{10,10,10,10,8,4,4,3,3,1}$ [90] | $W_{10,10,10,10,8,4,4,3,3,1,1}$ [90] |
| | [0,1,0,0,1,0,2,2,0,1] | [4,8,13,18,23,29,35,43,32,21,21] | $W_{10,10,10,10,8,5,3,3,2,2}$ [108] | $W_{10,10,10,10,8,5,3,3,2,2,1}$ [108] |
| | [0,1,3,0,0,0,0,1,2,3] | [3,6,10,17,24,31,38,45,32,21,21] | $W_{10,10,10,8,7,7,7,2,1,1}$ [72] | $W_{10,10,10,8,7,7,7,2,1,1,1}$ [72] |
| | [0,2,0,2,0,0,1,0,2,3] | [3,6,11,16,23,30,37,45,32,21,21] | $W_{10,10,10,8,8,6,6,3,1,1}$ [108] | $W_{10,10,10,8,8,6,6,3,1,1,1}$ [108] |
| | [0,2,1,0,0,2,0,0,2,3] | [3,6,11,17,23,29,37,45,32,21,21] | $W_{10,10,10,8,8,7,4,4,1,1}$ [96] | $W_{10,10,10,8,8,7,4,4,1,1,1}$ [96] |
| | [0,2,1,0,1,0,0,2,1,2] | [3,6,11,17,23,30,37,44,32,21,21] | $W_{10,10,10,8,8,7,5,2,2,1}$ [144] | $W_{10,10,10,8,8,7,5,2,2,1,1}$ [144] |
| | [0,3,0,0,0,0,2,1,1,2] | [3,6,12,18,24,30,36,44,32,21,21] | $W_{10,10,10,8,8,8,3,3,2,1}$ [72] | $W_{10,10,10,8,8,8,3,3,2,1,1}$ [72] |
| | [1,0,1,1,1,1,0,0,2,3] | [3,7,11,16,22,29,37,45,32,21,21] | $W_{10,10,10,9,7,6,5,4,1,1}$ [192] | $W_{10,10,10,9,7,6,5,4,1,1,1}$ [192] |
| | [1,0,1,2,0,0,0,2,1,2] | [3,7,11,16,23,30,37,44,32,21,21] | $W_{10,10,10,9,7,6,6,2,2,1}$ [120] | $W_{10,10,10,9,7,6,6,2,2,1,1}$ [120] |
| | [1,0,2,0,0,1,1,1,1,2] | [3,7,11,17,23,29,36,44,32,21,21] | $W_{10,10,10,9,7,7,4,3,2,1}$ [192] | $W_{10,10,10,9,7,7,4,3,2,1,1}$ [192] |
| | [1,1,0,0,2,0,1,1,1,2] | [3,7,12,17,22,29,36,44,32,21,21] | $W_{10,10,10,9,8,5,5,3,2,1}$ [192] | $W_{10,10,10,9,8,5,5,3,2,1,1}$ [192] |
| | [1,1,1,0,0,0,1,3,0,1] | [3,7,12,18,24,30,36,43,32,21,21] | $W_{10,10,10,9,8,7,3,2,2,2}$ [120] | $W_{10,10,10,9,8,7,3,2,2,2,1}$ [120] |
| | [1,3,1,0,0,0,0,0,3,4] | [2,5,11,18,25,32,39,46,32,21,21] | $W_{10,10,9,8,8,8,7,1,1,1}$ [56] | $W_{10,10,9,8,8,8,7,1,1,1,1}$ [56] |
| | [2,0,0,0,0,3,0,1,1,2] | [3,8,13,18,23,28,36,44,32,21,21] | $W_{10,10,10,9,9,4,4,4,2,1}$ [72] | $W_{10,10,10,9,9,4,4,4,2,1,1}$ [72] |
| | [2,0,0,0,1,0,3,0,1,2] | [3,8,13,18,23,29,35,44,32,21,21] | $W_{10,10,10,9,9,5,3,3,3,1}$ [90] | $W_{10,10,10,9,9,5,3,3,3,1,1}$ [90] |
| | [2,0,0,0,1,1,0,3,0,1] | [3,8,13,18,23,29,36,43,32,21,21] | $W_{10,10,10,9,9,5,4,2,2,2}$ [90] | $W_{10,10,10,9,9,5,4,2,2,2,1}$ [90] |
| | [2,1,1,0,1,0,1,0,2,3] | [2,6,11,17,23,30,37,45,32,21,21] | $W_{10,10,9,9,8,7,5,3,1,1}$ [216] | $W_{10,10,9,9,8,7,5,3,1,1,1}$ [216] |
| | [2,2,0,0,0,1,0,2,1,2] | [2,6,12,18,24,30,37,44,32,21,21] | $W_{10,10,9,9,8,8,4,2,2,1}$ [120] | $W_{10,10,9,9,8,8,4,2,2,1,1}$ [120] |
| | [3,0,0,1,0,2,0,0,2,3] | [2,7,12,17,23,29,37,45,32,21,21] | $W_{10,10,9,9,9,6,4,4,1,1}$ [96] | $W_{10,10,9,9,9,6,4,4,1,1,1}$ [96] |
| | [3,0,0,1,1,0,0,2,1,2] | [2,7,12,17,23,30,37,44,32,21,21] | $W_{10,10,9,9,9,6,5,2,2,1}$ [128] | $W_{10,10,9,9,9,6,5,2,2,1,1}$ [128] |
| | [3,0,1,0,0,0,2,1,1,2] | [2,7,12,18,24,30,36,44,32,21,21] | $W_{10,10,9,9,9,7,3,3,2,1}$ [120] | $W_{10,10,9,9,9,7,3,3,2,1,1}$ [120] |
| | [4,1,0,1,0,0,0,0,3,4] | [1,6,12,18,25,32,39,46,32,21,21] | $W_{10,9,9,9,9,8,6,1,1,1}$ [72] | $W_{10,9,9,9,9,8,6,1,1,1,1}$ [72] |
| | [5,0,0,0,0,1,0,1,2,3] | [1,7,13,19,25,31,38,45,32,21,21] | $W_{10,9,9,9,9,9,4,2,1,1}$ [72] | $W_{10,9,9,9,9,9,4,2,1,1,1}$ [72] |
| | [0,0,0,1,3,0,0,1,0,3] | [4,8,12,16,21,29,37,45,33,21,21] | $W_{10,10,10,10,6,5,5,5,2}$ [60] | $W_{10,10,10,10,6,5,5,5,2,1,1,1}$ [60] |
| | [0,0,0,2,0,2,1,0,0,3] | [4,8,12,16,22,28,36,45,33,21,21] | $W_{10,10,10,10,6,6,4,4,3}$ [60] | $W_{10,10,10,10,6,6,4,4,3,1,1,1}$ [60] |
| | [0,1,2,0,2,0,0,0,1,4] | [3,6,10,16,22,30,38,46,33,21,21] | $W_{10,10,10,8,7,7,5,5,1}$ [90] | $W_{10,10,10,8,7,7,5,5,1,1,1,1}$ [90] |
| | [0,1,2,1,0,0,1,1,0,3] | [3,6,10,16,23,30,37,45,33,21,21] | $W_{10,10,10,8,7,7,6,3,2}$ [144] | $W_{10,10,10,8,7,7,6,3,2,1,1,1}$ [144] |
| | [0,2,0,1,1,1,0,1,0,3] | [3,6,11,16,22,29,37,45,33,21,21] | $W_{10,10,10,8,8,6,5,4,2}$ [162] | $W_{10,10,10,8,8,6,5,4,2,1,1,1}$ [162] |
| | [0,2,1,0,0,1,2,0,0,3] | [3,6,11,17,23,29,36,45,33,21,21] | $W_{10,10,10,8,8,7,4,3,3}$ [96] | $W_{10,10,10,8,8,7,4,3,3,1,1,1}$ [96] |
| | [1,0,0,3,1,0,0,0,1,4] | [3,7,11,15,22,30,38,46,33,21,21] | $W_{10,10,10,9,6,6,6,5,1}$ [80] | $W_{10,10,10,9,6,6,6,5,1,1,1,1}$ [80] |
| | [1,0,1,1,1,0,2,0,0,3] | [3,7,11,16,22,29,36,45,33,21,21] | $W_{10,10,10,9,7,6,5,3,3}$ [144] | $W_{10,10,10,9,7,6,5,3,3,1,1,1}$ [144] |
| | [1,1,0,0,1,2,1,0,0,3] | [3,7,12,17,22,28,36,45,33,21,21] | $W_{10,10,10,9,8,5,4,4,3}$ [128] | $W_{10,10,10,9,8,5,4,4,3,1,1,1}$ [128] |
| | [1,2,2,0,0,0,1,0,1,4] | [2,5,10,17,24,31,38,46,33,21,21] | $W_{10,10,9,8,8,7,7,3,1}$ [120] | $W_{10,10,9,8,8,7,7,3,1,1,1,1}$ [120] |
| | [1,3,0,0,1,1,0,0,1,4] | [2,5,11,17,23,30,38,46,33,21,21] | $W_{10,10,9,8,8,8,5,4,1}$ [128] | $W_{10,10,9,8,8,8,5,4,1,1,1,1}$ [128] |
| | [1,3,0,1,0,0,0,2,0,3] | [2,5,11,17,24,31,38,45,33,21,21] | $W_{10,10,9,8,8,8,6,2,2}$ [90] | $W_{10,10,9,8,8,8,6,2,2,1,1,1}$ [90] |
| | [2,0,2,1,0,1,0,0,1,4] | [2,6,10,16,23,30,38,46,33,21,21] | $W_{10,10,9,9,7,7,6,4,1}$ [144] | $W_{10,10,9,9,7,7,6,4,1,1,1,1}$ [144] |
| | [2,0,3,0,0,0,0,2,0,3] | [2,6,10,17,24,31,38,45,33,21,21] | $W_{10,10,9,9,7,7,7,2,2}$ [54] | $W_{10,10,9,9,7,7,7,2,2,1,1,1}$ [54] |
| | [2,1,0,1,2,0,0,0,1,4] | [2,6,11,16,22,30,38,46,33,21,21] | $W_{10,10,9,9,8,6,5,5,1}$ [120] | $W_{10,10,9,9,8,6,5,5,1,1,1,1}$ [120] |
| | [2,1,0,2,0,0,1,1,0,3] | [2,6,11,16,23,30,37,45,33,21,21] | $W_{10,10,9,9,8,6,6,3,2}$ [144] | $W_{10,10,9,9,8,6,6,3,2,1,1,1}$ [144] |
| | [2,1,1,0,0,2,0,1,0,3] | [2,6,11,17,23,29,37,45,33,21,21] | $W_{10,10,9,9,8,7,4,4,2}$ [144] | $W_{10,10,9,9,8,7,4,4,2,1,1,1}$ [144] |
| | [2,2,0,0,0,0,3,0,0,3] | [2,6,12,18,24,30,36,45,33,21,21] | $W_{10,10,9,9,8,8,3,3,3}$ [48] | $W_{10,10,9,9,8,8,3,3,3,1,1,1}$ [48] |
| | [3,0,0,0,2,1,0,1,0,3] | [2,7,12,17,22,29,37,45,33,21,21] | $W_{10,10,9,9,9,5,5,4,2}$ [90] | $W_{10,10,9,9,9,5,5,4,2,1,1,1}$ [90] |
| | [3,0,0,1,0,1,2,0,0,3] | [2,7,12,17,23,29,36,45,33,21,21] | $W_{10,10,9,9,9,6,4,3,3}$ [96] | $W_{10,10,9,9,9,6,4,3,3,1,1,1}$ [96] |
| | [3,2,1,0,0,0,0,1,1,4] | [1,5,11,18,25,32,39,46,33,21,21] | $W_{10,9,9,9,8,8,7,2,1}$ [96] | $W_{10,9,9,9,8,8,7,2,1,1,1,1}$ [96] |
| | [4,0,1,1,0,0,1,0,1,4] | [1,6,11,17,24,31,38,46,33,21,21] | $W_{10,9,9,9,9,7,6,3,1}$ [144] | $W_{10,9,9,9,9,7,6,3,1,1,1,1}$ [144] |
| | [4,1,0,0,0,2,0,0,1,4] | [1,6,12,18,24,30,38,46,33,21,21] | $W_{10,9,9,9,9,8,4,4,1}$ [80] | $W_{10,9,9,9,9,8,4,4,1,1,1,1}$ [80] |
| | [4,1,0,0,1,0,0,2,0,3] | [1,6,12,18,24,31,38,45,33,21,21] | $W_{10,9,9,9,9,8,5,2,2}$ [96] | $W_{10,9,9,9,9,8,5,2,2,1,1,1}$ [96] |
| | [5,0,0,0,0,0,2,1,0,3] | [1,7,13,19,25,31,37,45,33,21,21] | $W_{10,9,9,9,9,9,3,3,2}$ [42] | $W_{10,9,9,9,9,9,3,3,2,1,1,1}$ [42] |
| | [0,1,1,3,0,0,0,0,0,5] | [3,6,10,15,23,31,39,47,34,21,21] | $W_{10,10,10,8,7,6,6,6}$ [42] | $W_{10,10,10,8,7,6,6,6,1,1,1,1,1}$ [42] |
| | [1,2,1,1,1,0,0,0,0,5] | [2,5,10,16,23,31,39,47,34,21,21] | $W_{10,10,9,8,8,7,6,5}$ [96] | $W_{10,10,9,8,8,7,6,5,1,1,1,1,1}$ [96] |
| | [3,2,0,1,0,1,0,0,0,5] | [1,5,11,17,24,31,39,47,34,21,21] | $W_{10,9,9,9,8,8,6,4}$ [90] | $W_{10,9,9,9,8,8,6,4,1,1,1,1,1}$ [90] |
| | [4,0,1,0,2,0,0,0,0,5] | [1,6,11,17,23,31,39,47,34,21,21] | $W_{10,9,9,9,9,7,5,5}$ [54] | $W_{10,9,9,9,9,7,5,5,1,1,1,1,1}$ [54] |
| | [6,1,0,0,0,0,0,0,1,6] | [0,6,13,20,27,34,41,48,34,21,21] | $W_{9,9,9,9,9,9,8,1}$ [32] | $W_{9,9,9,9,9,9,8,1,1,1,1,1,1}$ [32] |
| | [0,0,2,0,1,0,0,0,6,1] | [4,8,12,18,24,31,38,45,30,21,22] | $W_{10,10,10,10,7,7,5,1,1,1,1,1,1}$ [60] | $W_{10,10,10,10,7,7,5,1}$ [60] |
| | [0,1,0,1,0,1,0,1,5,0] | [4,8,13,18,24,30,37,44,30,21,22] | $W_{10,10,10,10,8,6,4,2,1,1,1,1,1}$ [121] | $W_{10,10,10,10,8,6,4,2}$ [122] |

| | | | | |
|---|---|---|---|---|
| | [1,0,0,0,1,0,2,0,5,0] | [4,9,14,19,24,30,36,44,30,21,22] | $W_{10,10,10,10,9,5,3,3,1,1,1,1,1}$ [60] | $W_{10,10,10,10,9,5,3,3}$ [60] |
| | [1,2,0,0,0,1,0,0,6,1] | [3,7,13,19,25,31,38,45,30,21,22] | $W_{10,10,10,9,8,8,4,1,1,1,1,1,1}$ [80] | $W_{10,10,10,9,8,8,4,1}$ [80] |
| | [2,0,0,1,1,0,0,0,6,1] | [3,8,13,18,24,31,38,45,30,21,22] | $W_{10,10,10,9,9,6,5,1,1,1,1,1,1}$ [80] | $W_{10,10,10,9,9,6,5,1}$ [80] |
| | [2,0,1,0,0,0,1,1,5,0] | [3,8,13,19,25,31,37,44,30,21,22] | $W_{10,10,10,9,9,7,3,2,1,1,1,1,1}$ [90] | $W_{10,10,10,9,9,7,3,2}$ [90] |
| | [0,0,0,2,1,1,0,0,4,1] | [4,8,12,16,22,29,37,45,31,21,22] | $W_{10,10,10,10,6,6,5,4,1,1,1,1}$ [80] | $W_{10,10,10,10,6,6,5,4,1}$ [80] |
| | [0,0,0,3,0,0,0,2,3,0] | [4,8,12,16,23,30,37,44,31,21,22] | $W_{10,10,10,10,6,6,6,2,2,1,1,1}$ [37] | $W_{10,10,10,10,6,6,6,2,2}$ [38] |
| | [0,0,1,0,2,0,1,1,3,0] | [4,8,12,17,22,29,36,44,31,21,22] | $W_{10,10,10,10,7,5,5,3,2,1,1,1}$ [108] | $W_{10,10,10,10,7,5,5,3,2}$ [108] |
| | [0,1,0,0,0,3,0,1,3,0] | [4,8,13,18,23,28,36,44,31,21,22] | $W_{10,10,10,10,8,4,4,4,2,1,1,1}$ [67] | $W_{10,10,10,10,8,4,4,4,2}$ [68] |
| | [0,1,0,0,1,0,3,0,3,0] | [4,8,13,18,23,29,35,44,31,21,22] | $W_{10,10,10,10,8,5,3,3,3,1,1,1}$ [72] | $W_{10,10,10,10,8,5,3,3,3}$ [72] |
| | [0,2,1,0,1,0,1,0,4,1] | [3,6,11,17,23,30,37,45,31,21,22] | $W_{10,10,10,8,8,7,5,3,1,1,1,1}$ [162] | $W_{10,10,10,8,8,7,5,3,1}$ [162] |
| | [0,3,0,0,0,1,0,2,3,0] | [3,6,12,18,24,30,37,44,31,21,22] | $W_{10,10,10,8,8,8,4,2,2,1,1,1}$ [67] | $W_{10,10,10,8,8,8,4,2,2}$ [68] |
| | [1,0,1,2,0,0,1,0,4,1] | [3,7,11,16,23,30,37,45,31,21,22] | $W_{10,10,10,9,7,6,6,3,1,1,1,1}$ [144] | $W_{10,10,10,9,7,6,6,3,1}$ [144] |
| | [1,0,2,0,0,2,0,0,4,1] | [3,7,11,17,23,29,37,45,31,21,22] | $W_{10,10,10,9,7,7,4,4,1,1,1,1}$ [96] | $W_{10,10,10,9,7,7,4,4,1}$ [96] |
| | [1,0,2,0,1,0,0,2,3,0] | [3,7,11,17,23,30,37,44,31,21,22] | $W_{10,10,10,9,7,7,5,2,2,1,1,1}$ [108] | $W_{10,10,10,9,7,7,5,2,2}$ [108] |
| | [1,1,0,0,2,1,0,0,4,1] | [3,7,12,17,22,29,37,45,31,21,22] | $W_{10,10,10,9,8,5,5,4,1,1,1,1}$ [128] | $W_{10,10,10,9,8,5,5,4,1}$ [128] |
| | [1,1,0,1,0,1,1,1,3,0] | [3,7,12,17,23,29,36,44,31,21,22] | $W_{10,10,10,9,8,6,4,3,2,1,1,1}$ [216] | $W_{10,10,10,9,8,6,4,3,2}$ [216] |
| | [2,1,1,1,0,0,0,1,4,1] | [2,6,11,17,24,31,38,45,31,21,22] | $W_{10,10,9,9,8,7,6,2,1,1,1,1}$ [160] | $W_{10,10,9,9,8,7,6,2,1}$ [160] |
| | [2,2,0,0,0,1,1,0,4,1] | [2,6,12,18,24,30,37,45,31,21,22] | $W_{10,10,9,9,8,8,4,3,1,1,1,1}$ [120] | $W_{10,10,9,9,8,8,4,3,1}$ [120] |
| | [3,0,0,1,1,0,1,0,4,1] | [2,7,12,17,23,30,37,45,31,21,22] | $W_{10,10,9,9,9,6,5,3,1,1,1,1}$ [144] | $W_{10,10,9,9,9,6,5,3,1}$ [144] |
| | [3,0,1,0,0,1,0,2,3,0] | [2,7,12,18,24,30,37,44,31,21,22] | $W_{10,10,9,9,9,7,4,2,2,1,1,1}$ [108] | $W_{10,10,9,9,9,7,4,2,2}$ [108] |
| | [5,0,0,0,1,0,0,0,5,2] | [1,7,13,19,25,32,39,46,31,21,22] | $W_{10,9,9,9,9,9,5,1,1,1,1,1}$ [50] | $W_{10,9,9,9,9,9,5,1,1}$ [50] |
| | [0,0,0,1,2,1,1,0,2,1] | [4,8,12,16,21,28,36,45,32,21,22] | $W_{10,10,10,10,6,5,5,4,3,1,1}$ [120] | $W_{10,10,10,10,6,5,5,4,3,1}$ [120] |
| | [0,0,0,2,0,2,0,2,1,0] | [4,8,12,16,22,28,36,44,32,21,22] | $W_{10,10,10,10,6,6,4,4,2,2,1}$ [67] | $W_{10,10,10,10,6,6,4,4,2,2}$ [68] |
| | [0,0,1,0,1,1,2,1,1,0] | [4,8,12,17,22,28,35,44,32,21,22] | $W_{10,10,10,10,7,5,4,3,3,2,1}$ [144] | $W_{10,10,10,10,7,5,4,3,3,2}$ [144] |
| | [0,1,1,2,1,0,0,0,3,2] | [3,6,10,15,22,30,38,46,32,21,22] | $W_{10,10,10,8,7,6,6,5,1,1,1}$ [120] | $W_{10,10,10,8,7,6,6,5,1,1}$ [120] |
| | [0,1,2,0,1,1,0,1,2,1] | [3,6,10,16,22,29,37,45,32,21,22] | $W_{10,10,10,8,7,7,5,4,2,1,1}$ [216] | $W_{10,10,10,8,7,7,5,4,2,1}$ [216] |
| | [0,2,0,1,1,0,2,0,2,1] | [3,6,11,16,22,29,36,45,32,21,22] | $W_{10,10,10,8,8,6,5,3,3,1,1}$ [162] | $W_{10,10,10,8,8,6,5,3,3,1}$ [162] |
| | [0,2,0,2,0,0,0,3,1,0] | [3,6,11,16,23,30,37,44,32,21,22] | $W_{10,10,10,8,8,6,6,2,2,2,1}$ [67] | $W_{10,10,10,8,8,6,6,2,2,2}$ [68] |
| | [0,2,1,0,0,1,1,2,1,0] | [3,6,11,17,23,29,36,44,32,21,22] | $W_{10,10,10,8,8,7,4,3,2,2,1}$ [144] | $W_{10,10,10,8,8,7,4,3,2,2}$ [144] |
| | [1,0,0,3,0,1,0,1,2,1] | [3,7,11,15,22,29,37,45,32,21,22] | $W_{10,10,10,9,6,6,6,4,2,1,1}$ [144] | $W_{10,10,10,9,6,6,6,4,2,1}$ [144] |
| | [1,0,1,0,3,0,0,1,2,1] | [3,7,11,16,21,29,37,45,32,21,22] | $W_{10,10,10,9,7,5,5,5,2,1,1}$ [144] | $W_{10,10,10,9,7,5,5,5,2,1}$ [144] |
| | [1,0,1,1,0,2,1,0,2,1] | [3,7,11,16,22,28,36,45,32,21,22] | $W_{10,10,10,9,7,6,4,4,3,1,1}$ [216] | $W_{10,10,10,9,7,6,4,4,3,1}$ [216] |
| | [1,0,1,1,1,0,1,2,1,0] | [3,7,11,16,22,29,36,44,32,21,22] | $W_{10,10,10,9,7,6,5,3,2,2,1}$ [216] | $W_{10,10,10,9,7,6,5,3,2,2}$ [216] |
| | [1,1,0,0,1,2,0,2,1,0] | [3,7,12,17,22,28,36,44,32,21,22] | $W_{10,10,10,9,8,5,4,4,2,2,1}$ [144] | $W_{10,10,10,9,8,5,4,4,2,2}$ [144] |
| | [1,1,0,1,0,0,3,1,1,0] | [3,7,12,17,23,29,35,44,32,21,22] | $W_{10,10,10,9,8,6,3,3,3,2,1}$ [144] | $W_{10,10,10,9,8,6,3,3,3,2}$ [144] |
| | [1,2,1,1,0,1,0,0,3,2] | [2,5,10,16,23,30,38,46,32,21,22] | $W_{10,10,9,8,8,7,6,4,1,1,1}$ [192] | $W_{10,10,9,8,8,7,6,4,1,1}$ [192] |
| | [1,2,2,0,0,0,0,2,2,1] | [2,5,10,17,24,31,38,45,32,21,22] | $W_{10,10,9,8,8,7,7,2,2,1,1}$ [96] | $W_{10,10,9,8,8,7,7,2,2,1}$ [96] |
| | [1,3,0,0,1,0,1,1,2,1] | [2,5,11,17,23,30,37,45,32,21,22] | $W_{10,10,9,8,8,8,5,3,2,1,1}$ [192] | $W_{10,10,9,8,8,8,5,3,2,1}$ [192] |
| | [2,0,0,0,0,2,2,1,1,0] | [3,8,13,18,23,28,35,44,32,21,22] | $W_{10,10,10,9,9,4,4,3,3,2,1}$ [72] | $W_{10,10,10,9,9,4,4,3,3,2}$ [72] |
| | [2,0,2,0,2,0,0,0,3,2] | [2,6,10,16,22,30,38,46,32,21,22] | $W_{10,10,9,9,7,7,5,5,1,1,1}$ [90] | $W_{10,10,9,9,7,7,5,5,1,1}$ [90] |
| | [2,0,2,1,0,0,1,1,2,1] | [2,6,10,16,23,30,37,45,32,21,22] | $W_{10,10,9,9,7,7,6,3,2,1,1}$ [192] | $W_{10,10,9,9,7,7,6,3,2,1}$ [192] |
| | [2,1,0,1,1,1,0,1,2,1] | [2,6,11,16,22,29,37,45,32,21,22] | $W_{10,10,9,9,8,6,5,4,2,1,1}$ [288] | $W_{10,10,9,9,8,6,5,4,2,1}$ [288] |
| | [2,1,1,0,0,1,2,0,2,1] | [2,6,11,17,23,29,36,45,32,21,22] | $W_{10,10,9,9,8,7,4,3,3,1,1}$ [192] | $W_{10,10,9,9,8,7,4,3,3,1}$ [192] |
| | [2,1,1,0,1,0,0,3,1,0] | [2,6,11,17,23,30,37,44,32,21,22] | $W_{10,10,9,9,8,7,5,2,2,2,1}$ [144] | $W_{10,10,9,9,8,7,5,2,2,2}$ [144] |
| | [2,2,0,0,0,0,2,2,1,0] | [2,6,12,18,24,30,36,44,32,21,22] | $W_{10,10,9,9,8,8,3,3,2,2,1}$ [72] | $W_{10,10,9,9,8,8,3,3,2,2}$ [72] |
| | [3,0,0,0,2,0,2,0,2,1] | [2,7,12,17,22,29,36,45,32,21,22] | $W_{10,10,9,9,9,5,5,3,3,1,1}$ [90] | $W_{10,10,9,9,9,5,5,3,3,1}$ [90] |
| | [3,0,0,1,0,1,1,2,1,0] | [2,7,12,17,23,29,36,44,32,21,22] | $W_{10,10,9,9,9,6,4,3,2,2,1}$ [144] | $W_{10,10,9,9,9,6,4,3,2,2}$ [144] |
| | [3,2,0,1,0,0,1,0,3,2] | [1,5,11,17,24,31,38,46,32,21,22] | $W_{10,9,9,9,8,8,6,3,1,1,1}$ [144] | $W_{10,9,9,9,8,8,6,3,1,1}$ [144] |
| | [4,0,1,0,1,1,0,0,3,2] | [1,6,11,17,23,30,38,46,32,21,22] | $W_{10,9,9,9,9,7,5,4,1,1,1}$ [144] | $W_{10,9,9,9,9,7,5,4,1,1}$ [144] |
| | [4,0,1,1,0,0,0,2,2,1] | [1,6,11,17,24,31,38,45,32,21,22] | $W_{10,9,9,9,9,7,6,2,2,1,1}$ [120] | $W_{10,9,9,9,9,7,6,2,2,1}$ [120] |
| | [4,1,0,0,0,1,1,1,2,1] | [1,6,12,18,24,30,37,45,32,21,22] | $W_{10,9,9,9,9,8,4,3,2,1,1}$ [160] | $W_{10,9,9,9,9,8,4,3,2,1}$ [160] |
| | [0,0,0,2,0,1,3,0,0,1] | [4,8,12,16,22,28,35,45,33,21,22] | $W_{10,10,10,10,6,6,4,3,3,3}$ [60] | $W_{10,10,10,10,6,6,4,3,3,3,1}$ [60] |
| | [0,0,1,0,0,4,0,1,0,1] | [4,8,12,17,22,27,36,45,33,21,22] | $W_{10,10,10,10,7,4,4,4,4,2}$ [72] | $W_{10,10,10,10,7,4,4,4,4,2,1}$ [72] |
| | [0,0,3,1,1,0,0,1,1,2] | [3,6,9,15,22,30,38,46,33,21,22] | $W_{10,10,10,7,7,7,6,5,2,1}$ [128] | $W_{10,10,10,7,7,7,6,5,2,1,1}$ [128] |
| | [0,0,4,0,0,0,2,0,1,2] | [3,6,9,16,23,30,37,46,33,21,22] | $W_{10,10,10,7,7,7,7,3,3,1}$ [60] | $W_{10,10,10,7,7,7,7,3,3,1,1}$ [60] |
| | [0,1,1,1,2,0,1,0,1,2] | [3,6,10,15,21,29,37,46,33,21,22] | $W_{10,10,10,8,7,6,5,5,3,1}$ [216] | $W_{10,10,10,8,7,6,5,5,3,1,1}$ [216] |
| | [0,1,1,2,0,1,0,2,0,1] | [3,6,10,15,22,29,37,45,33,21,22] | $W_{10,10,10,8,7,6,6,4,2,2}$ [162] | $W_{10,10,10,8,7,6,6,4,2,2,1}$ [162] |
| | [0,1,2,0,0,3,0,0,1,2] | [3,6,10,16,22,28,37,46,33,21,22] | $W_{10,10,10,8,7,7,4,4,4,1}$ [96] | $W_{10,10,10,8,7,7,4,4,4,1,1}$ [96] |
| | [0,1,2,0,1,0,2,1,0,1] | [3,6,10,16,22,29,36,45,33,21,22] | $W_{10,10,10,8,7,7,5,3,3,2}$ [162] | $W_{10,10,10,8,7,7,5,3,3,2,1}$ [162] |
| | [0,2,0,0,2,2,0,0,1,2] | [3,6,11,16,21,28,37,46,33,21,22] | $W_{10,10,10,8,8,5,5,4,4,1}$ [96] | $W_{10,10,10,8,8,5,5,4,4,1,1}$ [96] |
| | [0,2,0,0,3,0,0,2,0,1] | [3,6,11,16,21,29,37,45,33,21,22] | $W_{10,10,10,8,8,5,5,5,2,2}$ [72] | $W_{10,10,10,8,8,5,5,5,2,2,1}$ [72] |
| | [0,2,0,1,0,2,1,1,0,1] | [3,6,11,16,22,28,36,45,33,21,22] | $W_{10,10,10,8,8,6,4,4,3,2}$ [162] | $W_{10,10,10,8,8,6,4,4,3,2,1}$ [162] |
| | [0,4,0,1,1,0,0,0,2,3] | [2,4,10,16,23,31,39,47,33,21,22] | $W_{10,10,8,8,8,8,6,5,1,1}$ [90] | $W_{10,10,8,8,8,8,6,5,1,1,1}$ [90] |
| | [0,4,1,0,0,0,1,1,1,2] | [2,4,10,17,24,31,38,46,33,21,22] | $W_{10,10,8,8,8,8,7,3,2,1}$ [120] | $W_{10,10,8,8,8,8,7,3,2,1,1}$ [120] |
| | [1,0,0,2,1,2,0,0,1,2] | [3,7,11,15,21,28,37,46,33,21,22] | $W_{10,10,10,9,6,6,5,4,4,1}$ [128] | $W_{10,10,10,9,6,6,5,4,4,1,1}$ [128] |
| | [1,0,0,2,2,0,0,2,0,1] | [3,7,11,15,21,29,37,45,33,21,22] | $W_{10,10,10,9,6,6,5,5,2,2}$ [96] | $W_{10,10,10,9,6,6,5,5,2,2,1}$ [96] |
| | [1,0,0,3,0,0,2,1,0,1] | [3,7,11,15,22,29,36,45,33,21,22] | $W_{10,10,10,9,6,6,6,3,3,2}$ [96] | $W_{10,10,10,9,6,6,6,3,3,2,1}$ [96] |
| | [1,0,1,0,2,1,1,1,0,1] | [3,7,11,16,21,28,36,45,33,21,22] | $W_{10,10,10,9,7,5,5,4,3,2}$ [216] | $W_{10,10,10,9,7,5,5,4,3,2,1}$ [216] |
| | [1,0,2,0,0,0,4,0,0,1] | [3,7,11,17,23,29,35,45,33,21,22] | $W_{10,10,10,9,7,7,3,3,3,3}$ [60] | $W_{10,10,10,9,7,7,3,3,3,3,1}$ [60] |
| | [1,1,0,0,1,1,3,0,0,1] | [3,7,12,17,22,28,35,45,33,21,22] | $W_{10,10,10,9,8,5,4,3,3,3}$ [128] | $W_{10,10,10,9,8,5,4,3,3,3,1}$ [128] |
| | [1,1,2,2,0,0,0,0,2,3] | [2,5,9,15,23,31,39,47,33,21,22] | $W_{10,10,9,8,7,7,6,6,1,1}$ [96] | $W_{10,10,9,8,7,7,6,6,1,1,1}$ [96] |

| | | | | |
|---|---|---|---|---|
| | [1,1,3,0,0,1,0,1,1,2] | [2,5,9,16,23,30,38,46,33,21,22] | $W_{10,10,9,8,7,7,7,4,2,1}$ [192] | $W_{10,10,9,8,7,7,7,4,2,1,1}$ [192] |
| | [1,2,0,2,1,0,0,1,1,2] | [2,5,10,15,22,30,38,46,33,21,22] | $W_{10,10,9,8,8,6,6,5,2,1}$ [192] | $W_{10,10,9,8,8,6,6,5,2,1,1}$ [192] |
| | [1,2,1,0,1,1,1,0,1,2] | [2,5,10,16,22,29,37,46,33,21,22] | $W_{10,10,9,8,8,7,5,4,3,1}$ [288] | $W_{10,10,9,8,8,7,5,4,3,1,1}$ [288] |
| | [1,2,1,1,0,0,1,2,0,1] | [2,5,10,16,23,30,37,45,33,21,22] | $W_{10,10,9,8,8,7,6,3,2,2}$ [192] | $W_{10,10,9,8,8,7,6,3,2,2,1}$ [192] |
| | [1,3,0,0,0,2,0,2,0,1] | [2,5,11,17,23,29,37,45,33,21,22] | $W_{10,10,9,8,8,8,4,4,2,2}$ [90] | $W_{10,10,9,8,8,8,4,4,2,2,1}$ [90] |
| | [2,0,1,2,0,1,1,0,1,2] | [2,6,10,15,22,29,37,46,33,21,22] | $W_{10,10,9,9,7,6,6,4,3,1}$ [216] | $W_{10,10,9,9,7,6,6,4,3,1,1}$ [216] |
| | [2,0,2,0,1,1,0,2,0,1] | [2,6,10,16,22,29,37,45,33,21,22] | $W_{10,10,9,9,7,7,5,4,2,2}$ [162] | $W_{10,10,9,9,7,7,5,4,2,2,1}$ [162] |
| | [2,1,0,0,3,0,1,0,1,2] | [2,6,11,16,21,29,37,46,33,21,22] | $W_{10,10,9,9,8,5,5,5,3,1}$ [144] | $W_{10,10,9,9,8,5,5,5,3,1,1}$ [144] |
| | [2,1,0,1,0,3,0,0,1,2] | [2,6,11,16,22,28,37,46,33,21,22] | $W_{10,10,9,9,8,6,4,4,4,1}$ [144] | $W_{10,10,9,9,8,6,4,4,4,1,1}$ [144] |
| | [2,1,0,1,1,0,2,1,0,1] | [2,6,11,16,22,29,36,45,33,21,22] | $W_{10,10,9,9,8,6,5,3,3,2}$ [216] | $W_{10,10,9,9,8,6,5,3,3,2,1}$ [216] |
| | [2,3,1,0,0,1,0,0,2,3] | [1,4,10,17,24,31,39,47,33,21,22] | $W_{10,9,9,8,8,8,7,4,1,1}$ [128] | $W_{10,9,9,8,8,8,7,4,1,1,1}$ [128] |
| | [2,4,0,0,0,0,0,2,1,2] | [1,4,11,18,25,32,39,46,33,21,22] | $W_{10,9,9,8,8,8,8,2,2,1}$ [56] | $W_{10,9,9,8,8,8,8,2,2,1,1}$ [56] |
| | [3,0,0,0,1,2,1,1,0,1] | [2,7,12,17,22,28,36,45,33,21,22] | $W_{10,10,9,9,9,5,4,4,3,2}$ [120] | $W_{10,10,9,9,9,5,4,4,3,2,1}$ [120] |
| | [3,1,1,1,0,1,0,1,1,2] | [1,5,10,16,23,30,38,46,33,21,22] | $W_{10,9,9,9,8,7,6,4,2,1}$ [288] | $W_{10,9,9,9,8,7,6,4,2,1,1}$ [288] |
| | [3,2,0,0,1,0,2,0,1,2] | [1,5,11,17,23,30,37,46,33,21,22] | $W_{10,9,9,9,8,8,5,3,3,1}$ [144] | $W_{10,9,9,9,8,8,5,3,3,1,1}$ [144] |
| | [3,2,0,1,0,0,0,3,0,1] | [1,5,11,17,24,31,38,45,33,21,22] | $W_{10,9,9,9,8,8,6,2,2,2}$ [90] | $W_{10,9,9,9,8,8,6,2,2,2,1}$ [90] |
| | [4,0,0,1,2,0,0,1,1,2] | [1,6,11,16,22,30,38,46,33,21,22] | $W_{10,9,9,9,9,6,5,5,2,1}$ [128] | $W_{10,9,9,9,9,6,5,5,2,1,1}$ [128] |
| | [4,0,0,2,0,0,2,0,1,2] | [1,6,11,16,23,30,37,46,33,21,22] | $W_{10,9,9,9,9,6,6,3,3,1}$ [96] | $W_{10,9,9,9,9,6,6,3,3,1,1}$ [96] |
| | [4,0,1,0,0,2,1,0,1,2] | [1,6,11,17,23,29,37,46,33,21,22] | $W_{10,9,9,9,9,7,4,4,3,1}$ [144] | $W_{10,9,9,9,9,7,4,4,3,1,1}$ [144] |
| | [4,0,1,0,1,0,1,2,0,1] | [1,6,11,17,23,30,37,45,33,21,22] | $W_{10,9,9,9,9,7,5,3,2,2}$ [162] | $W_{10,9,9,9,9,7,5,3,2,2,1}$ [162] |
| | [5,1,1,0,0,0,1,0,2,3] | [0,5,11,18,25,32,39,47,33,21,22] | $W_{9,9,9,9,9,8,7,3,1,1}$ [120] | $W_{9,9,9,9,9,8,7,3,1,1,1}$ [120] |
| | [6,0,0,0,1,1,0,0,2,3] | [0,6,12,18,24,31,39,47,33,21,22] | $W_{9,9,9,9,9,9,5,4,1,1}$ [80] | $W_{9,9,9,9,9,9,5,4,1,1,1}$ [80] |
| | [6,0,0,1,0,0,0,2,1,2] | [0,6,12,18,25,32,39,46,33,21,22] | $W_{9,9,9,9,9,9,6,2,2,1}$ [80] | $W_{9,9,9,9,9,9,6,2,2,1,1}$ [80] |
| | [0,0,3,1,0,2,0,0,0,3] | [3,6,9,15,22,29,38,47,34,21,22] | $W_{10,10,10,7,7,7,6,4,4}$ [60] | $W_{10,10,10,7,7,7,6,4,4,1,1,1}$ [60] |
| | [0,1,0,4,0,0,1,0,0,3] | [3,6,10,14,22,30,38,47,34,21,22] | $W_{10,10,10,8,6,6,6,6,3}$ [72] | $W_{10,10,10,8,6,6,6,6,3,1,1,1}$ [72] |
| | [0,3,2,0,1,0,0,1,0,3] | [2,4,9,16,23,31,39,47,34,21,22] | $W_{10,10,8,8,8,7,7,5,2}$ [108] | $W_{10,10,8,8,8,7,7,5,2,1,1,1}$ [108] |
| | [0,4,0,1,0,1,1,0,0,3] | [2,4,10,16,23,30,38,47,34,21,22] | $W_{10,10,8,8,8,8,6,4,3}$ [108] | $W_{10,10,8,8,8,8,6,4,3,1,1,1}$ [108] |
| | [1,1,2,1,1,0,1,0,0,3] | [2,5,9,15,22,30,38,47,34,21,22] | $W_{10,10,9,8,7,7,6,5,3}$ [192] | $W_{10,10,9,8,7,7,6,5,3,1,1,1}$ [192] |
| | [1,2,0,2,0,2,0,0,0,3] | [2,5,10,15,22,29,38,47,34,21,22] | $W_{10,10,9,8,8,6,6,4,4}$ [90] | $W_{10,10,9,8,8,6,6,4,4,1,1,1}$ [90] |
| | [2,0,1,1,2,1,0,0,0,3] | [2,6,10,15,21,29,38,47,34,21,22] | $W_{10,10,9,9,7,6,5,5,4}$ [120] | $W_{10,10,9,9,7,6,5,5,4,1,1,1}$ [120] |
| | [2,2,2,1,0,0,0,0,1,4] | [1,4,9,16,24,32,40,48,34,21,22] | $W_{10,9,9,8,8,7,7,6,1}$ [96] | $W_{10,9,9,8,8,7,7,6,1,1,1,1}$ [96] |
| | [2,3,0,1,1,0,0,1,0,3] | [1,4,10,16,23,31,39,47,34,21,22] | $W_{10,9,9,8,8,8,6,5,2}$ [144] | $W_{10,9,9,8,8,8,6,5,2,1,1,1}$ [144] |
| | [2,3,1,0,0,0,2,0,0,3] | [1,4,10,17,24,31,38,47,34,21,22] | $W_{10,9,9,8,8,8,7,3,3}$ [80] | $W_{10,9,9,8,8,8,7,3,3,1,1,1}$ [80] |
| | [3,0,3,0,1,0,0,1,0,3] | [1,5,9,16,23,31,39,47,34,21,22] | $W_{10,9,9,9,7,7,7,5,2}$ [108] | $W_{10,9,9,9,7,7,7,5,2,1,1,1}$ [108] |
| | [3,1,0,3,0,0,0,1,0,3] | [1,5,10,15,23,31,39,47,34,21,22] | $W_{10,9,9,9,8,6,6,6,2}$ [90] | $W_{10,9,9,9,8,6,6,6,2,1,1,1}$ [90] |
| | [3,1,1,0,2,0,1,0,0,3] | [1,5,10,16,22,30,38,47,34,21,22] | $W_{10,9,9,9,8,7,5,5,3}$ [144] | $W_{10,9,9,9,8,7,5,5,3,1,1,1}$ [144] |
| | [3,2,0,0,0,3,0,0,0,3] | [1,5,11,17,23,29,38,47,34,21,22] | $W_{10,9,9,9,8,8,4,4,4}$ [50] | $W_{10,9,9,9,8,8,4,4,4,1,1,1}$ [50] |
| | [4,0,0,1,1,2,0,0,0,3] | [1,6,11,16,22,29,38,47,34,21,22] | $W_{10,9,9,9,9,6,5,4,4}$ [80] | $W_{10,9,9,9,9,6,5,4,4,1,1,1}$ [80] |
| | [4,3,0,0,0,1,0,0,1,4] | [0,4,11,18,25,32,40,48,34,21,22] | $W_{9,9,9,9,8,8,8,4,1}$ [80] | $W_{9,9,9,9,8,8,8,4,1,1,1,1}$ [80] |
| | [5,0,2,0,1,0,0,0,1,4] | [0,5,10,17,24,32,40,48,34,21,22] | $W_{9,9,9,9,9,7,7,5,1}$ [90] | $W_{9,9,9,9,9,7,7,5,1,1,1,1}$ [90] |
| | [5,1,0,1,0,1,0,1,0,3] | [0,5,11,17,24,31,39,47,34,21,22] | $W_{9,9,9,9,9,8,6,4,2}$ [162] | $W_{9,9,9,9,9,8,6,4,2,1,1,1}$ [162] |
| | [6,0,0,0,1,0,2,0,0,3] | [0,6,12,18,24,31,38,47,34,21,22] | $W_{9,9,9,9,9,9,5,3,3}$ [60] | $W_{9,9,9,9,9,9,5,3,3,1,1,1}$ [60] |
| | [4,2,1,1,0,0,0,0,0,5] | [0,4,10,17,25,33,41,49,35,21,22] | $W_{9,9,9,9,8,8,7,6}$ [56] | $W_{9,9,9,9,8,8,7,6,1,1,1,1,1}$ [56] |
| | [0,1,0,0,0,0,0,0,9,0] | [5,10,16,22,28,34,40,46,29,21,23] | $W_{10,10,10,10,10,8,1,1,1,1,1,1,1,1,1}$ [13] | $W_{10,10,10,10,10,8}$ [14] |
| | [1,1,1,1,0,0,0,0,7,0] | [3,7,12,18,25,32,39,46,30,21,23] | $W_{10,10,10,9,8,7,6,1,1,1,1,1,1,1}$ [56] | $W_{10,10,10,9,8,7,6}$ [56] |
| | [0,2,0,2,0,1,0,0,5,0] | [3,6,11,16,23,30,38,46,31,21,23] | $W_{10,10,10,8,8,6,6,4,1,1,1,1,1}$ [67] | $W_{10,10,10,8,8,6,6,4}$ [68] |
| | [1,0,1,1,2,0,0,0,5,0] | [3,7,11,16,22,30,38,46,31,21,23] | $W_{10,10,10,9,7,6,5,5,1,1,1,1,1}$ [72] | $W_{10,10,10,9,7,6,5,5}$ [72] |
| | [1,3,1,0,0,0,0,1,5,0] | [2,5,11,18,25,32,39,46,31,21,23] | $W_{10,10,9,8,8,8,7,2,1,1,1,1,1}$ [72] | $W_{10,10,9,8,8,8,7,2}$ [72] |
| | [2,1,1,0,1,1,0,0,5,0] | [2,6,11,17,23,30,38,46,31,21,23] | $W_{10,10,9,9,8,7,5,4,1,1,1,1,1}$ [120] | $W_{10,10,9,9,8,7,5,4}$ [120] |
| | [4,1,0,1,0,0,0,1,5,0] | [1,6,12,18,25,32,39,46,31,21,23] | $W_{10,9,9,9,9,8,6,2,1,1,1,1,1}$ [90] | $W_{10,9,9,9,9,8,6,2}$ [90] |
| | [5,0,0,0,0,1,1,0,5,0] | [1,7,13,19,25,31,38,46,31,21,23] | $W_{10,9,9,9,9,9,4,3,1,1,1,1,1}$ [48] | $W_{10,9,9,9,9,9,4,3}$ [48] |
| | [0,1,1,2,0,1,1,0,3,0] | [3,6,10,15,22,29,37,46,32,21,23] | $W_{10,10,10,8,7,6,6,4,3,1,1,1}$ [144] | $W_{10,10,10,8,7,6,6,4,3}$ [144] |
| | [0,2,0,0,3,0,1,0,3,0] | [3,6,11,16,21,29,37,46,32,21,23] | $W_{10,10,10,8,8,5,5,5,3,1,1,1}$ [72] | $W_{10,10,10,8,8,5,5,5,3}$ [72] |
| | [0,2,0,1,0,3,0,0,3,0] | [3,6,11,16,22,28,37,46,32,21,23] | $W_{10,10,10,8,8,6,4,4,4,1,1,1}$ [67] | $W_{10,10,10,8,8,6,4,4,4}$ [68] |
| | [0,4,1,0,0,1,0,0,4,1] | [2,4,10,17,24,31,39,47,32,21,23] | $W_{10,10,8,8,8,8,7,4,1,1,1,1}$ [96] | $W_{10,10,8,8,8,8,7,4,1}$ [96] |
| | [0,5,0,0,0,0,0,2,3,0] | [2,4,11,18,25,32,39,46,32,21,23] | $W_{10,10,8,8,8,8,8,2,2,1,1,1}$ [31] | $W_{10,10,8,8,8,8,8,2,2}$ [32] |
| | [1,0,0,2,2,0,1,0,3,0] | [3,7,11,15,21,29,37,46,32,21,23] | $W_{10,10,10,9,6,6,5,5,3,1,1,1}$ [96] | $W_{10,10,10,9,6,6,5,5,3}$ [96] |
| | [1,0,1,0,2,2,0,0,3,0] | [3,7,11,16,21,28,37,46,32,21,23] | $W_{10,10,10,9,7,5,5,4,4,1,1,1}$ [90] | $W_{10,10,10,9,7,5,5,4,4}$ [90] |
| | [1,2,0,3,0,0,0,0,4,1] | [2,5,10,15,23,31,39,47,32,21,23] | $W_{10,10,9,8,8,6,6,6,1,1,1,1}$ [72] | $W_{10,10,9,8,8,6,6,6,1}$ [72] |
| | [1,2,1,0,2,0,0,1,3,0] | [2,5,10,16,22,30,38,46,32,21,23] | $W_{10,10,9,8,8,7,5,5,2,1,1,1}$ [144] | $W_{10,10,9,8,8,7,5,5,2}$ [144] |
| | [1,2,1,1,0,0,2,0,3,0] | [2,5,10,16,23,30,37,46,32,21,23] | $W_{10,10,9,8,8,7,6,3,3,1,1,1}$ [128] | $W_{10,10,9,8,8,7,6,3,3}$ [128] |
| | [1,3,0,0,0,2,1,0,3,0] | [2,5,11,17,23,29,37,46,32,21,23] | $W_{10,10,9,8,8,8,4,4,3,1,1,1}$ [80] | $W_{10,10,9,8,8,8,4,4,3}$ [80] |
| | [2,0,1,2,1,0,0,1,3,0] | [2,6,10,15,22,30,38,46,32,21,23] | $W_{10,10,9,9,7,6,6,5,2,1,1,1}$ [144] | $W_{10,10,9,9,7,6,6,5,2}$ [144] |
| | [2,0,2,0,1,1,1,0,3,0] | [2,6,10,16,22,29,37,46,32,21,23] | $W_{10,10,9,9,7,7,5,4,3,1,1,1}$ [144] | $W_{10,10,9,9,7,7,5,4,3}$ [144] |
| | [2,4,0,0,0,0,1,0,4,1] | [1,4,11,18,25,32,39,47,32,21,23] | $W_{10,9,9,8,8,8,8,3,1,1,1,1}$ [72] | $W_{10,9,9,8,8,8,8,3,1}$ [72] |
| | [3,1,1,1,1,0,0,0,4,1] | [1,5,10,16,23,31,39,47,32,21,23] | $W_{10,9,9,9,8,7,6,5,1,1,1,1}$ [160] | $W_{10,9,9,9,8,7,6,5,1}$ [160] |
| | [3,1,2,0,0,0,1,1,3,0] | [1,5,10,17,24,31,38,46,32,21,23] | $W_{10,9,9,9,8,7,7,3,2,1,1,1}$ [120] | $W_{10,9,9,9,8,7,7,3,2}$ [120] |
| | [3,2,0,0,1,1,0,1,3,0] | [1,5,11,17,23,30,38,46,32,21,23] | $W_{10,9,9,9,8,8,5,4,2,1,1,1}$ [144] | $W_{10,9,9,9,8,8,5,4,2}$ [144] |
| | [4,0,0,2,0,1,0,1,3,0] | [1,6,11,16,23,30,38,46,32,21,23] | $W_{10,9,9,9,9,6,6,4,2,1,1,1}$ [108] | $W_{10,9,9,9,9,6,6,4,2}$ [108] |
| | [4,0,1,0,1,0,2,0,3,0] | [1,6,11,17,23,30,37,46,32,21,23] | $W_{10,9,9,9,9,7,5,3,3,1,1,1}$ [108] | $W_{10,9,9,9,9,7,5,3,3}$ [108] |
| | [5,2,0,0,0,0,0,1,4,1] | [0,5,12,19,26,33,40,47,32,21,23] | $W_{9,9,9,9,9,8,8,2,1,1,1,1}$ [56] | $W_{9,9,9,9,9,8,8,2,1}$ [56] |

| | | | | |
|---|---|---|---|---|
| | [6,0,0,1,0,0,1,0,4,1] | [0,6,12,18,25,32,39,47,32,21,23] | $W_{9,9,9,9,9,9,6,3,1,1,1,1}$ [96] | $W_{9,9,9,9,9,9,6,3,1}$ [96] |
| | [0,0,0,1,1,3,1,0,1,0] | [4,8,12,16,21,27,36,46,33,21,23] | $W_{10,10,10,10,6,5,4,4,4,3,1}$ [80] | $W_{10,10,10,10,6,5,4,4,4,3}$ [80] |
| | [0,0,2,3,0,0,1,0,2,1] | [3,6,9,14,22,30,38,47,33,21,23] | $W_{10,10,10,7,7,6,6,6,3,1,1}$ [96] | $W_{10,10,10,7,7,6,6,6,3,1}$ [96] |
| | [0,0,3,0,2,1,0,0,2,1] | [3,6,9,15,21,29,38,47,33,21,23] | $W_{10,10,10,7,7,7,5,5,4,1,1}$ [96] | $W_{10,10,10,7,7,7,5,5,4,1}$ [96] |
| | [0,0,3,1,0,1,1,1,1,0] | [3,6,9,15,22,29,37,46,33,21,23] | $W_{10,10,10,7,7,7,6,4,3,2,1}$ [144] | $W_{10,10,10,7,7,7,6,4,3,2}$ [144] |
| | [0,1,0,3,1,1,0,0,2,1] | [3,6,10,14,21,29,38,47,33,21,23] | $W_{10,10,10,8,6,6,6,5,4,1,1}$ [144] | $W_{10,10,10,8,6,6,6,5,4,1}$ [144] |
| | [0,1,0,4,0,0,0,2,1,0] | [3,6,10,14,22,30,38,46,33,21,23] | $W_{10,10,10,8,6,6,6,6,2,2,1}$ [67] | $W_{10,10,10,8,6,6,6,6,2,2}$ [68] |
| | [0,1,1,1,1,2,0,1,1,0] | [3,6,10,15,21,28,37,46,33,21,23] | $W_{10,10,10,8,7,6,5,4,4,2,1}$ [216] | $W_{10,10,10,8,7,6,5,4,4,2}$ [216] |
| | [0,1,1,2,0,0,3,0,1,0] | [3,6,10,15,22,29,36,46,33,21,23] | $W_{10,10,10,8,7,6,6,3,3,3,1}$ [96] | $W_{10,10,10,8,7,6,6,3,3,3}$ [96] |
| | [0,1,2,0,0,2,2,0,1,0] | [3,6,10,16,22,28,36,46,33,21,23] | $W_{10,10,10,8,7,7,4,4,3,3,1}$ [96] | $W_{10,10,10,8,7,7,4,4,3,3}$ [96] |
| | [0,2,0,0,2,1,2,0,1,0] | [3,6,11,16,21,28,36,46,33,21,23] | $W_{10,10,10,8,8,5,5,4,3,3,1}$ [96] | $W_{10,10,10,8,8,5,5,4,3,3}$ [96] |
| | [0,3,1,2,0,0,0,1,2,1] | [2,4,9,15,23,31,39,47,33,21,23] | $W_{10,10,8,8,8,7,6,6,2,1,1}$ [120] | $W_{10,10,8,8,8,7,6,6,2,1}$ [120] |
| | [0,3,2,0,0,1,1,0,2,1] | [2,4,9,16,23,30,38,47,33,21,23] | $W_{10,10,8,8,8,7,7,4,3,1,1}$ [144] | $W_{10,10,8,8,8,7,7,4,3,1}$ [144] |
| | [0,4,0,0,2,0,1,0,2,1] | [2,4,10,16,22,30,38,47,33,21,23] | $W_{10,10,8,8,8,8,5,5,3,1,1}$ [108] | $W_{10,10,8,8,8,8,5,5,3,1}$ [108] |
| | [0,4,0,1,0,1,0,2,1,0] | [2,4,10,16,23,30,38,46,33,21,23] | $W_{10,10,8,8,8,8,6,4,2,2,1}$ [121] | $W_{10,10,8,8,8,8,6,4,2,2}$ [122] |
| | [1,0,0,2,1,1,2,0,1,0] | [3,7,11,15,21,28,36,46,33,21,23] | $W_{10,10,10,9,6,6,5,4,3,3,1}$ [128] | $W_{10,10,10,9,6,6,5,4,3,3}$ [128] |
| | [1,1,0,0,0,4,1,0,1,0] | [3,7,12,17,22,27,36,46,33,21,23] | $W_{10,10,10,9,8,4,4,4,4,3,1}$ [80] | $W_{10,10,10,9,8,4,4,4,4,3}$ [80] |
| | [1,1,2,1,0,2,0,0,2,1] | [2,5,9,15,22,29,38,47,33,21,23] | $W_{10,10,9,8,7,7,6,4,4,1,1}$ [192] | $W_{10,10,9,8,7,7,6,4,4,1}$ [192] |
| | [1,1,2,1,1,0,0,2,1,0] | [2,5,9,15,22,30,38,46,33,21,23] | $W_{10,10,9,8,7,7,6,5,2,2,1}$ [192] | $W_{10,10,9,8,7,7,6,5,2,2}$ [192] |
| | [1,1,3,0,0,0,2,1,1,0] | [2,5,9,16,23,30,37,46,33,21,23] | $W_{10,10,9,8,7,7,7,3,3,2,1}$ [120] | $W_{10,10,9,8,7,7,7,3,3,2}$ [120] |
| | [1,2,0,1,2,1,0,0,2,1] | [2,5,10,15,21,29,38,47,33,21,23] | $W_{10,10,9,8,8,6,5,5,4,1,1}$ [192] | $W_{10,10,9,8,8,6,5,5,4,1}$ [192] |
| | [1,2,0,2,0,1,1,1,1,0] | [2,5,10,15,22,29,37,46,33,21,23] | $W_{10,10,9,8,8,6,6,4,3,2,1}$ [216] | $W_{10,10,9,8,8,6,6,4,3,2}$ [216] |
| | [2,0,0,4,0,0,1,0,2,1] | [2,6,10,14,22,30,38,47,33,21,23] | $W_{10,10,9,9,6,6,6,6,3,1,1}$ [96] | $W_{10,10,9,9,6,6,6,6,3,1}$ [96] |
| | [2,0,1,1,2,0,1,1,1,0] | [2,6,10,15,21,29,37,46,33,21,23] | $W_{10,10,9,9,7,6,5,5,3,2,1}$ [216] | $W_{10,10,9,9,7,6,5,5,3,2}$ [216] |
| | [2,0,2,0,0,3,0,1,1,0] | [2,6,10,16,22,28,37,46,33,21,23] | $W_{10,10,9,9,7,7,4,4,4,2,1}$ [108] | $W_{10,10,9,9,7,7,4,4,4,2}$ [108] |
| | [2,0,2,0,1,0,3,0,1,0] | [2,6,10,16,22,29,36,46,33,21,23] | $W_{10,10,9,9,7,7,5,3,3,3,1}$ [108] | $W_{10,10,9,9,7,7,5,3,3,3}$ [108] |
| | [2,1,0,0,2,2,0,1,1,0] | [2,6,11,16,21,28,37,46,33,21,23] | $W_{10,10,9,9,8,5,5,4,4,2,1}$ [144] | $W_{10,10,9,9,8,5,5,4,4,2}$ [144] |
| | [2,1,0,1,0,2,2,0,1,0] | [2,6,11,16,22,28,36,46,33,21,23] | $W_{10,10,9,9,8,6,4,4,3,3,1}$ [144] | $W_{10,10,9,9,8,6,4,4,3,3}$ [144] |
| | [2,2,2,0,1,0,0,1,2,1] | [1,4,9,16,23,31,39,47,33,21,23] | $W_{10,9,9,8,8,7,7,5,2,1,1}$ [192] | $W_{10,9,9,8,8,7,7,5,2,1}$ [192] |
| | [2,3,0,1,0,1,1,0,2,1] | [1,4,10,16,23,30,38,47,33,21,23] | $W_{10,9,9,8,8,8,6,4,3,1,1}$ [216] | $W_{10,9,9,8,8,8,6,4,3,1}$ [216] |
| | [2,3,1,0,0,0,1,2,1,0] | [1,4,10,17,24,31,38,46,33,21,23] | $W_{10,9,9,8,8,8,7,3,2,2,1}$ [120] | $W_{10,9,9,8,8,8,7,3,2,2}$ [120] |
| | [3,0,2,2,0,0,0,1,2,1] | [1,5,9,15,23,31,39,47,33,21,23] | $W_{10,9,9,9,7,7,6,6,2,1,1}$ [120] | $W_{10,9,9,9,7,7,6,6,2,1}$ [120] |
| | [3,0,3,0,0,1,1,0,2,1] | [1,5,9,16,23,30,38,47,33,21,23] | $W_{10,9,9,9,7,7,7,4,3,1,1}$ [144] | $W_{10,9,9,9,7,7,7,4,3,1}$ [144] |
| | [3,1,0,2,1,0,1,0,2,1] | [1,5,10,15,22,30,38,47,33,21,23] | $W_{10,9,9,9,8,6,6,5,3,1,1}$ [216] | $W_{10,9,9,9,8,6,6,5,3,1}$ [216] |
| | [3,1,1,0,1,2,0,0,2,1] | [1,5,10,16,22,29,38,47,33,21,23] | $W_{10,9,9,9,8,7,5,4,4,1,1}$ [192] | $W_{10,9,9,9,8,7,5,4,4,1}$ [192] |
| | [3,1,1,0,2,0,0,2,1,0] | [1,5,10,16,22,30,38,46,33,21,23] | $W_{10,9,9,9,8,7,5,5,2,2,1}$ [144] | $W_{10,9,9,9,8,7,5,5,2,2}$ [144] |
| | [3,1,1,1,0,0,2,1,1,0] | [1,5,10,16,23,30,37,46,33,21,23] | $W_{10,9,9,9,8,7,6,3,3,2,1}$ [192] | $W_{10,9,9,9,8,7,6,3,3,2}$ [192] |
| | [3,2,0,0,0,2,1,1,1,0] | [1,5,11,17,23,29,37,46,33,21,23] | $W_{10,9,9,9,8,8,4,4,3,2,1}$ [120] | $W_{10,9,9,9,8,8,4,4,3,2}$ [120] |
| | [4,0,0,1,1,1,1,1,1,0] | [1,6,11,16,22,29,37,46,33,21,23] | $W_{10,9,9,9,9,6,5,4,3,2,1}$ [192] | $W_{10,9,9,9,9,6,5,4,3,2}$ [192] |
| | [4,1,0,0,0,0,4,0,1,0] | [1,6,12,18,24,30,36,46,33,21,23] | $W_{10,9,9,9,9,8,3,3,3,3,1}$ [48] | $W_{10,9,9,9,9,8,3,3,3,3}$ [48] |
| | [4,2,1,0,1,0,0,0,3,2] | [0,4,10,17,24,32,40,48,33,21,23] | $W_{9,9,9,9,8,8,7,5,1,1,1}$ [120] | $W_{9,9,9,9,8,8,7,5,1,1}$ [120] |
| | [4,3,0,0,0,0,1,1,2,1] | [0,4,11,18,25,32,39,47,33,21,23] | $W_{9,9,9,9,8,8,8,3,2,1,1}$ [96] | $W_{9,9,9,9,8,8,8,3,2,1}$ [96] |
| | [5,0,1,2,0,0,0,0,3,2] | [0,5,10,16,24,32,40,48,33,21,23] | $W_{9,9,9,9,9,7,6,6,1,1,1}$ [72] | $W_{9,9,9,9,9,7,6,6,1,1}$ [72] |
| | [5,0,2,0,0,1,0,1,2,1] | [0,5,10,17,24,31,39,47,33,21,23] | $W_{9,9,9,9,9,7,7,4,2,1,1}$ [144] | $W_{9,9,9,9,9,7,7,4,2,1}$ [144] |
| | [5,1,0,0,2,0,0,1,2,1] | [0,5,11,17,23,31,39,47,33,21,23] | $W_{9,9,9,9,9,8,5,5,2,1,1}$ [128] | $W_{9,9,9,9,9,8,5,5,2,1}$ [128] |
| | [5,1,0,1,0,0,2,0,2,1] | [0,5,11,17,24,31,38,47,33,21,23] | $W_{9,9,9,9,9,8,6,3,3,1,1}$ [144] | $W_{9,9,9,9,9,8,6,3,3,1}$ [144] |
| | [5,1,1,0,0,0,0,3,1,0] | [0,5,11,18,25,32,39,46,33,21,23] | $W_{9,9,9,9,9,8,7,2,2,2,1}$ [72] | $W_{9,9,9,9,9,8,7,2,2,2}$ [72] |
| | [6,0,0,0,0,2,1,0,2,1] | [0,6,12,18,24,30,38,47,33,21,23] | $W_{9,9,9,9,9,9,4,4,3,1,1}$ [72] | $W_{9,9,9,9,9,9,4,4,3,1}$ [72] |
| | [6,0,0,0,1,0,1,2,1,0] | [0,6,12,18,24,31,38,46,33,21,23] | $W_{9,9,9,9,9,9,5,3,2,2,1}$ [90] | $W_{9,9,9,9,9,9,5,3,2,2}$ [90] |
| | [0,0,2,2,1,1,0,1,0,1] | [3,6,9,14,21,29,38,47,34,21,23] | $W_{10,10,10,7,7,6,6,5,4,2}$ [144] | $W_{10,10,10,7,7,6,6,5,4,2,1}$ [144] |
| | [0,0,3,0,2,0,2,0,0,1] | [3,6,9,15,21,29,37,47,34,21,23] | $W_{10,10,10,7,7,7,5,5,3,3}$ [72] | $W_{10,10,10,7,7,7,5,5,3,3,1}$ [72] |
| | [0,1,0,3,1,0,2,0,0,1] | [3,6,10,14,21,29,37,47,34,21,23] | $W_{10,10,10,8,6,6,6,5,3,3}$ [108] | $W_{10,10,10,8,6,6,6,5,3,3,1}$ [108] |
| | [0,2,3,1,0,0,1,0,1,2] | [2,4,8,15,23,31,39,48,34,21,23] | $W_{10,10,8,8,7,7,7,6,3,1}$ [144] | $W_{10,10,8,8,7,7,7,6,3,1,1}$ [144] |
| | [0,3,1,1,1,0,1,1,0,1] | [2,4,9,15,22,30,38,47,34,21,23] | $W_{10,10,8,8,8,7,6,5,3,2}$ [216] | $W_{10,10,8,8,8,7,6,5,3,2,1}$ [216] |
| | [0,4,0,0,1,2,0,1,0,1] | [2,4,10,16,22,29,38,47,34,21,23] | $W_{10,10,8,8,8,8,5,4,4,2}$ [108] | $W_{10,10,8,8,8,8,5,4,4,2,1}$ [108] |
| | [1,0,1,0,1,4,0,0,0,1] | [3,7,11,16,21,27,37,47,34,21,23] | $W_{10,10,10,9,7,5,4,4,4,4}$ [90] | $W_{10,10,10,9,7,5,4,4,4,4,1}$ [90] |
| | [1,0,4,0,1,1,0,0,1,2] | [2,5,8,15,22,30,39,48,34,21,23] | $W_{10,10,9,7,7,7,7,5,4,1}$ [144] | $W_{10,10,9,7,7,7,7,5,4,1,1}$ [144] |
| | [1,0,4,1,0,0,0,2,0,1] | [2,5,8,15,23,31,39,47,34,21,23] | $W_{10,10,9,7,7,7,7,6,2,2}$ [90] | $W_{10,10,9,7,7,7,7,6,2,2,1}$ [90] |
| | [1,1,1,2,2,0,0,0,1,2] | [2,5,9,14,21,30,39,48,34,21,23] | $W_{10,10,9,8,7,6,6,5,5,1}$ [160] | $W_{10,10,9,8,7,6,6,5,5,1,1}$ [160] |
| | [1,1,1,3,0,0,1,1,0,1] | [2,5,9,14,22,30,38,47,34,21,23] | $W_{10,10,9,8,7,6,6,6,3,2}$ [192] | $W_{10,10,9,8,7,6,6,6,3,2,1}$ [192] |
| | [1,1,2,0,2,1,0,1,0,1] | [2,5,9,15,21,29,38,47,34,21,23] | $W_{10,10,9,8,7,7,5,5,4,2}$ [216] | $W_{10,10,9,8,7,7,5,5,4,2,1}$ [216] |
| | [1,1,2,1,0,1,2,0,0,1] | [2,5,9,15,22,29,37,47,34,21,23] | $W_{10,10,9,8,7,7,6,4,3,3}$ [192] | $W_{10,10,9,8,7,7,6,4,3,3,1}$ [192] |
| | [1,2,0,1,2,0,2,0,0,1] | [2,5,10,15,21,29,37,47,34,21,23] | $W_{10,10,9,8,8,6,5,5,3,3}$ [144] | $W_{10,10,9,8,8,6,5,5,3,3,1}$ [144] |
| | [1,2,1,0,0,3,1,0,0,1] | [2,5,10,16,22,28,37,47,34,21,23] | $W_{10,10,9,8,8,7,4,4,4,3}$ [128] | $W_{10,10,9,8,8,7,4,4,4,3,1}$ [128] |
| | [1,4,1,1,0,0,0,1,1,2] | [1,3,9,16,24,32,40,48,34,21,23] | $W_{10,9,8,8,8,8,7,6,2,1}$ [160] | $W_{10,9,8,8,8,8,7,6,2,1,1}$ [160] |
| | [1,5,0,0,0,1,1,0,1,2] | [1,3,10,17,24,31,39,48,34,21,23] | $W_{10,9,8,8,8,8,8,4,3,1}$ [120] | $W_{10,9,8,8,8,8,8,4,3,1,1}$ [120] |
| | [2,0,0,3,1,1,0,1,0,1] | [2,6,10,14,21,29,38,47,34,21,23] | $W_{10,10,9,9,6,6,6,5,4,2}$ [144] | $W_{10,10,9,9,6,6,6,5,4,2,1}$ [144] |
| | [2,0,1,1,1,2,1,0,0,1] | [2,6,10,15,21,28,37,47,34,21,23] | $W_{10,10,9,9,7,6,5,4,4,3}$ [192] | $W_{10,10,9,9,7,6,5,4,4,3,1}$ [192] |
| | [2,1,4,0,0,0,0,1,1,2] | [1,4,8,16,24,32,40,48,34,21,23] | $W_{10,9,9,8,7,7,7,7,2,1}$ [96] | $W_{10,9,9,8,7,7,7,7,2,1,1}$ [96] |
| | [2,2,1,1,1,1,0,0,1,2] | [1,4,9,15,22,30,39,48,34,21,23] | $W_{10,9,9,8,8,7,6,5,4,1}$ [256] | $W_{10,9,9,8,8,7,6,5,4,1,1}$ [256] |
| | [2,2,1,2,0,0,0,2,0,1] | [1,4,9,15,23,31,39,47,34,21,23] | $W_{10,9,9,8,8,7,6,6,2,2}$ [120] | $W_{10,9,9,8,8,7,6,6,2,2,1}$ [120] |

| | | | | |
|---|---|---|---|---|
| | [2,2,2,0,0,1,1,1,0,1] | [1,4,9,16,23,30,38,47,34,21,23] | $W_{10,9,9,8,8,7,7,4,3,2}$ [192] | $W_{10,9,9,8,8,7,7,4,3,2,1}$ [192] |
| | [2,3,0,0,2,0,1,1,0,1] | [1,4,10,16,22,30,38,47,34,21,23] | $W_{10,9,9,8,8,8,5,5,3,2}$ [144] | $W_{10,9,9,8,8,8,5,5,3,2,1}$ [144] |
| | [3,0,2,1,1,0,1,1,0,1] | [1,5,9,15,22,30,38,47,34,21,23] | $W_{10,9,9,9,7,7,6,5,3,2}$ [216] | $W_{10,9,9,9,7,7,6,5,3,2,1}$ [216] |
| | [3,1,0,1,3,0,0,0,1,2] | [1,5,10,15,21,30,39,48,34,21,23] | $W_{10,9,9,9,8,6,5,5,5,1}$ [120] | $W_{10,9,9,9,8,6,5,5,5,1,1}$ [120] |
| | [3,1,0,2,0,2,0,1,0,1] | [1,5,10,15,22,29,38,47,34,21,23] | $W_{10,9,9,9,8,6,6,4,4,2}$ [162] | $W_{10,9,9,9,8,6,6,4,4,2,1}$ [162] |
| | [3,1,1,0,1,1,2,0,0,1] | [1,5,10,16,22,29,37,47,34,21,23] | $W_{10,9,9,9,8,7,5,4,3,3}$ [192] | $W_{10,9,9,9,8,7,5,4,3,3,1}$ [192] |
| | [3,4,0,1,0,0,0,0,2,3] | [0,3,10,17,25,33,41,49,34,21,23] | $W_{9,9,9,8,8,8,8,6,1,1}$ [72] | $W_{9,9,9,8,8,8,8,6,1,1,1}$ [72] |
| | [4,0,0,0,3,1,0,1,0,1] | [1,6,11,16,21,29,38,47,34,21,23] | $W_{10,9,9,9,9,5,5,5,4,2}$ [90] | $W_{10,9,9,9,9,5,5,5,4,2,1}$ [90] |
| | [4,1,2,1,0,0,0,1,1,2] | [0,4,9,16,24,32,40,48,34,21,23] | $W_{9,9,9,9,8,7,7,6,2,1}$ [160] | $W_{9,9,9,9,8,7,7,6,2,1,1}$ [160] |
| | [4,2,0,1,1,0,1,0,1,2] | [0,4,10,16,23,31,39,48,34,21,23] | $W_{9,9,9,9,8,8,6,5,3,1}$ [216] | $W_{9,9,9,9,8,8,6,5,3,1,1}$ [216] |
| | [4,2,1,0,0,1,0,2,0,1] | [0,4,10,17,24,31,39,47,34,21,23] | $W_{9,9,9,9,8,8,7,4,2,2}$ [144] | $W_{9,9,9,9,8,8,7,4,2,2,1}$ [144] |
| | [5,0,1,1,0,2,0,0,1,2] | [0,5,10,16,23,30,39,48,34,21,23] | $W_{9,9,9,9,9,7,6,4,4,1}$ [144] | $W_{9,9,9,9,9,7,6,4,4,1,1}$ [144] |
| | [5,0,1,1,1,0,0,2,0,1] | [0,5,10,16,23,31,39,47,34,21,23] | $W_{9,9,9,9,9,7,6,5,2,2}$ [144] | $W_{9,9,9,9,9,7,6,5,2,2,1}$ [144] |
| | [5,0,2,0,0,0,2,1,0,1] | [0,5,10,17,24,31,38,47,34,21,23] | $W_{9,9,9,9,9,7,7,3,3,2}$ [90] | $W_{9,9,9,9,9,7,7,3,3,2,1}$ [90] |
| | [5,1,0,0,1,1,1,1,0,1] | [0,5,11,17,23,30,38,47,34,21,23] | $W_{9,9,9,9,9,8,5,4,3,2}$ [192] | $W_{9,9,9,9,9,8,5,4,3,2,1}$ [192] |
| | [0,2,3,0,2,0,0,0,0,3] | [2,4,8,15,22,31,40,49,35,21,23] | $W_{10,10,8,8,7,7,7,5,5}$ [54] | $W_{10,10,8,8,7,7,7,5,5,1,1,1}$ [54] |
| | [1,0,3,2,1,0,0,0,0,3] | [2,5,8,14,22,31,40,49,35,21,23] | $W_{10,10,9,7,7,7,6,6,5}$ [72] | $W_{10,10,9,7,7,7,6,6,5,1,1,1}$ [72] |
| | [1,4,1,0,1,1,0,0,0,3] | [1,3,9,16,23,31,40,49,35,21,23] | $W_{10,9,8,8,8,8,7,5,4}$ [120] | $W_{10,9,8,8,8,8,7,5,4,1,1,1}$ [120] |
| | [2,1,3,1,0,1,0,0,0,3] | [1,4,8,15,23,31,40,49,35,21,23] | $W_{10,9,9,8,7,7,7,6,4}$ [120] | $W_{10,9,9,8,7,7,7,6,4,1,1,1}$ [120] |
| | [3,0,1,3,1,0,0,0,0,3] | [1,5,9,14,22,31,40,49,35,21,23] | $W_{10,9,9,9,7,6,6,6,5}$ [72] | $W_{10,9,9,9,7,6,6,6,5,1,1,1}$ [72] |
| | [3,3,2,0,0,0,0,1,0,3] | [0,3,9,17,25,33,41,49,35,21,23] | $W_{9,9,9,8,8,8,7,7,2}$ [72] | $W_{9,9,9,8,8,8,7,7,2,1,1,1}$ [72] |
| | [3,4,0,0,1,0,1,0,0,3] | [0,3,10,17,24,32,40,49,35,21,23] | $W_{9,9,9,8,8,8,8,5,3}$ [96] | $W_{9,9,9,8,8,8,8,5,3,1,1,1}$ [96] |
| | [4,1,2,0,1,1,0,0,0,3] | [0,4,9,16,23,31,40,49,35,21,23] | $W_{9,9,9,9,8,7,7,5,4}$ [120] | $W_{9,9,9,9,8,7,7,5,4,1,1,1}$ [120] |
| | [5,0,0,3,0,1,0,0,0,3] | [0,5,10,15,23,31,40,49,35,21,23] | $W_{9,9,9,9,9,6,6,6,4}$ [60] | $W_{9,9,9,9,9,6,6,6,4,1,1,1}$ [60] |
| | [5,0,1,0,3,0,0,0,0,3] | [0,5,10,16,22,31,40,49,35,21,23] | $W_{9,9,9,9,9,7,5,5,5}$ [54] | $W_{9,9,9,9,9,7,5,5,5,1,1,1}$ [54] |
| | [0,4,0,2,0,0,0,0,5,0] | [2,4,10,16,24,32,40,48,32,21,24] | $W_{10,10,8,8,8,8,6,6,1,1,1,1,1}$ [31] | $W_{10,10,8,8,8,8,6,6}$ [32] |
| | [2,3,1,0,1,0,0,0,5,0] | [1,4,10,17,24,32,40,48,32,21,24] | $W_{10,9,9,8,8,8,7,5,1,1,1,1,1}$ [72] | $W_{10,9,9,8,8,8,7,5}$ [72] |
| | [5,1,1,0,0,1,0,0,5,0] | [0,5,11,18,25,32,40,48,32,21,24] | $W_{9,9,9,9,9,8,7,4,1,1,1,1,1}$ [80] | $W_{9,9,9,9,9,8,7,4}$ [80] |
| | [6,0,0,0,2,0,0,0,5,0] | [0,6,12,18,24,32,40,48,32,21,24] | $W_{9,9,9,9,9,9,5,5,1,1,1,1,1}$ [30] | $W_{9,9,9,9,9,9,5,5}$ [30] |
| | [0,0,2,2,2,0,0,0,3,0] | [3,6,9,14,21,30,39,48,33,21,24] | $W_{10,10,10,7,7,6,6,5,5,1,1,1}$ [48] | $W_{10,10,10,7,7,6,6,5,5}$ [48] |
| | [0,3,1,1,1,1,0,0,3,0] | [2,4,9,15,22,30,39,48,33,21,24] | $W_{10,10,8,8,8,7,6,5,4,1,1,1}$ [120] | $W_{10,10,8,8,8,7,6,5,4}$ [120] |
| | [1,1,1,3,0,1,0,0,3,0] | [2,5,9,14,22,30,39,48,33,21,24] | $W_{10,10,9,8,7,6,6,6,4,1,1,1}$ [120] | $W_{10,10,9,8,7,6,6,6,4}$ [120] |
| | [1,1,2,0,3,0,0,0,3,0] | [2,5,9,15,21,30,39,48,33,21,24] | $W_{10,10,9,8,7,7,5,5,5,1,1,1}$ [72] | $W_{10,10,9,8,7,7,5,5,5}$ [72] |
| | [1,4,2,0,0,0,0,0,4,1] | [1,3,9,17,25,33,41,49,33,21,24] | $W_{10,9,8,8,8,8,7,7,1,1,1,1}$ [56] | $W_{10,9,8,8,8,8,7,7,1}$ [56] |
| | [1,5,0,0,1,0,0,1,3,0] | [1,3,10,17,24,32,40,48,33,21,24] | $W_{10,9,8,8,8,8,8,5,2,1,1,1}$ [96] | $W_{10,9,8,8,8,8,8,5,2}$ [96] |
| | [2,0,0,3,2,0,0,0,3,0] | [2,6,10,14,21,30,39,48,33,21,24] | $W_{10,10,9,9,6,6,6,5,5,1,1,1}$ [48] | $W_{10,10,9,9,6,6,6,5,5}$ [48] |
| | [2,2,1,2,0,0,1,0,3,0] | [1,4,9,15,23,31,39,48,33,21,24] | $W_{10,9,9,8,8,7,6,6,3,1,1,1}$ [128] | $W_{10,9,9,8,8,7,6,6,3}$ [128] |
| | [2,2,2,0,0,2,0,0,3,0] | [1,4,9,16,23,30,39,48,33,21,24] | $W_{10,9,9,8,8,7,7,4,4,1,1,1}$ [80] | $W_{10,9,9,8,8,7,7,4,4}$ [80] |
| | [2,3,0,0,2,1,0,0,3,0] | [1,4,10,16,22,30,39,48,33,21,24] | $W_{10,9,9,8,8,8,5,5,4,1,1,1}$ [80] | $W_{10,9,9,8,8,8,5,5,4}$ [80] |
| | [3,0,2,1,1,1,0,0,3,0] | [1,5,9,15,22,30,39,48,33,21,24] | $W_{10,9,9,9,7,7,6,5,4,1,1,1}$ [120] | $W_{10,9,9,9,7,7,6,5,4}$ [120] |
| | [4,0,0,0,4,0,0,0,3,0] | [1,6,11,16,21,30,39,48,33,21,24] | $W_{10,9,9,9,9,5,5,5,5,1,1,1}$ [30] | $W_{10,9,9,9,9,5,5,5,5}$ [30] |
| | [4,1,3,0,0,0,0,0,4,1] | [0,4,9,17,25,33,41,49,33,21,24] | $W_{9,9,9,9,8,7,7,7,1,1,1,1}$ [56] | $W_{9,9,9,9,8,7,7,7,1}$ [56] |
| | [4,2,0,2,0,0,0,1,3,0] | [0,4,10,16,24,32,40,48,33,21,24] | $W_{9,9,9,9,8,8,6,6,2,1,1,1}$ [90] | $W_{9,9,9,9,8,8,6,6,2}$ [90] |
| | [4,2,1,0,0,1,1,0,3,0] | [0,4,10,17,24,31,39,48,33,21,24] | $W_{9,9,9,9,8,8,7,4,3,1,1,1}$ [128] | $W_{9,9,9,9,8,8,7,4,3}$ [128] |
| | [5,0,1,1,1,0,1,0,3,0] | [0,5,10,16,23,31,39,48,33,21,24] | $W_{9,9,9,9,9,7,6,5,3,1,1,1}$ [144] | $W_{9,9,9,9,9,7,6,5,3}$ [144] |
| | [5,1,0,0,1,2,0,0,3,0] | [0,5,11,17,23,30,39,48,33,21,24] | $W_{9,9,9,9,9,8,5,4,4,1,1,1}$ [80] | $W_{9,9,9,9,9,8,5,4,4}$ [80] |
| | [0,0,1,5,0,0,0,0,2,1] | [3,6,9,13,22,31,40,49,34,21,24] | $W_{10,10,10,7,6,6,6,6,6,1,1}$ [48] | $W_{10,10,10,7,6,6,6,6,6,1}$ [48] |
| | [0,0,3,0,1,3,0,0,1,0] | [3,6,9,15,21,28,38,48,34,21,24] | $W_{10,10,10,7,7,7,5,4,4,4,1}$ [60] | $W_{10,10,10,7,7,7,5,4,4,4}$ [60] |
| | [0,1,0,3,0,3,0,0,1,0] | [3,6,10,14,21,28,38,48,34,21,24] | $W_{10,10,10,8,6,6,6,4,4,4,1}$ [67] | $W_{10,10,10,8,6,6,6,4,4,4}$ [68] |
| | [0,2,2,2,1,0,0,0,2,1] | [2,4,8,14,22,31,40,49,34,21,24] | $W_{10,10,8,8,7,7,6,6,5,1,1}$ [120] | $W_{10,10,8,8,7,7,6,6,5,1}$ [120] |
| | [0,2,3,0,1,1,0,1,1,0] | [2,4,8,15,22,30,39,48,34,21,24] | $W_{10,10,8,8,7,7,7,5,4,2,1}$ [162] | $W_{10,10,8,8,7,7,7,5,4,2}$ [162] |
| | [0,3,0,3,0,1,0,1,1,0] | [2,4,9,14,22,30,39,48,34,21,24] | $W_{10,10,8,8,8,6,6,6,4,2,1}$ [121] | $W_{10,10,8,8,8,6,6,6,4,2}$ [122] |
| | [0,3,1,0,3,0,0,1,1,0] | [2,4,9,15,21,30,39,48,34,21,24] | $W_{10,10,8,8,8,7,5,5,5,2,1}$ [108] | $W_{10,10,8,8,8,7,5,5,5,2}$ [108] |
| | [0,3,1,1,0,2,1,0,1,0] | [2,4,9,15,22,29,38,48,34,21,24] | $W_{10,10,8,8,8,7,6,4,4,3,1}$ [144] | $W_{10,10,8,8,8,7,6,4,4,3}$ [144] |
| | [1,0,3,2,0,1,0,1,1,0] | [2,5,8,14,22,30,39,48,34,21,24] | $W_{10,10,9,7,7,7,6,6,4,2,1}$ [162] | $W_{10,10,9,7,7,7,6,6,4,2}$ [162] |
| | [1,0,4,0,1,0,2,0,1,0] | [2,5,8,15,22,30,38,48,34,21,24] | $W_{10,10,9,7,7,7,7,5,3,3,1}$ [108] | $W_{10,10,9,7,7,7,7,5,3,3}$ [108] |
| | [1,1,1,2,1,1,1,0,1,0] | [2,5,9,14,21,29,38,48,34,21,24] | $W_{10,10,9,8,7,6,6,5,4,3,1}$ [256] | $W_{10,10,9,8,7,6,6,5,4,3}$ [256] |
| | [1,2,0,1,1,3,0,0,1,0] | [2,5,10,15,21,28,38,48,34,21,24] | $W_{10,10,9,8,8,6,5,4,4,4,1}$ [120] | $W_{10,10,9,8,8,6,5,4,4,4}$ [120] |
| | [1,3,3,0,0,0,1,0,2,1] | [1,3,8,16,24,32,40,49,34,21,24] | $W_{10,9,8,8,8,7,7,7,3,1,1}$ [120] | $W_{10,9,8,8,8,7,7,7,3,1}$ [120] |
| | [1,4,0,2,0,1,0,0,2,1] | [1,3,9,15,23,31,40,49,34,21,24] | $W_{10,9,8,8,8,8,6,6,4,1,1}$ [144] | $W_{10,9,8,8,8,8,6,6,4,1}$ [144] |
| | [1,4,1,0,1,0,1,1,1,0] | [1,3,9,16,23,31,39,48,34,21,24] | $W_{10,9,8,8,8,8,7,5,3,2,1}$ [216] | $W_{10,9,8,8,8,8,7,5,3,2}$ [216] |
| | [2,1,3,0,2,0,0,0,2,1] | [1,4,8,15,22,31,40,49,34,21,24] | $W_{10,9,9,8,7,7,7,5,5,1,1}$ [120] | $W_{10,9,9,8,7,7,7,5,5,1}$ [120] |
| | [2,1,3,1,0,0,1,1,1,0] | [1,4,8,15,23,31,39,48,34,21,24] | $W_{10,9,9,8,7,7,7,6,3,2,1}$ [192] | $W_{10,9,9,8,7,7,7,6,3,2}$ [192] |
| | [2,2,0,3,1,0,0,0,2,1] | [1,4,9,14,22,31,40,49,34,21,24] | $W_{10,9,9,8,8,6,6,6,5,1,1}$ [120] | $W_{10,9,9,8,8,6,6,6,5,1}$ [120] |
| | [2,2,1,1,1,0,2,0,1,0] | [1,4,9,15,22,30,38,48,34,21,24] | $W_{10,9,9,8,8,7,6,5,3,3,1}$ [192] | $W_{10,9,9,8,8,7,6,5,3,3}$ [192] |
| | [2,3,0,0,1,2,1,0,1,0] | [1,4,10,16,22,29,38,48,34,21,24] | $W_{10,9,9,8,8,8,5,4,4,3,1}$ [128] | $W_{10,9,9,8,8,8,5,4,4,3}$ [128] |
| | [3,0,1,3,0,1,0,1,1,0] | [1,5,9,14,22,30,39,48,34,21,24] | $W_{10,9,9,9,7,6,6,6,4,2,1}$ [162] | $W_{10,9,9,9,7,6,6,6,4,2}$ [162] |
| | [3,0,2,0,3,0,0,1,1,0] | [1,5,9,15,21,30,39,48,34,21,24] | $W_{10,9,9,9,7,7,5,5,5,2,1}$ [108] | $W_{10,9,9,9,7,7,5,5,5,2}$ [108] |
| | [3,0,2,1,0,2,1,0,1,0] | [1,5,9,15,22,29,38,48,34,21,24] | $W_{10,9,9,9,7,7,6,4,4,3,1}$ [144] | $W_{10,9,9,9,7,7,6,4,4,3}$ [144] |
| | [3,1,0,1,2,1,1,0,1,0] | [1,5,10,15,21,29,38,48,34,21,24] | $W_{10,9,9,9,8,6,5,5,4,3,1}$ [192] | $W_{10,9,9,9,8,6,5,5,4,3}$ [192] |
| | [3,3,1,1,0,0,1,0,2,1] | [0,3,9,16,24,32,40,49,34,21,24] | $W_{9,9,9,8,8,8,7,6,3,1,1}$ [192] | $W_{9,9,9,8,8,8,7,6,3,1}$ [192] |

| | | | | |
|---|---|---|---|---|
| | [3,4,0,0,0,2,0,0,2,1] | [0,3,10,17,24,31,40,49,34,21,24] | $W_{9,9,9,8,8,8,8,4,4,1,1}$ [80] | $W_{9,9,9,8,8,8,8,4,4,1}$ [80] |
| | [3,4,0,0,1,0,0,2,1,0] | [0,3,10,17,24,32,40,48,34,21,24] | $W_{9,9,9,8,8,8,8,5,2,2,1}$ [96] | $W_{9,9,9,8,8,8,8,5,2,2}$ [96] |
| | [4,0,0,1,0,4,0,0,1,0] | [1,6,11,16,22,28,38,48,34,21,24] | $W_{10,9,9,9,9,6,4,4,4,4,1}$ [60] | $W_{10,9,9,9,9,6,4,4,4,4}$ [60] |
| | [4,1,1,2,0,1,0,0,2,1] | [0,4,9,15,23,31,40,49,34,21,24] | $W_{9,9,9,9,8,7,6,6,4,1,1}$ [192] | $W_{9,9,9,9,8,7,6,6,4,1}$ [192] |
| | [4,1,2,0,1,0,1,1,1,0] | [0,4,9,16,23,31,39,48,34,21,24] | $W_{9,9,9,9,8,7,7,5,3,2,1}$ [216] | $W_{9,9,9,9,8,7,7,5,3,2}$ [216] |
| | [4,2,0,0,3,0,0,0,2,1] | [0,4,10,16,22,31,40,49,34,21,24] | $W_{9,9,9,9,8,8,5,5,5,1,1}$ [80] | $W_{9,9,9,9,8,8,5,5,5,1}$ [80] |
| | [4,2,0,1,0,2,0,1,1,0] | [0,4,10,16,23,30,39,48,34,21,24] | $W_{9,9,9,9,8,8,6,4,4,2,1}$ [162] | $W_{9,9,9,9,8,8,6,4,4,2}$ [162] |
| | [4,2,1,0,0,0,3,0,1,0] | [0,4,10,17,24,31,38,48,34,21,24] | $W_{9,9,9,9,8,8,7,3,3,3,1}$ [80] | $W_{9,9,9,9,8,8,7,3,3,3}$ [80] |
| | [5,0,0,2,2,0,0,0,2,1] | [0,5,10,15,22,31,40,49,34,21,24] | $W_{9,9,9,9,9,6,6,5,5,1,1}$ [80] | $W_{9,9,9,9,9,6,6,5,5,1}$ [80] |
| | [5,0,0,3,0,0,1,1,1,0] | [0,5,10,15,23,31,39,48,34,21,24] | $W_{9,9,9,9,9,6,6,6,3,2,1}$ [96] | $W_{9,9,9,9,9,6,6,6,3,2}$ [96] |
| | [5,0,1,0,2,1,0,1,1,0] | [0,5,10,16,22,30,39,48,34,21,24] | $W_{9,9,9,9,9,7,5,5,4,2,1}$ [162] | $W_{9,9,9,9,9,7,5,5,4,2}$ [162] |
| | [5,0,1,1,0,1,2,0,1,0] | [0,5,10,16,23,30,38,48,34,21,24] | $W_{9,9,9,9,9,7,6,4,3,3,1}$ [144] | $W_{9,9,9,9,9,7,6,4,3,3}$ [144] |
| | [0,0,1,4,1,0,1,0,0,1] | [3,6,9,13,21,30,39,49,35,21,24] | $W_{10,10,10,7,6,6,6,6,5,3}$ [96] | $W_{10,10,10,7,6,6,6,6,5,3,1}$ [96] |
| | [0,1,5,0,1,0,0,0,1,2] | [2,4,7,15,23,32,41,50,35,21,24] | $W_{10,10,8,7,7,7,7,7,5,1}$ [90] | $W_{10,10,8,7,7,7,7,7,5,1,1}$ [90] |
| | [0,2,2,2,0,1,1,0,0,1] | [2,4,8,14,22,30,39,49,35,21,24] | $W_{10,10,8,8,7,7,6,6,4,3}$ [144] | $W_{10,10,8,8,7,7,6,6,4,3,1}$ [144] |
| | [0,3,0,2,2,0,1,0,0,1] | [2,4,9,14,21,30,39,49,35,21,24] | $W_{10,10,8,8,8,6,6,5,5,3}$ [108] | $W_{10,10,8,8,8,6,6,5,5,3,1}$ [108] |
| | [0,3,1,0,2,2,0,0,0,1] | [2,4,9,15,21,29,39,49,35,21,24] | $W_{10,10,8,8,8,7,5,5,4,4}$ [90] | $W_{10,10,8,8,8,7,5,5,4,4,1}$ [90] |
| | [0,6,1,0,0,0,1,0,1,2] | [1,2,9,17,25,33,41,50,35,21,24] | $W_{10,8,8,8,8,8,8,7,3,1}$ [90] | $W_{10,8,8,8,8,8,8,7,3,1,1}$ [90] |
| | [1,0,3,1,2,0,1,0,0,1] | [2,5,8,14,21,30,39,49,35,21,24] | $W_{10,10,9,7,7,7,6,5,5,3}$ [144] | $W_{10,10,9,7,7,7,6,5,5,3,1}$ [144] |
| | [1,0,4,0,0,3,0,0,0,1] | [2,5,8,15,22,29,39,49,35,21,24] | $W_{10,10,9,7,7,7,7,4,4,4}$ [60] | $W_{10,10,9,7,7,7,7,4,4,4,1}$ [60] |
| | [1,1,0,5,0,0,0,1,0,1] | [2,5,9,13,22,31,40,49,35,21,24] | $W_{10,10,9,8,6,6,6,6,6,2}$ [90] | $W_{10,10,9,8,6,6,6,6,6,2,1}$ [90] |
| | [1,3,2,1,0,1,0,1,0,1] | [1,3,8,15,23,31,40,49,35,21,24] | $W_{10,9,8,8,8,7,7,6,4,2}$ [216] | $W_{10,9,8,8,8,7,7,6,4,2,1}$ [216] |
| | [1,4,0,1,2,0,0,1,0,1] | [1,3,9,15,22,31,40,49,35,21,24] | $W_{10,9,8,8,8,8,6,5,5,2}$ [144] | $W_{10,9,8,8,8,8,6,5,5,2,1}$ [144] |
| | [1,4,0,2,0,0,2,0,0,1] | [1,3,9,15,23,31,39,49,35,21,24] | $W_{10,9,8,8,8,8,6,6,3,3}$ [96] | $W_{10,9,8,8,8,8,6,6,3,3,1}$ [96] |
| | [1,4,1,0,0,2,1,0,0,1] | [1,3,9,16,23,30,39,49,35,21,24] | $W_{10,9,8,8,8,8,7,4,4,3}$ [128] | $W_{10,9,8,8,8,8,7,4,4,3,1}$ [128] |
| | [2,1,2,2,1,0,0,1,0,1] | [1,4,8,14,22,31,40,49,35,21,24] | $W_{10,9,9,8,7,7,6,6,5,2}$ [192] | $W_{10,9,9,8,7,7,6,6,5,2,1}$ [192] |
| | [2,1,3,0,1,1,1,0,0,1] | [1,4,8,15,22,30,39,49,35,21,24] | $W_{10,9,9,8,7,7,7,5,4,3}$ [192] | $W_{10,9,9,8,7,7,7,5,4,3,1}$ [192] |
| | [2,2,0,3,0,1,1,0,0,1] | [1,4,9,14,22,30,39,49,35,21,24] | $W_{10,9,9,8,8,6,6,6,4,3}$ [144] | $W_{10,9,9,8,8,6,6,6,4,3,1}$ [144] |
| | [2,2,1,0,3,0,1,0,0,1] | [1,4,9,15,21,30,39,49,35,21,24] | $W_{10,9,9,8,8,7,5,5,5,3}$ [144] | $W_{10,9,9,8,8,7,5,5,5,3,1}$ [144] |
| | [2,2,1,1,0,3,0,0,0,1] | [1,4,9,15,22,29,39,49,35,21,24] | $W_{10,9,9,8,8,7,6,4,4,4}$ [120] | $W_{10,9,9,8,8,7,6,4,4,4,1}$ [120] |
| | [2,6,0,0,0,0,0,1,1,2] | [0,2,10,18,26,34,42,50,35,21,24] | $W_{9,9,8,8,8,8,8,8,2,1}$ [56] | $W_{9,9,8,8,8,8,8,8,2,1,1}$ [56] |
| | [3,0,1,2,2,0,1,0,0,1] | [1,5,9,14,21,30,39,49,35,21,24] | $W_{10,9,9,9,7,6,6,5,5,3}$ [144] | $W_{10,9,9,9,7,6,6,5,5,3,1}$ [144] |
| | [3,0,2,0,2,2,0,0,0,1] | [1,5,9,15,21,29,39,49,35,21,24] | $W_{10,9,9,9,7,7,5,5,4,4}$ [90] | $W_{10,9,9,9,7,7,5,5,4,4,1}$ [90] |
| | [3,2,3,0,0,1,0,0,1,2] | [0,3,8,16,24,32,41,50,35,21,24] | $W_{9,9,9,8,8,7,7,7,4,1}$ [128] | $W_{9,9,9,8,8,7,7,7,4,1,1}$ [128] |
| | [3,3,0,2,1,0,0,0,1,2] | [0,3,9,15,23,32,41,50,35,21,24] | $W_{9,9,9,8,8,8,6,6,5,1}$ [120] | $W_{9,9,9,8,8,8,6,6,5,1,1}$ [120] |
| | [3,3,1,0,1,1,0,1,0,1] | [0,3,9,16,23,31,40,49,35,21,24] | $W_{9,9,9,8,8,8,7,5,4,2}$ [216] | $W_{9,9,9,8,8,8,7,5,4,2,1}$ [216] |
| | [3,4,0,0,0,1,2,0,0,1] | [0,3,10,17,24,31,39,49,35,21,24] | $W_{9,9,9,8,8,8,8,4,3,3}$ [80] | $W_{9,9,9,8,8,8,8,4,3,3,1}$ [80] |
| | [4,0,3,1,1,0,0,0,1,2] | [0,4,8,15,23,32,41,50,35,21,24] | $W_{9,9,9,9,7,7,7,6,5,1}$ [120] | $W_{9,9,9,9,7,7,7,6,5,1,1}$ [120] |
| | [4,0,4,0,0,0,1,1,0,1] | [0,4,8,16,24,32,40,49,35,21,24] | $W_{9,9,9,9,7,7,7,7,3,2}$ [90] | $W_{9,9,9,9,7,7,7,7,3,2,1}$ [90] |
| | [4,1,1,1,2,0,0,1,0,1] | [0,4,9,15,22,31,40,49,35,21,24] | $W_{9,9,9,9,8,7,6,5,5,2}$ [192] | $W_{9,9,9,9,8,7,6,5,5,2,1}$ [192] |
| | [4,1,1,2,0,0,2,0,0,1] | [0,4,9,15,23,31,39,49,35,21,24] | $W_{9,9,9,9,8,7,6,6,3,3}$ [128] | $W_{9,9,9,9,8,7,6,6,3,3,1}$ [128] |
| | [4,1,2,0,0,2,1,0,0,1] | [0,4,9,16,23,30,39,49,35,21,24] | $W_{9,9,9,9,8,7,7,4,4,3}$ [128] | $W_{9,9,9,9,8,7,7,4,4,3,1}$ [128] |
| | [4,2,0,0,2,1,1,0,0,1] | [0,4,10,16,22,30,39,49,35,21,24] | $W_{9,9,9,9,8,8,5,5,4,3}$ [128] | $W_{9,9,9,9,8,8,5,5,4,3,1}$ [128] |
| | [5,0,0,2,1,1,1,0,0,1] | [0,5,10,15,22,30,39,49,35,21,24] | $W_{9,9,9,9,9,6,6,5,4,3}$ [128] | $W_{9,9,9,9,9,6,6,5,4,3,1}$ [128] |
| | [5,1,0,0,0,4,0,0,0,1] | [0,5,11,17,23,29,39,49,35,21,24] | $W_{9,9,9,9,9,8,4,4,4,4}$ [50] | $W_{9,9,9,9,9,8,4,4,4,4,1}$ [50] |
| | [0,6,0,1,1,0,0,0,0,3] | [1,2,9,16,24,33,42,51,36,21,24] | $W_{10,8,8,8,8,8,8,6,5}$ [54] | $W_{10,8,8,8,8,8,8,6,5,1,1,1}$ [54] |
| | [2,0,5,1,0,0,0,0,0,3] | [1,4,7,15,24,33,42,51,36,21,24] | $W_{10,9,9,7,7,7,7,7,6}$ [42] | $W_{10,9,9,7,7,7,7,7,6,1,1,1}$ [42] |
| | [2,5,1,0,0,1,0,0,0,3] | [0,2,9,17,25,33,42,51,36,21,24] | $W_{9,9,8,8,8,8,8,7,4}$ [80] | $W_{9,9,8,8,8,8,8,7,4,1,1,1}$ [80] |
| | [3,2,2,2,0,0,0,0,0,3] | [0,3,8,15,24,33,42,51,36,21,24] | $W_{9,9,9,8,8,7,7,6,6}$ [56] | $W_{9,9,9,8,8,7,7,6,6,1,1,1}$ [56] |
| | [3,4,1,0,0,0,0,0,5,0] | [0,3,10,18,26,34,42,50,33,21,25] | $W_{9,9,9,8,8,8,8,7,1,1,1,1,1}$ [32] | $W_{9,9,9,8,8,8,8,7}$ [32] |
| | [0,7,0,0,0,0,0,1,3,0] | [1,2,10,18,26,34,42,50,34,21,25] | $W_{10,8,8,8,8,8,8,8,2,1,1,1}$ [31] | $W_{10,8,8,8,8,8,8,8,2}$ [32] |
| | [1,3,2,1,1,0,0,0,3,0] | [1,3,8,15,23,32,41,50,34,21,25] | $W_{10,9,8,8,8,7,7,6,5,1,1,1}$ [96] | $W_{10,9,8,8,8,7,7,6,5}$ [96] |
| | [2,1,2,3,0,0,0,0,3,0] | [1,4,8,14,23,32,41,50,34,21,25] | $W_{10,9,9,8,7,7,6,6,6,1,1,1}$ [56] | $W_{10,9,9,8,7,7,6,6,6}$ [56] |
| | [3,3,1,0,2,0,0,0,3,0] | [0,3,9,16,23,32,41,50,34,21,25] | $W_{9,9,9,8,8,8,7,5,5,1,1,1}$ [72] | $W_{9,9,9,8,8,8,7,5,5}$ [72] |
| | [4,0,4,0,0,1,0,0,3,0] | [0,4,8,16,24,32,41,50,34,21,25] | $W_{9,9,9,9,7,7,7,7,4,1,1,1}$ [60] | $W_{9,9,9,9,7,7,7,7,4}$ [60] |
| | [0,1,4,2,0,0,0,1,1,0] | [2,4,7,14,23,32,41,50,35,21,25] | $W_{10,10,8,7,7,7,7,6,6,2,1}$ [90] | $W_{10,10,8,7,7,7,7,6,6,2}$ [90] |
| | [0,1,5,0,0,1,1,0,1,0] | [2,4,7,15,23,31,40,50,35,21,25] | $W_{10,10,8,7,7,7,7,7,4,3,1}$ [96] | $W_{10,10,8,7,7,7,7,7,4,3}$ [96] |
| | [0,2,2,1,2,1,0,0,1,0] | [2,4,8,14,21,30,40,50,35,21,25] | $W_{10,10,8,8,7,7,6,5,5,4,1}$ [120] | $W_{10,10,8,8,7,7,6,5,5,4}$ [120] |
| | [0,5,2,0,1,0,0,0,2,1] | [1,2,8,16,24,33,42,51,35,21,25] | $W_{10,8,8,8,8,8,7,7,5,1,1}$ [90] | $W_{10,8,8,8,8,8,7,7,5,1}$ [90] |
| | [0,6,0,1,0,1,0,1,1,0] | [1,2,9,16,24,32,41,50,35,21,25] | $W_{10,8,8,8,8,8,8,6,4,2,1}$ [121] | $W_{10,8,8,8,8,8,8,6,4,2}$ [122] |
| | [1,0,2,4,0,0,1,0,1,0] | [2,5,8,13,22,31,40,50,35,21,25] | $W_{10,10,9,7,7,6,6,6,6,3,1}$ [96] | $W_{10,10,9,7,7,6,6,6,6,3}$ [96] |
| | [1,1,0,4,1,1,0,0,1,0] | [2,5,9,13,21,30,40,50,35,21,25] | $W_{10,10,9,8,6,6,6,6,5,4,1}$ [120] | $W_{10,10,9,8,6,6,6,6,5,4}$ [120] |
| | [1,2,4,1,0,0,0,0,2,1] | [1,3,7,15,24,33,42,51,35,21,25] | $W_{10,9,8,8,7,7,7,7,6,1,1}$ [96] | $W_{10,9,8,8,7,7,7,7,6,1}$ [96] |
| | [1,3,1,3,0,0,0,1,1,0] | [1,3,8,14,23,32,41,50,35,21,25] | $W_{10,9,8,8,8,7,6,6,6,2,1}$ [120] | $W_{10,9,8,8,8,7,6,6,6,2}$ [120] |
| | [1,3,2,0,2,0,1,0,1,0] | [1,3,8,15,22,31,40,50,35,21,25] | $W_{10,9,8,8,8,7,7,5,5,3,1}$ [144] | $W_{10,9,8,8,8,7,7,5,5,3}$ [144] |
| | [1,4,0,1,1,2,0,0,1,0] | [1,3,9,15,22,30,40,50,35,21,25] | $W_{10,9,8,8,8,8,6,5,4,4,1}$ [120] | $W_{10,9,8,8,8,8,6,5,4,4}$ [120] |
| | [2,0,5,0,1,0,0,1,1,0] | [1,4,7,15,23,32,41,50,35,21,25] | $W_{10,9,9,7,7,7,7,7,5,2,1}$ [108] | $W_{10,9,9,7,7,7,7,7,5,2}$ [108] |
| | [2,1,2,2,0,2,0,0,1,0] | [1,4,8,14,22,30,40,50,35,21,25] | $W_{10,9,9,8,7,7,6,6,4,4,1}$ [120] | $W_{10,9,9,8,7,7,6,6,4,4}$ [120] |
| | [2,2,0,2,2,1,0,0,1,0] | [1,4,9,14,21,30,40,50,35,21,25] | $W_{10,9,9,8,8,6,6,5,5,4,1}$ [120] | $W_{10,9,9,8,8,6,6,5,5,4}$ [120] |
| | [2,5,0,1,1,0,0,0,2,1] | [0,2,9,16,24,33,42,51,35,21,25] | $W_{9,9,8,8,8,8,8,6,5,1,1}$ [120] | $W_{9,9,8,8,8,8,8,6,5,1}$ [120] |
| | [2,5,1,0,0,0,1,1,1,0] | [0,2,9,17,25,33,41,50,35,21,25] | $W_{9,9,8,8,8,8,8,7,3,2,1}$ [120] | $W_{9,9,8,8,8,8,8,7,3,2}$ [120] |

| | | | | |
|---|---|---|---|---|
| | [3,2,2,1,1,0,0,1,1,0] | [0,3,8,15,23,32,41,50,35,21,25] | $W_{9,9,9,8,8,7,7,6,5,2,1}$ [192] | $W_{9,9,9,8,8,7,7,6,5,2}$ [192] |
| | [3,2,3,0,0,0,2,0,1,0] | [0,3,8,16,24,32,40,50,35,21,25] | $W_{9,9,9,8,8,7,7,7,3,3,1}$ [80] | $W_{9,9,9,8,8,7,7,7,3,3}$ [80] |
| | [3,3,0,2,0,1,1,0,1,0] | [0,3,9,15,23,31,40,50,35,21,25] | $W_{9,9,9,8,8,8,6,6,4,3,1}$ [144] | $W_{9,9,9,8,8,8,6,6,4,3}$ [144] |
| | [4,0,3,1,0,1,1,0,1,0] | [0,4,8,15,23,31,40,50,35,21,25] | $W_{9,9,9,9,7,7,7,6,4,3,1}$ [144] | $W_{9,9,9,9,7,7,7,6,4,3}$ [144] |
| | [4,1,0,4,0,0,0,1,1,0] | [0,4,9,14,23,32,41,50,35,21,25] | $W_{9,9,9,9,8,6,6,6,6,2,1}$ [90] | $W_{9,9,9,9,8,6,6,6,6,2}$ [90] |
| | [4,1,1,1,1,2,0,0,1,0] | [0,4,9,15,22,30,40,50,35,21,25] | $W_{9,9,9,9,8,7,6,5,4,4,1}$ [160] | $W_{9,9,9,9,8,7,6,5,4,4}$ [160] |
| | [0,1,4,1,1,1,0,0,0,1] | [2,4,7,14,22,31,41,51,36,21,25] | $W_{10,10,8,7,7,7,7,6,5,4}$ [120] | $W_{10,10,8,7,7,7,7,6,5,4,1}$ [120] |
| | [0,2,1,4,0,1,0,0,0,1] | [2,4,8,13,22,31,41,51,36,21,25] | $W_{10,10,8,8,7,6,6,6,6,4}$ [90] | $W_{10,10,8,8,7,6,6,6,6,4,1}$ [90] |
| | [0,5,1,2,0,0,0,1,0,1] | [1,2,8,15,24,33,42,51,36,21,25] | $W_{10,8,8,8,8,8,7,6,6,2}$ [90] | $W_{10,8,8,8,8,8,7,6,6,2,1}$ [90] |
| | [0,5,2,0,0,1,1,0,0,1] | [1,2,8,16,24,32,41,51,36,21,25] | $W_{10,8,8,8,8,8,7,7,4,3}$ [96] | $W_{10,8,8,8,8,8,7,7,4,3,1}$ [96] |
| | [0,6,0,0,2,0,1,0,0,1] | [1,2,9,16,23,32,41,51,36,21,25] | $W_{10,8,8,8,8,8,8,5,5,3}$ [72] | $W_{10,8,8,8,8,8,8,5,5,3,1}$ [72] |
| | [1,0,2,3,2,0,0,0,0,1] | [2,5,8,13,21,31,41,51,36,21,25] | $W_{10,10,9,7,7,6,6,6,5,5}$ [72] | $W_{10,10,9,7,7,6,6,6,5,5,1}$ [72] |
| | [1,2,4,0,1,0,1,0,0,1] | [1,3,7,15,23,32,41,51,36,21,25] | $W_{10,9,8,8,7,7,7,7,5,3}$ [144] | $W_{10,9,8,8,7,7,7,7,5,3,1}$ [144] |
| | [1,3,1,2,1,1,0,0,0,1] | [1,3,8,14,22,31,41,51,36,21,25] | $W_{10,9,8,8,8,7,6,6,5,4}$ [160] | $W_{10,9,8,8,8,7,6,6,5,4,1}$ [160] |
| | [2,0,4,2,0,0,1,0,0,1] | [1,4,7,14,23,32,41,51,36,21,25] | $W_{10,9,9,7,7,7,7,6,6,3}$ [96] | $W_{10,9,9,7,7,7,7,6,6,3,1}$ [96] |
| | [2,0,5,0,0,2,0,0,0,1] | [1,4,7,15,23,31,41,51,36,21,25] | $W_{10,9,9,7,7,7,7,7,4,4}$ [60] | $W_{10,9,9,7,7,7,7,7,4,4,1}$ [60] |
| | [2,1,2,1,3,0,0,0,0,1] | [1,4,8,14,21,31,41,51,36,21,25] | $W_{10,9,9,8,7,7,6,5,5,5}$ [96] | $W_{10,9,9,8,7,7,6,5,5,5,1}$ [96] |
| | [2,4,2,0,1,0,0,1,0,1] | [0,2,8,16,24,33,42,51,36,21,25] | $W_{9,9,8,8,8,8,7,7,5,2}$ [144] | $W_{9,9,8,8,8,8,7,7,5,2,1}$ [144] |
| | [2,5,0,1,0,1,1,0,0,1] | [0,2,9,16,24,32,41,51,36,21,25] | $W_{9,9,8,8,8,8,8,6,4,3}$ [144] | $W_{9,9,8,8,8,8,8,6,4,3,1}$ [144] |
| | [3,0,0,5,0,1,0,0,0,1] | [1,5,9,13,22,31,41,51,36,21,25] | $W_{10,9,9,9,6,6,6,6,6,4}$ [60] | $W_{10,9,9,9,6,6,6,6,6,4,1}$ [60] |
| | [3,1,5,0,0,0,0,0,1,2] | [0,3,7,16,25,34,43,52,36,21,25] | $W_{9,9,9,8,7,7,7,7,7,1}$ [56] | $W_{9,9,9,8,7,7,7,7,7,1,1}$ [56] |
| | [3,2,2,1,0,2,0,0,0,1] | [0,3,8,15,23,31,41,51,36,21,25] | $W_{9,9,9,8,8,7,7,6,4,4}$ [120] | $W_{9,9,9,8,8,7,7,6,4,4,1}$ [120] |
| | [3,3,0,1,2,1,0,0,0,1] | [0,3,9,15,22,31,41,51,36,21,25] | $W_{9,9,9,8,8,8,6,5,5,4}$ [120] | $W_{9,9,9,8,8,8,6,5,5,4,1}$ [120] |
| | [4,0,2,3,0,0,1,0,0,1] | [0,4,8,14,23,32,41,51,36,21,25] | $W_{9,9,9,9,7,7,6,6,6,3}$ [96] | $W_{9,9,9,9,7,7,6,6,6,3,1}$ [96] |
| | [4,0,3,0,2,1,0,0,0,1] | [0,4,8,15,22,31,41,51,36,21,25] | $W_{9,9,9,9,7,7,7,5,5,4}$ [90] | $W_{9,9,9,9,7,7,7,5,5,4,1}$ [90] |
| | [4,1,0,3,1,1,0,0,0,1] | [0,4,9,14,22,31,41,51,36,21,25] | $W_{9,9,9,9,8,6,6,6,5,4}$ [120] | $W_{9,9,9,9,8,6,6,6,5,4,1}$ [120] |
| | [5,0,0,1,4,0,0,0,0,1] | [0,5,10,15,21,31,41,51,36,21,25] | $W_{9,9,9,9,9,6,5,5,5,5}$ [48] | $W_{9,9,9,9,9,6,5,5,5,5,1}$ [48] |
| | [2,4,2,1,0,0,0,0,3,0] | [0,2,8,16,25,34,43,52,35,21,26] | $W_{9,9,8,8,8,8,7,7,6,1,1,1}$ [56] | $W_{9,9,8,8,8,8,7,7,6}$ [56] |
| | [0,4,4,0,0,0,0,1,1,0] | [1,2,7,16,25,34,43,52,36,21,26] | $W_{10,8,8,8,8,7,7,7,7,2,1}$ [54] | $W_{10,8,8,8,8,7,7,7,7,2}$ [54] |
| | [0,5,1,1,1,1,0,0,1,0] | [1,2,8,15,23,32,42,52,36,21,26] | $W_{10,8,8,8,8,8,7,6,5,4,1}$ [120] | $W_{10,8,8,8,8,8,7,6,5,4}$ [120] |
| | [1,2,3,2,0,1,0,0,1,0] | [1,3,7,14,23,32,42,52,36,21,26] | $W_{10,9,8,8,7,7,7,6,6,4,1}$ [120] | $W_{10,9,8,8,7,7,7,6,6,4}$ [120] |
| | [2,0,4,1,2,0,0,0,1,0] | [1,4,7,14,22,32,42,52,36,21,26] | $W_{10,9,9,7,7,7,7,6,5,5,1}$ [72] | $W_{10,9,9,7,7,7,7,6,5,5}$ [72] |
| | [2,1,1,4,1,0,0,0,1,0] | [1,4,8,13,22,32,42,52,36,21,26] | $W_{10,9,9,8,7,6,6,6,6,5,1}$ [96] | $W_{10,9,9,8,7,6,6,6,6,5}$ [96] |
| | [2,4,1,2,0,0,1,0,1,0] | [0,2,8,15,24,33,42,52,36,21,26] | $W_{9,9,8,8,8,8,7,6,6,3,1}$ [128] | $W_{9,9,8,8,8,8,7,6,6,3}$ [128] |
| | [2,4,2,0,0,2,0,0,1,0] | [0,2,8,16,24,32,42,52,36,21,26] | $W_{9,9,8,8,8,8,7,7,4,4,1}$ [80] | $W_{9,9,8,8,8,8,7,7,4,4}$ [80] |
| | [2,5,0,0,2,1,0,0,1,0] | [0,2,9,16,23,32,42,52,36,21,26] | $W_{9,9,8,8,8,8,8,5,5,4,1}$ [80] | $W_{9,9,8,8,8,8,8,5,5,4}$ [80] |
| | [3,1,4,1,0,0,1,0,1,0] | [0,3,7,15,24,33,42,52,36,21,26] | $W_{9,9,9,8,7,7,7,7,6,3,1}$ [128] | $W_{9,9,9,8,7,7,7,7,6,3}$ [128] |
| | [3,2,1,3,0,1,0,0,1,0] | [0,3,8,14,23,32,42,52,36,21,26] | $W_{9,9,9,8,8,7,6,6,6,4,1}$ [120] | $W_{9,9,9,8,8,7,6,6,6,4}$ [120] |
| | [3,2,2,0,3,0,0,0,1,0] | [0,3,8,15,22,32,42,52,36,21,26] | $W_{9,9,9,8,8,7,7,5,5,5,1}$ [72] | $W_{9,9,9,8,8,7,7,5,5,5}$ [72] |
| | [4,0,2,2,2,0,0,0,1,0] | [0,4,8,14,22,32,42,52,36,21,26] | $W_{9,9,9,9,7,7,6,6,5,5,1}$ [72] | $W_{9,9,9,9,7,7,6,6,5,5}$ [72] |
| | [0,4,3,1,0,1,0,0,0,1] | [1,2,7,15,24,33,43,53,37,21,26] | $W_{10,8,8,8,8,7,7,7,6,4}$ [90] | $W_{10,8,8,8,8,7,7,7,6,4,1}$ [90] |
| | [1,7,0,1,0,0,0,1,0,1] | [0,1,9,17,26,35,44,53,37,21,26] | $W_{9,8,8,8,8,8,8,8,6,2}$ [90] | $W_{9,8,8,8,8,8,8,8,6,2,1}$ [90] |
| | [2,3,4,0,0,0,1,0,0,1] | [0,2,7,16,25,34,43,53,37,21,26] | $W_{9,9,8,8,8,7,7,7,7,3}$ [80] | $W_{9,9,8,8,8,7,7,7,7,3,1}$ [80] |
| | [2,4,1,1,2,0,0,0,0,1] | [0,2,8,15,23,33,43,53,37,21,26] | $W_{9,9,8,8,8,8,7,6,5,5}$ [96] | $W_{9,9,8,8,8,8,7,6,5,5,1}$ [96] |
| | [3,1,4,0,2,0,0,0,0,1] | [0,3,7,15,23,33,43,53,37,21,26] | $W_{9,9,9,8,7,7,7,7,5,5}$ [72] | $W_{9,9,9,8,7,7,7,7,5,5,1}$ [72] |
| | [1,7,1,0,0,0,0,0,3,0] | [0,1,9,18,27,36,45,54,36,21,27] | $W_{9,8,8,8,8,8,8,8,7,1,1,1}$ [32] | $W_{9,8,8,8,8,8,8,8,7}$ [32] |
| | [0,0,7,0,1,0,0,0,1,0] | [2,4,6,15,24,34,44,54,37,21,27] | $W_{10,10,7,7,7,7,7,7,7,5,1}$ [36] | $W_{10,10,7,7,7,7,7,7,7,5}$ [36] |
| | [0,5,0,4,0,0,0,0,1,0] | [1,2,8,14,24,34,44,54,37,21,27] | $W_{10,8,8,8,8,8,6,6,6,6,1}$ [31] | $W_{10,8,8,8,8,8,6,6,6,6}$ [32] |
| | [1,6,2,0,0,0,1,0,1,0] | [0,1,8,17,26,35,44,54,37,21,27] | $W_{9,8,8,8,8,8,8,7,7,3,1}$ [80] | $W_{9,8,8,8,8,8,8,7,7,3}$ [80] |
| | [1,7,0,0,1,1,0,0,1,0] | [0,1,9,17,25,34,44,54,37,21,27] | $W_{9,8,8,8,8,8,8,8,5,4,1}$ [80] | $W_{9,8,8,8,8,8,8,8,5,4}$ [80] |
| | [2,3,3,1,1,0,0,0,1,0] | [0,2,7,15,24,34,44,54,37,21,27] | $W_{9,9,8,8,8,7,7,7,6,5,1}$ [96] | $W_{9,9,8,8,8,7,7,7,6,5}$ [96] |
| | [3,1,3,3,0,0,0,0,1,0] | [0,3,7,14,24,34,44,54,37,21,27] | $W_{9,9,9,8,7,7,7,6,6,6,1}$ [56] | $W_{9,9,9,8,7,7,7,6,6,6}$ [56] |
| | [1,1,6,1,0,0,0,0,0,1] | [1,3,6,15,25,35,45,55,38,21,27] | $W_{10,9,8,7,7,7,7,7,7,6}$ [56] | $W_{10,9,8,7,7,7,7,7,7,6,1}$ [56] |
| | [1,6,1,1,1,0,0,0,0,1] | [0,1,8,16,25,35,45,55,38,21,27] | $W_{9,8,8,8,8,8,8,7,6,5}$ [96] | $W_{9,8,8,8,8,8,8,7,6,5,1}$ [96] |
| | [1,5,4,0,0,0,0,0,0,1] | [0,1,7,17,27,37,47,57,39,21,28] | $W_{9,8,8,8,8,8,7,7,7,7}$ [32] | $W_{9,8,8,8,8,8,7,7,7,7,1}$ [32] |
| | [0,10,0,0,0,0,0,0,1,0] | [0,0,10,20,30,40,50,60,40,21,30] | $W_{8,8,8,8,8,8,8,8,8,8,1}$ [13] | $W_{8,8,8,8,8,8,8,8,8,8}$ [14] |
| 22 | [0,0,0,1,0,0,0,5,0,0] | [5,10,15,20,26,32,38,44,33,22,22] | $X_{10,10,10,10,10,6,2,2,2,2,2}$ [25] | |
| | [0,0,1,1,2,0,0,0,3,3] | [4,8,12,17,23,31,39,47,33,22,22] | $X_{10,10,10,10,7,6,5,5,1,1,1}$ [80] | |
| | [0,0,1,2,0,0,1,1,2,2] | [4,8,12,17,24,31,38,46,33,22,22] | $X_{10,10,10,10,7,6,6,3,2,1,1}$ [128] | |
| | [0,0,2,0,0,2,0,1,2,2] | [4,8,12,18,24,30,38,46,33,22,22] | $X_{10,10,10,10,7,7,4,4,2,1,1}$ [96] | |
| | [0,1,0,0,2,1,0,1,2,2] | [4,8,13,18,23,30,38,46,33,22,22] | $X_{10,10,10,10,8,5,5,4,2,1,1}$ [144] | |
| | [0,1,0,1,0,1,2,0,2,2] | [4,8,13,18,24,30,37,46,33,22,22] | $X_{10,10,10,10,8,6,4,3,3,1,1}$ [162] | |
| | [0,1,0,1,1,0,0,3,1,1] | [4,8,13,18,24,31,38,45,33,22,22] | $X_{10,10,10,10,8,6,5,2,2,2,1}$ [144] | |
| | [0,1,1,0,0,0,2,2,1,1] | [4,8,13,19,25,31,37,45,33,22,22] | $X_{10,10,10,10,8,7,3,3,2,2,1}$ [120] | |
| | [0,3,0,1,0,0,1,0,3,3] | [3,6,12,18,25,32,39,47,33,22,22] | $X_{10,10,10,8,8,8,6,3,1,1,1}$ [108] | |
| | [1,0,0,0,1,1,1,2,1,1] | [4,9,14,19,24,30,37,45,33,22,22] | $X_{10,10,10,10,9,5,4,3,2,2,1}$ [160] | |
| | [1,0,3,0,0,0,1,0,3,3] | [3,7,11,18,25,32,39,47,33,22,22] | $X_{10,10,10,9,7,7,7,3,1,1,1}$ [90] | |
| | [1,1,0,2,0,1,0,0,3,3] | [3,7,12,17,24,31,39,47,33,22,22] | $X_{10,10,10,9,8,6,6,4,1,1,1}$ [144] | |
| | [1,1,1,0,1,0,1,1,2,2] | [3,7,12,18,24,31,38,46,33,22,22] | $X_{10,10,10,9,8,7,5,3,2,1,1}$ [288] | |
| | [2,0,0,0,3,0,0,0,3,3] | [3,8,13,18,23,31,39,47,33,22,22] | $X_{10,10,10,9,9,5,5,5,1,1,1}$ [50] | |
| | [2,0,0,1,0,2,0,1,2,2] | [3,8,13,18,24,30,38,46,33,22,22] | $X_{10,10,10,9,9,6,4,4,2,1,1}$ [144] | |

| | | | |
|---|---|---|---|
| | [2,0,1,0,0,0,3,0,2,2] | [3,8,13,19,25,31,37,46,33,22,22] | $X_{10,10,10,9,9,7,3,3,3,1,1}$ [90] |
| | [2,0,1,0,0,1,0,3,1,1] | [3,8,13,19,25,31,38,45,33,22,22] | $X_{10,10,10,9,9,7,4,2,2,2,1}$ [144] |
| | [2,2,1,0,0,0,0,1,3,3] | [2,6,12,19,26,33,40,47,33,22,22] | $X_{10,10,9,9,8,8,7,2,1,1,1}$ [96] |
| | [3,0,1,1,0,0,1,0,3,3] | [2,7,12,18,25,32,39,47,33,22,22] | $X_{10,10,9,9,9,7,6,3,1,1,1}$ [144] |
| | [3,1,0,0,0,2,0,0,3,3] | [2,7,13,19,25,31,39,47,33,22,22] | $X_{10,10,9,9,9,8,4,4,1,1,1}$ [80] |
| | [3,1,0,0,1,0,0,2,2,2] | [2,7,13,19,25,32,39,46,33,22,22] | $X_{10,10,9,9,9,8,5,2,2,1,1}$ [128] |
| | [4,0,0,0,0,0,2,1,2,2] | [2,8,14,20,26,32,38,46,33,22,22] | $X_{10,10,9,9,9,9,3,3,2,1,1}$ [56] |
| | [0,0,0,2,2,0,1,1,1,1] | [4,8,12,16,22,30,38,47,34,22,23] | $X_{10,10,10,10,6,6,5,5,3,2,1}$ [120] |
| | [0,0,1,0,2,2,0,1,1,1] | [4,8,12,17,22,29,38,47,34,22,23] | $X_{10,10,10,10,7,5,5,4,4,2,1}$ [144] |
| | [0,0,1,1,0,2,2,0,1,1] | [4,8,12,17,23,29,37,47,34,22,23] | $X_{10,10,10,10,7,6,4,4,3,3,1}$ [144] |
| | [0,0,1,1,1,0,2,2,0,0] | [4,8,12,17,23,30,37,46,34,22,23] | $X_{10,10,10,10,7,6,5,3,3,2,2}$ [96] |
| | [0,1,0,0,1,2,1,2,0,0] | [4,8,13,18,23,29,37,46,34,22,23] | $X_{10,10,10,10,8,5,4,4,3,2,2}$ [96] |
| | [0,1,2,1,1,0,1,0,2,2] | [3,6,10,16,23,31,39,48,34,22,23] | $X_{10,10,10,8,7,7,6,5,3,1,1}$ [216] |
| | [0,1,3,0,0,1,0,2,1,1] | [3,6,10,17,24,31,39,47,34,22,23] | $X_{10,10,10,8,7,7,7,4,2,2,1}$ [144] |
| | [0,2,0,2,1,0,0,2,1,1] | [3,6,11,16,23,31,39,47,34,22,23] | $X_{10,10,10,8,8,6,6,5,2,2,1}$ [144] |
| | [0,2,1,0,1,1,1,1,1,1] | [3,6,11,17,23,30,38,47,34,22,23] | $X_{10,10,10,8,8,7,5,4,3,2,1}$ [288] |
| | [0,3,0,0,1,0,1,3,0,0] | [3,6,12,18,24,31,38,46,34,22,23] | $X_{10,10,10,8,8,8,5,3,2,2,2}$ [72] |
| | [1,0,0,0,1,0,4,1,0,0] | [4,9,14,19,24,30,36,46,34,22,23] | $X_{10,10,10,10,9,5,3,3,3,3,2}$ [60] |
| | [1,0,1,1,2,1,0,0,2,2] | [3,7,11,16,22,30,39,48,34,22,23] | $X_{10,10,10,9,7,6,5,5,4,1,1}$ [192] |
| | [1,0,1,2,0,1,1,1,1,1] | [3,7,11,16,23,30,38,47,34,22,23] | $X_{10,10,10,9,7,6,6,4,3,2,1}$ [288] |
| | [1,0,2,1,0,0,1,3,0,0] | [3,7,11,17,24,31,38,46,34,22,23] | $X_{10,10,10,9,7,7,6,3,2,2,2}$ [96] |
| | [1,1,0,0,3,0,1,1,1,1] | [3,7,12,17,22,30,38,47,34,22,23] | $X_{10,10,10,9,8,5,5,5,3,2,1}$ [192] |
| | [1,1,0,1,0,3,0,1,1,1] | [3,7,12,17,23,29,38,47,34,22,23] | $X_{10,10,10,9,8,6,4,4,4,2,1}$ [216] |
| | [1,1,0,1,1,0,3,0,1,1] | [3,7,12,17,23,30,37,47,34,22,23] | $X_{10,10,10,9,8,6,5,3,3,3,1}$ [216] |
| | [1,1,0,1,1,1,0,3,0,0] | [3,7,12,17,23,30,38,46,34,22,23] | $X_{10,10,10,9,8,6,5,4,2,2,2}$ [144] |
| | [1,1,1,0,0,1,2,2,0,0] | [3,7,12,18,24,30,37,46,34,22,23] | $X_{10,10,10,9,8,7,4,3,3,2,2}$ [128] |
| | [1,2,2,0,1,0,0,1,2,2] | [2,5,10,17,24,32,40,48,34,22,23] | $X_{10,10,9,8,8,7,7,5,2,1,1}$ [192] |
| | [1,3,0,1,0,1,1,0,2,2] | [2,5,11,17,24,31,39,48,34,22,23] | $X_{10,10,9,8,8,8,6,4,3,1,1}$ [216] |
| | [1,3,1,0,0,0,1,2,1,1] | [2,5,11,18,25,32,39,47,34,22,23] | $X_{10,10,9,8,8,8,7,3,2,2,1}$ [160] |
| | [2,0,0,0,1,2,2,0,1,1] | [3,8,13,18,23,29,37,47,34,22,23] | $X_{10,10,10,9,9,5,4,4,3,3,1}$ [120] |
| | [2,0,2,2,0,0,0,1,2,2] | [2,6,10,16,24,32,40,48,34,22,23] | $X_{10,10,9,9,7,7,6,6,2,1,1}$ [120] |
| | [2,0,3,0,0,1,1,0,2,2] | [2,6,10,17,24,31,39,48,34,22,23] | $X_{10,10,9,9,7,7,7,4,3,1,1}$ [144] |
| | [2,1,0,2,1,0,1,0,2,2] | [2,6,11,16,23,31,39,48,34,22,23] | $X_{10,10,9,9,8,6,6,5,3,1,1}$ [216] |
| | [2,1,1,0,1,2,0,0,2,2] | [2,6,11,17,23,30,39,48,34,22,23] | $X_{10,10,9,9,8,7,5,4,4,1,1}$ [192] |
| | [2,1,1,0,2,0,0,2,1,1] | [2,6,11,17,23,31,39,47,34,22,23] | $X_{10,10,9,9,8,7,5,5,2,2,1}$ [192] |
| | [2,1,1,1,0,0,2,1,1,1] | [2,6,11,17,24,31,38,47,34,22,23] | $X_{10,10,9,9,8,7,6,3,3,2,1}$ [256] |
| | [2,2,0,0,0,2,1,1,1,1] | [2,6,12,18,24,30,38,47,34,22,23] | $X_{10,10,9,9,8,8,4,4,3,2,1}$ [160] |
| | [2,2,0,1,0,0,0,4,0,0] | [2,6,12,18,25,32,39,46,34,22,23] | $X_{10,10,9,9,8,8,6,2,2,2,2}$ [60] |
| | [3,0,0,1,1,1,1,1,1,1] | [2,7,12,17,23,30,38,47,34,22,23] | $X_{10,10,9,9,9,6,5,4,3,2,1}$ [256] |
| | [3,0,1,0,1,0,1,3,0,0] | [2,7,12,18,24,31,38,46,34,22,23] | $X_{10,10,9,9,9,7,5,3,2,2,2}$ [108] |
| | [3,1,0,0,0,0,4,0,1,1] | [2,7,13,19,25,31,37,47,34,22,23] | $X_{10,10,9,9,9,8,3,3,3,3,1}$ [72] |
| | [3,2,0,2,0,0,0,0,3,3] | [1,5,11,17,25,33,41,49,34,22,23] | $X_{10,9,9,9,8,8,6,6,1,1,1}$ [72] |
| | [3,2,1,0,0,1,0,1,2,2] | [1,5,11,18,25,32,40,48,34,22,23] | $X_{10,9,9,9,8,8,7,4,2,1,1}$ [192] |
| | [4,0,1,1,1,0,0,1,2,2] | [1,6,11,17,24,32,40,48,34,22,23] | $X_{10,9,9,9,9,7,6,5,2,1,1}$ [192] |
| | [4,1,0,0,1,1,1,0,2,2] | [1,6,12,18,24,31,39,48,34,22,23] | $X_{10,9,9,9,9,8,5,4,3,1,1}$ [192] |
| | [4,1,0,1,0,0,1,2,1,1] | [1,6,12,18,25,32,39,47,34,22,23] | $X_{10,9,9,9,9,8,6,3,2,2,1}$ [192] |
| | [5,0,0,0,0,2,0,2,1,1] | [1,7,13,19,25,31,39,47,34,22,23] | $X_{10,9,9,9,9,9,4,4,2,2,1}$ [72] |
| | [6,1,0,0,0,0,1,0,3,3] | [0,6,13,20,27,34,41,49,34,22,23] | $X_{9,9,9,9,9,9,8,3,1,1,1}$ [72] |
| | [0,0,0,3,0,0,4,0,0,0] | [4,8,12,16,23,30,37,48,35,22,24] | $X_{10,10,10,10,6,6,6,3,3,3,3}$ [20] |
| | [0,0,1,0,2,1,3,0,0,0] | [4,8,12,17,22,29,37,48,35,22,24] | $X_{10,10,10,10,7,5,5,4,3,3,3}$ [48] |
| | [0,0,3,2,0,1,0,1,1,1] | [3,6,9,15,23,31,40,49,35,22,24] | $X_{10,10,10,7,7,7,6,6,4,2,1}$ [144] |
| | [0,0,4,0,1,0,2,0,1,1] | [3,6,9,16,23,31,39,49,35,22,24] | $X_{10,10,10,7,7,7,7,5,3,3,1}$ [108] |
| | [0,0,4,1,0,0,0,3,0,0] | [3,6,9,16,24,32,40,48,35,22,24] | $X_{10,10,10,7,7,7,7,6,2,2,2}$ [40] |
| | [0,1,0,0,0,5,0,1,0,0] | [4,8,13,18,23,28,38,48,35,22,24] | $X_{10,10,10,10,8,4,4,4,4,4,2}$ [45] |
| | [0,1,1,2,1,1,1,0,1,1] | [3,6,10,15,22,30,39,49,35,22,24] | $X_{10,10,10,8,7,6,6,5,4,3,1}$ [288] |
| | [0,1,1,3,0,0,1,2,0,0] | [3,6,10,15,23,31,39,48,35,22,24] | $X_{10,10,10,8,7,6,6,6,3,2,2}$ [96] |
| | [0,1,2,0,2,1,0,2,0,0] | [3,6,10,16,22,30,39,48,35,22,24] | $X_{10,10,10,8,7,7,5,5,4,2,2}$ [108] |
| | [0,1,2,1,0,1,2,1,0,0] | [3,6,10,16,23,30,38,48,35,22,24] | $X_{10,10,10,8,7,7,6,4,3,3,2}$ [144] |
| | [0,2,0,1,1,3,0,0,1,1] | [3,6,11,16,22,29,39,49,35,22,24] | $X_{10,10,10,8,8,6,5,4,4,4,1}$ [144] |
| | [0,2,0,1,2,0,2,1,0,0] | [3,6,11,16,22,30,38,48,35,22,24] | $X_{10,10,10,8,8,6,5,5,3,3,2}$ [108] |
| | [0,2,1,0,0,3,1,1,0,0] | [3,6,11,17,23,29,38,48,35,22,24] | $X_{10,10,10,8,8,7,4,4,4,3,2}$ [96] |
| | [0,3,2,1,0,1,0,0,2,2] | [2,4,9,16,24,32,41,50,35,22,24] | $X_{10,10,8,8,8,7,7,6,4,1,1}$ [144] |
| | [0,3,3,0,0,0,0,2,1,1] | [2,4,9,17,25,33,41,49,35,22,24] | $X_{10,10,8,8,8,7,7,7,2,2,1}$ [72] |
| | [0,4,0,1,2,0,0,0,2,2] | [2,4,10,16,23,32,41,50,35,22,24] | $X_{10,10,8,8,8,8,6,5,5,1,1}$ [90] |
| | [0,4,0,2,0,0,1,1,1,1] | [2,4,10,16,24,32,40,49,35,22,24] | $X_{10,10,8,8,8,8,6,6,3,2,1}$ [144] |
| | [0,4,1,0,0,2,0,1,1,1] | [2,4,10,17,24,31,40,49,35,22,24] | $X_{10,10,8,8,8,8,7,4,4,2,1}$ [144] |
| | [0,5,0,0,0,1,0,3,0,0] | [2,4,11,18,25,32,40,48,35,22,24] | $X_{10,10,8,8,8,8,8,4,2,2,2}$ [45] |
| | [1,0,0,3,1,1,0,2,0,0] | [3,7,11,15,22,30,39,48,35,22,24] | $X_{10,10,10,9,6,6,6,5,4,2,2}$ [96] |
| | [1,0,1,1,1,2,1,1,0,0] | [3,7,11,16,22,29,38,48,35,22,24] | $X_{10,10,10,9,7,6,5,4,4,3,2}$ [192] |
| | [1,0,2,0,1,0,4,0,0,0] | [3,7,11,17,23,30,37,48,35,22,24] | $X_{10,10,10,9,7,7,5,3,3,3,3}$ [54] |
| | [1,1,0,1,0,2,3,0,0,0] | [3,7,12,17,23,29,37,48,35,22,24] | $X_{10,10,10,9,8,6,4,4,3,3,3}$ [72] |

| | | | |
|---|---|---|---|
| | [1,1,2,2,1,0,0,0,2,2] | [2,5,9,15,23,32,41,50,35,22,24] | $X_{10,10,9,8,7,7,6,6,5,1,1}$ [160] |
| | [1,1,3,0,1,1,0,1,1,1] | [2,5,9,16,23,31,40,49,35,22,24] | $X_{10,10,9,8,7,7,7,5,4,2,1}$ [288] |
| | [1,2,0,3,0,1,0,1,1,1] | [2,5,10,15,23,31,40,49,35,22,24] | $X_{10,10,9,8,8,6,6,6,4,2,1}$ [216] |
| | [1,2,1,0,3,0,0,1,1,1] | [2,5,10,16,22,31,40,49,35,22,24] | $X_{10,10,9,8,8,7,5,5,5,2,1}$ [192] |
| | [1,2,1,1,0,2,1,0,1,1] | [2,5,10,16,23,30,39,49,35,22,24] | $X_{10,10,9,8,8,7,6,4,4,3,1}$ [288] |
| | [1,2,1,1,1,0,1,2,0,0] | [2,5,10,16,23,31,39,48,35,22,24] | $X_{10,10,9,8,8,7,6,5,3,2,2}$ [192] |
| | [1,3,0,0,1,2,0,2,0,0] | [2,5,11,17,23,30,39,48,35,22,24] | $X_{10,10,9,8,8,8,5,4,4,2,2}$ [96] |
| | [2,0,1,2,2,0,0,1,1,1] | [2,6,10,15,22,31,40,49,35,22,24] | $X_{10,10,9,9,7,6,6,5,5,2,1}$ [192] |
| | [2,0,1,3,0,0,2,0,1,1] | [2,6,10,15,23,31,39,49,35,22,24] | $X_{10,10,9,9,7,6,6,6,3,3,1}$ [144] |
| | [2,0,2,0,2,1,1,0,1,1] | [2,6,10,16,22,30,39,49,35,22,24] | $X_{10,10,9,9,7,7,5,5,4,3,1}$ [216] |
| | [2,0,2,1,0,2,0,2,0,0] | [2,6,10,16,23,30,39,48,35,22,24] | $X_{10,10,9,9,7,7,6,4,4,2,2}$ [108] |
| | [2,0,3,0,0,0,3,1,0,0] | [2,6,10,17,24,31,38,48,35,22,24] | $X_{10,10,9,9,7,7,7,3,3,3,2}$ [60] |
| | [2,1,0,1,2,1,0,2,0,0] | [2,6,11,16,22,30,39,48,35,22,24] | $X_{10,10,9,9,8,6,5,5,4,2,2}$ [144] |
| | [2,1,0,2,0,1,2,1,0,0] | [2,6,11,16,23,30,38,48,35,22,24] | $X_{10,10,9,9,8,6,6,4,3,3,2}$ [144] |
| | [2,1,1,0,0,4,0,0,1,1] | [2,6,11,17,23,29,39,49,35,22,24] | $X_{10,10,9,9,8,7,4,4,4,4,1}$ [128] |
| | [2,2,3,0,0,0,1,0,2,2] | [1,4,9,17,25,33,41,50,35,22,24] | $X_{10,9,9,8,8,7,7,7,3,1,1}$ [120] |
| | [2,3,0,2,0,1,0,0,2,2] | [1,4,10,16,24,32,41,50,35,22,24] | $X_{10,9,9,8,8,8,6,6,4,1,1}$ [144] |
| | [2,3,1,0,1,0,1,1,1,1] | [1,4,10,17,24,32,40,49,35,22,24] | $X_{10,9,9,8,8,8,7,5,3,2,1}$ [288] |
| | [3,0,0,0,2,3,0,0,1,1] | [2,7,12,17,22,29,39,49,35,22,24] | $X_{10,10,9,9,9,5,5,4,4,4,1}$ [80] |
| | [3,0,0,0,3,0,2,1,0,0] | [2,7,12,17,22,30,38,48,35,22,24] | $X_{10,10,9,9,9,5,5,5,3,3,2}$ [60] |
| | [3,0,0,1,0,3,1,1,0,0] | [2,7,12,17,23,29,38,48,35,22,24] | $X_{10,10,9,9,9,6,4,4,4,3,2}$ [96] |
| | [3,0,1,0,0,1,4,0,0,0] | [2,7,12,18,24,30,37,48,35,22,24] | $X_{10,10,9,9,9,7,4,3,3,3,3}$ [48] |
| | [3,0,3,1,0,1,0,0,2,2] | [1,5,9,16,24,32,41,50,35,22,24] | $X_{10,9,9,9,7,7,7,6,4,1,1}$ [144] |
| | [3,0,4,0,0,0,0,2,1,1] | [1,5,9,17,25,33,41,49,35,22,24] | $X_{10,9,9,9,7,7,7,7,2,2,1}$ [72] |
| | [3,1,1,1,1,1,0,1,1,1] | [1,5,10,16,23,31,40,49,35,22,24] | $X_{10,9,9,9,8,7,6,5,4,2,1}$ [384] |
| | [3,1,2,0,0,1,2,0,1,1] | [1,5,10,17,24,31,39,49,35,22,24] | $X_{10,9,9,9,8,7,7,4,3,3,1}$ [192] |
| | [3,1,2,0,1,0,0,3,0,0] | [1,5,10,17,24,32,40,48,35,22,24] | $X_{10,9,9,9,8,7,7,5,2,2,2}$ [96] |
| | [3,2,0,0,2,0,2,0,1,1] | [1,5,11,17,23,31,39,49,35,22,24] | $X_{10,9,9,9,8,8,5,5,3,3,1}$ [144] |
| | [3,2,0,1,0,1,1,2,0,0] | [1,5,11,17,24,31,39,48,35,22,24] | $X_{10,9,9,9,8,8,6,4,3,2,2}$ [144] |
| | [4,0,0,2,1,0,2,0,1,1] | [1,6,11,16,23,31,39,49,35,22,24] | $X_{10,9,9,9,9,6,6,5,3,3,1}$ [144] |
| | [4,0,1,0,1,2,1,0,1,1] | [1,6,11,17,23,30,39,49,35,22,24] | $X_{10,9,9,9,9,7,5,4,4,3,1}$ [216] |
| | [4,0,1,0,2,0,1,2,0,0] | [1,6,11,17,23,31,39,48,35,22,24] | $X_{10,9,9,9,9,7,5,5,3,2,2}$ [108] |
| | [4,1,0,0,0,3,0,2,0,0] | [1,6,12,18,24,30,39,48,35,22,24] | $X_{10,9,9,9,9,8,4,4,4,2,2}$ [60] |
| | [4,1,0,0,1,0,3,1,0,0] | [1,6,12,18,24,31,38,48,35,22,24] | $X_{10,9,9,9,9,8,5,3,3,3,2}$ [96] |
| | [4,2,2,0,0,0,0,1,2,2] | [0,4,10,18,26,34,42,50,35,22,24] | $X_{9,9,9,9,8,8,7,7,2,1,1}$ [96] |
| | [4,3,0,0,1,0,1,0,2,2] | [0,4,11,18,25,33,41,50,35,22,24] | $X_{9,9,9,9,8,8,8,5,3,1,1}$ [144] |
| | [5,0,2,1,0,0,1,0,2,2] | [0,5,10,17,25,33,41,50,35,22,24] | $X_{9,9,9,9,9,7,7,6,3,1,1}$ [144] |
| | [5,1,0,1,1,1,0,0,2,2] | [0,5,11,17,24,32,41,50,35,22,24] | $X_{9,9,9,9,9,8,6,5,4,1,1}$ [192] |
| | [5,1,0,2,0,0,0,2,1,1] | [0,5,11,17,25,33,41,49,35,22,24] | $X_{9,9,9,9,9,8,6,6,2,2,1}$ [120] |
| | [5,1,1,0,0,1,1,1,1,1] | [0,5,11,18,25,32,40,49,35,22,24] | $X_{9,9,9,9,9,8,7,4,3,2,1}$ [256] |
| | [6,0,0,0,2,0,1,1,1,1] | [0,6,12,18,24,32,40,49,35,22,24] | $X_{9,9,9,9,9,9,5,5,3,2,1}$ [120] |
| | [6,0,1,0,0,0,1,3,0,0] | [0,6,12,19,26,33,40,48,35,22,24] | $X_{9,9,9,9,9,9,7,3,2,2,2}$ [60] |
| | [0,0,1,0,1,5,0,0,0,0] | [4,8,12,17,22,28,39,50,36,22,25] | $X_{10,10,10,10,7,5,4,4,4,4,4}$ [24] |
| | [0,0,2,3,1,1,0,0,1,1] | [3,6,9,14,22,31,41,51,36,22,25] | $X_{10,10,10,7,7,6,6,6,5,4,1}$ [128] |
| | [0,0,3,1,1,2,0,1,0,0] | [3,6,9,15,22,30,40,50,36,22,25] | $X_{10,10,10,7,7,7,6,5,4,4,2}$ [96] |
| | [0,0,3,2,0,0,3,0,0,0] | [3,6,9,15,23,31,39,50,36,22,25] | $X_{10,10,10,7,7,7,6,6,3,3,3}$ [32] |
| | [0,1,0,4,1,0,1,1,0,0] | [3,6,10,14,22,31,40,50,36,22,25] | $X_{10,10,10,8,6,6,6,6,5,3,2}$ [108] |
| | [0,1,2,0,1,3,1,0,0,0] | [3,6,10,16,22,29,39,50,36,22,25] | $X_{10,10,10,8,7,7,5,4,4,4,3}$ [72] |
| | [0,2,3,2,0,0,0,1,1,1] | [2,4,8,15,24,33,42,51,36,22,25] | $X_{10,10,8,8,7,7,7,6,6,2,1}$ [120] |
| | [0,2,4,0,0,1,1,0,1,1] | [2,4,8,16,24,32,41,51,36,22,25] | $X_{10,10,8,8,7,7,7,7,4,3,1}$ [144] |
| | [0,3,1,2,0,2,0,0,1,1] | [2,4,9,15,23,31,41,51,36,22,25] | $X_{10,10,8,8,8,7,6,6,4,4,1}$ [144] |
| | [0,3,1,2,1,0,0,2,0,0] | [2,4,9,15,23,32,41,50,36,22,25] | $X_{10,10,8,8,8,7,6,6,5,2,2}$ [96] |
| | [0,3,2,0,1,1,1,1,0,0] | [2,4,9,16,23,31,40,50,36,22,25] | $X_{10,10,8,8,8,7,7,5,4,3,2}$ [144] |
| | [0,4,0,0,3,1,0,0,1,1] | [2,4,10,16,22,31,41,51,36,22,25] | $X_{10,10,8,8,8,8,5,5,5,4,1}$ [96] |
| | [1,0,0,3,0,3,1,0,0,0] | [3,7,11,15,22,29,39,50,36,22,25] | $X_{10,10,10,9,6,6,6,4,4,4,3}$ [48] |
| | [1,0,4,1,1,0,1,0,1,1] | [2,5,8,15,23,32,41,51,36,22,25] | $X_{10,10,9,7,7,7,7,6,5,3,1}$ [216] |
| | [1,0,5,0,0,1,0,2,0,0] | [2,5,8,16,24,32,41,50,36,22,25] | $X_{10,10,9,7,7,7,7,7,4,2,2}$ [72] |
| | [1,1,1,4,0,0,1,0,1,1] | [2,5,9,14,23,32,41,51,36,22,25] | $X_{10,10,9,8,7,6,6,6,6,3,1}$ [192] |
| | [1,1,2,1,2,0,1,1,0,0] | [2,5,9,15,22,31,40,50,36,22,25] | $X_{10,10,9,8,7,7,6,5,5,3,2}$ [192] |
| | [1,1,3,0,0,3,0,1,0,0] | [2,5,9,16,23,30,40,50,36,22,25] | $X_{10,10,9,8,7,7,7,4,4,4,2}$ [96] |
| | [1,1,3,0,1,0,3,0,0,0] | [2,5,9,16,23,31,39,50,36,22,25] | $X_{10,10,9,8,7,7,7,5,3,3,3}$ [72] |
| | [1,2,0,2,1,2,0,1,0,0] | [2,5,10,15,22,30,40,50,36,22,25] | $X_{10,10,9,8,8,6,6,5,4,4,2}$ [144] |
| | [1,2,0,3,0,0,3,0,0,0] | [2,5,10,15,23,31,39,50,36,22,25] | $X_{10,10,9,8,8,6,6,6,3,3,3}$ [48] |
| | [1,2,1,0,2,1,2,0,0,0] | [2,5,10,16,22,30,39,50,36,22,25] | $X_{10,10,9,8,8,7,5,5,4,3,3}$ [96] |
| | [1,4,1,1,1,0,0,1,1,1] | [1,3,9,16,24,33,42,51,36,22,25] | $X_{10,9,8,8,8,8,7,6,5,2,1}$ [256] |
| | [1,4,2,0,0,0,2,0,1,1] | [1,3,9,17,25,33,41,51,36,22,25] | $X_{10,9,8,8,8,8,7,7,3,3,1}$ [120] |
| | [1,5,0,0,1,1,1,0,1,1] | [1,3,10,17,24,32,41,51,36,22,25] | $X_{10,9,8,8,8,8,8,5,4,3,1}$ [192] |
| | [1,5,0,1,0,0,1,2,0,0] | [1,3,10,17,25,33,41,50,36,22,25] | $X_{10,9,8,8,8,8,8,6,3,2,2}$ [96] |
| | [2,0,0,4,1,1,0,0,1,1] | [2,6,10,14,22,31,41,51,36,22,25] | $X_{10,10,9,9,6,6,6,6,5,4,1}$ [128] |
| | [2,0,0,5,0,0,0,2,0,0] | [2,6,10,14,23,32,41,50,36,22,25] | $X_{10,10,9,9,6,6,6,6,6,2,2}$ [40] |
| | [2,0,1,2,1,1,2,0,0,0] | [2,6,10,15,22,30,39,50,36,22,25] | $X_{10,10,9,9,7,6,6,5,4,3,3}$ [96] |

| | | | |
|---|---|---|---|
| | [2,1,0,1,1,3,1,0,0,0] | [2,6,11,16,22,29,39,50,36,22,25] | $X_{10,10,9,9,8,6,5,4,4,4,3}$ [96] |
| | [2,1,4,0,1,0,0,1,1,1] | [1,4,8,16,24,33,42,51,36,22,25] | $X_{10,9,9,8,7,7,7,7,5,2,1}$ [192] |
| | [2,2,1,2,1,0,1,0,1,1] | [1,4,9,15,23,32,41,51,36,22,25] | $X_{10,9,9,8,8,7,6,6,5,3,1}$ [288] |
| | [2,2,2,0,1,2,0,0,1,1] | [1,4,9,16,23,31,41,51,36,22,25] | $X_{10,9,9,8,8,7,7,5,4,4,1}$ [192] |
| | [2,2,2,1,0,0,2,1,0,0] | [1,4,9,16,24,32,40,50,36,22,25] | $X_{10,9,9,8,8,7,7,6,3,3,2}$ [128] |
| | [2,3,0,1,1,1,1,1,0,0] | [1,4,10,16,23,31,40,50,36,22,25] | $X_{10,9,9,8,8,8,6,5,4,3,2}$ [192] |
| | [3,0,2,2,0,2,0,0,1,1] | [1,5,9,15,23,31,41,51,36,22,25] | $X_{10,9,9,9,7,7,6,6,4,4,1}$ [144] |
| | [3,0,2,2,1,0,0,2,0,0] | [1,5,9,15,23,32,41,50,36,22,25] | $X_{10,9,9,9,7,7,6,6,5,2,2}$ [96] |
| | [3,0,3,0,1,1,1,1,0,0] | [1,5,9,16,23,31,40,50,36,22,25] | $X_{10,9,9,9,7,7,7,5,4,3,2}$ [144] |
| | [3,1,0,2,2,1,0,0,1,1] | [1,5,10,15,22,31,41,51,36,22,25] | $X_{10,9,9,9,8,6,6,5,5,4,1}$ [192] |
| | [3,1,0,3,0,1,1,1,0,0] | [1,5,10,15,23,31,40,50,36,22,25] | $X_{10,9,9,9,8,6,6,6,4,3,2}$ [144] |
| | [3,1,1,0,3,0,1,1,0,0] | [1,5,10,16,22,31,40,50,36,22,25] | $X_{10,9,9,9,8,7,5,5,5,3,2}$ [144] |
| | [3,1,1,1,0,3,0,1,0,0] | [1,5,10,16,23,30,40,50,36,22,25] | $X_{10,9,9,9,8,7,6,4,4,4,2}$ [144] |
| | [3,1,1,1,1,0,3,0,0,0] | [1,5,10,16,23,31,39,50,36,22,25] | $X_{10,9,9,9,8,7,6,5,3,3,3}$ [96] |
| | [3,2,0,0,1,2,2,0,0,0] | [1,5,11,17,23,30,39,50,36,22,25] | $X_{10,9,9,9,8,8,5,4,4,3,3}$ [64] |
| | [3,3,2,0,1,0,0,0,2,2] | [0,3,9,17,25,34,43,52,36,22,25] | $X_{9,9,9,8,8,8,7,7,5,1,1}$ [120] |
| | [3,4,0,1,0,1,0,1,1,1] | [0,3,10,17,25,33,42,51,36,22,25] | $X_{9,9,9,8,8,8,8,6,4,2,1}$ [216] |
| | [4,0,0,1,2,2,0,1,0,0] | [1,6,11,16,22,30,40,50,36,22,25] | $X_{10,9,9,9,9,6,5,5,4,4,2}$ [96] |
| | [4,1,2,1,1,0,0,1,1,1] | [0,4,9,16,24,33,42,51,36,22,25] | $X_{9,9,9,9,8,7,7,6,5,2,1}$ [256] |
| | [4,1,3,0,0,0,2,0,1,1] | [0,4,9,17,25,33,41,51,36,22,25] | $X_{9,9,9,9,8,7,7,7,3,3,1}$ [120] |
| | [4,2,0,2,0,1,1,0,1,1] | [0,4,10,16,24,32,41,51,36,22,25] | $X_{9,9,9,9,8,8,6,6,4,3,1}$ [216] |
| | [4,2,1,0,1,1,0,2,0,0] | [0,4,10,17,24,32,41,50,36,22,25] | $X_{9,9,9,9,8,8,7,5,4,2,2}$ [144] |
| | [4,3,0,0,0,1,2,1,0,0] | [0,4,11,18,25,32,40,50,36,22,25] | $X_{9,9,9,9,8,8,8,4,3,3,2}$ [80] |
| | [5,0,1,1,2,0,1,0,1,1] | [0,5,10,16,23,32,41,51,36,22,25] | $X_{9,9,9,9,9,7,6,5,5,3,1}$ [216] |
| | [5,0,1,2,0,1,0,2,0,0] | [0,5,10,16,24,32,41,50,36,22,25] | $X_{9,9,9,9,9,7,6,6,4,2,2}$ [108] |
| | [5,0,2,0,0,3,0,0,1,1] | [0,5,10,17,24,31,41,51,36,22,25] | $X_{9,9,9,9,9,7,7,4,4,4,1}$ [96] |
| | [5,0,2,0,1,0,2,1,0,0] | [0,5,10,17,24,32,40,50,36,22,25] | $X_{9,9,9,9,9,7,7,5,3,3,2}$ [108] |
| | [5,1,0,0,2,2,0,0,1,1] | [0,5,11,17,23,31,41,51,36,22,25] | $X_{9,9,9,9,9,8,5,5,4,4,1}$ [128] |
| | [5,1,0,0,3,0,0,2,0,0] | [0,5,11,17,23,32,41,50,36,22,25] | $X_{9,9,9,9,9,8,5,5,5,2,2}$ [64] |
| | [5,1,0,1,0,2,1,1,0,0] | [0,5,11,17,24,31,40,50,36,22,25] | $X_{9,9,9,9,9,8,6,4,4,3,2}$ [144] |
| | [6,0,0,1,0,0,4,0,0,0] | [0,6,12,18,25,32,39,50,36,22,25] | $X_{9,9,9,9,9,9,6,3,3,3,3}$ [32] |
| | [0,1,0,4,0,3,0,0,0,0] | [3,6,10,14,22,30,41,52,37,22,26] | $X_{10,10,10,8,6,6,6,6,4,4,4}$ [27] |
| | [0,1,6,0,0,0,1,0,1,1] | [2,4,7,16,25,34,43,53,37,22,26] | $X_{10,10,8,7,7,7,7,7,7,3,1}$ [90] |
| | [0,2,2,3,1,0,0,0,1,1] | [2,4,8,14,23,33,43,53,37,22,26] | $X_{10,10,8,8,7,7,6,6,6,5,1}$ [120] |
| | [0,2,3,1,1,0,2,0,0,0] | [2,4,8,15,23,32,41,52,37,22,26] | $X_{10,10,8,8,7,7,7,6,5,3,3}$ [72] |
| | [0,3,0,4,0,1,0,1,0,0] | [2,4,9,14,23,32,42,52,37,22,26] | $X_{10,10,8,8,8,6,6,6,6,4,2}$ [81] |
| | [0,3,1,1,2,1,1,0,0,0] | [2,4,9,15,22,31,41,52,37,22,26] | $X_{10,10,8,8,8,7,6,5,5,4,3}$ [96] |
| | [0,4,0,1,0,4,0,0,0,0] | [2,4,10,16,23,30,41,52,37,22,26] | $X_{10,10,8,8,8,8,6,4,4,4,4}$ [27] |
| | [0,6,1,0,1,0,1,0,1,1] | [1,2,9,17,25,34,43,53,37,22,26] | $X_{10,8,8,8,8,8,8,7,5,3,1}$ [162] |
| | [0,7,0,0,0,1,0,2,0,0] | [1,2,10,18,26,34,43,52,37,22,26] | $X_{10,8,8,8,8,8,8,8,4,2,2}$ [45] |
| | [1,0,3,3,0,1,0,1,0,0] | [2,5,8,14,23,32,42,52,37,22,26] | $X_{10,10,9,7,7,7,6,6,6,4,2}$ [108] |
| | [1,0,4,0,3,0,0,1,0,0] | [2,5,8,15,22,32,42,52,37,22,26] | $X_{10,10,9,7,7,7,7,5,5,5,2}$ [72] |
| | [1,0,4,1,0,2,1,0,0,0] | [2,5,8,15,23,31,41,52,37,22,26] | $X_{10,10,9,7,7,7,7,6,4,4,3}$ [72] |
| | [1,1,1,3,1,1,1,0,0,0] | [2,5,9,14,22,31,41,52,37,22,26] | $X_{10,10,9,8,7,6,6,6,5,4,3}$ [128] |
| | [1,1,2,1,1,3,0,0,0,0] | [2,5,9,15,22,30,41,52,37,22,26] | $X_{10,10,9,8,7,7,6,5,4,4,4}$ [64] |
| | [1,3,2,2,0,1,0,0,1,1] | [1,3,8,15,24,33,43,53,37,22,26] | $X_{10,9,8,8,8,7,7,6,6,4,1}$ [192] |
| | [1,3,3,0,1,0,1,1,0,0] | [1,3,8,16,24,33,42,52,37,22,26] | $X_{10,9,8,8,8,7,7,7,5,3,2}$ [144] |
| | [1,4,0,2,2,0,0,0,1,1] | [1,3,9,15,23,33,43,53,37,22,26] | $X_{10,9,8,8,8,8,6,6,5,5,1}$ [120] |
| | [1,4,0,3,0,0,1,1,0,0] | [1,3,9,15,24,33,42,52,37,22,26] | $X_{10,9,8,8,8,8,6,6,6,3,2}$ [96] |
| | [1,4,1,0,2,1,0,1,0,0] | [1,3,9,16,23,32,42,52,37,22,26] | $X_{10,9,8,8,8,8,7,5,5,4,2}$ [144] |
| | [1,4,1,1,0,1,2,0,0,0] | [1,3,9,16,24,32,41,52,37,22,26] | $X_{10,9,8,8,8,8,7,6,4,3,3}$ [96] |
| | [2,1,3,1,1,1,0,1,0,0] | [1,4,8,15,23,32,42,52,37,22,26] | $X_{10,9,9,8,7,7,7,6,5,4,2}$ [192] |
| | [2,1,4,0,0,1,2,0,0,0] | [1,4,8,16,24,32,41,52,37,22,26] | $X_{10,9,9,8,7,7,7,7,4,3,3}$ [64] |
| | [2,2,0,4,1,0,0,0,1,1] | [1,4,9,14,23,33,43,53,37,22,26] | $X_{10,9,9,8,8,6,6,6,6,5,1}$ [120] |
| | [2,2,1,1,3,0,0,1,0,0] | [1,4,9,15,22,32,42,52,37,22,26] | $X_{10,9,9,8,8,7,6,5,5,5,2}$ [128] |
| | [2,2,1,2,0,2,1,0,0,0] | [1,4,9,15,23,31,41,52,37,22,26] | $X_{10,9,9,8,8,7,6,6,4,4,3}$ [96] |
| | [2,3,0,0,3,1,1,0,0,0] | [1,4,10,16,22,31,41,52,37,22,26] | $X_{10,9,9,8,8,8,5,5,5,4,3}$ [64] |
| | [2,5,1,1,0,0,0,1,1,1] | [0,2,9,17,26,35,44,53,37,22,26] | $X_{9,9,8,8,8,8,8,7,6,2,1}$ [160] |
| | [2,6,0,0,0,1,1,0,1,1] | [0,2,10,18,26,34,43,53,37,22,26] | $X_{9,9,8,8,8,8,8,8,4,3,1}$ [120] |
| | [3,0,1,4,0,1,0,1,0,0] | [1,5,9,14,23,32,42,52,37,22,26] | $X_{10,9,9,9,7,6,6,6,6,4,2}$ [108] |
| | [3,0,2,1,2,1,1,0,0,0] | [1,5,9,15,22,31,41,52,37,22,26] | $X_{10,9,9,9,7,7,6,5,5,4,3}$ [96] |
| | [3,1,1,0,2,3,0,0,0,0] | [1,5,10,16,22,30,41,52,37,22,26] | $X_{10,9,9,9,8,7,5,5,4,4,4}$ [48] |
| | [3,2,3,1,0,0,1,0,1,1] | [0,3,8,16,25,34,43,53,37,22,26] | $X_{9,9,9,8,8,7,7,7,6,3,1}$ [192] |
| | [3,3,1,1,1,0,1,1,0,0] | [0,3,9,16,24,33,42,52,37,22,26] | $X_{9,9,9,8,8,8,7,6,5,3,2}$ [192] |
| | [3,4,0,0,1,2,0,1,0,0] | [0,3,10,17,24,32,42,52,37,22,26] | $X_{9,9,9,8,8,8,8,5,4,4,2}$ [96] |
| | [3,4,0,1,0,0,3,0,0,0] | [0,3,10,17,25,33,41,52,37,22,26] | $X_{9,9,9,8,8,8,8,6,3,3,3}$ [48] |
| | [4,0,4,0,1,1,0,0,1,1] | [0,4,8,16,24,33,43,53,37,22,26] | $X_{9,9,9,9,7,7,7,7,5,4,1}$ [144] |
| | [4,0,4,1,0,0,0,2,0,0] | [0,4,8,16,25,34,43,52,37,22,26] | $X_{9,9,9,9,7,7,7,7,6,2,2}$ [60] |
| | [4,1,1,2,2,0,0,0,1,1] | [0,4,9,15,23,33,43,53,37,22,26] | $X_{9,9,9,9,8,7,6,6,5,5,1}$ [160] |
| | [4,1,1,3,0,0,1,1,0,0] | [0,4,9,15,24,33,42,52,37,22,26] | $X_{9,9,9,9,8,7,6,6,6,3,2}$ [128] |
| | [4,1,2,0,2,1,0,1,0,0] | [0,4,9,16,23,32,42,52,37,22,26] | $X_{9,9,9,9,8,7,7,5,5,4,2}$ [144] |

| | | | | |
|---|---|---|---|---|
| | [4,1,2,1,0,1,2,0,0,0] | [0,4,9,16,24,32,41,52,37,22,26] | $X_{9,9,9,9,8,7,7,6,4,3,3}$ [96] | |
| | [4,2,0,1,2,0,2,0,0,0] | [0,4,10,16,23,32,41,52,37,22,26] | $X_{9,9,9,9,8,8,6,5,5,3,3}$ [72] | |
| | [4,2,1,0,0,3,1,0,0,0] | [0,4,10,17,24,31,41,52,37,22,26] | $X_{9,9,9,9,8,8,7,4,4,4,3}$ [64] | |
| | [5,0,0,3,1,1,0,1,0,0] | [0,5,10,15,23,32,42,52,37,22,26] | $X_{9,9,9,9,9,6,6,6,5,4,2}$ [96] | |
| | [5,0,1,1,1,2,1,0,0,0] | [0,5,10,16,23,31,41,52,37,22,26] | $X_{9,9,9,9,9,7,6,5,4,4,3}$ [96] | |
| | [0,0,1,6,0,0,1,0,0,0] | [3,6,9,13,23,33,43,54,38,22,27] | $X_{10,10,10,7,6,6,6,6,6,6,3}$ [32] | |
| | [0,1,5,1,0,1,1,0,0,0] | [2,4,7,15,24,33,43,54,38,22,27] | $X_{10,10,8,7,7,7,7,7,6,4,3}$ [72] | |
| | [0,2,2,3,0,2,0,0,0,0] | [2,4,8,14,23,32,43,54,38,22,27] | $X_{10,10,8,8,7,7,6,6,6,4,4}$ [36] | |
| | [0,2,3,0,3,1,0,0,0,0] | [2,4,8,15,22,32,43,54,38,22,27] | $X_{10,10,8,8,7,7,7,5,5,5,4}$ [36] | |
| | [0,3,0,3,2,1,0,0,0,0] | [2,4,9,14,22,32,43,54,38,22,27] | $X_{10,10,8,8,8,6,6,6,5,5,4}$ [36] | |
| | [0,5,2,1,0,1,0,1,0,0] | [1,2,8,16,25,34,44,54,38,22,27] | $X_{10,8,8,8,8,8,7,7,6,4,2}$ [108] | |
| | [0,6,0,1,2,0,0,1,0,0] | [1,2,9,16,24,34,44,54,38,22,27] | $X_{10,8,8,8,8,8,8,6,5,5,2}$ [72] | |
| | [0,6,1,0,0,2,1,0,0,0] | [1,2,9,17,25,33,43,54,38,22,27] | $X_{10,8,8,8,8,8,8,7,4,4,3}$ [48] | |
| | [1,0,3,2,2,1,0,0,0,0] | [2,5,8,14,22,32,43,54,38,22,27] | $X_{10,10,9,7,7,7,6,6,5,5,4}$ [48] | |
| | [1,2,4,2,0,0,0,0,1,1] | [1,3,7,15,25,35,45,55,38,22,27] | $X_{10,9,8,8,7,7,7,7,6,6,1}$ [96] | |
| | [1,2,5,0,0,1,0,1,0,0] | [1,3,7,16,25,34,44,54,38,22,27] | $X_{10,9,8,8,7,7,7,7,7,4,2}$ [96] | |
| | [1,3,2,1,2,0,1,0,0,0] | [1,3,8,15,23,33,43,54,38,22,27] | $X_{10,9,8,8,8,7,7,6,5,5,3}$ [96] | |
| | [1,4,0,2,1,2,0,0,0,0] | [1,3,9,15,23,32,43,54,38,22,27] | $X_{10,9,8,8,8,8,6,6,5,4,4}$ [48] | |
| | [2,0,5,1,1,0,0,1,0,0] | [1,4,7,15,24,34,44,54,38,22,27] | $X_{10,9,9,7,7,7,7,7,6,5,2}$ [96] | |
| | [2,1,2,3,1,0,1,0,0,0] | [1,4,8,14,23,33,43,54,38,22,27] | $X_{10,9,9,8,7,7,6,6,6,5,3}$ [96] | |
| | [2,4,2,1,1,0,0,0,1,1] | [0,2,8,16,25,35,45,55,38,22,27] | $X_{9,9,8,8,8,8,7,7,6,5,1}$ [160] | |
| | [2,4,3,0,0,0,1,1,0,0] | [0,2,8,17,26,35,44,54,38,22,27] | $X_{9,9,8,8,8,8,7,7,7,3,2}$ [80] | |
| | [2,5,0,2,0,1,0,1,0,0] | [0,2,9,16,25,34,44,54,38,22,27] | $X_{9,9,8,8,8,8,8,6,6,4,2}$ [108] | |
| | [2,5,1,0,1,0,2,0,0,0] | [0,2,9,17,25,34,43,54,38,22,27] | $X_{9,9,8,8,8,8,8,7,5,3,3}$ [72] | |
| | [3,0,1,3,2,1,0,0,0,0] | [1,5,9,14,22,32,43,54,38,22,27] | $X_{10,9,9,9,7,6,6,6,5,5,4}$ [48] | |
| | [3,2,2,2,1,0,0,1,0,0] | [0,3,8,15,24,34,44,54,38,22,27] | $X_{9,9,9,8,8,7,7,6,6,5,2}$ [128] | |
| | [3,2,3,0,1,1,1,0,0,0] | [0,3,8,16,24,33,43,54,38,22,27] | $X_{9,9,9,8,8,7,7,7,5,4,3}$ [96] | |
| | [3,3,0,3,0,1,1,0,0,0] | [0,3,9,15,24,33,43,54,38,22,27] | $X_{9,9,9,8,8,8,6,6,6,4,3}$ [72] | |
| | [3,3,1,0,3,0,1,0,0,0] | [0,3,9,16,23,33,43,54,38,22,27] | $X_{9,9,9,8,8,8,7,5,5,5,3}$ [72] | |
| | [3,3,1,1,0,3,0,0,0,0] | [0,3,9,16,24,32,43,54,38,22,27] | $X_{9,9,9,8,8,8,7,6,4,4,4}$ [48] | |
| | [4,0,3,2,0,1,1,0,0,0] | [0,4,8,15,24,33,43,54,38,22,27] | $X_{9,9,9,9,7,7,7,6,6,4,3}$ [72] | |
| | [4,1,1,2,1,2,0,0,0,0] | [0,4,9,15,23,32,43,54,38,22,27] | $X_{9,9,9,9,8,7,6,6,5,4,4}$ [64] | |
| | [5,0,1,0,4,1,0,0,0,0] | [0,5,10,16,22,32,43,54,38,22,27] | $X_{9,9,9,9,9,7,5,5,5,5,4}$ [36] | |
| | [0,1,5,0,3,0,0,0,0,0] | [2,4,7,15,23,34,45,56,39,22,28] | $X_{10,10,8,7,7,7,7,7,5,5,5}$ [18] | |
| | [0,4,4,1,0,0,0,1,0,0] | [1,2,7,16,26,36,46,56,39,22,28] | $X_{10,8,8,8,8,7,7,7,7,6,2}$ [60] | |
| | [0,5,1,3,0,0,1,0,0,0] | [1,2,8,15,25,35,45,56,39,22,28] | $X_{10,8,8,8,8,8,7,6,6,6,3}$ [48] | |
| | [0,5,2,0,2,1,0,0,0,0] | [1,2,8,16,24,34,45,56,39,22,28] | $X_{10,8,8,8,8,8,7,7,5,5,4}$ [36] | |
| | [1,1,0,6,1,0,0,0,0,0] | [2,5,9,13,23,34,45,56,39,22,28] | $X_{10,10,9,8,6,6,6,6,6,6,5}$ [24] | |
| | [1,2,4,1,1,1,0,0,0,0] | [1,3,7,15,24,34,45,56,39,22,28] | $X_{10,9,8,8,7,7,7,7,6,5,4}$ [64] | |
| | [1,3,1,4,0,1,0,0,0,0] | [1,3,8,14,24,34,45,56,39,22,28] | $X_{10,9,8,8,8,7,6,6,6,6,4}$ [48] | |
| | [1,7,0,2,0,0,0,0,1,1] | [0,1,9,17,27,37,47,57,39,22,28] | $X_{9,8,8,8,8,8,8,8,6,6,1}$ [72] | |
| | [1,7,1,0,0,1,0,1,0,0] | [0,1,9,18,27,36,46,56,39,22,28] | $X_{9,8,8,8,8,8,8,8,7,4,2}$ [96] | |
| | [2,3,5,0,0,0,0,0,1,1] | [0,2,7,17,27,37,47,57,39,22,28] | $X_{9,9,8,8,8,7,7,7,7,7,1}$ [56] | |
| | [2,4,2,1,0,2,0,0,0,0] | [0,2,8,16,25,34,45,56,39,22,28] | $X_{9,9,8,8,8,8,7,7,6,4,4}$ [48] | |
| | [2,5,0,1,2,1,0,0,0,0] | [0,2,9,16,24,34,45,56,39,22,28] | $X_{9,9,8,8,8,8,8,6,5,5,4}$ [48] | |
| | [3,1,5,0,1,0,1,0,0,0] | [0,3,7,16,25,35,45,56,39,22,28] | $X_{9,9,9,8,7,7,7,7,7,5,3}$ [72] | |
| | [3,3,0,2,3,0,0,0,0,0] | [0,3,9,15,23,34,45,56,39,22,28] | $X_{9,9,9,8,8,8,6,6,5,5,5}$ [24] | |
| | [4,0,3,1,3,0,0,0,0,0] | [0,4,8,15,23,34,45,56,39,22,28] | $X_{9,9,9,9,7,7,7,6,5,5,5}$ [24] | |
| | [4,1,0,5,0,1,0,0,0,0] | [0,4,9,14,24,34,45,56,39,22,28] | $X_{9,9,9,9,8,6,6,6,6,6,4}$ [36] | |
| | [1,6,2,1,0,0,1,0,0,0] | [0,1,8,17,27,37,47,58,40,22,29] | $X_{9,8,8,8,8,8,8,7,7,6,3}$ [64] | |
| | [1,7,0,1,1,1,0,0,0,0] | [0,1,9,17,26,36,47,58,40,22,29] | $X_{9,8,8,8,8,8,8,8,6,5,4}$ [48] | |
| | [2,3,4,1,0,1,0,0,0,0] | [0,2,7,16,26,36,47,58,40,22,29] | $X_{9,9,8,8,8,7,7,7,7,6,4}$ [48] | |
| | [2,4,1,3,1,0,0,0,0,0] | [0,2,8,15,25,36,47,58,40,22,29] | $X_{9,9,8,8,8,8,7,6,6,6,5}$ [32] | |
| | [3,1,4,2,1,0,0,0,0,0] | [0,3,7,15,25,36,47,58,40,22,29] | $X_{9,9,9,8,7,7,7,7,6,6,5}$ [32] | |
| | [4,0,2,5,0,0,0,0,0,0] | [0,4,8,14,25,36,47,58,40,22,29] | $X_{9,9,9,9,7,7,6,6,6,6,6}$ [12] | |
| | [0,0,8,1,0,0,0,0,0,0] | [2,4,6,16,27,38,49,60,41,22,30] | $X_{10,10,7,7,7,7,7,7,7,7,6}$ [8] | |
| | [0,10,0,1,0,0,0,0,0,0] | [0,0,10,20,31,42,53,64,43,22,32] | $X_{8,8,8,8,8,8,8,8,8,8,6}$ [9] | |
| | [0,0,1,0,0,0,1,0,6,2] | [5,10,15,21,27,33,39,46,31,22,22] | $X_{10,10,10,10,10,7,3,1,1,1,1,1,1}$ [60] | $X_{10,10,10,10,10,7,3,1,1}$ [60] |
| | [2,0,0,0,0,0,0,1,6,2] | [4,10,16,22,28,34,40,46,31,22,22] | $X_{10,10,10,10,9,9,2,1,1,1,1,1,1}$ [32] | $X_{10,10,10,10,9,9,2,1,1}$ [32] |
| | [0,0,0,0,0,3,0,0,4,2] | [5,10,15,20,25,30,38,46,32,22,22] | $X_{10,10,10,10,10,4,4,4,1,1,1,1}$ [28] | $X_{10,10,10,10,10,4,4,4,1,1}$ [28] |
| | [0,0,0,0,1,0,2,1,3,1] | [5,10,15,20,25,31,37,45,32,22,22] | $X_{10,10,10,10,10,5,3,3,2,1,1,1}$ [72] | $X_{10,10,10,10,10,5,3,3,2,1}$ [72] |
| | [0,0,3,0,0,0,0,0,5,3] | [4,8,12,19,26,33,40,47,32,22,22] | $X_{10,10,10,10,7,7,7,1,1,1,1,1}$ [28] | $X_{10,10,10,10,7,7,7,1,1,1}$ [28] |
| | [0,1,0,2,0,0,0,1,4,2] | [4,8,13,18,25,32,39,46,32,22,22] | $X_{10,10,10,10,8,6,6,2,1,1,1,1}$ [90] | $X_{10,10,10,10,8,6,6,2,1,1}$ [90] |
| | [0,1,1,0,0,1,1,0,4,2] | [4,8,13,19,25,31,38,46,32,22,22] | $X_{10,10,10,10,8,7,4,3,1,1,1,1}$ [144] | $X_{10,10,10,10,8,7,4,3,1,1}$ [144] |
| | [0,2,0,0,0,0,1,2,3,1] | [4,8,14,20,26,32,38,45,32,22,22] | $X_{10,10,10,10,8,8,3,2,2,1,1,1}$ [72] | $X_{10,10,10,10,8,8,3,2,2,1}$ [72] |
| | [1,0,0,0,2,0,1,0,4,2] | [4,9,14,19,24,31,38,46,32,22,22] | $X_{10,10,10,10,9,5,5,3,1,1,1,1}$ [90] | $X_{10,10,10,10,9,5,5,3,1,1}$ [90] |
| | [1,0,0,1,0,1,0,2,3,1] | [4,9,14,19,25,31,38,45,32,22,22] | $X_{10,10,10,10,9,6,4,2,2,1,1,1}$ [144] | $X_{10,10,10,10,9,6,4,2,2,1}$ [144] |
| | [1,2,0,1,0,0,0,0,5,3] | [3,7,13,19,26,33,40,47,32,22,22] | $X_{10,10,10,9,8,8,6,1,1,1,1,1}$ [72] | $X_{10,10,10,9,8,8,6,1,1,1}$ [72] |
| | [2,0,1,0,1,0,0,1,4,2] | [3,8,13,19,25,32,39,46,32,22,22] | $X_{10,10,10,9,9,7,5,2,1,1,1,1}$ [144] | $X_{10,10,10,9,9,7,5,2,1,1}$ [144] |
| | [2,1,0,0,0,0,2,0,4,2] | [3,8,14,20,26,32,38,46,32,22,22] | $X_{10,10,10,9,9,8,3,3,1,1,1,1}$ [72] | $X_{10,10,10,9,9,8,3,3,1,1}$ [72] |
| | [3,0,0,0,0,0,0,3,3,1] | [3,9,15,21,27,33,39,45,32,22,22] | $X_{10,10,10,9,9,9,2,2,2,1,1,1}$ [32] | $X_{10,10,10,9,9,9,2,2,2,1}$ [32] |

| | | | | |
|---|---|---|---|---|
| | [0,0,0,0,0,1,4,0,0,2] | [5,10,15,20,25,30,36,46,34,22,22] | $X_{10,10,10,10,10,4,3,3,3,3}$ [28] | $X_{10,10,10,10,10,4,3,3,3,3,1,1}$ [28] |
| | [0,0,0,3,1,0,0,1,1,3] | [4,8,12,16,23,31,39,47,34,22,22] | $X_{10,10,10,10,6,6,6,5,2,1}$ [80] | $X_{10,10,10,10,6,6,6,5,2,1,1,1}$ [80] |
| | [0,0,1,1,1,1,0,2,0,2] | [4,8,12,17,23,30,38,46,34,22,22] | $X_{10,10,10,10,7,6,5,4,2,2}$ [144] | $X_{10,10,10,10,7,6,5,4,2,2,1,1}$ [144] |
| | [0,0,2,0,0,1,2,1,0,2] | [4,8,12,18,24,30,37,46,34,22,22] | $X_{10,10,10,10,7,7,4,3,3,2}$ [96] | $X_{10,10,10,10,7,7,4,3,3,2,1,1}$ [96] |
| | [0,1,0,0,1,3,0,0,1,3] | [4,8,13,18,23,29,38,47,34,22,22] | $X_{10,10,10,10,8,5,4,4,4,1}$ [96] | $X_{10,10,10,10,8,5,4,4,4,1,1,1}$ [96] |
| | [0,1,0,0,2,0,2,1,0,2] | [4,8,13,18,23,30,37,46,34,22,22] | $X_{10,10,10,10,8,5,5,3,3,2}$ [108] | $X_{10,10,10,10,8,5,5,3,3,2,1,1}$ [108] |
| | [0,2,1,1,0,1,0,1,1,3] | [3,6,11,17,24,31,39,47,34,22,22] | $X_{10,10,10,8,8,7,6,4,2,1}$ [216] | $X_{10,10,10,8,8,7,6,4,2,1,1,1}$ [216] |
| | [0,3,0,0,1,0,2,0,1,3] | [3,6,12,18,24,31,38,47,34,22,22] | $X_{10,10,10,8,8,8,5,3,3,1}$ [108] | $X_{10,10,10,8,8,8,5,3,3,1,1,1}$ [108] |
| | [0,3,0,1,0,0,0,3,0,2] | [3,6,12,18,25,32,39,46,34,22,22] | $X_{10,10,10,8,8,8,6,2,2,2}$ [68] | $X_{10,10,10,8,8,8,6,2,2,2,1,1}$ [67] |
| | [1,0,0,0,0,3,1,1,0,2] | [4,9,14,19,24,29,37,46,34,22,22] | $X_{10,10,10,10,9,4,4,4,3,2}$ [72] | $X_{10,10,10,10,9,4,4,4,3,2,1,1}$ [72] |
| | [1,0,1,3,0,0,0,0,2,4] | [3,7,11,16,24,32,40,48,34,22,22] | $X_{10,10,10,9,7,6,6,6,1,1}$ [72] | $X_{10,10,10,9,7,6,6,6,1,1,1,1}$ [72] |
| | [1,0,2,0,2,0,0,1,1,3] | [3,7,11,17,23,31,39,47,34,22,22] | $X_{10,10,10,9,7,7,5,5,2,1}$ [144] | $X_{10,10,10,9,7,7,5,5,2,1,1,1}$ [144] |
| | [1,0,2,1,0,0,2,0,1,3] | [3,7,11,17,24,31,38,47,34,22,22] | $X_{10,10,10,9,7,7,6,3,3,1}$ [144] | $X_{10,10,10,9,7,7,6,3,3,1,1,1}$ [144] |
| | [1,0,3,0,0,0,0,3,0,2] | [3,7,11,18,25,32,39,46,34,22,22] | $X_{10,10,10,9,7,7,7,2,2,2}$ [54] | $X_{10,10,10,9,7,7,7,2,2,2,1,1}$ [54] |
| | [1,1,0,1,1,1,1,0,1,3] | [3,7,12,17,23,30,38,47,34,22,22] | $X_{10,10,10,9,8,6,5,4,3,1}$ [288] | $X_{10,10,10,9,8,6,5,4,3,1,1,1}$ [288] |
| | [1,1,0,2,0,0,1,2,0,2] | [3,7,12,17,24,31,38,46,34,22,22] | $X_{10,10,10,9,8,6,6,3,2,2}$ [144] | $X_{10,10,10,9,8,6,6,3,2,2,1,1}$ [144] |
| | [1,1,1,0,0,2,0,2,0,2] | [3,7,12,18,24,30,38,46,34,22,22] | $X_{10,10,10,9,8,7,4,4,2,2}$ [144] | $X_{10,10,10,9,8,7,4,4,2,2,1,1}$ [144] |
| | [1,2,0,0,0,0,3,1,0,2] | [3,7,13,19,25,31,37,46,34,22,22] | $X_{10,10,10,9,8,8,3,3,3,2}$ [72] | $X_{10,10,10,9,8,8,3,3,3,2,1,1}$ [72] |
| | [1,4,0,0,0,0,1,0,2,4] | [2,5,12,19,26,33,40,48,34,22,22] | $X_{10,10,9,8,8,8,8,3,1,1}$ [72] | $X_{10,10,9,8,8,8,8,3,1,1,1,1}$ [72] |
| | [2,0,0,0,2,1,0,2,0,2] | [3,8,13,18,23,30,38,46,34,22,22] | $X_{10,10,10,9,9,5,5,4,2,2}$ [90] | $X_{10,10,10,9,9,5,5,4,2,2,1,1}$ [90] |
| | [2,0,0,1,0,1,2,1,0,2] | [3,8,13,18,24,30,37,46,34,22,22] | $X_{10,10,10,9,9,6,4,3,3,2}$ [144] | $X_{10,10,10,9,9,6,4,3,3,2,1,1}$ [144] |
| | [2,1,1,1,1,0,0,0,2,4] | [2,6,11,17,24,32,40,48,34,22,22] | $X_{10,10,9,9,8,7,6,5,1,1}$ [160] | $X_{10,10,9,9,8,7,6,5,1,1,1,1}$ [160] |
| | [2,1,2,0,0,0,1,1,1,3] | [2,6,11,18,25,32,39,47,34,22,22] | $X_{10,10,9,9,8,7,7,3,2,1}$ [160] | $X_{10,10,9,9,8,7,7,3,2,1,1,1}$ [160] |
| | [2,2,0,0,1,1,0,1,1,3] | [2,6,12,18,24,31,39,47,34,22,22] | $X_{10,10,9,9,8,8,5,4,2,1}$ [192] | $X_{10,10,9,9,8,8,5,4,2,1,1,1}$ [192] |
| | [3,0,0,2,0,1,0,1,1,3] | [2,7,12,17,24,31,39,47,34,22,22] | $X_{10,10,9,9,9,6,6,4,2,1}$ [144] | $X_{10,10,9,9,9,6,6,4,2,1,1,1}$ [144] |
| | [3,0,1,0,1,0,2,0,1,3] | [2,7,12,18,24,31,38,47,34,22,22] | $X_{10,10,9,9,9,7,5,3,3,1}$ [162] | $X_{10,10,9,9,9,7,5,3,3,1,1,1}$ [162] |
| | [3,0,1,1,0,0,0,3,0,2] | [2,7,12,18,25,32,39,46,34,22,22] | $X_{10,10,9,9,9,7,6,2,2,2}$ [90] | $X_{10,10,9,9,9,7,6,2,2,2,1,1}$ [90] |
| | [3,1,0,0,0,1,1,2,0,2] | [2,7,13,19,25,31,38,46,34,22,22] | $X_{10,10,9,9,9,8,4,3,2,2}$ [120] | $X_{10,10,9,9,9,8,4,3,2,2,1,1}$ [120] |
| | [4,1,1,0,0,0,1,0,2,4] | [1,6,12,19,26,33,40,48,34,22,22] | $X_{10,9,9,9,9,8,7,3,1,1}$ [120] | $X_{10,9,9,9,9,8,7,3,1,1,1,1}$ [120] |
| | [5,0,0,0,1,1,0,0,2,4] | [1,7,13,19,25,32,40,48,34,22,22] | $X_{10,9,9,9,9,9,5,4,1,1}$ [80] | $X_{10,9,9,9,9,9,5,4,1,1,1,1}$ [80] |
| | [5,0,0,1,0,0,0,2,1,3] | [1,7,13,19,26,33,40,47,34,22,22] | $X_{10,9,9,9,9,9,6,2,2,1}$ [80] | $X_{10,9,9,9,9,9,6,2,2,1,1,1}$ [80] |
| | [0,0,0,3,0,2,0,0,0,4] | [4,8,12,16,23,30,39,48,35,22,22] | $X_{10,10,10,10,6,6,6,4,4}$ [38] | $X_{10,10,10,10,6,6,6,4,4,1,1,1,1}$ [37] |
| | [0,0,1,0,3,1,0,0,0,4] | [4,8,12,17,22,30,39,48,35,22,22] | $X_{10,10,10,10,7,5,5,5,4}$ [60] | $X_{10,10,10,10,7,5,5,5,4,1,1,1,1}$ [60] |
| | [0,1,3,0,1,0,0,1,0,4] | [3,6,10,17,24,32,40,48,35,22,22] | $X_{10,10,10,8,7,7,7,5,2}$ [108] | $X_{10,10,10,8,7,7,7,5,2,1,1,1,1}$ [108] |
| | [0,2,0,3,0,0,0,1,0,4] | [3,6,11,16,24,32,40,48,35,22,22] | $X_{10,10,10,8,8,6,6,6,2}$ [68] | $X_{10,10,10,8,8,6,6,6,2,1,1,1,1}$ [67] |
| | [0,2,1,0,2,0,1,0,0,4] | [3,6,11,17,23,31,39,48,35,22,22] | $X_{10,10,10,8,8,7,5,5,3}$ [108] | $X_{10,10,10,8,8,7,5,5,3,1,1,1,1}$ [108] |
| | [0,3,0,0,0,3,0,0,0,4] | [3,6,12,18,24,30,39,48,35,22,22] | $X_{10,10,10,8,8,8,4,4,4}$ [38] | $X_{10,10,10,8,8,8,4,4,4,1,1,1,1}$ [37] |
| | [1,0,1,2,1,0,1,0,0,4] | [3,7,11,16,23,31,39,48,35,22,22] | $X_{10,10,10,9,7,6,6,5,3}$ [144] | $X_{10,10,10,9,7,6,6,5,3,1,1,1,1}$ [144] |
| | [1,0,2,0,1,2,0,0,0,4] | [3,7,11,17,23,30,39,48,35,22,22] | $X_{10,10,10,9,7,7,5,4,4}$ [90] | $X_{10,10,10,9,7,7,5,4,4,1,1,1,1}$ [90] |
| | [1,3,0,2,0,0,0,0,1,5] | [2,5,11,17,25,33,41,49,35,22,22] | $X_{10,10,9,8,8,8,6,6,1}$ [72] | $X_{10,10,9,8,8,8,6,6,1,1,1,1,1}$ [72] |
| | [1,3,1,0,0,1,0,1,0,4] | [2,5,11,18,25,32,40,48,35,22,22] | $X_{10,10,9,8,8,8,7,4,2}$ [144] | $X_{10,10,9,8,8,8,7,4,2,1,1,1,1}$ [144] |
| | [2,0,3,1,0,0,0,0,1,5] | [2,6,10,17,25,33,41,49,35,22,22] | $X_{10,10,9,9,7,7,7,6,1}$ [72] | $X_{10,10,9,9,7,7,7,6,1,1,1,1,1}$ [72] |
| | [2,1,1,1,0,1,1,0,0,4] | [2,6,11,17,24,31,39,48,35,22,22] | $X_{10,10,9,9,8,7,6,4,3}$ [192] | $X_{10,10,9,9,8,7,6,4,3,1,1,1,1}$ [192] |
| | [3,0,0,1,2,0,1,0,0,4] | [2,7,12,17,23,31,39,48,35,22,22] | $X_{10,10,9,9,9,6,5,5,3}$ [96] | $X_{10,10,9,9,9,6,5,5,3,1,1,1,1}$ [96] |
| | [3,0,1,0,0,3,0,0,0,4] | [2,7,12,18,24,30,39,48,35,22,22] | $X_{10,10,9,9,9,7,4,4,4}$ [60] | $X_{10,10,9,9,9,7,4,4,4,1,1,1,1}$ [60] |
| | [3,3,0,0,0,1,0,0,1,5] | [1,5,12,19,26,33,41,49,35,22,22] | $X_{10,9,9,9,8,8,8,4,1}$ [80] | $X_{10,9,9,9,8,8,8,4,1,1,1,1,1}$ [80] |
| | [4,0,2,0,1,0,0,0,1,5] | [1,6,11,18,25,33,41,49,35,22,22] | $X_{10,9,9,9,9,7,7,5,1}$ [90] | $X_{10,9,9,9,9,7,7,5,1,1,1,1,1}$ [90] |
| | [4,1,0,1,0,1,0,1,0,4] | [1,6,12,18,25,32,40,48,35,22,22] | $X_{10,9,9,9,9,8,6,4,2}$ [162] | $X_{10,9,9,9,9,8,6,4,2,1,1,1,1}$ [162] |
| | [5,0,0,0,1,0,2,0,0,4] | [1,7,13,19,25,32,39,48,35,22,22] | $X_{10,9,9,9,9,9,5,3,3}$ [60] | $X_{10,9,9,9,9,9,5,3,3,1,1,1,1}$ [60] |
| | [1,2,3,0,0,0,0,0,0,6] | [2,5,10,18,26,34,42,50,36,22,22] | $X_{10,10,9,8,8,7,7,7}$ [32] | $X_{10,10,9,8,8,7,7,7,1,1,1,1,1,1}$ [32] |
| | [3,2,1,1,0,0,0,0,0,6] | [1,5,11,18,26,34,42,50,36,22,22] | $X_{10,9,9,9,8,8,7,6}$ [56] | $X_{10,9,9,9,8,8,7,6,1,1,1,1,1,1}$ [56] |
| | [7,0,0,0,0,0,1,0,0,6] | [0,7,14,21,28,35,42,50,36,22,22] | $X_{9,9,9,9,9,9,9,3}$ [28] | $X_{9,9,9,9,9,9,9,3,1,1,1,1,1,1}$ [28] |
| | [0,0,0,1,0,1,0,1,6,0] | [5,10,15,20,26,32,39,46,31,22,23] | $X_{10,10,10,10,10,6,4,2,1,1,1,1,1,1}$ [67] | $X_{10,10,10,10,10,6,4,2}$ [68] |
| | [1,0,1,0,1,0,0,0,7,1] | [4,9,14,20,26,33,40,47,31,22,23] | $X_{10,10,10,10,9,7,5,1,1,1,1,1,1,1}$ [90] | $X_{10,10,10,10,9,7,5,1}$ [90] |
| | [1,1,0,0,0,0,1,1,6,0] | [4,9,15,21,27,33,39,46,31,22,23] | $X_{10,10,10,10,9,8,3,2,1,1,1,1,1,1}$ [72] | $X_{10,10,10,10,9,8,3,2}$ [72] |
| | [0,0,2,0,1,1,0,0,5,1] | [4,8,12,18,24,31,39,47,32,22,23] | $X_{10,10,10,10,7,7,5,4,1,1,1,1,1}$ [96] | $X_{10,10,10,10,7,7,5,4,1}$ [96] |
| | [0,0,2,1,0,0,0,2,4,0] | [4,8,12,18,25,32,39,46,32,22,23] | $X_{10,10,10,10,7,7,6,2,2,1,1,1,1}$ [60] | $X_{10,10,10,10,7,7,6,2,2}$ [60] |
| | [0,1,0,1,1,0,1,1,4,0] | [4,8,13,18,24,31,38,46,32,22,23] | $X_{10,10,10,10,8,6,5,3,2,1,1,1,1}$ [162] | $X_{10,10,10,10,8,6,5,3,2}$ [162] |
| | [1,0,0,0,1,2,0,1,4,0] | [4,9,14,19,24,30,38,46,32,22,23] | $X_{10,10,10,10,9,5,4,4,2,1,1,1,1}$ [90] | $X_{10,10,10,10,9,5,4,4,2}$ [90] |
| | [1,0,0,1,0,0,3,0,4,0] | [4,9,14,19,25,31,37,46,32,22,23] | $X_{10,10,10,10,9,6,3,3,3,1,1,1,1}$ [64] | $X_{10,10,10,10,9,6,3,3,3}$ [64] |
| | [1,1,1,1,0,0,1,0,5,1] | [3,7,12,18,25,32,39,47,32,22,23] | $X_{10,10,10,9,8,7,6,3,1,1,1,1,1}$ [192] | $X_{10,10,10,9,8,7,6,3,1}$ [192] |
| | [1,2,0,0,0,2,0,0,5,1] | [3,7,13,19,25,31,39,47,32,22,23] | $X_{10,10,10,9,8,8,4,4,1,1,1,1,1}$ [80] | $X_{10,10,10,9,8,8,4,4,1}$ [80] |
| | [1,2,0,0,1,0,0,2,4,0] | [3,7,13,19,25,32,39,46,32,22,23] | $X_{10,10,10,9,8,8,5,2,2,1,1,1,1}$ [96] | $X_{10,10,10,9,8,8,5,2,2}$ [96] |
| | [2,0,0,1,1,1,0,0,5,1] | [3,8,13,18,24,31,39,47,32,22,23] | $X_{10,10,10,9,9,6,5,4,1,1,1,1,1}$ [128] | $X_{10,10,10,9,9,6,5,4,1}$ [128] |
| | [2,0,1,0,0,1,1,1,4,0] | [3,8,13,19,25,31,38,46,32,22,23] | $X_{10,10,10,9,9,7,4,3,2,1,1,1,1}$ [144] | $X_{10,10,10,9,9,7,4,3,2}$ [144] |
| | [3,1,0,1,0,0,0,1,5,1] | [2,7,13,19,26,33,40,47,32,22,23] | $X_{10,10,9,9,9,8,6,2,1,1,1,1,1}$ [120] | $X_{10,10,9,9,9,8,6,2,1}$ [120] |
| | [4,0,0,0,0,1,1,0,5,1] | [2,8,14,20,26,32,39,47,32,22,23] | $X_{10,10,9,9,9,9,4,3,1,1,1,1,1}$ [72] | $X_{10,10,9,9,9,9,4,3,1}$ [72] |
| | [0,0,0,0,0,1,4,0,2,0] | [5,10,15,20,25,30,36,46,33,22,23] | $X_{10,10,10,10,10,4,3,3,3,3,1,1}$ [28] | $X_{10,10,10,10,10,4,3,3,3,3}$ [28] |
| | [0,0,0,3,1,0,0,1,3,1] | [4,8,12,16,23,31,39,47,33,22,23] | $X_{10,10,10,10,6,6,6,5,2,1,1,1}$ [80] | $X_{10,10,10,10,6,6,6,5,2,1}$ [80] |
| | [0,0,1,1,1,1,0,2,2,0] | [4,8,12,17,23,30,38,46,33,22,23] | $X_{10,10,10,10,7,6,5,4,2,2,1,1}$ [144] | $X_{10,10,10,10,7,6,5,4,2,2}$ [144] |
| | [0,0,2,0,0,1,2,1,2,0] | [4,8,12,18,24,30,37,46,33,22,23] | $X_{10,10,10,10,7,7,4,3,3,2,1,1}$ [96] | $X_{10,10,10,10,7,7,4,3,3,2}$ [96] |

| | | | | |
|---|---|---|---|---|
| | [0,1,0,0,1,3,0,0,3,1] | [4,8,13,18,23,29,38,47,33,22,23] | $X_{10,10,10,10,8,5,4,4,4,1,1,1}$ [96] | $X_{10,10,10,10,8,5,4,4,4,1}$ [96] |
| | [0,1,0,0,2,0,2,1,2,0] | [4,8,13,18,23,30,37,46,33,22,23] | $X_{10,10,10,10,8,5,5,3,3,2,1,1}$ [108] | $X_{10,10,10,10,8,5,5,3,3,2}$ [108] |
| | [0,2,1,1,0,1,0,1,3,1] | [3,6,11,17,24,31,39,47,33,22,23] | $X_{10,10,10,8,8,7,6,4,2,1,1,1}$ [216] | $X_{10,10,10,8,8,7,6,4,2,1}$ [216] |
| | [0,3,0,0,1,0,2,0,3,1] | [3,6,12,18,24,31,38,47,33,22,23] | $X_{10,10,10,8,8,8,5,3,3,1,1,1}$ [108] | $X_{10,10,10,8,8,8,5,3,3,1}$ [108] |
| | [0,3,0,1,0,0,0,3,2,0] | [3,6,12,18,25,32,39,46,33,22,23] | $X_{10,10,10,8,8,8,6,2,2,2,1,1}$ [67] | $X_{10,10,10,8,8,8,6,2,2,2}$ [68] |
| | [1,0,0,0,0,3,1,1,2,0] | [4,9,14,19,24,29,37,46,33,22,23] | $X_{10,10,10,10,9,4,4,4,3,2,1,1}$ [72] | $X_{10,10,10,10,9,4,4,4,3,2}$ [72] |
| | [1,0,1,3,0,0,0,0,4,2] | [3,7,11,16,24,32,40,48,33,22,23] | $X_{10,10,10,9,7,6,6,6,1,1,1,1}$ [72] | $X_{10,10,10,9,7,6,6,6,1,1}$ [72] |
| | [1,0,2,0,2,0,0,1,3,1] | [3,7,11,17,23,31,39,47,33,22,23] | $X_{10,10,10,9,7,7,5,5,2,1,1,1}$ [144] | $X_{10,10,10,9,7,7,5,5,2,1}$ [144] |
| | [1,0,2,1,0,0,2,0,3,1] | [3,7,11,17,24,31,38,47,33,22,23] | $X_{10,10,10,9,7,7,6,3,3,1,1,1}$ [144] | $X_{10,10,10,9,7,7,6,3,3,1}$ [144] |
| | [1,0,3,0,0,0,0,3,2,0] | [3,7,11,18,25,32,39,46,33,22,23] | $X_{10,10,10,9,7,7,7,2,2,2,1,1}$ [54] | $X_{10,10,10,9,7,7,7,2,2,2}$ [54] |
| | [1,1,0,1,1,1,1,0,3,1] | [3,7,12,17,23,30,38,47,33,22,23] | $X_{10,10,10,9,8,6,5,4,3,1,1,1}$ [288] | $X_{10,10,10,9,8,6,5,4,3,1}$ [288] |
| | [1,1,0,2,0,0,1,2,2,0] | [3,7,12,17,24,31,38,46,33,22,23] | $X_{10,10,10,9,8,6,6,3,2,2,1,1}$ [144] | $X_{10,10,10,9,8,6,6,3,2,2}$ [144] |
| | [1,1,1,0,0,2,0,2,2,0] | [3,7,12,18,24,30,38,46,33,22,23] | $X_{10,10,10,9,8,7,4,4,2,2,1,1}$ [144] | $X_{10,10,10,9,8,7,4,4,2,2}$ [144] |
| | [1,2,0,0,0,0,3,1,2,0] | [3,7,13,19,25,31,37,46,33,22,23] | $X_{10,10,10,9,8,8,3,3,3,2,1,1}$ [72] | $X_{10,10,10,9,8,8,3,3,3,2}$ [72] |
| | [1,4,0,0,0,0,1,0,4,2] | [2,5,12,19,26,33,40,48,33,22,23] | $X_{10,10,9,8,8,8,8,3,1,1,1,1}$ [72] | $X_{10,10,9,8,8,8,8,3,1,1}$ [72] |
| | [2,0,0,0,2,1,0,2,2,0] | [3,8,13,18,23,30,38,46,33,22,23] | $X_{10,10,10,9,9,5,5,4,2,2,1,1}$ [90] | $X_{10,10,10,9,9,5,5,4,2,2}$ [90] |
| | [2,0,0,1,0,1,2,1,2,0] | [3,8,13,18,24,30,37,46,33,22,23] | $X_{10,10,10,9,9,6,4,3,3,2,1,1}$ [144] | $X_{10,10,10,9,9,6,4,3,3,2}$ [144] |
| | [2,1,1,1,1,0,0,0,4,2] | [2,6,11,17,24,32,40,48,33,22,23] | $X_{10,10,9,9,8,7,6,5,1,1,1,1}$ [160] | $X_{10,10,9,9,8,7,6,5,1,1}$ [160] |
| | [2,1,2,0,0,0,1,1,3,1] | [2,6,11,18,25,32,39,47,33,22,23] | $X_{10,10,9,9,8,7,7,3,2,1,1,1}$ [160] | $X_{10,10,9,9,8,7,7,3,2,1}$ [160] |
| | [2,2,0,0,1,1,0,1,3,1] | [2,6,12,18,24,31,39,47,33,22,23] | $X_{10,10,9,9,8,8,5,4,2,1,1,1}$ [192] | $X_{10,10,9,9,8,8,5,4,2,1}$ [192] |
| | [3,0,0,2,0,1,0,1,3,1] | [2,7,12,17,24,31,39,47,33,22,23] | $X_{10,10,9,9,9,6,6,4,2,1,1,1}$ [144] | $X_{10,10,9,9,9,6,6,4,2,1}$ [144] |
| | [3,0,1,0,1,0,2,0,3,1] | [2,7,12,18,24,31,38,47,33,22,23] | $X_{10,10,9,9,9,7,5,3,3,1,1,1}$ [162] | $X_{10,10,9,9,9,7,5,3,3,1}$ [162] |
| | [3,0,1,1,0,0,0,3,2,0] | [2,7,12,18,25,32,39,46,33,22,23] | $X_{10,10,9,9,9,7,6,2,2,2,1,1}$ [90] | $X_{10,10,9,9,9,7,6,2,2,2}$ [90] |
| | [3,1,0,0,0,1,1,2,2,0] | [2,7,13,19,25,31,38,46,33,22,23] | $X_{10,10,9,9,9,8,4,3,2,2,1,1}$ [120] | $X_{10,10,9,9,9,8,4,3,2,2}$ [120] |
| | [4,1,1,0,0,0,1,0,4,2] | [1,6,12,19,26,33,40,48,33,22,23] | $X_{10,9,9,9,9,8,7,3,1,1,1,1}$ [120] | $X_{10,9,9,9,9,8,7,3,1,1}$ [120] |
| | [5,0,0,0,1,1,0,0,4,2] | [1,7,13,19,25,32,40,48,33,22,23] | $X_{10,9,9,9,9,9,5,4,1,1,1,1}$ [80] | $X_{10,9,9,9,9,9,5,4,1,1}$ [80] |
| | [5,0,0,1,0,0,0,2,3,1] | [1,7,13,19,26,33,40,47,33,22,23] | $X_{10,9,9,9,9,9,6,2,2,1,1,1}$ [80] | $X_{10,9,9,9,9,9,6,2,2,1}$ [80] |
| | [0,0,0,2,1,2,1,0,0,2] | [4,8,12,16,22,29,38,48,35,22,23] | $X_{10,10,10,10,6,6,5,4,4,3}$ [80] | $X_{10,10,10,10,6,6,5,4,4,3,1,1}$ [80] |
| | [0,0,4,1,0,0,1,0,1,3] | [3,6,9,16,24,32,40,49,35,22,23] | $X_{10,10,10,7,7,7,7,6,3,1}$ [96] | $X_{10,10,10,7,7,7,7,6,3,1,1,1}$ [96] |
| | [0,1,1,3,0,1,0,0,1,3] | [3,6,10,15,23,31,40,49,35,22,23] | $X_{10,10,10,8,7,6,6,6,4,1}$ [144] | $X_{10,10,10,8,7,6,6,6,4,1,1,1}$ [144] |
| | [0,1,2,0,3,0,0,0,1,3] | [3,6,10,16,22,31,40,49,35,22,23] | $X_{10,10,10,8,7,7,5,5,5,1}$ [90] | $X_{10,10,10,8,7,7,5,5,5,1,1,1}$ [90] |
| | [0,1,2,1,0,2,0,1,0,2] | [3,6,10,16,23,30,39,48,35,22,23] | $X_{10,10,10,8,7,7,6,4,4,2}$ [162] | $X_{10,10,10,8,7,7,6,4,4,2,1,1}$ [162] |
| | [0,1,3,0,0,0,3,0,0,2] | [3,6,10,17,24,31,38,48,35,22,23] | $X_{10,10,10,8,7,7,7,3,3,3}$ [60] | $X_{10,10,10,8,7,7,7,3,3,3,1,1}$ [60] |
| | [0,2,0,1,2,1,0,1,0,2] | [3,6,11,16,22,30,39,48,35,22,23] | $X_{10,10,10,8,8,6,5,5,4,2}$ [162] | $X_{10,10,10,8,8,6,5,5,4,2,1,1}$ [162] |
| | [0,2,0,2,0,1,2,0,0,2] | [3,6,11,16,23,30,38,48,35,22,23] | $X_{10,10,10,8,8,6,6,4,3,3}$ [108] | $X_{10,10,10,8,8,6,6,4,3,3,1,1}$ [108] |
| | [0,4,1,1,0,0,0,1,1,3] | [2,4,10,17,25,33,41,49,35,22,23] | $X_{10,10,8,8,8,8,7,6,2,1}$ [120] | $X_{10,10,8,8,8,8,7,6,2,1,1,1}$ [120] |
| | [0,5,0,0,0,1,1,0,1,3] | [2,4,11,18,25,32,40,49,35,22,23] | $X_{10,10,8,8,8,8,8,4,3,1}$ [90] | $X_{10,10,8,8,8,8,8,4,3,1,1,1}$ [90] |
| | [1,0,0,3,2,0,0,0,1,3] | [3,7,11,15,22,31,40,49,35,22,23] | $X_{10,10,10,9,6,6,6,5,5,1}$ [80] | $X_{10,10,10,9,6,6,6,5,5,1,1,1}$ [80] |
| | [1,0,0,4,0,0,1,1,0,2] | [3,7,11,15,23,31,39,48,35,22,23] | $X_{10,10,10,9,6,6,6,6,3,2}$ [96] | $X_{10,10,10,9,6,6,6,6,3,2,1,1}$ [96] |
| | [1,0,1,1,2,0,2,0,0,2] | [3,7,11,16,22,30,38,48,35,22,23] | $X_{10,10,10,9,7,6,5,5,3,3}$ [144] | $X_{10,10,10,9,7,6,5,5,3,3,1,1}$ [144] |
| | [1,0,2,0,0,3,1,0,0,2] | [3,7,11,17,23,29,38,48,35,22,23] | $X_{10,10,10,9,7,7,4,4,4,3}$ [96] | $X_{10,10,10,9,7,7,4,4,4,3,1,1}$ [96] |
| | [1,1,0,0,2,2,1,0,0,2] | [3,7,12,17,22,29,38,48,35,22,23] | $X_{10,10,10,9,8,5,5,4,4,3}$ [128] | $X_{10,10,10,9,8,5,5,4,4,3,1,1}$ [128] |
| | [1,1,4,0,0,0,0,1,1,3] | [2,5,9,17,25,33,41,49,35,22,23] | $X_{10,10,9,8,7,7,7,7,2,1}$ [96] | $X_{10,10,9,8,7,7,7,7,2,1,1,1}$ [96] |
| | [1,2,1,1,1,1,0,0,1,3] | [2,5,10,16,23,31,40,49,35,22,23] | $X_{10,10,9,8,8,7,6,5,4,1}$ [256] | $X_{10,10,9,8,8,7,6,5,4,1,1,1}$ [256] |
| | [1,2,1,2,0,0,0,2,0,2] | [2,5,10,16,24,32,40,48,35,22,23] | $X_{10,10,9,8,8,7,6,6,2,2}$ [120] | $X_{10,10,9,8,8,7,6,6,2,2,1,1}$ [120] |
| | [1,2,2,0,0,1,1,1,0,2] | [2,5,10,17,24,31,39,48,35,22,23] | $X_{10,10,9,8,8,7,7,4,3,2}$ [192] | $X_{10,10,9,8,8,7,7,4,3,2,1,1}$ [192] |
| | [1,3,0,0,2,0,1,1,0,2] | [2,5,11,17,23,31,39,48,35,22,23] | $X_{10,10,9,8,8,8,5,5,3,2}$ [144] | $X_{10,10,9,8,8,8,5,5,3,2,1,1}$ [144] |
| | [2,0,2,1,1,0,1,1,0,2] | [2,6,10,16,23,31,39,48,35,22,23] | $X_{10,10,9,9,7,7,6,5,3,2}$ [216] | $X_{10,10,9,9,7,7,6,5,3,2,1,1}$ [216] |
| | [2,1,0,1,3,0,0,0,1,3] | [2,6,11,16,22,31,40,49,35,22,23] | $X_{10,10,9,9,8,6,5,5,5,1}$ [120] | $X_{10,10,9,9,8,6,5,5,5,1,1,1}$ [120] |
| | [2,1,0,2,0,2,0,1,0,2] | [2,6,11,16,23,30,39,48,35,22,23] | $X_{10,10,9,9,8,6,6,4,4,2}$ [162] | $X_{10,10,9,9,8,6,6,4,4,2,1,1}$ [162] |
| | [2,1,1,0,1,1,2,0,0,2] | [2,6,11,17,23,30,38,48,35,22,23] | $X_{10,10,9,9,8,7,5,4,3,3}$ [192] | $X_{10,10,9,9,8,7,5,4,3,3,1,1}$ [192] |
| | [2,3,2,0,0,0,0,0,2,4] | [1,4,10,18,26,34,42,50,35,22,23] | $X_{10,9,9,8,8,8,7,7,1,1}$ [56] | $X_{10,9,9,8,8,8,7,7,1,1,1,1}$ [56] |
| | [2,4,0,0,1,0,0,1,1,3] | [1,4,11,18,25,33,41,49,35,22,23] | $X_{10,9,9,8,8,8,8,5,2,1}$ [128] | $X_{10,9,9,8,8,8,8,5,2,1,1,1}$ [128] |
| | [3,0,0,0,3,1,0,1,0,2] | [2,7,12,17,22,30,39,48,35,22,23] | $X_{10,10,9,9,9,5,5,5,4,2}$ [90] | $X_{10,10,9,9,9,5,5,5,4,2,1,1}$ [90] |
| | [3,1,2,0,1,0,1,0,1,3] | [1,5,10,17,24,32,40,49,35,22,23] | $X_{10,9,9,9,8,7,7,5,3,1}$ [216] | $X_{10,9,9,9,8,7,7,5,3,1,1,1}$ [216] |
| | [3,2,0,1,0,2,0,0,1,3] | [1,5,11,17,24,31,40,49,35,22,23] | $X_{10,9,9,9,8,8,6,4,4,1}$ [144] | $X_{10,9,9,9,8,8,6,4,4,1,1,1}$ [144] |
| | [3,2,0,1,1,0,0,2,0,2] | [1,5,11,17,24,32,40,48,35,22,23] | $X_{10,9,9,9,8,8,6,5,2,2}$ [144] | $X_{10,9,9,9,8,8,6,5,2,2,1,1}$ [144] |
| | [3,2,1,0,0,0,2,1,0,2] | [1,5,11,18,25,32,39,48,35,22,23] | $X_{10,9,9,9,8,8,7,3,3,2}$ [120] | $X_{10,9,9,9,8,8,7,3,3,2,1,1}$ [120] |
| | [4,0,0,3,0,0,1,0,1,3] | [1,6,11,16,24,32,40,49,35,22,23] | $X_{10,9,9,9,9,6,6,6,3,1}$ [96] | $X_{10,9,9,9,9,6,6,6,3,1,1,1}$ [96] |
| | [4,0,1,0,2,1,0,0,1,3] | [1,6,11,17,23,31,40,49,35,22,23] | $X_{10,9,9,9,9,7,5,5,4,1}$ [144] | $X_{10,9,9,9,9,7,5,5,4,1,1,1}$ [144] |
| | [4,0,1,1,0,1,1,1,0,2] | [1,6,11,17,24,31,39,48,35,22,23] | $X_{10,9,9,9,9,7,6,4,3,2}$ [216] | $X_{10,9,9,9,9,7,6,4,3,2,1,1}$ [216] |
| | [5,0,0,0,0,1,3,0,0,2] | [1,7,13,19,25,31,38,48,35,22,23] | $X_{10,9,9,9,9,9,4,3,3,3}$ [48] | $X_{10,9,9,9,9,9,4,3,3,3,1,1}$ [48] |
| | [5,1,1,1,0,0,0,0,2,4] | [0,5,11,18,26,34,42,50,35,22,23] | $X_{9,9,9,9,9,8,7,6,1,1}$ [96] | $X_{9,9,9,9,9,8,7,6,1,1,1,1}$ [96] |
| | [5,2,0,0,0,1,0,1,1,3] | [0,5,12,19,26,33,41,49,35,22,23] | $X_{9,9,9,9,9,8,8,4,2,1}$ [120] | $X_{9,9,9,9,9,8,8,4,2,1,1,1}$ [120] |
| | [6,0,0,1,1,0,0,1,1,3] | [0,6,12,18,25,33,41,49,35,22,23] | $X_{9,9,9,9,9,9,6,5,2,1}$ [128] | $X_{9,9,9,9,9,9,6,5,2,1,1,1}$ [128] |
| | [6,0,1,0,0,0,2,0,1,3] | [0,6,12,19,26,33,40,49,35,22,23] | $X_{9,9,9,9,9,9,7,3,3,1}$ [90] | $X_{9,9,9,9,9,9,7,3,3,1,1,1}$ [90] |
| | [6,1,0,0,0,0,0,3,0,2] | [0,6,13,20,27,34,41,48,35,22,23] | $X_{9,9,9,9,9,9,8,2,2,2}$ [42] | $X_{9,9,9,9,9,9,8,2,2,2,1,1}$ [42] |
| | [0,4,1,0,1,1,0,0,0,4] | [2,4,10,17,24,32,41,50,36,22,23] | $X_{10,10,8,8,8,8,7,5,4}$ [90] | $X_{10,10,8,8,8,8,7,5,4,1,1,1,1}$ [90] |
| | [1,1,3,1,0,1,0,0,0,4] | [2,5,9,16,24,32,41,50,36,22,23] | $X_{10,10,9,8,7,7,7,6,4}$ [120] | $X_{10,10,9,8,7,7,7,6,4,1,1,1,1}$ [120] |
| | [2,0,1,3,1,0,0,0,0,4] | [2,6,10,15,23,32,41,50,36,22,23] | $X_{10,10,9,9,7,6,6,6,5}$ [72] | $X_{10,10,9,9,7,6,6,6,5,1,1,1,1}$ [72] |
| | [2,3,1,1,0,0,1,0,0,4] | [1,4,10,17,25,33,41,50,36,22,23] | $X_{10,9,9,8,8,8,7,6,3}$ [128] | $X_{10,9,9,8,8,8,7,6,3,1,1,1,1}$ [128] |

| | | | | |
|---|---|---|---|---|
| | [3,1,1,2,0,1,0,0,0,4] | [1,5,10,16,24,32,41,50,36,22,23] | $X_{10,9,9,9,8,7,6,6,4}$ [120] | $X_{10,9,9,9,8,7,6,6,4,1,1,1,1}$ [120] |
| | [3,2,0,0,3,0,0,0,0,4] | [1,5,11,17,23,32,41,50,36,22,23] | $X_{10,9,9,9,8,8,5,5,5}$ [48] | $X_{10,9,9,9,8,8,5,5,5,1,1,1,1}$ [48] |
| | [4,3,1,0,0,0,0,0,1,5] | [0,4,11,19,27,35,43,51,36,22,23] | $X_{9,9,9,9,8,8,8,7,1}$ [56] | $X_{9,9,9,9,8,8,8,7,1,1,1,1,1}$ [56] |
| | [5,1,1,0,1,0,1,0,0,4] | [0,5,11,18,25,33,41,50,36,22,23] | $X_{9,9,9,9,9,8,7,5,3}$ [144] | $X_{9,9,9,9,9,8,7,5,3,1,1,1,1}$ [144] |
| | [6,0,0,1,0,2,0,0,0,4] | [0,6,12,18,25,32,41,50,36,22,23] | $X_{9,9,9,9,9,9,6,4,4}$ [60] | $X_{9,9,9,9,9,9,6,4,4,1,1,1,1}$ [60] |
| | [0,2,0,1,0,0,0,0,8,0] | [4,8,14,20,27,34,41,48,31,22,24] | $X_{10,10,10,10,8,8,6,1,1,1,1,1,1,1,1}$ [31] | $X_{10,10,10,10,8,8,6}$ [32] |
| | [0,0,1,2,1,0,0,0,6,0] | [4,8,12,17,24,32,40,48,32,22,24] | $X_{10,10,10,10,7,6,6,5,1,1,1,1,1,1}$ [48] | $X_{10,10,10,10,7,6,6,5}$ [48] |
| | [0,3,1,0,0,0,1,0,6,0] | [3,6,12,19,26,33,40,48,32,22,24] | $X_{10,10,10,8,8,8,7,3,1,1,1,1,1,1}$ [60] | $X_{10,10,10,8,8,8,7,3}$ [60] |
| | [1,1,1,0,2,0,0,0,6,0] | [3,7,12,18,24,32,40,48,32,22,24] | $X_{10,10,10,9,8,7,5,5,1,1,1,1,1,1}$ [72] | $X_{10,10,10,9,8,7,5,5}$ [72] |
| | [2,3,0,0,0,0,0,1,6,0] | [2,6,13,20,27,34,41,48,32,22,24] | $X_{10,10,9,9,8,8,8,2,1,1,1,1,1,1}$ [42] | $X_{10,10,9,9,8,8,8,2}$ [42] |
| | [3,0,2,0,0,0,1,0,6,0] | [2,7,12,19,26,33,40,48,32,22,24] | $X_{10,10,9,9,9,7,7,3,1,1,1,1,1,1}$ [60] | $X_{10,10,9,9,9,7,7,3}$ [60] |
| | [3,1,0,0,1,1,0,0,6,0] | [2,7,13,19,25,32,40,48,32,22,24] | $X_{10,10,9,9,9,8,5,4,1,1,1,1,1,1}$ [80] | $X_{10,10,9,9,9,8,5,4}$ [80] |
| | [0,0,0,3,0,2,0,0,4,0] | [4,8,12,16,23,30,39,48,33,22,24] | $X_{10,10,10,10,6,6,6,4,4,1,1,1,1}$ [37] | $X_{10,10,10,10,6,6,6,4,4}$ [38] |
| | [0,0,1,0,3,1,0,0,4,0] | [4,8,12,17,22,30,39,48,33,22,24] | $X_{10,10,10,10,7,5,5,5,4,1,1,1,1}$ [60] | $X_{10,10,10,10,7,5,5,5,4}$ [60] |
| | [0,2,0,3,0,0,0,1,4,0] | [3,6,11,16,24,32,40,48,33,22,24] | $X_{10,10,10,8,8,6,6,6,2,1,1,1,1}$ [67] | $X_{10,10,10,8,8,6,6,6,2}$ [68] |
| | [0,2,1,0,2,0,1,0,4,0] | [3,6,11,17,23,31,39,48,33,22,24] | $X_{10,10,10,8,8,7,5,5,3,1,1,1,1}$ [108] | $X_{10,10,10,8,8,7,5,5,3}$ [108] |
| | [0,3,0,0,0,3,0,0,4,0] | [3,6,12,18,24,30,39,48,33,22,24] | $X_{10,10,10,8,8,8,4,4,4,1,1,1,1}$ [37] | $X_{10,10,10,8,8,8,4,4,4}$ [38] |
| | [1,0,1,2,1,0,1,0,4,0] | [3,7,11,16,23,31,39,48,33,22,24] | $X_{10,10,10,9,7,6,6,5,3,1,1,1,1}$ [144] | $X_{10,10,10,9,7,6,6,5,3}$ [144] |
| | [1,0,2,0,1,2,0,0,4,0] | [3,7,11,17,23,30,39,48,33,22,24] | $X_{10,10,10,9,7,7,5,4,4,1,1,1,1}$ [90] | $X_{10,10,10,9,7,7,5,4,4}$ [90] |
| | [1,3,0,2,0,0,0,0,5,1] | [2,5,11,17,25,33,41,49,33,22,24] | $X_{10,10,9,8,8,8,6,6,1,1,1,1,1}$ [72] | $X_{10,10,9,8,8,8,6,6,1}$ [72] |
| | [1,3,1,0,0,1,0,1,4,0] | [2,5,11,18,25,32,40,48,33,22,24] | $X_{10,10,9,8,8,8,7,4,2,1,1,1,1}$ [144] | $X_{10,10,9,8,8,8,7,4,2}$ [144] |
| | [2,1,1,1,0,1,1,0,4,0] | [2,6,11,17,24,31,39,48,33,22,24] | $X_{10,10,9,9,8,7,6,4,3,1,1,1,1}$ [192] | $X_{10,10,9,9,8,7,6,4,3}$ [192] |
| | [3,0,0,1,2,0,1,0,4,0] | [2,7,12,17,23,31,39,48,33,22,24] | $X_{10,10,9,9,9,6,5,5,3,1,1,1,1}$ [96] | $X_{10,10,9,9,9,6,5,5,3}$ [96] |
| | [3,3,0,0,0,1,0,0,5,1] | [1,5,12,19,26,33,41,49,33,22,24] | $X_{10,9,9,9,8,8,8,4,1,1,1,1,1}$ [80] | $X_{10,9,9,9,8,8,8,4,1}$ [80] |
| | [4,0,2,0,1,0,0,0,5,1] | [1,6,11,18,25,33,41,49,33,22,24] | $X_{10,9,9,9,9,7,7,5,1,1,1,1,1}$ [90] | $X_{10,9,9,9,9,7,7,5,1}$ [90] |
| | [4,1,0,1,0,1,0,1,4,0] | [1,6,12,18,25,32,40,48,33,22,24] | $X_{10,9,9,9,9,8,6,4,2,1,1,1,1}$ [162] | $X_{10,9,9,9,9,8,6,4,2}$ [162] |
| | [5,0,0,0,1,0,2,0,4,0] | [1,7,13,19,25,32,39,48,33,22,24] | $X_{10,9,9,9,9,9,5,3,3,1,1,1,1}$ [60] | $X_{10,9,9,9,9,9,5,3,3}$ [60] |
| | [0,0,0,2,1,2,1,0,2,0] | [4,8,12,16,22,29,38,48,34,22,24] | $X_{10,10,10,10,6,6,5,4,4,3,1,1}$ [80] | $X_{10,10,10,10,6,6,5,4,4,3}$ [80] |
| | [0,1,1,3,0,1,0,0,3,1] | [3,6,10,15,23,31,40,49,34,22,24] | $X_{10,10,10,8,7,6,6,6,4,1,1,1}$ [144] | $X_{10,10,10,8,7,6,6,6,4,1}$ [144] |
| | [0,1,2,0,3,0,0,0,3,1] | [3,6,10,16,22,31,40,49,34,22,24] | $X_{10,10,10,8,7,7,5,5,5,1,1,1}$ [90] | $X_{10,10,10,8,7,7,5,5,5,1}$ [90] |
| | [0,1,2,1,0,2,0,1,2,0] | [3,6,10,16,23,30,39,48,34,22,24] | $X_{10,10,10,8,7,7,6,4,4,2,1,1}$ [162] | $X_{10,10,10,8,7,7,6,4,4,2}$ [162] |
| | [0,1,3,0,0,0,3,0,2,0] | [3,6,10,17,24,31,38,48,34,22,24] | $X_{10,10,10,8,7,7,7,3,3,3,1,1}$ [60] | $X_{10,10,10,8,7,7,7,3,3,3}$ [60] |
| | [0,2,0,1,2,1,0,1,2,0] | [3,6,11,16,22,30,39,48,34,22,24] | $X_{10,10,10,8,8,6,5,5,4,2,1,1}$ [162] | $X_{10,10,10,8,8,6,5,5,4,2}$ [162] |
| | [0,2,0,2,0,1,2,0,2,0] | [3,6,11,16,23,30,38,48,34,22,24] | $X_{10,10,10,8,8,6,6,4,3,3,1,1}$ [108] | $X_{10,10,10,8,8,6,6,4,3,3}$ [108] |
| | [0,4,1,1,0,0,0,1,3,1] | [2,4,10,17,25,33,41,49,34,22,24] | $X_{10,10,8,8,8,8,7,6,2,1,1,1}$ [120] | $X_{10,10,8,8,8,8,7,6,2,1}$ [120] |
| | [0,5,0,0,0,1,1,0,3,1] | [2,4,11,18,25,32,40,49,34,22,24] | $X_{10,10,8,8,8,8,8,4,3,1,1,1}$ [90] | $X_{10,10,8,8,8,8,8,4,3,1}$ [90] |
| | [1,0,0,3,2,0,0,0,3,1] | [3,7,11,15,22,31,40,49,34,22,24] | $X_{10,10,10,9,6,6,6,5,5,1,1,1}$ [80] | $X_{10,10,10,9,6,6,6,5,5,1}$ [80] |
| | [1,0,0,4,0,0,1,1,2,0] | [3,7,11,15,23,31,39,48,34,22,24] | $X_{10,10,10,9,6,6,6,6,3,2,1,1}$ [96] | $X_{10,10,10,9,6,6,6,6,3,2}$ [96] |
| | [1,0,1,1,2,0,2,0,2,0] | [3,7,11,16,22,30,38,48,34,22,24] | $X_{10,10,10,9,7,6,5,5,3,3,1,1}$ [144] | $X_{10,10,10,9,7,6,5,5,3,3}$ [144] |
| | [1,0,2,0,0,3,1,0,2,0] | [3,7,11,17,23,29,38,48,34,22,24] | $X_{10,10,10,9,7,7,4,4,4,3,1,1}$ [96] | $X_{10,10,10,9,7,7,4,4,4,3}$ [96] |
| | [1,1,0,0,2,2,1,0,2,0] | [3,7,12,17,22,29,38,48,34,22,24] | $X_{10,10,10,9,8,5,5,4,4,3,1,1}$ [128] | $X_{10,10,10,9,8,5,5,4,4,3}$ [128] |
| | [1,2,1,1,1,1,0,0,3,1] | [2,5,10,16,23,31,40,49,34,22,24] | $X_{10,10,9,8,8,7,6,5,4,1,1,1}$ [256] | $X_{10,10,9,8,8,7,6,5,4,1}$ [256] |
| | [1,2,1,2,0,0,0,2,2,0] | [2,5,10,16,24,32,40,48,34,22,24] | $X_{10,10,9,8,8,7,6,6,2,2,1,1}$ [120] | $X_{10,10,9,8,8,7,6,6,2,2}$ [120] |
| | [1,2,2,0,0,1,1,1,2,0] | [2,5,10,17,24,31,39,48,34,22,24] | $X_{10,10,9,8,8,7,7,4,3,2,1,1}$ [192] | $X_{10,10,9,8,8,7,7,4,3,2}$ [192] |
| | [1,3,0,0,2,0,1,1,2,0] | [2,5,11,17,23,31,39,48,34,22,24] | $X_{10,10,9,8,8,8,5,5,3,2,1,1}$ [144] | $X_{10,10,9,8,8,8,5,5,3,2}$ [144] |
| | [2,0,2,1,1,0,1,1,2,0] | [2,6,10,16,23,31,39,48,34,22,24] | $X_{10,10,9,9,7,7,6,5,3,2,1,1}$ [216] | $X_{10,10,9,9,7,7,6,5,3,2}$ [216] |
| | [2,1,0,1,3,0,0,0,3,1] | [2,6,11,16,22,31,40,49,34,22,24] | $X_{10,10,9,9,8,6,5,5,5,1,1,1}$ [120] | $X_{10,10,9,9,8,6,5,5,5,1}$ [120] |
| | [2,1,0,2,0,2,0,1,2,0] | [2,6,11,16,23,30,39,48,34,22,24] | $X_{10,10,9,9,8,6,6,4,4,2,1,1}$ [162] | $X_{10,10,9,9,8,6,6,4,4,2}$ [162] |
| | [2,1,1,0,1,1,2,0,2,0] | [2,6,11,17,23,30,38,48,34,22,24] | $X_{10,10,9,9,8,7,5,4,3,3,1,1}$ [192] | $X_{10,10,9,9,8,7,5,4,3,3}$ [192] |
| | [2,3,2,0,0,0,0,0,4,2] | [1,4,10,18,26,34,42,50,34,22,24] | $X_{10,9,9,8,8,8,7,7,1,1,1,1}$ [56] | $X_{10,9,9,8,8,8,7,7,1,1}$ [56] |
| | [2,4,0,0,1,0,0,1,3,1] | [1,4,11,18,25,33,41,49,34,22,24] | $X_{10,9,9,8,8,8,8,5,2,1,1,1}$ [128] | $X_{10,9,9,8,8,8,8,5,2,1}$ [128] |
| | [3,0,0,0,3,1,0,1,2,0] | [2,7,12,17,22,30,39,48,34,22,24] | $X_{10,10,9,9,9,5,5,5,4,2,1,1}$ [90] | $X_{10,10,9,9,9,5,5,5,4,2}$ [90] |
| | [3,1,2,0,1,0,1,0,3,1] | [1,5,10,17,24,32,40,49,34,22,24] | $X_{10,9,9,9,8,7,7,5,3,1,1,1}$ [216] | $X_{10,9,9,9,8,7,7,5,3,1}$ [216] |
| | [3,2,0,1,0,2,0,0,3,1] | [1,5,11,17,24,31,40,49,34,22,24] | $X_{10,9,9,9,8,8,6,4,4,1,1,1}$ [144] | $X_{10,9,9,9,8,8,6,4,4,1}$ [144] |
| | [3,2,0,1,1,0,0,2,2,0] | [1,5,11,17,24,32,40,48,34,22,24] | $X_{10,9,9,9,8,8,6,5,2,2,1,1}$ [144] | $X_{10,9,9,9,8,8,6,5,2,2}$ [144] |
| | [3,2,1,0,0,0,2,1,2,0] | [1,5,11,18,25,32,39,48,34,22,24] | $X_{10,9,9,9,8,8,7,3,3,2,1,1}$ [120] | $X_{10,9,9,9,8,8,7,3,3,2}$ [120] |
| | [4,0,0,3,0,0,1,0,3,1] | [1,6,11,16,24,32,40,49,34,22,24] | $X_{10,9,9,9,9,6,6,6,3,1,1,1}$ [96] | $X_{10,9,9,9,9,6,6,6,3,1}$ [96] |
| | [4,0,1,0,2,1,0,0,3,1] | [1,6,11,17,23,31,40,49,34,22,24] | $X_{10,9,9,9,9,7,5,5,4,1,1,1}$ [144] | $X_{10,9,9,9,9,7,5,5,4,1}$ [144] |
| | [4,0,1,1,0,1,1,1,2,0] | [1,6,11,17,24,31,39,48,34,22,24] | $X_{10,9,9,9,9,7,6,4,3,2,1,1}$ [216] | $X_{10,9,9,9,9,7,6,4,3,2}$ [216] |
| | [5,0,0,0,0,1,3,0,2,0] | [1,7,13,19,25,31,38,48,34,22,24] | $X_{10,9,9,9,9,9,4,3,3,3,1,1}$ [48] | $X_{10,9,9,9,9,9,4,3,3,3}$ [48] |
| | [5,1,1,1,0,0,0,0,4,2] | [0,5,11,18,26,34,42,50,34,22,24] | $X_{9,9,9,9,9,8,7,6,1,1,1,1}$ [96] | $X_{9,9,9,9,9,8,7,6,1,1}$ [96] |
| | [5,2,0,0,0,1,0,1,3,1] | [0,5,12,19,26,33,41,49,34,22,24] | $X_{9,9,9,9,9,8,8,4,2,1,1,1}$ [120] | $X_{9,9,9,9,9,8,8,4,2,1}$ [120] |
| | [6,0,0,1,1,0,0,1,3,1] | [0,6,12,18,25,33,41,49,34,22,24] | $X_{9,9,9,9,9,9,6,5,2,1,1,1}$ [128] | $X_{9,9,9,9,9,9,6,5,2,1}$ [128] |
| | [6,0,1,0,0,0,2,0,3,1] | [0,6,12,19,26,33,40,49,34,22,24] | $X_{9,9,9,9,9,9,7,3,3,1,1,1}$ [90] | $X_{9,9,9,9,9,9,7,3,3,1}$ [90] |
| | [6,1,0,0,0,0,0,3,2,0] | [0,6,13,20,27,34,41,48,34,22,24] | $X_{9,9,9,9,9,9,8,2,2,2,1,1}$ [42] | $X_{9,9,9,9,9,9,8,2,2,2}$ [42] |
| | [0,0,3,1,2,0,1,0,0,2] | [3,6,9,15,22,31,40,50,36,22,24] | $X_{10,10,10,7,7,7,6,5,5,3}$ [96] | $X_{10,10,10,7,7,7,6,5,5,3,1,1}$ [96] |
| | [0,0,4,0,0,3,0,0,0,2] | [3,6,9,16,23,30,40,50,36,22,24] | $X_{10,10,10,7,7,7,7,4,4,4}$ [40] | $X_{10,10,10,7,7,7,7,4,4,4,1,1}$ [40] |
| | [0,1,0,5,0,0,0,1,0,2] | [3,6,10,14,23,32,41,50,36,22,24] | $X_{10,10,10,8,6,6,6,6,6,2}$ [68] | $X_{10,10,10,8,6,6,6,6,6,2,1,1}$ [67] |
| | [0,3,2,0,2,0,0,1,0,2] | [2,4,9,16,23,32,41,50,36,22,24] | $X_{10,10,8,8,8,7,7,5,5,2}$ [108] | $X_{10,10,8,8,8,7,7,5,5,2,1,1}$ [108] |
| | [0,3,2,1,0,0,2,0,0,2] | [2,4,9,16,24,32,40,50,36,22,24] | $X_{10,10,8,8,8,7,7,6,3,3}$ [96] | $X_{10,10,8,8,8,7,7,6,3,3,1,1}$ [96] |
| | [0,4,0,1,1,1,1,0,0,2] | [2,4,10,16,23,31,40,50,36,22,24] | $X_{10,10,8,8,8,8,6,5,4,3}$ [144] | $X_{10,10,8,8,8,8,6,5,4,3,1,1}$ [144] |

| | | | | |
|---|---|---|---|---|
| | [1,0,5,0,1,0,0,0,1,3] | [2,5,8,16,24,33,42,51,36,22,24] | $X_{10,10,9,7,7,7,7,7,5,1}$ [90] | $X_{10,10,9,7,7,7,7,7,5,1,1,1}$ [90] |
| | [1,1,2,2,0,1,1,0,0,2] | [2,5,9,15,23,31,40,50,36,22,24] | $X_{10,10,9,8,7,7,6,6,4,3}$ [192] | $X_{10,10,9,8,7,7,6,6,4,3,1,1}$ [192] |
| | [1,2,0,2,2,0,1,0,0,2] | [2,5,10,15,22,31,40,50,36,22,24] | $X_{10,10,9,8,8,6,6,5,5,3}$ [144] | $X_{10,10,9,8,8,6,6,5,5,3,1,1}$ [144] |
| | [1,2,1,0,2,2,0,0,0,2] | [2,5,10,16,22,30,40,50,36,22,24] | $X_{10,10,9,8,8,7,5,5,4,4}$ [120] | $X_{10,10,9,8,8,7,5,5,4,4,1,1}$ [120] |
| | [1,5,0,1,0,1,0,0,1,3] | [1,3,10,17,25,33,42,51,36,22,24] | $X_{10,9,8,8,8,8,8,6,4,1}$ [144] | $X_{10,9,8,8,8,8,8,6,4,1,1,1}$ [144] |
| | [1,5,1,0,0,0,0,2,0,2] | [1,3,10,18,26,34,42,50,36,22,24] | $X_{10,9,8,8,8,8,8,7,2,2}$ [72] | $X_{10,9,8,8,8,8,8,7,2,2,1,1}$ [72] |
| | [2,0,1,2,1,2,0,0,0,2] | [2,6,10,15,22,30,40,50,36,22,24] | $X_{10,10,9,9,7,6,6,5,4,4}$ [120] | $X_{10,10,9,9,7,6,6,5,4,4,1,1}$ [120] |
| | [2,2,2,1,0,1,0,1,0,2] | [1,4,9,16,24,32,41,50,36,22,24] | $X_{10,9,9,8,8,7,7,6,4,2}$ [216] | $X_{10,9,9,8,8,7,7,6,4,2,1,1}$ [216] |
| | [2,3,0,1,2,0,0,1,0,2] | [1,4,10,16,23,32,41,50,36,22,24] | $X_{10,9,9,8,8,8,6,5,5,2}$ [144] | $X_{10,9,9,8,8,8,6,5,5,2,1,1}$ [144] |
| | [2,3,0,2,0,0,2,0,0,2] | [1,4,10,16,24,32,40,50,36,22,24] | $X_{10,9,9,8,8,8,6,6,3,3}$ [96] | $X_{10,9,9,8,8,8,6,6,3,3,1,1}$ [96] |
| | [2,3,1,0,0,2,1,0,0,2] | [1,4,10,17,24,31,40,50,36,22,24] | $X_{10,9,9,8,8,8,7,4,4,3}$ [128] | $X_{10,9,9,8,8,8,7,4,4,3,1,1}$ [128] |
| | [3,0,2,3,0,0,0,0,1,3] | [1,5,9,15,24,33,42,51,36,22,24] | $X_{10,9,9,9,7,7,6,6,6,1}$ [72] | $X_{10,9,9,9,7,7,6,6,6,1,1,1}$ [72] |
| | [3,0,3,0,2,0,0,1,0,2] | [1,5,9,16,23,32,41,50,36,22,24] | $X_{10,9,9,9,7,7,7,5,5,2}$ [108] | $X_{10,9,9,9,7,7,7,5,5,2,1,1}$ [108] |
| | [3,0,3,1,0,0,2,0,0,2] | [1,5,9,16,24,32,40,50,36,22,24] | $X_{10,9,9,9,7,7,7,6,3,3}$ [96] | $X_{10,9,9,9,7,7,7,6,3,3,1,1}$ [96] |
| | [3,1,0,3,1,0,0,1,0,2] | [1,5,10,15,23,32,41,50,36,22,24] | $X_{10,9,9,9,8,6,6,6,5,2}$ [144] | $X_{10,9,9,9,8,6,6,6,5,2,1,1}$ [144] |
| | [3,2,0,0,1,3,0,0,0,2] | [1,5,11,17,23,30,40,50,36,22,24] | $X_{10,9,9,9,8,8,5,4,4,4}$ [80] | $X_{10,9,9,9,8,8,5,4,4,4,1,1}$ [80] |
| | [3,5,0,0,0,0,0,1,1,3] | [0,3,11,19,27,35,43,51,36,22,24] | $X_{9,9,9,8,8,8,8,8,2,1}$ [56] | $X_{9,9,9,8,8,8,8,8,2,1,1,1}$ [56] |
| | [4,0,0,1,3,0,1,0,0,2] | [1,6,11,16,22,31,40,50,36,22,24] | $X_{10,9,9,9,9,6,5,5,5,3}$ [96] | $X_{10,9,9,9,9,6,5,5,5,3,1,1}$ [96] |
| | [4,0,0,2,0,3,0,0,0,2] | [1,6,11,16,23,30,40,50,36,22,24] | $X_{10,9,9,9,9,6,6,4,4,4}$ [60] | $X_{10,9,9,9,9,6,6,4,4,4,1,1}$ [60] |
| | [4,2,1,0,2,0,0,0,1,3] | [0,4,10,17,24,33,42,51,36,22,24] | $X_{9,9,9,9,8,8,7,5,5,1}$ [120] | $X_{9,9,9,9,8,8,7,5,5,1,1,1}$ [120] |
| | [4,2,1,1,0,0,1,1,0,2] | [0,4,10,17,25,33,41,50,36,22,24] | $X_{9,9,9,9,8,8,7,6,3,2}$ [192] | $X_{9,9,9,9,8,8,7,6,3,2,1,1}$ [192] |
| | [4,3,0,0,0,2,0,1,0,2] | [0,4,11,18,25,32,41,50,36,22,24] | $X_{9,9,9,9,8,8,8,4,4,2}$ [90] | $X_{9,9,9,9,8,8,8,4,4,2,1,1}$ [90] |
| | [5,0,1,2,1,0,0,0,1,3] | [0,5,10,16,24,33,42,51,36,22,24] | $X_{9,9,9,9,9,7,6,6,5,1}$ [120] | $X_{9,9,9,9,9,7,6,6,5,1,1,1}$ [120] |
| | [5,0,2,0,1,1,0,1,0,2] | [0,5,10,17,24,32,41,50,36,22,24] | $X_{9,9,9,9,9,7,7,5,4,2}$ [162] | $X_{9,9,9,9,9,7,7,5,4,2,1,1}$ [162] |
| | [5,1,0,1,1,0,2,0,0,2] | [0,5,11,17,24,32,40,50,36,22,24] | $X_{9,9,9,9,9,8,6,5,3,3}$ [144] | $X_{9,9,9,9,9,8,6,5,3,3,1,1}$ [144] |
| | [6,0,0,0,1,2,1,0,0,2] | [0,6,12,18,24,31,40,50,36,22,24] | $X_{9,9,9,9,9,9,5,4,4,3}$ [80] | $X_{9,9,9,9,9,9,5,4,4,3,1,1}$ [80] |
| | [0,2,4,1,0,0,0,0,0,4] | [2,4,8,16,25,34,43,52,37,22,24] | $X_{10,10,8,8,7,7,7,7,7,6}$ [42] | $X_{10,10,8,8,7,7,7,7,7,6,1,1,1,1}$ [42] |
| | [1,4,2,0,1,0,0,0,0,4] | [1,3,9,17,25,34,43,52,37,22,24] | $X_{10,9,8,8,8,8,7,7,5}$ [72] | $X_{10,9,8,8,8,8,7,7,5,1,1,1,1}$ [72] |
| | [3,4,1,0,0,1,0,0,0,4] | [0,3,10,18,26,34,43,52,37,22,24] | $X_{9,9,9,8,8,8,8,7,4}$ [80] | $X_{9,9,9,8,8,8,8,7,4,1,1,1,1}$ [80] |
| | [4,1,3,0,1,0,0,0,0,4] | [0,4,9,17,25,34,43,52,37,22,24] | $X_{9,9,9,9,8,7,7,7,5}$ [72] | $X_{9,9,9,9,8,7,7,7,5,1,1,1,1}$ [72] |
| | [4,2,0,3,0,0,0,0,0,4] | [0,4,10,16,25,34,43,52,37,22,24] | $X_{9,9,9,9,8,8,6,6,6}$ [42] | $X_{9,9,9,9,8,8,6,6,6,1,1,1,1}$ [42] |
| | [3,2,1,1,0,0,0,0,6,0] | [1,5,11,18,26,34,42,50,33,22,25] | $X_{10,9,9,9,8,8,7,6,1,1,1,1,1,1}$ [56] | $X_{10,9,9,9,8,8,7,6}$ [56] |
| | [7,0,0,0,0,0,1,0,6,0] | [0,7,14,21,28,35,42,50,33,22,25] | $X_{9,9,9,9,9,9,9,3,1,1,1,1,1,1}$ [28] | $X_{9,9,9,9,9,9,9,3}$ [28] |
| | [0,4,1,0,1,1,0,0,4,0] | [2,4,10,17,24,32,41,50,34,22,25] | $X_{10,10,8,8,8,8,7,5,4,1,1,1,1}$ [90] | $X_{10,10,8,8,8,8,7,5,4}$ [90] |
| | [2,0,1,3,1,0,0,0,4,0] | [2,6,10,15,23,32,41,50,34,22,25] | $X_{10,10,9,9,7,6,6,6,5,1,1,1,1}$ [72] | $X_{10,10,9,9,7,6,6,6,5}$ [72] |
| | [2,3,1,1,0,0,1,0,4,0] | [1,4,10,17,25,33,41,50,34,22,25] | $X_{10,9,9,8,8,8,7,6,3,1,1,1,1}$ [128] | $X_{10,9,9,8,8,8,7,6,3}$ [128] |
| | [3,1,1,2,0,1,0,0,4,0] | [1,5,10,16,24,32,41,50,34,22,25] | $X_{10,9,9,9,8,7,6,6,4,1,1,1,1}$ [120] | $X_{10,9,9,9,8,7,6,6,4}$ [120] |
| | [3,2,0,0,3,0,0,0,4,0] | [1,5,11,17,23,32,41,50,34,22,25] | $X_{10,9,9,9,8,8,5,5,5,1,1,1,1}$ [48] | $X_{10,9,9,9,8,8,5,5,5}$ [48] |
| | [4,3,1,0,0,0,0,0,5,1] | [0,4,11,19,27,35,43,51,34,22,25] | $X_{9,9,9,9,8,8,8,7,1,1,1,1,1}$ [56] | $X_{9,9,9,9,8,8,8,7,1}$ [56] |
| | [5,1,1,0,1,0,1,0,4,0] | [0,5,11,18,25,33,41,50,34,22,25] | $X_{9,9,9,9,9,8,7,5,3,1,1,1,1}$ [144] | $X_{9,9,9,9,9,8,7,5,3}$ [144] |
| | [6,0,0,1,0,2,0,0,4,0] | [0,6,12,18,25,32,41,50,34,22,25] | $X_{9,9,9,9,9,9,6,4,4,1,1,1,1}$ [60] | $X_{9,9,9,9,9,9,6,4,4}$ [60] |
| | [0,0,3,1,2,0,1,0,2,0] | [3,6,9,15,22,31,40,50,35,22,25] | $X_{10,10,10,7,7,7,6,5,5,3,1,1}$ [96] | $X_{10,10,10,7,7,7,6,5,5,3}$ [96] |
| | [0,0,4,0,0,3,0,0,2,0] | [3,6,9,16,23,30,40,50,35,22,25] | $X_{10,10,10,7,7,7,7,4,4,4,1,1}$ [40] | $X_{10,10,10,7,7,7,7,4,4,4}$ [40] |
| | [0,1,0,5,0,0,0,1,2,0] | [3,6,10,14,23,32,41,50,35,22,25] | $X_{10,10,10,8,6,6,6,6,6,2,1,1}$ [67] | $X_{10,10,10,8,6,6,6,6,6,2}$ [68] |
| | [0,3,1,3,0,0,0,0,3,1] | [2,4,9,15,24,33,42,51,35,22,25] | $X_{10,10,8,8,8,7,6,6,6,1,1,1}$ [72] | $X_{10,10,8,8,8,7,6,6,6,1}$ [72] |
| | [0,3,2,0,2,0,0,1,2,0] | [2,4,9,16,23,32,41,50,35,22,25] | $X_{10,10,8,8,8,7,7,5,5,2,1,1}$ [108] | $X_{10,10,8,8,8,7,7,5,5,2}$ [108] |
| | [0,3,2,1,0,0,2,0,2,0] | [2,4,9,16,24,32,40,50,35,22,25] | $X_{10,10,8,8,8,7,7,6,3,3,1,1}$ [96] | $X_{10,10,8,8,8,7,7,6,3,3}$ [96] |
| | [0,4,0,1,1,1,1,0,2,0] | [2,4,10,16,23,31,40,50,35,22,25] | $X_{10,10,8,8,8,8,6,5,4,3,1,1}$ [144] | $X_{10,10,8,8,8,8,6,5,4,3}$ [144] |
| | [1,1,2,2,0,1,1,0,2,0] | [2,5,9,15,23,31,40,50,35,22,25] | $X_{10,10,9,8,7,7,6,6,4,3,1,1}$ [192] | $X_{10,10,9,8,7,7,6,6,4,3}$ [192] |
| | [1,2,0,2,2,0,1,0,2,0] | [2,5,10,15,22,31,40,50,35,22,25] | $X_{10,10,9,8,8,6,6,5,5,3,1,1}$ [144] | $X_{10,10,9,8,8,6,6,5,5,3}$ [144] |
| | [1,2,1,0,2,2,0,0,2,0] | [2,5,10,16,22,30,40,50,35,22,25] | $X_{10,10,9,8,8,7,5,5,4,4,1,1}$ [120] | $X_{10,10,9,8,8,7,5,5,4,4}$ [120] |
| | [1,5,0,1,0,1,0,0,3,1] | [1,3,10,17,25,33,42,51,35,22,25] | $X_{10,9,8,8,8,8,8,6,4,1,1,1}$ [144] | $X_{10,9,8,8,8,8,8,6,4,1}$ [144] |
| | [1,5,1,0,0,0,0,2,2,0] | [1,3,10,18,26,34,42,50,35,22,25] | $X_{10,9,8,8,8,8,8,7,2,2,1,1}$ [72] | $X_{10,9,8,8,8,8,8,7,2,2}$ [72] |
| | [2,0,1,2,1,2,0,0,2,0] | [2,6,10,15,22,30,40,50,35,22,25] | $X_{10,10,9,9,7,6,6,5,4,4,1,1}$ [120] | $X_{10,10,9,9,7,6,6,5,4,4}$ [120] |
| | [2,2,2,1,0,1,0,1,2,0] | [1,4,9,16,24,32,41,50,35,22,25] | $X_{10,9,9,8,8,7,7,6,4,2,1,1}$ [216] | $X_{10,9,9,8,8,7,7,6,4,2}$ [216] |
| | [2,3,0,1,2,0,0,1,2,0] | [1,4,10,16,23,32,41,50,35,22,25] | $X_{10,9,9,8,8,8,6,5,5,2,1,1}$ [144] | $X_{10,9,9,8,8,8,6,5,5,2}$ [144] |
| | [2,3,0,2,0,0,2,0,2,0] | [1,4,10,16,24,32,40,50,35,22,25] | $X_{10,9,9,8,8,8,6,6,3,3,1,1}$ [96] | $X_{10,9,9,8,8,8,6,6,3,3}$ [96] |
| | [2,3,1,0,0,2,1,0,2,0] | [1,4,10,17,24,31,40,50,35,22,25] | $X_{10,9,9,8,8,8,7,4,4,3,1,1}$ [128] | $X_{10,9,9,8,8,8,7,4,4,3}$ [128] |
| | [3,0,2,3,0,0,0,0,3,1] | [1,5,9,15,24,33,42,51,35,22,25] | $X_{10,9,9,9,7,7,6,6,6,1,1,1}$ [72] | $X_{10,9,9,9,7,7,6,6,6,1}$ [72] |
| | [3,0,3,0,2,0,0,1,2,0] | [1,5,9,16,23,32,41,50,35,22,25] | $X_{10,9,9,9,7,7,7,5,5,2,1,1}$ [108] | $X_{10,9,9,9,7,7,7,5,5,2}$ [108] |
| | [3,0,3,1,0,0,2,0,2,0] | [1,5,9,16,24,32,40,50,35,22,25] | $X_{10,9,9,9,7,7,7,6,3,3,1,1}$ [96] | $X_{10,9,9,9,7,7,7,6,3,3}$ [96] |
| | [3,1,0,3,1,0,0,1,2,0] | [1,5,10,15,23,32,41,50,35,22,25] | $X_{10,9,9,9,8,6,6,6,5,2,1,1}$ [144] | $X_{10,9,9,9,8,6,6,6,5,2}$ [144] |
| | [3,2,0,0,1,3,0,0,2,0] | [1,5,11,17,23,30,40,50,35,22,25] | $X_{10,9,9,9,8,8,5,4,4,4,1,1}$ [80] | $X_{10,9,9,9,8,8,5,4,4,4}$ [80] |
| | [3,5,0,0,0,0,0,1,3,1] | [0,3,11,19,27,35,43,51,35,22,25] | $X_{9,9,9,8,8,8,8,8,2,1,1,1}$ [56] | $X_{9,9,9,8,8,8,8,8,2,1}$ [56] |
| | [4,0,0,1,3,0,1,0,2,0] | [1,6,11,16,22,31,40,50,35,22,25] | $X_{10,9,9,9,9,6,5,5,5,3,1,1}$ [96] | $X_{10,9,9,9,9,6,5,5,5,3}$ [96] |
| | [4,0,0,2,0,3,0,0,2,0] | [1,6,11,16,23,30,40,50,35,22,25] | $X_{10,9,9,9,9,6,6,4,4,4,1,1}$ [60] | $X_{10,9,9,9,9,6,6,4,4,4}$ [60] |
| | [4,2,1,0,2,0,0,0,3,1] | [0,4,10,17,24,33,42,51,35,22,25] | $X_{9,9,9,9,8,8,7,5,5,1,1,1}$ [120] | $X_{9,9,9,9,8,8,7,5,5,1}$ [120] |
| | [4,2,1,1,0,0,1,1,2,0] | [0,4,10,17,25,33,41,50,35,22,25] | $X_{9,9,9,9,8,8,7,6,3,2,1,1}$ [192] | $X_{9,9,9,9,8,8,7,6,3,2}$ [192] |
| | [4,3,0,0,0,2,0,1,2,0] | [0,4,11,18,25,32,41,50,35,22,25] | $X_{9,9,9,9,8,8,8,4,4,2,1,1}$ [90] | $X_{9,9,9,9,8,8,8,4,4,2}$ [90] |
| | [5,0,1,2,1,0,0,0,3,1] | [0,5,10,16,24,33,42,51,35,22,25] | $X_{9,9,9,9,9,7,6,6,5,1,1,1}$ [120] | $X_{9,9,9,9,9,7,6,6,5,1}$ [120] |
| | [5,0,2,0,1,1,0,1,2,0] | [0,5,10,17,24,32,41,50,35,22,25] | $X_{9,9,9,9,9,7,7,5,4,2,1,1}$ [162] | $X_{9,9,9,9,9,7,7,5,4,2}$ [162] |

| | | | | |
|---|---|---|---|---|
| | [5,1,0,1,1,0,2,0,2,0] | [0,5,11,17,24,32,40,50,35,22,25] | $X_{9,9,9,9,9,8,6,5,3,3,1,1}$ [144] | $X_{9,9,9,9,9,8,6,5,3,3}$ [144] |
| | [6,0,0,0,1,2,1,0,2,0] | [0,6,12,18,24,31,40,50,35,22,25] | $X_{9,9,9,9,9,9,5,4,4,3,1,1}$ [80] | $X_{9,9,9,9,9,9,5,4,4,3}$ [80] |
| | [0,2,3,1,1,1,0,0,0,2] | [2,4,8,15,23,32,42,52,37,22,25] | $X_{10,10,8,8,7,7,7,6,5,4}$ [120] | $X_{10,10,8,8,7,7,7,6,5,4,1,1}$ [120] |
| | [0,3,1,1,3,0,0,0,0,2] | [2,4,9,15,22,32,42,52,37,22,25] | $X_{10,10,8,8,8,7,6,5,5,5}$ [72] | $X_{10,10,8,8,8,7,6,5,5,5,1,1}$ [72] |
| | [0,7,0,0,1,0,0,0,1,3] | [1,2,10,18,26,35,44,53,37,22,25] | $X_{10,8,8,8,8,8,8,8,5,1}$ [60] | $X_{10,8,8,8,8,8,8,8,5,1,1,1}$ [60] |
| | [1,1,1,3,2,0,0,0,0,2] | [2,5,9,14,22,32,42,52,37,22,25] | $X_{10,10,9,8,7,6,6,6,5,5}$ [96] | $X_{10,10,9,8,7,6,6,6,5,5,1,1}$ [96] |
| | [1,3,3,1,0,0,0,1,0,2] | [1,3,8,16,25,34,43,52,37,22,25] | $X_{10,9,8,8,8,7,7,7,6,2}$ [120] | $X_{10,9,8,8,8,7,7,7,6,2,1,1}$ [120] |
| | [1,4,1,1,0,2,0,0,0,2] | [1,3,9,16,24,32,42,52,37,22,25] | $X_{10,9,8,8,8,8,7,6,4,4}$ [120] | $X_{10,9,8,8,8,8,7,6,4,4,1,1}$ [120] |
| | [2,1,3,2,0,0,1,0,0,2] | [1,4,8,15,24,33,42,52,37,22,25] | $X_{10,9,9,8,7,7,7,6,6,3}$ [128] | $X_{10,9,9,8,7,7,7,6,6,3,1,1}$ [128] |
| | [2,1,4,0,0,2,0,0,0,2] | [1,4,8,16,24,32,42,52,37,22,25] | $X_{10,9,9,8,7,7,7,7,4,4}$ [80] | $X_{10,9,9,8,7,7,7,7,4,4,1,1}$ [80] |
| | [2,3,0,0,4,0,0,0,0,2] | [1,4,10,16,22,32,42,52,37,22,25] | $X_{10,9,9,8,8,8,5,5,5,5}$ [48] | $X_{10,9,9,8,8,8,5,5,5,5,1,1}$ [48] |
| | [3,0,2,1,3,0,0,0,0,2] | [1,5,9,15,22,32,42,52,37,22,25] | $X_{10,9,9,9,7,7,6,5,5,5}$ [72] | $X_{10,9,9,9,7,7,6,5,5,5,1,1}$ [72] |
| | [3,3,1,2,0,0,0,1,0,2] | [0,3,9,16,25,34,43,52,37,22,25] | $X_{9,9,9,8,8,8,7,6,6,2}$ [120] | $X_{9,9,9,8,8,8,7,6,6,2,1,1}$ [120] |
| | [3,3,2,0,0,1,1,0,0,2] | [0,3,9,17,25,33,42,52,37,22,25] | $X_{9,9,9,8,8,8,7,7,4,3}$ [128] | $X_{9,9,9,8,8,8,7,7,4,3,1,1}$ [128] |
| | [3,4,0,0,2,0,1,0,0,2] | [0,3,10,17,24,33,42,52,37,22,25] | $X_{9,9,9,8,8,8,8,5,5,3}$ [96] | $X_{9,9,9,8,8,8,8,5,5,3,1,1}$ [96] |
| | [4,0,5,0,0,0,0,0,1,3] | [0,4,8,17,26,35,44,53,37,22,25] | $X_{9,9,9,9,7,7,7,7,7,1}$ [42] | $X_{9,9,9,9,7,7,7,7,7,1,1,1}$ [42] |
| | [4,1,2,1,0,2,0,0,0,2] | [0,4,9,16,24,32,42,52,37,22,25] | $X_{9,9,9,9,8,7,7,6,4,4}$ [120] | $X_{9,9,9,9,8,7,7,6,4,4,1,1}$ [120] |
| | [4,2,0,1,2,1,0,0,0,2] | [0,4,10,16,23,32,42,52,37,22,25] | $X_{9,9,9,9,8,8,6,5,5,4}$ [120] | $X_{9,9,9,9,8,8,6,5,5,4,1,1}$ [120] |
| | [5,0,0,4,0,0,1,0,0,2] | [0,5,10,15,24,33,42,52,37,22,25] | $X_{9,9,9,9,9,6,6,6,6,3}$ [64] | $X_{9,9,9,9,9,6,6,6,6,3,1,1}$ [64] |
| | [2,6,0,1,0,0,0,0,0,4] | [0,2,10,18,27,36,45,54,38,22,25] | $X_{9,9,8,8,8,8,8,8,6}$ [42] | $X_{9,9,8,8,8,8,8,8,6,1,1,1,1}$ [42] |
| | [1,4,2,0,1,0,0,0,4,0] | [1,3,9,17,25,34,43,52,35,22,26] | $X_{10,9,8,8,8,8,7,7,5,1,1,1,1}$ [72] | $X_{10,9,8,8,8,8,7,7,5}$ [72] |
| | [3,4,1,0,0,1,0,0,4,0] | [0,3,10,18,26,34,43,52,35,22,26] | $X_{9,9,9,8,8,8,8,7,4,1,1,1,1}$ [80] | $X_{9,9,9,8,8,8,8,7,4}$ [80] |
| | [4,1,3,0,1,0,0,0,4,0] | [0,4,9,17,25,34,43,52,35,22,26] | $X_{9,9,9,9,8,7,7,7,5,1,1,1,1}$ [72] | $X_{9,9,9,9,8,7,7,7,5}$ [72] |
| | [4,2,0,3,0,0,0,0,4,0] | [0,4,10,16,25,34,43,52,35,22,26] | $X_{9,9,9,9,8,8,6,6,6,1,1,1,1}$ [42] | $X_{9,9,9,9,8,8,6,6,6}$ [42] |
| | [0,2,3,1,1,1,0,0,2,0] | [2,4,8,15,23,32,42,52,36,22,26] | $X_{10,10,8,8,7,7,7,6,5,4,1,1}$ [120] | $X_{10,10,8,8,7,7,7,6,5,4}$ [120] |
| | [0,3,1,1,3,0,0,0,2,0] | [2,4,9,15,22,32,42,52,36,22,26] | $X_{10,10,8,8,8,7,6,5,5,5,1,1}$ [72] | $X_{10,10,8,8,8,7,6,5,5,5}$ [72] |
| | [0,7,0,0,1,0,0,0,3,1] | [1,2,10,18,26,35,44,53,36,22,26] | $X_{10,8,8,8,8,8,8,8,5,1,1,1}$ [60] | $X_{10,8,8,8,8,8,8,8,5,1}$ [60] |
| | [1,1,1,3,2,0,0,0,2,0] | [2,5,9,14,22,32,42,52,36,22,26] | $X_{10,10,9,8,7,6,6,6,5,5,1,1}$ [96] | $X_{10,10,9,8,7,6,6,6,5,5}$ [96] |
| | [1,3,3,1,0,0,0,1,2,0] | [1,3,8,16,25,34,43,52,36,22,26] | $X_{10,9,8,8,8,7,7,7,6,2,1,1}$ [120] | $X_{10,9,8,8,8,7,7,7,6,2}$ [120] |
| | [1,4,1,1,0,2,0,0,2,0] | [1,3,9,16,24,32,42,52,36,22,26] | $X_{10,9,8,8,8,8,7,6,4,4,1,1}$ [120] | $X_{10,9,8,8,8,8,7,6,4,4}$ [120] |
| | [2,1,3,2,0,0,1,0,2,0] | [1,4,8,15,24,33,42,52,36,22,26] | $X_{10,9,9,8,7,7,7,6,6,3,1,1}$ [128] | $X_{10,9,9,8,7,7,7,6,6,3}$ [128] |
| | [2,1,4,0,0,2,0,0,2,0] | [1,4,8,16,24,32,42,52,36,22,26] | $X_{10,9,9,8,7,7,7,7,4,4,1,1}$ [80] | $X_{10,9,9,8,7,7,7,7,4,4}$ [80] |
| | [2,3,0,0,4,0,0,0,2,0] | [1,4,10,16,22,32,42,52,36,22,26] | $X_{10,9,9,8,8,8,5,5,5,5,1,1}$ [48] | $X_{10,9,9,8,8,8,5,5,5,5}$ [48] |
| | [3,0,2,1,3,0,0,0,2,0] | [1,5,9,15,22,32,42,52,36,22,26] | $X_{10,9,9,9,7,7,6,5,5,5,1,1}$ [72] | $X_{10,9,9,9,7,7,6,5,5,5}$ [72] |
| | [3,3,1,2,0,0,0,1,2,0] | [0,3,9,16,25,34,43,52,36,22,26] | $X_{9,9,9,8,8,8,7,6,6,2,1,1}$ [120] | $X_{9,9,9,8,8,8,7,6,6,2}$ [120] |
| | [3,3,2,0,0,1,1,0,2,0] | [0,3,9,17,25,33,42,52,36,22,26] | $X_{9,9,9,8,8,8,7,7,4,3,1,1}$ [128] | $X_{9,9,9,8,8,8,7,7,4,3}$ [128] |
| | [3,4,0,0,2,0,1,0,2,0] | [0,3,10,17,24,33,42,52,36,22,26] | $X_{9,9,9,8,8,8,8,5,5,3,1,1}$ [96] | $X_{9,9,9,8,8,8,8,5,5,3}$ [96] |
| | [4,0,5,0,0,0,0,0,3,1] | [0,4,8,17,26,35,44,53,36,22,26] | $X_{9,9,9,9,7,7,7,7,7,1,1,1}$ [42] | $X_{9,9,9,9,7,7,7,7,7,1}$ [42] |
| | [4,1,2,1,0,2,0,0,2,0] | [0,4,9,16,24,32,42,52,36,22,26] | $X_{9,9,9,9,8,7,7,6,4,4,1,1}$ [120] | $X_{9,9,9,9,8,7,7,6,4,4}$ [120] |
| | [4,2,0,1,2,1,0,0,2,0] | [0,4,10,16,23,32,42,52,36,22,26] | $X_{9,9,9,9,8,8,6,5,5,4,1,1}$ [120] | $X_{9,9,9,9,8,8,6,5,5,4}$ [120] |
| | [5,0,0,4,0,0,1,0,2,0] | [0,5,10,15,24,33,42,52,36,22,26] | $X_{9,9,9,9,9,6,6,6,6,3,1,1}$ [64] | $X_{9,9,9,9,9,6,6,6,6,3}$ [64] |
| | [0,1,5,1,1,0,0,0,0,2] | [2,4,7,15,24,34,44,54,38,22,26] | $X_{10,10,8,7,7,7,7,7,6,5}$ [72] | $X_{10,10,8,7,7,7,7,7,6,5,1,1}$ [72] |
| | [0,5,3,0,0,0,1,0,0,2] | [1,2,8,17,26,35,44,54,38,22,26] | $X_{10,8,8,8,8,8,7,7,7,3}$ [60] | $X_{10,8,8,8,8,8,7,7,7,3,1,1}$ [60] |
| | [0,6,0,2,0,1,0,0,0,2] | [1,2,9,16,25,34,44,54,38,22,26] | $X_{10,8,8,8,8,8,8,6,6,4}$ [68] | $X_{10,8,8,8,8,8,8,6,6,4,1,1}$ [67] |
| | [2,0,6,0,0,1,0,0,0,2] | [1,4,7,16,25,34,44,54,38,22,26] | $X_{10,9,9,7,7,7,7,7,7,4}$ [60] | $X_{10,9,9,7,7,7,7,7,7,4,1,1}$ [60] |
| | [2,1,2,4,0,0,0,0,0,2] | [1,4,8,14,24,34,44,54,38,22,26] | $X_{10,9,9,8,7,7,6,6,6,6}$ [56] | $X_{10,9,9,8,7,7,6,6,6,6,1,1}$ [56] |
| | [2,5,1,0,1,1,0,0,0,2] | [0,2,9,17,25,34,44,54,38,22,26] | $X_{9,9,8,8,8,8,8,7,5,4}$ [120] | $X_{9,9,8,8,8,8,8,7,5,4,1,1}$ [120] |
| | [3,2,3,0,2,0,0,0,0,2] | [0,3,8,16,24,34,44,54,38,22,26] | $X_{9,9,9,8,8,7,7,7,5,5}$ [72] | $X_{9,9,9,8,8,7,7,7,5,5,1,1}$ [72] |
| | [3,3,0,3,1,0,0,0,0,2] | [0,3,9,15,24,34,44,54,38,22,26] | $X_{9,9,9,8,8,8,6,6,6,5}$ [72] | $X_{9,9,9,8,8,8,6,6,6,5,1,1}$ [72] |
| | [4,0,3,2,1,0,0,0,0,2] | [0,4,8,15,24,34,44,54,38,22,26] | $X_{9,9,9,9,7,7,7,6,6,5}$ [72] | $X_{9,9,9,9,7,7,7,6,6,5,1,1}$ [72] |
| | [2,6,0,1,0,0,0,0,4,0] | [0,2,10,18,27,36,45,54,36,22,27] | $X_{9,9,8,8,8,8,8,8,6,1,1,1,1}$ [42] | $X_{9,9,8,8,8,8,8,8,6}$ [42] |
| | [0,1,5,1,1,0,0,0,2,0] | [2,4,7,15,24,34,44,54,37,22,27] | $X_{10,10,8,7,7,7,7,7,6,5,1,1}$ [72] | $X_{10,10,8,7,7,7,7,7,6,5}$ [72] |
| | [0,5,3,0,0,0,1,0,2,0] | [1,2,8,17,26,35,44,54,37,22,27] | $X_{10,8,8,8,8,8,7,7,7,3,1,1}$ [60] | $X_{10,8,8,8,8,8,7,7,7,3}$ [60] |
| | [0,6,0,2,0,1,0,0,2,0] | [1,2,9,16,25,34,44,54,37,22,27] | $X_{10,8,8,8,8,8,8,6,6,4,1,1}$ [67] | $X_{10,8,8,8,8,8,8,6,6,4}$ [68] |
| | [2,0,6,0,0,1,0,0,2,0] | [1,4,7,16,25,34,44,54,37,22,27] | $X_{10,9,9,7,7,7,7,7,7,4,1,1}$ [60] | $X_{10,9,9,7,7,7,7,7,7,4}$ [60] |
| | [2,1,2,4,0,0,0,0,2,0] | [1,4,8,14,24,34,44,54,37,22,27] | $X_{10,9,9,8,7,7,6,6,6,6,1,1}$ [56] | $X_{10,9,9,8,7,7,6,6,6,6}$ [56] |
| | [2,5,1,0,1,1,0,0,2,0] | [0,2,9,17,25,34,44,54,37,22,27] | $X_{9,9,8,8,8,8,8,7,5,4,1,1}$ [120] | $X_{9,9,8,8,8,8,8,7,5,4}$ [120] |
| | [3,2,3,0,2,0,0,0,2,0] | [0,3,8,16,24,34,44,54,37,22,27] | $X_{9,9,9,8,8,7,7,7,5,5,1,1}$ [72] | $X_{9,9,9,8,8,7,7,7,5,5}$ [72] |
| | [3,3,0,3,1,0,0,0,2,0] | [0,3,9,15,24,34,44,54,37,22,27] | $X_{9,9,9,8,8,8,6,6,6,5,1,1}$ [72] | $X_{9,9,9,8,8,8,6,6,6,5}$ [72] |
| | [4,0,3,2,1,0,0,0,2,0] | [0,4,8,15,24,34,44,54,37,22,27] | $X_{9,9,9,9,7,7,7,6,6,5,1,1}$ [72] | $X_{9,9,9,9,7,7,7,6,6,5}$ [72] |
| | [1,8,0,0,0,0,1,0,0,2] | [0,1,10,19,28,37,46,56,39,22,27] | $X_{9,8,8,8,8,8,8,8,8,3}$ [48] | $X_{9,8,8,8,8,8,8,8,8,3,1,1}$ [48] |
| | [3,1,5,1,0,0,0,0,0,2] | [0,3,7,16,26,36,46,56,39,22,27] | $X_{9,9,9,8,7,7,7,7,7,6}$ [56] | $X_{9,9,9,8,7,7,7,7,7,6,1,1}$ [56] |
| | [1,8,0,0,0,0,1,0,2,0] | [0,1,10,19,28,37,46,56,38,22,28] | $X_{9,8,8,8,8,8,8,8,8,3,1,1}$ [48] | $X_{9,8,8,8,8,8,8,8,8,3}$ [48] |
| | [3,1,5,1,0,0,0,0,2,0] | [0,3,7,16,26,36,46,56,38,22,28] | $X_{9,9,9,8,7,7,7,7,7,6,1,1}$ [56] | $X_{9,9,9,8,7,7,7,7,7,6}$ [56] |
| | [1,6,3,0,0,0,0,0,0,2] | [0,1,8,18,28,38,48,58,40,22,28] | $X_{9,8,8,8,8,8,8,7,7,7}$ [32] | $X_{9,8,8,8,8,8,8,7,7,7,1,1}$ [32] |
| | [1,6,3,0,0,0,0,0,2,0] | [0,1,8,18,28,38,48,58,39,22,29] | $X_{9,8,8,8,8,8,8,7,7,7,1,1}$ [32] | $X_{9,8,8,8,8,8,8,7,7,7}$ [32] |
| 23 | [0,0,0,1,1,0,1,0,5,2] | [5,10,15,20,26,33,40,48,33,23,23] | $Y_{10,10,10,10,10,6,5,3,1,1,1,1,1}$ [90] | $Y_{10,10,10,10,10,6,5,3,1,1}$ [90] |
| | [0,0,1,0,0,1,0,2,4,1] | [5,10,15,21,27,33,40,47,33,23,23] | $Y_{10,10,10,10,10,7,4,2,2,1,1,1,1}$ [96] | $Y_{10,10,10,10,10,7,4,2,2,1}$ [96] |
| | [0,2,1,0,0,0,0,0,6,3] | [4,8,14,21,28,35,42,49,33,23,23] | $Y_{10,10,10,10,8,8,7,1,1,1,1,1,1}$ [42] | $Y_{10,10,10,10,8,8,7,1,1,1}$ [42] |
| | [1,0,1,1,0,0,0,1,5,2] | [4,9,14,20,27,34,41,48,33,23,23] | $Y_{10,10,10,10,9,7,6,2,1,1,1,1,1}$ [120] | $Y_{10,10,10,10,9,7,6,2,1,1}$ [120] |
| | [1,1,0,0,0,1,1,0,5,2] | [4,9,15,21,27,33,40,48,33,23,23] | $Y_{10,10,10,10,9,8,4,3,1,1,1,1,1}$ [120] | $Y_{10,10,10,10,9,8,4,3,1,1}$ [120] |

| | | | | |
|---|---|---|---|---|
| | [2,0,0,0,0,0,1,2,4,1] | [4,10,16,22,28,34,40,47,33,23,23] | $Y_{10,10,10,10,9,9,3,2,2,1,1,1,1}$ [56] | $Y_{10,10,10,10,9,9,3,2,2,1}$ [56] |
| | [3,0,0,1,0,0,0,0,6,3] | [3,9,15,21,28,35,42,49,33,23,23] | $Y_{10,10,10,9,9,9,6,1,1,1,1,1,1}$ [48] | $Y_{10,10,10,9,9,9,6,1,1,1}$ [48] |
| | [0,0,0,0,1,2,1,0,3,2] | [5,10,15,20,25,31,39,48,34,23,23] | $Y_{10,10,10,10,10,5,4,4,3,1,1,1}$ [72] | $Y_{10,10,10,10,10,5,4,4,3,1,1}$ [72] |
| | [0,0,0,0,2,0,1,2,2,1] | [5,10,15,20,25,32,39,47,34,23,23] | $Y_{10,10,10,10,10,5,5,3,2,2,1,1}$ [72] | $Y_{10,10,10,10,10,5,5,3,2,2,1}$ [72] |
| | [0,0,3,0,0,1,0,0,4,3] | [4,8,12,19,26,33,41,49,34,23,23] | $Y_{10,10,10,10,7,7,7,4,1,1,1,1}$ [64] | $Y_{10,10,10,10,7,7,7,4,1,1,1}$ [64] |
| | [0,1,0,0,0,0,0,5,1,0] | [5,10,16,22,28,34,40,46,34,23,23] | $Y_{10,10,10,10,10,8,2,2,2,2,2,1}$ [31] | $Y_{10,10,10,10,10,8,2,2,2,2,2}$ [32] |
| | [0,1,0,2,1,0,0,0,4,3] | [4,8,13,18,25,33,41,49,34,23,23] | $Y_{10,10,10,10,8,6,6,5,1,1,1,1}$ [90] | $Y_{10,10,10,10,8,6,6,5,1,1,1}$ [90] |
| | [0,1,1,0,1,1,0,1,3,2] | [4,8,13,19,25,32,40,48,34,23,23] | $Y_{10,10,10,10,8,7,5,4,2,1,1,1}$ [216] | $Y_{10,10,10,10,8,7,5,4,2,1,1}$ [216] |
| | [0,2,0,0,0,1,2,0,3,2] | [4,8,14,20,26,32,39,48,34,23,23] | $Y_{10,10,10,10,8,8,4,3,3,1,1,1}$ [90] | $Y_{10,10,10,10,8,8,4,3,3,1,1}$ [90] |
| | [0,2,0,0,1,0,0,3,2,1] | [4,8,14,20,26,33,40,47,34,23,23] | $Y_{10,10,10,10,8,8,5,2,2,2,1,1}$ [96] | $Y_{10,10,10,10,8,8,5,2,2,2,1}$ [96] |
| | [1,0,0,1,1,0,2,0,3,2] | [4,9,14,19,25,32,39,48,34,23,23] | $Y_{10,10,10,10,9,6,5,3,3,1,1,1}$ [144] | $Y_{10,10,10,10,9,6,5,3,3,1,1}$ [144] |
| | [1,0,0,2,0,0,0,3,2,1] | [4,9,14,19,26,33,40,47,34,23,23] | $Y_{10,10,10,10,9,6,6,2,2,2,1,1}$ [80] | $Y_{10,10,10,10,9,6,6,2,2,2,1}$ [80] |
| | [1,0,1,0,0,1,1,2,2,1] | [4,9,14,20,26,32,39,47,34,23,23] | $Y_{10,10,10,10,9,7,4,3,2,2,1,1}$ [192] | $Y_{10,10,10,10,9,7,4,3,2,2,1}$ [192] |
| | [1,2,0,1,0,1,0,0,4,3] | [3,7,13,19,26,33,41,49,34,23,23] | $Y_{10,10,10,9,8,8,6,4,1,1,1,1}$ [144] | $Y_{10,10,10,9,8,8,6,4,1,1,1}$ [144] |
| | [1,2,1,0,0,0,0,2,3,2] | [3,7,13,20,27,34,41,48,34,23,23] | $Y_{10,10,10,9,8,8,7,2,2,1,1,1}$ [96] | $Y_{10,10,10,9,8,8,7,2,2,1,1}$ [96] |
| | [2,0,1,0,2,0,0,0,4,3] | [3,8,13,19,25,33,41,49,34,23,23] | $Y_{10,10,10,9,9,7,5,5,1,1,1,1}$ [90] | $Y_{10,10,10,9,9,7,5,5,1,1,1}$ [90] |
| | [2,0,1,1,0,0,1,1,3,2] | [3,8,13,19,26,33,40,48,34,23,23] | $Y_{10,10,10,9,9,7,6,3,2,1,1,1}$ [192] | $Y_{10,10,10,9,9,7,6,3,2,1,1}$ [192] |
| | [2,1,0,0,0,2,0,1,3,2] | [3,8,14,20,26,32,40,48,34,23,23] | $Y_{10,10,10,9,9,8,4,4,2,1,1,1}$ [120] | $Y_{10,10,10,9,9,8,4,4,2,1,1}$ [120] |
| | [3,0,0,0,0,0,3,0,3,2] | [3,9,15,21,27,33,39,48,34,23,23] | $Y_{10,10,10,9,9,9,3,3,3,1,1,1}$ [42] | $Y_{10,10,10,9,9,9,3,3,3,1,1}$ [42] |
| | [3,0,0,0,0,1,0,3,2,1] | [3,9,15,21,27,33,40,47,34,23,23] | $Y_{10,10,10,9,9,9,4,2,2,2,1,1}$ [72] | $Y_{10,10,10,9,9,9,4,2,2,2,1}$ [72] |
| | [3,2,0,0,0,0,0,1,4,3] | [2,7,14,21,28,35,42,49,34,23,23] | $Y_{10,10,9,9,9,8,8,2,1,1,1,1}$ [56] | $Y_{10,10,9,9,9,8,8,2,1,1,1}$ [56] |
| | [4,0,0,1,0,0,1,0,4,3] | [2,8,14,20,27,34,41,49,34,23,23] | $Y_{10,10,9,9,9,9,6,3,1,1,1,1}$ [96] | $Y_{10,10,9,9,9,9,6,3,1,1,1}$ [96] |
| | [0,0,0,0,1,1,3,0,1,2] | [5,10,15,20,25,31,38,48,35,23,23] | $Y_{10,10,10,10,10,5,4,3,3,3,1}$ [72] | $Y_{10,10,10,10,10,5,4,3,3,3,1,1}$ [72] |
| | [0,0,0,0,1,2,0,3,0,1] | [5,10,15,20,25,31,39,47,35,23,23] | $Y_{10,10,10,10,10,5,4,4,2,2,2}$ [54] | $Y_{10,10,10,10,10,5,4,4,2,2,2,1}$ [54] |
| | [0,0,0,1,0,0,3,2,0,1] | [5,10,15,20,26,32,38,47,35,23,23] | $Y_{10,10,10,10,10,6,3,3,3,2,2}$ [60] | $Y_{10,10,10,10,10,6,3,3,3,2,2,1}$ [60] |
| | [0,0,1,3,0,0,0,1,2,3] | [4,8,12,17,25,33,41,49,35,23,23] | $Y_{10,10,10,10,7,6,6,6,2,1,1}$ [80] | $Y_{10,10,10,10,7,6,6,6,2,1,1,1}$ [80] |
| | [0,0,2,0,2,0,1,0,2,3] | [4,8,12,18,24,32,40,49,35,23,23] | $Y_{10,10,10,10,7,7,5,5,3,1,1}$ [108] | $Y_{10,10,10,10,7,7,5,5,3,1,1,1}$ [108] |
| | [0,0,2,1,0,1,0,2,1,2] | [4,8,12,18,25,32,40,48,35,23,23] | $Y_{10,10,10,10,7,7,6,4,2,2,1}$ [144] | $Y_{10,10,10,10,7,7,6,4,2,2,1,1}$ [144] |
| | [0,1,0,1,1,2,0,0,2,3] | [4,8,13,18,24,31,40,49,35,23,23] | $Y_{10,10,10,10,8,6,5,4,4,1,1}$ [144] | $Y_{10,10,10,10,8,6,5,4,4,1,1,1}$ [144] |
| | [0,1,0,1,2,0,0,2,1,2] | [4,8,13,18,24,32,40,48,35,23,23] | $Y_{10,10,10,10,8,6,5,5,2,2,1}$ [144] | $Y_{10,10,10,10,8,6,5,5,2,2,1,1}$ [144] |
| | [0,1,0,2,0,0,2,1,1,2] | [4,8,13,18,25,32,39,48,35,23,23] | $Y_{10,10,10,10,8,6,6,3,3,2,1}$ [144] | $Y_{10,10,10,10,8,6,6,3,3,2,1,1}$ [144] |
| | [0,1,1,0,0,2,1,1,1,2] | [4,8,13,19,25,31,39,48,35,23,23] | $Y_{10,10,10,10,8,7,4,4,3,2,1}$ [192] | $Y_{10,10,10,10,8,7,4,4,3,2,1,1}$ [192] |
| | [0,1,1,1,0,0,0,4,0,1] | [4,8,13,19,26,33,40,47,35,23,23] | $Y_{10,10,10,10,8,7,6,2,2,2,2}$ [90] | $Y_{10,10,10,10,8,7,6,2,2,2,2,1}$ [90] |
| | [0,2,0,0,0,1,1,3,0,1] | [4,8,14,20,26,32,39,47,35,23,23] | $Y_{10,10,10,10,8,8,4,3,2,2,2}$ [90] | $Y_{10,10,10,10,8,8,4,3,2,2,2,1}$ [90] |
| | [0,3,0,2,0,0,0,0,3,4] | [3,6,12,18,26,34,42,50,35,23,23] | $Y_{10,10,10,8,8,8,6,6,1,1,1}$ [54] | $Y_{10,10,10,8,8,8,6,6,1,1,1,1}$ [54] |
| | [0,3,1,0,0,1,0,1,2,3] | [3,6,12,19,26,33,41,49,35,23,23] | $Y_{10,10,10,8,8,8,7,4,2,1,1}$ [144] | $Y_{10,10,10,8,8,8,7,4,2,1,1,1}$ [144] |
| | [1,0,0,0,2,1,1,1,1,2] | [4,9,14,19,24,31,39,48,35,23,23] | $Y_{10,10,10,10,9,5,5,4,3,2,1}$ [160] | $Y_{10,10,10,10,9,5,5,4,3,2,1,1}$ [160] |
| | [1,0,0,1,1,0,1,3,0,1] | [4,9,14,19,25,32,39,47,35,23,23] | $Y_{10,10,10,10,9,6,5,3,2,2,2}$ [144] | $Y_{10,10,10,10,9,6,5,3,2,2,2,1}$ [144] |
| | [1,0,1,0,0,0,4,0,1,2] | [4,9,14,20,26,32,38,48,35,23,23] | $Y_{10,10,10,10,9,7,3,3,3,3,1}$ [90] | $Y_{10,10,10,10,9,7,3,3,3,3,1,1}$ [90] |
| | [1,0,3,1,0,0,0,0,3,4] | [3,7,11,18,26,34,42,50,35,23,23] | $Y_{10,10,10,9,7,7,7,6,1,1,1}$ [72] | $Y_{10,10,10,9,7,7,7,6,1,1,1,1}$ [72] |
| | [1,1,1,1,0,1,1,0,2,3] | [3,7,12,18,25,32,40,49,35,23,23] | $Y_{10,10,10,9,8,7,6,4,3,1,1}$ [288] | $Y_{10,10,10,9,8,7,6,4,3,1,1,1}$ [288] |
| | [1,1,2,0,0,0,1,2,1,2] | [3,7,12,19,26,33,40,48,35,23,23] | $Y_{10,10,10,9,8,7,7,3,2,2,1}$ [160] | $Y_{10,10,10,9,8,7,7,3,2,2,1,1}$ [160] |
| | [1,2,0,0,1,1,0,2,1,2] | [3,7,13,19,25,32,40,48,35,23,23] | $Y_{10,10,10,9,8,8,5,4,2,2,1}$ [192] | $Y_{10,10,10,9,8,8,5,4,2,2,1,1}$ [192] |
| | [2,0,0,1,2,0,1,0,2,3] | [3,8,13,18,24,32,40,49,35,23,23] | $Y_{10,10,10,9,9,6,5,5,3,1,1}$ [144] | $Y_{10,10,10,9,9,6,5,5,3,1,1,1}$ [144] |
| | [2,0,0,2,0,1,0,2,1,2] | [3,8,13,18,25,32,40,48,35,23,23] | $Y_{10,10,10,9,9,6,6,4,2,2,1}$ [144] | $Y_{10,10,10,9,9,6,6,4,2,2,1,1}$ [144] |
| | [2,0,1,0,0,3,0,0,2,3] | [3,8,13,19,25,31,40,49,35,23,23] | $Y_{10,10,10,9,9,7,4,4,4,1,1}$ [96] | $Y_{10,10,10,9,9,7,4,4,4,1,1,1}$ [96] |
| | [2,0,1,0,1,0,2,1,1,2] | [3,8,13,19,25,32,39,48,35,23,23] | $Y_{10,10,10,9,9,7,5,3,3,2,1}$ [216] | $Y_{10,10,10,9,9,7,5,3,3,2,1,1}$ [216] |
| | [2,1,0,0,1,0,0,4,0,1] | [3,8,14,20,26,33,40,47,35,23,23] | $Y_{10,10,10,9,9,8,5,2,2,2,2}$ [96] | $Y_{10,10,10,9,9,8,5,2,2,2,2,1}$ [96] |
| | [2,2,1,0,1,0,0,0,3,4] | [2,6,12,19,26,34,42,50,35,23,23] | $Y_{10,10,9,9,8,8,7,5,1,1,1}$ [120] | $Y_{10,10,9,9,8,8,7,5,1,1,1,1}$ [120] |
| | [2,3,0,0,0,0,1,1,2,3] | [2,6,13,20,27,34,41,49,35,23,23] | $Y_{10,10,9,9,8,8,8,3,2,1,1}$ [96] | $Y_{10,10,9,9,8,8,8,3,2,1,1,1}$ [96] |
| | [3,0,0,0,0,0,2,3,0,1] | [3,9,15,21,27,33,39,47,35,23,23] | $Y_{10,10,10,9,9,9,3,3,2,2,2}$ [42] | $Y_{10,10,10,9,9,9,3,3,2,2,2,1}$ [42] |
| | [3,0,1,2,0,0,0,0,3,4] | [2,7,12,18,26,34,42,50,35,23,23] | $Y_{10,10,9,9,9,7,6,6,1,1,1}$ [72] | $Y_{10,10,9,9,9,7,6,6,1,1,1,1}$ [72] |
| | [3,0,2,0,0,1,0,1,2,3] | [2,7,12,19,26,33,41,49,35,23,23] | $Y_{10,10,9,9,9,7,7,4,2,1,1}$ [144] | $Y_{10,10,9,9,9,7,7,4,2,1,1,1}$ [144] |
| | [3,1,0,0,2,0,0,1,2,3] | [2,7,13,19,25,33,41,49,35,23,23] | $Y_{10,10,9,9,9,8,5,5,2,1,1}$ [128] | $Y_{10,10,9,9,9,8,5,5,2,1,1,1}$ [128] |
| | [3,1,0,1,0,0,2,0,2,3] | [2,7,13,19,26,33,40,49,35,23,23] | $Y_{10,10,9,9,9,8,6,3,3,1,1}$ [144] | $Y_{10,10,9,9,9,8,6,3,3,1,1,1}$ [144] |
| | [3,1,1,0,0,0,0,3,1,2] | [2,7,13,20,27,34,41,48,35,23,23] | $Y_{10,10,9,9,9,8,7,2,2,2,1}$ [96] | $Y_{10,10,9,9,9,8,7,2,2,2,1,1}$ [96] |
| | [4,0,0,0,0,2,1,0,2,3] | [2,8,14,20,26,32,40,49,35,23,23] | $Y_{10,10,9,9,9,9,4,4,3,1,1}$ [72] | $Y_{10,10,9,9,9,9,4,4,3,1,1,1}$ [72] |
| | [4,0,0,0,1,0,1,2,1,2] | [2,8,14,20,26,33,40,48,35,23,23] | $Y_{10,10,9,9,9,9,5,3,2,2,1}$ [120] | $Y_{10,10,9,9,9,9,5,3,2,2,1,1}$ [120] |
| | [5,1,0,0,0,0,1,0,3,4] | [1,7,14,21,28,35,42,50,35,23,23] | $Y_{10,9,9,9,9,9,8,3,1,1,1}$ [72] | $Y_{10,9,9,9,9,9,8,3,1,1,1,1}$ [72] |
| | [0,0,0,0,0,4,1,0,0,3] | [5,10,15,20,25,30,39,49,36,23,23] | $Y_{10,10,10,10,10,4,4,4,4,3}$ [28] | $Y_{10,10,10,10,10,4,4,4,4,3,1,1,1}$ [28] |
| | [0,0,1,2,1,0,1,1,0,3] | [4,8,12,17,24,32,40,49,36,23,23] | $Y_{10,10,10,10,7,6,6,5,3,2}$ [144] | $Y_{10,10,10,10,7,6,6,5,3,2,1,1,1}$ [144] |
| | [0,0,2,0,1,2,0,1,0,3] | [4,8,12,18,24,31,40,49,36,23,23] | $Y_{10,10,10,10,7,7,5,4,4,2}$ [108] | $Y_{10,10,10,10,7,7,5,4,4,2,1,1,1}$ [108] |
| | [0,0,2,1,0,0,3,0,0,3] | [4,8,12,18,25,32,39,49,36,23,23] | $Y_{10,10,10,10,7,7,6,3,3,3}$ [64] | $Y_{10,10,10,10,7,7,6,3,3,3,1,1,1}$ [64] |
| | [0,1,0,0,4,0,0,0,1,4] | [4,8,13,18,23,32,41,50,36,23,23] | $Y_{10,10,10,10,8,5,5,5,5,1}$ [60] | $Y_{10,10,10,10,8,5,5,5,5,1,1,1,1}$ [60] |
| | [0,1,0,1,1,1,2,0,0,3] | [4,8,13,18,24,31,39,49,36,23,23] | $Y_{10,10,10,10,8,6,5,4,3,3}$ [144] | $Y_{10,10,10,10,8,6,5,4,3,3,1,1,1}$ [144] |
| | [0,2,2,0,1,0,1,0,1,4] | [3,6,11,18,25,33,41,50,36,23,23] | $Y_{10,10,10,8,8,7,7,5,3,1}$ [162] | $Y_{10,10,10,8,8,7,7,5,3,1,1,1,1}$ [162] |
| | [0,3,0,1,0,2,0,0,1,4] | [3,6,12,18,25,32,41,50,36,23,23] | $Y_{10,10,10,8,8,8,6,4,4,1}$ [108] | $Y_{10,10,10,8,8,8,6,4,4,1,1,1,1}$ [108] |
| | [0,3,0,1,1,0,0,2,0,3] | [3,6,12,18,25,33,41,49,36,23,23] | $Y_{10,10,10,8,8,8,6,5,2,2}$ [108] | $Y_{10,10,10,8,8,8,6,5,2,2,1,1,1}$ [108] |
| | [0,3,1,0,0,0,2,1,0,3] | [3,6,12,19,26,33,40,49,36,23,23] | $Y_{10,10,10,8,8,8,7,3,3,2}$ [90] | $Y_{10,10,10,8,8,8,7,3,3,2,1,1,1}$ [90] |
| | [1,0,2,2,0,0,1,0,1,4] | [3,7,11,17,25,33,41,50,36,23,23] | $Y_{10,10,10,9,7,7,6,6,3,1}$ [144] | $Y_{10,10,10,9,7,7,6,6,3,1,1,1,1}$ [144] |
| | [1,0,3,0,0,2,0,0,1,4] | [3,7,11,18,25,32,41,50,36,23,23] | $Y_{10,10,10,9,7,7,7,4,4,1}$ [96] | $Y_{10,10,10,9,7,7,7,4,4,1,1,1,1}$ [96] |

| | | | | |
|---|---|---|---|---|
| | [1,0,3,0,1,0,0,2,0,3] | [3,7,11,18,25,33,41,49,36,23,23] | $Y_{10,10,10,9,7,7,7,5,2,2}$ [108] | $Y_{10,10,10,9,7,7,7,5,2,2,1,1,1}$ [108] |
| | [1,1,0,2,1,1,0,0,1,4] | [3,7,12,17,24,32,41,50,36,23,23] | $Y_{10,10,10,9,8,6,6,5,4,1}$ [192] | $Y_{10,10,10,9,8,6,6,5,4,1,1,1,1}$ [192] |
| | [1,1,0,3,0,0,0,2,0,3] | [3,7,12,17,25,33,41,49,36,23,23] | $Y_{10,10,10,9,8,6,6,6,2,2}$ [90] | $Y_{10,10,10,9,8,6,6,6,2,2,1,1,1}$ [90] |
| | [1,1,1,0,2,0,1,1,0,3] | [3,7,12,18,24,32,40,49,36,23,23] | $Y_{10,10,10,9,8,7,5,5,3,2}$ [216] | $Y_{10,10,10,9,8,7,5,5,3,2,1,1,1}$ [216] |
| | [1,2,0,0,0,3,0,1,0,3] | [3,7,13,19,25,31,40,49,36,23,23] | $Y_{10,10,10,9,8,8,4,4,4,2}$ [90] | $Y_{10,10,10,9,8,8,4,4,4,2,1,1,1}$ [90] |
| | [1,2,0,0,1,0,3,0,0,3] | [3,7,13,19,25,32,39,49,36,23,23] | $Y_{10,10,10,9,8,8,5,3,3,3}$ [96] | $Y_{10,10,10,9,8,8,5,3,3,3,1,1,1}$ [96] |
| | [1,4,0,1,0,0,0,0,2,5] | [2,5,12,19,27,35,43,51,36,23,23] | $Y_{10,10,9,8,8,8,8,6,1,1}$ [72] | $Y_{10,10,9,8,8,8,8,6,1,1,1,1,1}$ [72] |
| | [2,0,0,1,1,2,0,1,0,3] | [3,8,13,18,24,31,40,49,36,23,23] | $Y_{10,10,10,9,9,6,5,4,4,2}$ [144] | $Y_{10,10,10,9,9,6,5,4,4,2,1,1,1}$ [144] |
| | [2,0,0,2,0,0,3,0,0,3] | [3,8,13,18,25,32,39,49,36,23,23] | $Y_{10,10,10,9,9,6,6,3,3,3}$ [64] | $Y_{10,10,10,9,9,6,6,3,3,3,1,1,1}$ [64] |
| | [2,0,1,0,0,2,2,0,0,3] | [3,8,13,19,25,31,39,49,36,23,23] | $Y_{10,10,10,9,9,7,4,4,3,3}$ [96] | $Y_{10,10,10,9,9,7,4,4,3,3,1,1,1}$ [96] |
| | [2,1,2,1,0,0,0,1,1,4] | [2,6,11,18,26,34,42,50,36,23,23] | $Y_{10,10,9,9,8,7,7,6,2,1}$ [160] | $Y_{10,10,9,9,8,7,7,6,2,1,1,1,1}$ [160] |
| | [2,2,0,1,1,0,1,0,1,4] | [2,6,12,18,25,33,41,50,36,23,23] | $Y_{10,10,9,9,8,8,6,5,3,1}$ [216] | $Y_{10,10,9,9,8,8,6,5,3,1,1,1,1}$ [216] |
| | [2,2,1,0,0,1,0,2,0,3] | [2,6,12,19,26,33,41,49,36,23,23] | $Y_{10,10,9,9,8,8,7,4,2,2}$ [144] | $Y_{10,10,9,9,8,8,7,4,2,2,1,1,1}$ [144] |
| | [3,0,1,1,0,2,0,0,1,4] | [2,7,12,18,25,32,41,50,36,23,23] | $Y_{10,10,9,9,9,7,6,4,4,1}$ [144] | $Y_{10,10,9,9,9,7,6,4,4,1,1,1,1}$ [144] |
| | [3,0,1,1,1,0,0,2,0,3] | [2,7,12,18,25,33,41,49,36,23,23] | $Y_{10,10,9,9,9,7,6,5,2,2}$ [144] | $Y_{10,10,9,9,9,7,6,5,2,2,1,1,1}$ [144] |
| | [3,0,2,0,0,0,2,1,0,3] | [2,7,12,19,26,33,40,49,36,23,23] | $Y_{10,10,9,9,9,7,7,3,3,2}$ [90] | $Y_{10,10,9,9,9,7,7,3,3,2,1,1,1}$ [90] |
| | [3,1,0,0,1,1,1,1,0,3] | [2,7,13,19,25,32,40,49,36,23,23] | $Y_{10,10,9,9,9,8,5,4,3,2}$ [192] | $Y_{10,10,9,9,9,8,5,4,3,2,1,1,1}$ [192] |
| | [4,1,1,1,0,0,0,0,2,5] | [1,6,12,19,27,35,43,51,36,23,23] | $Y_{10,9,9,9,9,8,7,6,1,1}$ [96] | $Y_{10,9,9,9,9,8,7,6,1,1,1,1,1}$ [96] |
| | [4,2,0,0,0,1,0,1,1,4] | [1,6,13,20,27,34,42,50,36,23,23] | $Y_{10,9,9,9,9,8,8,4,2,1}$ [120] | $Y_{10,9,9,9,9,8,8,4,2,1,1,1,1}$ [120] |
| | [5,0,0,1,1,0,0,1,1,4] | [1,7,13,19,26,34,42,50,36,23,23] | $Y_{10,9,9,9,9,9,6,5,2,1}$ [128] | $Y_{10,9,9,9,9,9,6,5,2,1,1,1,1}$ [128] |
| | [5,0,1,0,0,0,2,0,1,4] | [1,7,13,20,27,34,41,50,36,23,23] | $Y_{10,9,9,9,9,9,7,3,3,1}$ [90] | $Y_{10,9,9,9,9,9,7,3,3,1,1,1,1}$ [90] |
| | [5,1,0,0,0,0,0,3,0,3] | [1,7,14,21,28,35,42,49,36,23,23] | $Y_{10,9,9,9,9,9,8,2,2,2}$ [42] | $Y_{10,9,9,9,9,9,8,2,2,2,1,1,1}$ [42] |
| | [0,2,1,2,0,1,0,0,0,5] | [3,6,11,17,25,33,42,51,37,23,23] | $Y_{10,10,10,8,8,7,6,6,4}$ [90] | $Y_{10,10,10,8,8,7,6,6,4,1,1,1,1,1}$ [90] |
| | [0,3,0,0,3,0,0,0,0,5] | [3,6,12,18,24,33,42,51,37,23,23] | $Y_{10,10,10,8,8,8,5,5,5}$ [36] | $Y_{10,10,10,8,8,8,5,5,5,1,1,1,1,1}$ [36] |
| | [1,0,2,1,2,0,0,0,0,5] | [3,7,11,17,24,33,42,51,37,23,23] | $Y_{10,10,10,9,7,7,6,5,5}$ [72] | $Y_{10,10,10,9,7,7,6,5,5,1,1,1,1,1}$ [72] |
| | [1,3,2,0,0,0,0,1,0,5] | [2,5,11,19,27,35,43,51,37,23,23] | $Y_{10,10,9,8,8,8,7,7,2}$ [72] | $Y_{10,10,9,8,8,8,7,7,2,1,1,1,1,1}$ [72] |
| | [1,4,0,0,1,0,1,0,0,5] | [2,5,12,19,26,34,42,51,37,23,23] | $Y_{10,10,9,8,8,8,8,5,3}$ [96] | $Y_{10,10,9,8,8,8,8,5,3,1,1,1,1,1}$ [96] |
| | [2,1,2,0,1,1,0,0,0,5] | [2,6,11,18,25,33,42,51,37,23,23] | $Y_{10,10,9,9,8,7,7,5,4}$ [120] | $Y_{10,10,9,9,8,7,7,5,4,1,1,1,1,1}$ [120] |
| | [3,0,0,3,0,1,0,0,0,5] | [2,7,12,17,25,33,42,51,37,23,23] | $Y_{10,10,9,9,9,6,6,6,4}$ [60] | $Y_{10,10,9,9,9,6,6,6,4,1,1,1,1,1}$ [60] |
| | [3,0,1,0,3,0,0,0,0,5] | [2,7,12,18,24,33,42,51,37,23,23] | $Y_{10,10,9,9,9,7,5,5,5}$ [54] | $Y_{10,10,9,9,9,7,5,5,5,1,1,1,1,1}$ [54] |
| | [3,3,1,0,0,0,0,0,1,6] | [1,5,12,20,28,36,44,52,37,23,23] | $Y_{10,9,9,9,8,8,8,7,1}$ [56] | $Y_{10,9,9,9,8,8,8,7,1,1,1,1,1,1}$ [56] |
| | [4,1,1,0,1,0,1,0,0,5] | [1,6,12,19,26,34,42,51,37,23,23] | $Y_{10,9,9,9,9,8,7,5,3}$ [144] | $Y_{10,9,9,9,9,8,7,5,3,1,1,1,1,1}$ [144] |
| | [5,0,0,1,0,2,0,0,0,5] | [1,7,13,19,26,33,42,51,37,23,23] | $Y_{10,9,9,9,9,9,6,4,4}$ [60] | $Y_{10,9,9,9,9,9,6,4,4,1,1,1,1,1}$ [60] |
| | [7,0,0,1,0,0,0,0,0,7] | [0,7,14,21,29,37,45,53,38,23,23] | $Y_{9,9,9,9,9,9,9,6}$ [28] | $Y_{9,9,9,9,9,9,9,6,1,1,1,1,1,1}$ [28] |
| | [0,0,0,0,0,0,0,2,7,0] | [6,12,18,24,30,36,42,48,32,23,24] | $Y_{10,10,10,10,10,10,2,2,1,1,1,1,1,1,1}$ [13] | $Y_{10,10,10,10,10,10,2,2}$ [14] |
| | [1,0,0,0,0,1,0,0,8,1] | [5,11,17,23,29,35,42,49,32,23,24] | $Y_{10,10,10,10,10,9,4,1,1,1,1,1,1,1,1}$ [48] | $Y_{10,10,10,10,10,9,4,1}$ [48] |
| | [0,0,0,1,0,2,0,1,5,0] | [5,10,15,20,26,32,40,48,33,23,24] | $Y_{10,10,10,10,10,6,4,4,2,1,1,1,1,1}$ [67] | $Y_{10,10,10,10,10,6,4,4,2}$ [68] |
| | [0,0,1,0,0,0,3,0,5,0] | [5,10,15,21,27,33,39,48,33,23,24] | $Y_{10,10,10,10,10,7,3,3,3,1,1,1,1,1}$ [40] | $Y_{10,10,10,10,10,7,3,3,3}$ [40] |
| | [0,1,2,0,0,0,1,0,6,1] | [4,8,13,20,27,34,41,49,33,23,24] | $Y_{10,10,10,10,8,7,7,3,1,1,1,1,1,1}$ [90] | $Y_{10,10,10,10,8,7,7,3,1}$ [90] |
| | [0,2,0,0,1,1,0,0,6,1] | [4,8,14,20,26,33,41,49,33,23,24] | $Y_{10,10,10,10,8,8,5,4,1,1,1,1,1,1}$ [96] | $Y_{10,10,10,10,8,8,5,4,1}$ [96] |
| | [0,2,0,1,0,0,0,2,5,0] | [4,8,14,20,27,34,41,48,33,23,24] | $Y_{10,10,10,10,8,8,6,2,2,1,1,1,1,1}$ [67] | $Y_{10,10,10,10,8,8,6,2,2}$ [68] |
| | [1,0,0,2,0,1,0,0,6,1] | [4,9,14,19,26,33,41,49,33,23,24] | $Y_{10,10,10,10,9,6,6,4,1,1,1,1,1,1}$ [96] | $Y_{10,10,10,10,9,6,6,4,1}$ [96] |
| | [1,0,1,0,1,0,1,1,5,0] | [4,9,14,20,26,33,40,48,33,23,24] | $Y_{10,10,10,10,9,7,5,3,2,1,1,1,1,1}$ [162] | $Y_{10,10,10,10,9,7,5,3,2}$ [162] |
| | [2,1,0,1,0,0,1,0,6,1] | [3,8,14,20,27,34,41,49,33,23,24] | $Y_{10,10,10,9,9,8,6,3,1,1,1,1,1,1}$ [144] | $Y_{10,10,10,9,9,8,6,3,1}$ [144] |
| | [3,0,0,0,0,2,0,0,6,1] | [3,9,15,21,27,33,41,49,33,23,24] | $Y_{10,10,10,9,9,9,4,4,1,1,1,1,1,1}$ [48] | $Y_{10,10,10,9,9,9,4,4,1}$ [48] |
| | [3,0,0,0,1,0,0,2,5,0] | [3,9,15,21,27,34,41,48,33,23,24] | $Y_{10,10,10,9,9,9,5,2,2,1,1,1,1,1}$ [60] | $Y_{10,10,10,9,9,9,5,2,2}$ [60] |
| | [0,0,0,1,0,0,4,0,3,0] | [5,10,15,20,26,32,38,48,34,23,24] | $Y_{10,10,10,10,10,6,3,3,3,3,1,1,1}$ [40] | $Y_{10,10,10,10,10,6,3,3,3,3}$ [40] |
| | [0,0,2,1,0,1,1,0,4,1] | [4,8,12,18,25,32,40,49,34,23,24] | $Y_{10,10,10,10,7,7,6,4,3,1,1,1,1}$ [144] | $Y_{10,10,10,10,7,7,6,4,3,1}$ [144] |
| | [0,0,3,0,0,0,1,2,3,0] | [4,8,12,19,26,33,40,48,34,23,24] | $Y_{10,10,10,10,7,7,7,3,2,2,1,1,1}$ [60] | $Y_{10,10,10,10,7,7,7,3,2,2}$ [60] |
| | [0,1,0,1,2,0,1,0,4,1] | [4,8,13,18,24,32,40,49,34,23,24] | $Y_{10,10,10,10,8,6,5,5,3,1,1,1,1}$ [162] | $Y_{10,10,10,10,8,6,5,5,3,1}$ [162] |
| | [0,1,0,2,0,1,0,2,3,0] | [4,8,13,18,25,32,40,48,34,23,24] | $Y_{10,10,10,10,8,6,6,4,2,2,1,1,1}$ [121] | $Y_{10,10,10,10,8,6,6,4,2,2}$ [122] |
| | [0,1,1,0,0,3,0,0,4,1] | [4,8,13,19,25,31,40,49,34,23,24] | $Y_{10,10,10,10,8,7,4,4,4,1,1,1,1}$ [96] | $Y_{10,10,10,10,8,7,4,4,4,1}$ [96] |
| | [0,1,1,0,1,0,2,1,3,0] | [4,8,13,19,25,32,39,48,34,23,24] | $Y_{10,10,10,10,8,7,5,3,3,2,1,1,1}$ [162] | $Y_{10,10,10,10,8,7,5,3,3,2}$ [162] |
| | [0,3,1,0,1,0,0,0,5,2] | [3,6,12,19,26,34,42,50,34,23,24] | $Y_{10,10,10,8,8,8,7,5,1,1,1,1,1}$ [90] | $Y_{10,10,10,8,8,8,7,5,1,1}$ [90] |
| | [0,4,0,0,0,0,1,1,4,1] | [3,6,13,20,27,34,41,49,34,23,24] | $Y_{10,10,10,8,8,8,8,3,2,1,1,1,1}$ [72] | $Y_{10,10,10,8,8,8,8,3,2,1}$ [72] |
| | [1,0,0,0,2,2,0,0,4,1] | [4,9,14,19,24,31,40,49,34,23,24] | $Y_{10,10,10,10,9,5,5,4,4,1,1,1,1}$ [80] | $Y_{10,10,10,10,9,5,5,4,4,1}$ [80] |
| | [1,0,0,0,3,0,0,2,3,0] | [4,9,14,19,24,32,40,48,34,23,24] | $Y_{10,10,10,10,9,5,5,5,2,2,1,1,1}$ [60] | $Y_{10,10,10,10,9,5,5,5,2,2}$ [60] |
| | [1,0,0,1,0,2,1,1,3,0] | [4,9,14,19,25,31,39,48,34,23,24] | $Y_{10,10,10,10,9,6,4,4,3,2,1,1,1}$ [144] | $Y_{10,10,10,10,9,6,4,4,3,2}$ [144] |
| | [1,1,1,1,1,0,0,1,4,1] | [3,7,12,18,25,33,41,49,34,23,24] | $Y_{10,10,10,9,8,7,6,5,2,1,1,1,1}$ [256] | $Y_{10,10,10,9,8,7,6,5,2,1}$ [256] |
| | [1,1,2,0,0,0,2,0,4,1] | [3,7,12,19,26,33,40,49,34,23,24] | $Y_{10,10,10,9,8,7,7,3,3,1,1,1,1}$ [120] | $Y_{10,10,10,9,8,7,7,3,3,1}$ [120] |
| | [1,2,0,0,1,1,1,0,4,1] | [3,7,13,19,25,32,40,49,34,23,24] | $Y_{10,10,10,9,8,8,5,4,3,1,1,1,1}$ [192] | $Y_{10,10,10,9,8,8,5,4,3,1}$ [192] |
| | [1,2,0,1,0,0,1,2,3,0] | [3,7,13,19,26,33,40,48,34,23,24] | $Y_{10,10,10,9,8,8,6,3,2,2,1,1,1}$ [144] | $Y_{10,10,10,9,8,8,6,3,2,2}$ [144] |
| | [2,0,0,2,0,1,1,0,4,1] | [3,8,13,18,25,32,40,49,34,23,24] | $Y_{10,10,10,9,9,6,6,4,3,1,1,1,1}$ [144] | $Y_{10,10,10,9,9,6,6,4,3,1}$ [144] |
| | [2,0,1,0,1,1,0,2,3,0] | [3,8,13,19,25,32,40,48,34,23,24] | $Y_{10,10,10,9,9,7,5,4,2,2,1,1,1}$ [162] | $Y_{10,10,10,9,9,7,5,4,2,2}$ [162] |
| | [2,1,0,0,0,1,2,1,3,0] | [3,8,14,20,26,32,39,48,34,23,24] | $Y_{10,10,10,9,9,8,4,3,3,2,1,1,1}$ [120] | $Y_{10,10,10,9,9,8,4,3,3,2}$ [120] |
| | [2,3,0,0,0,1,0,0,5,2] | [2,6,13,20,27,34,42,50,34,23,24] | $Y_{10,10,9,9,8,8,8,4,1,1,1,1,1}$ [80] | $Y_{10,10,9,9,8,8,8,4,1,1}$ [80] |
| | [3,0,2,0,1,0,0,0,5,2] | [2,7,12,19,26,34,42,50,34,23,24] | $Y_{10,10,9,9,9,7,7,5,1,1,1,1,1}$ [90] | $Y_{10,10,9,9,9,7,7,5,1,1}$ [90] |
| | [3,1,0,1,0,1,0,1,4,1] | [2,7,13,19,26,33,41,49,34,23,24] | $Y_{10,10,9,9,9,8,6,4,2,1,1,1,1}$ [216] | $Y_{10,10,9,9,9,8,6,4,2,1}$ [216] |
| | [4,0,0,0,1,0,2,0,4,1] | [2,8,14,20,26,33,40,49,34,23,24] | $Y_{10,10,9,9,9,9,5,3,3,1,1,1,1}$ [90] | $Y_{10,10,9,9,9,9,5,3,3,1}$ [90] |
| | [4,0,0,1,0,0,0,3,3,0] | [2,8,14,20,27,34,41,48,34,23,24] | $Y_{10,10,9,9,9,9,6,2,2,2,1,1,1}$ [60] | $Y_{10,10,9,9,9,9,6,2,2,2}$ [60] |
| | [6,0,0,0,0,0,0,1,5,2] | [1,8,15,22,29,36,43,50,34,23,24] | $Y_{10,9,9,9,9,9,9,2,1,1,1,1,1}$ [32] | $Y_{10,9,9,9,9,9,9,2,1,1}$ [32] |

| | | | | |
|---|---|---|---|---|
| | [0,0,0,0,0,4,0,2,1,0] | [5,10,15,20,25,30,39,48,35,23,24] | $Y_{10,10,10,10,10,4,4,4,4,2,2,1}$ [31] | $Y_{10,10,10,10,10,4,4,4,4,2,2}$ [32] |
| | [0,0,1,1,3,0,0,0,3,2] | [4,8,12,17,23,32,41,50,35,23,24] | $Y_{10,10,10,10,7,6,5,5,5,1,1,1}$ [80] | $Y_{10,10,10,10,7,6,5,5,5,1,1}$ [80] |
| | [0,0,1,2,0,2,0,1,2,1] | [4,8,12,17,24,31,40,49,35,23,24] | $Y_{10,10,10,10,7,6,6,4,4,2,1,1}$ [144] | $Y_{10,10,10,10,7,6,6,4,4,2,1}$ [144] |
| | [0,0,2,0,1,1,2,0,2,1] | [4,8,12,18,24,31,39,49,35,23,24] | $Y_{10,10,10,10,7,7,5,4,3,3,1,1}$ [144] | $Y_{10,10,10,10,7,7,5,4,3,3,1}$ [144] |
| | [0,0,2,0,2,0,0,3,1,0] | [4,8,12,18,24,32,40,48,35,23,24] | $Y_{10,10,10,10,7,7,5,5,2,2,2,1}$ [72] | $Y_{10,10,10,10,7,7,5,5,2,2,2}$ [72] |
| | [0,0,2,1,0,0,2,2,1,0] | [4,8,12,18,25,32,39,48,35,23,24] | $Y_{10,10,10,10,7,7,6,3,3,2,2,1}$ [96] | $Y_{10,10,10,10,7,7,6,3,3,2,2}$ [96] |
| | [0,1,0,0,3,1,0,1,2,1] | [4,8,13,18,23,31,40,49,35,23,24] | $Y_{10,10,10,10,8,5,5,5,4,2,1,1}$ [144] | $Y_{10,10,10,10,8,5,5,5,4,2,1}$ [144] |
| | [0,1,0,1,1,1,1,2,1,0] | [4,8,13,18,24,31,39,48,35,23,24] | $Y_{10,10,10,10,8,6,5,4,3,2,2,1}$ [216] | $Y_{10,10,10,10,8,6,5,4,3,2,2}$ [216] |
| | [0,2,0,0,0,0,4,1,1,0] | [4,8,14,20,26,32,38,48,35,23,24] | $Y_{10,10,10,10,8,8,3,3,3,3,2,1}$ [54] | $Y_{10,10,10,10,8,8,3,3,3,3,2}$ [54] |
| | [0,2,1,2,0,0,1,0,3,2] | [3,6,11,17,25,33,41,50,35,23,24] | $Y_{10,10,10,8,8,7,6,6,3,1,1,1}$ [144] | $Y_{10,10,10,8,8,7,6,6,3,1,1}$ [144] |
| | [0,2,2,0,0,2,0,0,3,2] | [3,6,11,18,25,32,41,50,35,23,24] | $Y_{10,10,10,8,8,7,7,4,4,1,1,1}$ [96] | $Y_{10,10,10,8,8,7,7,4,4,1,1}$ [96] |
| | [0,2,2,0,1,0,0,2,2,1] | [3,6,11,18,25,33,41,49,35,23,24] | $Y_{10,10,10,8,8,7,7,5,2,2,1,1}$ [144] | $Y_{10,10,10,8,8,7,7,5,2,2,1}$ [144] |
| | [0,3,0,0,2,1,0,0,3,2] | [3,6,12,18,24,32,41,50,35,23,24] | $Y_{10,10,10,8,8,8,5,5,4,1,1,1}$ [96] | $Y_{10,10,10,8,8,8,5,5,4,1,1}$ [96] |
| | [0,3,0,1,0,1,1,1,2,1] | [3,6,12,18,25,32,40,49,35,23,24] | $Y_{10,10,10,8,8,8,6,4,3,2,1,1}$ [216] | $Y_{10,10,10,8,8,8,6,4,3,2,1}$ [216] |
| | [0,4,0,0,0,0,0,4,1,0] | [3,6,13,20,27,34,41,48,35,23,24] | $Y_{10,10,10,8,8,8,8,2,2,2,2,1}$ [31] | $Y_{10,10,10,8,8,8,8,2,2,2,2}$ [32] |
| | [1,0,0,0,1,3,1,0,2,1] | [4,9,14,19,24,30,39,49,35,23,24] | $Y_{10,10,10,10,9,5,4,4,4,3,1,1}$ [120] | $Y_{10,10,10,10,9,5,4,4,4,3,1}$ [120] |
| | [1,0,0,1,0,1,3,1,1,0] | [4,9,14,19,25,31,38,48,35,23,24] | $Y_{10,10,10,10,9,6,4,3,3,3,2,1}$ [144] | $Y_{10,10,10,10,9,6,4,3,3,3,2}$ [144] |
| | [1,0,2,1,1,1,0,0,3,2] | [3,7,11,17,24,32,41,50,35,23,24] | $Y_{10,10,10,9,7,7,6,5,4,1,1,1}$ [192] | $Y_{10,10,10,9,7,7,6,5,4,1,1}$ [192] |
| | [1,0,2,2,0,0,0,2,2,1] | [3,7,11,17,25,33,41,49,35,23,24] | $Y_{10,10,10,9,7,7,6,6,2,2,1,1}$ [120] | $Y_{10,10,10,9,7,7,6,6,2,2,1}$ [120] |
| | [1,0,3,0,0,1,1,1,2,1] | [3,7,11,18,25,32,40,49,35,23,24] | $Y_{10,10,10,9,7,7,7,4,3,2,1,1}$ [192] | $Y_{10,10,10,9,7,7,7,4,3,2,1}$ [192] |
| | [1,1,0,2,1,0,1,1,2,1] | [3,7,12,17,24,32,40,49,35,23,24] | $Y_{10,10,10,9,8,6,6,5,3,2,1,1}$ [288] | $Y_{10,10,10,9,8,6,6,5,3,2,1}$ [288] |
| | [1,1,1,0,1,2,0,1,2,1] | [3,7,12,18,24,31,40,49,35,23,24] | $Y_{10,10,10,9,8,7,5,4,4,2,1,1}$ [288] | $Y_{10,10,10,9,8,7,5,4,4,2,1}$ [288] |
| | [1,1,1,1,0,0,3,0,2,1] | [3,7,12,18,25,32,39,49,35,23,24] | $Y_{10,10,10,9,8,7,6,3,3,3,1,1}$ [192] | $Y_{10,10,10,9,8,7,6,3,3,3,1}$ [192] |
| | [1,1,1,1,0,1,0,3,1,0] | [3,7,12,18,25,32,40,48,35,23,24] | $Y_{10,10,10,9,8,7,6,4,2,2,2,1}$ [216] | $Y_{10,10,10,9,8,7,6,4,2,2,2}$ [216] |
| | [1,2,0,0,0,2,2,0,2,1] | [3,7,13,19,25,31,39,49,35,23,24] | $Y_{10,10,10,9,8,8,4,4,3,3,1,1}$ [120] | $Y_{10,10,10,9,8,8,4,4,3,3,1}$ [120] |
| | [1,2,0,0,1,0,2,2,1,0] | [3,7,13,19,25,32,39,48,35,23,24] | $Y_{10,10,10,9,8,8,5,3,3,2,2,1}$ [144] | $Y_{10,10,10,9,8,8,5,3,3,2,2}$ [144] |
| | [1,3,2,0,0,0,0,0,4,3] | [2,5,11,19,27,35,43,51,35,23,24] | $Y_{10,10,9,8,8,8,7,7,1,1,1,1}$ [56] | $Y_{10,10,9,8,8,8,7,7,1,1,1}$ [56] |
| | [1,4,0,0,1,0,0,1,3,2] | [2,5,12,19,26,34,42,50,35,23,24] | $Y_{10,10,9,8,8,8,8,5,2,1,1,1}$ [128] | $Y_{10,10,9,8,8,8,8,5,2,1,1}$ [128] |
| | [2,0,0,0,4,0,0,0,3,2] | [3,8,13,18,23,32,41,50,35,23,24] | $Y_{10,10,10,9,9,5,5,5,5,1,1,1}$ [50] | $Y_{10,10,10,9,9,5,5,5,5,1,1}$ [50] |
| | [2,0,0,1,1,1,2,0,2,1] | [3,8,13,18,24,31,39,49,35,23,24] | $Y_{10,10,10,9,9,6,5,4,3,3,1,1}$ [192] | $Y_{10,10,10,9,9,6,5,4,3,3,1}$ [192] |
| | [2,0,0,1,2,0,0,3,1,0] | [3,8,13,18,24,32,40,48,35,23,24] | $Y_{10,10,10,9,9,6,5,5,2,2,2,1}$ [96] | $Y_{10,10,10,9,9,6,5,5,2,2,2}$ [96] |
| | [2,0,0,2,0,0,2,2,1,0] | [3,8,13,18,25,32,39,48,35,23,24] | $Y_{10,10,10,9,9,6,6,3,3,2,2,1}$ [96] | $Y_{10,10,10,9,9,6,6,3,3,2,2}$ [96] |
| | [2,0,1,0,0,2,1,2,1,0] | [3,8,13,19,25,31,39,48,35,23,24] | $Y_{10,10,10,9,9,7,4,4,3,2,2,1}$ [144] | $Y_{10,10,10,9,9,7,4,4,3,2,2}$ [144] |
| | [2,1,2,0,1,0,1,0,3,2] | [2,6,11,18,25,33,41,50,35,23,24] | $Y_{10,10,9,9,8,7,7,5,3,1,1,1}$ [216] | $Y_{10,10,9,9,8,7,7,5,3,1,1}$ [216] |
| | [2,2,0,1,0,2,0,0,3,2] | [2,6,12,18,25,32,41,50,35,23,24] | $Y_{10,10,9,9,8,8,6,4,4,1,1,1}$ [144] | $Y_{10,10,9,9,8,8,6,4,4,1,1}$ [144] |
| | [2,2,0,1,1,0,0,2,2,1] | [2,6,12,18,25,33,41,49,35,23,24] | $Y_{10,10,9,9,8,8,6,5,2,2,1,1}$ [192] | $Y_{10,10,9,9,8,8,6,5,2,2,1}$ [192] |
| | [2,2,1,0,0,0,2,1,2,1] | [2,6,12,19,26,33,40,49,35,23,24] | $Y_{10,10,9,9,8,8,7,3,3,2,1,1}$ [160] | $Y_{10,10,9,9,8,8,7,3,3,2,1}$ [160] |
| | [3,0,0,3,0,0,1,0,3,2] | [2,7,12,17,25,33,41,50,35,23,24] | $Y_{10,10,9,9,9,6,6,6,3,1,1,1}$ [96] | $Y_{10,10,9,9,9,6,6,6,3,1,1}$ [96] |
| | [3,0,1,0,2,1,0,0,3,2] | [2,7,12,18,24,32,41,50,35,23,24] | $Y_{10,10,9,9,9,7,5,5,4,1,1,1}$ [144] | $Y_{10,10,9,9,9,7,5,5,4,1,1}$ [144] |
| | [3,0,1,1,0,1,1,1,2,1] | [2,7,12,18,25,32,40,49,35,23,24] | $Y_{10,10,9,9,9,7,6,4,3,2,1,1}$ [288] | $Y_{10,10,9,9,9,7,6,4,3,2,1}$ [288] |
| | [3,1,0,1,0,0,1,3,1,0] | [2,7,13,19,26,33,40,48,35,23,24] | $Y_{10,10,9,9,9,8,6,3,2,2,2,1}$ [144] | $Y_{10,10,9,9,9,8,6,3,2,2,2}$ [144] |
| | [4,0,0,0,0,1,3,0,2,1] | [2,8,14,20,26,32,39,49,35,23,24] | $Y_{10,10,9,9,9,9,4,3,3,3,1,1}$ [72] | $Y_{10,10,9,9,9,9,4,3,3,3,1}$ [72] |
| | [4,0,0,0,0,2,0,3,1,0] | [2,8,14,20,26,32,40,48,35,23,24] | $Y_{10,10,9,9,9,9,4,4,2,2,2,1}$ [54] | $Y_{10,10,9,9,9,9,4,4,2,2,2}$ [54] |
| | [4,1,1,0,1,0,0,1,3,2] | [1,6,12,19,26,34,42,50,35,23,24] | $Y_{10,9,9,9,9,8,7,5,2,1,1,1}$ [192] | $Y_{10,9,9,9,9,8,7,5,2,1,1}$ [192] |
| | [4,2,0,0,0,0,2,0,3,2] | [1,6,13,20,27,34,41,50,35,23,24] | $Y_{10,9,9,9,9,8,8,3,3,1,1,1}$ [72] | $Y_{10,9,9,9,9,8,8,3,3,1,1}$ [72] |
| | [5,0,0,1,0,1,1,0,3,2] | [1,7,13,19,26,33,41,50,35,23,24] | $Y_{10,9,9,9,9,9,6,4,3,1,1,1}$ [144] | $Y_{10,9,9,9,9,9,6,4,3,1,1}$ [144] |
| | [5,0,1,0,0,0,1,2,2,1] | [1,7,13,20,27,34,41,49,35,23,24] | $Y_{10,9,9,9,9,9,7,3,2,2,1,1}$ [120] | $Y_{10,9,9,9,9,9,7,3,2,2,1}$ [120] |
| | [0,0,0,3,2,0,0,1,1,2] | [4,8,12,16,23,32,41,50,36,23,24] | $Y_{10,10,10,10,6,6,6,5,5,2,1}$ [80] | $Y_{10,10,10,10,6,6,6,5,5,2,1,1}$ [80] |
| | [0,0,0,4,0,0,2,0,1,2] | [4,8,12,16,24,32,40,50,36,23,24] | $Y_{10,10,10,10,6,6,6,6,3,3,1}$ [60] | $Y_{10,10,10,10,6,6,6,6,3,3,1,1}$ [60] |
| | [0,0,1,1,2,1,0,2,0,1] | [4,8,12,17,23,31,40,49,36,23,24] | $Y_{10,10,10,10,7,6,5,5,4,2,2}$ [144] | $Y_{10,10,10,10,7,6,5,5,4,2,2,1}$ [144] |
| | [0,0,1,2,0,1,2,1,0,1] | [4,8,12,17,24,31,39,49,36,23,24] | $Y_{10,10,10,10,7,6,6,4,3,3,2}$ [144] | $Y_{10,10,10,10,7,6,6,4,3,3,2,1}$ [144] |
| | [0,0,2,0,0,4,0,0,1,2] | [4,8,12,18,24,30,40,50,36,23,24] | $Y_{10,10,10,10,7,7,4,4,4,4,1}$ [64] | $Y_{10,10,10,10,7,7,4,4,4,4,1,1}$ [64] |
| | [0,1,0,0,2,3,0,0,1,2] | [4,8,13,18,23,30,40,50,36,23,24] | $Y_{10,10,10,10,8,5,5,4,4,4,1}$ [96] | $Y_{10,10,10,10,8,5,5,4,4,4,1,1}$ [96] |
| | [0,1,0,0,3,0,2,1,0,1] | [4,8,13,18,23,31,39,49,36,23,24] | $Y_{10,10,10,10,8,5,5,5,3,3,2}$ [108] | $Y_{10,10,10,10,8,5,5,5,3,3,2,1}$ [108] |
| | [0,1,0,1,0,3,1,1,0,1] | [4,8,13,18,24,30,39,49,36,23,24] | $Y_{10,10,10,10,8,6,4,4,4,3,2}$ [162] | $Y_{10,10,10,10,8,6,4,4,4,3,2,1}$ [162] |
| | [0,1,1,0,0,1,4,0,0,1] | [4,8,13,19,25,31,38,49,36,23,24] | $Y_{10,10,10,10,8,7,4,3,3,3,3}$ [96] | $Y_{10,10,10,10,8,7,4,3,3,3,3,1}$ [96] |
| | [0,1,3,0,2,0,0,0,2,3] | [3,6,10,17,24,33,42,51,36,23,24] | $Y_{10,10,10,8,7,7,7,5,5,1,1}$ [90] | $Y_{10,10,10,8,7,7,7,5,5,1,1,1}$ [90] |
| | [0,1,3,1,0,0,1,1,1,2] | [3,6,10,17,25,33,41,50,36,23,24] | $Y_{10,10,10,8,7,7,7,6,3,2,1}$ [192] | $Y_{10,10,10,8,7,7,7,6,3,2,1,1}$ [192] |
| | [0,2,0,3,1,0,0,0,2,3] | [3,6,11,16,24,33,42,51,36,23,24] | $Y_{10,10,10,8,8,6,6,6,5,1,1}$ [90] | $Y_{10,10,10,8,8,6,6,6,5,1,1,1}$ [90] |
| | [0,2,1,1,1,0,2,0,1,2] | [3,6,11,17,24,32,40,50,36,23,24] | $Y_{10,10,10,8,8,7,6,5,3,3,1}$ [216] | $Y_{10,10,10,8,8,7,6,5,3,3,1,1}$ [216] |
| | [0,2,1,2,0,0,0,3,0,1] | [3,6,11,17,25,33,41,49,36,23,24] | $Y_{10,10,10,8,8,7,6,6,2,2,2}$ [90] | $Y_{10,10,10,8,8,7,6,6,2,2,2,1}$ [90] |
| | [0,2,2,0,0,1,1,2,0,1] | [3,6,11,18,25,32,40,49,36,23,24] | $Y_{10,10,10,8,8,7,7,4,3,2,2}$ [144] | $Y_{10,10,10,8,8,7,7,4,3,2,2,1}$ [144] |
| | [0,3,0,0,1,2,1,0,1,2] | [3,6,12,18,24,31,40,50,36,23,24] | $Y_{10,10,10,8,8,8,5,4,4,3,1}$ [144] | $Y_{10,10,10,8,8,8,5,4,4,3,1,1}$ [144] |
| | [0,3,0,0,2,0,1,2,0,1] | [3,6,12,18,24,32,40,49,36,23,24] | $Y_{10,10,10,8,8,8,5,5,3,2,2}$ [108] | $Y_{10,10,10,8,8,8,5,5,3,2,2,1}$ [108] |
| | [1,0,0,0,2,0,4,0,0,1] | [4,9,14,19,24,31,38,49,36,23,24] | $Y_{10,10,10,10,9,5,5,3,3,3,3}$ [60] | $Y_{10,10,10,10,9,5,5,3,3,3,3,1}$ [60] |
| | [1,0,1,3,0,1,0,1,1,2] | [3,7,11,16,24,32,41,50,36,23,24] | $Y_{10,10,10,9,7,6,6,6,4,2,1}$ [216] | $Y_{10,10,10,9,7,6,6,6,4,2,1,1}$ [216] |
| | [1,0,2,0,3,0,0,1,1,2] | [3,7,11,17,23,32,41,50,36,23,24] | $Y_{10,10,10,9,7,7,5,5,5,2,1}$ [144] | $Y_{10,10,10,9,7,7,5,5,5,2,1,1}$ [144] |
| | [1,0,2,1,0,2,1,0,1,2] | [3,7,11,17,24,31,40,50,36,23,24] | $Y_{10,10,10,9,7,7,6,4,4,3,1}$ [216] | $Y_{10,10,10,9,7,7,6,4,4,3,1,1}$ [216] |
| | [1,0,2,1,1,0,1,2,0,1] | [3,7,11,17,24,32,40,49,36,23,24] | $Y_{10,10,10,9,7,7,6,5,3,2,2}$ [216] | $Y_{10,10,10,9,7,7,6,5,3,2,2,1}$ [216] |
| | [1,1,0,1,2,1,1,0,1,2] | [3,7,12,17,23,31,40,50,36,23,24] | $Y_{10,10,10,9,8,6,5,5,4,3,1}$ [288] | $Y_{10,10,10,9,8,6,5,5,4,3,1,1}$ [288] |
| | [1,1,0,2,0,2,0,2,0,1] | [3,7,12,17,24,31,40,49,36,23,24] | $Y_{10,10,10,9,8,6,6,4,4,2,2}$ [162] | $Y_{10,10,10,9,8,6,6,4,4,2,2,1}$ [162] |

| | | | | |
|---|---|---|---|---|
| | [1,1,1,0,1,1,2,1,0,1] | [3,7,12,18,24,31,39,49,36,23,24] | $Y_{10,10,10,9,8,7,5,4,3,3,2}$ [288] | $Y_{10,10,10,9,8,7,5,4,3,3,2,1}$ [288] |
| | [1,2,3,0,0,0,1,0,2,3] | [2,5,10,18,26,34,42,51,36,23,24] | $Y_{10,10,9,8,8,7,7,7,3,1,1}$ [120] | $Y_{10,10,9,8,8,7,7,7,3,1,1,1}$ [120] |
| | [1,3,0,2,0,1,0,0,2,3] | [2,5,11,17,25,33,42,51,36,23,24] | $Y_{10,10,9,8,8,8,6,6,4,1,1}$ [144] | $Y_{10,10,9,8,8,8,6,6,4,1,1,1}$ [144] |
| | [1,3,1,0,1,0,1,1,1,2] | [2,5,11,18,25,33,41,50,36,23,24] | $Y_{10,10,9,8,8,8,7,5,3,2,1}$ [288] | $Y_{10,10,9,8,8,8,7,5,3,2,1,1}$ [288] |
| | [2,0,0,0,3,1,0,2,0,1] | [3,8,13,18,23,31,40,49,36,23,24] | $Y_{10,10,10,9,9,5,5,5,4,2,2}$ [90] | $Y_{10,10,10,9,9,5,5,5,4,2,2,1}$ [90] |
| | [2,0,0,1,0,4,0,0,1,2] | [3,8,13,18,24,30,40,50,36,23,24] | $Y_{10,10,10,9,9,6,4,4,4,4,1}$ [96] | $Y_{10,10,10,9,9,6,4,4,4,4,1,1}$ [96] |
| | [2,0,3,1,0,1,0,0,2,3] | [2,6,10,17,25,33,42,51,36,23,24] | $Y_{10,10,9,9,7,7,7,6,4,1,1}$ [144] | $Y_{10,10,9,9,7,7,7,6,4,1,1,1}$ [144] |
| | [2,0,4,0,0,0,0,2,1,2] | [2,6,10,18,26,34,42,50,36,23,24] | $Y_{10,10,9,9,7,7,7,7,2,2,1}$ [72] | $Y_{10,10,9,9,7,7,7,7,2,2,1,1}$ [72] |
| | [2,1,0,0,0,0,5,0,0,1] | [3,8,14,20,26,32,38,49,36,23,24] | $Y_{10,10,10,9,9,8,3,3,3,3,3}$ [48] | $Y_{10,10,10,9,9,8,3,3,3,3,3,1}$ [48] |
| | [2,1,1,1,1,1,0,1,1,2] | [2,6,11,17,24,32,41,50,36,23,24] | $Y_{10,10,9,9,8,7,6,5,4,2,1}$ [384] | $Y_{10,10,9,9,8,7,6,5,4,2,1,1}$ [384] |
| | [2,1,2,0,0,1,2,0,1,2] | [2,6,11,18,25,32,40,50,36,23,24] | $Y_{10,10,9,9,8,7,7,4,3,3,1}$ [192] | $Y_{10,10,9,9,8,7,7,4,3,3,1,1}$ [192] |
| | [2,1,2,0,1,0,0,3,0,1] | [2,6,11,18,25,33,41,49,36,23,24] | $Y_{10,10,9,9,8,7,7,5,2,2,2}$ [144] | $Y_{10,10,9,9,8,7,7,5,2,2,2,1}$ [144] |
| | [2,2,0,0,2,0,2,0,1,2] | [2,6,12,18,24,32,40,50,36,23,24] | $Y_{10,10,9,9,8,8,5,5,3,3,1}$ [144] | $Y_{10,10,9,9,8,8,5,5,3,3,1,1}$ [144] |
| | [2,2,0,1,0,1,1,2,0,1] | [2,6,12,18,25,32,40,49,36,23,24] | $Y_{10,10,9,9,8,8,6,4,3,2,2}$ [216] | $Y_{10,10,9,9,8,8,6,4,3,2,2,1}$ [216] |
| | [3,0,0,2,1,0,2,0,1,2] | [2,7,12,17,24,32,40,50,36,23,24] | $Y_{10,10,9,9,9,6,6,5,3,3,1}$ [144] | $Y_{10,10,9,9,9,6,6,5,3,3,1,1}$ [144] |
| | [3,0,1,0,1,2,1,0,1,2] | [2,7,12,18,24,31,40,50,36,23,24] | $Y_{10,10,9,9,9,7,5,4,4,3,1}$ [216] | $Y_{10,10,9,9,9,7,5,4,4,3,1,1}$ [216] |
| | [3,0,1,0,2,0,1,2,0,1] | [2,7,12,18,24,32,40,49,36,23,24] | $Y_{10,10,9,9,9,7,5,5,3,2,2}$ [162] | $Y_{10,10,9,9,9,7,5,5,3,2,2,1}$ [162] |
| | [3,1,0,0,0,3,0,2,0,1] | [2,7,13,19,25,31,40,49,36,23,24] | $Y_{10,10,9,9,9,8,4,4,4,2,2}$ [90] | $Y_{10,10,9,9,9,8,4,4,4,2,2,1}$ [90] |
| | [3,1,0,0,1,0,3,1,0,1] | [2,7,13,19,25,32,39,49,36,23,24] | $Y_{10,10,9,9,9,8,5,3,3,3,2}$ [144] | $Y_{10,10,9,9,9,8,5,3,3,3,2,1}$ [144] |
| | [3,2,1,1,0,0,1,0,2,3] | [1,5,11,18,26,34,42,51,36,23,24] | $Y_{10,9,9,9,8,8,7,6,3,1,1}$ [192] | $Y_{10,9,9,9,8,8,7,6,3,1,1,1}$ [192] |
| | [3,3,0,0,0,2,0,0,2,3] | [1,5,12,19,26,33,42,51,36,23,24] | $Y_{10,9,9,9,8,8,8,4,4,1,1}$ [80] | $Y_{10,9,9,9,8,8,8,4,4,1,1,1}$ [80] |
| | [3,3,0,0,1,0,0,2,1,2] | [1,5,12,19,26,34,42,50,36,23,24] | $Y_{10,9,9,9,8,8,8,5,2,2,1}$ [128] | $Y_{10,9,9,9,8,8,8,5,2,2,1,1}$ [128] |
| | [4,0,2,0,1,1,0,0,2,3] | [1,6,11,18,25,33,42,51,36,23,24] | $Y_{10,9,9,9,9,7,7,5,4,1,1}$ [144] | $Y_{10,9,9,9,9,7,7,5,4,1,1,1}$ [144] |
| | [4,0,2,1,0,0,0,2,1,2] | [1,6,11,18,26,34,42,50,36,23,24] | $Y_{10,9,9,9,9,7,7,6,2,2,1}$ [120] | $Y_{10,9,9,9,9,7,7,6,2,2,1,1}$ [120] |
| | [4,1,0,1,1,0,1,1,1,2] | [1,6,12,18,25,33,41,50,36,23,24] | $Y_{10,9,9,9,9,8,6,5,3,2,1}$ [288] | $Y_{10,9,9,9,9,8,6,5,3,2,1,1}$ [288] |
| | [4,2,0,0,0,0,1,3,0,1] | [1,6,13,20,27,34,41,49,36,23,24] | $Y_{10,9,9,9,9,8,8,3,2,2,2}$ [72] | $Y_{10,9,9,9,9,8,8,3,2,2,2,1}$ [72] |
| | [5,0,0,0,1,2,0,1,1,2] | [1,7,13,19,25,32,41,50,36,23,24] | $Y_{10,9,9,9,9,9,5,4,4,2,1}$ [120] | $Y_{10,9,9,9,9,9,5,4,4,2,1,1}$ [120] |
| | [5,0,0,1,0,0,3,0,1,2] | [1,7,13,19,26,33,40,50,36,23,24] | $Y_{10,9,9,9,9,9,6,3,3,3,1}$ [96] | $Y_{10,9,9,9,9,9,6,3,3,3,1,1}$ [96] |
| | [5,0,0,1,0,1,0,3,0,1] | [1,7,13,19,26,33,41,49,36,23,24] | $Y_{10,9,9,9,9,9,6,4,2,2,2}$ [108] | $Y_{10,9,9,9,9,9,6,4,2,2,2,1}$ [108] |
| | [6,0,2,0,0,0,0,0,3,4] | [0,6,12,20,28,36,44,52,36,23,24] | $Y_{9,9,9,9,9,9,7,7,1,1,1}$ [42] | $Y_{9,9,9,9,9,9,7,7,1,1,1,1}$ [42] |
| | [6,1,0,0,1,0,0,1,2,3] | [0,6,13,20,27,35,43,51,36,23,24] | $Y_{9,9,9,9,9,9,8,5,2,1,1}$ [128] | $Y_{9,9,9,9,9,9,8,5,2,1,1,1}$ [128] |
| | [7,0,0,0,0,0,2,0,2,3] | [0,7,14,21,28,35,42,51,36,23,24] | $Y_{9,9,9,9,9,9,9,3,3,1,1}$ [42] | $Y_{9,9,9,9,9,9,9,3,3,1,1,1}$ [42] |
| | [0,0,0,3,1,2,0,0,0,3] | [4,8,12,16,23,31,41,51,37,23,24] | $Y_{10,10,10,10,6,6,6,5,4,4}$ [50] | $Y_{10,10,10,10,6,6,6,5,4,4,1,1,1}$ [50] |
| | [0,1,2,2,1,0,0,1,0,3] | [3,6,10,16,24,33,42,51,37,23,24] | $Y_{10,10,10,8,7,7,6,6,5,2}$ [144] | $Y_{10,10,10,8,7,7,6,6,5,2,1,1,1}$ [144] |
| | [0,1,3,0,1,1,1,0,0,3] | [3,6,10,17,24,32,41,51,37,23,24] | $Y_{10,10,10,8,7,7,7,5,4,3}$ [144] | $Y_{10,10,10,8,7,7,7,5,4,3,1,1,1}$ [144] |
| | [0,2,0,3,0,1,1,0,0,3] | [3,6,11,16,24,32,41,51,37,23,24] | $Y_{10,10,10,8,8,6,6,6,4,3}$ [108] | $Y_{10,10,10,8,8,6,6,6,4,3,1,1,1}$ [108] |
| | [0,2,1,0,3,0,1,0,0,3] | [3,6,11,17,23,32,41,51,37,23,24] | $Y_{10,10,10,8,8,7,5,5,5,3}$ [108] | $Y_{10,10,10,8,8,7,5,5,5,3,1,1,1}$ [108] |
| | [0,2,1,1,0,3,0,0,0,3] | [3,6,11,17,24,31,41,51,37,23,24] | $Y_{10,10,10,8,8,7,6,4,4,4}$ [90] | $Y_{10,10,10,8,8,7,6,4,4,4,1,1,1}$ [90] |
| | [0,5,0,1,0,1,0,0,1,4] | [2,4,11,18,26,34,43,52,37,23,24] | $Y_{10,10,8,8,8,8,8,6,4,1}$ [108] | $Y_{10,10,8,8,8,8,8,6,4,1,1,1,1}$ [108] |
| | [0,5,1,0,0,0,0,2,0,3] | [2,4,11,19,27,35,43,51,37,23,24] | $Y_{10,10,8,8,8,8,8,7,2,2}$ [54] | $Y_{10,10,8,8,8,8,8,7,2,2,1,1,1}$ [54] |
| | [1,0,1,2,2,0,1,0,0,3] | [3,7,11,16,23,32,41,51,37,23,24] | $Y_{10,10,10,9,7,6,6,5,5,3}$ [144] | $Y_{10,10,10,9,7,6,6,5,5,3,1,1,1}$ [144] |
| | [1,0,2,0,2,2,0,0,0,3] | [3,7,11,17,23,31,41,51,37,23,24] | $Y_{10,10,10,9,7,7,5,5,4,4}$ [90] | $Y_{10,10,10,9,7,7,5,5,4,4,1,1,1}$ [90] |
| | [1,2,2,1,0,1,0,1,0,3] | [2,5,10,17,25,33,42,51,37,23,24] | $Y_{10,10,9,8,8,7,7,6,4,2}$ [216] | $Y_{10,10,9,8,8,7,7,6,4,2,1,1,1}$ [216] |
| | [1,3,0,1,2,0,0,1,0,3] | [2,5,11,17,24,33,42,51,37,23,24] | $Y_{10,10,9,8,8,8,6,5,5,2}$ [144] | $Y_{10,10,9,8,8,8,6,5,5,2,1,1,1}$ [144] |
| | [1,3,0,2,0,0,2,0,0,3] | [2,5,11,17,25,33,41,51,37,23,24] | $Y_{10,10,9,8,8,8,6,6,3,3}$ [96] | $Y_{10,10,9,8,8,8,6,6,3,3,1,1,1}$ [96] |
| | [1,3,1,0,0,2,1,0,0,3] | [2,5,11,18,25,32,41,51,37,23,24] | $Y_{10,10,9,8,8,8,7,4,4,3}$ [128] | $Y_{10,10,9,8,8,8,7,4,4,3,1,1,1}$ [128] |
| | [2,0,2,3,0,0,0,0,1,4] | [2,6,10,16,25,34,43,52,37,23,24] | $Y_{10,10,9,9,7,7,6,6,6,1}$ [72] | $Y_{10,10,9,9,7,7,6,6,6,1,1,1,1}$ [72] |
| | [2,0,3,0,2,0,0,1,0,3] | [2,6,10,17,24,33,42,51,37,23,24] | $Y_{10,10,9,9,7,7,7,5,5,2}$ [108] | $Y_{10,10,9,9,7,7,7,5,5,2,1,1,1}$ [108] |
| | [2,0,3,1,0,0,2,0,0,3] | [2,6,10,17,25,33,41,51,37,23,24] | $Y_{10,10,9,9,7,7,7,6,3,3}$ [96] | $Y_{10,10,9,9,7,7,7,6,3,3,1,1,1}$ [96] |
| | [2,1,0,3,1,0,0,1,0,3] | [2,6,11,16,24,33,42,51,37,23,24] | $Y_{10,10,9,9,8,6,6,6,5,2}$ [144] | $Y_{10,10,9,9,8,6,6,6,5,2,1,1,1}$ [144] |
| | [2,2,0,0,1,3,0,0,0,3] | [2,6,12,18,24,31,41,51,37,23,24] | $Y_{10,10,9,9,8,8,5,4,4,4}$ [80] | $Y_{10,10,9,9,8,8,5,4,4,4,1,1,1}$ [80] |
| | [2,4,1,0,0,0,1,0,1,4] | [1,4,11,19,27,35,43,52,37,23,24] | $Y_{10,9,9,8,8,8,8,7,3,1}$ [120] | $Y_{10,9,9,8,8,8,8,7,3,1,1,1,1}$ [120] |
| | [3,0,0,1,3,0,1,0,0,3] | [2,7,12,17,23,32,41,51,37,23,24] | $Y_{10,10,9,9,9,6,5,5,5,3}$ [96] | $Y_{10,10,9,9,9,6,5,5,5,3,1,1,1}$ [96] |
| | [3,0,0,2,0,3,0,0,0,3] | [2,7,12,17,24,31,41,51,37,23,24] | $Y_{10,10,9,9,9,6,6,4,4,4}$ [60] | $Y_{10,10,9,9,9,6,6,4,4,4,1,1,1}$ [60] |
| | [3,1,3,0,0,1,0,0,1,4] | [1,5,10,18,26,34,43,52,37,23,24] | $Y_{10,9,9,9,8,7,7,7,4,1}$ [128] | $Y_{10,9,9,9,8,7,7,7,4,1,1,1,1}$ [128] |
| | [3,2,0,2,1,0,0,0,1,4] | [1,5,11,17,25,34,43,52,37,23,24] | $Y_{10,9,9,9,8,8,6,6,5,1}$ [120] | $Y_{10,9,9,9,8,8,6,6,5,1,1,1,1}$ [120] |
| | [3,2,1,0,1,1,0,1,0,3] | [1,5,11,18,25,33,42,51,37,23,24] | $Y_{10,9,9,9,8,8,7,5,4,2}$ [216] | $Y_{10,9,9,9,8,8,7,5,4,2,1,1,1}$ [216] |
| | [3,3,0,0,0,1,2,0,0,3] | [1,5,12,19,26,33,41,51,37,23,24] | $Y_{10,9,9,9,8,8,8,4,3,3}$ [80] | $Y_{10,9,9,9,8,8,8,4,3,3,1,1,1}$ [80] |
| | [4,0,1,2,0,1,0,1,0,3] | [1,6,11,17,25,33,42,51,37,23,24] | $Y_{10,9,9,9,9,7,6,6,4,2}$ [162] | $Y_{10,9,9,9,9,7,6,6,4,2,1,1,1}$ [162] |
| | [4,0,2,0,1,0,2,0,0,3] | [1,6,11,18,25,33,41,51,37,23,24] | $Y_{10,9,9,9,9,7,7,5,3,3}$ [108] | $Y_{10,9,9,9,9,7,7,5,3,3,1,1,1}$ [108] |
| | [4,1,0,0,3,0,0,1,0,3] | [1,6,12,18,24,33,42,51,37,23,24] | $Y_{10,9,9,9,9,8,5,5,5,2}$ [96] | $Y_{10,9,9,9,9,8,5,5,5,2,1,1,1}$ [96] |
| | [4,1,0,1,0,2,1,0,0,3] | [1,6,12,18,25,32,41,51,37,23,24] | $Y_{10,9,9,9,9,8,6,4,4,3}$ [144] | $Y_{10,9,9,9,9,8,6,4,4,3,1,1,1}$ [144] |
| | [5,2,0,1,0,0,1,0,1,4] | [0,5,12,19,27,35,43,52,37,23,24] | $Y_{9,9,9,9,9,8,8,6,3,1}$ [144] | $Y_{9,9,9,9,9,8,8,6,3,1,1,1,1}$ [144] |
| | [6,0,1,0,1,1,0,0,1,4] | [0,6,12,19,26,34,43,52,37,23,24] | $Y_{9,9,9,9,9,9,7,5,4,1}$ [144] | $Y_{9,9,9,9,9,9,7,5,4,1,1,1,1}$ [144] |
| | [6,0,1,1,0,0,0,2,0,3] | [0,6,12,19,27,35,43,51,37,23,24] | $Y_{9,9,9,9,9,9,7,6,2,2}$ [90] | $Y_{9,9,9,9,9,9,7,6,2,2,1,1,1}$ [90] |
| | [6,1,0,0,0,1,1,1,0,3] | [0,6,13,20,27,34,42,51,37,23,24] | $Y_{9,9,9,9,9,9,8,4,3,2}$ [120] | $Y_{9,9,9,9,9,9,8,4,3,2,1,1,1}$ [120] |
| | [0,0,5,1,0,0,0,0,0,5] | [3,6,9,17,26,35,44,53,38,23,24] | $Y_{10,10,10,7,7,7,7,7,6}$ [28] | $Y_{10,10,10,7,7,7,7,7,6,1,1,1,1,1}$ [28] |
| | [0,4,2,0,1,0,0,0,0,5] | [2,4,10,18,26,35,44,53,38,23,24] | $Y_{10,10,8,8,8,8,7,7,5}$ [54] | $Y_{10,10,8,8,8,8,7,7,5,1,1,1,1,1}$ [54] |
| | [2,4,0,1,1,0,0,0,0,5] | [1,4,11,18,26,35,44,53,38,23,24] | $Y_{10,9,9,8,8,8,8,6,5}$ [72] | $Y_{10,9,9,8,8,8,8,6,5,1,1,1,1,1}$ [72] |
| | [3,1,2,2,0,0,0,0,0,5] | [1,5,10,17,26,35,44,53,38,23,24] | $Y_{10,9,9,9,8,7,7,6,6}$ [56] | $Y_{10,9,9,9,8,7,7,6,6,1,1,1,1,1}$ [56] |
| | [5,1,2,0,0,1,0,0,0,5] | [0,5,11,19,27,35,44,53,38,23,24] | $Y_{9,9,9,9,9,8,7,7,4}$ [80] | $Y_{9,9,9,9,9,8,7,7,4,1,1,1,1,1}$ [80] |

| | | | | |
|---|---|---|---|---|
| | [5,2,0,0,2,0,0,0,0,5] | [0,5,12,19,26,35,44,53,38,23,24] | $Y_{9,9,9,9,9,8,8,5,5}$ [48] | $Y_{9,9,9,9,9,8,8,5,5,1,1,1,1,1}$ [48] |
| | [6,0,0,2,1,0,0,0,0,5] | [0,6,12,18,26,35,44,53,38,23,24] | $Y_{9,9,9,9,9,9,6,6,5}$ [48] | $Y_{9,9,9,9,9,9,6,6,5,1,1,1,1,1}$ [48] |
| | [0,1,0,1,0,0,0,0,9,0] | [5,10,16,22,29,36,43,50,32,23,25] | $Y_{10,10,10,10,10,8,6,1,1,1,1,1,1,1,1,1}$ [31] | $Y_{10,10,10,10,10,8,6}$ [32] |
| | [0,1,1,1,1,0,0,0,7,0] | [4,8,13,19,26,34,42,50,33,23,25] | $Y_{10,10,10,10,8,7,6,5,1,1,1,1,1,1,1}$ [72] | $Y_{10,10,10,10,8,7,6,5}$ [72] |
| | [1,3,0,0,0,0,1,0,7,0] | [3,7,14,21,28,35,42,50,33,23,25] | $Y_{10,10,10,9,8,8,8,3,1,1,1,1,1,1,1}$ [48] | $Y_{10,10,10,9,8,8,8,3}$ [48] |
| | [2,0,2,0,0,1,0,0,7,0] | [3,8,13,20,27,34,42,50,33,23,25] | $Y_{10,10,10,9,9,7,7,4,1,1,1,1,1,1,1}$ [60] | $Y_{10,10,10,9,9,7,7,4}$ [60] |
| | [2,1,0,0,2,0,0,0,7,0] | [3,8,14,20,26,34,42,50,33,23,25] | $Y_{10,10,10,9,9,8,5,5,1,1,1,1,1,1,1}$ [48] | $Y_{10,10,10,9,9,8,5,5}$ [48] |
| | [0,0,1,3,0,0,1,0,5,0] | [4,8,12,17,25,33,41,50,34,23,25] | $Y_{10,10,10,10,7,6,6,6,3,1,1,1,1,1}$ [64] | $Y_{10,10,10,10,7,6,6,6,3}$ [64] |
| | [0,0,2,0,2,1,0,0,5,0] | [4,8,12,18,24,32,41,50,34,23,25] | $Y_{10,10,10,10,7,7,5,5,4,1,1,1,1,1}$ [60] | $Y_{10,10,10,10,7,7,5,5,4}$ [60] |
| | [0,3,0,2,0,0,0,1,5,0] | [3,6,12,18,26,34,42,50,34,23,25] | $Y_{10,10,10,8,8,8,6,6,2,1,1,1,1,1}$ [67] | $Y_{10,10,10,8,8,8,6,6,2}$ [68] |
| | [0,3,1,0,0,1,1,0,5,0] | [3,6,12,19,26,33,41,50,34,23,25] | $Y_{10,10,10,8,8,8,7,4,3,1,1,1,1,1}$ [96] | $Y_{10,10,10,8,8,8,7,4,3}$ [96] |
| | [1,1,1,1,0,2,0,0,5,0] | [3,7,12,18,25,32,41,50,34,23,25] | $Y_{10,10,10,9,8,7,6,4,4,1,1,1,1,1}$ [120] | $Y_{10,10,10,9,8,7,6,4,4}$ [120] |
| | [2,0,0,1,2,1,0,0,5,0] | [3,8,13,18,24,32,41,50,34,23,25] | $Y_{10,10,10,9,9,6,5,5,4,1,1,1,1,1}$ [80] | $Y_{10,10,10,9,9,6,5,5,4}$ [80] |
| | [2,2,1,0,1,0,0,1,5,0] | [2,6,12,19,26,34,42,50,34,23,25] | $Y_{10,10,9,9,8,8,7,5,2,1,1,1,1,1}$ [144] | $Y_{10,10,9,9,8,8,7,5,2}$ [144] |
| | [2,3,0,0,0,0,2,0,5,0] | [2,6,13,20,27,34,41,50,34,23,25] | $Y_{10,10,9,9,8,8,8,3,3,1,1,1,1,1}$ [48] | $Y_{10,10,9,9,8,8,8,3,3}$ [48] |
| | [3,0,1,2,0,0,0,1,5,0] | [2,7,12,18,26,34,42,50,34,23,25] | $Y_{10,10,9,9,9,7,6,6,2,1,1,1,1,1}$ [90] | $Y_{10,10,9,9,9,7,6,6,2}$ [90] |
| | [3,0,2,0,0,1,1,0,5,0] | [2,7,12,19,26,33,41,50,34,23,25] | $Y_{10,10,9,9,9,7,7,4,3,1,1,1,1,1}$ [96] | $Y_{10,10,9,9,9,7,7,4,3}$ [96] |
| | [3,1,0,0,2,0,1,0,5,0] | [2,7,13,19,25,33,41,50,34,23,25] | $Y_{10,10,9,9,9,8,5,5,3,1,1,1,1,1}$ [96] | $Y_{10,10,9,9,9,8,5,5,3}$ [96] |
| | [5,0,1,0,1,0,0,0,6,1] | [1,7,13,20,27,35,43,51,34,23,25] | $Y_{10,9,9,9,9,9,7,5,1,1,1,1,1,1}$ [90] | $Y_{10,9,9,9,9,9,7,5,1}$ [90] |
| | [5,1,0,0,0,0,1,1,5,0] | [1,7,14,21,28,35,42,50,34,23,25] | $Y_{10,9,9,9,9,9,8,3,2,1,1,1,1,1}$ [72] | $Y_{10,9,9,9,9,9,8,3,2}$ [72] |
| | [0,0,0,4,0,1,0,1,3,0] | [4,8,12,16,24,32,41,50,35,23,25] | $Y_{10,10,10,10,6,6,6,6,4,2,1,1,1}$ [67] | $Y_{10,10,10,10,6,6,6,6,4,2}$ [68] |
| | [0,0,1,1,2,1,1,0,3,0] | [4,8,12,17,23,31,40,50,35,23,25] | $Y_{10,10,10,10,7,6,5,5,4,3,1,1,1}$ [128] | $Y_{10,10,10,10,7,6,5,5,4,3}$ [128] |
| | [0,1,0,1,0,4,0,0,3,0] | [4,8,13,18,24,30,40,50,35,23,25] | $Y_{10,10,10,10,8,6,4,4,4,4,1,1,1}$ [67] | $Y_{10,10,10,10,8,6,4,4,4,4}$ [68] |
| | [0,2,1,1,1,1,0,1,3,0] | [3,6,11,17,24,32,41,50,35,23,25] | $Y_{10,10,10,8,8,7,6,5,4,2,1,1,1}$ [216] | $Y_{10,10,10,8,8,7,6,5,4,2}$ [216] |
| | [0,2,2,0,0,1,2,0,3,0] | [3,6,11,18,25,32,40,50,35,23,25] | $Y_{10,10,10,8,8,7,7,4,3,3,1,1,1}$ [96] | $Y_{10,10,10,8,8,7,7,4,3,3}$ [96] |
| | [0,3,0,0,2,0,2,0,3,0] | [3,6,12,18,24,32,40,50,35,23,25] | $Y_{10,10,10,8,8,8,5,5,3,3,1,1,1}$ [72] | $Y_{10,10,10,8,8,8,5,5,3,3}$ [72] |
| | [1,0,1,3,1,0,0,0,4,1] | [3,7,11,16,24,33,42,51,35,23,25] | $Y_{10,10,10,9,7,6,6,6,5,1,1,1,1}$ [120] | $Y_{10,10,10,9,7,6,6,6,5,1}$ [120] |
| | [1,0,2,1,1,0,2,0,3,0] | [3,7,11,17,24,32,40,50,35,23,25] | $Y_{10,10,10,9,7,7,6,5,3,3,1,1,1}$ [144] | $Y_{10,10,10,9,7,7,6,5,3,3}$ [144] |
| | [1,1,0,1,3,0,0,1,3,0] | [3,7,12,17,23,32,41,50,35,23,25] | $Y_{10,10,10,9,8,6,5,5,5,2,1,1,1}$ [144] | $Y_{10,10,10,9,8,6,5,5,5,2}$ [144] |
| | [1,1,0,2,0,2,1,0,3,0] | [3,7,12,17,24,31,40,50,35,23,25] | $Y_{10,10,10,9,8,6,6,4,4,3,1,1,1}$ [144] | $Y_{10,10,10,9,8,6,6,4,4,3}$ [144] |
| | [1,3,1,0,1,1,0,0,4,1] | [2,5,11,18,25,33,42,51,35,23,25] | $Y_{10,10,9,8,8,8,7,5,4,1,1,1,1}$ [192] | $Y_{10,10,9,8,8,8,7,5,4,1}$ [192] |
| | [1,3,1,1,0,0,0,2,3,0] | [2,5,11,18,26,34,42,50,35,23,25] | $Y_{10,10,9,8,8,8,7,6,2,2,1,1,1}$ [120] | $Y_{10,10,9,8,8,8,7,6,2,2}$ [120] |
| | [1,4,0,0,0,1,1,1,3,0] | [2,5,12,19,26,33,41,50,35,23,25] | $Y_{10,10,9,8,8,8,8,4,3,2,1,1,1}$ [120] | $Y_{10,10,9,8,8,8,8,4,3,2}$ [120] |
| | [2,0,0,0,3,1,1,0,3,0] | [3,8,13,18,23,31,40,50,35,23,25] | $Y_{10,10,10,9,9,5,5,5,4,3,1,1,1}$ [80] | $Y_{10,10,10,9,9,5,5,5,4,3}$ [80] |
| | [2,1,1,1,2,0,0,0,4,1] | [2,6,11,17,24,33,42,51,35,23,25] | $Y_{10,10,9,9,8,7,6,5,5,1,1,1,1}$ [160] | $Y_{10,10,9,9,8,7,6,5,5,1}$ [160] |
| | [2,1,1,2,0,0,1,1,3,0] | [2,6,11,17,25,33,41,50,35,23,25] | $Y_{10,10,9,9,8,7,6,6,3,2,1,1,1}$ [192] | $Y_{10,10,9,9,8,7,6,6,3,2}$ [192] |
| | [2,1,2,0,0,2,0,1,3,0] | [2,6,11,18,25,32,41,50,35,23,25] | $Y_{10,10,9,9,8,7,7,4,4,2,1,1,1}$ [144] | $Y_{10,10,9,9,8,7,7,4,4,2}$ [144] |
| | [2,2,0,0,2,1,0,1,3,0] | [2,6,12,18,24,32,41,50,35,23,25] | $Y_{10,10,9,9,8,8,5,5,4,2,1,1,1}$ [144] | $Y_{10,10,9,9,8,8,5,5,4,2}$ [144] |
| | [2,2,0,1,0,1,2,0,3,0] | [2,6,12,18,25,32,40,50,35,23,25] | $Y_{10,10,9,9,8,8,6,4,3,3,1,1,1}$ [144] | $Y_{10,10,9,9,8,8,6,4,3,3}$ [144] |
| | [3,0,0,2,1,1,0,1,3,0] | [2,7,12,17,24,32,41,50,35,23,25] | $Y_{10,10,9,9,9,6,6,5,4,2,1,1,1}$ [144] | $Y_{10,10,9,9,9,6,6,5,4,2}$ [144] |
| | [3,0,1,0,2,0,2,0,3,0] | [2,7,12,18,24,32,40,50,35,23,25] | $Y_{10,10,9,9,9,7,5,5,3,3,1,1,1}$ [108] | $Y_{10,10,9,9,9,7,5,5,3,3}$ [108] |
| | [3,2,2,0,0,0,0,1,4,1] | [1,5,11,19,27,35,43,51,35,23,25] | $Y_{10,9,9,9,8,8,7,7,2,1,1,1,1}$ [96] | $Y_{10,9,9,9,8,8,7,7,2,1}$ [96] |
| | [3,3,0,0,1,0,1,0,4,1] | [1,5,12,19,26,34,42,51,35,23,25] | $Y_{10,9,9,9,8,8,8,5,3,1,1,1,1}$ [144] | $Y_{10,9,9,9,8,8,8,5,3,1}$ [144] |
| | [4,0,2,1,0,0,1,0,4,1] | [1,6,11,18,26,34,42,51,35,23,25] | $Y_{10,9,9,9,9,7,7,6,3,1,1,1,1}$ [144] | $Y_{10,9,9,9,9,7,7,6,3,1}$ [144] |
| | [4,1,0,1,1,1,0,0,4,1] | [1,6,12,18,25,33,42,51,35,23,25] | $Y_{10,9,9,9,9,8,6,5,4,1,1,1,1}$ [192] | $Y_{10,9,9,9,9,8,6,5,4,1}$ [192] |
| | [4,1,0,2,0,0,0,2,3,0] | [1,6,12,18,26,34,42,50,35,23,25] | $Y_{10,9,9,9,9,8,6,6,2,2,1,1,1}$ [90] | $Y_{10,9,9,9,9,8,6,6,2,2}$ [90] |
| | [4,1,1,0,0,1,1,1,3,0] | [1,6,12,19,26,33,41,50,35,23,25] | $Y_{10,9,9,9,9,8,7,4,3,2,1,1,1}$ [192] | $Y_{10,9,9,9,9,8,7,4,3,2}$ [192] |
| | [5,0,0,0,2,0,1,1,3,0] | [1,7,13,19,25,33,41,50,35,23,25] | $Y_{10,9,9,9,9,9,5,5,3,2,1,1,1}$ [90] | $Y_{10,9,9,9,9,9,5,5,3,2}$ [90] |
| | [6,1,0,1,0,0,0,0,5,2] | [0,6,13,20,28,36,44,52,35,23,25] | $Y_{9,9,9,9,9,9,8,6,1,1,1,1,1}$ [72] | $Y_{9,9,9,9,9,9,8,6,1,1}$ [72] |
| | [7,0,0,0,0,1,0,1,4,1] | [0,7,14,21,28,35,43,51,35,23,25] | $Y_{9,9,9,9,9,9,9,4,2,1,1,1,1}$ [72] | $Y_{9,9,9,9,9,9,9,4,2,1}$ [72] |
| | [0,0,0,3,1,1,1,1,1,0] | [4,8,12,16,23,31,40,50,36,23,25] | $Y_{10,10,10,10,6,6,6,5,4,3,2,1}$ [120] | $Y_{10,10,10,10,6,6,6,5,4,3,2}$ [120] |
| | [0,0,1,1,1,3,0,1,1,0] | [4,8,12,17,23,30,40,50,36,23,25] | $Y_{10,10,10,10,7,6,5,4,4,4,2,1}$ [144] | $Y_{10,10,10,10,7,6,5,4,4,4,2}$ [144] |
| | [0,0,1,1,2,0,3,0,1,0] | [4,8,12,17,23,31,39,50,36,23,25] | $Y_{10,10,10,10,7,6,5,5,3,3,3,1}$ [96] | $Y_{10,10,10,10,7,6,5,5,3,3,3}$ [96] |
| | [0,0,2,0,0,3,2,0,1,0] | [4,8,12,18,24,30,39,50,36,23,25] | $Y_{10,10,10,10,7,7,4,4,4,3,3,1}$ [64] | $Y_{10,10,10,10,7,7,4,4,4,3,3}$ [64] |
| | [0,1,0,0,2,2,2,0,1,0] | [4,8,13,18,23,30,39,50,36,23,25] | $Y_{10,10,10,10,8,5,5,4,4,3,3,1}$ [96] | $Y_{10,10,10,10,8,5,5,4,4,3,3}$ [96] |
| | [0,1,2,2,0,1,1,0,2,1] | [3,6,10,16,24,32,41,51,36,23,25] | $Y_{10,10,10,8,7,7,6,6,4,3,1,1}$ [216] | $Y_{10,10,10,8,7,7,6,6,4,3,1}$ [216] |
| | [0,1,3,0,1,1,0,2,1,0] | [3,6,10,17,24,32,41,50,36,23,25] | $Y_{10,10,10,8,7,7,7,5,4,2,2,1}$ [162] | $Y_{10,10,10,8,7,7,7,5,4,2,2}$ [162] |
| | [0,2,0,2,2,0,1,0,2,1] | [3,6,11,16,23,32,41,51,36,23,25] | $Y_{10,10,10,8,8,6,6,5,5,3,1,1}$ [162] | $Y_{10,10,10,8,8,6,6,5,5,3,1}$ [162] |
| | [0,2,0,3,0,1,0,2,1,0] | [3,6,11,16,24,32,41,50,36,23,25] | $Y_{10,10,10,8,8,6,6,6,4,2,2,1}$ [121] | $Y_{10,10,10,8,8,6,6,6,4,2,2}$ [122] |
| | [0,2,1,0,2,2,0,0,2,1] | [3,6,11,17,23,31,41,51,36,23,25] | $Y_{10,10,10,8,8,7,5,5,4,4,1,1}$ [144] | $Y_{10,10,10,8,8,7,5,5,4,4,1}$ [144] |
| | [0,2,1,0,3,0,0,2,1,0] | [3,6,11,17,23,32,41,50,36,23,25] | $Y_{10,10,10,8,8,7,5,5,5,2,2,1}$ [108] | $Y_{10,10,10,8,8,7,5,5,5,2,2}$ [108] |
| | [0,2,1,1,0,2,1,1,1,0] | [3,6,11,17,24,31,40,50,36,23,25] | $Y_{10,10,10,8,8,7,6,4,4,3,2,1}$ [216] | $Y_{10,10,10,8,8,7,6,4,4,3,2}$ [216] |
| | [0,4,2,0,0,1,0,0,3,2] | [2,4,10,18,26,34,43,52,36,23,25] | $Y_{10,10,8,8,8,8,7,7,4,1,1,1}$ [96] | $Y_{10,10,8,8,8,8,7,7,4,1,1}$ [96] |
| | [0,5,0,0,2,0,0,0,3,2] | [2,4,11,18,25,34,43,52,36,23,25] | $Y_{10,10,8,8,8,8,8,5,5,1,1,1}$ [60] | $Y_{10,10,8,8,8,8,8,5,5,1,1}$ [60] |
| | [0,5,0,1,0,0,1,1,2,1] | [2,4,11,18,26,34,42,51,36,23,25] | $Y_{10,10,8,8,8,8,8,6,3,2,1,1}$ [144] | $Y_{10,10,8,8,8,8,8,6,3,2,1}$ [144] |
| | [1,0,1,2,1,2,0,0,2,1] | [3,7,11,16,23,31,41,51,36,23,25] | $Y_{10,10,10,9,7,6,6,5,4,4,1,1}$ [192] | $Y_{10,10,10,9,7,6,6,5,4,4,1}$ [192] |
| | [1,0,1,2,2,0,0,2,1,0] | [3,7,11,16,23,32,41,50,36,23,25] | $Y_{10,10,10,9,7,6,6,5,5,2,2,1}$ [144] | $Y_{10,10,10,9,7,6,6,5,5,2,2}$ [144] |
| | [1,0,1,3,0,0,2,1,1,0] | [3,7,11,16,24,32,40,50,36,23,25] | $Y_{10,10,10,9,7,6,6,6,3,3,2,1}$ [144] | $Y_{10,10,10,9,7,6,6,6,3,3,2}$ [144] |
| | [1,0,2,0,2,1,1,1,1,0] | [3,7,11,17,23,31,40,50,36,23,25] | $Y_{10,10,10,9,7,7,5,5,4,3,2,1}$ [216] | $Y_{10,10,10,9,7,7,5,5,4,3,2}$ [216] |
| | [1,0,3,0,0,0,4,0,1,0] | [3,7,11,18,25,32,39,50,36,23,25] | $Y_{10,10,10,9,7,7,7,3,3,3,3,1}$ [60] | $Y_{10,10,10,9,7,7,7,3,3,3,3}$ [60] |
| | [1,1,0,2,0,1,3,0,1,0] | [3,7,12,17,24,31,39,50,36,23,25] | $Y_{10,10,10,9,8,6,6,4,3,3,3,1}$ [144] | $Y_{10,10,10,9,8,6,6,4,3,3,3}$ [144] |

| | | | | |
|---|---|---|---|---|
| | [1,1,1,0,0,4,0,1,1,0] | [3,7,12,18,24,30,40,50,36,23,25] | $Y_{10,10,10,9,8,7,4,4,4,4,2,1}$ [144] | $Y_{10,10,10,9,8,7,4,4,4,4,2}$ [144] |
| | [1,2,1,3,0,0,0,0,3,2] | [2,5,10,16,25,34,43,52,36,23,25] | $Y_{10,10,9,8,8,7,6,6,6,1,1,1}$ [96] | $Y_{10,10,9,8,8,7,6,6,6,1,1}$ [96] |
| | [1,2,2,0,2,0,0,1,2,1] | [2,5,10,17,24,33,42,51,36,23,25] | $Y_{10,10,9,8,8,7,7,5,5,2,1,1}$ [192] | $Y_{10,10,9,8,8,7,7,5,5,2,1}$ [192] |
| | [1,2,2,1,0,0,2,0,2,1] | [2,5,10,17,25,33,41,51,36,23,25] | $Y_{10,10,9,8,8,7,7,6,3,3,1,1}$ [192] | $Y_{10,10,9,8,8,7,7,6,3,3,1}$ [192] |
| | [1,2,3,0,0,0,0,3,1,0] | [2,5,10,18,26,34,42,50,36,23,25] | $Y_{10,10,9,8,8,7,7,7,2,2,2,1}$ [72] | $Y_{10,10,9,8,8,7,7,7,2,2,2}$ [72] |
| | [1,3,0,1,1,1,1,0,2,1] | [2,5,11,17,24,32,41,51,36,23,25] | $Y_{10,10,9,8,8,8,6,5,4,3,1,1}$ [288] | $Y_{10,10,9,8,8,8,6,5,4,3,1}$ [288] |
| | [1,3,0,2,0,0,1,2,1,0] | [2,5,11,17,25,33,41,50,36,23,25] | $Y_{10,10,9,8,8,8,6,6,3,2,2,1}$ [144] | $Y_{10,10,9,8,8,8,6,6,3,2,2}$ [144] |
| | [1,3,1,0,0,2,0,2,1,0] | [2,5,11,18,25,32,41,50,36,23,25] | $Y_{10,10,9,8,8,8,7,4,4,2,2,1}$ [144] | $Y_{10,10,9,8,8,8,7,4,4,2,2}$ [144] |
| | [2,0,0,0,2,3,0,1,1,0] | [3,8,13,18,23,30,40,50,36,23,25] | $Y_{10,10,10,9,9,5,5,4,4,4,2,1}$ [90] | $Y_{10,10,10,9,9,5,5,4,4,4,2}$ [90] |
| | [2,0,0,0,3,0,3,0,1,0] | [3,8,13,18,23,31,39,50,36,23,25] | $Y_{10,10,10,9,9,5,5,5,3,3,3,1}$ [60] | $Y_{10,10,10,9,9,5,5,5,3,3,3}$ [60] |
| | [2,0,0,1,0,3,2,0,1,0] | [3,8,13,18,24,30,39,50,36,23,25] | $Y_{10,10,10,9,9,6,4,4,4,3,3,1}$ [96] | $Y_{10,10,10,9,9,6,4,4,4,3,3}$ [96] |
| | [2,0,2,2,1,0,0,1,2,1] | [2,6,10,16,24,33,42,51,36,23,25] | $Y_{10,10,9,9,7,7,6,6,5,2,1,1}$ [192] | $Y_{10,10,9,9,7,7,6,6,5,2,1}$ [192] |
| | [2,0,3,0,1,1,1,0,2,1] | [2,6,10,17,24,32,41,51,36,23,25] | $Y_{10,10,9,9,7,7,7,5,4,3,1,1}$ [216] | $Y_{10,10,9,9,7,7,7,5,4,3,1}$ [216] |
| | [2,0,3,1,0,0,1,2,1,0] | [2,6,10,17,25,33,41,50,36,23,25] | $Y_{10,10,9,9,7,7,7,6,3,2,2,1}$ [144] | $Y_{10,10,9,9,7,7,7,6,3,2,2}$ [144] |
| | [2,1,0,3,0,1,1,0,2,1] | [2,6,11,16,24,32,41,51,36,23,25] | $Y_{10,10,9,9,8,6,6,6,4,3,1,1}$ [216] | $Y_{10,10,9,9,8,6,6,6,4,3,1}$ [216] |
| | [2,1,1,0,3,0,1,0,2,1] | [2,6,11,17,23,32,41,51,36,23,25] | $Y_{10,10,9,9,8,7,5,5,5,3,1,1}$ [216] | $Y_{10,10,9,9,8,7,5,5,5,3,1}$ [216] |
| | [2,1,1,1,0,3,0,0,2,1] | [2,6,11,17,24,31,41,51,36,23,25] | $Y_{10,10,9,9,8,7,6,4,4,4,1,1}$ [192] | $Y_{10,10,9,9,8,7,6,4,4,4,1}$ [192] |
| | [2,1,1,1,1,0,2,1,1,0] | [2,6,11,17,24,32,40,50,36,23,25] | $Y_{10,10,9,9,8,7,6,5,3,3,2,1}$ [288] | $Y_{10,10,9,9,8,7,6,5,3,3,2}$ [288] |
| | [2,2,0,0,1,2,1,1,1,0] | [2,6,12,18,24,31,40,50,36,23,25] | $Y_{10,10,9,9,8,8,5,4,4,3,2,1}$ [192] | $Y_{10,10,9,9,8,8,5,4,4,3,2}$ [192] |
| | [2,4,0,1,0,1,0,0,3,2] | [1,4,11,18,26,34,43,52,36,23,25] | $Y_{10,9,9,8,8,8,8,6,4,1,1,1}$ [144] | $Y_{10,9,9,8,8,8,8,6,4,1,1}$ [144] |
| | [2,4,1,0,0,0,0,2,2,1] | [1,4,11,19,27,35,43,51,36,23,25] | $Y_{10,9,9,8,8,8,8,7,2,2,1,1}$ [96] | $Y_{10,9,9,8,8,8,8,7,2,2,1}$ [96] |
| | [3,0,0,1,2,2,0,0,2,1] | [2,7,12,17,23,31,41,51,36,23,25] | $Y_{10,10,9,9,9,6,5,5,4,4,1,1}$ [128] | $Y_{10,10,9,9,9,6,5,5,4,4,1}$ [128] |
| | [3,0,0,1,3,0,0,2,1,0] | [2,7,12,17,23,32,41,50,36,23,25] | $Y_{10,10,9,9,9,6,5,5,5,2,2,1}$ [96] | $Y_{10,10,9,9,9,6,5,5,5,2,2}$ [96] |
| | [3,0,0,2,0,2,1,1,1,0] | [2,7,12,17,24,31,40,50,36,23,25] | $Y_{10,10,9,9,9,6,6,4,4,3,2,1}$ [144] | $Y_{10,10,9,9,9,6,6,4,4,3,2}$ [144] |
| | [3,0,1,1,0,0,4,0,1,0] | [2,7,12,18,25,32,39,50,36,23,25] | $Y_{10,10,9,9,9,7,6,3,3,3,3,1}$ [96] | $Y_{10,10,9,9,9,7,6,3,3,3,3}$ [96] |
| | [3,1,0,0,0,2,3,0,1,0] | [2,7,13,19,25,31,39,50,36,23,25] | $Y_{10,10,9,9,9,8,4,4,3,3,3,1}$ [80] | $Y_{10,10,9,9,9,8,4,4,3,3,3}$ [80] |
| | [3,1,2,1,1,0,0,0,3,2] | [1,5,10,17,25,34,43,52,36,23,25] | $Y_{10,9,9,9,8,7,7,6,5,1,1,1}$ [160] | $Y_{10,9,9,9,8,7,7,6,5,1,1}$ [160] |
| | [3,1,3,0,0,0,1,1,2,1] | [1,5,10,18,26,34,42,51,36,23,25] | $Y_{10,9,9,9,8,7,7,7,3,2,1,1}$ [160] | $Y_{10,9,9,9,8,7,7,7,3,2,1}$ [160] |
| | [3,2,0,2,0,1,0,1,2,1] | [1,5,11,17,25,33,42,51,36,23,25] | $Y_{10,9,9,9,8,8,6,6,4,2,1,1}$ [216] | $Y_{10,9,9,9,8,8,6,6,4,2,1}$ [216] |
| | [3,2,1,0,1,0,2,0,2,1] | [1,5,11,18,25,33,41,51,36,23,25] | $Y_{10,9,9,9,8,8,7,5,3,3,1,1}$ [216] | $Y_{10,9,9,9,8,8,7,5,3,3,1}$ [216] |
| | [3,2,1,1,0,0,0,3,1,0] | [1,5,11,18,26,34,42,50,36,23,25] | $Y_{10,9,9,9,8,8,7,6,2,2,2,1}$ [120] | $Y_{10,9,9,9,8,8,7,6,2,2,2}$ [120] |
| | [3,3,0,0,0,1,1,2,1,0] | [1,5,12,19,26,33,41,50,36,23,25] | $Y_{10,9,9,9,8,8,8,4,3,2,2,1}$ [120] | $Y_{10,9,9,9,8,8,8,4,3,2,2}$ [120] |
| | [4,0,1,1,2,0,0,1,2,1] | [1,6,11,17,24,33,42,51,36,23,25] | $Y_{10,9,9,9,9,7,6,5,5,2,1,1}$ [192] | $Y_{10,9,9,9,9,7,6,5,5,2,1}$ [192] |
| | [4,0,1,2,0,0,2,0,2,1] | [1,6,11,17,25,33,41,51,36,23,25] | $Y_{10,9,9,9,9,7,6,6,3,3,1,1}$ [144] | $Y_{10,9,9,9,9,7,6,6,3,3,1}$ [144] |
| | [4,0,2,0,0,2,1,0,2,1] | [1,6,11,18,25,32,41,51,36,23,25] | $Y_{10,9,9,9,9,7,7,4,4,3,1,1}$ [144] | $Y_{10,9,9,9,9,7,7,4,4,3,1}$ [144] |
| | [4,0,2,0,1,0,1,2,1,0] | [1,6,11,18,25,33,41,50,36,23,25] | $Y_{10,9,9,9,9,7,7,5,3,2,2,1}$ [162] | $Y_{10,9,9,9,9,7,7,5,3,2,2}$ [162] |
| | [4,1,0,0,2,1,1,0,2,1] | [1,6,12,18,24,32,41,51,36,23,25] | $Y_{10,9,9,9,9,8,5,5,4,3,1,1}$ [192] | $Y_{10,9,9,9,9,8,5,5,4,3,1}$ [192] |
| | [4,1,0,1,0,2,0,2,1,0] | [1,6,12,18,25,32,41,50,36,23,25] | $Y_{10,9,9,9,9,8,6,4,4,2,2,1}$ [162] | $Y_{10,9,9,9,9,8,6,4,4,2,2}$ [162] |
| | [4,1,1,0,0,0,3,1,1,0] | [1,6,12,19,26,33,40,50,36,23,25] | $Y_{10,9,9,9,9,8,7,3,3,3,2,1}$ [120] | $Y_{10,9,9,9,9,8,7,3,3,3,2}$ [120] |
| | [5,0,0,0,1,1,2,1,1,0] | [1,7,13,19,25,32,40,50,36,23,25] | $Y_{10,9,9,9,9,9,5,4,3,3,2,1}$ [120] | $Y_{10,9,9,9,9,9,5,4,3,3,2}$ [120] |
| | [5,1,2,0,0,0,1,0,3,2] | [0,5,11,19,27,35,43,52,36,23,25] | $Y_{9,9,9,9,9,8,7,7,3,1,1,1}$ [120] | $Y_{9,9,9,9,9,8,7,7,3,1,1}$ [120] |
| | [5,2,0,0,1,1,0,0,3,2] | [0,5,12,19,26,34,43,52,36,23,25] | $Y_{9,9,9,9,9,8,8,5,4,1,1,1}$ [128] | $Y_{9,9,9,9,9,8,8,5,4,1,1}$ [128] |
| | [5,2,0,1,0,0,0,2,2,1] | [0,5,12,19,27,35,43,51,36,23,25] | $Y_{9,9,9,9,9,8,8,6,2,2,1,1}$ [120] | $Y_{9,9,9,9,9,8,8,6,2,2,1}$ [120] |
| | [6,0,0,2,0,1,0,0,3,2] | [0,6,12,18,26,34,43,52,36,23,25] | $Y_{9,9,9,9,9,9,6,6,4,1,1,1}$ [96] | $Y_{9,9,9,9,9,9,6,6,4,1,1}$ [96] |
| | [6,0,1,0,1,0,1,1,2,1] | [0,6,12,19,26,34,42,51,36,23,25] | $Y_{9,9,9,9,9,9,7,5,3,2,1,1}$ [216] | $Y_{9,9,9,9,9,9,7,5,3,2,1}$ [216] |
| | [7,0,0,0,0,0,1,3,1,0] | [0,7,14,21,28,35,42,50,36,23,25] | $Y_{9,9,9,9,9,9,9,3,2,2,2,1}$ [42] | $Y_{9,9,9,9,9,9,9,3,2,2,2}$ [42] |
| | [0,0,4,1,1,0,1,0,1,2] | [3,6,9,16,24,33,42,52,37,23,25] | $Y_{10,10,10,7,7,7,7,6,5,3,1}$ [144] | $Y_{10,10,10,7,7,7,7,6,5,3,1,1}$ [144] |
| | [0,0,5,0,0,1,0,2,0,1] | [3,6,9,17,25,33,42,51,37,23,25] | $Y_{10,10,10,7,7,7,7,7,4,2,2}$ [72] | $Y_{10,10,10,7,7,7,7,7,4,2,2,1}$ [72] |
| | [0,1,1,4,0,0,1,0,1,2] | [3,6,10,15,24,33,42,52,37,23,25] | $Y_{10,10,10,8,7,6,6,6,6,3,1}$ [144] | $Y_{10,10,10,8,7,6,6,6,6,3,1,1}$ [144] |
| | [0,1,2,1,2,0,1,1,0,1] | [3,6,10,16,23,32,41,51,37,23,25] | $Y_{10,10,10,8,7,7,6,5,5,3,2}$ [216] | $Y_{10,10,10,8,7,7,6,5,5,3,2,1}$ [216] |
| | [0,1,3,0,0,3,0,1,0,1] | [3,6,10,17,24,31,41,51,37,23,25] | $Y_{10,10,10,8,7,7,7,4,4,4,2}$ [108] | $Y_{10,10,10,8,7,7,7,4,4,4,2,1}$ [108] |
| | [0,1,3,0,1,0,3,0,0,1] | [3,6,10,17,24,32,40,51,37,23,25] | $Y_{10,10,10,8,7,7,7,5,3,3,3}$ [108] | $Y_{10,10,10,8,7,7,7,5,3,3,3,1}$ [108] |
| | [0,2,0,2,1,2,0,1,0,1] | [3,6,11,16,23,31,41,51,37,23,25] | $Y_{10,10,10,8,8,6,6,5,4,4,2}$ [162] | $Y_{10,10,10,8,8,6,6,5,4,4,2,1}$ [162] |
| | [0,2,0,3,0,0,3,0,0,1] | [3,6,11,16,24,32,40,51,37,23,25] | $Y_{10,10,10,8,8,6,6,6,3,3,3}$ [72] | $Y_{10,10,10,8,8,6,6,6,3,3,3,1}$ [72] |
| | [0,2,1,0,2,1,2,0,0,1] | [3,6,11,17,23,31,40,51,37,23,25] | $Y_{10,10,10,8,8,7,5,5,4,3,3}$ [144] | $Y_{10,10,10,8,8,7,5,5,4,3,3,1}$ [144] |
| | [0,3,3,1,0,0,0,0,2,3] | [2,4,9,17,26,35,44,53,37,23,25] | $Y_{10,10,8,8,8,7,7,7,6,1,1}$ [72] | $Y_{10,10,8,8,8,7,7,7,6,1,1,1}$ [72] |
| | [0,4,1,1,0,1,1,0,1,2] | [2,4,10,17,25,33,42,52,37,23,25] | $Y_{10,10,8,8,8,8,7,6,4,3,1}$ [216] | $Y_{10,10,8,8,8,8,7,6,4,3,1,1}$ [216] |
| | [0,4,2,0,0,0,1,2,0,1] | [2,4,10,18,26,34,42,51,37,23,25] | $Y_{10,10,8,8,8,8,7,7,3,2,2}$ [90] | $Y_{10,10,8,8,8,8,7,7,3,2,2,1}$ [90] |
| | [0,5,0,0,1,1,0,2,0,1] | [2,4,11,18,25,33,42,51,37,23,25] | $Y_{10,10,8,8,8,8,8,5,4,2,2}$ [108] | $Y_{10,10,8,8,8,8,8,5,4,2,2,1}$ [108] |
| | [1,0,0,4,1,1,0,0,1,2] | [3,7,11,15,23,32,42,52,37,23,25] | $Y_{10,10,10,9,6,6,6,6,5,4,1}$ [128] | $Y_{10,10,10,9,6,6,6,6,5,4,1,1}$ [128] |
| | [1,0,0,5,0,0,0,2,0,1] | [3,7,11,15,24,33,42,51,37,23,25] | $Y_{10,10,10,9,6,6,6,6,6,2,2}$ [60] | $Y_{10,10,10,9,6,6,6,6,6,2,2,1}$ [60] |
| | [1,0,1,2,1,1,2,0,0,1] | [3,7,11,16,23,31,40,51,37,23,25] | $Y_{10,10,10,9,7,6,6,5,4,3,3}$ [192] | $Y_{10,10,10,9,7,6,6,5,4,3,3,1}$ [192] |
| | [1,1,0,1,1,3,1,0,0,1] | [3,7,12,17,23,30,40,51,37,23,25] | $Y_{10,10,10,9,8,6,5,4,4,4,3}$ [192] | $Y_{10,10,10,9,8,6,5,4,4,4,3,1}$ [192] |
| | [1,1,3,2,0,0,0,1,1,2] | [2,5,9,16,25,34,43,52,37,23,25] | $Y_{10,10,9,8,7,7,7,6,6,2,1}$ [160] | $Y_{10,10,9,8,7,7,7,6,6,2,1,1}$ [160] |
| | [1,1,4,0,0,1,1,0,1,2] | [2,5,9,17,25,33,42,52,37,23,25] | $Y_{10,10,9,8,7,7,7,7,4,3,1}$ [192] | $Y_{10,10,9,8,7,7,7,7,4,3,1,1}$ [192] |
| | [1,2,1,2,0,2,0,0,1,2] | [2,5,10,16,24,32,42,52,37,23,25] | $Y_{10,10,9,8,8,7,6,6,4,4,1}$ [192] | $Y_{10,10,9,8,8,7,6,6,4,4,1,1}$ [192] |
| | [1,2,1,2,1,0,0,2,0,1] | [2,5,10,16,24,33,42,51,37,23,25] | $Y_{10,10,9,8,8,7,6,6,5,2,2}$ [192] | $Y_{10,10,9,8,8,7,6,6,5,2,2,1}$ [192] |
| | [1,2,2,0,1,1,1,1,0,1] | [2,5,10,17,24,32,41,51,37,23,25] | $Y_{10,10,9,8,8,7,7,5,4,3,2}$ [288] | $Y_{10,10,9,8,8,7,7,5,4,3,2,1}$ [288] |
| | [1,3,0,0,3,1,0,0,1,2] | [2,5,11,17,23,32,42,52,37,23,25] | $Y_{10,10,9,8,8,8,5,5,5,4,1}$ [128] | $Y_{10,10,9,8,8,8,5,5,5,4,1,1}$ [128] |
| | [2,0,2,1,2,1,0,0,1,2] | [2,6,10,16,23,32,42,52,37,23,25] | $Y_{10,10,9,9,7,7,6,5,5,4,1}$ [192] | $Y_{10,10,9,9,7,7,6,5,5,4,1,1}$ [192] |
| | [2,0,2,2,0,1,1,1,0,1] | [2,6,10,16,24,32,41,51,37,23,25] | $Y_{10,10,9,9,7,7,6,6,4,3,2}$ [216] | $Y_{10,10,9,9,7,7,6,6,4,3,2,1}$ [216] |

| | | | | |
|---|---|---|---|---|
| | [2,1,0,2,2,0,1,1,0,1] | [2,6,11,16,23,32,41,51,37,23,25] | $Y_{10,10,9,9,8,6,6,5,5,3,2}$ [216] | $Y_{10,10,9,9,8,6,6,5,5,3,2,1}$ [216] |
| | [2,1,1,0,2,2,0,1,0,1] | [2,6,11,17,23,31,41,51,37,23,25] | $Y_{10,10,9,9,8,7,5,5,4,4,2}$ [216] | $Y_{10,10,9,9,8,7,5,5,4,4,2,1}$ [216] |
| | [2,1,1,1,0,2,2,0,0,1] | [2,6,11,17,24,31,40,51,37,23,25] | $Y_{10,10,9,9,8,7,6,4,4,3,3}$ [192] | $Y_{10,10,9,9,8,7,6,4,4,3,3,1}$ [192] |
| | [2,3,1,1,1,0,0,1,1,2] | [1,4,10,17,25,34,43,52,37,23,25] | $Y_{10,9,9,8,8,8,7,6,5,2,1}$ [256] | $Y_{10,9,9,8,8,8,7,6,5,2,1,1}$ [256] |
| | [2,3,2,0,0,0,2,0,1,2] | [1,4,10,18,26,34,42,52,37,23,25] | $Y_{10,9,9,8,8,8,7,7,3,3,1}$ [120] | $Y_{10,9,9,8,8,8,7,7,3,3,1,1}$ [120] |
| | [2,4,0,0,1,1,1,0,1,2] | [1,4,11,18,25,33,42,52,37,23,25] | $Y_{10,9,9,8,8,8,8,5,4,3,1}$ [192] | $Y_{10,9,9,8,8,8,8,5,4,3,1,1}$ [192] |
| | [2,4,0,1,0,0,1,2,0,1] | [1,4,11,18,26,34,42,51,37,23,25] | $Y_{10,9,9,8,8,8,8,6,3,2,2}$ [144] | $Y_{10,9,9,8,8,8,8,6,3,2,2,1}$ [144] |
| | [3,0,0,1,2,1,2,0,0,1] | [2,7,12,17,23,31,40,51,37,23,25] | $Y_{10,10,9,9,9,6,5,5,4,3,3}$ [128] | $Y_{10,10,9,9,9,6,5,5,4,3,3,1}$ [128] |
| | [3,0,4,1,0,0,0,0,2,3] | [1,5,9,17,26,35,44,53,37,23,25] | $Y_{10,9,9,9,7,7,7,7,6,1,1}$ [72] | $Y_{10,9,9,9,7,7,7,7,6,1,1,1}$ [72] |
| | [3,1,1,3,0,0,0,1,1,2] | [1,5,10,16,25,34,43,52,37,23,25] | $Y_{10,9,9,9,8,7,6,6,6,2,1}$ [160] | $Y_{10,9,9,9,8,7,6,6,6,2,1,1}$ [160] |
| | [3,1,2,0,2,0,1,0,1,2] | [1,5,10,17,24,33,42,52,37,23,25] | $Y_{10,9,9,9,8,7,7,5,5,3,1}$ [216] | $Y_{10,9,9,9,8,7,7,5,5,3,1,1}$ [216] |
| | [3,1,2,1,0,1,0,2,0,1] | [1,5,10,17,25,33,42,51,37,23,25] | $Y_{10,9,9,9,8,7,7,6,4,2,2}$ [216] | $Y_{10,9,9,9,8,7,7,6,4,2,2,1}$ [216] |
| | [3,2,0,1,1,2,0,0,1,2] | [1,5,11,17,24,32,42,52,37,23,25] | $Y_{10,9,9,9,8,8,6,5,4,4,1}$ [192] | $Y_{10,9,9,9,8,8,6,5,4,4,1,1}$ [192] |
| | [3,2,0,1,2,0,0,2,0,1] | [1,5,11,17,24,33,42,51,37,23,25] | $Y_{10,9,9,9,8,8,6,5,5,2,2}$ [144] | $Y_{10,9,9,9,8,8,6,5,5,2,2,1}$ [144] |
| | [3,2,0,2,0,0,2,1,0,1] | [1,5,11,17,25,33,41,51,37,23,25] | $Y_{10,9,9,9,8,8,6,6,3,3,2}$ [144] | $Y_{10,9,9,9,8,8,6,6,3,3,2,1}$ [144] |
| | [3,2,1,0,0,2,1,1,0,1] | [1,5,11,18,25,32,41,51,37,23,25] | $Y_{10,9,9,9,8,8,7,4,4,3,2}$ [192] | $Y_{10,9,9,9,8,8,7,4,4,3,2,1}$ [192] |
| | [4,0,0,3,1,0,1,0,1,2] | [1,6,11,16,24,33,42,52,37,23,25] | $Y_{10,9,9,9,9,6,6,6,5,3,1}$ [144] | $Y_{10,9,9,9,9,6,6,6,5,3,1,1}$ [144] |
| | [4,0,1,1,1,1,1,1,0,1] | [1,6,11,17,24,32,41,51,37,23,25] | $Y_{10,9,9,9,9,7,6,5,4,3,2}$ [288] | $Y_{10,9,9,9,9,7,6,5,4,3,2,1}$ [288] |
| | [4,1,0,1,0,1,3,0,0,1] | [1,6,12,18,25,32,40,51,37,23,25] | $Y_{10,9,9,9,9,8,6,4,3,3,3}$ [144] | $Y_{10,9,9,9,9,8,6,4,3,3,3,1}$ [144] |
| | [4,3,0,1,1,0,0,0,2,3] | [0,4,11,18,26,35,44,53,37,23,25] | $Y_{9,9,9,9,8,8,8,6,5,1,1}$ [120] | $Y_{9,9,9,9,8,8,8,6,5,1,1,1}$ [120] |
| | [4,3,1,0,0,0,1,1,1,2] | [0,4,11,19,27,35,43,52,37,23,25] | $Y_{9,9,9,9,8,8,8,7,3,2,1}$ [160] | $Y_{9,9,9,9,8,8,8,7,3,2,1,1}$ [160] |
| | [5,0,0,0,0,4,0,1,0,1] | [1,7,13,19,25,31,41,51,37,23,25] | $Y_{10,9,9,9,9,9,4,4,4,4,2}$ [54] | $Y_{10,9,9,9,9,9,4,4,4,4,2,1}$ [54] |
| | [5,0,3,0,1,0,0,0,2,3] | [0,5,10,18,26,35,44,53,37,23,25] | $Y_{9,9,9,9,9,7,7,7,5,1,1}$ [90] | $Y_{9,9,9,9,9,7,7,7,5,1,1,1}$ [90] |
| | [5,1,0,3,0,0,0,0,2,3] | [0,5,11,17,26,35,44,53,37,23,25] | $Y_{9,9,9,9,9,8,6,6,6,1,1}$ [72] | $Y_{9,9,9,9,9,8,6,6,6,1,1,1}$ [72] |
| | [5,1,1,0,2,0,0,1,1,2] | [0,5,11,18,25,34,43,52,37,23,25] | $Y_{9,9,9,9,9,8,7,5,5,2,1}$ [192] | $Y_{9,9,9,9,9,8,7,5,5,2,1,1}$ [192] |
| | [5,1,1,1,0,0,2,0,1,2] | [0,5,11,18,26,34,42,52,37,23,25] | $Y_{9,9,9,9,9,8,7,6,3,3,1}$ [192] | $Y_{9,9,9,9,9,8,7,6,3,3,1,1}$ [192] |
| | [5,1,2,0,0,0,0,3,0,1] | [0,5,11,19,27,35,43,51,37,23,25] | $Y_{9,9,9,9,9,8,7,7,2,2,2}$ [72] | $Y_{9,9,9,9,9,8,7,7,2,2,2,1}$ [72] |
| | [5,2,0,0,0,2,1,0,1,2] | [0,5,12,19,26,33,42,52,37,23,25] | $Y_{9,9,9,9,9,8,8,4,4,3,1}$ [120] | $Y_{9,9,9,9,9,8,8,4,4,3,1,1}$ [120] |
| | [5,2,0,0,1,0,1,2,0,1] | [0,5,12,19,26,34,42,51,37,23,25] | $Y_{9,9,9,9,9,8,8,5,3,2,2}$ [144] | $Y_{9,9,9,9,9,8,8,5,3,2,2,1}$ [144] |
| | [6,0,0,1,1,1,1,0,1,2] | [0,6,12,18,25,33,42,52,37,23,25] | $Y_{9,9,9,9,9,9,6,5,4,3,1}$ [192] | $Y_{9,9,9,9,9,9,6,5,4,3,1,1}$ [192] |
| | [6,0,0,2,0,0,1,2,0,1] | [0,6,12,18,26,34,42,51,37,23,25] | $Y_{9,9,9,9,9,9,6,6,3,2,2}$ [96] | $Y_{9,9,9,9,9,9,6,6,3,2,2,1}$ [96] |
| | [6,0,1,0,0,2,0,2,0,1] | [0,6,12,19,26,33,42,51,37,23,25] | $Y_{9,9,9,9,9,9,7,4,4,2,2}$ [108] | $Y_{9,9,9,9,9,9,7,4,4,2,2,1}$ [108] |
| | [6,1,0,0,0,0,3,1,0,1] | [0,6,13,20,27,34,41,51,37,23,25] | $Y_{9,9,9,9,9,9,8,3,3,3,2}$ [72] | $Y_{9,9,9,9,9,9,8,3,3,3,2,1}$ [72] |
| | [0,1,1,3,2,0,0,0,0,3] | [3,6,10,15,23,33,43,53,38,23,25] | $Y_{10,10,10,8,7,6,6,6,5,5}$ [72] | $Y_{10,10,10,8,7,6,6,6,5,5,1,1,1}$ [72] |
| | [0,3,3,0,1,0,1,0,0,3] | [2,4,9,17,25,34,43,53,38,23,25] | $Y_{10,10,8,8,8,7,7,7,5,3}$ [108] | $Y_{10,10,8,8,8,7,7,7,5,3,1,1,1}$ [108] |
| | [0,4,1,0,2,1,0,0,0,3] | [2,4,10,17,24,33,43,53,38,23,25] | $Y_{10,10,8,8,8,8,7,5,5,4}$ [90] | $Y_{10,10,8,8,8,8,7,5,5,4,1,1,1}$ [90] |
| | [1,1,3,1,1,1,0,0,0,3] | [2,5,9,16,24,33,43,53,38,23,25] | $Y_{10,10,9,8,7,7,7,6,5,4}$ [160] | $Y_{10,10,9,8,7,7,7,6,5,4,1,1,1}$ [160] |
| | [1,2,1,1,3,0,0,0,0,3] | [2,5,10,16,23,33,43,53,38,23,25] | $Y_{10,10,9,8,8,7,6,5,5,5}$ [96] | $Y_{10,10,9,8,8,7,6,5,5,5,1,1,1}$ [96] |
| | [1,5,1,1,0,0,0,0,1,4] | [1,3,10,18,27,36,45,54,38,23,25] | $Y_{10,9,8,8,8,8,8,7,6,1}$ [96] | $Y_{10,9,8,8,8,8,8,7,6,1,1,1,1}$ [96] |
| | [1,6,0,0,0,1,0,1,0,3] | [1,3,11,19,27,35,44,53,38,23,25] | $Y_{10,9,8,8,8,8,8,8,4,2}$ [90] | $Y_{10,9,8,8,8,8,8,8,4,2,1,1,1}$ [90] |
| | [2,0,1,4,0,1,0,0,0,3] | [2,6,10,15,24,33,43,53,38,23,25] | $Y_{10,10,9,9,7,6,6,6,6,4}$ [90] | $Y_{10,10,9,9,7,6,6,6,6,4,1,1,1}$ [90] |
| | [2,2,3,1,0,0,0,1,0,3] | [1,4,9,17,26,35,44,53,38,23,25] | $Y_{10,9,9,8,8,7,7,7,6,2}$ [120] | $Y_{10,9,9,8,8,7,7,7,6,2,1,1,1}$ [120] |
| | [2,3,1,1,0,2,0,0,0,3] | [1,4,10,17,25,33,43,53,38,23,25] | $Y_{10,9,9,8,8,8,7,6,4,4}$ [120] | $Y_{10,9,9,8,8,8,7,6,4,4,1,1,1}$ [120] |
| | [3,0,4,0,1,0,1,0,0,3] | [1,5,9,17,25,34,43,53,38,23,25] | $Y_{10,9,9,9,7,7,7,7,5,3}$ [108] | $Y_{10,9,9,9,7,7,7,7,5,3,1,1,1}$ [108] |
| | [3,1,1,2,1,1,0,0,0,3] | [1,5,10,16,24,33,43,53,38,23,25] | $Y_{10,9,9,9,8,7,6,6,5,4}$ [160] | $Y_{10,9,9,9,8,7,6,6,5,4,1,1,1}$ [160] |
| | [4,0,1,0,4,0,0,0,0,3] | [1,6,11,17,23,33,43,53,38,23,25] | $Y_{10,9,9,9,9,7,5,5,5,5}$ [54] | $Y_{10,9,9,9,9,7,5,5,5,5,1,1,1}$ [54] |
| | [4,2,2,0,1,0,0,1,0,3] | [0,4,10,18,26,35,44,53,38,23,25] | $Y_{9,9,9,9,8,8,7,7,5,2}$ [144] | $Y_{9,9,9,9,8,8,7,7,5,2,1,1,1}$ [144] |
| | [4,3,0,1,0,1,1,0,0,3] | [0,4,11,18,26,34,43,53,38,23,25] | $Y_{9,9,9,9,8,8,8,6,4,3}$ [144] | $Y_{9,9,9,9,8,8,8,6,4,3,1,1,1}$ [144] |
| | [5,0,2,2,0,0,0,1,0,3] | [0,5,10,17,26,35,44,53,38,23,25] | $Y_{9,9,9,9,9,7,7,6,6,2}$ [90] | $Y_{9,9,9,9,9,7,7,6,6,2,1,1,1}$ [90] |
| | [5,0,3,0,0,1,1,0,0,3] | [0,5,10,18,26,34,43,53,38,23,25] | $Y_{9,9,9,9,9,7,7,7,4,3}$ [96] | $Y_{9,9,9,9,9,7,7,7,4,3,1,1,1}$ [96] |
| | [5,1,0,2,1,0,1,0,0,3] | [0,5,11,17,25,34,43,53,38,23,25] | $Y_{9,9,9,9,9,8,6,6,5,3}$ [144] | $Y_{9,9,9,9,9,8,6,6,5,3,1,1,1}$ [144] |
| | [5,1,1,0,1,2,0,0,0,3] | [0,5,11,18,25,33,43,53,38,23,25] | $Y_{9,9,9,9,9,8,7,5,4,4}$ [120] | $Y_{9,9,9,9,9,8,7,5,4,4,1,1,1}$ [120] |
| | [3,5,0,1,0,0,0,0,0,5] | [0,3,11,19,28,37,46,55,39,23,25] | $Y_{9,9,9,8,8,8,8,8,8,6}$ [42] | $Y_{9,9,9,8,8,8,8,8,8,6,1,1,1,1,1}$ [42] |
| | [4,2,0,1,0,0,0,0,7,0] | [1,6,13,20,28,36,44,52,34,23,26] | $Y_{10,9,9,9,9,8,8,6,1,1,1,1,1,1,1}$ [42] | $Y_{10,9,9,9,9,8,8,6}$ [42] |
| | [0,2,0,4,0,0,0,0,5,0] | [3,6,11,16,25,34,43,52,35,23,26] | $Y_{10,10,10,8,8,6,6,6,6,1,1,1,1,1}$ [31] | $Y_{10,10,10,8,8,6,6,6,6}$ [32] |
| | [0,6,0,0,0,0,0,1,5,0] | [2,4,12,20,28,36,44,52,35,23,26] | $Y_{10,10,8,8,8,8,8,8,2,1,1,1,1,1}$ [31] | $Y_{10,10,8,8,8,8,8,8,2}$ [32] |
| | [1,3,0,2,1,0,0,0,5,0] | [2,5,11,17,25,34,43,52,35,23,26] | $Y_{10,10,9,8,8,6,6,5,1,1,1,1,1}$ [72] | $Y_{10,10,9,8,8,6,6,5}$ [72] |
| | [3,2,1,1,0,1,0,0,5,0] | [1,5,11,18,26,34,43,52,35,23,26] | $Y_{10,9,9,9,8,8,7,6,4,1,1,1,1,1}$ [120] | $Y_{10,9,9,9,8,8,7,6,4}$ [120] |
| | [4,0,2,0,2,0,0,0,5,0] | [1,6,11,18,25,34,43,52,35,23,26] | $Y_{10,9,9,9,9,7,7,5,5,1,1,1,1,1}$ [54] | $Y_{10,9,9,9,9,7,7,5,5}$ [54] |
| | [5,3,0,0,0,0,0,0,6,1] | [0,5,13,21,29,37,45,53,35,23,26] | $Y_{9,9,9,9,9,8,8,8,1,1,1,1,1,1}$ [32] | $Y_{9,9,9,9,9,8,8,8,1}$ [32] |
| | [6,0,2,0,0,0,0,1,5,0] | [0,6,12,20,28,36,44,52,35,23,26] | $Y_{9,9,9,9,9,9,7,7,2,1,1,1,1,1}$ [54] | $Y_{9,9,9,9,9,9,7,7,2}$ [54] |
| | [6,1,0,0,1,0,1,0,5,0] | [0,6,13,20,27,35,43,52,35,23,26] | $Y_{9,9,9,9,9,9,8,5,3,1,1,1,1,1}$ [96] | $Y_{9,9,9,9,9,9,8,5,3}$ [96] |
| | [0,1,2,1,2,1,0,0,3,0] | [3,6,10,16,23,32,42,52,36,23,26] | $Y_{10,10,10,8,7,7,6,5,5,4,1,1,1}$ [120] | $Y_{10,10,10,8,7,7,6,5,5,4}$ [120] |
| | [0,4,1,1,1,0,0,1,3,0] | [2,4,10,17,25,34,43,52,36,23,26] | $Y_{10,10,8,8,8,8,7,6,5,2,1,1,1}$ [144] | $Y_{10,10,8,8,8,8,7,6,5,2}$ [144] |
| | [0,4,2,0,0,0,2,0,3,0] | [2,4,10,18,26,34,42,52,36,23,26] | $Y_{10,10,8,8,8,8,7,7,3,3,1,1,1}$ [60] | $Y_{10,10,8,8,8,8,7,7,3,3}$ [60] |
| | [0,5,0,0,1,1,1,0,3,0] | [2,4,11,18,25,33,42,52,36,23,26] | $Y_{10,10,8,8,8,8,8,5,4,3,1,1,1}$ [96] | $Y_{10,10,8,8,8,8,8,5,4,3}$ [96] |
| | [1,0,0,5,0,0,1,0,3,0] | [3,7,11,15,24,33,42,52,36,23,26] | $Y_{10,10,10,9,6,6,6,6,6,3,1,1,1}$ [64] | $Y_{10,10,10,9,6,6,6,6,6,3}$ [64] |
| | [1,2,1,2,1,0,1,0,3,0] | [2,5,10,16,24,33,42,52,36,23,26] | $Y_{10,10,9,8,8,7,6,6,5,3,1,1,1}$ [192] | $Y_{10,10,9,8,8,7,6,6,5,3}$ [192] |
| | [1,2,2,0,1,2,0,0,3,0] | [2,5,10,17,24,32,42,52,36,23,26] | $Y_{10,10,9,8,8,7,7,5,4,4,1,1,1}$ [120] | $Y_{10,10,9,8,8,7,7,5,4,4}$ [120] |
| | [2,0,2,2,0,2,0,0,3,0] | [2,6,10,16,24,32,42,52,36,23,26] | $Y_{10,10,9,9,7,7,6,6,4,4,1,1,1}$ [90] | $Y_{10,10,9,9,7,7,6,6,4,4}$ [90] |
| | [2,1,0,2,2,1,0,0,3,0] | [2,6,11,16,23,32,42,52,36,23,26] | $Y_{10,10,9,9,8,6,6,5,5,4,1,1,1}$ [120] | $Y_{10,10,9,9,8,6,6,5,5,4}$ [120] |

| | | | | |
|---|---|---|---|---|
| | [2,3,1,2,0,0,0,0,4,1] | [1,4,10,17,26,35,44,53,36,23,26] | $Y_{10,9,9,8,8,8,7,6,6,1,1,1,1}$ [96] | $Y_{10,9,9,8,8,8,7,6,6,1}$ [96] |
| | [2,3,2,0,0,1,0,1,3,0] | [1,4,10,18,26,34,43,52,36,23,26] | $Y_{10,9,9,8,8,8,7,7,4,2,1,1,1}$ [144] | $Y_{10,9,9,8,8,8,7,7,4,2}$ [144] |
| | [2,4,0,0,2,0,0,1,3,0] | [1,4,11,18,25,34,43,52,36,23,26] | $Y_{10,9,9,8,8,8,8,5,5,2,1,1,1}$ [96] | $Y_{10,9,9,8,8,8,8,5,5,2}$ [96] |
| | [2,4,0,1,0,0,2,0,3,0] | [1,4,11,18,26,34,42,52,36,23,26] | $Y_{10,9,9,8,8,8,8,6,3,3,1,1,1}$ [96] | $Y_{10,9,9,8,8,8,8,6,3,3}$ [96] |
| | [3,1,2,1,0,1,1,0,3,0] | [1,5,10,17,25,33,42,52,36,23,26] | $Y_{10,9,9,9,8,7,7,6,4,3,1,1,1}$ [192] | $Y_{10,9,9,9,8,7,7,6,4,3}$ [192] |
| | [3,2,0,1,2,0,1,0,3,0] | [1,5,11,17,24,33,42,52,36,23,26] | $Y_{10,9,9,9,8,8,6,5,5,3,1,1,1}$ [144] | $Y_{10,9,9,9,8,8,6,5,5,3}$ [144] |
| | [3,2,1,0,0,3,0,0,3,0] | [1,5,11,18,25,32,42,52,36,23,26] | $Y_{10,9,9,9,8,8,7,4,4,4,1,1,1}$ [80] | $Y_{10,9,9,9,8,8,7,4,4,4}$ [80] |
| | [4,0,0,4,0,0,0,1,3,0] | [1,6,11,16,25,34,43,52,36,23,26] | $Y_{10,9,9,9,9,6,6,6,6,2,1,1,1}$ [60] | $Y_{10,9,9,9,9,6,6,6,6,2}$ [60] |
| | [4,0,1,1,1,2,0,0,3,0] | [1,6,11,17,24,32,42,52,36,23,26] | $Y_{10,9,9,9,9,7,6,5,4,4,1,1,1}$ [120] | $Y_{10,9,9,9,9,7,6,5,4,4}$ [120] |
| | [4,3,1,0,0,1,0,0,4,1] | [0,4,11,19,27,35,44,53,36,23,26] | $Y_{9,9,9,9,8,8,8,7,4,1,1,1,1}$ [128] | $Y_{9,9,9,9,8,8,8,7,4,1}$ [128] |
| | [4,4,0,0,0,0,0,2,3,0] | [0,4,12,20,28,36,44,52,36,23,26] | $Y_{9,9,9,9,8,8,8,8,2,2,1,1,1}$ [42] | $Y_{9,9,9,9,8,8,8,8,2,2}$ [42] |
| | [5,1,1,1,0,1,0,1,3,0] | [0,5,11,18,26,34,43,52,36,23,26] | $Y_{9,9,9,9,9,8,7,6,4,2,1,1,1}$ [216] | $Y_{9,9,9,9,9,8,7,6,4,2}$ [216] |
| | [5,2,0,0,1,0,2,0,3,0] | [0,5,12,19,26,34,42,52,36,23,26] | $Y_{9,9,9,9,9,8,8,5,3,3,1,1,1}$ [96] | $Y_{9,9,9,9,9,8,8,5,3,3}$ [96] |
| | [6,0,0,1,2,0,0,1,3,0] | [0,6,12,18,25,34,43,52,36,23,26] | $Y_{9,9,9,9,9,9,6,5,5,2,1,1,1}$ [96] | $Y_{9,9,9,9,9,9,6,5,5,2}$ [96] |
| | [6,0,0,2,0,0,2,0,3,0] | [0,6,12,18,26,34,42,52,36,23,26] | $Y_{9,9,9,9,9,9,6,6,3,3,1,1,1}$ [64] | $Y_{9,9,9,9,9,9,6,6,3,3}$ [64] |
| | [6,0,1,0,0,2,1,0,3,0] | [0,6,12,19,26,33,42,52,36,23,26] | $Y_{9,9,9,9,9,9,7,4,4,3,1,1,1}$ [96] | $Y_{9,9,9,9,9,9,7,4,4,3}$ [96] |
| | [0,0,0,3,0,4,0,0,1,0] | [4,8,12,16,23,30,41,52,37,23,26] | $Y_{10,10,10,10,6,6,6,4,4,4,4,1}$ [37] | $Y_{10,10,10,10,6,6,6,4,4,4,4}$ [38] |
| | [0,0,3,3,0,1,0,0,2,1] | [3,6,9,15,24,33,43,53,37,23,26] | $Y_{10,10,10,7,7,7,6,6,6,4,1,1}$ [96] | $Y_{10,10,10,7,7,7,6,6,6,4,1}$ [96] |
| | [0,0,4,0,3,0,0,0,2,1] | [3,6,9,16,23,33,43,53,37,23,26] | $Y_{10,10,10,7,7,7,7,5,5,5,1,1}$ [60] | $Y_{10,10,10,7,7,7,7,5,5,5,1}$ [60] |
| | [0,0,4,1,0,2,0,1,1,0] | [3,6,9,16,24,32,42,52,37,23,26] | $Y_{10,10,10,7,7,7,7,6,4,4,2,1}$ [108] | $Y_{10,10,10,7,7,7,7,6,4,4,2}$ [108] |
| | [0,0,5,0,0,0,3,0,1,0] | [3,6,9,17,25,33,41,52,37,23,26] | $Y_{10,10,10,7,7,7,7,7,3,3,3,1}$ [40] | $Y_{10,10,10,7,7,7,7,7,3,3,3}$ [40] |
| | [0,1,1,3,1,1,0,1,1,0] | [3,6,10,15,23,32,42,52,37,23,26] | $Y_{10,10,10,8,7,6,6,6,5,4,2,1}$ [216] | $Y_{10,10,10,8,7,6,6,6,5,4,2}$ [216] |
| | [0,1,2,1,1,2,1,0,1,0] | [3,6,10,16,23,31,41,52,37,23,26] | $Y_{10,10,10,8,7,7,6,5,4,4,3,1}$ [192] | $Y_{10,10,10,8,7,7,6,5,4,4,3}$ [192] |
| | [0,3,0,0,0,5,0,0,1,0] | [3,6,12,18,24,30,41,52,37,23,26] | $Y_{10,10,10,8,8,8,4,4,4,4,4,1}$ [37] | $Y_{10,10,10,8,8,8,4,4,4,4,4}$ [38] |
| | [0,3,2,2,0,0,1,0,2,1] | [2,4,9,16,25,34,43,53,37,23,26] | $Y_{10,10,8,8,8,7,7,6,6,3,1,1}$ [144] | $Y_{10,10,8,8,8,7,7,6,6,3,1}$ [144] |
| | [0,3,3,0,0,2,0,0,2,1] | [2,4,9,17,25,33,43,53,37,23,26] | $Y_{10,10,8,8,8,7,7,7,4,4,1,1}$ [96] | $Y_{10,10,8,8,8,7,7,7,4,4,1}$ [96] |
| | [0,3,3,0,1,0,0,2,1,0] | [2,4,9,17,25,34,43,52,37,23,26] | $Y_{10,10,8,8,8,7,7,7,5,2,2,1}$ [108] | $Y_{10,10,8,8,8,7,7,7,5,2,2}$ [108] |
| | [0,4,0,2,1,1,0,0,2,1] | [2,4,10,16,24,33,43,53,37,23,26] | $Y_{10,10,8,8,8,8,6,6,5,4,1,1}$ [144] | $Y_{10,10,8,8,8,8,6,6,5,4,1}$ [144] |
| | [0,4,0,3,0,0,0,2,1,0] | [2,4,10,16,25,34,43,52,37,23,26] | $Y_{10,10,8,8,8,8,6,6,6,2,2,1}$ [67] | $Y_{10,10,8,8,8,8,6,6,6,2,2}$ [68] |
| | [0,4,1,0,2,0,1,1,1,0] | [2,4,10,17,24,33,42,52,37,23,26] | $Y_{10,10,8,8,8,8,7,5,5,3,2,1}$ [162] | $Y_{10,10,8,8,8,8,7,5,5,3,2}$ [162] |
| | [0,5,0,0,0,3,0,1,1,0] | [2,4,11,18,25,32,42,52,37,23,26] | $Y_{10,10,8,8,8,8,8,4,4,4,2,1}$ [67] | $Y_{10,10,8,8,8,8,8,4,4,4,2}$ [68] |
| | [1,0,0,4,1,0,2,0,1,0] | [3,7,11,15,23,32,41,52,37,23,26] | $Y_{10,10,10,9,6,6,6,6,5,3,3,1}$ [96] | $Y_{10,10,10,9,6,6,6,6,5,3,3}$ [96] |
| | [1,0,2,0,1,4,0,0,1,0] | [3,7,11,17,23,30,41,52,37,23,26] | $Y_{10,10,10,9,7,7,5,4,4,4,4,1}$ [90] | $Y_{10,10,10,9,7,7,5,4,4,4,4}$ [90] |
| | [1,1,3,1,1,0,1,1,1,0] | [2,5,9,16,24,33,42,52,37,23,26] | $Y_{10,10,9,8,7,7,7,6,5,3,2,1}$ [288] | $Y_{10,10,9,8,7,7,7,6,5,3,2}$ [288] |
| | [1,2,0,4,0,1,0,0,2,1] | [2,5,10,15,24,33,43,53,37,23,26] | $Y_{10,10,9,8,8,6,6,6,6,4,1,1}$ [144] | $Y_{10,10,9,8,8,6,6,6,6,4,1}$ [144] |
| | [1,2,1,1,2,1,0,1,1,0] | [2,5,10,16,23,32,42,52,37,23,26] | $Y_{10,10,9,8,8,7,6,5,5,4,2,1}$ [288] | $Y_{10,10,9,8,8,7,6,5,5,4,2}$ [288] |
| | [1,2,1,2,0,1,2,0,1,0] | [2,5,10,16,24,32,41,52,37,23,26] | $Y_{10,10,9,8,8,7,6,6,4,3,3,1}$ [192] | $Y_{10,10,9,8,8,7,6,6,4,3,3}$ [192] |
| | [1,3,0,0,3,0,2,0,1,0] | [2,5,11,17,23,32,41,52,37,23,26] | $Y_{10,10,9,8,8,8,5,5,5,3,3,1}$ [96] | $Y_{10,10,9,8,8,8,5,5,5,3,3}$ [96] |
| | [1,3,0,1,0,3,1,0,1,0] | [2,5,11,17,24,31,41,52,37,23,26] | $Y_{10,10,9,8,8,8,6,4,4,4,3,1}$ [144] | $Y_{10,10,9,8,8,8,6,4,4,4,3}$ [144] |
| | [1,5,1,0,1,0,0,1,2,1] | [1,3,10,18,26,35,44,53,37,23,26] | $Y_{10,9,8,8,8,8,8,7,5,2,1,1}$ [192] | $Y_{10,9,8,8,8,8,8,7,5,2,1}$ [192] |
| | [1,6,0,0,0,0,2,0,2,1] | [1,3,11,19,27,35,43,53,37,23,26] | $Y_{10,9,8,8,8,8,8,8,3,3,1,1}$ [72] | $Y_{10,9,8,8,8,8,8,8,3,3,1}$ [72] |
| | [2,0,1,3,2,0,0,0,2,1] | [2,6,10,15,23,33,43,53,37,23,26] | $Y_{10,10,9,9,7,6,6,6,5,5,1,1}$ [120] | $Y_{10,10,9,9,7,6,6,6,5,5,1}$ [120] |
| | [2,0,1,4,0,0,1,1,1,0] | [2,6,10,15,24,33,42,52,37,23,26] | $Y_{10,10,9,9,7,6,6,6,6,3,2,1}$ [144] | $Y_{10,10,9,9,7,6,6,6,6,3,2}$ [144] |
| | [2,0,2,1,2,0,2,0,1,0] | [2,6,10,16,23,32,41,52,37,23,26] | $Y_{10,10,9,9,7,7,6,5,5,3,3,1}$ [144] | $Y_{10,10,9,9,7,7,6,5,5,3,3}$ [144] |
| | [2,0,3,0,0,3,1,0,1,0] | [2,6,10,17,24,31,41,52,37,23,26] | $Y_{10,10,9,9,7,7,7,4,4,4,3,1}$ [96] | $Y_{10,10,9,9,7,7,7,4,4,4,3}$ [96] |
| | [2,1,0,2,1,2,1,0,1,0] | [2,6,11,16,23,31,41,52,37,23,26] | $Y_{10,10,9,9,8,6,6,5,4,4,3,1}$ [192] | $Y_{10,10,9,9,8,6,6,5,4,4,3}$ [192] |
| | [2,2,3,0,1,0,1,0,2,1] | [1,4,9,17,25,34,43,53,37,23,26] | $Y_{10,9,9,8,8,7,7,7,5,3,1,1}$ [216] | $Y_{10,9,9,8,8,7,7,7,5,3,1}$ [216] |
| | [2,3,0,3,0,0,1,0,2,1] | [1,4,10,16,25,34,43,53,37,23,26] | $Y_{10,9,9,8,8,8,6,6,6,3,1,1}$ [144] | $Y_{10,9,9,8,8,8,6,6,6,3,1}$ [144] |
| | [2,3,1,0,2,1,0,0,2,1] | [1,4,10,17,24,33,43,53,37,23,26] | $Y_{10,9,9,8,8,8,7,5,5,4,1,1}$ [192] | $Y_{10,9,9,8,8,8,7,5,5,4,1}$ [192] |
| | [2,3,1,1,0,1,1,1,1,0] | [1,4,10,17,25,33,42,52,37,23,26] | $Y_{10,9,9,8,8,8,7,6,4,3,2,1}$ [288] | $Y_{10,9,9,8,8,8,7,6,4,3,2}$ [288] |
| | [3,0,1,0,0,5,0,0,1,0] | [2,7,12,18,24,30,41,52,37,23,26] | $Y_{10,10,9,9,9,7,4,4,4,4,4,1}$ [60] | $Y_{10,10,9,9,9,7,4,4,4,4,4}$ [60] |
| | [3,0,3,2,0,0,1,0,2,1] | [1,5,9,16,25,34,43,53,37,23,26] | $Y_{10,9,9,9,7,7,7,6,6,3,1,1}$ [144] | $Y_{10,9,9,9,7,7,7,6,6,3,1}$ [144] |
| | [3,0,4,0,0,2,0,0,2,1] | [1,5,9,17,25,33,43,53,37,23,26] | $Y_{10,9,9,9,7,7,7,7,4,4,1,1}$ [96] | $Y_{10,9,9,9,7,7,7,7,4,4,1}$ [96] |
| | [3,0,4,0,1,0,0,2,1,0] | [1,5,9,17,25,34,43,52,37,23,26] | $Y_{10,9,9,9,7,7,7,7,5,2,2,1}$ [108] | $Y_{10,9,9,9,7,7,7,7,5,2,2}$ [108] |
| | [3,1,1,2,1,0,1,1,1,0] | [1,5,10,16,24,33,42,52,37,23,26] | $Y_{10,9,9,9,8,7,6,6,5,3,2,1}$ [288] | $Y_{10,9,9,9,8,7,6,6,5,3,2}$ [288] |
| | [3,1,2,0,1,2,0,1,1,0] | [1,5,10,17,24,32,42,52,37,23,26] | $Y_{10,9,9,9,8,7,7,5,4,4,2,1}$ [216] | $Y_{10,9,9,9,8,7,7,5,4,4,2}$ [216] |
| | [3,1,2,1,0,0,3,0,1,0] | [1,5,10,17,25,33,41,52,37,23,26] | $Y_{10,9,9,9,8,7,7,6,3,3,3,1}$ [128] | $Y_{10,9,9,9,8,7,7,6,3,3,3}$ [128] |
| | [3,2,0,0,4,0,0,0,2,1] | [1,5,11,17,23,33,43,53,37,23,26] | $Y_{10,9,9,9,8,8,5,5,5,5,1,1}$ [80] | $Y_{10,9,9,9,8,8,5,5,5,5,1}$ [80] |
| | [3,2,0,1,1,1,2,0,1,0] | [1,5,11,17,24,32,41,52,37,23,26] | $Y_{10,9,9,9,8,8,6,5,4,3,3,1}$ [192] | $Y_{10,9,9,9,8,8,6,5,4,3,3}$ [192] |
| | [3,5,0,0,1,0,0,0,3,2] | [0,3,11,19,27,36,45,54,37,23,26] | $Y_{9,9,9,8,8,8,8,8,5,1,1,1}$ [80] | $Y_{9,9,9,8,8,8,8,8,5,1,1}$ [80] |
| | [4,0,0,2,3,0,0,0,2,1] | [1,6,11,16,23,33,43,53,37,23,26] | $Y_{10,9,9,9,9,6,6,5,5,5,1,1}$ [80] | $Y_{10,9,9,9,9,6,6,5,5,5,1}$ [80] |
| | [4,0,0,3,0,2,0,1,1,0] | [1,6,11,16,24,32,42,52,37,23,26] | $Y_{10,9,9,9,9,6,6,6,4,4,2,1}$ [108] | $Y_{10,9,9,9,9,6,6,6,4,4,2}$ [108] |
| | [4,0,1,0,3,1,0,1,1,0] | [1,6,11,17,23,32,42,52,37,23,26] | $Y_{10,9,9,9,9,7,5,5,5,4,2,1}$ [162] | $Y_{10,9,9,9,9,7,5,5,5,4,2}$ [162] |
| | [4,1,0,0,1,3,1,0,1,0] | [1,6,12,18,24,31,41,52,37,23,26] | $Y_{10,9,9,9,9,8,5,4,4,4,3,1}$ [128] | $Y_{10,9,9,9,9,8,5,4,4,4,3}$ [128] |
| | [4,2,1,2,0,0,0,1,2,1] | [0,4,10,17,26,35,44,53,37,23,26] | $Y_{9,9,9,9,8,8,7,6,6,2,1,1}$ [160] | $Y_{9,9,9,9,8,8,7,6,6,2,1}$ [160] |
| | [4,2,2,0,0,1,1,0,2,1] | [0,4,10,18,26,34,43,53,37,23,26] | $Y_{9,9,9,9,8,8,7,7,4,3,1,1}$ [192] | $Y_{9,9,9,9,8,8,7,7,4,3,1}$ [192] |
| | [4,3,0,0,2,0,1,0,2,1] | [0,4,11,18,25,34,43,53,37,23,26] | $Y_{9,9,9,9,8,8,8,5,5,3,1,1}$ [144] | $Y_{9,9,9,9,8,8,8,5,5,3,1}$ [144] |
| | [4,3,0,1,0,1,0,2,1,0] | [0,4,11,18,26,34,43,52,37,23,26] | $Y_{9,9,9,9,8,8,8,6,4,2,2,1}$ [162] | $Y_{9,9,9,9,8,8,8,6,4,2,2}$ [162] |
| | [5,0,2,1,1,0,1,0,2,1] | [0,5,10,17,25,34,43,53,37,23,26] | $Y_{9,9,9,9,9,7,7,6,5,3,1,1}$ [216] | $Y_{9,9,9,9,9,7,7,6,5,3,1}$ [216] |
| | [5,0,3,0,0,1,0,2,1,0] | [0,5,10,18,26,34,43,52,37,23,26] | $Y_{9,9,9,9,9,7,7,7,4,2,2,1}$ [108] | $Y_{9,9,9,9,9,7,7,7,4,2,2}$ [108] |
| | [5,1,0,2,0,2,0,0,2,1] | [0,5,11,17,25,33,43,53,37,23,26] | $Y_{9,9,9,9,9,8,6,6,4,4,1,1}$ [144] | $Y_{9,9,9,9,9,8,6,6,4,4,1}$ [144] |

| | | | | |
|---|---|---|---|---|
| | [5,1,0,2,1,0,0,2,1,0] | [0,5,11,17,25,34,43,52,37,23,26] | $Y_{9,9,9,9,9,8,6,6,5,2,2,1}$ [144] | $Y_{9,9,9,9,9,8,6,6,5,2,2}$ [144] |
| | [5,1,1,0,1,1,1,1,1,0] | [0,5,11,18,25,33,42,52,37,23,26] | $Y_{9,9,9,9,9,8,7,5,4,3,2,1}$ [288] | $Y_{9,9,9,9,9,8,7,5,4,3,2}$ [288] |
| | [6,0,0,0,3,1,0,0,2,1] | [0,6,12,18,24,33,43,53,37,23,26] | $Y_{9,9,9,9,9,9,5,5,5,4,1,1}$ [80] | $Y_{9,9,9,9,9,9,5,5,5,4,1}$ [80] |
| | [6,0,1,0,0,1,3,0,1,0] | [0,6,12,19,26,33,41,52,37,23,26] | $Y_{9,9,9,9,9,9,7,4,3,3,3,1}$ [96] | $Y_{9,9,9,9,9,9,7,4,3,3,3}$ [96] |
| | [0,0,3,2,2,0,0,1,0,1] | [3,6,9,15,23,33,43,53,38,23,26] | $Y_{10,10,10,7,7,7,6,6,5,5,2}$ [96] | $Y_{10,10,10,7,7,7,6,6,5,5,2,1}$ [96] |
| | [0,0,3,3,0,0,2,0,0,1] | [3,6,9,15,24,33,42,53,38,23,26] | $Y_{10,10,10,7,7,7,6,6,6,3,3}$ [64] | $Y_{10,10,10,7,7,7,6,6,6,3,3,1}$ [64] |
| | [0,0,4,0,2,1,1,0,0,1] | [3,6,9,16,23,32,42,53,38,23,26] | $Y_{10,10,10,7,7,7,7,5,5,4,3}$ [96] | $Y_{10,10,10,7,7,7,7,5,5,4,3,1}$ [96] |
| | [0,2,5,0,0,0,1,0,1,2] | [2,4,8,17,26,35,44,54,38,23,26] | $Y_{10,10,8,8,7,7,7,7,7,3,1}$ [90] | $Y_{10,10,8,8,7,7,7,7,7,3,1,1}$ [90] |
| | [0,3,2,1,1,1,0,1,0,1] | [2,4,9,16,24,33,43,53,38,23,26] | $Y_{10,10,8,8,8,7,7,6,5,4,2}$ [216] | $Y_{10,10,8,8,8,7,7,6,5,4,2,1}$ [216] |
| | [0,3,3,0,0,1,2,0,0,1] | [2,4,9,17,25,33,42,53,38,23,26] | $Y_{10,10,8,8,8,7,7,7,4,3,3}$ [96] | $Y_{10,10,8,8,8,7,7,7,4,3,3,1}$ [96] |
| | [0,4,0,2,1,0,2,0,0,1] | [2,4,10,16,24,33,42,53,38,23,26] | $Y_{10,10,8,8,8,8,6,6,5,3,3}$ [108] | $Y_{10,10,8,8,8,8,6,6,5,3,3,1}$ [108] |
| | [0,4,1,0,1,2,1,0,0,1] | [2,4,10,17,24,32,42,53,38,23,26] | $Y_{10,10,8,8,8,8,7,5,4,4,3}$ [144] | $Y_{10,10,8,8,8,8,7,5,4,4,3,1}$ [144] |
| | [1,0,0,4,0,3,0,0,0,1] | [3,7,11,15,23,31,42,53,38,23,26] | $Y_{10,10,10,9,6,6,6,6,4,4,4}$ [60] | $Y_{10,10,10,9,6,6,6,6,4,4,4,1}$ [60] |
| | [1,0,5,1,0,1,0,0,1,2] | [2,5,8,16,25,34,44,54,38,23,26] | $Y_{10,10,9,7,7,7,7,7,6,4,1}$ [144] | $Y_{10,10,9,7,7,7,7,7,6,4,1,1}$ [144] |
| | [1,0,6,0,0,0,0,2,0,1] | [2,5,8,17,26,35,44,53,38,23,26] | $Y_{10,10,9,7,7,7,7,7,7,2,2}$ [54] | $Y_{10,10,9,7,7,7,7,7,7,2,2,1}$ [54] |
| | [1,1,2,3,0,1,0,1,0,1] | [2,5,9,15,24,33,43,53,38,23,26] | $Y_{10,10,9,8,7,7,6,6,6,4,2}$ [216] | $Y_{10,10,9,8,7,7,6,6,6,4,2,1}$ [216] |
| | [1,1,3,0,3,0,0,1,0,1] | [2,5,9,16,23,33,43,53,38,23,26] | $Y_{10,10,9,8,7,7,7,5,5,5,2}$ [144] | $Y_{10,10,9,8,7,7,7,5,5,5,2,1}$ [144] |
| | [1,1,3,1,0,2,1,0,0,1] | [2,5,9,16,24,32,42,53,38,23,26] | $Y_{10,10,9,8,7,7,7,6,4,4,3}$ [192] | $Y_{10,10,9,8,7,7,7,6,4,4,3,1}$ [192] |
| | [1,2,0,3,2,0,0,1,0,1] | [2,5,10,15,23,33,43,53,38,23,26] | $Y_{10,10,9,8,8,6,6,6,5,5,2}$ [144] | $Y_{10,10,9,8,8,6,6,6,5,5,2,1}$ [144] |
| | [1,2,0,4,0,0,2,0,0,1] | [2,5,10,15,24,33,42,53,38,23,26] | $Y_{10,10,9,8,8,6,6,6,6,3,3}$ [96] | $Y_{10,10,9,8,8,6,6,6,6,3,3,1}$ [96] |
| | [1,2,2,0,0,4,0,0,0,1] | [2,5,10,17,24,31,42,53,38,23,26] | $Y_{10,10,9,8,8,7,7,4,4,4,4}$ [80] | $Y_{10,10,9,8,8,7,7,4,4,4,4,1}$ [80] |
| | [1,3,0,0,2,3,0,0,0,1] | [2,5,11,17,23,31,42,53,38,23,26] | $Y_{10,10,9,8,8,8,5,5,4,4,4}$ [80] | $Y_{10,10,9,8,8,8,5,5,4,4,4,1}$ [80] |
| | [1,4,2,1,0,0,1,0,1,2] | [1,3,9,17,26,35,44,54,38,23,26] | $Y_{10,9,8,8,8,8,7,7,6,3,1}$ [192] | $Y_{10,9,8,8,8,8,7,7,6,3,1,1}$ [192] |
| | [1,5,0,1,1,1,0,0,1,2] | [1,3,10,17,25,34,44,54,38,23,26] | $Y_{10,9,8,8,8,8,8,6,5,4,1}$ [192] | $Y_{10,9,8,8,8,8,8,6,5,4,1,1}$ [192] |
| | [1,5,0,2,0,0,0,2,0,1] | [1,3,10,17,26,35,44,53,38,23,26] | $Y_{10,9,8,8,8,8,8,6,6,2,2}$ [90] | $Y_{10,9,8,8,8,8,8,6,6,2,2,1}$ [90] |
| | [1,5,1,0,0,1,1,1,0,1] | [1,3,10,18,26,34,43,53,38,23,26] | $Y_{10,9,8,8,8,8,8,7,4,3,2}$ [192] | $Y_{10,9,8,8,8,8,8,7,4,3,2,1}$ [192] |
| | [2,0,1,3,1,1,1,0,0,1] | [2,6,10,15,23,32,42,53,38,23,26] | $Y_{10,10,9,9,7,6,6,6,5,4,3}$ [192] | $Y_{10,10,9,9,7,6,6,6,5,4,3,1}$ [192] |
| | [2,0,2,1,1,3,0,0,0,1] | [2,6,10,16,23,31,42,53,38,23,26] | $Y_{10,10,9,9,7,7,6,5,4,4,4}$ [120] | $Y_{10,10,9,9,7,7,6,5,4,4,4,1}$ [120] |
| | [2,2,2,1,2,0,0,0,1,2] | [1,4,9,16,24,34,44,54,38,23,26] | $Y_{10,9,9,8,8,7,7,6,5,5,1}$ [160] | $Y_{10,9,9,8,8,7,7,6,5,5,1,1}$ [160] |
| | [2,2,2,2,0,0,1,1,0,1] | [1,4,9,16,25,34,43,53,38,23,26] | $Y_{10,9,9,8,8,7,7,6,6,3,2}$ [192] | $Y_{10,9,9,8,8,7,7,6,6,3,2,1}$ [192] |
| | [2,2,3,0,0,2,0,1,0,1] | [1,4,9,17,25,33,43,53,38,23,26] | $Y_{10,9,9,8,8,7,7,7,4,4,2}$ [144] | $Y_{10,9,9,8,8,7,7,7,4,4,2,1}$ [144] |
| | [2,3,0,2,1,1,0,1,0,1] | [1,4,10,16,24,33,43,53,38,23,26] | $Y_{10,9,9,8,8,8,6,6,5,4,2}$ [216] | $Y_{10,9,9,8,8,8,6,6,5,4,2,1}$ [216] |
| | [2,3,1,0,2,0,2,0,0,1] | [1,4,10,17,24,33,42,53,38,23,26] | $Y_{10,9,9,8,8,8,7,5,5,3,3}$ [144] | $Y_{10,9,9,8,8,8,7,5,5,3,3,1}$ [144] |
| | [2,4,0,0,0,3,1,0,0,1] | [1,4,11,18,25,32,42,53,38,23,26] | $Y_{10,9,9,8,8,8,8,4,4,4,3}$ [80] | $Y_{10,9,9,8,8,8,8,4,4,4,3,1}$ [80] |
| | [3,0,3,1,1,1,0,1,0,1] | [1,5,9,16,24,33,43,53,38,23,26] | $Y_{10,9,9,9,7,7,7,6,5,4,2}$ [216] | $Y_{10,9,9,9,7,7,7,6,5,4,2,1}$ [216] |
| | [3,0,4,0,0,1,2,0,0,1] | [1,5,9,17,25,33,42,53,38,23,26] | $Y_{10,9,9,9,7,7,7,7,4,3,3}$ [96] | $Y_{10,9,9,9,7,7,7,7,4,3,3,1}$ [96] |
| | [3,1,0,4,1,0,0,0,1,2] | [1,5,10,15,24,34,44,54,38,23,26] | $Y_{10,9,9,9,8,6,6,6,6,5,1}$ [120] | $Y_{10,9,9,9,8,6,6,6,6,5,1,1}$ [120] |
| | [3,1,1,1,3,0,0,1,0,1] | [1,5,10,16,23,33,43,53,38,23,26] | $Y_{10,9,9,9,8,7,6,5,5,5,2}$ [192] | $Y_{10,9,9,9,8,7,6,5,5,5,2,1}$ [192] |
| | [3,1,1,2,0,2,1,0,0,1] | [1,5,10,16,24,32,42,53,38,23,26] | $Y_{10,9,9,9,8,7,6,6,4,4,3}$ [192] | $Y_{10,9,9,9,8,7,6,6,4,4,3,1}$ [192] |
| | [3,2,0,0,3,1,1,0,0,1] | [1,5,11,17,23,32,42,53,38,23,26] | $Y_{10,9,9,9,8,8,5,5,5,4,3}$ [128] | $Y_{10,9,9,9,8,8,5,5,5,4,3,1}$ [128] |
| | [3,4,1,0,1,0,1,0,1,2] | [0,3,10,18,26,35,44,54,38,23,26] | $Y_{9,9,9,8,8,8,8,7,5,3,1}$ [216] | $Y_{9,9,9,8,8,8,8,7,5,3,1,1}$ [216] |
| | [3,5,0,0,0,1,0,2,0,1] | [0,3,11,19,27,35,44,53,38,23,26] | $Y_{9,9,9,8,8,8,8,8,4,2,2}$ [90] | $Y_{9,9,9,8,8,8,8,8,4,2,2,1}$ [90] |
| | [4,0,0,2,2,1,1,0,0,1] | [1,6,11,16,23,32,42,53,38,23,26] | $Y_{10,9,9,9,9,6,6,5,5,4,3}$ [128] | $Y_{10,9,9,9,9,6,6,5,5,4,3,1}$ [128] |
| | [4,0,1,1,0,4,0,0,0,1] | [1,6,11,17,24,31,42,53,38,23,26] | $Y_{10,9,9,9,9,7,6,4,4,4,4}$ [90] | $Y_{10,9,9,9,9,7,6,4,4,4,4,1}$ [90] |
| | [4,1,3,1,0,0,1,0,1,2] | [0,4,9,17,26,35,44,54,38,23,26] | $Y_{9,9,9,9,8,7,7,7,6,3,1}$ [192] | $Y_{9,9,9,9,8,7,7,7,6,3,1,1}$ [192] |
| | [4,2,1,1,1,0,1,1,0,1] | [0,4,10,17,25,34,43,53,38,23,26] | $Y_{9,9,9,9,8,8,7,6,5,3,2}$ [288] | $Y_{9,9,9,9,8,8,7,6,5,3,2,1}$ [288] |
| | [4,3,0,0,1,2,0,1,0,1] | [0,4,11,18,25,33,43,53,38,23,26] | $Y_{9,9,9,9,8,8,8,5,4,4,2}$ [144] | $Y_{9,9,9,9,8,8,8,5,4,4,2,1}$ [144] |
| | [4,3,0,1,0,0,3,0,0,1] | [0,4,11,18,26,34,42,53,38,23,26] | $Y_{9,9,9,9,8,8,8,6,3,3,3}$ [96] | $Y_{9,9,9,9,8,8,8,6,3,3,3,1}$ [96] |
| | [5,0,1,3,0,1,0,0,1,2] | [0,5,10,16,25,34,44,54,38,23,26] | $Y_{9,9,9,9,9,7,6,6,6,4,1}$ [144] | $Y_{9,9,9,9,9,7,6,6,6,4,1,1}$ [144] |
| | [5,0,2,0,3,0,0,0,1,2] | [0,5,10,17,24,34,44,54,38,23,26] | $Y_{9,9,9,9,9,7,7,5,5,5,1}$ [90] | $Y_{9,9,9,9,9,7,7,5,5,5,1,1}$ [90] |
| | [5,0,2,1,0,2,0,1,0,1] | [0,5,10,17,25,33,43,53,38,23,26] | $Y_{9,9,9,9,9,7,7,6,4,4,2}$ [162] | $Y_{9,9,9,9,9,7,7,6,4,4,2,1}$ [162] |
| | [5,0,3,0,0,0,3,0,0,1] | [0,5,10,18,26,34,42,53,38,23,26] | $Y_{9,9,9,9,9,7,7,7,3,3,3}$ [60] | $Y_{9,9,9,9,9,7,7,7,3,3,3,1}$ [60] |
| | [5,1,0,1,2,1,0,1,0,1] | [0,5,11,17,24,33,43,53,38,23,26] | $Y_{9,9,9,9,9,8,6,5,5,4,2}$ [216] | $Y_{9,9,9,9,9,8,6,5,5,4,2,1}$ [216] |
| | [5,1,0,2,0,1,2,0,0,1] | [0,5,11,17,25,33,42,53,38,23,26] | $Y_{9,9,9,9,9,8,6,6,4,3,3}$ [144] | $Y_{9,9,9,9,9,8,6,6,4,3,3,1}$ [144] |
| | [6,0,0,0,3,0,2,0,0,1] | [0,6,12,18,24,33,42,53,38,23,26] | $Y_{9,9,9,9,9,9,5,5,5,3,3}$ [60] | $Y_{9,9,9,9,9,9,5,5,5,3,3,1}$ [60] |
| | [6,0,0,1,0,3,1,0,0,1] | [0,6,12,18,25,32,42,53,38,23,26] | $Y_{9,9,9,9,9,9,6,4,4,4,3}$ [96] | $Y_{9,9,9,9,9,9,6,4,4,4,3,1}$ [96] |
| | [0,2,4,1,1,0,0,0,0,3] | [2,4,8,16,25,35,45,55,39,23,26] | $Y_{10,10,8,8,7,7,7,7,6,5}$ [72] | $Y_{10,10,8,8,7,7,7,7,6,5,1,1,1}$ [72] |
| | [0,8,0,0,0,0,0,0,1,4] | [1,2,11,20,29,38,47,56,39,23,26] | $Y_{10,8,8,8,8,8,8,8,8,1}$ [24] | $Y_{10,8,8,8,8,8,8,8,8,1,1,1,1}$ [24] |
| | [1,4,2,0,2,0,0,0,0,3] | [1,3,9,17,25,35,45,55,39,23,26] | $Y_{10,9,8,8,8,8,7,7,5,5}$ [72] | $Y_{10,9,8,8,8,8,7,7,5,5,1,1,1}$ [72] |
| | [2,1,5,0,0,1,0,0,0,3] | [1,4,8,17,26,35,45,55,39,23,26] | $Y_{10,9,9,8,7,7,7,7,7,4}$ [80] | $Y_{10,9,9,8,7,7,7,7,7,4,1,1,1}$ [80] |
| | [3,0,2,4,0,0,0,0,0,3] | [1,5,9,15,25,35,45,55,39,23,26] | $Y_{10,9,9,9,7,7,6,6,6,6}$ [42] | $Y_{10,9,9,9,7,7,6,6,6,6,1,1,1}$ [42] |
| | [3,3,3,0,0,0,1,0,0,3] | [0,3,9,18,27,36,45,55,39,23,26] | $Y_{9,9,9,8,8,8,7,7,7,3}$ [80] | $Y_{9,9,9,8,8,8,7,7,7,3,1,1,1}$ [80] |
| | [3,4,0,2,0,1,0,0,0,3] | [0,3,10,17,26,35,45,55,39,23,26] | $Y_{9,9,9,8,8,8,8,6,6,4}$ [90] | $Y_{9,9,9,8,8,8,8,6,6,4,1,1,1}$ [90] |
| | [4,1,3,0,2,0,0,0,0,3] | [0,4,9,17,25,35,45,55,39,23,26] | $Y_{9,9,9,9,8,7,7,7,5,5}$ [72] | $Y_{9,9,9,9,8,7,7,7,5,5,1,1,1}$ [72] |
| | [4,2,0,3,1,0,0,0,0,3] | [0,4,10,16,25,35,45,55,39,23,26] | $Y_{9,9,9,9,8,8,6,6,6,5}$ [72] | $Y_{9,9,9,9,8,8,6,6,6,5,1,1,1}$ [72] |
| | [4,3,0,2,0,0,0,0,5,0] | [0,4,11,18,27,36,45,54,36,23,27] | $Y_{9,9,9,9,8,8,8,6,6,1,1,1,1,1}$ [42] | $Y_{9,9,9,9,8,8,8,6,6}$ [42] |
| | [5,0,3,1,0,0,0,0,5,0] | [0,5,10,18,27,36,45,54,36,23,27] | $Y_{9,9,9,9,9,7,7,7,6,1,1,1,1,1}$ [42] | $Y_{9,9,9,9,9,7,7,7,6}$ [42] |
| | [0,3,2,1,2,0,0,0,3,0] | [2,4,9,16,24,34,44,54,37,23,27] | $Y_{10,10,8,8,8,7,7,6,5,5,1,1,1}$ [72] | $Y_{10,10,8,8,8,7,7,6,5,5}$ [72] |
| | [1,1,2,3,1,0,0,0,3,0] | [2,5,9,15,24,34,44,54,37,23,27] | $Y_{10,10,9,8,7,7,6,6,6,5,1,1,1}$ [96] | $Y_{10,10,9,8,7,7,6,6,6,5}$ [96] |
| | [1,4,3,0,0,0,0,1,3,0] | [1,3,9,18,27,36,45,54,37,23,27] | $Y_{10,9,8,8,8,8,7,7,7,2,1,1,1}$ [72] | $Y_{10,9,8,8,8,8,7,7,7,2}$ [72] |
| | [1,5,0,2,0,0,1,0,3,0] | [1,3,10,17,26,35,44,54,37,23,27] | $Y_{10,9,8,8,8,8,8,6,6,3,1,1,1}$ [96] | $Y_{10,9,8,8,8,8,8,6,6,3}$ [96] |

| | | | | |
|---|---|---|---|---|
| | [1,5,1,0,0,2,0,0,3,0] | [1,3,10,18,26,34,44,54,37,23,27] | $Y_{10,9,8,8,8,8,8,7,4,4,1,1,1}$ [80] | $Y_{10,9,8,8,8,8,8,7,4,4}$ [80] |
| | [2,2,2,2,0,1,0,0,3,0] | [1,4,9,16,25,34,44,54,37,23,27] | $Y_{10,9,9,8,8,7,7,6,6,4,1,1,1}$ [120] | $Y_{10,9,9,8,8,7,7,6,6,4}$ [120] |
| | [2,3,0,2,2,0,0,0,3,0] | [1,4,10,16,24,34,44,54,37,23,27] | $Y_{10,9,9,8,8,8,6,6,5,5,1,1,1}$ [72] | $Y_{10,9,9,8,8,8,6,6,5,5}$ [72] |
| | [3,0,3,1,2,0,0,0,3,0] | [1,5,9,16,24,34,44,54,37,23,27] | $Y_{10,9,9,9,7,7,7,6,5,5,1,1,1}$ [72] | $Y_{10,9,9,9,7,7,7,6,5,5}$ [72] |
| | [3,4,1,1,0,0,0,1,3,0] | [0,3,10,18,27,36,45,54,37,23,27] | $Y_{9,9,9,8,8,8,8,7,6,2,1,1,1}$ [120] | $Y_{9,9,9,8,8,8,8,7,6,2}$ [120] |
| | [3,5,0,0,0,1,1,0,3,0] | [0,3,11,19,27,35,44,54,37,23,27] | $Y_{9,9,9,8,8,8,8,8,4,3,1,1,1}$ [80] | $Y_{9,9,9,8,8,8,8,8,4,3}$ [80] |
| | [4,1,4,0,0,0,0,1,3,0] | [0,4,9,18,27,36,45,54,37,23,27] | $Y_{9,9,9,9,8,7,7,7,7,2,1,1,1}$ [72] | $Y_{9,9,9,9,8,7,7,7,7,2}$ [72] |
| | [4,2,1,1,1,1,0,0,3,0] | [0,4,10,17,25,34,44,54,37,23,27] | $Y_{9,9,9,9,8,8,7,6,5,4,1,1,1}$ [160] | $Y_{9,9,9,9,8,8,7,6,5,4}$ [160] |
| | [5,1,0,1,3,0,0,0,3,0] | [0,5,11,17,24,34,44,54,37,23,27] | $Y_{9,9,9,9,9,8,6,5,5,5,1,1,1}$ [72] | $Y_{9,9,9,9,9,8,6,5,5,5}$ [72] |
| | [0,0,3,2,1,2,0,0,1,0] | [3,6,9,15,23,32,43,54,38,23,27] | $Y_{10,10,10,7,7,7,6,6,5,4,4,1}$ [80] | $Y_{10,10,10,7,7,7,6,6,5,4,4}$ [80] |
| | [0,1,0,6,0,0,0,1,1,0] | [3,6,10,14,24,34,44,54,38,23,27] | $Y_{10,10,10,8,6,6,6,6,6,6,2,1}$ [67] | $Y_{10,10,10,8,6,6,6,6,6,6,2}$ [68] |
| | [0,2,4,1,0,1,0,1,1,0] | [2,4,8,16,25,34,44,54,38,23,27] | $Y_{10,10,8,8,7,7,7,7,6,4,2,1}$ [162] | $Y_{10,10,8,8,7,7,7,7,6,4,2}$ [162] |
| | [0,3,1,3,1,0,0,1,1,0] | [2,4,9,15,24,34,44,54,38,23,27] | $Y_{10,10,8,8,8,7,6,6,6,5,2,1}$ [144] | $Y_{10,10,8,8,8,7,6,6,6,5,2}$ [144] |
| | [0,4,0,1,3,0,1,0,1,0] | [2,4,10,16,23,33,43,54,38,23,27] | $Y_{10,10,8,8,8,8,6,5,5,5,3,1}$ [108] | $Y_{10,10,8,8,8,8,6,5,5,5,3}$ [108] |
| | [0,4,0,2,0,3,0,0,1,0] | [2,4,10,16,24,32,43,54,38,23,27] | $Y_{10,10,8,8,8,8,6,6,4,4,4,1}$ [67] | $Y_{10,10,8,8,8,8,6,6,4,4,4}$ [68] |
| | [0,7,1,0,0,0,0,1,2,1] | [1,2,10,19,28,37,46,55,38,23,27] | $Y_{10,8,8,8,8,8,8,8,7,2,1,1}$ [72] | $Y_{10,8,8,8,8,8,8,8,7,2,1}$ [72] |
| | [1,0,4,3,0,0,0,0,2,1] | [2,5,8,15,25,35,45,55,38,23,27] | $Y_{10,10,9,7,7,7,7,6,6,6,1,1}$ [72] | $Y_{10,10,9,7,7,7,7,6,6,6,1}$ [72] |
| | [1,0,5,0,2,0,0,1,1,0] | [2,5,8,16,24,34,44,54,38,23,27] | $Y_{10,10,9,7,7,7,7,7,5,5,2,1}$ [108] | $Y_{10,10,9,7,7,7,7,7,5,5,2}$ [108] |
| | [1,0,5,1,0,0,2,0,1,0] | [2,5,8,16,25,34,43,54,38,23,27] | $Y_{10,10,9,7,7,7,7,7,6,3,3,1}$ [96] | $Y_{10,10,9,7,7,7,7,7,6,3,3}$ [96] |
| | [1,1,2,2,2,0,1,0,1,0] | [2,5,9,15,23,33,43,54,38,23,27] | $Y_{10,10,9,8,7,7,6,6,5,5,3,1}$ [192] | $Y_{10,10,9,8,7,7,6,6,5,5,3}$ [192] |
| | [1,1,3,0,2,2,0,0,1,0] | [2,5,9,16,23,32,43,54,38,23,27] | $Y_{10,10,9,8,7,7,7,5,5,4,4,1}$ [120] | $Y_{10,10,9,8,7,7,7,5,5,4,4}$ [120] |
| | [1,2,0,3,1,2,0,0,1,0] | [2,5,10,15,23,32,43,54,38,23,27] | $Y_{10,10,9,8,8,6,6,6,5,4,4,1}$ [120] | $Y_{10,10,9,8,8,6,6,6,5,4,4}$ [120] |
| | [1,4,1,2,1,0,0,0,2,1] | [1,3,9,16,25,35,45,55,38,23,27] | $Y_{10,9,8,8,8,8,7,6,6,5,1,1}$ [160] | $Y_{10,9,8,8,8,8,7,6,6,5,1}$ [160] |
| | [1,4,2,0,1,1,0,1,1,0] | [1,3,9,17,25,34,44,54,38,23,27] | $Y_{10,9,8,8,8,8,7,7,5,4,2,1}$ [216] | $Y_{10,9,8,8,8,8,7,7,5,4,2}$ [216] |
| | [1,5,0,1,1,0,2,0,1,0] | [1,3,10,17,25,34,43,54,38,23,27] | $Y_{10,9,8,8,8,8,8,6,5,3,3,1}$ [144] | $Y_{10,9,8,8,8,8,8,6,5,3,3}$ [144] |
| | [2,1,4,1,1,0,0,0,2,1] | [1,4,8,16,25,35,45,55,38,23,27] | $Y_{10,9,9,8,7,7,7,7,6,5,1,1}$ [160] | $Y_{10,9,9,8,7,7,7,7,6,5,1}$ [160] |
| | [2,1,5,0,0,0,1,1,1,0] | [1,4,8,17,26,35,44,54,38,23,27] | $Y_{10,9,9,8,7,7,7,7,7,3,2,1}$ [120] | $Y_{10,9,9,8,7,7,7,7,7,3,2}$ [120] |
| | [2,2,1,4,0,0,0,0,2,1] | [1,4,9,15,25,35,45,55,38,23,27] | $Y_{10,9,9,8,8,7,6,6,6,6,1,1}$ [96] | $Y_{10,9,9,8,8,7,6,6,6,6,1}$ [96] |
| | [2,2,2,1,1,1,1,0,1,0] | [1,4,9,16,24,33,43,54,38,23,27] | $Y_{10,9,9,8,8,7,7,6,5,4,3,1}$ [256] | $Y_{10,9,9,8,8,7,7,6,5,4,3}$ [256] |
| | [2,3,1,0,1,3,0,0,1,0] | [1,4,10,17,24,32,43,54,38,23,27] | $Y_{10,9,9,8,8,8,7,5,4,4,4,1}$ [120] | $Y_{10,9,9,8,8,8,7,5,4,4,4}$ [120] |
| | [2,7,0,0,0,0,0,0,3,2] | [0,2,11,20,29,38,47,56,38,23,27] | $Y_{9,9,8,8,8,8,8,8,8,1,1,1}$ [32] | $Y_{9,9,8,8,8,8,8,8,8,1,1}$ [32] |
| | [3,0,2,3,1,0,0,1,1,0] | [1,5,9,15,24,34,44,54,38,23,27] | $Y_{10,9,9,9,7,7,6,6,6,5,2,1}$ [144] | $Y_{10,9,9,9,7,7,6,6,6,5,2}$ [144] |
| | [3,1,0,4,0,1,1,0,1,0] | [1,5,10,15,24,33,43,54,38,23,27] | $Y_{10,9,9,9,8,6,6,6,6,4,3,1}$ [144] | $Y_{10,9,9,9,8,6,6,6,6,4,3}$ [144] |
| | [3,1,1,1,2,2,0,0,1,0] | [1,5,10,16,23,32,43,54,38,23,27] | $Y_{10,9,9,9,8,7,6,5,5,4,4,1}$ [160] | $Y_{10,9,9,9,8,7,6,5,5,4,4}$ [160] |
| | [3,3,2,1,0,1,0,0,2,1] | [0,3,9,17,26,35,45,55,38,23,27] | $Y_{9,9,9,8,8,8,7,7,6,4,1,1}$ [192] | $Y_{9,9,9,8,8,8,7,7,6,4,1}$ [192] |
| | [3,3,3,0,0,0,0,2,1,0] | [0,3,9,18,27,36,45,54,38,23,27] | $Y_{9,9,9,8,8,8,7,7,7,2,2,1}$ [72] | $Y_{9,9,9,8,8,8,7,7,7,2,2}$ [72] |
| | [3,4,0,1,2,0,0,0,2,1] | [0,3,10,17,25,35,45,55,38,23,27] | $Y_{9,9,9,8,8,8,8,6,5,5,1,1}$ [120] | $Y_{9,9,9,8,8,8,8,6,5,5,1}$ [120] |
| | [3,4,0,2,0,0,1,1,1,0] | [0,3,10,17,26,35,44,54,38,23,27] | $Y_{9,9,9,8,8,8,8,6,6,3,2,1}$ [144] | $Y_{9,9,9,8,8,8,8,6,6,3,2}$ [144] |
| | [3,4,1,0,0,2,0,1,1,0] | [0,3,10,18,26,34,44,54,38,23,27] | $Y_{9,9,9,8,8,8,8,7,4,4,2,1}$ [144] | $Y_{9,9,9,8,8,8,8,7,4,4,2}$ [144] |
| | [3,5,0,0,0,0,3,0,1,0] | [0,3,11,19,27,35,43,54,38,23,27] | $Y_{9,9,9,8,8,8,8,8,3,3,3,1}$ [48] | $Y_{9,9,9,8,8,8,8,8,3,3,3}$ [48] |
| | [4,1,2,2,1,0,0,0,2,1] | [0,4,9,16,25,35,45,55,38,23,27] | $Y_{9,9,9,9,8,7,7,6,6,5,1,1}$ [160] | $Y_{9,9,9,9,8,7,7,6,6,5,1}$ [160] |
| | [4,1,3,0,1,1,0,1,1,0] | [0,4,9,17,25,34,44,54,38,23,27] | $Y_{9,9,9,9,8,7,7,7,5,4,2,1}$ [216] | $Y_{9,9,9,9,8,7,7,7,5,4,2}$ [216] |
| | [4,2,0,3,0,1,0,1,1,0] | [0,4,10,16,25,34,44,54,38,23,27] | $Y_{9,9,9,9,8,8,6,6,6,4,2,1}$ [162] | $Y_{9,9,9,9,8,8,6,6,6,4,2}$ [162] |
| | [4,2,1,0,3,0,0,1,1,0] | [0,4,10,17,24,34,44,54,38,23,27] | $Y_{9,9,9,9,8,8,7,5,5,5,2,1}$ [144] | $Y_{9,9,9,9,8,8,7,5,5,5,2}$ [144] |
| | [4,2,1,1,0,2,1,0,1,0] | [0,4,10,17,25,33,43,54,38,23,27] | $Y_{9,9,9,9,8,8,7,6,4,4,3,1}$ [192] | $Y_{9,9,9,9,8,8,7,6,4,4,3}$ [192] |
| | [5,0,1,2,2,0,0,1,1,0] | [0,5,10,16,24,34,44,54,38,23,27] | $Y_{9,9,9,9,9,7,6,6,5,5,2,1}$ [144] | $Y_{9,9,9,9,9,7,6,6,5,5,2}$ [144] |
| | [5,0,1,3,0,0,2,0,1,0] | [0,5,10,16,25,34,43,54,38,23,27] | $Y_{9,9,9,9,9,7,6,6,6,3,3,1}$ [96] | $Y_{9,9,9,9,9,7,6,6,6,3,3}$ [96] |
| | [5,0,2,0,2,1,1,0,1,0] | [0,5,10,17,24,33,43,54,38,23,27] | $Y_{9,9,9,9,9,7,7,5,5,4,3,1}$ [144] | $Y_{9,9,9,9,9,7,7,5,5,4,3}$ [144] |
| | [5,1,1,0,0,4,0,0,1,0] | [0,5,11,18,25,32,43,54,38,23,27] | $Y_{9,9,9,9,9,8,7,4,4,4,4,1}$ [80] | $Y_{9,9,9,9,9,8,7,4,4,4,4}$ [80] |
| | [6,0,0,0,2,3,0,0,1,0] | [0,6,12,18,24,32,43,54,38,23,27] | $Y_{9,9,9,9,9,9,5,5,4,4,4,1}$ [50] | $Y_{9,9,9,9,9,9,5,5,4,4,4}$ [50] |
| | [0,0,2,5,0,0,1,0,0,1] | [3,6,9,14,24,34,44,55,39,23,27] | $Y_{10,10,10,7,7,6,6,6,6,6,3}$ [64] | $Y_{10,10,10,7,7,6,6,6,6,6,3,1}$ [64] |
| | [0,1,0,5,1,1,0,0,0,1] | [3,6,10,14,23,33,44,55,39,23,27] | $Y_{10,10,10,8,6,6,6,6,6,5,4}$ [90] | $Y_{10,10,10,8,6,6,6,6,6,5,4,1}$ [90] |
| | [0,2,3,3,0,0,0,1,0,1] | [2,4,8,15,25,35,45,55,39,23,27] | $Y_{10,10,8,8,7,7,7,6,6,6,2}$ [90] | $Y_{10,10,8,8,7,7,7,6,6,6,2,1}$ [90] |
| | [0,2,4,0,2,0,1,0,0,1] | [2,4,8,16,24,34,44,55,39,23,27] | $Y_{10,10,8,8,7,7,7,7,5,5,3}$ [108] | $Y_{10,10,8,8,7,7,7,7,5,5,3,1}$ [108] |
| | [0,3,1,3,0,2,0,0,0,1] | [2,4,9,15,24,33,44,55,39,23,27] | $Y_{10,10,8,8,8,7,6,6,6,4,4}$ [90] | $Y_{10,10,8,8,8,7,6,6,6,4,4,1}$ [90] |
| | [0,3,2,0,3,1,0,0,0,1] | [2,4,9,16,23,33,44,55,39,23,27] | $Y_{10,10,8,8,8,7,7,5,5,5,4}$ [90] | $Y_{10,10,8,8,8,7,7,5,5,5,4,1}$ [90] |
| | [0,6,2,0,0,1,0,0,1,2] | [1,2,9,18,27,36,46,56,39,23,27] | $Y_{10,8,8,8,8,8,8,7,7,4,1}$ [96] | $Y_{10,8,8,8,8,8,8,7,7,4,1,1}$ [96] |
| | [0,7,0,0,2,0,0,0,1,2] | [1,2,10,18,26,36,46,56,39,23,27] | $Y_{10,8,8,8,8,8,8,8,5,5,1}$ [60] | $Y_{10,8,8,8,8,8,8,8,5,5,1,1}$ [60] |
| | [0,7,0,1,0,0,1,1,0,1] | [1,2,10,18,27,36,45,55,39,23,27] | $Y_{10,8,8,8,8,8,8,8,6,3,2}$ [108] | $Y_{10,8,8,8,8,8,8,8,6,3,2,1}$ [108] |
| | [1,0,4,2,1,0,1,0,0,1] | [2,5,8,15,24,34,44,55,39,23,27] | $Y_{10,10,9,7,7,7,7,6,6,5,3}$ [144] | $Y_{10,10,9,7,7,7,7,6,6,5,3,1}$ [144] |
| | [1,0,5,0,1,2,0,0,0,1] | [2,5,8,16,24,33,44,55,39,23,27] | $Y_{10,10,9,7,7,7,7,7,5,4,4}$ [90] | $Y_{10,10,9,7,7,7,7,7,5,4,4,1}$ [90] |
| | [1,3,3,2,0,0,0,0,1,2] | [1,3,8,16,26,36,46,56,39,23,27] | $Y_{10,9,8,8,8,7,7,7,6,6,1}$ [96] | $Y_{10,9,8,8,8,7,7,7,6,6,1,1}$ [96] |
| | [1,3,4,0,0,1,0,1,0,1] | [1,3,8,17,26,35,45,55,39,23,27] | $Y_{10,9,8,8,8,7,7,7,7,4,2}$ [144] | $Y_{10,9,8,8,8,7,7,7,7,4,2,1}$ [144] |
| | [1,4,1,2,0,1,1,0,0,1] | [1,3,9,16,25,34,44,55,39,23,27] | $Y_{10,9,8,8,8,8,7,6,6,4,3}$ [192] | $Y_{10,9,8,8,8,8,7,6,6,4,3,1}$ [192] |
| | [1,5,0,0,3,0,1,0,0,1] | [1,3,10,17,24,34,44,55,39,23,27] | $Y_{10,9,8,8,8,8,8,5,5,5,3}$ [96] | $Y_{10,9,8,8,8,8,8,5,5,5,3,1}$ [96] |
| | [1,5,0,1,0,3,0,0,0,1] | [1,3,10,17,25,33,44,55,39,23,27] | $Y_{10,9,8,8,8,8,8,6,4,4,4}$ [90] | $Y_{10,9,8,8,8,8,8,6,4,4,4,1}$ [90] |
| | [2,0,0,6,0,0,1,0,0,1] | [2,6,10,14,24,34,44,55,39,23,27] | $Y_{10,10,9,9,6,6,6,6,6,6,3}$ [64] | $Y_{10,10,9,9,6,6,6,6,6,6,3,1}$ [64] |
| | [2,1,4,1,0,1,1,0,0,1] | [1,4,8,16,25,34,44,55,39,23,27] | $Y_{10,9,9,8,7,7,7,7,6,4,3}$ [192] | $Y_{10,9,9,8,7,7,7,7,6,4,3,1}$ [192] |
| | [2,2,1,3,1,0,1,0,0,1] | [1,4,9,15,24,34,44,55,39,23,27] | $Y_{10,9,9,8,8,7,6,6,6,5,3}$ [192] | $Y_{10,9,9,8,8,7,6,6,6,5,3,1}$ [192] |
| | [2,3,0,1,3,1,0,0,0,1] | [1,4,10,16,23,33,44,55,39,23,27] | $Y_{10,9,9,8,8,8,6,5,5,5,4}$ [120] | $Y_{10,9,9,8,8,8,6,5,5,5,4,1}$ [120] |
| | [2,6,0,1,0,1,0,0,1,2] | [0,2,10,18,27,36,46,56,39,23,27] | $Y_{9,9,8,8,8,8,8,8,6,4,1}$ [144] | $Y_{9,9,8,8,8,8,8,8,6,4,1,1}$ [144] |

| | | | | |
|---|---|---|---|---|
| | [2,6,1,0,0,0,0,2,0,1] | [0,2,10,19,28,37,46,55,39,23,27] | $Y_{9,9,8,8,8,8,8,8,7,2,2}$ [72] | $Y_{9,9,8,8,8,8,8,8,7,2,2,1}$ [72] |
| | [3,0,2,3,0,2,0,0,0,1] | [1,5,9,15,24,33,44,55,39,23,27] | $Y_{10,9,9,9,7,7,6,6,6,4,4}$ [90] | $Y_{10,9,9,9,7,7,6,6,6,4,4,1}$ [90] |
| | [3,0,3,0,3,1,0,0,0,1] | [1,5,9,16,23,33,44,55,39,23,27] | $Y_{10,9,9,9,7,7,7,5,5,5,4}$ [90] | $Y_{10,9,9,9,7,7,7,5,5,5,4,1}$ [90] |
| | [3,1,0,3,2,1,0,0,0,1] | [1,5,10,15,23,33,44,55,39,23,27] | $Y_{10,9,9,9,8,6,6,6,5,5,4}$ [120] | $Y_{10,9,9,9,8,6,6,6,5,5,4,1}$ [120] |
| | [3,3,1,3,0,0,0,0,1,2] | [0,3,9,16,26,36,46,56,39,23,27] | $Y_{9,9,9,8,8,8,7,6,6,6,1}$ [96] | $Y_{9,9,9,8,8,8,7,6,6,6,1,1}$ [96] |
| | [3,3,2,0,2,0,0,1,0,1] | [0,3,9,17,25,35,45,55,39,23,27] | $Y_{9,9,9,8,8,8,7,7,5,5,2}$ [144] | $Y_{9,9,9,8,8,8,7,7,5,5,2,1}$ [144] |
| | [3,3,2,1,0,0,2,0,0,1] | [0,3,9,17,26,35,44,55,39,23,27] | $Y_{9,9,9,8,8,8,7,7,6,3,3}$ [128] | $Y_{9,9,9,8,8,8,7,7,6,3,3,1}$ [128] |
| | [3,4,0,1,1,1,1,0,0,1] | [0,3,10,17,25,34,44,55,39,23,27] | $Y_{9,9,9,8,8,8,8,6,5,4,3}$ [192] | $Y_{9,9,9,8,8,8,8,6,5,4,3,1}$ [192] |
| | [4,0,5,0,1,0,0,0,1,2] | [0,4,8,17,26,36,46,56,39,23,27] | $Y_{9,9,9,9,7,7,7,7,7,5,1}$ [90] | $Y_{9,9,9,9,7,7,7,7,7,5,1,1}$ [90] |
| | [4,1,2,2,0,1,1,0,0,1] | [0,4,9,16,25,34,44,55,39,23,27] | $Y_{9,9,9,9,8,7,7,6,6,4,3}$ [192] | $Y_{9,9,9,9,8,7,7,6,6,4,3,1}$ [192] |
| | [4,2,0,2,2,0,1,0,0,1] | [0,4,10,16,24,34,44,55,39,23,27] | $Y_{9,9,9,9,8,8,6,6,5,5,3}$ [144] | $Y_{9,9,9,9,8,8,6,6,5,5,3,1}$ [144] |
| | [4,2,1,0,2,2,0,0,0,1] | [0,4,10,17,24,33,44,55,39,23,27] | $Y_{9,9,9,9,8,8,7,5,5,4,4}$ [120] | $Y_{9,9,9,9,8,8,7,5,5,4,4,1}$ [120] |
| | [5,0,1,2,1,2,0,0,0,1] | [0,5,10,16,24,33,44,55,39,23,27] | $Y_{9,9,9,9,9,7,6,6,5,4,4}$ [120] | $Y_{9,9,9,9,9,7,6,6,5,4,4,1}$ [120] |
| | [0,6,1,2,0,0,0,0,0,3] | [1,2,9,17,27,37,47,57,40,23,27] | $Y_{10,8,8,8,8,8,8,7,6,6}$ [42] | $Y_{10,8,8,8,8,8,8,7,6,6,1,1,1}$ [42] |
| | [2,5,2,0,1,0,0,0,0,3] | [0,2,9,18,27,37,47,57,40,23,27] | $Y_{9,9,8,8,8,8,8,7,7,5}$ [72] | $Y_{9,9,8,8,8,8,8,7,7,5,1,1,1}$ [72] |
| | [3,2,4,1,0,0,0,0,0,3] | [0,3,8,17,27,37,47,57,40,23,27] | $Y_{9,9,9,8,8,7,7,7,7,6}$ [56] | $Y_{9,9,9,8,8,7,7,7,7,6,1,1,1}$ [56] |
| | [0,7,0,1,0,1,0,0,3,0] | [1,2,10,18,27,36,46,56,38,23,28] | $Y_{10,8,8,8,8,8,8,8,6,4,1,1,1}$ [67] | $Y_{10,8,8,8,8,8,8,8,6,4}$ [68] |
| | [1,3,4,0,1,0,0,0,3,0] | [1,3,8,17,26,36,46,56,38,23,28] | $Y_{10,9,8,8,8,7,7,7,7,5,1,1,1}$ [72] | $Y_{10,9,8,8,8,7,7,7,7,5}$ [72] |
| | [2,6,1,0,0,0,1,0,3,0] | [0,2,10,19,28,37,46,56,38,23,28] | $Y_{9,9,8,8,8,8,8,8,7,3,1,1,1}$ [80] | $Y_{9,9,8,8,8,8,8,8,7,3}$ [80] |
| | [0,0,2,4,2,0,0,0,1,0] | [3,6,9,14,23,34,45,56,39,23,28] | $Y_{10,10,10,7,7,6,6,6,6,5,5,1}$ [48] | $Y_{10,10,10,7,7,6,6,6,6,5,5}$ [48] |
| | [0,1,7,0,0,0,0,0,2,1] | [2,4,7,17,27,37,47,57,39,23,28] | $Y_{10,10,8,7,7,7,7,7,7,7,1,1}$ [42] | $Y_{10,10,8,7,7,7,7,7,7,7,1}$ [42] |
| | [0,2,3,2,1,1,0,0,1,0] | [2,4,8,15,24,34,45,56,39,23,28] | $Y_{10,10,8,8,7,7,7,6,6,5,4,1}$ [120] | $Y_{10,10,8,8,7,7,7,6,6,5,4}$ [120] |
| | [0,3,1,2,3,0,0,0,1,0] | [2,4,9,15,23,34,45,56,39,23,28] | $Y_{10,10,8,8,8,7,6,6,5,5,5,1}$ [72] | $Y_{10,10,8,8,8,7,6,6,5,5,5}$ [72] |
| | [0,6,1,1,1,0,0,1,1,0] | [1,2,9,17,26,36,46,56,39,23,28] | $Y_{10,8,8,8,8,8,8,7,6,5,2,1}$ [144] | $Y_{10,8,8,8,8,8,8,7,6,5,2}$ [144] |
| | [0,6,2,0,0,0,2,0,1,0] | [1,2,9,18,27,36,45,56,39,23,28] | $Y_{10,8,8,8,8,8,8,7,7,3,3,1}$ [60] | $Y_{10,8,8,8,8,8,8,7,7,3,3}$ [60] |
| | [0,7,0,0,1,1,1,0,1,0] | [1,2,10,18,26,35,45,56,39,23,28] | $Y_{10,8,8,8,8,8,8,8,5,4,3,1}$ [96] | $Y_{10,8,8,8,8,8,8,8,5,4,3}$ [96] |
| | [1,1,1,5,0,1,0,0,1,0] | [2,5,9,14,24,34,45,56,39,23,28] | $Y_{10,10,9,8,7,6,6,6,6,6,4,1}$ [120] | $Y_{10,10,9,8,7,6,6,6,6,6,4}$ [120] |
| | [1,3,3,1,1,0,1,0,1,0] | [1,3,8,16,25,35,45,56,39,23,28] | $Y_{10,9,8,8,8,7,7,7,6,5,3,1}$ [192] | $Y_{10,9,8,8,8,7,7,7,6,5,3}$ [192] |
| | [1,4,1,1,2,1,0,0,1,0] | [1,3,9,16,24,34,45,56,39,23,28] | $Y_{10,9,8,8,8,8,7,6,5,5,4,1}$ [160] | $Y_{10,9,8,8,8,8,7,6,5,5,4}$ [160] |
| | [2,0,0,5,2,0,0,0,1,0] | [2,6,10,14,23,34,45,56,39,23,28] | $Y_{10,10,9,9,6,6,6,6,6,5,5,1}$ [48] | $Y_{10,10,9,9,6,6,6,6,6,5,5}$ [48] |
| | [2,1,3,3,0,0,1,0,1,0] | [1,4,8,15,25,35,45,56,39,23,28] | $Y_{10,9,9,8,7,7,7,6,6,6,3,1}$ [128] | $Y_{10,9,9,8,7,7,7,6,6,6,3}$ [128] |
| | [2,1,4,0,2,1,0,0,1,0] | [1,4,8,16,24,34,45,56,39,23,28] | $Y_{10,9,9,8,7,7,7,7,5,5,4,1}$ [120] | $Y_{10,9,9,8,7,7,7,7,5,5,4}$ [120] |
| | [2,2,2,0,4,0,0,0,1,0] | [1,4,9,16,23,34,45,56,39,23,28] | $Y_{10,9,9,8,8,7,7,5,5,5,5,1}$ [72] | $Y_{10,9,9,8,8,7,7,5,5,5,5}$ [72] |
| | [2,5,1,2,0,0,0,0,2,1] | [0,2,9,17,27,37,47,57,39,23,28] | $Y_{9,9,8,8,8,8,8,7,6,6,1,1}$ [96] | $Y_{9,9,8,8,8,8,8,7,6,6,1}$ [96] |
| | [2,5,2,0,0,1,0,1,1,0] | [0,2,9,18,27,36,46,56,39,23,28] | $Y_{9,9,8,8,8,8,8,7,7,4,2,1}$ [144] | $Y_{9,9,8,8,8,8,8,7,7,4,2}$ [144] |
| | [2,6,0,0,2,0,0,1,1,0] | [0,2,10,18,26,36,46,56,39,23,28] | $Y_{9,9,8,8,8,8,8,8,5,5,2,1}$ [96] | $Y_{9,9,8,8,8,8,8,8,5,5,2}$ [96] |
| | [2,6,0,1,0,0,2,0,1,0] | [0,2,10,18,27,36,45,56,39,23,28] | $Y_{9,9,8,8,8,8,8,8,6,3,3,1}$ [96] | $Y_{9,9,8,8,8,8,8,8,6,3,3}$ [96] |
| | [3,0,2,2,3,0,0,0,1,0] | [1,5,9,15,23,34,45,56,39,23,28] | $Y_{10,9,9,9,7,7,6,6,5,5,5,1}$ [72] | $Y_{10,9,9,9,7,7,6,6,5,5,5}$ [72] |
| | [3,2,4,0,1,0,0,1,1,0] | [0,3,8,17,26,36,46,56,39,23,28] | $Y_{9,9,9,8,8,7,7,7,7,5,2,1}$ [144] | $Y_{9,9,9,8,8,7,7,7,7,5,2}$ [144] |
| | [3,3,1,2,1,0,1,0,1,0] | [0,3,9,16,25,35,45,56,39,23,28] | $Y_{9,9,9,8,8,8,7,6,6,5,3,1}$ [192] | $Y_{9,9,9,8,8,8,7,6,6,5,3}$ [192] |
| | [3,3,2,0,1,2,0,0,1,0] | [0,3,9,17,25,34,45,56,39,23,28] | $Y_{9,9,9,8,8,8,7,7,5,4,4,1}$ [120] | $Y_{9,9,9,8,8,8,7,7,5,4,4}$ [120] |
| | [4,0,4,2,0,0,0,1,1,0] | [0,4,8,16,26,36,46,56,39,23,28] | $Y_{9,9,9,9,7,7,7,7,6,6,2,1}$ [90] | $Y_{9,9,9,9,7,7,7,7,6,6,2}$ [90] |
| | [4,0,5,0,0,1,1,0,1,0] | [0,4,8,17,26,35,45,56,39,23,28] | $Y_{9,9,9,9,7,7,7,7,7,4,3,1}$ [96] | $Y_{9,9,9,9,7,7,7,7,7,4,3}$ [96] |
| | [4,1,2,1,2,1,0,0,1,0] | [0,4,9,16,24,34,45,56,39,23,28] | $Y_{9,9,9,9,8,7,7,6,5,5,4,1}$ [160] | $Y_{9,9,9,9,8,7,7,6,5,5,4}$ [160] |
| | [5,0,0,5,0,0,1,0,1,0] | [0,5,10,15,25,35,45,56,39,23,28] | $Y_{9,9,9,9,9,6,6,6,6,6,3,1}$ [64] | $Y_{9,9,9,9,9,6,6,6,6,6,3}$ [64] |
| | [5,1,0,0,5,0,0,0,1,0] | [0,5,11,17,23,34,45,56,39,23,28] | $Y_{9,9,9,9,9,8,5,5,5,5,5,1}$ [48] | $Y_{9,9,9,9,9,8,5,5,5,5,5}$ [48] |
| | [0,1,6,1,0,0,1,0,0,1] | [2,4,7,16,26,36,46,57,40,23,28] | $Y_{10,10,8,7,7,7,7,7,7,6,3}$ [96] | $Y_{10,10,8,7,7,7,7,7,7,6,3,1}$ [96] |
| | [0,5,3,1,0,0,0,1,0,1] | [1,2,8,17,27,37,47,57,40,23,28] | $Y_{10,8,8,8,8,8,7,7,7,6,2}$ [90] | $Y_{10,8,8,8,8,8,7,7,7,6,2,1}$ [90] |
| | [0,6,1,1,0,2,0,0,0,1] | [1,2,9,17,26,35,46,57,40,23,28] | $Y_{10,8,8,8,8,8,8,7,6,4,4}$ [90] | $Y_{10,8,8,8,8,8,8,7,6,4,4,1}$ [90] |
| | [1,4,0,4,0,1,0,0,0,1] | [1,3,9,15,25,35,46,57,40,23,28] | $Y_{10,9,8,8,8,8,6,6,6,6,4}$ [90] | $Y_{10,9,8,8,8,8,6,6,6,6,4,1}$ [90] |
| | [2,0,7,0,0,0,0,1,0,1] | [1,4,7,17,27,37,47,57,40,23,28] | $Y_{10,9,9,7,7,7,7,7,7,7,2}$ [54] | $Y_{10,9,9,7,7,7,7,7,7,7,2,1}$ [54] |
| | [2,1,3,2,2,0,0,0,0,1] | [1,4,8,15,24,35,46,57,40,23,28] | $Y_{10,9,9,8,7,7,7,6,6,5,5}$ [96] | $Y_{10,9,9,8,7,7,7,6,6,5,5,1}$ [96] |
| | [2,4,4,0,0,0,0,0,1,2] | [0,2,8,18,28,38,48,58,40,23,28] | $Y_{9,9,8,8,8,8,7,7,7,7,1}$ [56] | $Y_{9,9,8,8,8,8,7,7,7,7,1,1}$ [56] |
| | [2,5,1,1,1,0,1,0,0,1] | [0,2,9,17,26,36,46,57,40,23,28] | $Y_{9,9,8,8,8,8,8,7,6,5,3}$ [192] | $Y_{9,9,8,8,8,8,8,7,6,5,3,1}$ [192] |
| | [2,6,0,0,1,2,0,0,0,1] | [0,2,10,18,26,35,46,57,40,23,28] | $Y_{9,9,8,8,8,8,8,8,5,4,4}$ [80] | $Y_{9,9,8,8,8,8,8,8,5,4,4,1}$ [80] |
| | [3,2,3,2,0,0,1,0,0,1] | [0,3,8,16,26,36,46,57,40,23,28] | $Y_{9,9,9,8,8,7,7,7,6,6,3}$ [128] | $Y_{9,9,9,8,8,7,7,7,6,6,3,1}$ [128] |
| | [3,2,4,0,0,2,0,0,0,1] | [0,3,8,17,26,35,46,57,40,23,28] | $Y_{9,9,9,8,8,7,7,7,7,4,4}$ [80] | $Y_{9,9,9,8,8,7,7,7,7,4,4,1}$ [80] |
| | [3,4,0,0,4,0,0,0,0,1] | [0,3,10,17,24,35,46,57,40,23,28] | $Y_{9,9,9,8,8,8,8,5,5,5,5}$ [48] | $Y_{9,9,9,8,8,8,8,5,5,5,5,1}$ [48] |
| | [4,0,4,1,1,1,0,0,0,1] | [0,4,8,16,25,35,46,57,40,23,28] | $Y_{9,9,9,9,7,7,7,7,6,5,4}$ [120] | $Y_{9,9,9,9,7,7,7,7,6,5,4,1}$ [120] |
| | [4,1,1,4,0,1,0,0,0,1] | [0,4,9,15,25,35,46,57,40,23,28] | $Y_{9,9,9,9,8,7,6,6,6,6,4}$ [120] | $Y_{9,9,9,9,8,7,6,6,6,6,4,1}$ [120] |
| | [5,0,0,4,2,0,0,0,0,1] | [0,5,10,15,24,35,46,57,40,23,28] | $Y_{9,9,9,9,9,6,6,6,6,5,5}$ [48] | $Y_{9,9,9,9,9,6,6,6,6,5,5,1}$ [48] |
| | [0,5,4,0,0,0,0,0,3,0] | [1,2,8,18,28,38,48,58,39,23,29] | $Y_{10,8,8,8,8,8,7,7,7,7,1,1,1}$ [24] | $Y_{10,8,8,8,8,8,7,7,7,7}$ [24] |
| | [0,1,6,0,2,0,0,0,1,0] | [2,4,7,16,25,36,47,58,40,23,29] | $Y_{10,10,8,7,7,7,7,7,7,5,5,1}$ [54] | $Y_{10,10,8,7,7,7,7,7,7,5,5}$ [54] |
| | [0,3,0,6,0,0,0,0,1,0] | [2,4,9,14,25,36,47,58,40,23,29] | $Y_{10,10,8,8,8,6,6,6,6,6,6,1}$ [31] | $Y_{10,10,8,8,8,6,6,6,6,6,6}$ [32] |
| | [0,5,3,0,1,1,0,0,1,0] | [1,2,8,17,26,36,47,58,40,23,29] | $Y_{10,8,8,8,8,8,7,7,7,5,4,1}$ [90] | $Y_{10,8,8,8,8,8,7,7,7,5,4}$ [90] |
| | [0,6,0,3,0,1,0,0,1,0] | [1,2,9,16,26,36,47,58,40,23,29] | $Y_{10,8,8,8,8,8,8,6,6,6,4,1}$ [67] | $Y_{10,8,8,8,8,8,8,6,6,6,4}$ [68] |
| | [0,6,1,0,3,0,0,0,1,0] | [1,2,9,17,25,36,47,58,40,23,29] | $Y_{10,8,8,8,8,8,8,7,5,5,5,1}$ [54] | $Y_{10,8,8,8,8,8,8,7,5,5,5}$ [54] |
| | [1,2,6,0,0,0,1,0,1,0] | [1,3,7,17,27,37,47,58,40,23,29] | $Y_{10,9,8,8,7,7,7,7,7,7,3,1}$ [80] | $Y_{10,9,8,8,7,7,7,7,7,7,3}$ [80] |
| | [1,3,2,3,1,0,0,0,1,0] | [1,3,8,15,25,36,47,58,40,23,29] | $Y_{10,9,8,8,8,7,7,6,6,6,5,1}$ [96] | $Y_{10,9,8,8,8,7,7,6,6,6,5}$ [96] |
| | [1,8,0,1,0,0,0,0,2,1] | [0,1,10,19,29,39,49,59,40,23,29] | $Y_{9,8,8,8,8,8,8,8,8,6,1,1}$ [72] | $Y_{9,8,8,8,8,8,8,8,8,6,1}$ [72] |
| | [2,0,6,1,0,1,0,0,1,0] | [1,4,7,16,26,36,47,58,40,23,29] | $Y_{10,9,9,7,7,7,7,7,7,6,4,1}$ [90] | $Y_{10,9,9,7,7,7,7,7,7,6,4}$ [90] |

| | | | | |
|---|---|---|---|---|
| | [2,4,3,1,0,0,1,0,1,0] | [0,2,8,17,27,37,47,58,40,23,29] | $Y_{9,9,8,8,8,8,7,7,7,6,3,1}$ [128] | $Y_{9,9,8,8,8,8,7,7,7,6,3}$ [128] |
| | [3,0,1,6,0,0,0,0,1,0] | [1,5,9,14,25,36,47,58,40,23,29] | $Y_{10,9,9,9,7,6,6,6,6,6,6,1}$ [42] | $Y_{10,9,9,9,7,6,6,6,6,6,6}$ [42] |
| | [3,2,3,1,2,0,0,0,1,0] | [0,3,8,16,25,36,47,58,40,23,29] | $Y_{9,9,9,8,8,7,7,7,6,5,5,1}$ [96] | $Y_{9,9,9,8,8,7,7,7,6,5,5}$ [96] |
| | [0,5,2,2,1,0,0,0,0,1] | [1,2,8,16,26,37,48,59,41,23,29] | $Y_{10,8,8,8,8,8,7,7,6,6,5}$ [72] | $Y_{10,8,8,8,8,8,7,7,6,6,5,1}$ [72] |
| | [1,2,5,1,1,0,0,0,0,1] | [1,3,7,16,26,37,48,59,41,23,29] | $Y_{10,9,8,8,7,7,7,7,7,6,5}$ [96] | $Y_{10,9,8,8,7,7,7,7,7,6,5,1}$ [96] |
| | [1,7,2,0,0,0,0,1,0,1] | [0,1,9,19,29,39,49,59,41,23,29] | $Y_{9,8,8,8,8,8,8,8,7,7,2}$ [72] | $Y_{9,8,8,8,8,8,8,8,7,7,2,1}$ [72] |
| | [1,8,0,0,1,0,1,0,0,1] | [0,1,10,19,28,38,48,59,41,23,29] | $Y_{9,8,8,8,8,8,8,8,8,5,3}$ [96] | $Y_{9,8,8,8,8,8,8,8,8,5,3,1}$ [96] |
| | [2,4,3,0,2,0,0,0,0,1] | [0,2,8,17,26,37,48,59,41,23,29] | $Y_{9,9,8,8,8,8,7,7,7,5,5}$ [72] | $Y_{9,9,8,8,8,8,7,7,7,5,5,1}$ [72] |
| | [2,5,0,3,1,0,0,0,0,1] | [0,2,9,16,26,37,48,59,41,23,29] | $Y_{9,9,8,8,8,8,8,6,6,6,5}$ [72] | $Y_{9,9,8,8,8,8,8,6,6,6,5,1}$ [72] |
| | [3,3,0,5,0,0,0,0,0,1] | [0,3,9,15,26,37,48,59,41,23,29] | $Y_{9,9,9,8,8,8,6,6,6,6,6}$ [42] | $Y_{9,9,9,8,8,8,6,6,6,6,6,1}$ [42] |
| | [4,0,3,4,0,0,0,0,0,1] | [0,4,8,15,26,37,48,59,41,23,29] | $Y_{9,9,9,9,7,7,7,6,6,6,6}$ [42] | $Y_{9,9,9,9,7,7,7,6,6,6,6,1}$ [42] |
| | [1,7,1,1,0,1,0,0,1,0] | [0,1,9,18,28,38,49,60,41,23,30] | $Y_{9,8,8,8,8,8,8,8,7,6,4,1}$ [120] | $Y_{9,8,8,8,8,8,8,8,7,6,4}$ [120] |
| | [2,4,2,3,0,0,0,0,1,0] | [0,2,8,16,27,38,49,60,41,23,30] | $Y_{9,9,8,8,8,8,7,7,6,6,6,1}$ [56] | $Y_{9,9,8,8,8,8,7,7,6,6,6}$ [56] |
| | [3,1,6,0,1,0,0,0,1,0] | [0,3,7,17,27,38,49,60,41,23,30] | $Y_{9,9,9,8,7,7,7,7,7,7,5,1}$ [72] | $Y_{9,9,9,8,7,7,7,7,7,7,5}$ [72] |
| | [0,4,5,1,0,0,0,0,0,1] | [1,2,7,17,28,39,50,61,42,23,30] | $Y_{10,8,8,8,8,7,7,7,7,7,6}$ [42] | $Y_{10,8,8,8,8,7,7,7,7,7,6,1}$ [42] |
| | [1,6,3,1,0,0,0,0,1,0] | [0,1,8,18,29,40,51,62,42,23,31] | $Y_{9,8,8,8,8,8,8,7,7,7,6,1}$ [56] | $Y_{9,8,8,8,8,8,8,7,7,7,6}$ [56] |
| | [2,3,6,0,0,0,0,0,1,0] | [0,2,7,18,29,40,51,62,42,23,31] | $Y_{9,9,8,8,8,7,7,7,7,7,7,1}$ [32] | $Y_{9,9,8,8,8,7,7,7,7,7,7}$ [32] |
| | [0,11,0,0,0,0,0,0,1,0] | [0,0,11,22,33,44,55,66,44,23,33] | $Y_{8,8,8,8,8,8,8,8,8,8,8,1}$ [13] | $Y_{8,8,8,8,8,8,8,8,8,8,8}$ [14] |
| 24 | [0,0,0,0,3,0,1,1,2,2] | [5,10,15,20,25,33,41,50,36,24,24] | $Z_{10,10,10,10,10,5,5,5,3,2,1,1}$ [72] | |
| | [0,0,0,1,0,3,0,1,2,2] | [5,10,15,20,26,32,41,50,36,24,24] | $Z_{10,10,10,10,10,6,4,4,4,2,1,1}$ [90] | |
| | [0,0,0,1,1,0,3,0,2,2] | [5,10,15,20,26,33,40,50,36,24,24] | $Z_{10,10,10,10,10,6,5,3,3,3,1,1}$ [90] | |
| | [0,0,0,1,1,1,0,3,1,1] | [5,10,15,20,26,33,41,49,36,24,24] | $Z_{10,10,10,10,10,6,5,4,2,2,2,1}$ [120] | |
| | [0,0,1,0,0,1,2,2,1,1] | [5,10,15,21,27,33,40,49,36,24,24] | $Z_{10,10,10,10,10,7,4,3,3,2,2,1}$ [128] | |
| | [0,0,3,1,0,0,0,1,3,3] | [4,8,12,19,27,35,43,51,36,24,24] | $Z_{10,10,10,10,7,7,7,6,2,1,1,1}$ [80] | |
| | [0,1,1,1,0,2,0,0,3,3] | [4,8,13,19,26,33,42,51,36,24,24] | $Z_{10,10,10,10,8,7,6,4,4,1,1,1}$ [144] | |
| | [0,1,1,1,1,0,0,2,2,2] | [4,8,13,19,26,34,42,50,36,24,24] | $Z_{10,10,10,10,8,7,6,5,2,2,1,1}$ [192] | |
| | [0,1,2,0,0,0,2,1,2,2] | [4,8,13,20,27,34,41,50,36,24,24] | $Z_{10,10,10,10,8,7,7,3,3,2,1,1}$ [120] | |
| | [0,2,0,0,1,1,1,1,2,2] | [4,8,14,20,26,33,41,50,36,24,24] | $Z_{10,10,10,10,8,8,5,4,3,2,1,1}$ [192] | |
| | [0,2,1,0,0,0,0,4,1,1] | [4,8,14,21,28,35,42,49,36,24,24] | $Z_{10,10,10,10,8,8,7,2,2,2,2,1}$ [72] | |
| | [1,0,0,0,0,0,1,5,0,0] | [5,11,17,23,29,35,41,48,36,24,24] | $Z_{10,10,10,10,10,9,3,2,2,2,2,2}$ [28] | |
| | [1,0,0,1,2,1,0,0,3,3] | [4,9,14,19,25,33,42,51,36,24,24] | $Z_{10,10,10,10,9,6,5,5,4,1,1,1}$ [128] | |
| | [1,0,0,2,0,1,1,1,2,2] | [4,9,14,19,26,33,41,50,36,24,24] | $Z_{10,10,10,10,9,6,6,4,3,2,1,1}$ [192] | |
| | [1,0,1,1,0,0,1,3,1,1] | [4,9,14,20,27,34,41,49,36,24,24] | $Z_{10,10,10,10,9,7,6,3,2,2,2,1}$ [192] | |
| | [1,1,0,0,0,1,3,0,2,2] | [4,9,15,21,27,33,40,50,36,24,24] | $Z_{10,10,10,10,9,8,4,3,3,3,1,1}$ [120] | |
| | [1,1,0,0,0,2,0,3,1,1] | [4,9,15,21,27,33,41,49,36,24,24] | $Z_{10,10,10,10,9,8,4,4,2,2,2,1}$ [120] | |
| | [1,1,3,0,0,0,0,0,4,4] | [3,7,12,20,28,36,44,52,36,24,24] | $Z_{10,10,10,9,8,7,7,7,1,1,1,1}$ [56] | |
| | [1,2,0,2,0,0,0,1,3,3] | [3,7,13,19,27,35,43,51,36,24,24] | $Z_{10,10,10,9,8,8,6,6,2,1,1,1}$ [120] | |
| | [1,2,1,0,0,1,1,0,3,3] | [3,7,13,20,27,34,42,51,36,24,24] | $Z_{10,10,10,9,8,8,7,4,3,1,1,1}$ [192] | |
| | [1,3,0,0,0,0,1,2,2,2] | [3,7,14,21,28,35,42,50,36,24,24] | $Z_{10,10,10,9,8,8,8,3,2,2,1,1}$ [96] | |
| | [2,0,0,0,0,0,3,2,1,1] | [4,10,16,22,28,34,40,49,36,24,24] | $Z_{10,10,10,10,9,9,3,3,3,2,2,1}$ [56] | |
| | [2,0,1,1,1,0,1,0,3,3] | [3,8,13,19,26,34,42,51,36,24,24] | $Z_{10,10,10,9,9,7,6,5,3,1,1,1}$ [216] | |
| | [2,0,2,0,0,1,0,2,2,2] | [3,8,13,20,27,34,42,50,36,24,24] | $Z_{10,10,10,9,9,7,7,4,2,2,1,1}$ [144] | |
| | [2,1,0,0,1,2,0,0,3,3] | [3,8,14,20,26,33,42,51,36,24,24] | $Z_{10,10,10,9,9,8,5,4,4,1,1,1}$ [128] | |
| | [2,1,0,0,2,0,0,2,2,2] | [3,8,14,20,26,34,42,50,36,24,24] | $Z_{10,10,10,9,9,8,5,5,2,2,1,1}$ [128] | |
| | [2,1,0,1,0,0,2,1,2,2] | [3,8,14,20,27,34,41,50,36,24,24] | $Z_{10,10,10,9,9,8,6,3,3,2,1,1}$ [192] | |
| | [3,0,0,0,0,2,1,1,2,2] | [3,9,15,21,27,33,41,50,36,24,24] | $Z_{10,10,10,9,9,9,4,4,3,2,1,1}$ [96] | |
| | [3,0,0,1,0,0,0,4,1,1] | [3,9,15,21,28,35,42,49,36,24,24] | $Z_{10,10,10,9,9,9,6,2,2,2,2,1}$ [80] | |
| | [3,1,1,1,0,0,0,0,4,4] | [2,7,13,20,28,36,44,52,36,24,24] | $Z_{10,10,9,9,9,8,7,6,1,1,1,1}$ [96] | |
| | [3,2,0,0,0,1,0,1,3,3] | [2,7,14,21,28,35,43,51,36,24,24] | $Z_{10,10,9,9,9,8,8,4,2,1,1,1}$ [120] | |
| | [4,0,0,1,1,0,0,1,3,3] | [2,8,14,20,27,35,43,51,36,24,24] | $Z_{10,10,9,9,9,9,6,5,2,1,1,1}$ [128] | |
| | [4,0,1,0,0,0,2,0,3,3] | [2,8,14,21,28,35,42,51,36,24,24] | $Z_{10,10,9,9,9,9,7,3,3,1,1,1}$ [90] | |
| | [4,1,0,0,0,0,0,3,2,2] | [2,8,15,22,29,36,43,50,36,24,24] | $Z_{10,10,9,9,9,9,8,2,2,2,1,1}$ [56] | |
| | [0,0,0,0,1,4,0,1,1,1] | [5,10,15,20,25,31,41,51,37,24,25] | $Z_{10,10,10,10,10,5,4,4,4,4,2,1}$ [72] | |
| | [0,0,0,0,2,1,2,2,0,0] | [5,10,15,20,25,32,40,50,37,24,25] | $Z_{10,10,10,10,10,5,5,4,3,3,2,2}$ [48] | |
| | [0,0,1,3,0,1,1,0,2,2] | [4,8,12,17,25,33,42,52,37,24,25] | $Z_{10,10,10,10,7,6,6,6,4,3,1,1}$ [144] | |
| | [0,0,2,0,3,0,1,0,2,2] | [4,8,12,18,24,33,42,52,37,24,25] | $Z_{10,10,10,10,7,7,5,5,5,3,1,1}$ [108] | |
| | [0,0,2,1,0,3,0,0,2,2] | [4,8,12,18,25,32,42,52,37,24,25] | $Z_{10,10,10,10,7,7,6,4,4,4,1,1}$ [96] | |
| | [0,0,2,1,1,0,2,1,1,1] | [4,8,12,18,25,33,41,51,37,24,25] | $Z_{10,10,10,10,7,7,6,5,3,3,2,1}$ [192] | |
| | [0,0,3,0,1,0,0,4,0,0] | [4,8,12,19,26,34,42,50,37,24,25] | $Z_{10,10,10,10,7,7,7,5,2,2,2,2}$ [48] | |
| | [0,1,0,1,2,2,0,0,2,2] | [4,8,13,18,24,32,42,52,37,24,25] | $Z_{10,10,10,10,8,6,5,5,4,4,1,1}$ [144] | |
| | [0,1,0,1,3,0,0,2,1,1] | [4,8,13,18,24,33,42,51,37,24,25] | $Z_{10,10,10,10,8,6,5,5,5,2,2,1}$ [144] | |
| | [0,1,0,2,0,2,1,1,1,1] | [4,8,13,18,25,32,41,51,37,24,25] | $Z_{10,10,10,10,8,6,6,4,4,3,2,1}$ [216] | |
| | [0,1,0,3,0,0,0,4,0,0] | [4,8,13,18,26,34,42,50,37,24,25] | $Z_{10,10,10,10,8,6,6,6,2,2,2,2}$ [45] | |
| | [0,1,1,0,2,0,1,3,0,0] | [4,8,13,19,25,33,41,50,37,24,25] | $Z_{10,10,10,10,8,7,5,5,3,2,2,2}$ [108] | |
| | [0,1,1,1,0,0,4,0,1,1] | [4,8,13,19,26,33,40,51,37,24,25] | $Z_{10,10,10,10,8,7,6,3,3,3,3,1}$ [144] | |
| | [0,2,0,0,0,2,3,0,1,1] | [4,8,14,20,26,32,40,51,37,24,25] | $Z_{10,10,10,10,8,8,4,4,3,3,3,1}$ [90] | |
| | [0,2,0,0,0,3,0,3,0,0] | [4,8,14,20,26,32,41,50,37,24,25] | $Z_{10,10,10,10,8,8,4,4,4,2,2,2}$ [45] | |
| | [0,2,0,0,1,0,3,2,0,0] | [4,8,14,20,26,33,40,50,37,24,25] | $Z_{10,10,10,10,8,8,5,3,3,3,2,2}$ [72] | |
| | [0,2,2,1,0,1,0,1,2,2] | [3,6,11,18,26,34,43,52,37,24,25] | $Z_{10,10,10,8,8,7,7,6,4,2,1,1}$ [216] | |
| | [0,3,0,1,2,0,0,1,2,2] | [3,6,12,18,25,34,43,52,37,24,25] | $Z_{10,10,10,8,8,8,6,5,5,2,1,1}$ [144] | |
| | [0,3,0,2,0,0,2,0,2,2] | [3,6,12,18,26,34,42,52,37,24,25] | $Z_{10,10,10,8,8,8,6,6,3,3,1,1}$ [108] | |

| | | | |
|---|---|---|---|
| | [0,3,1,0,0,2,1,0,2,2] | [3,6,12,19,26,33,42,52,37,24,25] | $Z_{10,10,10,8,8,8,7,4,4,3,1,1}$ [144] |
| | [0,3,1,0,1,0,1,2,1,1] | [3,6,12,19,26,34,42,51,37,24,25] | $Z_{10,10,10,8,8,8,7,5,3,2,2,1}$ [216] |
| | [1,0,0,0,3,1,1,1,1,1] | [4,9,14,19,24,32,41,51,37,24,25] | $Z_{10,10,10,10,9,5,5,5,4,3,2,1}$ [160] |
| | [1,0,0,1,1,1,3,0,1,1] | [4,9,14,19,25,32,40,51,37,24,25] | $Z_{10,10,10,10,9,6,5,4,3,3,3,1}$ [192] |
| | [1,0,0,1,1,2,0,3,0,0] | [4,9,14,19,25,32,41,50,37,24,25] | $Z_{10,10,10,10,9,6,5,4,4,2,2,2}$ [96] |
| | [1,0,0,2,0,0,3,2,0,0] | [4,9,14,19,26,33,40,50,37,24,25] | $Z_{10,10,10,10,9,6,6,3,3,3,2,2}$ [64] |
| | [1,0,1,0,0,2,2,2,0,0] | [4,9,14,20,26,32,40,50,37,24,25] | $Z_{10,10,10,10,9,7,4,4,3,3,2,2}$ [96] |
| | [1,0,2,3,0,0,0,0,3,3] | [3,7,11,17,26,35,44,53,37,24,25] | $Z_{10,10,10,9,7,7,6,6,6,1,1,1}$ [72] |
| | [1,0,3,0,2,0,0,1,2,2] | [3,7,11,18,25,34,43,52,37,24,25] | $Z_{10,10,10,9,7,7,7,5,5,2,1,1}$ [144] |
| | [1,0,3,1,0,0,2,0,2,2] | [3,7,11,18,26,34,42,52,37,24,25] | $Z_{10,10,10,9,7,7,7,6,3,3,1,1}$ [144] |
| | [1,0,4,0,0,0,0,3,1,1] | [3,7,11,19,27,35,43,51,37,24,25] | $Z_{10,10,10,9,7,7,7,7,2,2,2,1}$ [72] |
| | [1,1,0,3,1,0,0,1,2,2] | [3,7,12,17,25,34,43,52,37,24,25] | $Z_{10,10,10,9,8,6,6,6,5,2,1,1}$ [192] |
| | [1,1,1,1,1,1,0,2,1,1] | [3,7,12,18,25,33,42,51,37,24,25] | $Z_{10,10,10,9,8,7,6,5,4,2,2,1}$ [384] |
| | [1,1,2,0,0,1,2,1,1,1] | [3,7,12,19,26,33,41,51,37,24,25] | $Z_{10,10,10,9,8,7,7,4,3,3,2,1}$ [256] |
| | [1,2,0,0,1,3,0,0,2,2] | [3,7,13,19,25,32,42,52,37,24,25] | $Z_{10,10,10,9,8,8,5,4,4,4,1,1}$ [128] |
| | [1,2,0,0,2,0,2,1,1,1] | [3,7,13,19,25,33,41,51,37,24,25] | $Z_{10,10,10,9,8,8,5,5,3,3,2,1}$ [192] |
| | [1,2,0,1,1,0,0,4,0,0] | [3,7,13,19,26,34,42,50,37,24,25] | $Z_{10,10,10,9,8,8,6,5,2,2,2,2}$ [96] |
| | [1,2,1,0,0,0,2,3,0,0] | [3,7,13,20,27,34,41,50,37,24,25] | $Z_{10,10,10,9,8,8,7,3,3,2,2,2}$ [80] |
| | [1,4,0,1,0,1,0,0,3,3] | [2,5,12,19,27,35,44,53,37,24,25] | $Z_{10,10,9,8,8,8,8,6,4,1,1,1}$ [144] |
| | [1,4,1,0,0,0,0,2,2,2] | [2,5,12,20,28,36,44,52,37,24,25] | $Z_{10,10,9,8,8,8,8,7,2,2,1,1}$ [96] |
| | [2,0,0,1,3,0,1,0,2,2] | [3,8,13,18,24,33,42,52,37,24,25] | $Z_{10,10,10,9,9,6,5,5,5,3,1,1}$ [144] |
| | [2,0,0,2,0,3,0,0,2,2] | [3,8,13,18,25,32,42,52,37,24,25] | $Z_{10,10,10,9,9,6,6,4,4,4,1,1}$ [96] |
| | [2,0,0,2,1,0,2,1,1,1] | [3,8,13,18,25,33,41,51,37,24,25] | $Z_{10,10,10,9,9,6,6,5,3,3,2,1}$ [192] |
| | [2,0,1,0,1,2,1,1,1,1] | [3,8,13,19,25,32,41,51,37,24,25] | $Z_{10,10,10,9,9,7,5,4,4,3,2,1}$ [288] |
| | [2,0,1,1,0,1,1,3,0,0] | [3,8,13,19,26,33,41,50,37,24,25] | $Z_{10,10,10,9,9,7,6,4,3,2,2,2}$ [144] |
| | [2,1,0,0,1,0,4,0,1,1] | [3,8,14,20,26,33,40,51,37,24,25] | $Z_{10,10,10,9,9,8,5,3,3,3,3,1}$ [144] |
| | [2,1,2,1,1,0,0,0,3,3] | [2,6,11,18,26,35,44,53,37,24,25] | $Z_{10,10,9,9,8,7,7,6,5,1,1,1}$ [160] |
| | [2,1,3,0,0,0,1,1,2,2] | [2,6,11,19,27,35,43,52,37,24,25] | $Z_{10,10,9,9,8,7,7,7,3,2,1,1}$ [160] |
| | [2,2,0,2,0,1,0,1,2,2] | [2,6,12,18,26,34,43,52,37,24,25] | $Z_{10,10,9,9,8,8,6,6,4,2,1,1}$ [216] |
| | [2,2,1,0,1,0,2,0,2,2] | [2,6,12,19,26,34,42,52,37,24,25] | $Z_{10,10,9,9,8,8,7,5,3,3,1,1}$ [216] |
| | [2,2,1,1,0,0,0,3,1,1] | [2,6,12,19,27,35,43,51,37,24,25] | $Z_{10,10,9,9,8,8,7,6,2,2,2,1}$ [160] |
| | [2,3,0,0,0,1,1,2,1,1] | [2,6,13,20,27,34,42,51,37,24,25] | $Z_{10,10,9,9,8,8,8,4,3,2,2,1}$ [160] |
| | [3,0,0,0,0,1,3,2,0,0] | [3,9,15,21,27,33,40,50,37,24,25] | $Z_{10,10,10,9,9,9,4,3,3,3,2,2}$ [48] |
| | [3,0,1,1,2,0,0,1,2,2] | [2,7,12,18,25,34,43,52,37,24,25] | $Z_{10,10,9,9,9,7,6,5,5,2,1,1}$ [192] |
| | [3,0,1,2,0,0,2,0,2,2] | [2,7,12,18,26,34,42,52,37,24,25] | $Z_{10,10,9,9,9,7,6,6,3,3,1,1}$ [144] |
| | [3,0,2,0,0,2,1,0,2,2] | [2,7,12,19,26,33,42,52,37,24,25] | $Z_{10,10,9,9,9,7,7,4,4,3,1,1}$ [144] |
| | [3,0,2,0,1,0,1,2,1,1] | [2,7,12,19,26,34,42,51,37,24,25] | $Z_{10,10,9,9,9,7,7,5,3,2,2,1}$ [216] |
| | [3,1,0,0,2,1,1,0,2,2] | [2,7,13,19,25,33,42,52,37,24,25] | $Z_{10,10,9,9,9,8,5,5,4,3,1,1}$ [192] |
| | [3,1,0,1,0,2,0,2,1,1] | [2,7,13,19,26,33,42,51,37,24,25] | $Z_{10,10,9,9,9,8,6,4,4,2,2,1}$ [216] |
| | [3,1,1,0,0,0,3,1,1,1] | [2,7,13,20,27,34,41,51,37,24,25] | $Z_{10,10,9,9,9,8,7,3,3,3,2,1}$ [160] |
| | [3,2,0,0,0,0,1,4,0,0] | [2,7,14,21,28,35,42,50,37,24,25] | $Z_{10,10,9,9,9,8,8,3,2,2,2,2}$ [48] |
| | [3,4,0,0,0,0,0,1,3,3] | [1,5,13,21,29,37,45,53,37,24,25] | $Z_{10,9,9,9,8,8,8,8,2,1,1,1}$ [56] |
| | [4,0,0,0,1,1,2,1,1,1] | [2,8,14,20,26,33,41,51,37,24,25] | $Z_{10,10,9,9,9,9,5,4,3,3,2,1}$ [160] |
| | [4,0,0,1,0,1,0,4,0,0] | [2,8,14,20,27,34,42,50,37,24,25] | $Z_{10,10,9,9,9,9,6,4,2,2,2,2}$ [72] |
| | [4,1,1,1,0,1,0,0,3,3] | [1,6,12,19,27,35,44,53,37,24,25] | $Z_{10,9,9,9,9,8,7,6,4,1,1,1}$ [192] |
| | [4,1,2,0,0,0,0,2,2,2] | [1,6,12,20,28,36,44,52,37,24,25] | $Z_{10,9,9,9,9,8,7,7,2,2,1,1}$ [96] |
| | [4,2,0,0,1,0,1,1,2,2] | [1,6,13,20,27,35,43,52,37,24,25] | $Z_{10,9,9,9,9,8,8,5,3,2,1,1}$ [192] |
| | [5,0,0,1,2,0,0,0,3,3] | [1,7,13,19,26,35,44,53,37,24,25] | $Z_{10,9,9,9,9,9,6,5,5,1,1,1}$ [80] |
| | [5,0,0,2,0,0,1,1,2,2] | [1,7,13,19,27,35,43,52,37,24,25] | $Z_{10,9,9,9,9,9,6,6,3,2,1,1}$ [128] |
| | [5,0,1,0,0,2,0,1,2,2] | [1,7,13,20,27,34,43,52,37,24,25] | $Z_{10,9,9,9,9,9,7,4,4,2,1,1}$ [144] |
| | [5,1,0,0,0,0,3,0,2,2] | [1,7,14,21,28,35,42,52,37,24,25] | $Z_{10,9,9,9,9,9,8,3,3,3,1,1}$ [72] |
| | [5,1,0,0,0,1,0,3,1,1] | [1,7,14,21,28,35,43,51,37,24,25] | $Z_{10,9,9,9,9,9,8,4,2,2,2,1}$ [120] |
| | [7,0,1,0,0,0,0,0,4,4] | [0,7,14,22,30,38,46,54,37,24,25] | $Z_{9,9,9,9,9,9,9,7,1,1,1,1}$ [42] |
| | [0,0,0,4,1,1,0,1,1,1] | [4,8,12,16,24,33,43,53,38,24,26] | $Z_{10,10,10,10,6,6,6,6,5,4,2,1}$ [120] |
| | [0,0,1,2,1,2,0,2,0,0] | [4,8,12,17,24,32,42,52,38,24,26] | $Z_{10,10,10,10,7,6,6,5,4,4,2,2}$ [96] |
| | [0,0,1,3,0,0,3,1,0,0] | [4,8,12,17,25,33,41,52,38,24,26] | $Z_{10,10,10,10,7,6,6,6,3,3,3,2}$ [64] |
| | [0,0,2,0,2,1,2,1,0,0] | [4,8,12,18,24,32,41,52,38,24,26] | $Z_{10,10,10,10,7,7,5,5,4,3,3,2}$ [96] |
| | [0,1,0,1,1,4,0,0,1,1] | [4,8,13,18,24,31,42,53,38,24,26] | $Z_{10,10,10,10,8,6,5,4,4,4,4,1}$ [144] |
| | [0,1,1,0,0,4,1,1,0,0] | [4,8,13,19,25,31,41,52,38,24,26] | $Z_{10,10,10,10,8,7,4,4,4,4,3,2}$ [96] |
| | [0,1,1,0,1,1,4,0,0,0] | [4,8,13,19,25,32,40,52,38,24,26] | $Z_{10,10,10,10,8,7,5,4,3,3,3,3}$ [72] |
| | [0,1,3,1,1,0,1,1,1,1] | [3,6,10,17,25,34,43,53,38,24,26] | $Z_{10,10,10,8,7,7,7,6,5,3,2,1}$ [288] |
| | [0,2,0,4,0,1,0,0,2,2] | [3,6,11,16,25,34,44,54,38,24,26] | $Z_{10,10,10,8,8,6,6,6,6,4,1,1}$ [108] |
| | [0,2,1,1,2,1,0,1,1,1] | [3,6,11,17,24,33,43,53,38,24,26] | $Z_{10,10,10,8,8,7,6,5,5,4,2,1}$ [288] |
| | [0,2,1,2,0,1,2,0,1,1] | [3,6,11,17,25,33,42,53,38,24,26] | $Z_{10,10,10,8,8,7,6,6,4,3,3,1}$ [216] |
| | [0,2,1,2,1,0,0,3,0,0] | [3,6,11,17,25,34,43,52,38,24,26] | $Z_{10,10,10,8,8,7,6,6,5,2,2,2}$ [96] |
| | [0,2,2,0,1,1,1,2,0,0] | [3,6,11,18,25,33,42,52,38,24,26] | $Z_{10,10,10,8,8,7,7,5,4,3,2,2}$ [144] |
| | [0,3,0,0,3,0,2,0,1,1] | [3,6,12,18,24,33,42,53,38,24,26] | $Z_{10,10,10,8,8,8,5,5,5,3,3,1}$ [108] |
| | [0,3,0,1,0,3,1,0,1,1] | [3,6,12,18,25,32,42,53,38,24,26] | $Z_{10,10,10,8,8,8,6,4,4,4,3,1}$ [162] |
| | [0,4,3,0,0,0,0,0,3,3] | [2,4,10,19,28,37,46,55,38,24,26] | $Z_{10,10,8,8,8,8,7,7,7,1,1,1}$ [42] |
| | [0,5,0,2,0,0,0,1,2,2] | [2,4,11,18,27,36,45,54,38,24,26] | $Z_{10,10,8,8,8,8,8,6,6,2,1,1}$ [90] |
| | [0,5,1,0,0,1,1,0,2,2] | [2,4,11,19,27,35,44,54,38,24,26] | $Z_{10,10,8,8,8,8,8,7,4,3,1,1}$ [144] |

| | | | |
|---|---|---|---|
| | [0,6,0,0,0,0,1,2,1,1] | [2,4,12,20,28,36,44,53,38,24,26] | $Z_{10,10,8,8,8,8,8,8,3,2,2,1}$ [72] |
| | [1,0,0,0,2,3,1,1,0,0] | [4,9,14,19,24,31,41,52,38,24,26] | $Z_{10,10,10,10,9,5,5,4,4,4,3,2}$ [80] |
| | [1,0,1,3,2,0,0,0,2,2] | [3,7,11,16,24,34,44,54,38,24,26] | $Z_{10,10,10,9,7,6,6,6,5,5,1,1}$ [120] |
| | [1,0,1,4,0,0,1,1,1,1] | [3,7,11,16,25,34,43,53,38,24,26] | $Z_{10,10,10,9,7,6,6,6,6,3,2,1}$ [192] |
| | [1,0,2,1,2,0,2,0,1,1] | [3,7,11,17,24,33,42,53,38,24,26] | $Z_{10,10,10,9,7,7,6,5,5,3,3,1}$ [216] |
| | [1,0,2,2,0,1,1,2,0,0] | [3,7,11,17,25,33,42,52,38,24,26] | $Z_{10,10,10,9,7,7,6,6,4,3,2,2}$ [144] |
| | [1,0,3,0,0,3,1,0,1,1] | [3,7,11,18,25,32,42,53,38,24,26] | $Z_{10,10,10,9,7,7,7,4,4,4,3,1}$ [144] |
| | [1,1,0,2,1,2,1,0,1,1] | [3,7,12,17,24,32,42,53,38,24,26] | $Z_{10,10,10,9,8,6,6,5,4,4,3,1}$ [288] |
| | [1,1,0,2,2,0,1,2,0,0] | [3,7,12,17,24,33,42,52,38,24,26] | $Z_{10,10,10,9,8,6,6,5,5,3,2,2}$ [144] |
| | [1,1,1,0,2,2,0,2,0,0] | [3,7,12,18,24,32,42,52,38,24,26] | $Z_{10,10,10,9,8,7,5,5,4,4,2,2}$ [144] |
| | [1,1,1,1,0,2,2,1,0,0] | [3,7,12,18,25,32,41,52,38,24,26] | $Z_{10,10,10,9,8,7,6,4,4,3,3,2}$ [192] |
| | [1,2,2,2,0,0,1,0,2,2] | [2,5,10,17,26,35,44,54,38,24,26] | $Z_{10,10,9,8,8,7,7,6,6,3,1,1}$ [192] |
| | [1,2,3,0,0,2,0,0,2,2] | [2,5,10,18,26,34,44,54,38,24,26] | $Z_{10,10,9,8,8,7,7,7,4,4,1,1}$ [128] |
| | [1,2,3,0,1,0,0,2,1,1] | [2,5,10,18,26,35,44,53,38,24,26] | $Z_{10,10,9,8,8,7,7,7,5,2,2,1}$ [192] |
| | [1,3,0,2,1,1,0,0,2,2] | [2,5,11,17,25,34,44,54,38,24,26] | $Z_{10,10,9,8,8,8,6,6,5,4,1,1}$ [192] |
| | [1,3,0,3,0,0,0,2,1,1] | [2,5,11,17,26,35,44,53,38,24,26] | $Z_{10,10,9,8,8,8,6,6,6,2,2,1}$ [120] |
| | [1,3,1,0,2,0,1,1,1,1] | [2,5,11,18,25,34,43,53,38,24,26] | $Z_{10,10,9,8,8,8,7,5,5,3,2,1}$ [288] |
| | [1,3,2,0,0,0,1,3,0,0] | [2,5,11,19,27,35,43,52,38,24,26] | $Z_{10,10,9,8,8,8,7,7,3,2,2,2}$ [80] |
| | [1,4,0,0,0,3,0,1,1,1] | [2,5,12,19,26,33,43,53,38,24,26] | $Z_{10,10,9,8,8,8,8,4,4,4,2,1}$ [120] |
| | [1,4,0,0,1,1,0,3,0,0] | [2,5,12,19,26,34,43,52,38,24,26] | $Z_{10,10,9,8,8,8,8,5,4,2,2,2}$ [96] |
| | [2,0,0,1,2,1,2,1,0,0] | [3,8,13,18,24,32,41,52,38,24,26] | $Z_{10,10,10,9,9,6,5,5,4,3,3,2}$ [128] |
| | [2,0,1,0,0,5,0,0,1,1] | [3,8,13,19,25,31,42,53,38,24,26] | $Z_{10,10,10,9,9,7,4,4,4,4,4,1}$ [96] |
| | [2,0,1,1,0,0,5,0,0,0] | [3,8,13,19,26,33,40,52,38,24,26] | $Z_{10,10,10,9,9,7,6,3,3,3,3,3}$ [48] |
| | [2,0,3,1,1,1,0,0,2,2] | [2,6,10,17,25,34,44,54,38,24,26] | $Z_{10,10,9,9,7,7,7,6,5,4,1,1}$ [192] |
| | [2,0,3,2,0,0,0,2,1,1] | [2,6,10,17,26,35,44,53,38,24,26] | $Z_{10,10,9,9,7,7,7,6,6,2,2,1}$ [120] |
| | [2,0,4,0,0,1,1,1,1,1] | [2,6,10,18,26,34,43,53,38,24,26] | $Z_{10,10,9,9,7,7,7,7,4,3,2,1}$ [192] |
| | [2,1,0,0,0,2,4,0,0,0] | [3,8,14,20,26,32,40,52,38,24,26] | $Z_{10,10,10,9,9,8,4,4,3,3,3,3}$ [40] |
| | [2,1,1,1,3,0,0,0,2,2] | [2,6,11,17,24,34,44,54,38,24,26] | $Z_{10,10,9,9,8,7,6,5,5,5,1,1}$ [160] |
| | [2,1,1,2,0,2,0,1,1,1] | [2,6,11,17,25,33,43,53,38,24,26] | $Z_{10,10,9,9,8,7,6,6,4,4,2,1}$ [288] |
| | [2,1,2,0,1,1,2,0,1,1] | [2,6,11,18,25,33,42,53,38,24,26] | $Z_{10,10,9,9,8,7,7,5,4,3,3,1}$ [288] |
| | [2,1,2,0,2,0,0,3,0,0] | [2,6,11,18,25,34,43,52,38,24,26] | $Z_{10,10,9,9,8,7,7,5,5,2,2,2}$ [96] |
| | [2,1,2,1,0,0,2,2,0,0] | [2,6,11,18,26,34,42,52,38,24,26] | $Z_{10,10,9,9,8,7,7,6,3,3,2,2}$ [128] |
| | [2,2,0,0,3,1,0,1,1,1] | [2,6,12,18,24,33,43,53,38,24,26] | $Z_{10,10,9,9,8,8,5,5,5,4,2,1}$ [192] |
| | [2,2,0,1,1,1,1,2,0,0] | [2,6,12,18,25,33,42,52,38,24,26] | $Z_{10,10,9,9,8,8,6,5,4,3,2,2}$ [192] |
| | [2,4,1,0,1,0,0,1,2,2] | [1,4,11,19,27,36,45,54,38,24,26] | $Z_{10,9,9,8,8,8,8,7,5,2,1,1}$ [192] |
| | [2,5,0,0,0,0,2,0,2,2] | [1,4,12,20,28,36,44,54,38,24,26] | $Z_{10,9,9,8,8,8,8,8,3,3,1,1}$ [72] |
| | [3,0,0,2,2,1,0,1,1,1] | [2,7,12,17,24,33,43,53,38,24,26] | $Z_{10,10,9,9,9,6,6,5,5,4,2,1}$ [192] |
| | [3,0,0,3,0,1,2,0,1,1] | [2,7,12,17,25,33,42,53,38,24,26] | $Z_{10,10,9,9,9,6,6,6,4,3,3,1}$ [144] |
| | [3,0,1,0,3,0,2,0,1,1] | [2,7,12,18,24,33,42,53,38,24,26] | $Z_{10,10,9,9,9,7,5,5,5,3,3,1}$ [162] |
| | [3,0,1,1,0,3,1,0,1,1] | [2,7,12,18,25,32,42,53,38,24,26] | $Z_{10,10,9,9,9,7,6,4,4,4,3,1}$ [216] |
| | [3,0,2,0,0,1,3,1,0,0] | [2,7,12,19,26,33,41,52,38,24,26] | $Z_{10,10,9,9,9,7,7,4,3,3,3,2}$ [96] |
| | [3,1,0,0,1,3,0,2,0,0] | [2,7,13,19,25,32,42,52,38,24,26] | $Z_{10,10,9,9,9,8,5,4,4,4,2,2}$ [96] |
| | [3,1,0,0,2,0,3,1,0,0] | [2,7,13,19,25,33,41,52,38,24,26] | $Z_{10,10,9,9,9,8,5,5,3,3,3,2}$ [96] |
| | [3,1,3,1,0,0,0,1,2,2] | [1,5,10,18,27,36,45,54,38,24,26] | $Z_{10,9,9,9,8,7,7,7,6,2,1,1}$ [160] |
| | [3,2,1,1,0,2,0,0,2,2] | [1,5,11,18,26,34,44,54,38,24,26] | $Z_{10,9,9,9,8,8,7,6,4,4,1,1}$ [192] |
| | [3,2,1,1,1,0,0,2,1,1] | [1,5,11,18,26,35,44,53,38,24,26] | $Z_{10,9,9,9,8,8,7,6,5,2,2,1}$ [256] |
| | [3,2,2,0,0,0,2,1,1,1] | [1,5,11,19,27,35,43,53,38,24,26] | $Z_{10,9,9,9,8,8,7,7,3,3,2,1}$ [160] |
| | [3,3,0,0,1,1,1,1,1,1] | [1,5,12,19,26,34,43,53,38,24,26] | $Z_{10,9,9,9,8,8,8,5,4,3,2,1}$ [256] |
| | [3,3,1,0,0,0,0,4,0,0] | [1,5,12,20,28,36,44,52,38,24,26] | $Z_{10,9,9,9,8,8,8,7,2,2,2,2}$ [48] |
| | [4,0,0,0,0,3,2,1,0,0] | [2,8,14,20,26,32,41,52,38,24,26] | $Z_{10,10,9,9,9,9,4,4,4,3,3,2}$ [48] |
| | [4,0,1,3,0,0,1,0,2,2] | [1,6,11,17,26,35,44,54,38,24,26] | $Z_{10,9,9,9,9,7,6,6,6,3,1,1}$ [144] |
| | [4,0,2,0,2,1,0,0,2,2] | [1,6,11,18,25,34,44,54,38,24,26] | $Z_{10,9,9,9,9,7,7,5,5,4,1,1}$ [144] |
| | [4,0,2,1,0,1,1,1,1,1] | [1,6,11,18,26,34,43,53,38,24,26] | $Z_{10,9,9,9,9,7,7,6,4,3,2,1}$ [288] |
| | [4,1,0,1,2,0,1,1,1,1] | [1,6,12,18,25,34,43,53,38,24,26] | $Z_{10,9,9,9,9,8,6,5,5,3,2,1}$ [288] |
| | [4,1,1,0,0,3,0,1,1,1] | [1,6,12,19,26,33,43,53,38,24,26] | $Z_{10,9,9,9,9,8,7,4,4,4,2,1}$ [192] |
| | [4,1,1,0,1,0,3,0,1,1] | [1,6,12,19,26,34,42,53,38,24,26] | $Z_{10,9,9,9,9,8,7,5,3,3,3,1}$ [216] |
| | [4,1,1,0,1,1,0,3,0,0] | [1,6,12,19,26,34,43,52,38,24,26] | $Z_{10,9,9,9,9,8,7,5,4,2,2,2}$ [144] |
| | [4,2,0,0,0,1,2,2,0,0] | [1,6,13,20,27,34,42,52,38,24,26] | $Z_{10,9,9,9,9,8,8,4,3,3,2,2}$ [80] |
| | [5,0,0,0,2,2,0,1,1,1] | [1,7,13,19,25,33,43,53,38,24,26] | $Z_{10,9,9,9,9,9,5,5,4,4,2,1}$ [120] |
| | [5,0,0,1,0,2,2,0,1,1] | [1,7,13,19,26,33,42,53,38,24,26] | $Z_{10,9,9,9,9,9,6,4,4,3,3,1}$ [144] |
| | [5,0,0,1,1,0,2,2,0,0] | [1,7,13,19,26,34,42,52,38,24,26] | $Z_{10,9,9,9,9,9,6,5,3,3,2,2}$ [96] |
| | [5,1,2,1,0,0,0,0,3,3] | [0,5,11,19,28,37,46,55,38,24,26] | $Z_{9,9,9,9,9,8,7,7,6,1,1,1}$ [96] |
| | [5,2,0,1,1,0,0,1,2,2] | [0,5,12,19,27,36,45,54,38,24,26] | $Z_{9,9,9,9,9,8,8,6,5,2,1,1}$ [192] |
| | [5,2,1,0,0,0,2,0,2,2] | [0,5,12,20,28,36,44,54,38,24,26] | $Z_{9,9,9,9,9,8,8,7,3,3,1,1}$ [120] |
| | [5,3,0,0,0,0,0,3,1,1] | [0,5,13,21,29,37,45,53,38,24,26] | $Z_{9,9,9,9,9,8,8,8,2,2,2,1}$ [56] |
| | [6,0,1,1,0,1,1,0,2,2] | [0,6,12,19,27,35,44,54,38,24,26] | $Z_{9,9,9,9,9,9,7,6,4,3,1,1}$ [216] |
| | [6,0,2,0,0,0,1,2,1,1] | [0,6,12,20,28,36,44,53,38,24,26] | $Z_{9,9,9,9,9,9,7,7,3,2,2,1}$ [120] |
| | [6,1,0,0,1,1,0,2,1,1] | [0,6,13,20,27,35,44,53,38,24,26] | $Z_{9,9,9,9,9,9,8,5,4,2,2,1}$ [192] |
| | [7,0,0,0,0,1,2,1,1,1] | [0,7,14,21,28,35,43,53,38,24,26] | $Z_{9,9,9,9,9,9,9,4,3,3,2,1}$ [96] |
| | [0,0,0,4,0,3,0,1,0,0] | [4,8,12,16,24,32,43,54,39,24,27] | $Z_{10,10,10,10,6,6,6,6,4,4,4,2}$ [45] |
| | [0,0,0,4,1,0,3,0,0,0] | [4,8,12,16,24,33,42,54,39,24,27] | $Z_{10,10,10,10,6,6,6,6,5,3,3,3}$ [30] |

| | | | |
|---|---|---|---|
| | [0,0,2,0,1,4,1,0,0,0] | [4,8,12,18,24,31,42,54,39,24,27] | $Z_{10,10,10,10,7,7,5,4,4,4,4,3}$ [48] |
| | [0,0,4,2,1,0,0,1,1,1] | [3,6,9,16,25,35,45,55,39,24,27] | $Z_{10,10,10,7,7,7,7,6,6,5,2,1}$ [128] |
| | [0,0,5,0,1,1,1,0,1,1] | [3,6,9,17,25,34,44,55,39,24,27] | $Z_{10,10,10,7,7,7,7,7,5,4,3,1}$ [144] |
| | [0,0,5,1,0,0,1,2,0,0] | [3,6,9,17,26,35,44,54,39,24,27] | $Z_{10,10,10,7,7,7,7,7,6,3,2,2}$ [64] |
| | [0,1,2,2,1,2,0,0,1,1] | [3,6,10,16,24,33,44,55,39,24,27] | $Z_{10,10,10,8,7,7,6,6,5,4,4,1}$ [192] |
| | [0,1,2,2,2,0,0,2,0,0] | [3,6,10,16,24,34,44,54,39,24,27] | $Z_{10,10,10,8,7,7,6,6,5,5,2,2}$ [96] |
| | [0,1,2,3,0,0,2,1,0,0] | [3,6,10,16,25,34,43,54,39,24,27] | $Z_{10,10,10,8,7,7,6,6,6,3,3,2}$ [96] |
| | [0,1,3,0,2,1,1,1,0,0] | [3,6,10,17,24,33,43,54,39,24,27] | $Z_{10,10,10,8,7,7,7,5,5,4,3,2}$ [144] |
| | [0,1,4,0,0,0,4,0,0,0] | [3,6,10,18,26,34,42,54,39,24,27] | $Z_{10,10,10,8,7,7,7,7,3,3,3,3}$ [30] |
| | [0,2,0,3,1,1,1,1,0,0] | [3,6,11,16,24,33,43,54,39,24,27] | $Z_{10,10,10,8,8,6,6,6,5,4,3,2}$ [144] |
| | [0,2,1,1,1,3,0,1,0,0] | [3,6,11,17,24,32,43,54,39,24,27] | $Z_{10,10,10,8,8,7,6,5,4,4,4,2}$ [144] |
| | [0,2,1,1,2,0,3,0,0,0] | [3,6,11,17,24,33,42,54,39,24,27] | $Z_{10,10,10,8,8,7,6,5,5,3,3,3}$ [72] |
| | [0,2,2,0,0,3,2,0,0,0] | [3,6,11,18,25,32,42,54,39,24,27] | $Z_{10,10,10,8,8,7,7,4,4,4,3,3}$ [48] |
| | [0,3,0,0,2,2,2,0,0,0] | [3,6,12,18,24,32,42,54,39,24,27] | $Z_{10,10,10,8,8,8,5,5,4,4,3,3}$ [48] |
| | [0,3,3,1,1,0,0,0,2,2] | [2,4,9,17,26,36,46,56,39,24,27] | $Z_{10,10,8,8,8,7,7,7,6,5,1,1}$ [120] |
| | [0,3,4,0,0,0,1,1,1,1] | [2,4,9,18,27,36,45,55,39,24,27] | $Z_{10,10,8,8,8,7,7,7,7,3,2,1}$ [120] |
| | [0,4,1,1,2,0,0,1,1,1] | [2,4,10,17,25,35,45,55,39,24,27] | $Z_{10,10,8,8,8,8,7,6,5,5,2,1}$ [192] |
| | [0,4,1,2,0,0,2,0,1,1] | [2,4,10,17,26,35,44,55,39,24,27] | $Z_{10,10,8,8,8,8,7,6,6,3,3,1}$ [144] |
| | [0,4,2,0,0,2,1,0,1,1] | [2,4,10,18,26,34,44,55,39,24,27] | $Z_{10,10,8,8,8,8,7,7,4,4,3,1}$ [144] |
| | [0,4,2,0,1,0,1,2,0,0] | [2,4,10,18,26,35,44,54,39,24,27] | $Z_{10,10,8,8,8,8,7,7,5,3,2,2}$ [108] |
| | [0,5,0,0,2,1,1,0,1,1] | [2,4,11,18,25,34,44,55,39,24,27] | $Z_{10,10,8,8,8,8,8,5,5,4,3,1}$ [144] |
| | [0,5,0,1,0,2,0,2,0,0] | [2,4,11,18,26,34,44,54,39,24,27] | $Z_{10,10,8,8,8,8,8,6,4,4,2,2}$ [81] |
| | [1,0,0,6,0,0,0,1,1,1] | [3,7,11,15,25,35,45,55,39,24,27] | $Z_{10,10,10,9,6,6,6,6,6,6,2,1}$ [80] |
| | [1,0,2,1,1,2,2,0,0,0] | [3,7,11,17,24,32,42,54,39,24,27] | $Z_{10,10,10,9,7,7,6,5,4,4,3,3}$ [96] |
| | [1,1,3,3,0,0,0,0,2,2] | [2,5,9,16,26,36,46,56,39,24,27] | $Z_{10,10,9,8,7,7,7,6,6,6,1,1}$ [96] |
| | [1,1,4,0,2,0,0,1,1,1] | [2,5,9,17,25,35,45,55,39,24,27] | $Z_{10,10,9,8,7,7,7,7,5,5,2,1}$ [192] |
| | [1,1,4,1,0,0,2,0,1,1] | [2,5,9,17,26,35,44,55,39,24,27] | $Z_{10,10,9,8,7,7,7,7,6,3,3,1}$ [192] |
| | [1,1,5,0,0,0,0,3,0,0] | [2,5,9,18,27,36,45,54,39,24,27] | $Z_{10,10,9,8,7,7,7,7,7,2,2,2}$ [48] |
| | [1,2,0,0,0,5,1,0,0,0] | [3,7,13,19,25,31,42,54,39,24,27] | $Z_{10,10,10,9,8,8,4,4,4,4,4,3}$ [40] |
| | [1,2,1,3,0,1,1,0,1,1] | [2,5,10,16,25,34,44,55,39,24,27] | $Z_{10,10,9,8,8,7,6,6,6,4,3,1}$ [288] |
| | [1,2,2,0,3,0,1,0,1,1] | [2,5,10,17,24,34,44,55,39,24,27] | $Z_{10,10,9,8,8,7,7,5,5,5,3,1}$ [216] |
| | [1,2,2,1,0,3,0,0,1,1] | [2,5,10,17,25,33,44,55,39,24,27] | $Z_{10,10,9,8,8,7,7,6,4,4,4,1}$ [192] |
| | [1,2,2,1,1,0,2,1,0,0] | [2,5,10,17,25,34,43,54,39,24,27] | $Z_{10,10,9,8,8,7,7,6,5,3,3,2}$ [192] |
| | [1,3,0,1,2,2,0,0,1,1] | [2,5,11,17,24,33,44,55,39,24,27] | $Z_{10,10,9,8,8,8,6,5,5,4,4,1}$ [192] |
| | [1,3,0,1,3,0,0,2,0,0] | [2,5,11,17,24,34,44,54,39,24,27] | $Z_{10,10,9,8,8,8,6,5,5,5,2,2}$ [96] |
| | [1,3,0,2,0,2,1,1,0,0] | [2,5,11,17,25,33,43,54,39,24,27] | $Z_{10,10,9,8,8,8,6,6,4,4,3,2}$ [144] |
| | [1,5,2,0,0,0,1,0,2,2] | [1,3,10,19,28,37,46,56,39,24,27] | $Z_{10,9,8,8,8,8,8,7,7,3,1,1}$ [120] |
| | [1,6,0,0,1,1,0,0,2,2] | [1,3,11,19,27,36,46,56,39,24,27] | $Z_{10,9,8,8,8,8,8,8,5,4,1,1}$ [128] |
| | [1,6,0,1,0,0,0,2,1,1] | [1,3,11,19,28,37,46,55,39,24,27] | $Z_{10,9,8,8,8,8,8,8,6,2,2,1}$ [120] |
| | [2,0,0,1,1,4,1,0,0,0] | [3,8,13,18,24,31,42,54,39,24,27] | $Z_{10,10,10,9,9,6,5,4,4,4,4,3}$ [64] |
| | [2,0,2,2,2,0,1,0,1,1] | [2,6,10,16,24,34,44,55,39,24,27] | $Z_{10,10,9,9,7,7,6,6,5,5,3,1}$ [216] |
| | [2,0,2,3,0,1,0,2,0,0] | [2,6,10,16,25,34,44,54,39,24,27] | $Z_{10,10,9,9,7,7,6,6,6,4,2,2}$ [108] |
| | [2,0,3,0,2,2,0,0,1,1] | [2,6,10,17,24,33,44,55,39,24,27] | $Z_{10,10,9,9,7,7,7,5,5,4,4,1}$ [144] |
| | [2,0,3,0,3,0,0,2,0,0] | [2,6,10,17,24,34,44,54,39,24,27] | $Z_{10,10,9,9,7,7,7,5,5,5,2,2}$ [72] |
| | [2,0,3,1,0,2,1,1,0,0] | [2,6,10,17,25,33,43,54,39,24,27] | $Z_{10,10,9,9,7,7,7,6,4,4,3,2}$ [144] |
| | [2,1,0,3,1,2,0,0,1,1] | [2,6,11,16,24,33,44,55,39,24,27] | $Z_{10,10,9,9,8,6,6,6,5,4,4,1}$ [192] |
| | [2,1,0,3,2,0,0,2,0,0] | [2,6,11,16,24,34,44,54,39,24,27] | $Z_{10,10,9,9,8,6,6,6,5,5,2,2}$ [96] |
| | [2,1,0,4,0,0,2,1,0,0] | [2,6,11,16,25,34,43,54,39,24,27] | $Z_{10,10,9,9,8,6,6,6,6,3,3,2}$ [96] |
| | [2,1,1,2,0,1,3,0,0,0] | [2,6,11,17,25,33,42,54,39,24,27] | $Z_{10,10,9,9,8,7,6,6,4,3,3,3}$ [96] |
| | [2,1,2,0,0,4,0,1,0,0] | [2,6,11,18,25,32,43,54,39,24,27] | $Z_{10,10,9,9,8,7,7,4,4,4,4,2}$ [96] |
| | [2,2,0,0,2,3,0,1,0,0] | [2,6,12,18,24,32,43,54,39,24,27] | $Z_{10,10,9,9,8,8,5,5,4,4,4,2}$ [96] |
| | [2,2,0,0,3,0,3,0,0,0] | [2,6,12,18,24,33,42,54,39,24,27] | $Z_{10,10,9,9,8,8,5,5,5,3,3,3}$ [48] |
| | [2,2,0,1,0,3,2,0,0,0] | [2,6,12,18,25,32,42,54,39,24,27] | $Z_{10,10,9,9,8,8,6,4,4,4,3,3}$ [72] |
| | [2,2,4,0,0,1,0,0,2,2] | [1,4,9,18,27,36,46,56,39,24,27] | $Z_{10,9,9,8,8,7,7,7,7,4,1,1}$ [128] |
| | [2,3,1,2,0,1,0,1,1,1] | [1,4,10,17,26,35,45,55,39,24,27] | $Z_{10,9,9,8,8,8,7,6,6,4,2,1}$ [288] |
| | [2,3,2,0,1,0,2,0,1,1] | [1,4,10,18,26,35,44,55,39,24,27] | $Z_{10,9,9,8,8,8,7,7,5,3,3,1}$ [216] |
| | [2,3,2,1,0,0,0,3,0,0] | [1,4,10,18,27,36,45,54,39,24,27] | $Z_{10,9,9,8,8,8,7,7,6,2,2,2}$ [80] |
| | [2,4,0,0,3,0,0,1,1,1] | [1,4,11,18,25,35,45,55,39,24,27] | $Z_{10,9,9,8,8,8,8,5,5,5,2,1}$ [128] |
| | [2,4,0,1,0,2,1,0,1,1] | [1,4,11,18,26,34,44,55,39,24,27] | $Z_{10,9,9,8,8,8,8,6,4,4,3,1}$ [216] |
| | [2,4,0,1,1,0,1,2,0,0] | [1,4,11,18,26,35,44,54,39,24,27] | $Z_{10,9,9,8,8,8,8,6,5,3,2,2}$ [144] |
| | [3,0,0,2,1,3,0,1,0,0] | [2,7,12,17,24,32,43,54,39,24,27] | $Z_{10,10,9,9,9,6,6,5,4,4,4,2}$ [96] |
| | [3,0,0,2,2,0,3,0,0,0] | [2,7,12,17,24,33,42,54,39,24,27] | $Z_{10,10,9,9,9,6,6,5,5,3,3,3}$ [48] |
| | [3,0,1,0,2,2,2,0,0,0] | [2,7,12,18,24,32,42,54,39,24,27] | $Z_{10,10,9,9,9,7,5,5,4,4,3,3}$ [72] |
| | [3,0,4,1,1,0,0,0,2,2] | [1,5,9,17,26,36,46,56,39,24,27] | $Z_{10,9,9,9,7,7,7,7,6,5,1,1}$ [120] |
| | [3,0,5,0,0,0,1,1,1,1] | [1,5,9,18,27,36,45,55,39,24,27] | $Z_{10,9,9,9,7,7,7,7,7,3,2,1}$ [120] |
| | [3,1,1,4,0,0,0,0,2,2] | [1,5,10,16,26,36,46,56,39,24,27] | $Z_{10,9,9,9,8,7,6,6,6,6,1,1}$ [96] |
| | [3,1,2,1,1,1,1,0,1,1] | [1,5,10,17,25,34,44,55,39,24,27] | $Z_{10,9,9,9,8,7,7,6,5,4,3,1}$ [384] |
| | [3,1,2,2,0,0,1,2,0,0] | [1,5,10,17,26,35,44,54,39,24,27] | $Z_{10,9,9,9,8,7,7,6,6,3,2,2}$ [128] |
| | [3,1,3,0,0,2,0,2,0,0] | [1,5,10,18,26,34,44,54,39,24,27] | $Z_{10,9,9,9,8,7,7,7,4,4,2,2}$ [96] |
| | [3,2,0,2,1,1,0,2,0,0] | [1,5,11,17,25,34,44,54,39,24,27] | $Z_{10,9,9,9,8,8,6,6,5,4,2,2}$ [144] |
| | [3,2,1,0,1,3,0,0,1,1] | [1,5,11,18,25,33,44,55,39,24,27] | $Z_{10,9,9,9,8,8,7,5,4,4,4,1}$ [192] |

| | | | |
|---|---|---|---|
| | [3,2,1,0,2,0,2,1,0,0] | [1,5,11,18,25,34,43,54,39,24,27] | $Z_{10,9,9,9,8,8,7,5,5,3,3,2}$ [144] |
| | [3,3,0,0,0,3,1,1,0,0] | [1,5,12,19,26,33,43,54,39,24,27] | $Z_{10,9,9,9,8,8,8,4,4,4,3,2}$ [80] |
| | [3,5,1,0,0,0,0,1,2,2] | [0,3,11,20,29,38,47,56,39,24,27] | $Z_{9,9,9,8,8,8,8,8,7,2,1,1}$ [96] |
| | [4,0,0,4,1,0,0,1,1,1] | [1,6,11,16,25,35,45,55,39,24,27] | $Z_{10,9,9,9,9,6,6,6,6,5,2,1}$ [128] |
| | [4,0,1,1,3,0,1,0,1,1] | [1,6,11,17,24,34,44,55,39,24,27] | $Z_{10,9,9,9,9,7,6,5,5,5,3,1}$ [216] |
| | [4,0,1,2,0,3,0,0,1,1] | [1,6,11,17,25,33,44,55,39,24,27] | $Z_{10,9,9,9,9,7,6,6,4,4,4,1}$ [144] |
| | [4,0,1,2,1,0,2,1,0,0] | [1,6,11,17,25,34,43,54,39,24,27] | $Z_{10,9,9,9,9,7,6,6,5,3,3,2}$ [144] |
| | [4,0,2,0,1,2,1,1,0,0] | [1,6,11,18,25,33,43,54,39,24,27] | $Z_{10,9,9,9,9,7,7,5,4,4,3,2}$ [144] |
| | [4,1,0,0,3,2,0,0,1,1] | [1,6,12,18,24,33,44,55,39,24,27] | $Z_{10,9,9,9,9,8,5,5,5,4,4,1}$ [128] |
| | [4,1,0,0,4,0,0,2,0,0] | [1,6,12,18,24,34,44,54,39,24,27] | $Z_{10,9,9,9,9,8,5,5,5,5,2,2}$ [64] |
| | [4,1,0,2,0,0,4,0,0,0] | [1,6,12,18,26,34,42,54,39,24,27] | $Z_{10,9,9,9,9,8,6,6,3,3,3,3}$ [48] |
| | [4,1,1,0,0,2,3,0,0,0] | [1,6,12,19,26,33,42,54,39,24,27] | $Z_{10,9,9,9,9,8,7,4,4,3,3,3}$ [64] |
| | [4,2,2,1,0,1,0,0,2,2] | [0,4,10,18,27,36,46,56,39,24,27] | $Z_{9,9,9,9,8,8,7,7,6,4,1,1}$ [192] |
| | [4,2,3,0,0,0,0,2,1,1] | [0,4,10,19,28,37,46,55,39,24,27] | $Z_{9,9,9,9,8,8,7,7,7,2,2,1}$ [96] |
| | [4,3,0,1,2,0,0,0,2,2] | [0,4,11,18,26,36,46,56,39,24,27] | $Z_{9,9,9,9,8,8,8,6,5,5,1,1}$ [120] |
| | [4,3,0,2,0,0,1,1,1,1] | [0,4,11,18,27,36,45,55,39,24,27] | $Z_{9,9,9,9,8,8,8,6,6,3,2,1}$ [192] |
| | [4,3,1,0,0,2,0,1,1,1] | [0,4,11,19,27,35,45,55,39,24,27] | $Z_{9,9,9,9,8,8,8,7,4,4,2,1}$ [192] |
| | [4,4,0,0,0,0,3,0,1,1] | [0,4,12,20,28,36,44,55,39,24,27] | $Z_{9,9,9,9,8,8,8,8,3,3,3,1}$ [72] |
| | [4,4,0,0,0,1,0,3,0,0] | [0,4,12,20,28,36,45,54,39,24,27] | $Z_{9,9,9,9,8,8,8,8,4,2,2,2}$ [60] |
| | [5,0,0,0,2,1,3,0,0,0] | [1,7,13,19,25,33,42,54,39,24,27] | $Z_{10,9,9,9,9,9,5,5,4,3,3,3}$ [40] |
| | [5,0,3,0,2,0,0,0,2,2] | [0,5,10,18,26,36,46,56,39,24,27] | $Z_{9,9,9,9,9,7,7,7,5,5,1,1}$ [90] |
| | [5,0,3,1,0,0,1,1,1,1] | [0,5,10,18,27,36,45,55,39,24,27] | $Z_{9,9,9,9,9,7,7,7,6,3,2,1}$ [192] |
| | [5,1,0,3,1,0,0,0,2,2] | [0,5,11,17,26,36,46,56,39,24,27] | $Z_{9,9,9,9,9,8,6,6,6,5,1,1}$ [120] |
| | [5,1,1,1,1,0,2,0,1,1] | [0,5,11,18,26,35,44,55,39,24,27] | $Z_{9,9,9,9,9,8,7,6,5,3,3,1}$ [288] |
| | [5,1,1,2,0,0,0,3,0,0] | [0,5,11,18,27,36,45,54,39,24,27] | $Z_{9,9,9,9,9,8,7,6,6,2,2,2}$ [80] |
| | [5,1,2,0,0,1,1,2,0,0] | [0,5,11,19,27,35,44,54,39,24,27] | $Z_{9,9,9,9,9,8,7,7,4,3,2,2}$ [128] |
| | [5,2,0,0,1,2,1,0,1,1] | [0,5,12,19,26,34,44,55,39,24,27] | $Z_{9,9,9,9,9,8,8,5,4,4,3,1}$ [192] |
| | [5,2,0,0,2,0,1,2,0,0] | [0,5,12,19,26,35,44,54,39,24,27] | $Z_{9,9,9,9,9,8,8,5,5,3,2,2}$ [96] |
| | [6,0,0,1,3,0,0,1,1,1] | [0,6,12,18,25,35,45,55,39,24,27] | $Z_{9,9,9,9,9,9,6,5,5,5,2,1}$ [128] |
| | [6,0,0,2,0,2,1,0,1,1] | [0,6,12,18,26,34,44,55,39,24,27] | $Z_{9,9,9,9,9,9,6,6,4,4,3,1}$ [144] |
| | [6,0,0,2,1,0,1,2,0,0] | [0,6,12,18,26,35,44,54,39,24,27] | $Z_{9,9,9,9,9,9,6,6,5,3,2,2}$ [96] |
| | [6,0,1,0,1,2,0,2,0,0] | [0,6,12,19,26,34,44,54,39,24,27] | $Z_{9,9,9,9,9,9,7,5,4,4,2,2}$ [108] |
| | [6,0,1,1,0,0,3,1,0,0] | [0,6,12,19,27,35,43,54,39,24,27] | $Z_{9,9,9,9,9,9,7,6,3,3,3,2}$ [96] |
| | [6,1,0,0,0,2,2,1,0,0] | [0,6,13,20,27,34,43,54,39,24,27] | $Z_{9,9,9,9,9,9,8,4,4,3,3,2}$ [80] |
| | [0,0,3,4,0,1,0,0,1,1] | [3,6,9,15,25,35,46,57,40,24,28] | $Z_{10,10,10,7,7,7,6,6,6,6,4,1}$ [96] |
| | [0,0,4,1,2,1,0,1,0,0] | [3,6,9,16,24,34,45,56,40,24,28] | $Z_{10,10,10,7,7,7,7,6,5,5,4,2}$ [96] |
| | [0,0,4,2,0,1,2,0,0,0] | [3,6,9,16,25,34,44,56,40,24,28] | $Z_{10,10,10,7,7,7,7,6,6,4,3,3}$ [48] |
| | [0,1,1,4,1,1,0,1,0,0] | [3,6,10,15,24,34,45,56,40,24,28] | $Z_{10,10,10,8,7,6,6,6,6,5,4,2}$ [144] |
| | [0,2,5,1,0,0,0,1,1,1] | [2,4,8,17,27,37,47,57,40,24,28] | $Z_{10,10,8,8,7,7,7,7,7,6,2,1}$ [120] |
| | [0,3,2,2,1,1,0,0,1,1] | [2,4,9,16,25,35,46,57,40,24,28] | $Z_{10,10,8,8,8,7,7,6,6,5,4,1}$ [192] |
| | [0,3,2,3,0,0,0,2,0,0] | [2,4,9,16,26,36,46,56,40,24,28] | $Z_{10,10,8,8,8,7,7,6,6,6,2,2}$ [60] |
| | [0,3,3,0,2,0,1,1,0,0] | [2,4,9,17,25,35,45,56,40,24,28] | $Z_{10,10,8,8,8,7,7,7,5,5,3,2}$ [108] |
| | [0,4,0,3,1,0,1,1,0,0] | [2,4,10,16,25,35,45,56,40,24,28] | $Z_{10,10,8,8,8,8,6,6,6,5,3,2}$ [108] |
| | [0,4,1,0,4,0,0,0,1,1] | [2,4,10,17,24,35,46,57,40,24,28] | $Z_{10,10,8,8,8,8,7,5,5,5,5,1}$ [90] |
| | [0,4,1,1,1,1,2,0,0,0] | [2,4,10,17,25,34,44,56,40,24,28] | $Z_{10,10,8,8,8,8,7,6,5,4,3,3}$ [96] |
| | [0,8,0,0,0,1,0,0,2,2] | [1,2,11,20,29,38,48,58,40,24,28] | $Z_{10,8,8,8,8,8,8,8,8,4,1,1}$ [60] |
| | [1,0,0,5,1,0,2,0,0,0] | [3,7,11,15,24,34,44,56,40,24,28] | $Z_{10,10,10,9,6,6,6,6,6,5,3,3}$ [48] |
| | [1,0,1,3,0,4,0,0,0,0] | [3,7,11,16,24,32,44,56,40,24,28] | $Z_{10,10,10,9,7,6,6,6,4,4,4,4}$ [36] |
| | [1,0,6,0,1,0,1,0,1,1] | [2,5,8,17,26,36,46,57,40,24,28] | $Z_{10,10,9,7,7,7,7,7,7,5,3,1}$ [162] |
| | [1,1,3,1,3,0,0,0,1,1] | [2,5,9,16,24,35,46,57,40,24,28] | $Z_{10,10,9,8,7,7,7,6,5,5,5,1}$ [160] |
| | [1,1,3,2,0,2,0,1,0,0] | [2,5,9,16,25,34,45,56,40,24,28] | $Z_{10,10,9,8,7,7,7,6,6,4,4,2}$ [144] |
| | [1,1,4,0,1,1,2,0,0,0] | [2,5,9,17,25,34,44,56,40,24,28] | $Z_{10,10,9,8,7,7,7,7,5,4,3,3}$ [96] |
| | [1,2,0,5,0,1,0,0,1,1] | [2,5,10,15,25,35,46,57,40,24,28] | $Z_{10,10,9,8,8,6,6,6,6,6,4,1}$ [144] |
| | [1,2,1,2,2,0,2,0,0,0] | [2,5,10,16,24,34,44,56,40,24,28] | $Z_{10,10,9,8,8,7,6,6,5,5,3,3}$ [96] |
| | [1,2,2,0,2,2,1,0,0,0] | [2,5,10,17,24,33,44,56,40,24,28] | $Z_{10,10,9,8,8,7,7,5,5,4,4,3}$ [96] |
| | [1,4,2,2,0,0,0,1,1,1] | [1,3,9,17,27,37,47,57,40,24,28] | $Z_{10,9,8,8,8,8,7,7,6,6,2,1}$ [160] |
| | [1,4,3,0,0,1,1,0,1,1] | [1,3,9,18,27,36,46,57,40,24,28] | $Z_{10,9,8,8,8,8,7,7,7,4,3,1}$ [192] |
| | [1,5,0,2,1,0,1,0,1,1] | [1,3,10,17,26,36,46,57,40,24,28] | $Z_{10,9,8,8,8,8,8,6,6,5,3,1}$ [216] |
| | [1,5,1,0,1,2,0,0,1,1] | [1,3,10,18,26,35,46,57,40,24,28] | $Z_{10,9,8,8,8,8,8,7,5,4,4,1}$ [192] |
| | [1,5,1,0,2,0,0,2,0,0] | [1,3,10,18,26,36,46,56,40,24,28] | $Z_{10,9,8,8,8,8,8,7,5,5,2,2}$ [96] |
| | [1,5,1,1,0,0,2,1,0,0] | [1,3,10,18,27,36,45,56,40,24,28] | $Z_{10,9,8,8,8,8,8,7,6,3,3,2}$ [128] |
| | [1,6,0,0,0,2,1,1,0,0] | [1,3,11,19,27,35,45,56,40,24,28] | $Z_{10,9,8,8,8,8,8,8,4,4,3,2}$ [80] |
| | [2,0,1,4,2,0,0,0,1,1] | [2,6,10,15,24,35,46,57,40,24,28] | $Z_{10,10,9,9,7,6,6,6,6,5,5,1}$ [120] |
| | [2,0,1,5,0,0,1,1,0,0] | [2,6,10,15,25,35,45,56,40,24,28] | $Z_{10,10,9,9,7,6,6,6,6,6,3,2}$ [96] |
| | [2,0,2,2,1,2,1,0,0,0] | [2,6,10,16,24,33,44,56,40,24,28] | $Z_{10,10,9,9,7,7,6,6,5,4,4,3}$ [96] |
| | [2,1,1,1,1,4,0,0,0,0] | [2,6,11,17,24,32,44,56,40,24,28] | $Z_{10,10,9,9,8,7,6,5,4,4,4,4}$ [64] |
| | [2,1,6,0,0,0,0,0,2,2] | [1,4,8,18,28,38,48,58,40,24,28] | $Z_{10,9,9,8,7,7,7,7,7,7,1,1}$ [56] |
| | [2,2,2,3,0,0,1,0,1,1] | [1,4,9,16,26,36,46,57,40,24,28] | $Z_{10,9,9,8,8,7,7,6,6,6,3,1}$ [192] |
| | [2,2,3,0,2,1,0,0,1,1] | [1,4,9,17,25,35,46,57,40,24,28] | $Z_{10,9,9,8,8,7,7,7,5,5,4,1}$ [192] |
| | [2,2,3,1,0,1,1,1,0,0] | [1,4,9,17,26,35,45,56,40,24,28] | $Z_{10,9,9,8,8,7,7,7,6,4,3,2}$ [192] |
| | [2,3,0,3,1,1,0,0,1,1] | [1,4,10,16,25,35,46,57,40,24,28] | $Z_{10,9,9,8,8,8,6,6,6,5,4,1}$ [192] |

| | | | |
|---|---|---|---|
| | [2,3,0,4,0,0,0,2,0,0] | [1,4,10,16,26,36,46,56,40,24,28] | $Z_{10,9,9,8,8,8,6,6,6,6,2,2}$ [60] |
| | [2,3,1,1,1,2,0,1,0,0] | [1,4,10,17,25,34,45,56,40,24,28] | $Z_{10,9,9,8,8,8,7,6,5,4,4,2}$ [192] |
| | [2,3,1,2,0,0,3,0,0,0] | [1,4,10,17,26,35,44,56,40,24,28] | $Z_{10,9,9,8,8,8,7,6,6,3,3,3}$ [64] |
| | [2,3,2,0,0,2,2,0,0,0] | [1,4,10,18,26,34,44,56,40,24,28] | $Z_{10,9,9,8,8,8,7,7,4,4,3,3}$ [64] |
| | [2,4,0,0,2,1,2,0,0,0] | [1,4,11,18,25,34,44,56,40,24,28] | $Z_{10,9,9,8,8,8,8,5,5,4,3,3}$ [64] |
| | [3,0,3,2,1,1,0,0,1,1] | [1,5,9,16,25,35,46,57,40,24,28] | $Z_{10,9,9,9,7,7,7,6,6,5,4,1}$ [192] |
| | [3,0,3,3,0,0,0,2,0,0] | [1,5,9,16,26,36,46,56,40,24,28] | $Z_{10,9,9,9,7,7,7,6,6,6,2,2}$ [60] |
| | [3,0,4,0,2,0,1,1,0,0] | [1,5,9,17,25,35,45,56,40,24,28] | $Z_{10,9,9,9,7,7,7,7,5,5,3,2}$ [108] |
| | [3,1,1,2,3,0,0,0,1,1] | [1,5,10,16,24,35,46,57,40,24,28] | $Z_{10,9,9,9,8,7,6,6,5,5,5,1}$ [160] |
| | [3,1,1,3,0,2,0,1,0,0] | [1,5,10,16,25,34,45,56,40,24,28] | $Z_{10,9,9,9,8,7,6,6,6,4,4,2}$ [144] |
| | [3,1,2,0,3,1,0,1,0,0] | [1,5,10,17,24,34,45,56,40,24,28] | $Z_{10,9,9,9,8,7,7,5,5,5,4,2}$ [144] |
| | [3,2,0,1,3,0,2,0,0,0] | [1,5,11,17,24,34,44,56,40,24,28] | $Z_{10,9,9,9,8,8,6,5,5,5,3,3}$ [72] |
| | [3,2,0,2,0,3,1,0,0,0] | [1,5,11,17,25,33,44,56,40,24,28] | $Z_{10,9,9,9,8,8,6,6,4,4,4,3}$ [72] |
| | [3,3,3,1,0,0,0,0,2,2] | [0,3,9,18,28,38,48,58,40,24,28] | $Z_{9,9,9,8,8,8,7,7,7,6,1,1}$ [96] |
| | [3,4,1,1,0,1,1,0,1,1] | [0,3,10,18,27,36,46,57,40,24,28] | $Z_{9,9,9,8,8,8,8,7,6,4,3,1}$ [288] |
| | [3,4,2,0,0,0,1,2,0,0] | [0,3,10,19,28,37,46,56,40,24,28] | $Z_{9,9,9,8,8,8,8,7,7,3,2,2}$ [80] |
| | [3,5,0,0,1,1,0,2,0,0] | [0,3,11,19,27,36,46,56,40,24,28] | $Z_{9,9,9,8,8,8,8,8,5,4,2,2}$ [96] |
| | [4,0,0,3,2,1,0,1,0,0] | [1,6,11,16,24,34,45,56,40,24,28] | $Z_{10,9,9,9,9,6,6,6,5,5,4,2}$ [96] |
| | [4,0,0,4,0,1,2,0,0,0] | [1,6,11,16,25,34,44,56,40,24,28] | $Z_{10,9,9,9,9,6,6,6,6,4,3,3}$ [48] |
| | [4,0,1,1,2,2,1,0,0,0] | [1,6,11,17,24,33,44,56,40,24,28] | $Z_{10,9,9,9,9,7,6,5,5,4,4,3}$ [96] |
| | [4,1,3,2,0,0,0,1,1,1] | [0,4,9,17,27,37,47,57,40,24,28] | $Z_{9,9,9,9,8,7,7,7,6,6,2,1}$ [160] |
| | [4,1,4,0,0,1,1,0,1,1] | [0,4,9,18,27,36,46,57,40,24,28] | $Z_{9,9,9,9,8,7,7,7,7,4,3,1}$ [192] |
| | [4,2,1,2,0,2,0,0,1,1] | [0,4,10,17,26,35,46,57,40,24,28] | $Z_{9,9,9,9,8,8,7,6,6,4,4,1}$ [192] |
| | [4,2,1,2,1,0,0,2,0,0] | [0,4,10,17,26,36,46,56,40,24,28] | $Z_{9,9,9,9,8,8,7,6,6,5,2,2}$ [128] |
| | [4,2,2,0,1,1,1,1,0,0] | [0,4,10,18,26,35,45,56,40,24,28] | $Z_{9,9,9,9,8,8,7,7,5,4,3,2}$ [192] |
| | [4,3,0,0,3,1,0,0,1,1] | [0,4,11,18,25,35,46,57,40,24,28] | $Z_{9,9,9,9,8,8,8,5,5,5,4,1}$ [128] |
| | [4,3,1,0,0,1,3,0,0,0] | [0,4,11,19,27,35,44,56,40,24,28] | $Z_{9,9,9,9,8,8,8,7,4,3,3,3}$ [64] |
| | [5,0,0,0,1,5,0,0,0,0] | [1,7,13,19,25,32,44,56,40,24,28] | $Z_{10,9,9,9,9,9,5,4,4,4,4,4}$ [20] |
| | [5,0,2,1,2,1,0,0,1,1] | [0,5,10,17,25,35,46,57,40,24,28] | $Z_{9,9,9,9,9,7,7,6,5,5,4,1}$ [192] |
| | [5,0,2,2,0,1,1,1,0,0] | [0,5,10,17,26,35,45,56,40,24,28] | $Z_{9,9,9,9,9,7,7,6,6,4,3,2}$ [144] |
| | [5,1,0,2,2,0,1,1,0,0] | [0,5,11,17,25,35,45,56,40,24,28] | $Z_{9,9,9,9,9,8,6,6,5,5,3,2}$ [144] |
| | [5,1,1,0,2,2,0,1,0,0] | [0,5,11,18,25,34,45,56,40,24,28] | $Z_{9,9,9,9,9,8,7,5,5,4,4,2}$ [144] |
| | [5,1,1,1,0,2,2,0,0,0] | [0,5,11,18,26,34,44,56,40,24,28] | $Z_{9,9,9,9,9,8,7,6,4,4,3,3}$ [96] |
| | [6,0,0,1,2,1,2,0,0,0] | [0,6,12,18,25,34,44,56,40,24,28] | $Z_{9,9,9,9,9,9,6,5,5,4,3,3}$ [64] |
| | [0,0,3,3,2,0,1,0,0,0] | [3,6,9,15,24,35,46,58,41,24,29] | $Z_{10,10,10,7,7,7,6,6,6,5,5,3}$ [48] |
| | [0,2,4,2,0,1,0,1,0,0] | [2,4,8,16,26,36,47,58,41,24,29] | $Z_{10,10,8,8,7,7,7,7,6,6,4,2}$ [108] |
| | [0,2,5,0,1,0,2,0,0,0] | [2,4,8,17,26,36,46,58,41,24,29] | $Z_{10,10,8,8,7,7,7,7,7,5,3,3}$ [54] |
| | [0,3,1,5,0,0,0,0,1,1] | [2,4,9,15,26,37,48,59,41,24,29] | $Z_{10,10,8,8,8,7,6,6,6,6,6,1}$ [72] |
| | [0,4,0,2,3,0,1,0,0,0] | [2,4,10,16,24,35,46,58,41,24,29] | $Z_{10,10,8,8,8,8,6,6,5,5,5,3}$ [54] |
| | [0,4,0,3,0,3,0,0,0,0] | [2,4,10,16,25,34,46,58,41,24,29] | $Z_{10,10,8,8,8,8,6,6,6,4,4,4}$ [27] |
| | [0,4,1,0,3,2,0,0,0,0] | [2,4,10,17,24,34,46,58,41,24,29] | $Z_{10,10,8,8,8,8,7,5,5,5,4,4}$ [36] |
| | [0,6,2,1,0,0,1,0,1,1] | [1,2,9,18,28,38,48,59,41,24,29] | $Z_{10,8,8,8,8,8,8,7,7,6,3,1}$ [144] |
| | [0,7,0,1,1,1,0,0,1,1] | [1,2,10,18,27,37,48,59,41,24,29] | $Z_{10,8,8,8,8,8,8,8,6,5,4,1}$ [144] |
| | [0,7,0,2,0,0,0,2,0,0] | [1,2,10,18,28,38,48,58,41,24,29] | $Z_{10,8,8,8,8,8,8,8,6,6,2,2}$ [45] |
| | [0,7,1,0,0,1,1,1,0,0] | [1,2,10,19,28,37,47,58,41,24,29] | $Z_{10,8,8,8,8,8,8,8,7,4,3,2}$ [96] |
| | [1,0,5,1,2,0,0,1,0,0] | [2,5,8,16,25,36,47,58,41,24,29] | $Z_{10,10,9,7,7,7,7,7,6,5,5,2}$ [96] |
| | [1,0,5,2,0,0,2,0,0,0] | [2,5,8,16,26,36,46,58,41,24,29] | $Z_{10,10,9,7,7,7,7,7,6,6,3,3}$ [48] |
| | [1,0,6,0,0,2,1,0,0,0] | [2,5,8,17,26,35,46,58,41,24,29] | $Z_{10,10,9,7,7,7,7,7,7,4,4,3}$ [48] |
| | [1,1,2,4,0,1,1,0,0,0] | [2,5,9,15,25,35,46,58,41,24,29] | $Z_{10,10,9,8,7,7,6,6,6,6,4,3}$ [96] |
| | [1,1,3,1,2,2,0,0,0,0] | [2,5,9,16,24,34,46,58,41,24,29] | $Z_{10,10,9,8,7,7,7,6,5,5,4,4}$ [64] |
| | [1,2,0,4,2,0,1,0,0,0] | [2,5,10,15,24,35,46,58,41,24,29] | $Z_{10,10,9,8,8,6,6,6,6,5,5,3}$ [72] |
| | [1,3,4,1,0,1,0,0,1,1] | [1,3,8,17,27,37,48,59,41,24,29] | $Z_{10,9,8,8,8,7,7,7,7,6,4,1}$ [192] |
| | [1,3,5,0,0,0,0,2,0,0] | [1,3,8,18,28,38,48,58,41,24,29] | $Z_{10,9,8,8,8,7,7,7,7,7,2,2}$ [48] |
| | [1,4,1,3,1,0,0,0,1,1] | [1,3,9,16,26,37,48,59,41,24,29] | $Z_{10,9,8,8,8,8,7,6,6,6,5,1}$ [160] |
| | [1,4,2,1,1,0,2,0,0,0] | [1,3,9,17,26,36,46,58,41,24,29] | $Z_{10,9,8,8,8,8,7,7,6,5,3,3}$ [96] |
| | [1,5,0,1,3,0,0,1,0,0] | [1,3,10,17,25,36,47,58,41,24,29] | $Z_{10,9,8,8,8,8,8,6,5,5,5,2}$ [96] |
| | [1,5,0,2,0,2,1,0,0,0] | [1,3,10,17,26,35,46,58,41,24,29] | $Z_{10,9,8,8,8,8,8,6,6,4,4,3}$ [72] |
| | [2,0,1,4,1,2,0,0,0,0] | [2,6,10,15,24,34,46,58,41,24,29] | $Z_{10,10,9,9,7,6,6,6,6,5,4,4}$ [48] |
| | [2,1,4,2,1,0,0,0,1,1] | [1,4,8,16,26,37,48,59,41,24,29] | $Z_{10,9,9,8,7,7,7,7,6,6,5,1}$ [160] |
| | [2,1,5,0,1,1,0,1,0,0] | [1,4,8,17,26,36,47,58,41,24,29] | $Z_{10,9,9,8,7,7,7,7,7,5,4,2}$ [144] |
| | [2,2,2,2,1,1,1,0,0,0] | [1,4,9,16,25,35,46,58,41,24,29] | $Z_{10,9,9,8,8,7,7,6,6,5,4,3}$ [128] |
| | [2,3,1,0,4,0,1,0,0,0] | [1,4,10,17,24,35,46,58,41,24,29] | $Z_{10,9,9,8,8,8,7,5,5,5,5,3}$ [72] |
| | [2,5,3,0,0,0,0,1,1,1] | [0,2,9,19,29,39,49,59,41,24,29] | $Z_{9,9,8,8,8,8,8,7,7,7,2,1}$ [96] |
| | [2,6,0,2,0,0,1,0,1,1] | [0,2,10,18,28,38,48,59,41,24,29] | $Z_{9,9,8,8,8,8,8,8,6,6,3,1}$ [144] |
| | [2,6,1,0,0,2,0,0,1,1] | [0,2,10,19,28,37,48,59,41,24,29] | $Z_{9,9,8,8,8,8,8,8,7,4,4,1}$ [128] |
| | [2,6,1,0,1,0,0,2,0,0] | [0,2,10,19,28,38,48,58,41,24,29] | $Z_{9,9,8,8,8,8,8,8,7,5,2,2}$ [96] |
| | [2,7,0,0,0,0,2,1,0,0] | [0,2,11,20,29,38,47,58,41,24,29] | $Z_{9,9,8,8,8,8,8,8,8,3,3,2}$ [48] |
| | [3,0,2,5,0,0,0,0,1,1] | [1,5,9,15,26,37,48,59,41,24,29] | $Z_{10,9,9,9,7,7,6,6,6,6,6,1}$ [72] |
| | [3,0,4,0,1,3,0,0,0,0] | [1,5,9,17,25,34,46,58,41,24,29] | $Z_{10,9,9,9,7,7,7,7,5,4,4,4}$ [36] |
| | [3,1,0,5,1,0,0,1,0,0] | [1,5,10,15,25,36,47,58,41,24,29] | $Z_{10,9,9,9,8,6,6,6,6,6,5,2}$ [96] |
| | [3,1,1,2,2,2,0,0,0,0] | [1,5,10,16,24,34,46,58,41,24,29] | $Z_{10,9,9,9,8,7,6,6,5,5,4,4}$ [64] |

| | | | |
|---|---|---|---|
| | [3,3,2,1,2,0,0,0,1,1] | [0,3,9,17,26,37,48,59,41,24,29] | $Z_{9,9,9,8,8,8,7,7,6,5,5,1}$ [160] |
| | [3,3,2,2,0,0,1,1,0,0] | [0,3,9,17,27,37,47,58,41,24,29] | $Z_{9,9,9,8,8,8,7,7,6,6,3,2}$ [128] |
| | [3,3,3,0,0,2,0,1,0,0] | [0,3,9,18,27,36,47,58,41,24,29] | $Z_{9,9,9,8,8,8,7,7,7,4,4,2}$ [96] |
| | [3,4,0,2,1,1,0,1,0,0] | [0,3,10,17,26,36,47,58,41,24,29] | $Z_{9,9,9,8,8,8,8,6,6,5,4,2}$ [144] |
| | [3,4,1,0,2,0,2,0,0,0] | [0,3,10,18,26,36,46,58,41,24,29] | $Z_{9,9,9,8,8,8,8,7,5,5,3,3}$ [72] |
| | [3,5,0,0,0,3,1,0,0,0] | [0,3,11,19,27,35,46,58,41,24,29] | $Z_{9,9,9,8,8,8,8,8,4,4,4,3}$ [40] |
| | [4,0,6,0,0,0,1,0,1,1] | [0,4,8,18,28,38,48,59,41,24,29] | $Z_{9,9,9,9,7,7,7,7,7,7,3,1}$ [90] |
| | [4,1,2,3,1,0,0,0,1,1] | [0,4,9,16,26,37,48,59,41,24,29] | $Z_{9,9,9,9,8,7,7,6,6,6,5,1}$ [160] |
| | [4,1,3,1,1,0,2,0,0,0] | [0,4,9,17,26,36,46,58,41,24,29] | $Z_{9,9,9,9,8,7,7,7,6,5,3,3}$ [96] |
| | [4,2,0,4,0,1,0,1,0,0] | [0,4,10,16,26,36,47,58,41,24,29] | $Z_{9,9,9,9,8,8,6,6,6,6,4,2}$ [108] |
| | [4,2,1,1,2,1,1,0,0,0] | [0,4,10,17,25,35,46,58,41,24,29] | $Z_{9,9,9,9,8,8,7,6,5,5,4,3}$ [128] |
| | [4,3,0,1,0,4,0,0,0,0] | [0,4,11,18,26,34,46,58,41,24,29] | $Z_{9,9,9,9,8,8,8,6,4,4,4,4}$ [36] |
| | [5,0,1,3,2,0,0,1,0,0] | [0,5,10,16,25,36,47,58,41,24,29] | $Z_{9,9,9,9,9,7,6,6,6,5,5,2}$ [96] |
| | [5,0,1,4,0,0,2,0,0,0] | [0,5,10,16,26,36,46,58,41,24,29] | $Z_{9,9,9,9,9,7,6,6,6,6,3,3}$ [48] |
| | [5,0,3,0,0,4,0,0,0,0] | [0,5,10,18,26,34,46,58,41,24,29] | $Z_{9,9,9,9,9,7,7,7,4,4,4,4}$ [24] |
| | [5,1,0,2,1,3,0,0,0,0] | [0,5,11,17,25,34,46,58,41,24,29] | $Z_{9,9,9,9,9,8,6,6,5,4,4,4}$ [48] |
| | [6,0,0,0,5,0,1,0,0,0] | [0,6,12,18,24,35,46,58,41,24,29] | $Z_{9,9,9,9,9,9,5,5,5,5,5,3}$ [30] |
| | [0,1,7,1,0,0,0,0,1,1] | [2,4,7,17,28,39,50,61,42,24,30] | $Z_{10,10,8,7,7,7,7,7,7,7,6,1}$ [72] |
| | [0,2,4,1,2,1,0,0,0,0] | [2,4,8,16,25,36,48,60,42,24,30] | $Z_{10,10,8,8,7,7,7,7,6,5,5,4}$ [48] |
| | [0,3,1,4,1,1,0,0,0,0] | [2,4,9,15,25,36,48,60,42,24,30] | $Z_{10,10,8,8,8,7,6,6,6,6,5,4}$ [48] |
| | [0,3,2,1,4,0,0,0,0,0] | [2,4,9,16,24,36,48,60,42,24,30] | $Z_{10,10,8,8,8,7,7,6,5,5,5,5}$ [24] |
| | [0,5,4,0,1,0,0,0,1,1] | [1,2,8,18,28,39,50,61,42,24,30] | $Z_{10,8,8,8,8,8,7,7,7,7,5,1}$ [90] |
| | [0,6,1,2,1,0,0,1,0,0] | [1,2,9,17,27,38,49,60,42,24,30] | $Z_{10,8,8,8,8,8,8,7,6,6,5,2}$ [96] |
| | [0,6,2,0,1,1,1,0,0,0] | [1,2,9,18,27,37,48,60,42,24,30] | $Z_{10,8,8,8,8,8,8,7,7,5,4,3}$ [72] |
| | [1,1,2,3,3,0,0,0,0,0] | [2,5,9,15,24,36,48,60,42,24,30] | $Z_{10,10,9,8,7,7,6,6,6,5,5,5}$ [32] |
| | [1,3,3,3,0,0,0,1,0,0] | [1,3,8,16,27,38,49,60,42,24,30] | $Z_{10,9,8,8,8,7,7,7,6,6,6,2}$ [80] |
| | [1,3,4,0,2,0,1,0,0,0] | [1,3,8,17,26,37,48,60,42,24,30] | $Z_{10,9,8,8,8,7,7,7,7,5,5,3}$ [72] |
| | [1,4,1,3,0,2,0,0,0,0] | [1,3,9,16,26,36,48,60,42,24,30] | $Z_{10,9,8,8,8,8,7,6,6,6,4,4}$ [48] |
| | [1,4,2,0,3,1,0,0,0,0] | [1,3,9,17,25,36,48,60,42,24,30] | $Z_{10,9,8,8,8,8,7,7,5,5,5,4}$ [48] |
| | [1,9,0,0,0,0,0,1,1,1] | [0,1,11,21,31,41,51,61,42,24,30] | $Z_{9,8,8,8,8,8,8,8,8,8,2,1}$ [56] |
| | [2,1,4,2,0,2,0,0,0,0] | [1,4,8,16,26,36,48,60,42,24,30] | $Z_{10,9,9,8,7,7,7,7,6,6,4,4}$ [48] |
| | [2,2,1,5,0,0,1,0,0,0] | [1,4,9,15,26,37,48,60,42,24,30] | $Z_{10,9,9,8,8,7,6,6,6,6,6,3}$ [64] |
| | [2,3,0,2,4,0,0,0,0,0] | [1,4,10,16,24,36,48,60,42,24,30] | $Z_{10,9,9,8,8,8,6,6,5,5,5,5}$ [24] |
| | [2,5,1,3,0,0,0,0,1,1] | [0,2,9,17,28,39,50,61,42,24,30] | $Z_{9,9,8,8,8,8,8,7,6,6,6,1}$ [96] |
| | [2,5,2,0,2,0,0,1,0,0] | [0,2,9,18,27,38,49,60,42,24,30] | $Z_{9,9,8,8,8,8,8,7,7,5,5,2}$ [96] |
| | [2,5,2,1,0,0,2,0,0,0] | [0,2,9,18,28,38,48,60,42,24,30] | $Z_{9,9,8,8,8,8,8,7,7,6,3,3}$ [64] |
| | [2,6,0,1,1,1,1,0,0,0] | [0,2,10,18,27,37,48,60,42,24,30] | $Z_{9,9,8,8,8,8,8,8,6,5,4,3}$ [96] |
| | [3,0,2,4,1,1,0,0,0,0] | [1,5,9,15,25,36,48,60,42,24,30] | $Z_{10,9,9,9,7,7,6,6,6,6,5,4}$ [48] |
| | [3,0,3,1,4,0,0,0,0,0] | [1,5,9,16,24,36,48,60,42,24,30] | $Z_{10,9,9,9,7,7,7,6,5,5,5,5}$ [24] |
| | [3,2,4,1,1,0,0,1,0,0] | [0,3,8,17,27,38,49,60,42,24,30] | $Z_{9,9,9,8,8,7,7,7,7,6,5,2}$ [128] |
| | [3,2,5,0,0,0,2,0,0,0] | [0,3,8,18,28,38,48,60,42,24,30] | $Z_{9,9,9,8,8,7,7,7,7,7,3,3}$ [40] |
| | [3,3,1,4,0,0,0,1,0,0] | [0,3,9,16,27,38,49,60,42,24,30] | $Z_{9,9,9,8,8,8,7,6,6,6,6,2}$ [80] |
| | [3,3,2,1,1,2,0,0,0,0] | [0,3,9,17,26,36,48,60,42,24,30] | $Z_{9,9,9,8,8,8,7,7,6,5,4,4}$ [64] |
| | [4,0,5,1,0,1,1,0,0,0] | [0,4,8,17,27,37,48,60,42,24,30] | $Z_{9,9,9,9,7,7,7,7,7,6,4,3}$ [72] |
| | [4,1,2,3,0,2,0,0,0,0] | [0,4,9,16,26,36,48,60,42,24,30] | $Z_{9,9,9,9,8,7,7,6,6,6,4,4}$ [48] |
| | [4,1,3,0,3,1,0,0,0,0] | [0,4,9,17,25,36,48,60,42,24,30] | $Z_{9,9,9,9,8,7,7,7,5,5,5,4}$ [48] |
| | [4,2,0,3,2,1,0,0,0,0] | [0,4,10,16,25,36,48,60,42,24,30] | $Z_{9,9,9,9,8,8,6,6,6,5,5,4}$ [48] |
| | [5,1,0,1,5,0,0,0,0,0] | [0,5,11,17,24,36,48,60,42,24,30] | $Z_{9,9,9,9,9,8,6,5,5,5,5,5}$ [24] |
| | [0,1,0,8,0,0,0,0,0,0] | [3,6,10,14,26,38,50,62,43,24,31] | $Z_{10,10,10,8,6,6,6,6,6,6,6,6}$ [9] |
| | [0,1,7,0,1,1,0,0,0,0] | [2,4,7,17,27,38,50,62,43,24,31] | $Z_{10,10,8,7,7,7,7,7,7,7,5,4}$ [36] |
| | [0,5,3,2,0,0,1,0,0,0] | [1,2,8,17,28,39,50,62,43,24,31] | $Z_{10,8,8,8,8,8,7,7,7,6,6,3}$ [48] |
| | [0,5,4,0,0,2,0,0,0,0] | [1,2,8,18,28,38,50,62,43,24,31] | $Z_{10,8,8,8,8,8,7,7,7,7,4,4}$ [24] |
| | [0,7,0,0,4,0,0,0,0,0] | [1,2,10,18,26,38,50,62,43,24,31] | $Z_{10,8,8,8,8,8,8,8,5,5,5,5}$ [12] |
| | [1,2,7,0,0,0,0,1,0,0] | [1,3,7,18,29,40,51,62,43,24,31] | $Z_{10,9,8,8,7,7,7,7,7,7,7,2}$ [48] |
| | [1,3,3,2,2,0,0,0,0,0] | [1,3,8,16,26,38,50,62,43,24,31] | $Z_{10,9,8,8,8,7,7,7,6,6,5,5}$ [32] |
| | [1,7,2,1,0,0,0,0,1,1] | [0,1,9,19,30,41,52,63,43,24,31] | $Z_{9,8,8,8,8,8,8,8,7,7,6,1}$ [96] |
| | [1,8,0,1,1,0,0,1,0,0] | [0,1,10,19,29,40,51,62,43,24,31] | $Z_{9,8,8,8,8,8,8,8,8,6,5,2}$ [96] |
| | [1,8,1,0,0,0,2,0,0,0] | [0,1,10,20,30,40,50,62,43,24,31] | $Z_{9,8,8,8,8,8,8,8,8,7,3,3}$ [40] |
| | [2,0,7,1,0,0,1,0,0,0] | [1,4,7,17,28,39,50,62,43,24,31] | $Z_{10,9,9,7,7,7,7,7,7,7,6,3}$ [48] |
| | [2,4,4,0,1,0,1,0,0,0] | [0,2,8,18,28,39,50,62,43,24,31] | $Z_{9,9,8,8,8,8,7,7,7,7,5,3}$ [72] |
| | [2,5,1,2,1,1,0,0,0,0] | [0,2,9,17,27,38,50,62,43,24,31] | $Z_{9,9,8,8,8,8,8,7,6,6,5,4}$ [64] |
| | [3,3,1,3,2,0,0,0,0,0] | [0,3,9,16,26,38,50,62,43,24,31] | $Z_{9,9,9,8,8,8,7,6,6,6,5,5}$ [32] |
| | [4,0,4,3,0,1,0,0,0,0] | [0,4,8,16,27,38,50,62,43,24,31] | $Z_{9,9,9,9,7,7,7,7,6,6,6,4}$ [36] |
| | [4,0,5,0,3,0,0,0,0,0] | [0,4,8,17,26,38,50,62,43,24,31] | $Z_{9,9,9,9,7,7,7,7,7,5,5,5}$ [18] |
| | [1,2,6,1,1,0,0,0,0,0] | [1,3,7,17,28,40,52,64,44,24,32] | $Z_{10,9,8,8,7,7,7,7,7,7,6,5}$ [32] |
| | [1,7,2,0,1,1,0,0,0,0] | [0,1,9,19,29,40,52,64,44,24,32] | $Z_{9,8,8,8,8,8,8,8,7,7,5,4}$ [48] |
| | [2,4,3,2,1,0,0,0,0,0] | [0,2,8,17,28,40,52,64,44,24,32] | $Z_{9,9,8,8,8,8,7,7,7,6,6,5}$ [32] |
| | [3,2,3,4,0,0,0,0,0,0] | [0,3,8,16,28,40,52,64,44,24,32] | $Z_{9,9,9,8,8,7,7,7,6,6,6,6}$ [16] |
| | [1,7,1,3,0,0,0,0,0,0] | [0,1,9,18,30,42,54,66,45,24,33] | $Z_{9,8,8,8,8,8,8,8,7,6,6,6}$ [16] |
| | [3,1,7,1,0,0,0,0,0,0] | [0,3,7,18,30,42,54,66,45,24,33] | $Z_{9,9,9,8,7,7,7,7,7,7,7,6}$ [16] |
| | [1,6,5,0,0,0,0,0,0,0] | [0,1,8,20,32,44,56,68,46,24,34] | $Z_{9,8,8,8,8,8,8,7,7,7,7,7}$ [8] |

| | | | | |
|---|---|---|---|---|
| | [0,11,0,1,0,0,0,0,0,0] | [0,0,11,22,34,46,58,70,47,24,35] | $Z_{8,8,8,8,8,8,8,8,8,8,8,6}$ [9] | |
| | [0,0,0,0,0,0,1,2,5,1] | [6,12,18,24,30,36,42,49,34,24,24] | $Z_{10,10,10,10,10,10,3,2,2,1,1,1,1,1}$ [32] | $Z_{10,10,10,10,10,10,3,2,2,1}$ [32] |
| | [0,1,0,1,0,0,0,1,6,2] | [5,10,16,22,29,36,43,50,34,24,24] | $Z_{10,10,10,10,10,8,6,2,1,1,1,1,1,1}$ [90] | $Z_{10,10,10,10,10,8,6,2,1,1}$ [90] |
| | [1,0,0,0,0,1,1,0,6,2] | [5,11,17,23,29,35,42,50,34,24,24] | $Z_{10,10,10,10,10,9,4,3,1,1,1,1,1,1}$ [72] | $Z_{10,10,10,10,10,9,4,3,1,1}$ [72] |
| | [2,0,1,0,0,0,0,0,7,3] | [4,10,16,23,30,37,44,51,34,24,24] | $Z_{10,10,10,10,9,9,7,1,1,1,1,1,1,1}$ [42] | $Z_{10,10,10,10,9,9,7,1,1,1}$ [42] |
| | [0,0,0,0,0,0,0,5,2,0] | [6,12,18,24,30,36,42,48,35,24,24] | $Z_{10,10,10,10,10,10,2,2,2,2,2,1,1}$ [13] | $Z_{10,10,10,10,10,10,2,2,2,2,2}$ [14] |
| | [0,0,0,1,2,0,0,1,4,2] | [5,10,15,20,26,34,42,50,35,24,24] | $Z_{10,10,10,10,10,6,5,5,2,1,1,1,1}$ [80] | $Z_{10,10,10,10,10,6,5,5,2,1,1}$ [80] |
| | [0,0,0,2,0,0,2,0,4,2] | [5,10,15,20,27,34,41,50,35,24,24] | $Z_{10,10,10,10,10,6,6,3,3,1,1,1,1}$ [60] | $Z_{10,10,10,10,10,6,6,3,3,1,1}$ [60] |
| | [0,0,1,0,0,2,1,0,4,2] | [5,10,15,21,27,33,41,50,35,24,24] | $Z_{10,10,10,10,10,7,4,4,3,1,1,1,1}$ [96] | $Z_{10,10,10,10,10,7,4,4,3,1,1}$ [96] |
| | [0,0,1,0,1,0,1,2,3,1] | [5,10,15,21,27,34,41,49,35,24,24] | $Z_{10,10,10,10,10,7,5,3,2,2,1,1,1}$ [144] | $Z_{10,10,10,10,10,7,5,3,2,2,1}$ [144] |
| | [0,2,0,1,1,0,0,0,5,3] | [4,8,14,20,27,35,43,51,35,24,24] | $Z_{10,10,10,10,8,8,6,5,1,1,1,1,1}$ [90] | $Z_{10,10,10,10,8,8,6,5,1,1,1}$ [90] |
| | [0,2,1,0,0,0,1,1,4,2] | [4,8,14,21,28,35,42,50,35,24,24] | $Z_{10,10,10,10,8,8,7,3,2,1,1,1,1}$ [120] | $Z_{10,10,10,10,8,8,7,3,2,1,1}$ [120] |
| | [1,0,1,1,0,1,0,1,4,2] | [4,9,14,20,27,34,42,50,35,24,24] | $Z_{10,10,10,10,9,7,6,4,2,1,1,1,1}$ [216] | $Z_{10,10,10,10,9,7,6,4,2,1,1}$ [216] |
| | [1,1,0,0,1,0,2,0,4,2] | [4,9,15,21,27,34,41,50,35,24,24] | $Z_{10,10,10,10,9,8,5,3,3,1,1,1,1}$ [144] | $Z_{10,10,10,10,9,8,5,3,3,1,1}$ [144] |
| | [1,1,0,1,0,0,0,3,3,1] | [4,9,15,21,28,35,42,49,35,24,24] | $Z_{10,10,10,10,9,8,6,2,2,2,1,1,1}$ [120] | $Z_{10,10,10,10,9,8,6,2,2,2,1}$ [120] |
| | [2,0,0,0,0,1,1,2,3,1] | [4,10,16,22,28,34,41,49,35,24,24] | $Z_{10,10,10,10,9,9,4,3,2,2,1,1,1}$ [96] | $Z_{10,10,10,10,9,9,4,3,2,2,1}$ [96] |
| | [2,1,1,0,0,1,0,0,5,3] | [3,8,14,21,28,35,43,51,35,24,24] | $Z_{10,10,10,9,9,8,7,4,1,1,1,1,1}$ [128] | $Z_{10,10,10,9,9,8,7,4,1,1,1}$ [128] |
| | [2,2,0,0,0,0,0,2,4,2] | [3,8,15,22,29,36,43,50,35,24,24] | $Z_{10,10,10,9,9,8,8,2,2,1,1,1,1}$ [56] | $Z_{10,10,10,9,9,8,8,2,2,1,1}$ [56] |
| | [3,0,0,0,2,0,0,0,5,3] | [3,9,15,21,27,35,43,51,35,24,24] | $Z_{10,10,10,9,9,9,5,5,1,1,1,1,1}$ [50] | $Z_{10,10,10,9,9,9,5,5,1,1,1}$ [50] |
| | [3,0,0,1,0,0,1,1,4,2] | [3,9,15,21,28,35,42,50,35,24,24] | $Z_{10,10,10,9,9,9,6,3,2,1,1,1,1}$ [128] | $Z_{10,10,10,9,9,9,6,3,2,1,1}$ [128] |
| | [0,0,0,0,2,2,0,2,0,2] | [5,10,15,20,25,32,41,50,37,24,24] | $Z_{10,10,10,10,10,5,5,4,4,2,2}$ [54] | $Z_{10,10,10,10,10,5,5,4,4,2,2,1,1}$ [54] |
| | [0,0,0,1,0,2,2,1,0,2] | [5,10,15,20,26,32,40,50,37,24,24] | $Z_{10,10,10,10,10,6,4,4,3,3,2}$ [90] | $Z_{10,10,10,10,10,6,4,4,3,3,2,1,1}$ [90] |
| | [0,0,2,1,2,0,0,0,2,4] | [4,8,12,18,25,34,43,52,37,24,24] | $Z_{10,10,10,10,7,7,6,5,5,1,1}$ [80] | $Z_{10,10,10,10,7,7,6,5,5,1,1,1,1}$ [80] |
| | [0,0,2,2,0,0,1,1,1,3] | [4,8,12,18,26,34,42,51,37,24,24] | $Z_{10,10,10,10,7,7,6,6,3,2,1}$ [128] | $Z_{10,10,10,10,7,7,6,6,3,2,1,1,1}$ [128] |
| | [0,0,3,0,0,2,0,1,1,3] | [4,8,12,19,26,33,42,51,37,24,24] | $Z_{10,10,10,10,7,7,7,4,4,2,1}$ [96] | $Z_{10,10,10,10,7,7,7,4,4,2,1,1,1}$ [96] |
| | [0,1,0,2,1,1,0,1,1,3] | [4,8,13,18,25,33,42,51,37,24,24] | $Z_{10,10,10,10,8,6,6,5,4,2,1}$ [216] | $Z_{10,10,10,10,8,6,6,5,4,2,1,1,1}$ [216] |
| | [0,1,1,0,2,0,2,0,1,3] | [4,8,13,19,25,33,41,51,37,24,24] | $Z_{10,10,10,10,8,7,5,5,3,3,1}$ [162] | $Z_{10,10,10,10,8,7,5,5,3,3,1,1,1}$ [162] |
| | [0,1,1,1,0,1,1,2,0,2] | [4,8,13,19,26,33,41,50,37,24,24] | $Z_{10,10,10,10,8,7,6,4,3,2,2}$ [216] | $Z_{10,10,10,10,8,7,6,4,3,2,2,1,1}$ [216] |
| | [0,2,0,0,0,3,1,0,1,3] | [4,8,14,20,26,32,41,51,37,24,24] | $Z_{10,10,10,10,8,8,4,4,4,3,1}$ [90] | $Z_{10,10,10,10,8,8,4,4,4,3,1,1,1}$ [90] |
| | [0,3,1,1,0,0,1,0,2,4] | [3,6,12,19,27,35,43,52,37,24,24] | $Z_{10,10,10,8,8,8,7,6,3,1,1}$ [144] | $Z_{10,10,10,8,8,8,7,6,3,1,1,1,1}$ [144] |
| | [0,4,0,0,0,2,0,0,2,4] | [3,6,13,20,27,34,43,52,37,24,24] | $Z_{10,10,10,8,8,8,8,4,4,1,1}$ [60] | $Z_{10,10,10,8,8,8,8,4,4,1,1,1,1}$ [60] |
| | [0,4,0,0,1,0,0,2,1,3] | [3,6,13,20,27,35,43,51,37,24,24] | $Z_{10,10,10,8,8,8,8,5,2,2,1}$ [96] | $Z_{10,10,10,8,8,8,8,5,2,2,1,1,1}$ [96] |
| | [1,0,0,1,1,2,1,0,1,3] | [4,9,14,19,25,32,41,51,37,24,24] | $Z_{10,10,10,10,9,6,5,4,4,3,1}$ [192] | $Z_{10,10,10,10,9,6,5,4,4,3,1,1,1}$ [192] |
| | [1,0,0,1,2,0,1,2,0,2] | [4,9,14,19,25,33,41,50,37,24,24] | $Z_{10,10,10,10,9,6,5,5,3,2,2}$ [144] | $Z_{10,10,10,10,9,6,5,5,3,2,2,1,1}$ [144] |
| | [1,0,1,0,0,3,0,2,0,2] | [4,9,14,20,26,32,41,50,37,24,24] | $Z_{10,10,10,10,9,7,4,4,4,2,2}$ [108] | $Z_{10,10,10,10,9,7,4,4,4,2,2,1,1}$ [108] |
| | [1,0,1,0,1,0,3,1,0,2] | [4,9,14,20,26,33,40,50,37,24,24] | $Z_{10,10,10,10,9,7,5,3,3,3,2}$ [162] | $Z_{10,10,10,10,9,7,5,3,3,3,2,1,1}$ [162] |
| | [1,1,1,2,0,1,0,0,2,4] | [3,7,12,18,26,34,43,52,37,24,24] | $Z_{10,10,10,9,8,7,6,6,4,1,1}$ [192] | $Z_{10,10,10,9,8,7,6,6,4,1,1,1,1}$ [192] |
| | [1,1,2,0,1,0,1,1,1,3] | [3,7,12,19,26,34,42,51,37,24,24] | $Z_{10,10,10,9,8,7,7,5,3,2,1}$ [288] | $Z_{10,10,10,9,8,7,7,5,3,2,1,1,1}$ [288] |
| | [1,2,0,0,3,0,0,0,2,4] | [3,7,13,19,25,34,43,52,37,24,24] | $Z_{10,10,10,9,8,8,5,5,5,1,1}$ [80] | $Z_{10,10,10,9,8,8,5,5,5,1,1,1,1}$ [80] |
| | [1,2,0,1,0,2,0,1,1,3] | [3,7,13,19,26,33,42,51,37,24,24] | $Z_{10,10,10,9,8,8,6,4,4,2,1}$ [216] | $Z_{10,10,10,9,8,8,6,4,4,2,1,1,1}$ [216] |
| | [1,2,1,0,0,0,3,0,1,3] | [3,7,13,20,27,34,41,51,37,24,24] | $Z_{10,10,10,9,8,8,7,3,3,3,1}$ [120] | $Z_{10,10,10,9,8,8,7,3,3,3,1,1,1}$ [120] |
| | [1,2,1,0,0,1,0,3,0,2] | [3,7,13,20,27,34,42,50,37,24,24] | $Z_{10,10,10,9,8,8,7,4,2,2,2}$ [144] | $Z_{10,10,10,9,8,8,7,4,2,2,2,1,1}$ [144] |
| | [2,0,0,2,2,0,0,0,2,4] | [3,8,13,18,25,34,43,52,37,24,24] | $Z_{10,10,10,9,9,6,6,5,5,1,1}$ [80] | $Z_{10,10,10,9,9,6,6,5,5,1,1,1,1}$ [80] |
| | [2,0,0,3,0,0,1,1,1,3] | [3,8,13,18,26,34,42,51,37,24,24] | $Z_{10,10,10,9,9,6,6,6,3,2,1}$ [128] | $Z_{10,10,10,9,9,6,6,6,3,2,1,1,1}$ [128] |
| | [2,0,1,0,2,1,0,1,1,3] | [3,8,13,19,25,33,42,51,37,24,24] | $Z_{10,10,10,9,9,7,5,5,4,2,1}$ [216] | $Z_{10,10,10,9,9,7,5,5,4,2,1,1,1}$ [216] |
| | [2,0,1,1,0,1,2,0,1,3] | [3,8,13,19,26,33,41,51,37,24,24] | $Z_{10,10,10,9,9,7,6,4,3,3,1}$ [216] | $Z_{10,10,10,9,9,7,6,4,3,3,1,1,1}$ [216] |
| | [2,0,1,1,1,0,0,3,0,2] | [3,8,13,19,26,34,42,50,37,24,24] | $Z_{10,10,10,9,9,7,6,5,2,2,2}$ [144] | $Z_{10,10,10,9,9,7,6,5,2,2,2,1,1}$ [144] |
| | [2,0,2,0,0,0,2,2,0,2] | [3,8,13,20,27,34,41,50,37,24,24] | $Z_{10,10,10,9,9,7,7,3,3,2,2}$ [90] | $Z_{10,10,10,9,9,7,7,3,3,2,2,1,1}$ [90] |
| | [2,1,0,0,1,1,1,2,0,2] | [3,8,14,20,26,33,41,50,37,24,24] | $Z_{10,10,10,9,9,8,5,4,3,2,2}$ [192] | $Z_{10,10,10,9,9,8,5,4,3,2,2,1,1}$ [192] |
| | [2,2,2,0,0,0,0,1,2,4] | [2,6,12,20,28,36,44,52,37,24,24] | $Z_{10,10,9,9,8,8,7,7,2,1,1}$ [96] | $Z_{10,10,9,9,8,8,7,7,2,1,1,1,1}$ [96] |
| | [2,3,0,0,1,0,1,0,2,4] | [2,6,13,20,27,35,43,52,37,24,24] | $Z_{10,10,9,9,8,8,8,5,3,1,1}$ [144] | $Z_{10,10,9,9,8,8,8,5,3,1,1,1,1}$ [144] |
| | [3,0,2,1,0,0,1,0,2,4] | [2,7,12,19,27,35,43,52,37,24,24] | $Z_{10,10,9,9,9,7,7,6,3,1,1}$ [144] | $Z_{10,10,9,9,9,7,7,6,3,1,1,1,1}$ [144] |
| | [3,1,0,1,1,1,0,0,2,4] | [2,7,13,19,26,34,43,52,37,24,24] | $Z_{10,10,9,9,9,8,6,5,4,1,1}$ [192] | $Z_{10,10,9,9,9,8,6,5,4,1,1,1,1}$ [192] |
| | [3,1,0,2,0,0,0,2,1,3] | [2,7,13,19,27,35,43,51,37,24,24] | $Z_{10,10,9,9,9,8,6,6,2,2,1}$ [120] | $Z_{10,10,9,9,9,8,6,6,2,2,1,1,1}$ [120] |
| | [3,1,1,0,0,1,1,1,1,3] | [2,7,13,20,27,34,42,51,37,24,24] | $Z_{10,10,9,9,9,8,7,4,3,2,1}$ [256] | $Z_{10,10,9,9,9,8,7,4,3,2,1,1,1}$ [256] |
| | [4,0,0,0,2,0,1,1,1,3] | [2,8,14,20,26,34,42,51,37,24,24] | $Z_{10,10,9,9,9,9,5,5,3,2,1}$ [120] | $Z_{10,10,9,9,9,9,5,5,3,2,1,1,1}$ [120] |
| | [4,0,1,0,0,0,1,3,0,2] | [2,8,14,21,28,35,42,50,37,24,24] | $Z_{10,10,9,9,9,9,7,3,2,2,2}$ [90] | $Z_{10,10,9,9,9,9,7,3,2,2,2,1,1}$ [90] |
| | [5,0,2,0,0,0,0,0,3,5] | [1,7,13,21,29,37,45,53,37,24,24] | $Z_{10,9,9,9,9,9,7,7,1,1,1}$ [42] | $Z_{10,9,9,9,9,9,7,7,1,1,1,1,1}$ [42] |
| | [5,1,0,0,1,0,0,1,2,4] | [1,7,14,21,28,36,44,52,37,24,24] | $Z_{10,9,9,9,9,9,8,5,2,1,1}$ [128] | $Z_{10,9,9,9,9,9,8,5,2,1,1,1,1}$ [128] |
| | [6,0,0,0,0,0,2,0,2,4] | [1,8,15,22,29,36,43,52,37,24,24] | $Z_{10,9,9,9,9,9,9,3,3,1,1}$ [42] | $Z_{10,9,9,9,9,9,9,3,3,1,1,1,1}$ [42] |
| | [0,0,1,4,0,0,0,0,1,5] | [4,8,12,17,26,35,44,53,38,24,24] | $Z_{10,10,10,10,7,6,6,6,6,1}$ [48] | $Z_{10,10,10,10,7,6,6,6,6,1,1,1,1,1}$ [48] |
| | [0,0,2,1,1,1,1,0,0,4] | [4,8,12,18,25,33,42,52,38,24,24] | $Z_{10,10,10,10,7,7,6,5,4,3}$ [128] | $Z_{10,10,10,10,7,7,6,5,4,3,1,1,1,1}$ [128] |
| | [0,1,1,0,1,3,0,0,0,4] | [4,8,13,19,25,32,42,52,38,24,24] | $Z_{10,10,10,10,8,7,5,4,4,4}$ [90] | $Z_{10,10,10,10,8,7,5,4,4,4,1,1,1,1}$ [90] |
| | [0,2,3,0,0,1,0,0,1,5] | [3,6,11,19,27,35,44,53,38,24,24] | $Z_{10,10,10,8,8,7,7,7,4,1}$ [96] | $Z_{10,10,10,8,8,7,7,7,4,1,1,1,1,1}$ [96] |
| | [0,3,0,2,1,0,0,0,1,5] | [3,6,12,18,26,35,44,53,38,24,24] | $Z_{10,10,10,8,8,8,6,6,5,1}$ [90] | $Z_{10,10,10,8,8,8,6,6,5,1,1,1,1,1}$ [90] |
| | [0,3,1,0,1,1,0,1,0,4] | [3,6,12,19,26,34,43,52,38,24,24] | $Z_{10,10,10,8,8,8,7,5,4,2}$ [162] | $Z_{10,10,10,8,8,8,7,5,4,2,1,1,1,1}$ [162] |
| | [0,4,0,0,0,1,2,0,0,4] | [3,6,13,20,27,34,42,52,38,24,24] | $Z_{10,10,10,8,8,8,8,4,3,3}$ [60] | $Z_{10,10,10,8,8,8,8,4,3,3,1,1,1,1}$ [60] |
| | [1,0,0,0,4,0,1,0,0,4] | [4,9,14,19,24,33,42,52,38,24,24] | $Z_{10,10,10,10,9,5,5,5,5,3}$ [60] | $Z_{10,10,10,10,9,5,5,5,5,3,1,1,1,1}$ [60] |
| | [1,0,3,1,1,0,0,0,1,5] | [3,7,11,18,26,35,44,53,38,24,24] | $Z_{10,10,10,9,7,7,7,6,5,1}$ [120] | $Z_{10,10,10,9,7,7,7,6,5,1,1,1,1,1}$ [120] |
| | [1,0,4,0,0,0,1,1,0,4] | [3,7,11,19,27,35,43,52,38,24,24] | $Z_{10,10,10,9,7,7,7,7,3,2}$ [90] | $Z_{10,10,10,9,7,7,7,7,3,2,1,1,1,1}$ [90] |
| | [1,1,1,1,2,0,0,1,0,4] | [3,7,12,18,25,34,43,52,38,24,24] | $Z_{10,10,10,9,8,7,6,5,5,2}$ [192] | $Z_{10,10,10,9,8,7,6,5,5,2,1,1,1,1}$ [192] |

| | | | | |
|---|---|---|---|---|
| | [1,1,1,2,0,0,2,0,0,4] | [3,7,12,18,26,34,42,52,38,24,24] | $Z_{10,10,10,9,8,7,6,6,3,3}$ [128] | $Z_{10,10,10,9,8,7,6,6,3,3,1,1,1,1}$ [128] |
| | [1,1,2,0,0,2,1,0,0,4] | [3,7,12,19,26,33,42,52,38,24,24] | $Z_{10,10,10,9,8,7,7,4,4,3}$ [128] | $Z_{10,10,10,9,8,7,7,4,4,3,1,1,1,1}$ [128] |
| | [1,2,0,0,2,1,1,0,0,4] | [3,7,13,19,25,33,42,52,38,24,24] | $Z_{10,10,10,9,8,8,5,5,4,3}$ [128] | $Z_{10,10,10,9,8,8,5,5,4,3,1,1,1,1}$ [128] |
| | [1,5,0,0,0,0,0,1,1,5] | [2,5,13,21,29,37,45,53,38,24,24] | $Z_{10,10,9,8,8,8,8,8,2,1}$ [56] | $Z_{10,10,9,8,8,8,8,8,2,1,1,1,1,1}$ [56] |
| | [2,0,0,2,1,1,1,0,0,4] | [3,8,13,18,25,33,42,52,38,24,24] | $Z_{10,10,10,9,9,6,6,5,4,3}$ [128] | $Z_{10,10,10,9,9,6,6,5,4,3,1,1,1,1}$ [128] |
| | [2,1,0,0,0,4,0,0,0,4] | [3,8,14,20,26,32,42,52,38,24,24] | $Z_{10,10,10,9,9,8,4,4,4,4}$ [50] | $Z_{10,10,10,9,9,8,4,4,4,4,1,1,1,1}$ [50] |
| | [2,2,1,0,2,0,0,0,1,5] | [2,6,12,19,26,35,44,53,38,24,24] | $Z_{10,10,9,9,8,8,7,5,5,1}$ [120] | $Z_{10,10,9,9,8,8,7,5,5,1,1,1,1,1}$ [120] |
| | [2,2,1,1,0,0,1,1,0,4] | [2,6,12,19,27,35,43,52,38,24,24] | $Z_{10,10,9,9,8,8,7,6,3,2}$ [192] | $Z_{10,10,9,9,8,8,7,6,3,2,1,1,1,1}$ [192] |
| | [2,3,0,0,0,2,0,1,0,4] | [2,6,13,20,27,34,43,52,38,24,24] | $Z_{10,10,9,9,8,8,8,4,4,2}$ [90] | $Z_{10,10,9,9,8,8,8,4,4,2,1,1,1,1}$ [90] |
| | [3,0,1,2,1,0,0,0,1,5] | [2,7,12,18,26,35,44,53,38,24,24] | $Z_{10,10,9,9,9,7,6,6,5,1}$ [120] | $Z_{10,10,9,9,9,7,6,6,5,1,1,1,1,1}$ [120] |
| | [3,0,2,0,1,1,0,1,0,4] | [2,7,12,19,26,34,43,52,38,24,24] | $Z_{10,10,9,9,9,7,7,5,4,2}$ [162] | $Z_{10,10,9,9,9,7,7,5,4,2,1,1,1,1}$ [162] |
| | [3,1,0,1,1,0,2,0,0,4] | [2,7,13,19,26,34,42,52,38,24,24] | $Z_{10,10,9,9,9,8,6,5,3,3}$ [144] | $Z_{10,10,9,9,9,8,6,5,3,3,1,1,1,1}$ [144] |
| | [4,0,0,0,1,2,1,0,0,4] | [2,8,14,20,26,33,42,52,38,24,24] | $Z_{10,10,9,9,9,9,5,4,4,3}$ [80] | $Z_{10,10,9,9,9,9,5,4,4,3,1,1,1,1}$ [80] |
| | [4,2,0,1,0,0,1,0,1,5] | [1,6,13,20,28,36,44,53,38,24,24] | $Z_{10,9,9,9,9,8,8,6,3,1}$ [144] | $Z_{10,9,9,9,9,8,8,6,3,1,1,1,1,1}$ [144] |
| | [5,0,1,0,1,1,0,0,1,5] | [1,7,13,20,27,35,44,53,38,24,24] | $Z_{10,9,9,9,9,9,7,5,4,1}$ [144] | $Z_{10,9,9,9,9,9,7,5,4,1,1,1,1,1}$ [144] |
| | [5,0,1,1,0,0,0,2,0,4] | [1,7,13,20,28,36,44,52,38,24,24] | $Z_{10,9,9,9,9,9,7,6,2,2}$ [90] | $Z_{10,9,9,9,9,9,7,6,2,2,1,1,1,1}$ [90] |
| | [5,1,0,0,0,1,1,1,0,4] | [1,7,14,21,28,35,43,52,38,24,24] | $Z_{10,9,9,9,9,9,8,4,3,2}$ [120] | $Z_{10,9,9,9,9,9,8,4,3,2,1,1,1,1}$ [120] |
| | [0,2,2,2,0,0,0,0,0,6] | [3,6,11,18,27,36,45,54,39,24,24] | $Z_{10,10,10,8,8,7,7,6,6}$ [42] | $Z_{10,10,10,8,8,7,7,6,6,1,1,1,1,1,1}$ [42] |
| | [1,4,1,0,0,1,0,0,0,6] | [2,5,12,20,28,36,45,54,39,24,24] | $Z_{10,10,9,8,8,8,8,7,4}$ [80] | $Z_{10,10,9,8,8,8,8,7,4,1,1,1,1,1,1}$ [80] |
| | [2,1,3,0,1,0,0,0,0,6] | [2,6,11,19,27,36,45,54,39,24,24] | $Z_{10,10,9,9,8,7,7,7,5}$ [72] | $Z_{10,10,9,9,8,7,7,7,5,1,1,1,1,1,1}$ [72] |
| | [2,2,0,3,0,0,0,0,0,6] | [2,6,12,18,27,36,45,54,39,24,24] | $Z_{10,10,9,9,8,8,6,6,6}$ [42] | $Z_{10,10,9,9,8,8,6,6,6,1,1,1,1,1,1}$ [42] |
| | [4,1,2,0,0,1,0,0,0,6] | [1,6,12,20,28,36,45,54,39,24,24] | $Z_{10,9,9,9,9,8,7,7,4}$ [80] | $Z_{10,9,9,9,9,8,7,7,4,1,1,1,1,1,1}$ [80] |
| | [4,2,0,0,2,0,0,0,0,6] | [1,6,13,20,27,36,45,54,39,24,24] | $Z_{10,9,9,9,9,8,8,5,5}$ [48] | $Z_{10,9,9,9,9,8,8,5,5,1,1,1,1,1,1}$ [48] |
| | [5,0,0,2,1,0,0,0,0,6] | [1,7,13,19,27,36,45,54,39,24,24] | $Z_{10,9,9,9,9,9,6,6,5}$ [48] | $Z_{10,9,9,9,9,9,6,6,5,1,1,1,1,1,1}$ [48] |
| | [7,1,0,0,0,0,0,0,1,7] | [0,7,15,23,31,39,47,55,39,24,24] | $Z_{9,9,9,9,9,9,9,8,1}$ [32] | $Z_{9,9,9,9,9,9,9,8,1,1,1,1,1,1,1}$ [32] |
| | [0,0,1,1,0,1,0,0,7,1] | [5,10,15,21,28,35,43,51,34,24,25] | $Z_{10,10,10,10,10,7,6,4,1,1,1,1,1,1,1}$ [96] | $Z_{10,10,10,10,10,7,6,4,1}$ [96] |
| | [0,1,0,0,1,0,1,1,6,0] | [5,10,16,22,28,35,42,50,34,24,25] | $Z_{10,10,10,10,10,8,5,3,2,1,1,1,1,1,1}$ [108] | $Z_{10,10,10,10,10,8,5,3,2}$ [108] |
| | [1,1,1,0,0,0,1,0,7,1] | [4,9,15,22,29,36,43,51,34,24,25] | $Z_{10,10,10,10,9,8,7,3,1,1,1,1,1,1,1}$ [120] | $Z_{10,10,10,10,9,8,7,3,1}$ [120] |
| | [2,0,0,0,1,1,0,0,7,1] | [4,10,16,22,28,35,43,51,34,24,25] | $Z_{10,10,10,10,9,9,5,4,1,1,1,1,1,1,1}$ [80] | $Z_{10,10,10,10,9,9,5,4,1}$ [80] |
| | [2,0,0,1,0,0,0,2,6,0] | [4,10,16,22,29,36,43,50,34,24,25] | $Z_{10,10,10,10,9,9,6,2,2,1,1,1,1,1,1}$ [60] | $Z_{10,10,10,10,9,9,6,2,2}$ [60] |
| | [0,0,0,1,1,1,1,1,4,0] | [5,10,15,20,26,33,41,50,35,24,25] | $Z_{10,10,10,10,10,6,5,4,3,2,1,1,1,1}$ [120] | $Z_{10,10,10,10,10,6,5,4,3,2}$ [120] |
| | [0,1,0,0,0,0,4,0,4,0] | [5,10,16,22,28,34,40,50,35,24,25] | $Z_{10,10,10,10,10,8,3,3,3,3,1,1,1,1}$ [36] | $Z_{10,10,10,10,10,8,3,3,3,3}$ [36] |
| | [0,1,1,2,0,0,0,1,5,1] | [4,8,13,19,27,35,43,51,35,24,25] | $Z_{10,10,10,10,8,7,6,6,2,1,1,1,1,1}$ [120] | $Z_{10,10,10,10,8,7,6,6,2,1}$ [120] |
| | [0,1,2,0,0,1,1,0,5,1] | [4,8,13,20,27,34,42,51,35,24,25] | $Z_{10,10,10,10,8,7,7,4,3,1,1,1,1,1}$ [144] | $Z_{10,10,10,10,8,7,7,4,3,1}$ [144] |
| | [0,2,0,0,2,0,1,0,5,1] | [4,8,14,20,26,34,42,51,35,24,25] | $Z_{10,10,10,10,8,8,5,5,3,1,1,1,1,1}$ [108] | $Z_{10,10,10,10,8,8,5,5,3,1}$ [108] |
| | [0,2,0,1,0,1,0,2,4,0] | [4,8,14,20,27,34,42,50,35,24,25] | $Z_{10,10,10,10,8,8,6,4,2,2,1,1,1,1}$ [121] | $Z_{10,10,10,10,8,8,6,4,2,2}$ [122] |
| | [1,0,0,2,1,0,1,0,5,1] | [4,9,14,19,26,34,42,51,35,24,25] | $Z_{10,10,10,10,9,6,6,5,3,1,1,1,1,1}$ [144] | $Z_{10,10,10,10,9,6,6,5,3,1}$ [144] |
| | [1,0,1,0,1,2,0,0,5,1] | [4,9,14,20,26,33,42,51,35,24,25] | $Z_{10,10,10,10,9,7,5,4,4,1,1,1,1,1}$ [144] | $Z_{10,10,10,10,9,7,5,4,4,1}$ [144] |
| | [1,0,1,0,2,0,0,2,4,0] | [4,9,14,20,26,34,42,50,35,24,25] | $Z_{10,10,10,10,9,7,5,5,2,2,1,1,1,1}$ [108] | $Z_{10,10,10,10,9,7,5,5,2,2}$ [108] |
| | [1,0,1,1,0,0,2,1,4,0] | [4,9,14,20,27,34,41,50,35,24,25] | $Z_{10,10,10,10,9,7,6,3,3,2,1,1,1,1}$ [144] | $Z_{10,10,10,10,9,7,6,3,3,2}$ [144] |
| | [1,1,0,0,0,2,1,1,4,0] | [4,9,15,21,27,33,41,50,35,24,25] | $Z_{10,10,10,10,9,8,4,4,3,2,1,1,1,1}$ [120] | $Z_{10,10,10,10,9,8,4,4,3,2}$ [120] |
| | [1,2,1,1,0,0,0,0,6,2] | [3,7,13,20,28,36,44,52,35,24,25] | $Z_{10,10,10,9,8,8,7,6,1,1,1,1,1,1}$ [96] | $Z_{10,10,10,9,8,8,7,6,1,1}$ [96] |
| | [1,3,0,0,0,1,0,1,5,1] | [3,7,14,21,28,35,43,51,35,24,25] | $Z_{10,10,10,9,8,8,8,4,2,1,1,1,1,1}$ [120] | $Z_{10,10,10,9,8,8,8,4,2,1}$ [120] |
| | [2,0,2,0,1,0,0,1,5,1] | [3,8,13,20,27,35,43,51,35,24,25] | $Z_{10,10,10,9,9,7,7,5,2,1,1,1,1,1}$ [144] | $Z_{10,10,10,9,9,7,7,5,2,1}$ [144] |
| | [2,1,0,1,0,1,1,0,5,1] | [3,8,14,20,27,34,42,51,35,24,25] | $Z_{10,10,10,9,9,8,6,4,3,1,1,1,1,1}$ [216] | $Z_{10,10,10,9,9,8,6,4,3,1}$ [216] |
| | [2,1,1,0,0,0,1,2,4,0] | [3,8,14,21,28,35,42,50,35,24,25] | $Z_{10,10,10,9,9,8,7,3,2,2,1,1,1,1}$ [120] | $Z_{10,10,10,9,9,8,7,3,2,2}$ [120] |
| | [3,0,0,0,1,1,0,2,4,0] | [3,9,15,21,27,34,42,50,35,24,25] | $Z_{10,10,10,9,9,9,5,4,2,2,1,1,1,1}$ [90] | $Z_{10,10,10,9,9,9,5,4,2,2}$ [90] |
| | [4,0,1,0,1,0,0,0,6,2] | [2,8,14,21,28,36,44,52,35,24,25] | $Z_{10,10,9,9,9,9,7,5,1,1,1,1,1,1}$ [90] | $Z_{10,10,9,9,9,9,7,5,1,1}$ [90] |
| | [4,1,0,0,0,0,1,1,5,1] | [2,8,15,22,29,36,43,51,35,24,25] | $Z_{10,10,9,9,9,9,8,3,2,1,1,1,1,1}$ [96] | $Z_{10,10,9,9,9,9,8,3,2,1}$ [96] |
| | [0,0,0,1,0,2,2,1,2,0] | [5,10,15,20,26,32,40,50,36,24,25] | $Z_{10,10,10,10,10,6,4,4,3,3,2,1,1}$ [90] | $Z_{10,10,10,10,10,6,4,4,3,3,2}$ [90] |
| | [0,0,2,1,2,0,0,0,4,2] | [4,8,12,18,25,34,43,52,36,24,25] | $Z_{10,10,10,10,7,7,6,5,5,1,1,1,1}$ [80] | $Z_{10,10,10,10,7,7,6,5,5,1,1}$ [80] |
| | [0,0,2,2,0,0,1,1,3,1] | [4,8,12,18,26,34,42,51,36,24,25] | $Z_{10,10,10,10,7,7,6,6,3,2,1,1,1}$ [128] | $Z_{10,10,10,10,7,7,6,6,3,2,1}$ [128] |
| | [0,0,3,0,0,2,0,1,3,1] | [4,8,12,19,26,33,42,51,36,24,25] | $Z_{10,10,10,10,7,7,7,4,4,2,1,1,1}$ [96] | $Z_{10,10,10,10,7,7,7,4,4,2,1}$ [96] |
| | [0,1,0,2,1,1,0,1,3,1] | [4,8,13,18,25,33,42,51,36,24,25] | $Z_{10,10,10,10,8,6,6,5,4,2,1,1,1}$ [216] | $Z_{10,10,10,10,8,6,6,5,4,2,1}$ [216] |
| | [0,1,1,0,2,0,2,0,3,1] | [4,8,13,19,25,33,41,51,36,24,25] | $Z_{10,10,10,10,8,7,5,5,3,3,1,1,1}$ [162] | $Z_{10,10,10,10,8,7,5,5,3,3,1}$ [162] |
| | [0,1,1,1,0,1,1,2,2,0] | [4,8,13,19,26,33,41,50,36,24,25] | $Z_{10,10,10,10,8,7,6,4,3,2,2,1,1}$ [216] | $Z_{10,10,10,10,8,7,6,4,3,2,2}$ [216] |
| | [0,2,0,0,0,3,1,0,3,1] | [4,8,14,20,26,32,41,51,36,24,25] | $Z_{10,10,10,10,8,8,4,4,4,3,1,1,1}$ [90] | $Z_{10,10,10,10,8,8,4,4,4,3,1}$ [90] |
| | [0,3,1,1,0,0,1,0,4,2] | [3,6,12,19,27,35,43,52,36,24,25] | $Z_{10,10,10,8,8,8,7,6,3,1,1,1,1}$ [144] | $Z_{10,10,10,8,8,8,7,6,3,1,1}$ [144] |
| | [0,4,0,0,1,0,0,2,3,1] | [3,6,13,20,27,35,43,51,36,24,25] | $Z_{10,10,10,8,8,8,8,5,2,2,1,1,1}$ [96] | $Z_{10,10,10,8,8,8,8,5,2,2,1}$ [96] |
| | [1,0,0,1,1,2,1,0,3,1] | [4,9,14,19,25,32,41,51,36,24,25] | $Z_{10,10,10,10,9,6,5,4,4,3,1,1,1}$ [192] | $Z_{10,10,10,10,9,6,5,4,4,3,1}$ [192] |
| | [1,0,0,1,2,0,1,2,2,0] | [4,9,14,19,25,33,41,50,36,24,25] | $Z_{10,10,10,10,9,6,5,5,3,2,2,1,1}$ [144] | $Z_{10,10,10,10,9,6,5,5,3,2,2}$ [144] |
| | [1,0,1,0,0,3,0,2,2,0] | [4,9,14,20,26,32,41,50,36,24,25] | $Z_{10,10,10,10,9,7,4,4,4,2,2,1,1}$ [108] | $Z_{10,10,10,10,9,7,4,4,4,2,2}$ [108] |
| | [1,0,1,0,1,0,3,1,2,0] | [4,9,14,20,26,33,40,50,36,24,25] | $Z_{10,10,10,10,9,7,5,3,3,3,2,1,1}$ [162] | $Z_{10,10,10,10,9,7,5,3,3,3,2}$ [162] |
| | [1,1,1,2,0,1,0,0,4,2] | [3,7,12,18,26,34,43,52,36,24,25] | $Z_{10,10,10,9,8,7,6,6,4,1,1,1,1}$ [192] | $Z_{10,10,10,9,8,7,6,6,4,1,1}$ [192] |
| | [1,1,2,0,1,0,1,1,3,1] | [3,7,12,19,26,34,42,51,36,24,25] | $Z_{10,10,10,9,8,7,7,5,3,2,1,1,1}$ [288] | $Z_{10,10,10,9,8,7,7,5,3,2,1}$ [288] |
| | [1,2,0,0,3,0,0,0,4,2] | [3,7,13,19,25,34,43,52,36,24,25] | $Z_{10,10,10,9,8,8,5,5,5,1,1,1,1}$ [80] | $Z_{10,10,10,9,8,8,5,5,5,1,1}$ [80] |
| | [1,2,0,1,0,2,0,1,3,1] | [3,7,13,19,26,33,42,51,36,24,25] | $Z_{10,10,10,9,8,8,6,4,4,2,1,1,1}$ [216] | $Z_{10,10,10,9,8,8,6,4,4,2,1}$ [216] |
| | [1,2,1,0,0,0,3,0,3,1] | [3,7,13,20,27,34,41,51,36,24,25] | $Z_{10,10,10,9,8,8,7,3,3,3,1,1,1}$ [120] | $Z_{10,10,10,9,8,8,7,3,3,3,1}$ [120] |
| | [1,2,1,0,0,1,0,3,2,0] | [3,7,13,20,27,34,42,50,36,24,25] | $Z_{10,10,10,9,8,8,7,4,2,2,2,1,1}$ [144] | $Z_{10,10,10,9,8,8,7,4,2,2,2}$ [144] |
| | [2,0,0,3,0,0,1,1,3,1] | [3,8,13,18,26,34,42,51,36,24,25] | $Z_{10,10,10,9,9,6,6,6,3,2,1,1,1}$ [128] | $Z_{10,10,10,9,9,6,6,6,3,2,1}$ [128] |
| | [2,0,1,0,2,1,0,1,3,1] | [3,8,13,19,25,33,42,51,36,24,25] | $Z_{10,10,10,9,9,7,5,5,4,2,1,1,1}$ [216] | $Z_{10,10,10,9,9,7,5,5,4,2,1}$ [216] |

| | | | | |
|---|---|---|---|---|
| | [2,0,1,1,0,1,2,0,3,1] | [3,8,13,19,26,33,41,51,36,24,25] | $Z_{10,10,10,9,9,7,6,4,3,3,1,1,1}$ [216] | $Z_{10,10,10,9,9,7,6,4,3,3,1}$ [216] |
| | [2,0,1,1,1,0,0,3,2,0] | [3,8,13,19,26,34,42,50,36,24,25] | $Z_{10,10,10,9,9,7,6,5,2,2,2,1,1}$ [144] | $Z_{10,10,10,9,9,7,6,5,2,2,2}$ [144] |
| | [2,1,0,0,1,1,1,2,2,0] | [3,8,14,20,26,33,41,50,36,24,25] | $Z_{10,10,10,9,9,8,5,4,3,2,2,1,1}$ [192] | $Z_{10,10,10,9,9,8,5,4,3,2,2}$ [192] |
| | [2,2,2,0,0,0,0,1,4,2] | [2,6,12,20,28,36,44,52,36,24,25] | $Z_{10,10,9,9,8,8,7,7,2,1,1,1,1}$ [96] | $Z_{10,10,9,9,8,8,7,7,2,1,1}$ [96] |
| | [2,3,0,0,1,0,1,0,4,2] | [2,6,13,20,27,35,43,52,36,24,25] | $Z_{10,10,9,9,8,8,8,5,3,1,1,1,1}$ [144] | $Z_{10,10,9,9,8,8,8,5,3,1,1}$ [144] |
| | [3,0,2,1,0,0,1,0,4,2] | [2,7,12,19,27,35,43,52,36,24,25] | $Z_{10,10,9,9,9,7,7,6,3,1,1,1,1}$ [144] | $Z_{10,10,9,9,9,7,7,6,3,1,1}$ [144] |
| | [3,1,0,1,1,1,0,0,4,2] | [2,7,13,19,26,34,43,52,36,24,25] | $Z_{10,10,9,9,9,8,6,5,4,1,1,1,1}$ [192] | $Z_{10,10,9,9,9,8,6,5,4,1,1}$ [192] |
| | [3,1,0,2,0,0,0,2,3,1] | [2,7,13,19,27,35,43,51,36,24,25] | $Z_{10,10,9,9,9,8,6,6,2,2,1,1,1}$ [120] | $Z_{10,10,9,9,9,8,6,6,2,2,1}$ [120] |
| | [3,1,1,0,0,1,1,1,3,1] | [2,7,13,20,27,34,42,51,36,24,25] | $Z_{10,10,9,9,9,8,7,4,3,2,1,1,1}$ [256] | $Z_{10,10,9,9,9,8,7,4,3,2,1}$ [256] |
| | [4,0,0,0,2,0,1,1,3,1] | [2,8,14,20,26,34,42,51,36,24,25] | $Z_{10,10,9,9,9,9,5,5,3,2,1,1,1}$ [120] | $Z_{10,10,9,9,9,9,5,5,3,2,1}$ [120] |
| | [4,0,1,0,0,0,1,3,2,0] | [2,8,14,21,28,35,42,50,36,24,25] | $Z_{10,10,9,9,9,9,7,3,2,2,2,1,1}$ [90] | $Z_{10,10,9,9,9,9,7,3,2,2,2}$ [90] |
| | [5,0,2,0,0,0,0,0,5,3] | [1,7,13,21,29,37,45,53,36,24,25] | $Z_{10,9,9,9,9,9,7,7,1,1,1,1,1}$ [42] | $Z_{10,9,9,9,9,9,7,7,1,1,1}$ [42] |
| | [5,1,0,0,1,0,0,1,4,2] | [1,7,14,21,28,36,44,52,36,24,25] | $Z_{10,9,9,9,9,9,8,5,2,1,1,1,1}$ [128] | $Z_{10,9,9,9,9,9,8,5,2,1,1}$ [128] |
| | [0,0,1,2,2,0,1,1,0,2] | [4,8,12,17,24,33,42,52,38,24,25] | $Z_{10,10,10,10,7,6,6,5,5,3,2}$ [144] | $Z_{10,10,10,10,7,6,6,5,5,3,2,1,1}$ [144] |
| | [0,0,2,0,2,2,0,1,0,2] | [4,8,12,18,24,32,42,52,38,24,25] | $Z_{10,10,10,10,7,7,5,5,4,4,2}$ [108] | $Z_{10,10,10,10,7,7,5,5,4,4,2,1,1}$ [108] |
| | [0,0,2,1,0,2,2,0,0,2] | [4,8,12,18,25,32,41,52,38,24,25] | $Z_{10,10,10,10,7,7,6,4,4,3,3}$ [96] | $Z_{10,10,10,10,7,7,6,4,4,3,3,1,1}$ [96] |
| | [0,1,0,1,2,1,2,0,0,2] | [4,8,13,18,24,32,41,52,38,24,25] | $Z_{10,10,10,10,8,6,5,5,4,3,3}$ [144] | $Z_{10,10,10,10,8,6,5,5,4,3,3,1,1}$ [144] |
| | [0,1,4,0,1,0,0,1,1,3] | [3,6,10,18,26,35,44,53,38,24,25] | $Z_{10,10,10,8,7,7,7,7,5,2,1}$ [144] | $Z_{10,10,10,8,7,7,7,7,5,2,1,1,1}$ [144] |
| | [0,2,1,2,1,0,1,0,1,3] | [3,6,11,17,25,34,43,53,38,24,25] | $Z_{10,10,10,8,8,7,6,6,5,3,1}$ [216] | $Z_{10,10,10,8,8,7,6,6,5,3,1,1,1}$ [216] |
| | [0,2,2,0,1,2,0,0,1,3] | [3,6,11,18,25,33,43,53,38,24,25] | $Z_{10,10,10,8,8,7,7,5,4,4,1}$ [144] | $Z_{10,10,10,8,8,7,7,5,4,4,1,1,1}$ [144] |
| | [0,2,2,1,0,0,2,1,0,2] | [3,6,11,18,26,34,42,52,38,24,25] | $Z_{10,10,10,8,8,7,7,6,3,3,2}$ [144] | $Z_{10,10,10,8,8,7,7,6,3,3,2,1,1}$ [144] |
| | [0,3,0,1,1,1,1,1,0,2] | [3,6,12,18,25,33,42,52,38,24,25] | $Z_{10,10,10,8,8,8,6,5,4,3,2}$ [216] | $Z_{10,10,10,8,8,8,6,5,4,3,2,1,1}$ [216] |
| | [1,0,0,1,0,4,1,0,0,2] | [4,9,14,19,25,31,41,52,38,24,25] | $Z_{10,10,10,10,9,6,4,4,4,4,3}$ [96] | $Z_{10,10,10,10,9,6,4,4,4,4,3,1,1}$ [96] |
| | [1,0,2,2,0,2,0,0,1,3] | [3,7,11,17,25,33,43,53,38,24,25] | $Z_{10,10,10,9,7,7,6,6,4,4,1}$ [144] | $Z_{10,10,10,9,7,7,6,6,4,4,1,1,1}$ [144] |
| | [1,0,2,2,1,0,0,2,0,2] | [3,7,11,17,25,34,43,52,38,24,25] | $Z_{10,10,10,9,7,7,6,6,5,2,2}$ [144] | $Z_{10,10,10,9,7,7,6,6,5,2,2,1,1}$ [144] |
| | [1,0,3,0,1,1,1,1,0,2] | [3,7,11,18,25,33,42,52,38,24,25] | $Z_{10,10,10,9,7,7,7,5,4,3,2}$ [216] | $Z_{10,10,10,9,7,7,7,5,4,3,2,1,1}$ [216] |
| | [1,1,0,2,2,1,0,0,1,3] | [3,7,12,17,24,33,43,53,38,24,25] | $Z_{10,10,10,9,8,6,6,5,5,4,1}$ [192] | $Z_{10,10,10,9,8,6,6,5,5,4,1,1,1}$ [192] |
| | [1,1,0,3,0,1,1,1,0,2] | [3,7,12,17,25,33,42,52,38,24,25] | $Z_{10,10,10,9,8,6,6,6,4,3,2}$ [216] | $Z_{10,10,10,9,8,6,6,6,4,3,2,1,1}$ [216] |
| | [1,1,1,0,3,0,1,1,0,2] | [3,7,12,18,24,33,42,52,38,24,25] | $Z_{10,10,10,9,8,7,5,5,5,3,2}$ [216] | $Z_{10,10,10,9,8,7,5,5,5,3,2,1,1}$ [216] |
| | [1,1,1,1,0,3,0,1,0,2] | [3,7,12,18,25,32,42,52,38,24,25] | $Z_{10,10,10,9,8,7,6,4,4,4,2}$ [216] | $Z_{10,10,10,9,8,7,6,4,4,4,2,1,1}$ [216] |
| | [1,1,1,1,1,0,3,0,0,2] | [3,7,12,18,25,33,41,52,38,24,25] | $Z_{10,10,10,9,8,7,6,5,3,3,3}$ [192] | $Z_{10,10,10,9,8,7,6,5,3,3,3,1,1}$ [192] |
| | [1,2,0,0,1,2,2,0,0,2] | [3,7,13,19,25,32,41,52,38,24,25] | $Z_{10,10,10,9,8,8,5,4,4,3,3}$ [128] | $Z_{10,10,10,9,8,8,5,4,4,3,3,1,1}$ [128] |
| | [1,3,1,1,1,0,0,1,1,3] | [2,5,11,18,26,35,44,53,38,24,25] | $Z_{10,10,9,8,8,8,7,6,5,2,1}$ [256] | $Z_{10,10,9,8,8,8,7,6,5,2,1,1,1}$ [256] |
| | [1,3,2,0,0,0,2,0,1,3] | [2,5,11,19,27,35,43,53,38,24,25] | $Z_{10,10,9,8,8,8,7,7,3,3,1}$ [120] | $Z_{10,10,9,8,8,8,7,7,3,3,1,1,1}$ [120] |
| | [1,4,0,0,1,1,1,0,1,3] | [2,5,12,19,26,34,43,53,38,24,25] | $Z_{10,10,9,8,8,8,8,5,4,3,1}$ [192] | $Z_{10,10,9,8,8,8,8,5,4,3,1,1,1}$ [192] |
| | [1,4,0,1,0,0,1,2,0,2] | [2,5,12,19,27,35,43,52,38,24,25] | $Z_{10,10,9,8,8,8,8,6,3,2,2}$ [144] | $Z_{10,10,9,8,8,8,8,6,3,2,2,1,1}$ [144] |
| | [2,0,0,1,2,2,0,1,0,2] | [3,8,13,18,24,32,42,52,38,24,25] | $Z_{10,10,10,9,9,6,5,5,4,4,2}$ [144] | $Z_{10,10,10,9,9,6,5,5,4,4,2,1,1}$ [144] |
| | [2,0,4,1,0,0,0,0,2,4] | [2,6,10,18,27,36,45,54,38,24,25] | $Z_{10,10,9,9,7,7,7,7,6,1,1}$ [72] | $Z_{10,10,9,9,7,7,7,7,6,1,1,1,1}$ [72] |
| | [2,1,1,3,0,0,0,1,1,3] | [2,6,11,17,26,35,44,53,38,24,25] | $Z_{10,10,9,9,8,7,6,6,6,2,1}$ [160] | $Z_{10,10,9,9,8,7,6,6,6,2,1,1,1}$ [160] |
| | [2,1,2,0,2,0,1,0,1,3] | [2,6,11,18,25,34,43,53,38,24,25] | $Z_{10,10,9,9,8,7,7,5,5,3,1}$ [216] | $Z_{10,10,9,9,8,7,7,5,5,3,1,1,1}$ [216] |
| | [2,1,2,1,0,1,0,2,0,2] | [2,6,11,18,26,34,43,52,38,24,25] | $Z_{10,10,9,9,8,7,7,6,4,2,2}$ [216] | $Z_{10,10,9,9,8,7,7,6,4,2,2,1,1}$ [216] |
| | [2,2,0,1,1,2,0,0,1,3] | [2,6,12,18,25,33,43,53,38,24,25] | $Z_{10,10,9,9,8,8,6,5,4,4,1}$ [192] | $Z_{10,10,9,9,8,8,6,5,4,4,1,1,1}$ [192] |
| | [2,2,0,1,2,0,0,2,0,2] | [2,6,12,18,25,34,43,52,38,24,25] | $Z_{10,10,9,9,8,8,6,5,5,2,2}$ [144] | $Z_{10,10,9,9,8,8,6,5,5,2,2,1,1}$ [144] |
| | [2,2,0,2,0,0,2,1,0,2] | [2,6,12,18,26,34,42,52,38,24,25] | $Z_{10,10,9,9,8,8,6,6,3,3,2}$ [144] | $Z_{10,10,9,9,8,8,6,6,3,3,2,1,1}$ [144] |
| | [2,2,1,0,0,2,1,1,0,2] | [2,6,12,19,26,33,42,52,38,24,25] | $Z_{10,10,9,9,8,8,7,4,4,3,2}$ [192] | $Z_{10,10,9,9,8,8,7,4,4,3,2,1,1}$ [192] |
| | [3,0,0,3,1,0,1,0,1,3] | [2,7,12,17,25,34,43,53,38,24,25] | $Z_{10,10,9,9,9,6,6,6,5,3,1}$ [144] | $Z_{10,10,9,9,9,6,6,6,5,3,1,1,1}$ [144] |
| | [3,0,1,1,1,1,1,1,0,2] | [2,7,12,18,25,33,42,52,38,24,25] | $Z_{10,10,9,9,9,7,6,5,4,3,2}$ [288] | $Z_{10,10,9,9,9,7,6,5,4,3,2,1,1}$ [288] |
| | [3,1,0,1,0,1,3,0,0,2] | [2,7,13,19,26,33,41,52,38,24,25] | $Z_{10,10,9,9,9,8,6,4,3,3,3}$ [144] | $Z_{10,10,9,9,9,8,6,4,3,3,3,1,1}$ [144] |
| | [3,2,2,0,1,0,0,0,2,4] | [1,5,11,19,27,36,45,54,38,24,25] | $Z_{10,9,9,9,8,8,7,7,5,1,1}$ [120] | $Z_{10,9,9,9,8,8,7,7,5,1,1,1,1}$ [120] |
| | [3,3,0,1,0,1,0,1,1,3] | [1,5,12,19,27,35,44,53,38,24,25] | $Z_{10,9,9,9,8,8,8,6,4,2,1}$ [216] | $Z_{10,9,9,9,8,8,8,6,4,2,1,1,1}$ [216] |
| | [4,0,0,0,0,4,0,1,0,2] | [2,8,14,20,26,32,42,52,38,24,25] | $Z_{10,10,9,9,9,9,4,4,4,4,2}$ [54] | $Z_{10,10,9,9,9,9,4,4,4,4,2,1,1}$ [54] |
| | [4,0,3,0,0,1,0,1,1,3] | [1,6,11,19,27,35,44,53,38,24,25] | $Z_{10,9,9,9,9,7,7,7,4,2,1}$ [144] | $Z_{10,9,9,9,9,7,7,7,4,2,1,1,1}$ [144] |
| | [4,1,0,2,1,0,0,1,1,3] | [1,6,12,18,26,35,44,53,38,24,25] | $Z_{10,9,9,9,9,8,6,6,5,2,1}$ [192] | $Z_{10,9,9,9,9,8,6,6,5,2,1,1,1}$ [192] |
| | [4,1,1,0,1,1,1,0,1,3] | [1,6,12,19,26,34,43,53,38,24,25] | $Z_{10,9,9,9,9,8,7,5,4,3,1}$ [288] | $Z_{10,9,9,9,9,8,7,5,4,3,1,1,1}$ [288] |
| | [4,1,1,1,0,0,1,2,0,2] | [1,6,12,19,27,35,43,52,38,24,25] | $Z_{10,9,9,9,9,8,7,6,3,2,2}$ [192] | $Z_{10,9,9,9,9,8,7,6,3,2,2,1,1}$ [192] |
| | [5,0,0,1,1,1,0,2,0,2] | [1,7,13,19,26,34,43,52,38,24,25] | $Z_{10,9,9,9,9,9,6,5,4,2,2}$ [144] | $Z_{10,9,9,9,9,9,6,5,4,2,2,1,1}$ [144] |
| | [5,0,1,0,0,1,2,1,0,2] | [1,7,13,20,27,34,42,52,38,24,25] | $Z_{10,9,9,9,9,9,7,4,3,3,2}$ [144] | $Z_{10,9,9,9,9,9,7,4,3,3,2,1,1}$ [144] |
| | [6,1,0,1,0,1,0,0,2,4] | [0,6,13,20,28,36,45,54,38,24,25] | $Z_{9,9,9,9,9,9,8,6,4,1,1}$ [144] | $Z_{9,9,9,9,9,9,8,6,4,1,1,1,1}$ [144] |
| | [6,1,1,0,0,0,0,2,1,3] | [0,6,13,21,29,37,45,53,38,24,25] | $Z_{9,9,9,9,9,9,8,7,2,2,1}$ [96] | $Z_{9,9,9,9,9,9,8,7,2,2,1,1,1}$ [96] |
| | [7,0,0,0,1,0,1,1,1,3] | [0,7,14,21,28,36,44,53,38,24,25] | $Z_{9,9,9,9,9,9,9,5,3,2,1}$ [120] | $Z_{9,9,9,9,9,9,9,5,3,2,1,1,1}$ [120] |
| | [0,0,0,5,0,1,0,0,0,4] | [4,8,12,16,25,34,44,54,39,24,25] | $Z_{10,10,10,10,6,6,6,6,6,4}$ [38] | $Z_{10,10,10,10,6,6,6,6,6,4,1,1,1,1}$ [37] |
| | [0,1,3,2,0,0,1,0,0,4] | [3,6,10,17,26,35,44,54,39,24,25] | $Z_{10,10,10,8,7,7,7,6,6,3}$ [96] | $Z_{10,10,10,8,7,7,7,6,6,3,1,1,1,1}$ [96] |
| | [0,1,4,0,0,2,0,0,0,4] | [3,6,10,18,26,34,44,54,39,24,25] | $Z_{10,10,10,8,7,7,7,7,4,4}$ [60] | $Z_{10,10,10,8,7,7,7,7,4,4,1,1,1,1}$ [60] |
| | [0,3,0,0,4,0,0,0,0,4] | [3,6,12,18,24,34,44,54,39,24,25] | $Z_{10,10,10,8,8,8,5,5,5,5}$ [36] | $Z_{10,10,10,8,8,8,5,5,5,5,1,1,1,1}$ [36] |
| | [0,5,1,1,0,0,0,0,1,5] | [2,4,11,19,28,37,46,55,39,24,25] | $Z_{10,10,8,8,8,8,8,7,6,1}$ [72] | $Z_{10,10,8,8,8,8,8,7,6,1,1,1,1,1}$ [72] |
| | [0,6,0,0,0,1,0,1,0,4] | [2,4,12,20,28,36,45,54,39,24,25] | $Z_{10,10,8,8,8,8,8,8,4,2}$ [68] | $Z_{10,10,8,8,8,8,8,8,4,2,1,1,1,1}$ [67] |
| | [1,0,2,1,3,0,0,0,0,4] | [3,7,11,17,24,34,44,54,39,24,25] | $Z_{10,10,10,9,7,7,6,5,5,5}$ [72] | $Z_{10,10,10,9,7,7,6,5,5,5,1,1,1,1}$ [72] |
| | [1,2,3,1,0,0,0,1,0,4] | [2,5,10,18,27,36,45,54,39,24,25] | $Z_{10,10,9,8,8,7,7,7,6,2}$ [120] | $Z_{10,10,9,8,8,7,7,7,6,2,1,1,1,1}$ [120] |
| | [1,3,1,1,0,2,0,0,0,4] | [2,5,11,18,26,34,44,54,39,24,25] | $Z_{10,10,9,8,8,8,7,6,4,4}$ [120] | $Z_{10,10,9,8,8,8,7,6,4,4,1,1,1,1}$ [120] |
| | [2,0,4,0,1,0,1,0,0,4] | [2,6,10,18,26,35,44,54,39,24,25] | $Z_{10,10,9,9,7,7,7,7,5,3}$ [108] | $Z_{10,10,9,9,7,7,7,7,5,3,1,1,1,1}$ [108] |
| | [2,1,1,2,1,1,0,0,0,4] | [2,6,11,17,25,34,44,54,39,24,25] | $Z_{10,10,9,9,8,7,6,6,5,4}$ [160] | $Z_{10,10,9,9,8,7,6,6,5,4,1,1,1,1}$ [160] |

| | | | | |
|---|---|---|---|---|
| | [2,5,0,0,1,0,0,0,1,5] | [1,4,12,20,28,37,46,55,39,24,25] | $Z_{10,9,9,8,8,8,8,8,5,1}$ [80] | $Z_{10,9,9,8,8,8,8,8,5,1,1,1,1,1}$ [80] |
| | [3,0,1,0,4,0,0,0,0,4] | [2,7,12,18,24,34,44,54,39,24,25] | $Z_{10,10,9,9,9,7,5,5,5,5}$ [54] | $Z_{10,10,9,9,9,7,5,5,5,5,1,1,1,1}$ [54] |
| | [3,2,1,2,0,0,0,1,0,4] | [1,5,11,18,27,36,45,54,39,24,25] | $Z_{10,9,9,9,8,8,7,6,6,2}$ [120] | $Z_{10,9,9,9,8,8,7,6,6,2,1,1,1,1}$ [120] |
| | [3,2,2,0,0,1,1,0,0,4] | [1,5,11,19,27,35,44,54,39,24,25] | $Z_{10,9,9,9,8,8,7,7,4,3}$ [128] | $Z_{10,9,9,9,8,8,7,7,4,3,1,1,1,1}$ [128] |
| | [3,3,0,0,2,0,1,0,0,4] | [1,5,12,19,26,35,44,54,39,24,25] | $Z_{10,9,9,9,8,8,8,5,5,3}$ [96] | $Z_{10,9,9,9,8,8,8,5,5,3,1,1,1,1}$ [96] |
| | [4,0,2,1,1,0,1,0,0,4] | [1,6,11,18,26,35,44,54,39,24,25] | $Z_{10,9,9,9,9,7,7,6,5,3}$ [144] | $Z_{10,9,9,9,9,7,7,6,5,3,1,1,1,1}$ [144] |
| | [4,1,0,2,0,2,0,0,0,4] | [1,6,12,18,26,34,44,54,39,24,25] | $Z_{10,9,9,9,9,8,6,6,4,4}$ [90] | $Z_{10,9,9,9,9,8,6,6,4,4,1,1,1,1}$ [90] |
| | [5,0,0,0,3,1,0,0,0,4] | [1,7,13,19,25,34,44,54,39,24,25] | $Z_{10,9,9,9,9,9,5,5,5,4}$ [50] | $Z_{10,9,9,9,9,9,5,5,5,4,1,1,1,1}$ [50] |
| | [5,2,1,0,1,0,0,0,1,5] | [0,5,12,20,28,37,46,55,39,24,25] | $Z_{9,9,9,9,9,8,8,7,5,1}$ [120] | $Z_{9,9,9,9,9,8,8,7,5,1,1,1,1,1}$ [120] |
| | [5,3,0,0,0,0,1,1,0,4] | [0,5,13,21,29,37,45,54,39,24,25] | $Z_{9,9,9,9,9,8,8,8,3,2}$ [72] | $Z_{9,9,9,9,9,8,8,8,3,2,1,1,1,1}$ [72] |
| | [6,0,1,2,0,0,0,0,1,5] | [0,6,12,19,28,37,46,55,39,24,25] | $Z_{9,9,9,9,9,9,7,6,6,1}$ [72] | $Z_{9,9,9,9,9,9,7,6,6,1,1,1,1,1}$ [72] |
| | [6,0,2,0,0,1,0,1,0,4] | [0,6,12,20,28,36,45,54,39,24,25] | $Z_{9,9,9,9,9,9,7,7,4,2}$ [108] | $Z_{9,9,9,9,9,9,7,7,4,2,1,1,1,1}$ [108] |
| | [6,1,0,0,2,0,0,1,0,4] | [0,6,13,20,27,36,45,54,39,24,25] | $Z_{9,9,9,9,9,9,8,5,5,2}$ [96] | $Z_{9,9,9,9,9,9,8,5,5,2,1,1,1,1}$ [96] |
| | [6,1,0,1,0,0,2,0,0,4] | [0,6,13,20,28,36,44,54,39,24,25] | $Z_{9,9,9,9,9,9,8,6,3,3}$ [96] | $Z_{9,9,9,9,9,9,8,6,3,3,1,1,1,1}$ [96] |
| | [7,0,0,0,0,2,1,0,0,4] | [0,7,14,21,28,35,44,54,39,24,25] | $Z_{9,9,9,9,9,9,9,4,4,3}$ [48] | $Z_{9,9,9,9,9,9,9,4,4,3,1,1,1,1}$ [48] |
| | [1,1,0,1,1,0,0,0,8,0] | [4,9,15,21,28,36,44,52,34,24,26] | $Z_{10,10,10,10,9,8,6,5,1,1,1,1,1,1,1,1}$ [72] | $Z_{10,10,10,10,9,8,6,5}$ [72] |
| | [0,1,1,1,1,1,0,0,6,0] | [4,8,13,19,26,34,43,52,35,24,26] | $Z_{10,10,10,10,8,7,6,5,4,1,1,1,1,1,1}$ [120] | $Z_{10,10,10,10,8,7,6,5,4}$ [120] |
| | [1,2,1,0,1,0,1,0,6,0] | [3,7,13,20,27,35,43,52,35,24,26] | $Z_{10,10,10,9,8,8,7,5,3,1,1,1,1,1,1}$ [144] | $Z_{10,10,10,9,8,8,7,5,3}$ [144] |
| | [2,0,1,2,0,0,1,0,6,0] | [3,8,13,19,27,35,43,52,35,24,26] | $Z_{10,10,10,9,9,7,6,6,3,1,1,1,1,1,1}$ [96] | $Z_{10,10,10,9,9,7,6,6,3}$ [96] |
| | [2,0,2,0,0,2,0,0,6,0] | [3,8,13,20,27,34,43,52,35,24,26] | $Z_{10,10,10,9,9,7,7,4,4,1,1,1,1,1,1}$ [60] | $Z_{10,10,10,9,9,7,7,4,4}$ [60] |
| | [2,1,0,0,2,1,0,0,6,0] | [3,8,14,20,26,34,43,52,35,24,26] | $Z_{10,10,10,9,9,8,5,5,4,1,1,1,1,1,1}$ [80] | $Z_{10,10,10,9,9,8,5,5,4}$ [80] |
| | [3,1,2,0,0,0,0,0,7,1] | [2,7,13,21,29,37,45,53,35,24,26] | $Z_{10,10,9,9,9,8,7,7,1,1,1,1,1,1,1}$ [56] | $Z_{10,10,9,9,9,8,7,7,1}$ [56] |
| | [3,2,0,0,1,0,0,1,6,0] | [2,7,14,21,28,36,44,52,35,24,26] | $Z_{10,10,9,9,9,8,8,5,2,1,1,1,1,1,1}$ [96] | $Z_{10,10,9,9,9,8,8,5,2}$ [96] |
| | [4,0,0,2,0,0,0,1,6,0] | [2,8,14,20,28,36,44,52,35,24,26] | $Z_{10,10,9,9,9,9,6,6,2,1,1,1,1,1,1}$ [60] | $Z_{10,10,9,9,9,9,6,6,2}$ [60] |
| | [4,0,1,0,0,1,1,0,6,0] | [2,8,14,21,28,35,43,52,35,24,26] | $Z_{10,10,9,9,9,9,7,4,3,1,1,1,1,1,1}$ [96] | $Z_{10,10,9,9,9,9,7,4,3}$ [96] |
| | [0,0,1,4,0,0,0,0,5,1] | [4,8,12,17,26,35,44,53,36,24,26] | $Z_{10,10,10,10,7,6,6,6,6,1,1,1,1,1}$ [48] | $Z_{10,10,10,10,7,6,6,6,6,1}$ [48] |
| | [0,0,2,1,1,1,1,0,4,0] | [4,8,12,18,25,33,42,52,36,24,26] | $Z_{10,10,10,10,7,7,6,5,4,3,1,1,1,1}$ [128] | $Z_{10,10,10,10,7,7,6,5,4,3}$ [128] |
| | [0,1,1,0,1,3,0,0,4,0] | [4,8,13,19,25,32,42,52,36,24,26] | $Z_{10,10,10,10,8,7,5,4,4,4,1,1,1,1}$ [90] | $Z_{10,10,10,10,8,7,5,4,4,4}$ [90] |
| | [0,3,0,2,1,0,0,0,5,1] | [3,6,12,18,26,35,44,53,36,24,26] | $Z_{10,10,10,8,8,8,6,6,5,1,1,1,1,1}$ [90] | $Z_{10,10,10,8,8,8,6,6,5,1}$ [90] |
| | [0,3,1,0,1,1,0,1,4,0] | [3,6,12,19,26,34,43,52,36,24,26] | $Z_{10,10,10,8,8,8,7,5,4,2,1,1,1,1}$ [162] | $Z_{10,10,10,8,8,8,7,5,4,2}$ [162] |
| | [0,4,0,0,0,1,2,0,4,0] | [3,6,13,20,27,34,42,52,36,24,26] | $Z_{10,10,10,8,8,8,8,4,3,3,1,1,1,1}$ [60] | $Z_{10,10,10,8,8,8,8,4,3,3}$ [60] |
| | [1,0,0,0,4,0,1,0,4,0] | [4,9,14,19,24,33,42,52,36,24,26] | $Z_{10,10,10,10,9,5,5,5,5,3,1,1,1,1}$ [60] | $Z_{10,10,10,10,9,5,5,5,5,3}$ [60] |
| | [1,1,1,1,2,0,0,1,4,0] | [3,7,12,18,25,34,43,52,36,24,26] | $Z_{10,10,10,9,8,7,6,5,5,2,1,1,1,1}$ [192] | $Z_{10,10,10,9,8,7,6,5,5,2}$ [192] |
| | [1,1,1,2,0,0,2,0,4,0] | [3,7,12,18,26,34,42,52,36,24,26] | $Z_{10,10,10,9,8,7,6,6,3,3,1,1,1,1}$ [128] | $Z_{10,10,10,9,8,7,6,6,3,3}$ [128] |
| | [1,1,2,0,0,2,1,0,4,0] | [3,7,12,19,26,33,42,52,36,24,26] | $Z_{10,10,10,9,8,7,7,4,4,3,1,1,1,1}$ [128] | $Z_{10,10,10,9,8,7,7,4,4,3}$ [128] |
| | [1,2,0,0,2,1,1,0,4,0] | [3,7,13,19,25,33,42,52,36,24,26] | $Z_{10,10,10,9,8,8,5,5,4,3,1,1,1,1}$ [128] | $Z_{10,10,10,9,8,8,5,5,4,3}$ [128] |
| | [1,5,0,0,0,0,0,1,5,1] | [2,5,13,21,29,37,45,53,36,24,26] | $Z_{10,10,9,8,8,8,8,8,2,1,1,1,1,1}$ [56] | $Z_{10,10,9,8,8,8,8,8,2,1}$ [56] |
| | [2,0,0,2,1,1,1,0,4,0] | [3,8,13,18,25,33,42,52,36,24,26] | $Z_{10,10,10,9,9,6,6,5,4,3,1,1,1,1}$ [128] | $Z_{10,10,10,9,9,6,6,5,4,3}$ [128] |
| | [2,2,1,0,2,0,0,0,5,1] | [2,6,12,19,26,35,44,53,36,24,26] | $Z_{10,10,9,9,8,8,7,5,5,1,1,1,1,1}$ [120] | $Z_{10,10,9,9,8,8,7,5,5,1}$ [120] |
| | [2,2,1,1,0,0,1,1,4,0] | [2,6,12,19,27,35,43,52,36,24,26] | $Z_{10,10,9,9,8,8,7,6,3,2,1,1,1,1}$ [192] | $Z_{10,10,9,9,8,8,7,6,3,2}$ [192] |
| | [2,3,0,0,0,2,0,1,4,0] | [2,6,13,20,27,34,43,52,36,24,26] | $Z_{10,10,9,9,8,8,8,4,4,2,1,1,1,1}$ [90] | $Z_{10,10,9,9,8,8,8,4,4,2}$ [90] |
| | [3,0,1,2,1,0,0,0,5,1] | [2,7,12,18,26,35,44,53,36,24,26] | $Z_{10,10,9,9,9,7,6,6,5,1,1,1,1,1}$ [120] | $Z_{10,10,9,9,9,7,6,6,5,1}$ [120] |
| | [3,0,2,0,1,1,0,1,4,0] | [2,7,12,19,26,34,43,52,36,24,26] | $Z_{10,10,9,9,9,7,7,5,4,2,1,1,1,1}$ [162] | $Z_{10,10,9,9,9,7,7,5,4,2}$ [162] |
| | [3,1,0,1,1,0,2,0,4,0] | [2,7,13,19,26,34,42,52,36,24,26] | $Z_{10,10,9,9,9,8,6,5,3,3,1,1,1,1}$ [144] | $Z_{10,10,9,9,9,8,6,5,3,3}$ [144] |
| | [4,2,0,1,0,0,1,0,5,1] | [1,6,13,20,28,36,44,53,36,24,26] | $Z_{10,9,9,9,9,8,8,6,3,1,1,1,1,1}$ [144] | $Z_{10,9,9,9,9,8,8,6,3,1}$ [144] |
| | [5,0,1,0,1,1,0,0,5,1] | [1,7,13,20,27,35,44,53,36,24,26] | $Z_{10,9,9,9,9,9,7,5,4,1,1,1,1,1}$ [144] | $Z_{10,9,9,9,9,9,7,5,4,1}$ [144] |
| | [5,0,1,1,0,0,0,2,4,0] | [1,7,13,20,28,36,44,52,36,24,26] | $Z_{10,9,9,9,9,9,7,6,2,2,1,1,1,1}$ [90] | $Z_{10,9,9,9,9,9,7,6,2,2}$ [90] |
| | [5,1,0,0,0,1,1,1,4,0] | [1,7,14,21,28,35,43,52,36,24,26] | $Z_{10,9,9,9,9,9,8,4,3,2,1,1,1,1}$ [120] | $Z_{10,9,9,9,9,9,8,4,3,2}$ [120] |
| | [0,0,1,2,2,0,1,1,2,0] | [4,8,12,17,24,33,42,52,37,24,26] | $Z_{10,10,10,10,7,6,6,5,5,3,2,1,1}$ [144] | $Z_{10,10,10,10,7,6,6,5,5,3,2}$ [144] |
| | [0,0,2,0,2,2,0,1,2,0] | [4,8,12,18,24,32,42,52,37,24,26] | $Z_{10,10,10,10,7,7,5,5,4,4,2,1,1}$ [108] | $Z_{10,10,10,10,7,7,5,5,4,4,2}$ [108] |
| | [0,0,2,1,0,2,2,0,2,0] | [4,8,12,18,25,32,41,52,37,24,26] | $Z_{10,10,10,10,7,7,6,4,4,3,3,1,1}$ [96] | $Z_{10,10,10,10,7,7,6,4,4,3,3}$ [96] |
| | [0,1,0,1,2,1,2,0,2,0] | [4,8,13,18,24,32,41,52,37,24,26] | $Z_{10,10,10,10,8,6,5,5,4,3,3,1,1}$ [144] | $Z_{10,10,10,10,8,6,5,5,4,3,3}$ [144] |
| | [0,2,1,2,1,0,1,0,3,1] | [3,6,11,17,25,34,43,53,37,24,26] | $Z_{10,10,10,8,8,7,6,6,5,3,1,1,1}$ [216] | $Z_{10,10,10,8,8,7,6,6,5,3,1}$ [216] |
| | [0,2,2,0,1,2,0,0,3,1] | [3,6,11,18,25,33,43,53,37,24,26] | $Z_{10,10,10,8,8,7,7,5,4,4,1,1,1}$ [144] | $Z_{10,10,10,8,8,7,7,5,4,4,1}$ [144] |
| | [0,2,2,0,2,0,0,2,2,0] | [3,6,11,18,25,34,43,52,37,24,26] | $Z_{10,10,10,8,8,7,7,5,5,2,2,1,1}$ [108] | $Z_{10,10,10,8,8,7,7,5,5,2,2}$ [108] |
| | [0,2,2,1,0,0,2,1,2,0] | [3,6,11,18,26,34,42,52,37,24,26] | $Z_{10,10,10,8,8,7,7,6,3,3,2,1,1}$ [144] | $Z_{10,10,10,8,8,7,7,6,3,3,2}$ [144] |
| | [0,3,0,1,1,1,1,1,2,0] | [3,6,12,18,25,33,42,52,37,24,26] | $Z_{10,10,10,8,8,8,6,5,4,3,2,1,1}$ [216] | $Z_{10,10,10,8,8,8,6,5,4,3,2}$ [216] |
| | [1,0,0,1,0,4,1,0,2,0] | [4,9,14,19,25,31,41,52,37,24,26] | $Z_{10,10,10,10,9,6,4,4,4,4,3,1,1}$ [96] | $Z_{10,10,10,10,9,6,4,4,4,4,3}$ [96] |
| | [1,0,2,2,0,2,0,0,3,1] | [3,7,11,17,25,33,43,53,37,24,26] | $Z_{10,10,10,9,7,7,6,6,4,4,1,1,1}$ [144] | $Z_{10,10,10,9,7,7,6,6,4,4,1}$ [144] |
| | [1,0,2,2,1,0,0,2,2,0] | [3,7,11,17,25,34,43,52,37,24,26] | $Z_{10,10,10,9,7,7,6,6,5,2,2,1,1}$ [144] | $Z_{10,10,10,9,7,7,6,6,5,2,2}$ [144] |
| | [1,0,3,0,1,1,1,1,2,0] | [3,7,11,18,25,33,42,52,37,24,26] | $Z_{10,10,10,9,7,7,7,5,4,3,2,1,1}$ [216] | $Z_{10,10,10,9,7,7,7,5,4,3,2}$ [216] |
| | [1,1,0,2,2,1,0,0,3,1] | [3,7,12,17,24,33,43,53,37,24,26] | $Z_{10,10,10,9,8,6,6,5,5,4,1,1,1}$ [192] | $Z_{10,10,10,9,8,6,6,5,5,4,1}$ [192] |
| | [1,1,0,3,0,1,1,1,2,0] | [3,7,12,17,25,33,42,52,37,24,26] | $Z_{10,10,10,9,8,6,6,6,4,3,2,1,1}$ [216] | $Z_{10,10,10,9,8,6,6,6,4,3,2}$ [216] |
| | [1,1,1,0,3,0,1,1,2,0] | [3,7,12,18,24,33,42,52,37,24,26] | $Z_{10,10,10,9,8,7,5,5,5,3,2,1,1}$ [216] | $Z_{10,10,10,9,8,7,5,5,5,3,2}$ [216] |
| | [1,1,1,1,0,3,0,1,2,0] | [3,7,12,18,25,32,42,52,37,24,26] | $Z_{10,10,10,9,8,7,6,4,4,4,2,1,1}$ [216] | $Z_{10,10,10,9,8,7,6,4,4,4,2}$ [216] |
| | [1,1,1,1,1,0,3,0,2,0] | [3,7,12,18,25,33,41,52,37,24,26] | $Z_{10,10,10,9,8,7,6,5,3,3,3,1,1}$ [192] | $Z_{10,10,10,9,8,7,6,5,3,3,3}$ [192] |
| | [1,2,0,0,1,2,2,0,2,0] | [3,7,13,19,25,32,41,52,37,24,26] | $Z_{10,10,10,9,8,8,5,4,4,3,3,1,1}$ [128] | $Z_{10,10,10,9,8,8,5,4,4,3,3}$ [128] |
| | [1,3,1,1,1,0,0,1,3,1] | [2,5,11,18,26,35,44,53,37,24,26] | $Z_{10,10,9,8,8,8,7,6,5,2,1,1,1}$ [256] | $Z_{10,10,9,8,8,8,7,6,5,2,1}$ [256] |
| | [1,3,2,0,0,0,2,0,3,1] | [2,5,11,19,27,35,43,53,37,24,26] | $Z_{10,10,9,8,8,8,7,7,3,3,1,1,1}$ [120] | $Z_{10,10,9,8,8,8,7,7,3,3,1}$ [120] |
| | [1,4,0,0,1,1,1,0,3,1] | [2,5,12,19,26,34,43,53,37,24,26] | $Z_{10,10,9,8,8,8,8,5,4,3,1,1,1}$ [192] | $Z_{10,10,9,8,8,8,8,5,4,3,1}$ [192] |
| | [1,4,0,1,0,0,1,2,2,0] | [2,5,12,19,27,35,43,52,37,24,26] | $Z_{10,10,9,8,8,8,8,6,3,2,2,1,1}$ [144] | $Z_{10,10,9,8,8,8,8,6,3,2,2}$ [144] |

| | | | | |
|---|---|---|---|---|
| | [2,0,0,1,2,2,0,1,2,0] | [3,8,13,18,24,32,42,52,37,24,26] | $Z_{10,10,10,9,9,6,5,5,4,4,2,1,1}$ [144] | $Z_{10,10,10,9,9,6,5,5,4,4,2}$ [144] |
| | [2,0,0,2,0,2,2,0,2,0] | [3,8,13,18,25,32,41,52,37,24,26] | $Z_{10,10,10,9,9,6,6,4,4,3,3,1,1}$ [96] | $Z_{10,10,10,9,9,6,6,4,4,3,3}$ [96] |
| | [2,1,1,3,0,0,0,1,3,1] | [2,6,11,17,26,35,44,53,37,24,26] | $Z_{10,10,9,9,8,7,6,6,6,2,1,1,1}$ [160] | $Z_{10,10,9,9,8,7,6,6,6,2,1}$ [160] |
| | [2,1,2,0,2,0,1,0,3,1] | [2,6,11,18,25,34,43,53,37,24,26] | $Z_{10,10,9,9,8,7,7,5,5,3,1,1,1}$ [216] | $Z_{10,10,9,9,8,7,7,5,5,3,1}$ [216] |
| | [2,1,2,1,0,1,0,2,2,0] | [2,6,11,18,26,34,43,52,37,24,26] | $Z_{10,10,9,9,8,7,7,6,4,2,2,1,1}$ [216] | $Z_{10,10,9,9,8,7,7,6,4,2,2}$ [216] |
| | [2,2,0,1,1,2,0,0,3,1] | [2,6,12,18,25,33,43,53,37,24,26] | $Z_{10,10,9,9,8,8,6,5,4,4,1,1,1}$ [192] | $Z_{10,10,9,9,8,8,6,5,4,4,1}$ [192] |
| | [2,2,0,1,2,0,0,2,2,0] | [2,6,12,18,25,34,43,52,37,24,26] | $Z_{10,10,9,9,8,8,6,5,5,2,2,1,1}$ [144] | $Z_{10,10,9,9,8,8,6,5,5,2,2}$ [144] |
| | [2,2,0,2,0,0,2,1,2,0] | [2,6,12,18,26,34,42,52,37,24,26] | $Z_{10,10,9,9,8,8,6,6,3,3,2,1,1}$ [144] | $Z_{10,10,9,9,8,8,6,6,3,3,2}$ [144] |
| | [2,2,1,0,0,2,1,1,2,0] | [2,6,12,19,26,33,42,52,37,24,26] | $Z_{10,10,9,9,8,8,7,4,4,3,2,1,1}$ [192] | $Z_{10,10,9,9,8,8,7,4,4,3,2}$ [192] |
| | [3,0,0,3,1,0,1,0,3,1] | [2,7,12,17,25,34,43,53,37,24,26] | $Z_{10,10,9,9,9,6,6,6,5,3,1,1,1}$ [144] | $Z_{10,10,9,9,9,6,6,6,5,3,1}$ [144] |
| | [3,0,1,1,1,1,1,1,2,0] | [2,7,12,18,25,33,42,52,37,24,26] | $Z_{10,10,9,9,9,7,6,5,4,3,2,1,1}$ [288] | $Z_{10,10,9,9,9,7,6,5,4,3,2}$ [288] |
| | [3,1,0,1,0,1,3,0,2,0] | [2,7,13,19,26,33,41,52,37,24,26] | $Z_{10,10,9,9,9,8,6,4,3,3,3,1,1}$ [144] | $Z_{10,10,9,9,9,8,6,4,3,3,3}$ [144] |
| | [3,2,2,0,1,0,0,0,4,2] | [1,5,11,19,27,36,45,54,37,24,26] | $Z_{10,9,9,9,8,8,7,7,5,1,1,1,1}$ [120] | $Z_{10,9,9,9,8,8,7,7,5,1,1}$ [120] |
| | [3,3,0,1,0,1,0,1,3,1] | [1,5,12,19,27,35,44,53,37,24,26] | $Z_{10,9,9,9,8,8,8,6,4,2,1,1,1}$ [216] | $Z_{10,9,9,9,8,8,8,6,4,2,1}$ [216] |
| | [4,0,2,2,0,0,0,0,4,2] | [1,6,11,18,27,36,45,54,37,24,26] | $Z_{10,9,9,9,9,7,7,6,6,1,1,1,1}$ [72] | $Z_{10,9,9,9,9,7,7,6,6,1,1}$ [72] |
| | [4,0,3,0,0,1,0,1,3,1] | [1,6,11,19,27,35,44,53,37,24,26] | $Z_{10,9,9,9,9,7,7,7,4,2,1,1,1}$ [144] | $Z_{10,9,9,9,9,7,7,7,4,2,1}$ [144] |
| | [4,1,0,2,1,0,0,1,3,1] | [1,6,12,18,26,35,44,53,37,24,26] | $Z_{10,9,9,9,9,8,6,6,5,2,1,1,1}$ [192] | $Z_{10,9,9,9,9,8,6,6,5,2,1}$ [192] |
| | [4,1,1,0,1,1,1,0,3,1] | [1,6,12,19,26,34,43,53,37,24,26] | $Z_{10,9,9,9,9,8,7,5,4,3,1,1,1}$ [288] | $Z_{10,9,9,9,9,8,7,5,4,3,1}$ [288] |
| | [4,1,1,1,0,0,1,2,2,0] | [1,6,12,19,27,35,43,52,37,24,26] | $Z_{10,9,9,9,9,8,7,6,3,2,2,1,1}$ [192] | $Z_{10,9,9,9,9,8,7,6,3,2,2}$ [192] |
| | [4,2,0,0,0,2,0,2,2,0] | [1,6,13,20,27,34,43,52,37,24,26] | $Z_{10,9,9,9,9,8,8,4,4,2,2,1,1}$ [90] | $Z_{10,9,9,9,9,8,8,4,4,2,2}$ [90] |
| | [5,0,0,1,1,1,0,2,2,0] | [1,7,13,19,26,34,43,52,37,24,26] | $Z_{10,9,9,9,9,9,6,5,4,2,2,1,1}$ [144] | $Z_{10,9,9,9,9,9,6,5,4,2,2}$ [144] |
| | [5,0,1,0,0,1,2,1,2,0] | [1,7,13,20,27,34,42,52,37,24,26] | $Z_{10,9,9,9,9,9,7,4,3,3,2,1,1}$ [144] | $Z_{10,9,9,9,9,9,7,4,3,3,2}$ [144] |
| | [6,1,0,1,0,1,0,0,4,2] | [0,6,13,20,28,36,45,54,37,24,26] | $Z_{9,9,9,9,9,9,8,6,4,1,1,1,1}$ [144] | $Z_{9,9,9,9,9,9,8,6,4,1,1}$ [144] |
| | [6,1,1,0,0,0,0,2,3,1] | [0,6,13,21,29,37,45,53,37,24,26] | $Z_{9,9,9,9,9,9,8,7,2,2,1,1,1}$ [96] | $Z_{9,9,9,9,9,9,8,7,2,2,1}$ [96] |
| | [7,0,0,0,1,0,1,1,3,1] | [0,7,14,21,28,36,44,53,37,24,26] | $Z_{9,9,9,9,9,9,9,5,3,2,1,1,1}$ [120] | $Z_{9,9,9,9,9,9,9,5,3,2,1}$ [120] |
| | [0,0,5,1,0,1,0,0,1,3] | [3,6,9,17,26,35,45,55,39,24,26] | $Z_{10,10,10,7,7,7,7,7,6,4,1}$ [96] | $Z_{10,10,10,7,7,7,7,7,6,4,1,1,1}$ [96] |
| | [0,0,6,0,0,0,0,2,0,2] | [3,6,9,18,27,36,45,54,39,24,26] | $Z_{10,10,10,7,7,7,7,7,7,2,2}$ [36] | $Z_{10,10,10,7,7,7,7,7,7,2,2,1,1}$ [36] |
| | [0,1,2,3,0,1,0,1,0,2] | [3,6,10,16,25,34,44,54,39,24,26] | $Z_{10,10,10,8,7,7,6,6,6,4,2}$ [162] | $Z_{10,10,10,8,7,7,6,6,6,4,2,1,1}$ [162] |
| | [0,1,3,0,3,0,0,1,0,2] | [3,6,10,17,24,34,44,54,39,24,26] | $Z_{10,10,10,8,7,7,7,5,5,5,2}$ [108] | $Z_{10,10,10,8,7,7,7,5,5,5,2,1,1}$ [108] |
| | [0,1,3,1,0,2,1,0,0,2] | [3,6,10,17,25,33,43,54,39,24,26] | $Z_{10,10,10,8,7,7,7,6,4,4,3}$ [144] | $Z_{10,10,10,8,7,7,7,6,4,4,3,1,1}$ [144] |
| | [0,2,0,3,2,0,0,1,0,2] | [3,6,11,16,24,34,44,54,39,24,26] | $Z_{10,10,10,8,8,6,6,6,5,5,2}$ [108] | $Z_{10,10,10,8,8,6,6,6,5,5,2,1,1}$ [108] |
| | [0,2,0,4,0,0,2,0,0,2] | [3,6,11,16,25,34,43,54,39,24,26] | $Z_{10,10,10,8,8,6,6,6,6,3,3}$ [72] | $Z_{10,10,10,8,8,6,6,6,6,3,3,1,1}$ [72] |
| | [0,2,2,0,0,4,0,0,0,2] | [3,6,11,18,25,32,43,54,39,24,26] | $Z_{10,10,10,8,8,7,7,4,4,4,4}$ [60] | $Z_{10,10,10,8,8,7,7,4,4,4,4,1,1}$ [60] |
| | [0,3,0,0,2,3,0,0,0,2] | [3,6,12,18,24,32,43,54,39,24,26] | $Z_{10,10,10,8,8,8,5,5,4,4,4}$ [60] | $Z_{10,10,10,8,8,8,5,5,4,4,4,1,1}$ [60] |
| | [0,4,2,0,1,1,0,0,1,3] | [2,4,10,18,26,35,45,55,39,24,26] | $Z_{10,10,8,8,8,8,7,7,5,4,1}$ [144] | $Z_{10,10,8,8,8,8,7,7,5,4,1,1,1}$ [144] |
| | [0,4,2,1,0,0,0,2,0,2] | [2,4,10,18,27,36,45,54,39,24,26] | $Z_{10,10,8,8,8,8,7,7,6,2,2}$ [90] | $Z_{10,10,8,8,8,8,7,7,6,2,2,1,1}$ [90] |
| | [0,5,0,1,1,0,1,1,0,2] | [2,4,11,18,26,35,44,54,39,24,26] | $Z_{10,10,8,8,8,8,8,6,5,3,2}$ [162] | $Z_{10,10,8,8,8,8,8,6,5,3,2,1,1}$ [162] |
| | [1,0,1,3,1,1,1,0,0,2] | [3,7,11,16,24,33,43,54,39,24,26] | $Z_{10,10,10,9,7,6,6,6,5,4,3}$ [192] | $Z_{10,10,10,9,7,6,6,6,5,4,3,1,1}$ [192] |
| | [1,0,2,1,1,3,0,0,0,2] | [3,7,11,17,24,32,43,54,39,24,26] | $Z_{10,10,10,9,7,7,6,5,4,4,4}$ [120] | $Z_{10,10,10,9,7,7,6,5,4,4,4,1,1}$ [120] |
| | [1,1,5,0,0,0,1,0,1,3] | [2,5,9,18,27,36,45,55,39,24,26] | $Z_{10,10,9,8,7,7,7,7,7,3,1}$ [120] | $Z_{10,10,9,8,7,7,7,7,7,3,1,1,1}$ [120] |
| | [1,2,2,1,1,1,0,1,0,2] | [2,5,10,17,25,34,44,54,39,24,26] | $Z_{10,10,9,8,8,7,7,6,5,4,2}$ [288] | $Z_{10,10,9,8,8,7,7,6,5,4,2,1,1}$ [288] |
| | [1,2,3,0,0,1,2,0,0,2] | [2,5,10,18,26,34,43,54,39,24,26] | $Z_{10,10,9,8,8,7,7,7,4,3,3}$ [128] | $Z_{10,10,9,8,8,7,7,7,4,3,3,1,1}$ [128] |
| | [1,3,0,2,1,0,2,0,0,2] | [2,5,11,17,25,34,43,54,39,24,26] | $Z_{10,10,9,8,8,8,6,6,5,3,3}$ [144] | $Z_{10,10,9,8,8,8,6,6,5,3,3,1,1}$ [144] |
| | [1,3,1,0,1,2,1,0,0,2] | [2,5,11,18,25,33,43,54,39,24,26] | $Z_{10,10,9,8,8,8,7,5,4,4,3}$ [192] | $Z_{10,10,9,8,8,8,7,5,4,4,3,1,1}$ [192] |
| | [2,0,2,3,1,0,0,0,1,3] | [2,6,10,16,25,35,45,55,39,24,26] | $Z_{10,10,9,9,7,7,6,6,6,5,1}$ [120] | $Z_{10,10,9,9,7,7,6,6,6,5,1,1,1}$ [120] |
| | [2,0,3,1,1,0,2,0,0,2] | [2,6,10,17,25,34,43,54,39,24,26] | $Z_{10,10,9,9,7,7,7,6,5,3,3}$ [144] | $Z_{10,10,9,9,7,7,7,6,5,3,3,1,1}$ [144] |
| | [2,1,0,4,0,1,0,1,0,2] | [2,6,11,16,25,34,44,54,39,24,26] | $Z_{10,10,9,9,8,6,6,6,6,4,2}$ [162] | $Z_{10,10,9,9,8,6,6,6,6,4,2,1,1}$ [162] |
| | [2,1,1,1,2,1,1,0,0,2] | [2,6,11,17,24,33,43,54,39,24,26] | $Z_{10,10,9,9,8,7,6,5,5,4,3}$ [256] | $Z_{10,10,9,9,8,7,6,5,5,4,3,1,1}$ [256] |
| | [2,2,0,1,0,4,0,0,0,2] | [2,6,12,18,25,32,43,54,39,24,26] | $Z_{10,10,9,9,8,8,6,4,4,4,4}$ [90] | $Z_{10,10,9,9,8,8,6,4,4,4,4,1,1}$ [90] |
| | [2,3,2,1,0,0,1,0,1,3] | [1,4,10,18,27,36,45,55,39,24,26] | $Z_{10,9,9,8,8,8,7,7,6,3,1}$ [192] | $Z_{10,9,9,8,8,8,7,7,6,3,1,1,1}$ [192] |
| | [2,4,0,1,1,1,0,0,1,3] | [1,4,11,18,26,35,45,55,39,24,26] | $Z_{10,9,9,8,8,8,8,6,5,4,1}$ [192] | $Z_{10,9,9,8,8,8,8,6,5,4,1,1,1}$ [192] |
| | [2,4,0,2,0,0,0,2,0,2] | [1,4,11,18,27,36,45,54,39,24,26] | $Z_{10,9,9,8,8,8,8,6,6,2,2}$ [90] | $Z_{10,9,9,8,8,8,8,6,6,2,2,1,1}$ [90] |
| | [2,4,1,0,0,1,1,1,0,2] | [1,4,11,19,27,35,44,54,39,24,26] | $Z_{10,9,9,8,8,8,8,7,4,3,2}$ [192] | $Z_{10,9,9,8,8,8,8,7,4,3,2,1,1}$ [192] |
| | [3,0,1,0,2,3,0,0,0,2] | [2,7,12,18,24,32,43,54,39,24,26] | $Z_{10,10,9,9,9,7,5,5,4,4,4}$ [90] | $Z_{10,10,9,9,9,7,5,5,4,4,4,1,1}$ [90] |
| | [3,1,2,2,0,1,0,0,1,3] | [1,5,10,17,26,35,45,55,39,24,26] | $Z_{10,9,9,9,8,7,7,6,6,4,1}$ [192] | $Z_{10,9,9,9,8,7,7,6,6,4,1,1,1}$ [192] |
| | [3,1,3,0,1,0,1,1,0,2] | [1,5,10,18,26,35,44,54,39,24,26] | $Z_{10,9,9,9,8,7,7,7,5,3,2}$ [216] | $Z_{10,9,9,9,8,7,7,7,5,3,2,1,1}$ [216] |
| | [3,2,0,2,2,0,0,0,1,3] | [1,5,11,17,25,35,45,55,39,24,26] | $Z_{10,9,9,9,8,8,6,6,5,5,1}$ [120] | $Z_{10,9,9,9,8,8,6,6,5,5,1,1,1}$ [120] |
| | [3,2,0,3,0,0,1,1,0,2] | [1,5,11,17,26,35,44,54,39,24,26] | $Z_{10,9,9,9,8,8,6,6,6,3,2}$ [144] | $Z_{10,9,9,9,8,8,6,6,6,3,2,1,1}$ [144] |
| | [3,2,1,0,2,1,0,1,0,2] | [1,5,11,18,25,34,44,54,39,24,26] | $Z_{10,9,9,9,8,8,7,5,5,4,2}$ [216] | $Z_{10,9,9,9,8,8,7,5,5,4,2,1,1}$ [216] |
| | [3,2,1,1,0,1,2,0,0,2] | [1,5,11,18,26,34,43,54,39,24,26] | $Z_{10,9,9,9,8,8,7,6,4,3,3}$ [192] | $Z_{10,9,9,9,8,8,7,6,4,3,3,1,1}$ [192] |
| | [4,0,1,2,1,1,0,1,0,2] | [1,6,11,17,25,34,44,54,39,24,26] | $Z_{10,9,9,9,9,7,6,6,5,4,2}$ [216] | $Z_{10,9,9,9,9,7,6,6,5,4,2,1,1}$ [216] |
| | [4,0,2,0,2,0,2,0,0,2] | [1,6,11,18,25,34,43,54,39,24,26] | $Z_{10,9,9,9,9,7,7,5,5,3,3}$ [108] | $Z_{10,9,9,9,9,7,7,5,5,3,3,1,1}$ [108] |
| | [4,1,0,1,1,2,1,0,0,2] | [1,6,12,18,25,33,43,54,39,24,26] | $Z_{10,9,9,9,9,8,6,5,4,4,3}$ [192] | $Z_{10,9,9,9,9,8,6,5,4,4,3,1,1}$ [192] |
| | [4,3,1,1,0,0,0,1,1,3] | [0,4,11,19,28,37,46,55,39,24,26] | $Z_{9,9,9,9,8,8,8,7,6,2,1}$ [160] | $Z_{9,9,9,9,8,8,8,7,6,2,1,1,1}$ [160] |
| | [4,4,0,0,0,1,1,0,1,3] | [0,4,12,20,28,36,45,55,39,24,26] | $Z_{9,9,9,9,8,8,8,8,4,3,1}$ [120] | $Z_{9,9,9,9,8,8,8,8,4,3,1,1,1}$ [120] |
| | [5,1,1,2,0,0,1,0,1,3] | [0,5,11,18,27,36,45,55,39,24,26] | $Z_{9,9,9,9,9,8,7,6,6,3,1}$ [192] | $Z_{9,9,9,9,9,8,7,6,6,3,1,1,1}$ [192] |
| | [5,1,2,0,0,2,0,0,1,3] | [0,5,11,19,27,35,45,55,39,24,26] | $Z_{9,9,9,9,9,8,7,7,4,4,1}$ [128] | $Z_{9,9,9,9,9,8,7,7,4,4,1,1,1}$ [128] |
| | [5,1,2,0,1,0,0,2,0,2] | [0,5,11,19,27,36,45,54,39,24,26] | $Z_{9,9,9,9,9,8,7,7,5,2,2}$ [144] | $Z_{9,9,9,9,9,8,7,7,5,2,2,1,1}$ [144] |
| | [5,2,0,0,2,1,0,0,1,3] | [0,5,12,19,26,35,45,55,39,24,26] | $Z_{9,9,9,9,9,8,8,5,5,4,1}$ [128] | $Z_{9,9,9,9,9,8,8,5,5,4,1,1,1}$ [128] |
| | [5,2,0,1,0,1,1,1,0,2] | [0,5,12,19,27,35,44,54,39,24,26] | $Z_{9,9,9,9,9,8,8,6,4,3,2}$ [216] | $Z_{9,9,9,9,9,8,8,6,4,3,2,1,1}$ [216] |
| | [6,0,0,2,1,1,0,0,1,3] | [0,6,12,18,26,35,45,55,39,24,26] | $Z_{9,9,9,9,9,9,6,6,5,4,1}$ [128] | $Z_{9,9,9,9,9,9,6,6,5,4,1,1,1}$ [128] |

| | | | | |
|---|---|---|---|---|
| | [6,0,0,3,0,0,0,2,0,2] | [0,6,12,18,27,36,45,54,39,24,26] | $Z_{9,9,9,9,9,9,6,6,6,2,2}$ [60] | $Z_{9,9,9,9,9,9,6,6,6,2,2,1,1}$ [60] |
| | [6,0,1,0,2,0,1,1,0,2] | [0,6,12,19,26,35,44,54,39,24,26] | $Z_{9,9,9,9,9,9,7,5,5,3,2}$ [162] | $Z_{9,9,9,9,9,9,7,5,5,3,2,1,1}$ [162] |
| | [6,1,0,0,0,3,0,1,0,2] | [0,6,13,20,27,34,44,54,39,24,26] | $Z_{9,9,9,9,9,9,8,4,4,4,2}$ [90] | $Z_{9,9,9,9,9,9,8,4,4,4,2,1,1}$ [90] |
| | [6,1,0,0,1,0,3,0,0,2] | [0,6,13,20,27,35,43,54,39,24,26] | $Z_{9,9,9,9,9,9,8,5,3,3,3}$ [96] | $Z_{9,9,9,9,9,9,8,5,3,3,3,1,1}$ [96] |
| | [1,1,4,1,1,0,0,0,0,4] | [2,5,9,17,26,36,46,56,40,24,26] | $Z_{10,10,9,8,7,7,7,7,6,5}$ [96] | $Z_{10,10,9,8,7,7,7,7,6,5,1,1,1,1}$ [96] |
| | [1,6,1,0,0,0,0,1,0,4] | [1,3,11,20,29,38,47,56,40,24,26] | $Z_{10,9,8,8,8,8,8,8,7,2}$ [72] | $Z_{10,9,8,8,8,8,8,8,7,2,1,1,1,1}$ [72] |
| | [2,3,2,0,2,0,0,0,0,4] | [1,4,10,18,26,36,46,56,40,24,26] | $Z_{10,9,9,8,8,8,7,7,5,5}$ [72] | $Z_{10,9,9,8,8,8,7,7,5,5,1,1,1,1}$ [72] |
| | [4,3,1,0,1,1,0,0,0,4] | [0,4,11,19,27,36,46,56,40,24,26] | $Z_{9,9,9,9,8,8,8,7,5,4}$ [120] | $Z_{9,9,9,9,8,8,8,7,5,4,1,1,1,1}$ [120] |
| | [5,0,4,0,0,0,1,0,0,4] | [0,5,10,19,28,37,46,56,40,24,26] | $Z_{9,9,9,9,9,7,7,7,7,3}$ [60] | $Z_{9,9,9,9,9,7,7,7,7,3,1,1,1,1}$ [60] |
| | [5,1,1,1,2,0,0,0,0,4] | [0,5,11,18,26,36,46,56,40,24,26] | $Z_{9,9,9,9,9,8,7,6,5,5}$ [96] | $Z_{9,9,9,9,9,8,7,6,5,5,1,1,1,1}$ [96] |
| | [0,5,0,0,0,0,0,0,8,0] | [3,6,14,22,30,38,46,54,35,24,27] | $Z_{10,10,10,8,8,8,8,8,1,1,1,1,1,1,1,1}$ [13] | $Z_{10,10,10,8,8,8,8,8}$ [14] |
| | [1,4,1,0,0,1,0,0,6,0] | [2,5,12,20,28,36,45,54,36,24,27] | $Z_{10,10,9,8,8,8,8,7,4,1,1,1,1,1,1}$ [80] | $Z_{10,10,9,8,8,8,8,7,4}$ [80] |
| | [2,2,0,3,0,0,0,0,6,0] | [2,6,12,18,27,36,45,54,36,24,27] | $Z_{10,10,9,9,8,8,6,6,6,1,1,1,1,1,1}$ [42] | $Z_{10,10,9,9,8,8,6,6,6}$ [42] |
| | [4,1,2,0,0,1,0,0,6,0] | [1,6,12,20,28,36,45,54,36,24,27] | $Z_{10,9,9,9,9,8,7,7,4,1,1,1,1,1,1}$ [80] | $Z_{10,9,9,9,9,8,7,7,4}$ [80] |
| | [5,0,0,2,1,0,0,0,6,0] | [1,7,13,19,27,36,45,54,36,24,27] | $Z_{10,9,9,9,9,9,6,6,5,1,1,1,1,1,1}$ [48] | $Z_{10,9,9,9,9,9,6,6,5}$ [48] |
| | [7,1,0,0,0,0,0,0,7,1] | [0,7,15,23,31,39,47,55,36,24,27] | $Z_{9,9,9,9,9,9,9,8,1,1,1,1,1,1,1}$ [32] | $Z_{9,9,9,9,9,9,9,8,1}$ [32] |
| | [0,0,0,5,0,1,0,0,4,0] | [4,8,12,16,25,34,44,54,37,24,27] | $Z_{10,10,10,10,6,6,6,6,6,4,1,1,1,1}$ [37] | $Z_{10,10,10,10,6,6,6,6,6,4}$ [38] |
| | [0,3,0,0,4,0,0,0,4,0] | [3,6,12,18,24,34,44,54,37,24,27] | $Z_{10,10,10,8,8,8,5,5,5,5,1,1,1,1}$ [36] | $Z_{10,10,10,8,8,8,5,5,5,5}$ [36] |
| | [0,5,1,1,0,0,0,0,5,1] | [2,4,11,19,28,37,46,55,37,24,27] | $Z_{10,10,8,8,8,8,8,7,6,1,1,1,1,1}$ [72] | $Z_{10,10,8,8,8,8,8,7,6,1}$ [72] |
| | [0,6,0,0,0,1,0,1,4,0] | [2,4,12,20,28,36,45,54,37,24,27] | $Z_{10,10,8,8,8,8,8,8,4,2,1,1,1,1}$ [67] | $Z_{10,10,8,8,8,8,8,8,4,2}$ [68] |
| | [1,0,2,1,3,0,0,0,4,0] | [3,7,11,17,24,34,44,54,37,24,27] | $Z_{10,10,10,9,7,7,6,5,5,5,1,1,1,1}$ [72] | $Z_{10,10,10,9,7,7,6,5,5,5}$ [72] |
| | [1,3,1,1,0,2,0,0,4,0] | [2,5,11,18,26,34,44,54,37,24,27] | $Z_{10,10,9,8,8,8,7,6,4,4,1,1,1,1}$ [120] | $Z_{10,10,9,8,8,8,7,6,4,4}$ [120] |
| | [2,1,1,2,1,1,0,0,4,0] | [2,6,11,17,25,34,44,54,37,24,27] | $Z_{10,10,9,9,8,7,6,6,5,4,1,1,1,1}$ [160] | $Z_{10,10,9,9,8,7,6,6,5,4}$ [160] |
| | [2,5,0,0,1,0,0,0,5,1] | [1,4,12,20,28,37,46,55,37,24,27] | $Z_{10,9,9,8,8,8,8,8,5,1,1,1,1,1}$ [80] | $Z_{10,9,9,8,8,8,8,8,5,1}$ [80] |
| | [3,0,1,0,4,0,0,0,4,0] | [2,7,12,18,24,34,44,54,37,24,27] | $Z_{10,10,9,9,9,7,5,5,5,5,1,1,1,1}$ [54] | $Z_{10,10,9,9,9,7,5,5,5,5}$ [54] |
| | [3,2,1,2,0,0,0,1,4,0] | [1,5,11,18,27,36,45,54,37,24,27] | $Z_{10,9,9,9,8,8,7,6,6,2,1,1,1,1}$ [120] | $Z_{10,9,9,9,8,8,7,6,6,2}$ [120] |
| | [3,2,2,0,0,1,1,0,4,0] | [1,5,11,19,27,35,44,54,37,24,27] | $Z_{10,9,9,9,8,8,7,7,4,3,1,1,1,1}$ [128] | $Z_{10,9,9,9,8,8,7,7,4,3}$ [128] |
| | [3,3,0,0,2,0,1,0,4,0] | [1,5,12,19,26,35,44,54,37,24,27] | $Z_{10,9,9,9,8,8,8,5,5,3,1,1,1,1}$ [96] | $Z_{10,9,9,9,8,8,8,5,5,3}$ [96] |
| | [4,0,2,1,1,0,1,0,4,0] | [1,6,11,18,26,35,44,54,37,24,27] | $Z_{10,9,9,9,9,7,7,6,5,3,1,1,1,1}$ [144] | $Z_{10,9,9,9,9,7,7,6,5,3}$ [144] |
| | [4,1,0,2,0,2,0,0,4,0] | [1,6,12,18,26,34,44,54,37,24,27] | $Z_{10,9,9,9,9,8,6,6,4,4,1,1,1,1}$ [90] | $Z_{10,9,9,9,9,8,6,6,4,4}$ [90] |
| | [5,0,0,0,3,1,0,0,4,0] | [1,7,13,19,25,34,44,54,37,24,27] | $Z_{10,9,9,9,9,9,5,5,5,4,1,1,1,1}$ [50] | $Z_{10,9,9,9,9,9,5,5,5,4}$ [50] |
| | [5,2,1,0,1,0,0,0,5,1] | [0,5,12,20,28,37,46,55,37,24,27] | $Z_{9,9,9,9,9,8,8,7,5,1,1,1,1,1}$ [120] | $Z_{9,9,9,9,9,8,8,7,5,1}$ [120] |
| | [5,3,0,0,0,0,1,1,4,0] | [0,5,13,21,29,37,45,54,37,24,27] | $Z_{9,9,9,9,9,8,8,8,3,2,1,1,1,1}$ [72] | $Z_{9,9,9,9,9,8,8,8,3,2}$ [72] |
| | [6,0,1,2,0,0,0,0,5,1] | [0,6,12,19,28,37,46,55,37,24,27] | $Z_{9,9,9,9,9,9,7,6,6,1,1,1,1,1}$ [72] | $Z_{9,9,9,9,9,9,7,6,6,1}$ [72] |
| | [6,0,2,0,0,1,0,1,4,0] | [0,6,12,20,28,36,45,54,37,24,27] | $Z_{9,9,9,9,9,9,7,7,4,2,1,1,1,1}$ [108] | $Z_{9,9,9,9,9,9,7,7,4,2}$ [108] |
| | [6,1,0,0,2,0,0,1,4,0] | [0,6,13,20,27,36,45,54,37,24,27] | $Z_{9,9,9,9,9,9,8,5,5,2,1,1,1,1}$ [96] | $Z_{9,9,9,9,9,9,8,5,5,2}$ [96] |
| | [6,1,0,1,0,0,2,0,4,0] | [0,6,13,20,28,36,44,54,37,24,27] | $Z_{9,9,9,9,9,9,8,6,3,3,1,1,1,1}$ [96] | $Z_{9,9,9,9,9,9,8,6,3,3}$ [96] |
| | [7,0,0,0,0,2,1,0,4,0] | [0,7,14,21,28,35,44,54,37,24,27] | $Z_{9,9,9,9,9,9,9,4,4,3,1,1,1,1}$ [48] | $Z_{9,9,9,9,9,9,9,4,4,3}$ [48] |
| | [0,1,2,3,0,1,0,1,2,0] | [3,6,10,16,25,34,44,54,38,24,27] | $Z_{10,10,10,8,7,7,6,6,6,4,2,1,1}$ [162] | $Z_{10,10,10,8,7,7,6,6,6,4,2}$ [162] |
| | [0,1,3,0,3,0,0,1,2,0] | [3,6,10,17,24,34,44,54,38,24,27] | $Z_{10,10,10,8,7,7,7,5,5,5,2,1,1}$ [108] | $Z_{10,10,10,8,7,7,7,5,5,5,2}$ [108] |
| | [0,1,3,1,0,2,1,0,2,0] | [3,6,10,17,25,33,43,54,38,24,27] | $Z_{10,10,10,8,7,7,7,6,4,4,3,1,1}$ [144] | $Z_{10,10,10,8,7,7,7,6,4,4,3}$ [144] |
| | [0,2,0,3,2,0,0,1,2,0] | [3,6,11,16,24,34,44,54,38,24,27] | $Z_{10,10,10,8,8,6,6,6,5,5,2,1,1}$ [108] | $Z_{10,10,10,8,8,6,6,6,5,5,2}$ [108] |
| | [0,3,0,0,2,3,0,0,2,0] | [3,6,12,18,24,32,43,54,38,24,27] | $Z_{10,10,10,8,8,8,5,5,4,4,4,1,1}$ [60] | $Z_{10,10,10,8,8,8,5,5,4,4,4}$ [60] |
| | [0,4,2,0,1,1,0,0,3,1] | [2,4,10,18,26,35,45,55,38,24,27] | $Z_{10,10,8,8,8,8,7,7,5,4,1,1,1}$ [144] | $Z_{10,10,8,8,8,8,7,7,5,4,1}$ [144] |
| | [0,4,2,1,0,0,0,2,2,0] | [2,4,10,18,27,36,45,54,38,24,27] | $Z_{10,10,8,8,8,8,7,7,6,2,2,1,1}$ [90] | $Z_{10,10,8,8,8,8,7,7,6,2,2}$ [90] |
| | [0,5,0,1,1,0,1,1,2,0] | [2,4,11,18,26,35,44,54,38,24,27] | $Z_{10,10,8,8,8,8,8,6,5,3,2,1,1}$ [162] | $Z_{10,10,8,8,8,8,8,6,5,3,2}$ [162] |
| | [1,0,1,3,1,1,1,0,2,0] | [3,7,11,16,24,33,43,54,38,24,27] | $Z_{10,10,10,9,7,6,6,6,5,4,3,1,1}$ [192] | $Z_{10,10,10,9,7,6,6,6,5,4,3}$ [192] |
| | [1,0,2,1,1,3,0,0,2,0] | [3,7,11,17,24,32,43,54,38,24,27] | $Z_{10,10,10,9,7,7,6,5,4,4,4,1,1}$ [120] | $Z_{10,10,10,9,7,7,6,5,4,4,4}$ [120] |
| | [1,2,2,1,1,1,0,1,2,0] | [2,5,10,17,25,34,44,54,38,24,27] | $Z_{10,10,9,8,8,7,7,6,5,4,2,1,1}$ [288] | $Z_{10,10,9,8,8,7,7,6,5,4,2}$ [288] |
| | [1,2,3,0,0,1,2,0,2,0] | [2,5,10,18,26,34,43,54,38,24,27] | $Z_{10,10,9,8,8,7,7,7,4,3,3,1,1}$ [128] | $Z_{10,10,9,8,8,7,7,7,4,3,3}$ [128] |
| | [1,3,0,2,1,0,2,0,2,0] | [2,5,11,17,25,34,43,54,38,24,27] | $Z_{10,10,9,8,8,8,6,6,5,3,3,1,1}$ [144] | $Z_{10,10,9,8,8,8,6,6,5,3,3}$ [144] |
| | [1,3,1,0,1,2,1,0,2,0] | [2,5,11,18,25,33,43,54,38,24,27] | $Z_{10,10,9,8,8,8,7,5,4,4,3,1,1}$ [192] | $Z_{10,10,9,8,8,8,7,5,4,4,3}$ [192] |
| | [2,0,2,3,1,0,0,0,3,1] | [2,6,10,16,25,35,45,55,38,24,27] | $Z_{10,10,9,9,7,7,6,6,6,5,1,1,1}$ [120] | $Z_{10,10,9,9,7,7,6,6,6,5,1}$ [120] |
| | [2,0,3,1,1,0,2,0,2,0] | [2,6,10,17,25,34,43,54,38,24,27] | $Z_{10,10,9,9,7,7,7,6,5,3,3,1,1}$ [144] | $Z_{10,10,9,9,7,7,7,6,5,3,3}$ [144] |
| | [2,1,0,4,0,1,0,1,2,0] | [2,6,11,16,25,34,44,54,38,24,27] | $Z_{10,10,9,9,8,6,6,6,6,4,2,1,1}$ [162] | $Z_{10,10,9,9,8,6,6,6,6,4,2}$ [162] |
| | [2,1,1,1,2,1,1,0,2,0] | [2,6,11,17,24,33,43,54,38,24,27] | $Z_{10,10,9,9,8,7,6,5,5,4,3,1,1}$ [256] | $Z_{10,10,9,9,8,7,6,5,5,4,3}$ [256] |
| | [2,2,0,1,0,4,0,0,2,0] | [2,6,12,18,25,32,43,54,38,24,27] | $Z_{10,10,9,9,8,8,6,4,4,4,4,1,1}$ [90] | $Z_{10,10,9,9,8,8,6,4,4,4,4}$ [90] |
| | [2,3,2,1,0,0,1,0,3,1] | [1,4,10,18,27,36,45,55,38,24,27] | $Z_{10,9,9,8,8,8,7,7,6,3,1,1,1}$ [192] | $Z_{10,9,9,8,8,8,7,7,6,3,1}$ [192] |
| | [2,4,0,1,1,1,0,0,3,1] | [1,4,11,18,26,35,45,55,38,24,27] | $Z_{10,9,9,8,8,8,8,6,5,4,1,1,1}$ [192] | $Z_{10,9,9,8,8,8,8,6,5,4,1}$ [192] |
| | [2,4,1,0,0,1,1,1,2,0] | [1,4,11,19,27,35,44,54,38,24,27] | $Z_{10,9,9,8,8,8,8,7,4,3,2,1,1}$ [192] | $Z_{10,9,9,8,8,8,8,7,4,3,2}$ [192] |
| | [3,0,1,0,2,3,0,0,2,0] | [2,7,12,18,24,32,43,54,38,24,27] | $Z_{10,10,9,9,9,7,5,5,4,4,4,1,1}$ [90] | $Z_{10,10,9,9,9,7,5,5,4,4,4}$ [90] |
| | [3,1,2,2,0,1,0,0,3,1] | [1,5,10,17,26,35,45,55,38,24,27] | $Z_{10,9,9,9,8,7,7,6,6,4,1,1,1}$ [192] | $Z_{10,9,9,9,8,7,7,6,6,4,1}$ [192] |
| | [3,1,3,0,1,0,1,1,2,0] | [1,5,10,18,26,35,44,54,38,24,27] | $Z_{10,9,9,9,8,7,7,7,5,3,2,1,1}$ [216] | $Z_{10,9,9,9,8,7,7,7,5,3,2}$ [216] |
| | [3,2,0,2,2,0,0,0,3,1] | [1,5,11,17,25,35,45,55,38,24,27] | $Z_{10,9,9,9,8,8,6,6,5,5,1,1,1}$ [120] | $Z_{10,9,9,9,8,8,6,6,5,5,1}$ [120] |
| | [3,2,0,3,0,0,1,1,2,0] | [1,5,11,17,26,35,44,54,38,24,27] | $Z_{10,9,9,9,8,8,6,6,6,3,2,1,1}$ [144] | $Z_{10,9,9,9,8,8,6,6,6,3,2}$ [144] |
| | [3,2,1,0,2,1,0,1,2,0] | [1,5,11,18,25,34,44,54,38,24,27] | $Z_{10,9,9,9,8,8,7,5,5,4,2,1,1}$ [216] | $Z_{10,9,9,9,8,8,7,5,5,4,2}$ [216] |
| | [3,2,1,1,0,1,2,0,2,0] | [1,5,11,18,26,34,43,54,38,24,27] | $Z_{10,9,9,9,8,8,7,6,4,3,3,1,1}$ [192] | $Z_{10,9,9,9,8,8,7,6,4,3,3}$ [192] |
| | [4,0,1,2,1,1,0,1,2,0] | [1,6,11,17,25,34,44,54,38,24,27] | $Z_{10,9,9,9,9,7,6,6,5,4,2,1,1}$ [216] | $Z_{10,9,9,9,9,7,6,6,5,4,2}$ [216] |
| | [4,1,0,1,1,2,1,0,2,0] | [1,6,12,18,25,33,43,54,38,24,27] | $Z_{10,9,9,9,9,8,6,5,4,4,3,1,1}$ [192] | $Z_{10,9,9,9,9,8,6,5,4,4,3}$ [192] |
| | [4,3,1,1,0,0,0,1,3,1] | [0,4,11,19,28,37,46,55,38,24,27] | $Z_{9,9,9,9,8,8,8,7,6,2,1,1,1}$ [160] | $Z_{9,9,9,9,8,8,8,7,6,2,1}$ [160] |
| | [4,4,0,0,0,1,1,0,3,1] | [0,4,12,20,28,36,45,55,38,24,27] | $Z_{9,9,9,9,8,8,8,8,4,3,1,1,1}$ [120] | $Z_{9,9,9,9,8,8,8,8,4,3,1}$ [120] |

| | | | | |
|---|---|---|---|---|
| | [5,1,1,2,0,0,1,0,3,1] | [0,5,11,18,27,36,45,55,38,24,27] | $Z_{9,9,9,9,9,8,7,6,6,3,1,1,1}$ [192] | $Z_{9,9,9,9,9,8,7,6,6,3,1}$ [192] |
| | [5,1,2,0,0,2,0,0,3,1] | [0,5,11,19,27,35,45,55,38,24,27] | $Z_{9,9,9,9,9,8,7,7,4,4,1,1,1}$ [128] | $Z_{9,9,9,9,9,8,7,7,4,4,1}$ [128] |
| | [5,1,2,0,1,0,0,2,2,0] | [0,5,11,19,27,36,45,54,38,24,27] | $Z_{9,9,9,9,9,8,7,7,5,2,2,1,1}$ [144] | $Z_{9,9,9,9,9,8,7,7,5,2,2}$ [144] |
| | [5,2,0,0,2,1,0,0,3,1] | [0,5,12,19,26,35,45,55,38,24,27] | $Z_{9,9,9,9,9,8,8,5,5,4,1,1,1}$ [128] | $Z_{9,9,9,9,9,8,8,5,5,4,1}$ [128] |
| | [5,2,0,1,0,1,1,1,2,0] | [0,5,12,19,27,35,44,54,38,24,27] | $Z_{9,9,9,9,9,8,8,6,4,3,2,1,1}$ [216] | $Z_{9,9,9,9,9,8,8,6,4,3,2}$ [216] |
| | [6,0,0,2,1,1,0,0,3,1] | [0,6,12,18,26,35,45,55,38,24,27] | $Z_{9,9,9,9,9,9,6,6,5,4,1,1,1}$ [128] | $Z_{9,9,9,9,9,9,6,6,5,4,1}$ [128] |
| | [6,0,0,3,0,0,0,2,2,0] | [0,6,12,18,27,36,45,54,38,24,27] | $Z_{9,9,9,9,9,9,6,6,6,2,2,1,1}$ [60] | $Z_{9,9,9,9,9,9,6,6,6,2,2}$ [60] |
| | [6,0,1,0,2,0,1,1,2,0] | [0,6,12,19,26,35,44,54,38,24,27] | $Z_{9,9,9,9,9,9,7,5,5,3,2,1,1}$ [162] | $Z_{9,9,9,9,9,9,7,5,5,3,2}$ [162] |
| | [6,1,0,0,0,3,0,1,2,0] | [0,6,13,20,27,34,44,54,38,24,27] | $Z_{9,9,9,9,9,9,8,4,4,4,2,1,1}$ [90] | $Z_{9,9,9,9,9,9,8,4,4,4,2}$ [90] |
| | [6,1,0,0,1,0,3,0,2,0] | [0,6,13,20,27,35,43,54,38,24,27] | $Z_{9,9,9,9,9,9,8,5,3,3,3,1,1}$ [96] | $Z_{9,9,9,9,9,9,8,5,3,3,3}$ [96] |
| | [0,1,1,5,0,0,1,0,0,2] | [3,6,10,15,25,35,45,56,40,24,27] | $Z_{10,10,10,8,7,6,6,6,6,6,3}$ [96] | $Z_{10,10,10,8,7,6,6,6,6,6,3,1,1}$ [96] |
| | [0,3,3,1,0,1,1,0,0,2] | [2,4,9,17,26,35,45,56,40,24,27] | $Z_{10,10,8,8,8,7,7,7,6,4,3}$ [144] | $Z_{10,10,8,8,8,7,7,7,6,4,3,1,1}$ [144] |
| | [0,4,1,1,1,2,0,0,0,2] | [2,4,10,17,25,34,45,56,40,24,27] | $Z_{10,10,8,8,8,8,7,6,5,4,4}$ [120] | $Z_{10,10,8,8,8,8,7,6,5,4,4,1,1}$ [120] |
| | [1,0,0,5,1,1,0,0,0,2] | [3,7,11,15,24,34,45,56,40,24,27] | $Z_{10,10,10,9,6,6,6,6,6,5,4}$ [80] | $Z_{10,10,10,9,6,6,6,6,6,5,4,1,1}$ [80] |
| | [1,1,3,2,1,0,1,0,0,2] | [2,5,9,16,25,35,45,56,40,24,27] | $Z_{10,10,9,8,7,7,7,6,6,5,3}$ [192] | $Z_{10,10,9,8,7,7,7,6,6,5,3,1,1}$ [192] |
| | [1,1,4,0,1,2,0,0,0,2] | [2,5,9,17,25,34,45,56,40,24,27] | $Z_{10,10,9,8,7,7,7,7,5,4,4}$ [120] | $Z_{10,10,9,8,7,7,7,7,5,4,4,1,1}$ [120] |
| | [1,2,1,2,2,1,0,0,0,2] | [2,5,10,16,24,34,45,56,40,24,27] | $Z_{10,10,9,8,8,7,6,6,5,5,4}$ [160] | $Z_{10,10,9,8,8,7,6,6,5,5,4,1,1}$ [160] |
| | [1,5,1,1,0,1,0,1,0,2] | [1,3,10,18,27,36,46,56,40,24,27] | $Z_{10,9,8,8,8,8,8,7,6,4,2}$ [216] | $Z_{10,9,8,8,8,8,8,7,6,4,2,1,1}$ [216] |
| | [1,6,0,0,1,0,2,0,0,2] | [1,3,11,19,27,36,45,56,40,24,27] | $Z_{10,9,8,8,8,8,8,8,5,3,3}$ [96] | $Z_{10,9,8,8,8,8,8,8,5,3,3,1,1}$ [96] |
| | [2,2,3,1,1,0,0,1,0,2] | [1,4,9,17,26,36,46,56,40,24,27] | $Z_{10,9,9,8,8,7,7,7,6,5,2}$ [192] | $Z_{10,9,9,8,8,7,7,7,6,5,2,1,1}$ [192] |
| | [2,3,1,1,2,0,1,0,0,2] | [1,4,10,17,25,35,45,56,40,24,27] | $Z_{10,9,9,8,8,8,7,6,5,5,3}$ [192] | $Z_{10,9,9,8,8,8,7,6,5,5,3,1,1}$ [192] |
| | [2,3,2,0,0,3,0,0,0,2] | [1,4,10,18,26,34,45,56,40,24,27] | $Z_{10,9,9,8,8,8,7,7,4,4,4}$ [80] | $Z_{10,9,9,8,8,8,7,7,4,4,4,1,1}$ [80] |
| | [3,0,4,1,0,1,1,0,0,2] | [1,5,9,17,26,35,45,56,40,24,27] | $Z_{10,9,9,9,7,7,7,7,6,4,3}$ [144] | $Z_{10,9,9,9,7,7,7,7,6,4,3,1,1}$ [144] |
| | [3,1,1,3,1,0,1,0,0,2] | [1,5,10,16,25,35,45,56,40,24,27] | $Z_{10,9,9,9,8,7,6,6,6,5,3}$ [192] | $Z_{10,9,9,9,8,7,6,6,6,5,3,1,1}$ [192] |
| | [3,2,0,1,3,1,0,0,0,2] | [1,5,11,17,24,34,45,56,40,24,27] | $Z_{10,9,9,9,8,8,6,5,5,5,4}$ [120] | $Z_{10,9,9,9,8,8,6,5,5,5,4,1,1}$ [120] |
| | [3,4,2,0,0,1,0,0,1,3] | [0,3,10,19,28,37,47,57,40,24,27] | $Z_{9,9,9,8,8,8,8,7,7,4,1}$ [128] | $Z_{9,9,9,8,8,8,8,7,7,4,1,1,1}$ [128] |
| | [3,5,0,0,2,0,0,0,1,3] | [0,3,11,19,27,37,47,57,40,24,27] | $Z_{9,9,9,8,8,8,8,8,5,5,1}$ [80] | $Z_{9,9,9,8,8,8,8,8,5,5,1,1,1}$ [80] |
| | [3,5,0,1,0,0,1,1,0,2] | [0,3,11,19,28,37,46,56,40,24,27] | $Z_{9,9,9,8,8,8,8,8,6,3,2}$ [144] | $Z_{9,9,9,8,8,8,8,8,6,3,2,1,1}$ [144] |
| | [4,2,1,3,0,0,0,0,1,3] | [0,4,10,17,27,37,47,57,40,24,27] | $Z_{9,9,9,9,8,8,7,6,6,6,1}$ [96] | $Z_{9,9,9,9,8,8,7,6,6,6,1,1,1}$ [96] |
| | [4,2,2,0,2,0,0,1,0,2] | [0,4,10,18,26,36,46,56,40,24,27] | $Z_{9,9,9,9,8,8,7,7,5,5,2}$ [144] | $Z_{9,9,9,9,8,8,7,7,5,5,2,1,1}$ [144] |
| | [4,2,2,1,0,0,2,0,0,2] | [0,4,10,18,27,36,45,56,40,24,27] | $Z_{9,9,9,9,8,8,7,7,6,3,3}$ [128] | $Z_{9,9,9,9,8,8,7,7,6,3,3,1,1}$ [128] |
| | [4,3,0,1,1,1,1,0,0,2] | [0,4,11,18,26,35,45,56,40,24,27] | $Z_{9,9,9,9,8,8,8,6,5,4,3}$ [192] | $Z_{9,9,9,9,8,8,8,6,5,4,3,1,1}$ [192] |
| | [5,0,2,2,1,0,0,1,0,2] | [0,5,10,17,26,36,46,56,40,24,27] | $Z_{9,9,9,9,9,7,7,6,6,5,2}$ [144] | $Z_{9,9,9,9,9,7,7,6,6,5,2,1,1}$ [144] |
| | [5,0,3,0,1,1,1,0,0,2] | [0,5,10,18,26,35,45,56,40,24,27] | $Z_{9,9,9,9,9,7,7,7,5,4,3}$ [144] | $Z_{9,9,9,9,9,7,7,7,5,4,3,1,1}$ [144] |
| | [5,1,0,3,0,1,1,0,0,2] | [0,5,11,17,26,35,45,56,40,24,27] | $Z_{9,9,9,9,9,8,6,6,6,4,3}$ [144] | $Z_{9,9,9,9,9,8,6,6,6,4,3,1,1}$ [144] |
| | [5,1,1,0,3,0,1,0,0,2] | [0,5,11,18,25,35,45,56,40,24,27] | $Z_{9,9,9,9,9,8,7,5,5,5,3}$ [144] | $Z_{9,9,9,9,9,8,7,5,5,5,3,1,1}$ [144] |
| | [5,1,1,1,0,3,0,0,0,2] | [0,5,11,18,26,34,45,56,40,24,27] | $Z_{9,9,9,9,9,8,7,6,4,4,4}$ [120] | $Z_{9,9,9,9,9,8,7,6,4,4,4,1,1}$ [120] |
| | [6,0,0,1,2,2,0,0,0,2] | [0,6,12,18,25,34,45,56,40,24,27] | $Z_{9,9,9,9,9,9,6,5,5,4,4}$ [80] | $Z_{9,9,9,9,9,9,6,5,5,4,4,1,1}$ [80] |
| | [1,0,7,0,0,0,0,0,0,4] | [2,5,8,18,28,38,48,58,41,24,27] | $Z_{10,10,9,7,7,7,7,7,7,7}$ [24] | $Z_{10,10,9,7,7,7,7,7,7,7,1,1,1,1}$ [24] |
| | [1,4,3,1,0,0,0,0,0,4] | [1,3,9,18,28,38,48,58,41,24,27] | $Z_{10,9,8,8,8,8,7,7,7,6}$ [56] | $Z_{10,9,8,8,8,8,7,7,7,6,1,1,1,1}$ [56] |
| | [3,4,1,2,0,0,0,0,0,4] | [0,3,10,18,28,38,48,58,41,24,27] | $Z_{9,9,9,8,8,8,8,7,6,6}$ [56] | $Z_{9,9,9,8,8,8,8,7,6,6,1,1,1,1}$ [56] |
| | [4,1,4,1,0,0,0,0,0,4] | [0,4,9,18,28,38,48,58,41,24,27] | $Z_{9,9,9,9,8,7,7,7,7,6}$ [56] | $Z_{9,9,9,9,8,7,7,7,7,6,1,1,1,1}$ [56] |
| | [2,4,2,0,0,0,0,0,6,0] | [1,4,11,20,29,38,47,56,37,24,28] | $Z_{10,9,9,8,8,8,8,7,7,1,1,1,1,1,1}$ [32] | $Z_{10,9,9,8,8,8,8,7,7}$ [32] |
| | [0,4,1,2,1,0,0,0,4,0] | [2,4,10,17,26,36,46,56,38,24,28] | $Z_{10,10,8,8,8,8,7,6,6,5,1,1,1,1}$ [72] | $Z_{10,10,8,8,8,8,7,6,6,5}$ [72] |
| | [1,2,1,4,0,0,0,0,4,0] | [2,5,10,16,26,36,46,56,38,24,28] | $Z_{10,10,9,8,8,7,6,6,6,6,1,1,1,1}$ [56] | $Z_{10,10,9,8,8,7,6,6,6,6}$ [56] |
| | [1,6,1,0,0,0,0,1,4,0] | [1,3,11,20,29,38,47,56,38,24,28] | $Z_{10,9,8,8,8,8,8,8,7,2,1,1,1,1}$ [72] | $Z_{10,9,8,8,8,8,8,8,7,2}$ [72] |
| | [2,3,2,0,2,0,0,0,4,0] | [1,4,10,18,26,36,46,56,38,24,28] | $Z_{10,9,9,8,8,8,7,7,5,5,1,1,1,1}$ [72] | $Z_{10,9,9,8,8,8,7,7,5,5}$ [72] |
| | [4,3,1,0,1,1,0,0,4,0] | [0,4,11,19,27,36,46,56,38,24,28] | $Z_{9,9,9,9,8,8,8,7,5,4,1,1,1,1}$ [120] | $Z_{9,9,9,9,8,8,8,7,5,4}$ [120] |
| | [5,0,4,0,0,0,1,0,4,0] | [0,5,10,19,28,37,46,56,38,24,28] | $Z_{9,9,9,9,9,7,7,7,7,3,1,1,1,1}$ [60] | $Z_{9,9,9,9,9,7,7,7,7,3}$ [60] |
| | [5,1,1,1,2,0,0,0,4,0] | [0,5,11,18,26,36,46,56,38,24,28] | $Z_{9,9,9,9,9,8,7,6,5,5,1,1,1,1}$ [96] | $Z_{9,9,9,9,9,8,7,6,5,5}$ [96] |
| | [0,0,4,2,0,2,0,0,2,0] | [3,6,9,16,25,34,45,56,39,24,28] | $Z_{10,10,10,7,7,7,7,6,6,4,4,1,1}$ [60] | $Z_{10,10,10,7,7,7,7,6,6,4,4}$ [60] |
| | [0,1,1,5,0,0,1,0,2,0] | [3,6,10,15,25,35,45,56,39,24,28] | $Z_{10,10,10,8,7,6,6,6,6,6,3,1,1}$ [96] | $Z_{10,10,10,8,7,6,6,6,6,6,3}$ [96] |
| | [0,3,3,1,0,1,1,0,2,0] | [2,4,9,17,26,35,45,56,39,24,28] | $Z_{10,10,8,8,8,7,7,7,6,4,3,1,1}$ [144] | $Z_{10,10,8,8,8,7,7,7,6,4,3}$ [144] |
| | [0,4,0,4,0,0,0,1,2,0] | [2,4,10,16,26,36,46,56,39,24,28] | $Z_{10,10,8,8,8,8,6,6,6,6,2,1,1}$ [67] | $Z_{10,10,8,8,8,8,6,6,6,6,2}$ [68] |
| | [0,4,1,1,1,2,0,0,2,0] | [2,4,10,17,25,34,45,56,39,24,28] | $Z_{10,10,8,8,8,8,7,6,5,4,4,1,1}$ [120] | $Z_{10,10,8,8,8,8,7,6,5,4,4}$ [120] |
| | [1,0,0,5,1,1,0,0,2,0] | [3,7,11,15,24,34,45,56,39,24,28] | $Z_{10,10,10,9,6,6,6,6,6,5,4,1,1}$ [80] | $Z_{10,10,10,9,6,6,6,6,6,5,4}$ [80] |
| | [1,1,3,2,1,0,1,0,2,0] | [2,5,9,16,25,35,45,56,39,24,28] | $Z_{10,10,9,8,7,7,7,6,6,5,3,1,1}$ [192] | $Z_{10,10,9,8,7,7,7,6,6,5,3}$ [192] |
| | [1,1,4,0,1,2,0,0,2,0] | [2,5,9,17,25,34,45,56,39,24,28] | $Z_{10,10,9,8,7,7,7,7,5,4,4,1,1}$ [120] | $Z_{10,10,9,8,7,7,7,7,5,4,4}$ [120] |
| | [1,2,1,2,2,1,0,0,2,0] | [2,5,10,16,24,34,45,56,39,24,28] | $Z_{10,10,9,8,8,7,6,6,5,5,4,1,1}$ [160] | $Z_{10,10,9,8,8,7,6,6,5,5,4}$ [160] |
| | [1,5,1,1,0,1,0,1,2,0] | [1,3,10,18,27,36,46,56,39,24,28] | $Z_{10,9,8,8,8,8,8,7,6,4,2,1,1}$ [216] | $Z_{10,9,8,8,8,8,8,7,6,4,2}$ [216] |
| | [1,6,0,0,1,0,2,0,2,0] | [1,3,11,19,27,36,45,56,39,24,28] | $Z_{10,9,8,8,8,8,8,8,5,3,3,1,1}$ [96] | $Z_{10,9,8,8,8,8,8,8,5,3,3}$ [96] |
| | [2,2,3,1,1,0,0,1,2,0] | [1,4,9,17,26,36,46,56,39,24,28] | $Z_{10,9,9,8,8,7,7,7,6,5,2,1,1}$ [192] | $Z_{10,9,9,8,8,7,7,7,6,5,2}$ [192] |
| | [2,2,4,0,0,0,2,0,2,0] | [1,4,9,18,27,36,45,56,39,24,28] | $Z_{10,9,9,8,8,7,7,7,7,3,3,1,1}$ [80] | $Z_{10,9,9,8,8,7,7,7,7,3,3}$ [80] |
| | [2,3,1,1,2,0,1,0,2,0] | [1,4,10,17,25,35,45,56,39,24,28] | $Z_{10,9,9,8,8,8,7,6,5,5,3,1,1}$ [192] | $Z_{10,9,9,8,8,8,7,6,5,5,3}$ [192] |
| | [2,3,2,0,0,3,0,0,2,0] | [1,4,10,18,26,34,45,56,39,24,28] | $Z_{10,9,9,8,8,8,7,7,4,4,4,1,1}$ [80] | $Z_{10,9,9,8,8,8,7,7,4,4,4}$ [80] |
| | [2,4,0,0,2,2,0,0,2,0] | [1,4,11,18,25,34,45,56,39,24,28] | $Z_{10,9,9,8,8,8,8,5,5,4,4,1,1}$ [80] | $Z_{10,9,9,8,8,8,8,5,5,4,4}$ [80] |
| | [3,0,4,1,0,1,1,0,2,0] | [1,5,9,17,26,35,45,56,39,24,28] | $Z_{10,9,9,9,7,7,7,7,6,4,3,1,1}$ [144] | $Z_{10,9,9,9,7,7,7,7,6,4,3}$ [144] |
| | [3,1,1,3,1,0,1,0,2,0] | [1,5,10,16,25,35,45,56,39,24,28] | $Z_{10,9,9,9,8,7,6,6,6,5,3,1,1}$ [192] | $Z_{10,9,9,9,8,7,6,6,6,5,3}$ [192] |
| | [3,2,0,1,3,1,0,0,2,0] | [1,5,11,17,24,34,45,56,39,24,28] | $Z_{10,9,9,9,8,8,6,5,5,5,4,1,1}$ [120] | $Z_{10,9,9,9,8,8,6,5,5,5,4}$ [120] |
| | [3,4,2,0,0,1,0,0,3,1] | [0,3,10,19,28,37,47,57,39,24,28] | $Z_{9,9,9,8,8,8,8,7,7,4,1,1,1}$ [128] | $Z_{9,9,9,8,8,8,8,7,7,4,1}$ [128] |
| | [3,5,0,0,2,0,0,0,3,1] | [0,3,11,19,27,37,47,57,39,24,28] | $Z_{9,9,9,8,8,8,8,8,5,5,1,1,1}$ [80] | $Z_{9,9,9,8,8,8,8,8,5,5,1}$ [80] |

| | | | | |
|---|---|---|---|---|
| | [3,5,0,1,0,0,1,1,2,0] | [0,3,11,19,28,37,46,56,39,24,28] | $Z_{9,9,9,8,8,8,8,8,6,3,2,1,1}$ [144] | $Z_{9,9,9,8,8,8,8,8,6,3,2}$ [144] |
| | [4,0,0,4,0,2,0,0,2,0] | [1,6,11,16,25,34,45,56,39,24,28] | $Z_{10,9,9,9,9,6,6,6,6,4,4,1,1}$ [60] | $Z_{10,9,9,9,9,6,6,6,6,4,4}$ [60] |
| | [4,2,1,3,0,0,0,0,3,1] | [0,4,10,17,27,37,47,57,39,24,28] | $Z_{9,9,9,9,8,8,7,6,6,6,1,1,1}$ [96] | $Z_{9,9,9,9,8,8,7,6,6,6,1}$ [96] |
| | [4,2,2,0,2,0,0,1,2,0] | [0,4,10,18,26,36,46,56,39,24,28] | $Z_{9,9,9,9,8,8,7,7,5,5,2,1,1}$ [144] | $Z_{9,9,9,9,8,8,7,7,5,5,2}$ [144] |
| | [4,2,2,1,0,0,2,0,2,0] | [0,4,10,18,27,36,45,56,39,24,28] | $Z_{9,9,9,9,8,8,7,7,6,3,3,1,1}$ [128] | $Z_{9,9,9,9,8,8,7,7,6,3,3}$ [128] |
| | [4,3,0,1,1,1,1,0,2,0] | [0,4,11,18,26,35,45,56,39,24,28] | $Z_{9,9,9,9,8,8,8,6,5,4,3,1,1}$ [192] | $Z_{9,9,9,9,8,8,8,6,5,4,3}$ [192] |
| | [5,0,2,2,1,0,0,1,2,0] | [0,5,10,17,26,36,46,56,39,24,28] | $Z_{9,9,9,9,9,7,7,6,6,5,2,1,1}$ [144] | $Z_{9,9,9,9,9,7,7,6,6,5,2}$ [144] |
| | [5,0,3,0,1,1,1,0,2,0] | [0,5,10,18,26,35,45,56,39,24,28] | $Z_{9,9,9,9,9,7,7,7,5,4,3,1,1}$ [144] | $Z_{9,9,9,9,9,7,7,7,5,4,3}$ [144] |
| | [5,1,0,3,0,1,1,0,2,0] | [0,5,11,17,26,35,45,56,39,24,28] | $Z_{9,9,9,9,9,8,6,6,6,4,3,1,1}$ [144] | $Z_{9,9,9,9,9,8,6,6,6,4,3}$ [144] |
| | [5,1,1,0,3,0,1,0,2,0] | [0,5,11,18,25,35,45,56,39,24,28] | $Z_{9,9,9,9,9,8,7,5,5,5,3,1,1}$ [144] | $Z_{9,9,9,9,9,8,7,5,5,5,3}$ [144] |
| | [5,1,1,1,0,3,0,0,2,0] | [0,5,11,18,26,34,45,56,39,24,28] | $Z_{9,9,9,9,9,8,7,6,4,4,4,1,1}$ [120] | $Z_{9,9,9,9,9,8,7,6,4,4,4}$ [120] |
| | [6,0,0,1,2,2,0,0,2,0] | [0,6,12,18,25,34,45,56,39,24,28] | $Z_{9,9,9,9,9,9,6,5,5,4,4,1,1}$ [80] | $Z_{9,9,9,9,9,9,6,5,5,4,4}$ [80] |
| | [0,2,5,0,1,1,0,0,0,2] | [2,4,8,17,26,36,47,58,41,24,28] | $Z_{10,10,8,8,7,7,7,7,7,5,4}$ [90] | $Z_{10,10,8,8,7,7,7,7,7,5,4,1,1}$ [90] |
| | [0,7,1,0,1,0,0,1,0,2] | [1,2,10,19,28,38,48,58,41,24,28] | $Z_{10,8,8,8,8,8,8,8,7,5,2}$ [108] | $Z_{10,8,8,8,8,8,8,8,7,5,2,1,1}$ [108] |
| | [0,8,0,0,0,0,2,0,0,2] | [1,2,11,20,29,38,47,58,41,24,28] | $Z_{10,8,8,8,8,8,8,8,8,3,3}$ [36] | $Z_{10,8,8,8,8,8,8,8,8,3,3,1,1}$ [36] |
| | [1,0,5,2,0,1,0,0,0,2] | [2,5,8,16,26,36,47,58,41,24,28] | $Z_{10,10,9,7,7,7,7,7,6,6,4}$ [90] | $Z_{10,10,9,7,7,7,7,7,6,6,4,1,1}$ [90] |
| | [1,1,2,4,1,0,0,0,0,2] | [2,5,9,15,25,36,47,58,41,24,28] | $Z_{10,10,9,8,7,7,6,6,6,6,5}$ [96] | $Z_{10,10,9,8,7,7,6,6,6,6,5,1,1}$ [96] |
| | [1,4,2,1,1,1,0,0,0,2] | [1,3,9,17,26,36,47,58,41,24,28] | $Z_{10,9,8,8,8,8,7,7,6,5,4}$ [160] | $Z_{10,9,8,8,8,8,7,7,6,5,4,1,1}$ [160] |
| | [2,1,5,1,0,0,1,0,0,2] | [1,4,8,17,27,37,47,58,41,24,28] | $Z_{10,9,9,8,7,7,7,7,7,6,3}$ [128] | $Z_{10,9,9,8,7,7,7,7,7,6,3,1,1}$ [128] |
| | [2,2,2,2,2,0,0,0,0,2] | [1,4,9,16,25,36,47,58,41,24,28] | $Z_{10,9,9,8,8,7,7,6,6,5,5}$ [96] | $Z_{10,9,9,8,8,7,7,6,6,5,5,1,1}$ [96] |
| | [2,6,1,1,0,0,0,0,1,3] | [0,2,10,19,29,39,49,59,41,24,28] | $Z_{9,9,8,8,8,8,8,8,7,6,1}$ [96] | $Z_{9,9,8,8,8,8,8,8,7,6,1,1,1}$ [96] |
| | [2,7,0,0,0,1,0,1,0,2] | [0,2,11,20,29,38,48,58,41,24,28] | $Z_{9,9,8,8,8,8,8,8,8,4,2}$ [90] | $Z_{9,9,8,8,8,8,8,8,8,4,2,1,1}$ [90] |
| | [3,3,3,0,1,0,1,0,0,2] | [0,3,9,18,27,37,47,58,41,24,28] | $Z_{9,9,9,8,8,8,7,7,7,5,3}$ [144] | $Z_{9,9,9,8,8,8,7,7,7,5,3,1,1}$ [144] |
| | [3,4,0,3,0,0,1,0,0,2] | [0,3,10,17,27,37,47,58,41,24,28] | $Z_{9,9,9,8,8,8,8,6,6,6,3}$ [96] | $Z_{9,9,9,8,8,8,8,6,6,6,3,1,1}$ [96] |
| | [3,4,1,0,2,1,0,0,0,2] | [0,3,10,18,26,36,47,58,41,24,28] | $Z_{9,9,9,8,8,8,8,7,5,5,4}$ [120] | $Z_{9,9,9,8,8,8,8,7,5,5,4,1,1}$ [120] |
| | [4,1,3,1,1,1,0,0,0,2] | [0,4,9,17,26,36,47,58,41,24,28] | $Z_{9,9,9,9,8,7,7,7,6,5,4}$ [160] | $Z_{9,9,9,9,8,7,7,7,6,5,4,1,1}$ [160] |
| | [4,2,1,1,3,0,0,0,0,2] | [0,4,10,17,25,36,47,58,41,24,28] | $Z_{9,9,9,9,8,8,7,6,5,5,5}$ [96] | $Z_{9,9,9,9,8,8,7,6,5,5,5,1,1}$ [96] |
| | [5,0,1,4,0,1,0,0,0,2] | [0,5,10,16,26,36,47,58,41,24,28] | $Z_{9,9,9,9,9,7,6,6,6,6,4}$ [90] | $Z_{9,9,9,9,9,7,6,6,6,6,4,1,1}$ [90] |
| | [1,4,3,1,0,0,0,0,4,0] | [1,3,9,18,28,38,48,58,39,24,29] | $Z_{10,9,8,8,8,8,7,7,7,6,1,1,1,1}$ [56] | $Z_{10,9,8,8,8,8,7,7,7,6}$ [56] |
| | [3,4,1,2,0,0,0,0,4,0] | [0,3,10,18,28,38,48,58,39,24,29] | $Z_{9,9,9,8,8,8,8,7,6,6,1,1,1,1}$ [56] | $Z_{9,9,9,8,8,8,8,7,6,6}$ [56] |
| | [4,1,4,1,0,0,0,0,4,0] | [0,4,9,18,28,38,48,58,39,24,29] | $Z_{9,9,9,9,8,7,7,7,7,6,1,1,1,1}$ [56] | $Z_{9,9,9,9,8,7,7,7,7,6}$ [56] |
| | [0,2,5,0,1,1,0,0,2,0] | [2,4,8,17,26,36,47,58,40,24,29] | $Z_{10,10,8,8,7,7,7,7,7,5,4,1,1}$ [90] | $Z_{10,10,8,8,7,7,7,7,7,5,4}$ [90] |
| | [0,7,1,0,1,0,0,1,2,0] | [1,2,10,19,28,38,48,58,40,24,29] | $Z_{10,8,8,8,8,8,8,8,7,5,2,1,1}$ [108] | $Z_{10,8,8,8,8,8,8,8,7,5,2}$ [108] |
| | [1,0,5,2,0,1,0,0,2,0] | [2,5,8,16,26,36,47,58,40,24,29] | $Z_{10,10,9,7,7,7,7,7,6,6,4,1,1}$ [90] | $Z_{10,10,9,7,7,7,7,7,6,6,4}$ [90] |
| | [1,1,2,4,1,0,0,0,2,0] | [2,5,9,15,25,36,47,58,40,24,29] | $Z_{10,10,9,8,7,7,6,6,6,6,5,1,1}$ [96] | $Z_{10,10,9,8,7,7,6,6,6,6,5}$ [96] |
| | [1,4,2,1,1,1,0,0,2,0] | [1,3,9,17,26,36,47,58,40,24,29] | $Z_{10,9,8,8,8,8,7,7,6,5,4,1,1}$ [160] | $Z_{10,9,8,8,8,8,7,7,6,5,4}$ [160] |
| | [2,1,5,1,0,0,1,0,2,0] | [1,4,8,17,27,37,47,58,40,24,29] | $Z_{10,9,9,8,7,7,7,7,7,6,3,1,1}$ [128] | $Z_{10,9,9,8,7,7,7,7,7,6,3}$ [128] |
| | [2,6,1,1,0,0,0,0,3,1] | [0,2,10,19,29,39,49,59,40,24,29] | $Z_{9,9,8,8,8,8,8,8,7,6,1,1,1}$ [96] | $Z_{9,9,8,8,8,8,8,8,7,6,1}$ [96] |
| | [2,7,0,0,0,1,0,1,2,0] | [0,2,11,20,29,38,48,58,40,24,29] | $Z_{9,9,8,8,8,8,8,8,8,4,2,1,1}$ [90] | $Z_{9,9,8,8,8,8,8,8,8,4,2}$ [90] |
| | [3,3,3,0,1,0,1,0,2,0] | [0,3,9,18,27,37,47,58,40,24,29] | $Z_{9,9,9,8,8,8,7,7,7,5,3,1,1}$ [144] | $Z_{9,9,9,8,8,8,7,7,7,5,3}$ [144] |
| | [3,4,0,3,0,0,1,0,2,0] | [0,3,10,17,27,37,47,58,40,24,29] | $Z_{9,9,9,8,8,8,8,6,6,6,3,1,1}$ [96] | $Z_{9,9,9,8,8,8,8,6,6,6,3}$ [96] |
| | [3,4,1,0,2,1,0,0,2,0] | [0,3,10,18,26,36,47,58,40,24,29] | $Z_{9,9,9,8,8,8,8,7,5,5,4,1,1}$ [120] | $Z_{9,9,9,8,8,8,8,7,5,5,4}$ [120] |
| | [4,1,3,1,1,1,0,0,2,0] | [0,4,9,17,26,36,47,58,40,24,29] | $Z_{9,9,9,9,8,7,7,7,6,5,4,1,1}$ [160] | $Z_{9,9,9,9,8,7,7,7,6,5,4}$ [160] |
| | [4,2,1,1,3,0,0,0,2,0] | [0,4,10,17,25,36,47,58,40,24,29] | $Z_{9,9,9,9,8,8,7,6,5,5,5,1,1}$ [96] | $Z_{9,9,9,9,8,8,7,6,5,5,5}$ [96] |
| | [5,0,1,4,0,1,0,0,2,0] | [0,5,10,16,26,36,47,58,40,24,29] | $Z_{9,9,9,9,9,7,6,6,6,6,4,1,1}$ [90] | $Z_{9,9,9,9,9,7,6,6,6,6,4}$ [90] |
| | [2,5,2,1,0,1,0,0,0,2] | [0,2,9,18,28,38,49,60,42,24,29] | $Z_{9,9,8,8,8,8,8,7,7,6,4}$ [120] | $Z_{9,9,8,8,8,8,8,7,7,6,4,1,1}$ [120] |
| | [2,6,0,1,2,0,0,0,0,2] | [0,2,10,18,27,38,49,60,42,24,29] | $Z_{9,9,8,8,8,8,8,8,6,5,5}$ [72] | $Z_{9,9,8,8,8,8,8,8,6,5,5,1,1}$ [72] |
| | [3,2,5,0,0,1,0,0,0,2] | [0,3,8,18,28,38,49,60,42,24,29] | $Z_{9,9,9,8,8,7,7,7,7,7,4}$ [80] | $Z_{9,9,9,8,8,7,7,7,7,7,4,1,1}$ [80] |
| | [4,0,5,1,1,0,0,0,0,2] | [0,4,8,17,27,38,49,60,42,24,29] | $Z_{9,9,9,9,7,7,7,7,7,6,5}$ [72] | $Z_{9,9,9,9,7,7,7,7,7,6,5,1,1}$ [72] |
| | [0,6,2,0,2,0,0,0,2,0] | [1,2,9,18,27,38,49,60,41,24,30] | $Z_{10,8,8,8,8,8,8,7,7,5,5,1,1}$ [54] | $Z_{10,8,8,8,8,8,8,7,7,5,5}$ [54] |
| | [2,5,2,1,0,1,0,0,2,0] | [0,2,9,18,28,38,49,60,41,24,30] | $Z_{9,9,8,8,8,8,8,7,7,6,4,1,1}$ [120] | $Z_{9,9,8,8,8,8,8,7,7,6,4}$ [120] |
| | [2,6,0,1,2,0,0,0,2,0] | [0,2,10,18,27,38,49,60,41,24,30] | $Z_{9,9,8,8,8,8,8,8,6,5,5,1,1}$ [72] | $Z_{9,9,8,8,8,8,8,8,6,5,5}$ [72] |
| | [3,2,5,0,0,1,0,0,2,0] | [0,3,8,18,28,38,49,60,41,24,30] | $Z_{9,9,9,8,8,7,7,7,7,7,4,1,1}$ [80] | $Z_{9,9,9,8,8,7,7,7,7,7,4}$ [80] |
| | [4,0,5,1,1,0,0,0,2,0] | [0,4,8,17,27,38,49,60,41,24,30] | $Z_{9,9,9,9,7,7,7,7,7,6,5,1,1}$ [72] | $Z_{9,9,9,9,7,7,7,7,7,6,5}$ [72] |
| | [1,8,1,0,0,1,0,0,0,2] | [0,1,10,20,30,40,51,62,43,24,30] | $Z_{9,8,8,8,8,8,8,8,8,7,4}$ [80] | $Z_{9,8,8,8,8,8,8,8,8,7,4,1,1}$ [80] |
| | [2,0,8,0,0,0,0,0,0,2] | [1,4,7,18,29,40,51,62,43,24,30] | $Z_{10,9,9,7,7,7,7,7,7,7,7}$ [24] | $Z_{10,9,9,7,7,7,7,7,7,7,7,1,1}$ [24] |
| | [2,4,4,1,0,0,0,0,0,2] | [0,2,8,18,29,40,51,62,43,24,30] | $Z_{9,9,8,8,8,8,7,7,7,7,6}$ [56] | $Z_{9,9,8,8,8,8,7,7,7,7,6,1,1}$ [56] |
| | [1,8,1,0,0,1,0,0,2,0] | [0,1,10,20,30,40,51,62,42,24,31] | $Z_{9,8,8,8,8,8,8,8,8,7,4,1,1}$ [80] | $Z_{9,8,8,8,8,8,8,8,8,7,4}$ [80] |
| | [2,4,4,1,0,0,0,0,2,0] | [0,2,8,18,29,40,51,62,42,24,31] | $Z_{9,9,8,8,8,8,7,7,7,7,6,1,1}$ [56] | $Z_{9,9,8,8,8,8,7,7,7,7,6}$ [56] |
